# Supplementary material for: A Comparative Study of Different Edit Distance-Based Methods for Feature Tracking using Merge Trees on Time-Varying Scalar Fields
Source: arXiv:2509.17974 source file (2025-10-12)
Supplement: Supplementary file 1 [file SupplementaryMaterial.tex]

% $Id: template.tex 11 2007-04-03 22:25:53Z jpeltier $

\documentclass{vgtc}                          % final (conference style)

\newif\ifwarntodo %Warn on encountering a \todo or \anno?
\warntodotrue
%\warntodofalse

%Eliminate all todo's appearance in the text
\newif\ifshowtodo
% \showtodofalse
\showtodotrue

%% Uncomment one of the lines above depending on where your paper is
%% in the conference process. ``review'' and ``widereview'' are for review
%% submission, ``preprint'' is for pre-publication, and the final version
%% doesn't use a specific qualifier. Further, ``electronic'' includes
%% hyperreferences for more convenient online viewing.

%% Please use one of the ``review'' options in combination with the
%% assigned online id (see below) ONLY if your paper uses a double blind
%% review process. Some conferences, like IEEE Vis and InfoVis, have NOT
%% in the past.

%% Figures should be in CMYK or Grey scale format, otherwise, colour 
%% shifting may occur during the printing process.

%% it is recomended to use ``\cref{sec:bla}'' instead of ``Fig.~\ref{sec:bla}''

\usepackage{times}                     % we use Times as the main font
         % a nicer typewriter font

%% Only used in the template examples. You can remove these lines.
\usepackage{tabu}                      % only used for the table example
\usepackage{booktabs}                  % only used for the table example
\usepackage{lipsum}                    % used to generate placeholder text
\usepackage{mwe}                       % used to generate placeholder figures

%% We encourage the use of mathptmx for consistent usage of times font
%% throughout the proceedings. However, if you encounter conflicts
%% with other math-related packages, you may want to disable it.
\usepackage{mathptmx}                  % use matching math font
%% Packages for Graphics & Figures %%%%%%%%%%%%%%%%%%%%%%%%%%
%\usepackage{graphicx}                % allow us to embed graphics files
%\DeclareGraphicsExtensions{.pdf,.png,.jpg,.jpeg} % for pdflatex we expect .pdf, .png, or .jpg files
\graphicspath{{pdfimages/}, {images/}} % where to search for the images
\usepackage{subcaption}   % For subfig environment

\usepackage{booktabs}
\usepackage{multirow}
\usepackage{microtype}

\usepackage[svgnames]{xcolor}

\usepackage{makecell}   % For table with cell in multiple lines

\usepackage{tikz}
\usetikzlibrary{patterns,shapes.arrows}
\usetikzlibrary{positioning}
\usetikzlibrary{arrows.meta}
% \usetikzlibrary{matrix}
% \usetikzlibrary{backgrounds}

\usetikzlibrary{external}
% \tikzexternalize[optimize=false, prefix=tikzternal/]
\tikzset{external/only named=true}
%\tikzexternaldisable

\usepackage{tikzscale}

\usepackage{pgfplots}
\usepackage{pgfplotstable}
\usepgfplotslibrary{groupplots}
\pgfplotsset{compat=newest}
%\DeclareUnicodeCharacter{2212}{−}

%% Math Packages %%%%%%%%%%%%%%%%%%%%%%%%%%%%%%%%%%%%%%%%%%%%
\usepackage{amsmath}
\usepackage{amsbsy}
\usepackage{amsfonts}
\usepackage{mathtools}
\usepackage{amssymb, amsthm}  % For \varnothing, proof environment
\usepackage{nicefrac}

\usepackage{cite}                      % needed to automatically sort the references

\hyphenation{con-secu-tive} %The u can be by itself, but that looks ga

%% If you are submitting a paper to a conference for review with a double
%% blind reviewing process, please replace the value ``0'' below with your
%% OnlineID. Otherwise, you may safely leave it at ``0''.
\onlineid{1028}

%% declare the category of your paper, only shown in review mode
\vgtccategory{Research}

%% allow for this line if you want the electronic option to work properly
\vgtcinsertpkg

%% In preprint mode you may define your own headline. If not, the default IEEE copyright message will appear in preprint mode.
%\preprinttext{To appear in an IEEE VGTC sponsored conference.}

%% This adds a link to the version of the paper on IEEEXplore
%% Uncomment this line when you produce a preprint version of the article 
%% after the article receives a DOI for the paper from IEEE
%\ieeedoi{xx.xxxx/TVCG.201x.xxxxxxx}

%% Paper title.

% \title{Comparing Different Merge Tree-Based Tracking Methods\\for Time-Varying Scalar Fields}
\title{A Comparative Study of Different Edit Distance-Based Methods\\
for Feature Tracking using Merge Trees\\on Time-Varying Scalar Fields}

%% This is how authors are specified in the conference style

%% Author and Affiliation (multiple authors with single affiliations).
\author{Son Le Thanh\thanks{e-mail: sonlt@kth.se} %
\and Tino Weinkauf\thanks{e-mail: weinkauf@kth.se} %
}
\affiliation{\scriptsize KTH Royal Institute of Technology\\Stockholm, Sweden}

% 
% Further, please bring the word compare/comparison into the abstract. Please also mention the methods that you compare. That is not easy, since you cannot cite.
% 
% Scale down a bit on explaining to the reader what tracking is. Rather focus more on your work: how you selected these scenarios, if that is possible to say. Can you already mention some more results than you do at this point?

%% Abstract section.
%% Keywords that describe your work. Will show as 'Index Terms' in journal
%% please capitalize first letter and insert punctuation after last keyword.
%% Copyright space is enabled by default as required by guidelines.
%% It is disabled by the 'review' option or via the following command:
% \nocopyrightspace

%%%%%%%%%%%%%%%%%%%%%%%%%%%%%%%%%%%%%%%%%%%%%%%%%%%%%%%%%%%%%%%%
%%%%%%%%%%%%%%%%%%%%%% START OF THE PAPER %%%%%%%%%%%%%%%%%%%%%%
%%%%%%%%%%%%%%%%%%%%%%%%%%%%%%%%%%%%%%%%%%%%%%%%%%%%%%%%%%%%%%%%%

\begin{document}
\input{macros}
%% The ``\maketitle'' command must be the first command after the
%% ``\begin{document}'' command. It prepares and prints the title block.

%% the only exception to this rule is the \firstsection command

\maketitle
We include further results that
did not appear in the main text due to the page limit.
We experiment with the same four algorithms:
constrained edit distance $d_e$ \cite{sridharamurthy2018edit},
the Wasserstein distance $d_w$ \cite{pont22},
the branch mapping $d_b$ \cite{wetzels2022branch} and 
path mapping $d_p$ \cite{wetzels2022path} distances.

\section*{Stability with respect to Noise}
In the section, we show the results of the stability score 
with $\epsilon_\text{max} = 5\%$. 
The results can be seen 
in \Cref{fig-stab10}, \Cref{fig-stab15}, and \Cref{fig-stab20}.

\begin{figure}
    \centering
    \includegraphics[width=0.8\linewidth]{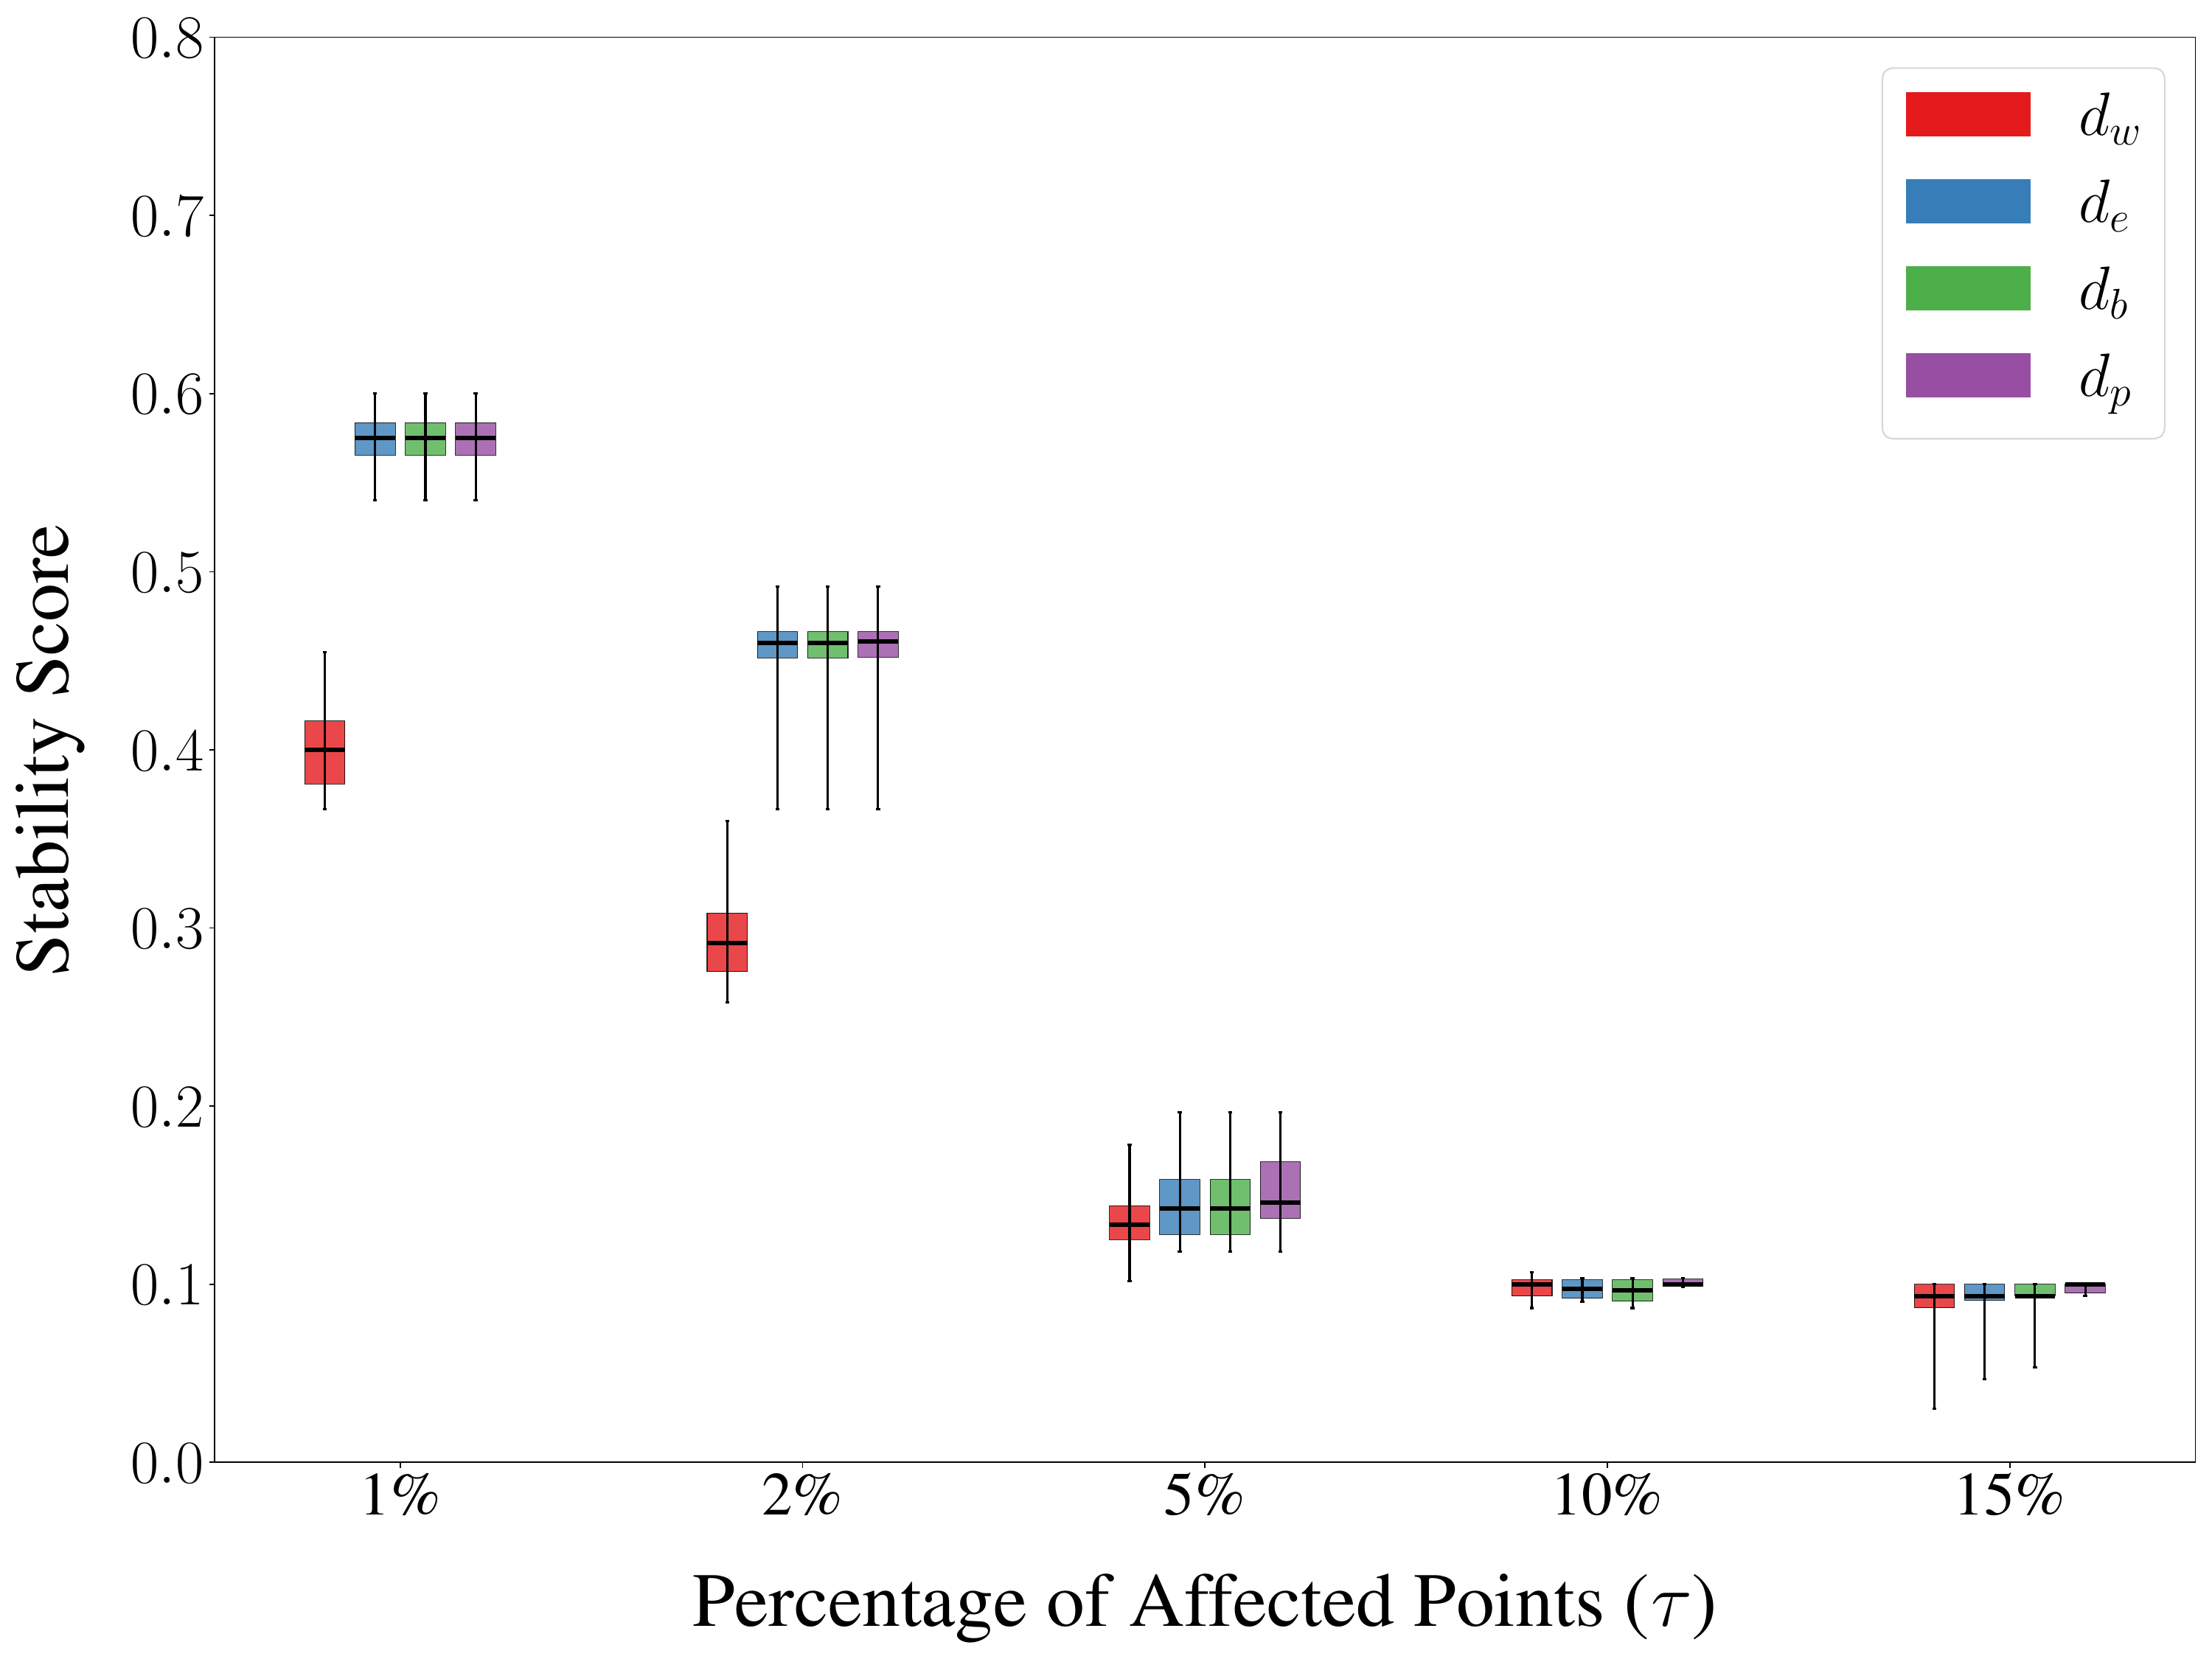}
    \caption{The tracking stability of the extrema of the for methods 
    if we stop at $\epsilon_\text{max}=10\%$. 
    }
    \label{fig-stab10}
\end{figure}

\begin{figure}
    \centering
    \includegraphics[width=0.8\linewidth]{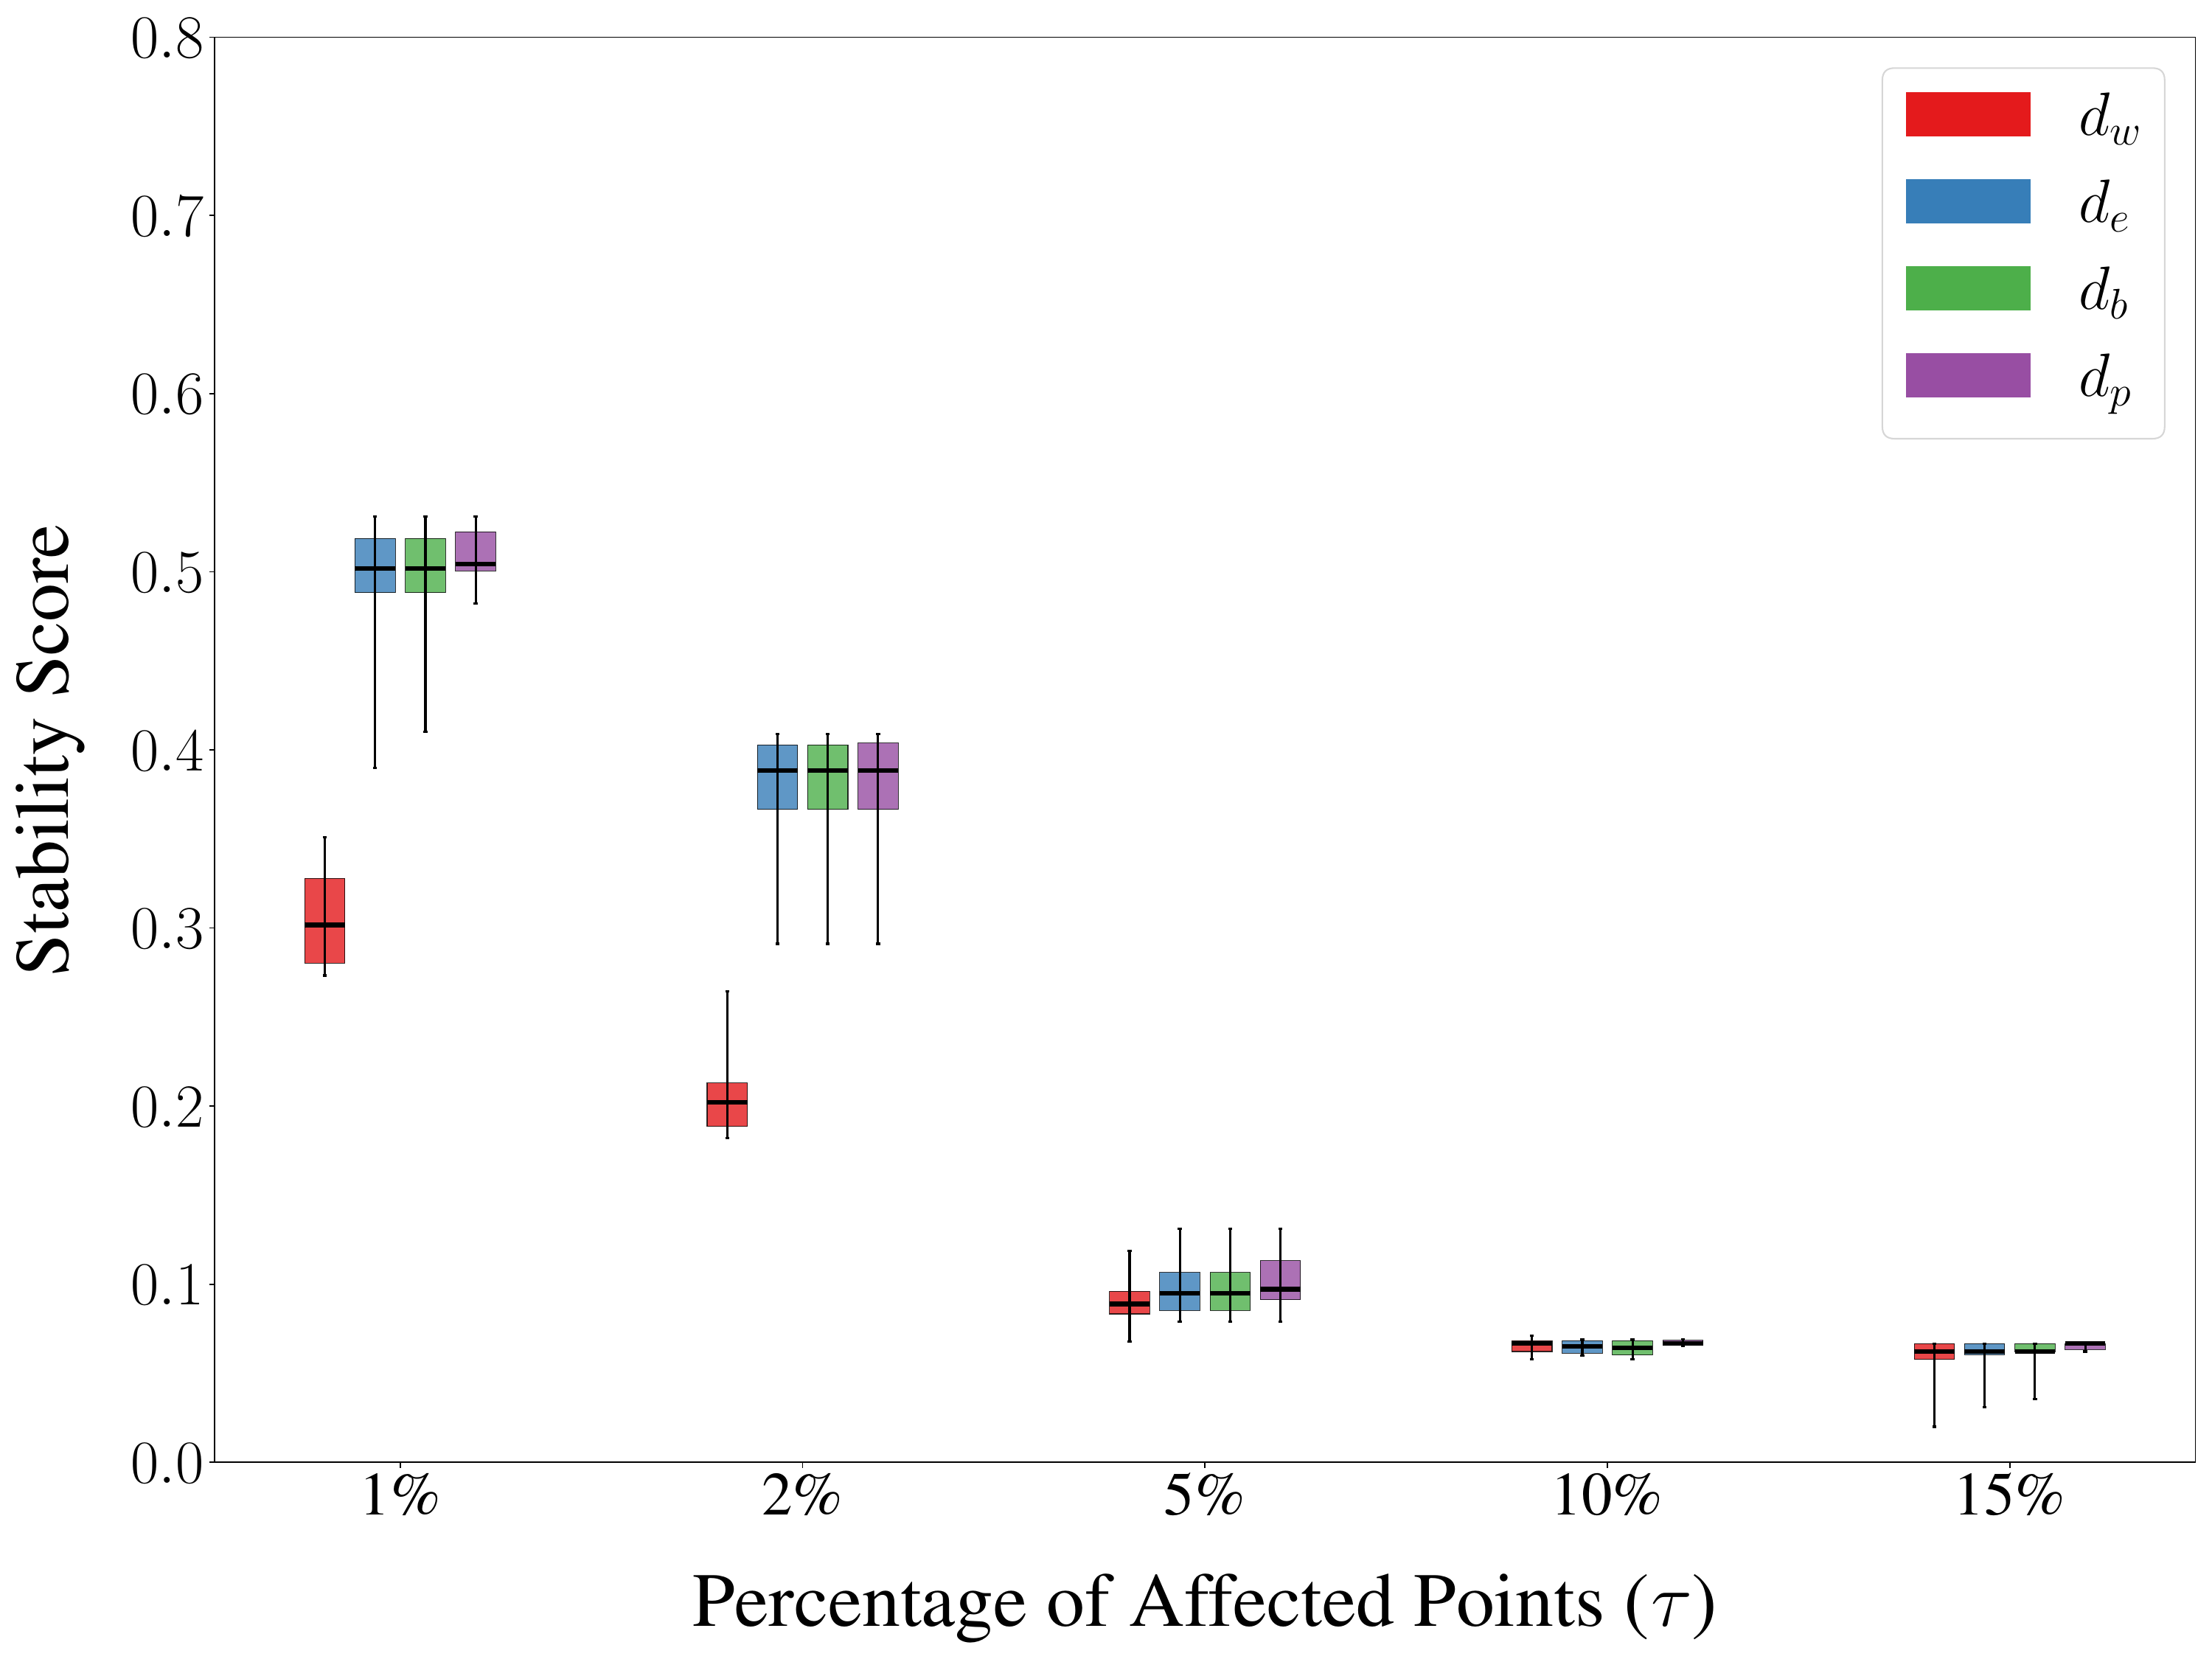}
    \caption{The tracking stability of the extrema of the for methods 
    if we stop at $\epsilon_\text{max}=15\%$.}
    \label{fig-stab15}
\end{figure}

\begin{figure}
    \centering
    \includegraphics[width=0.8\linewidth]{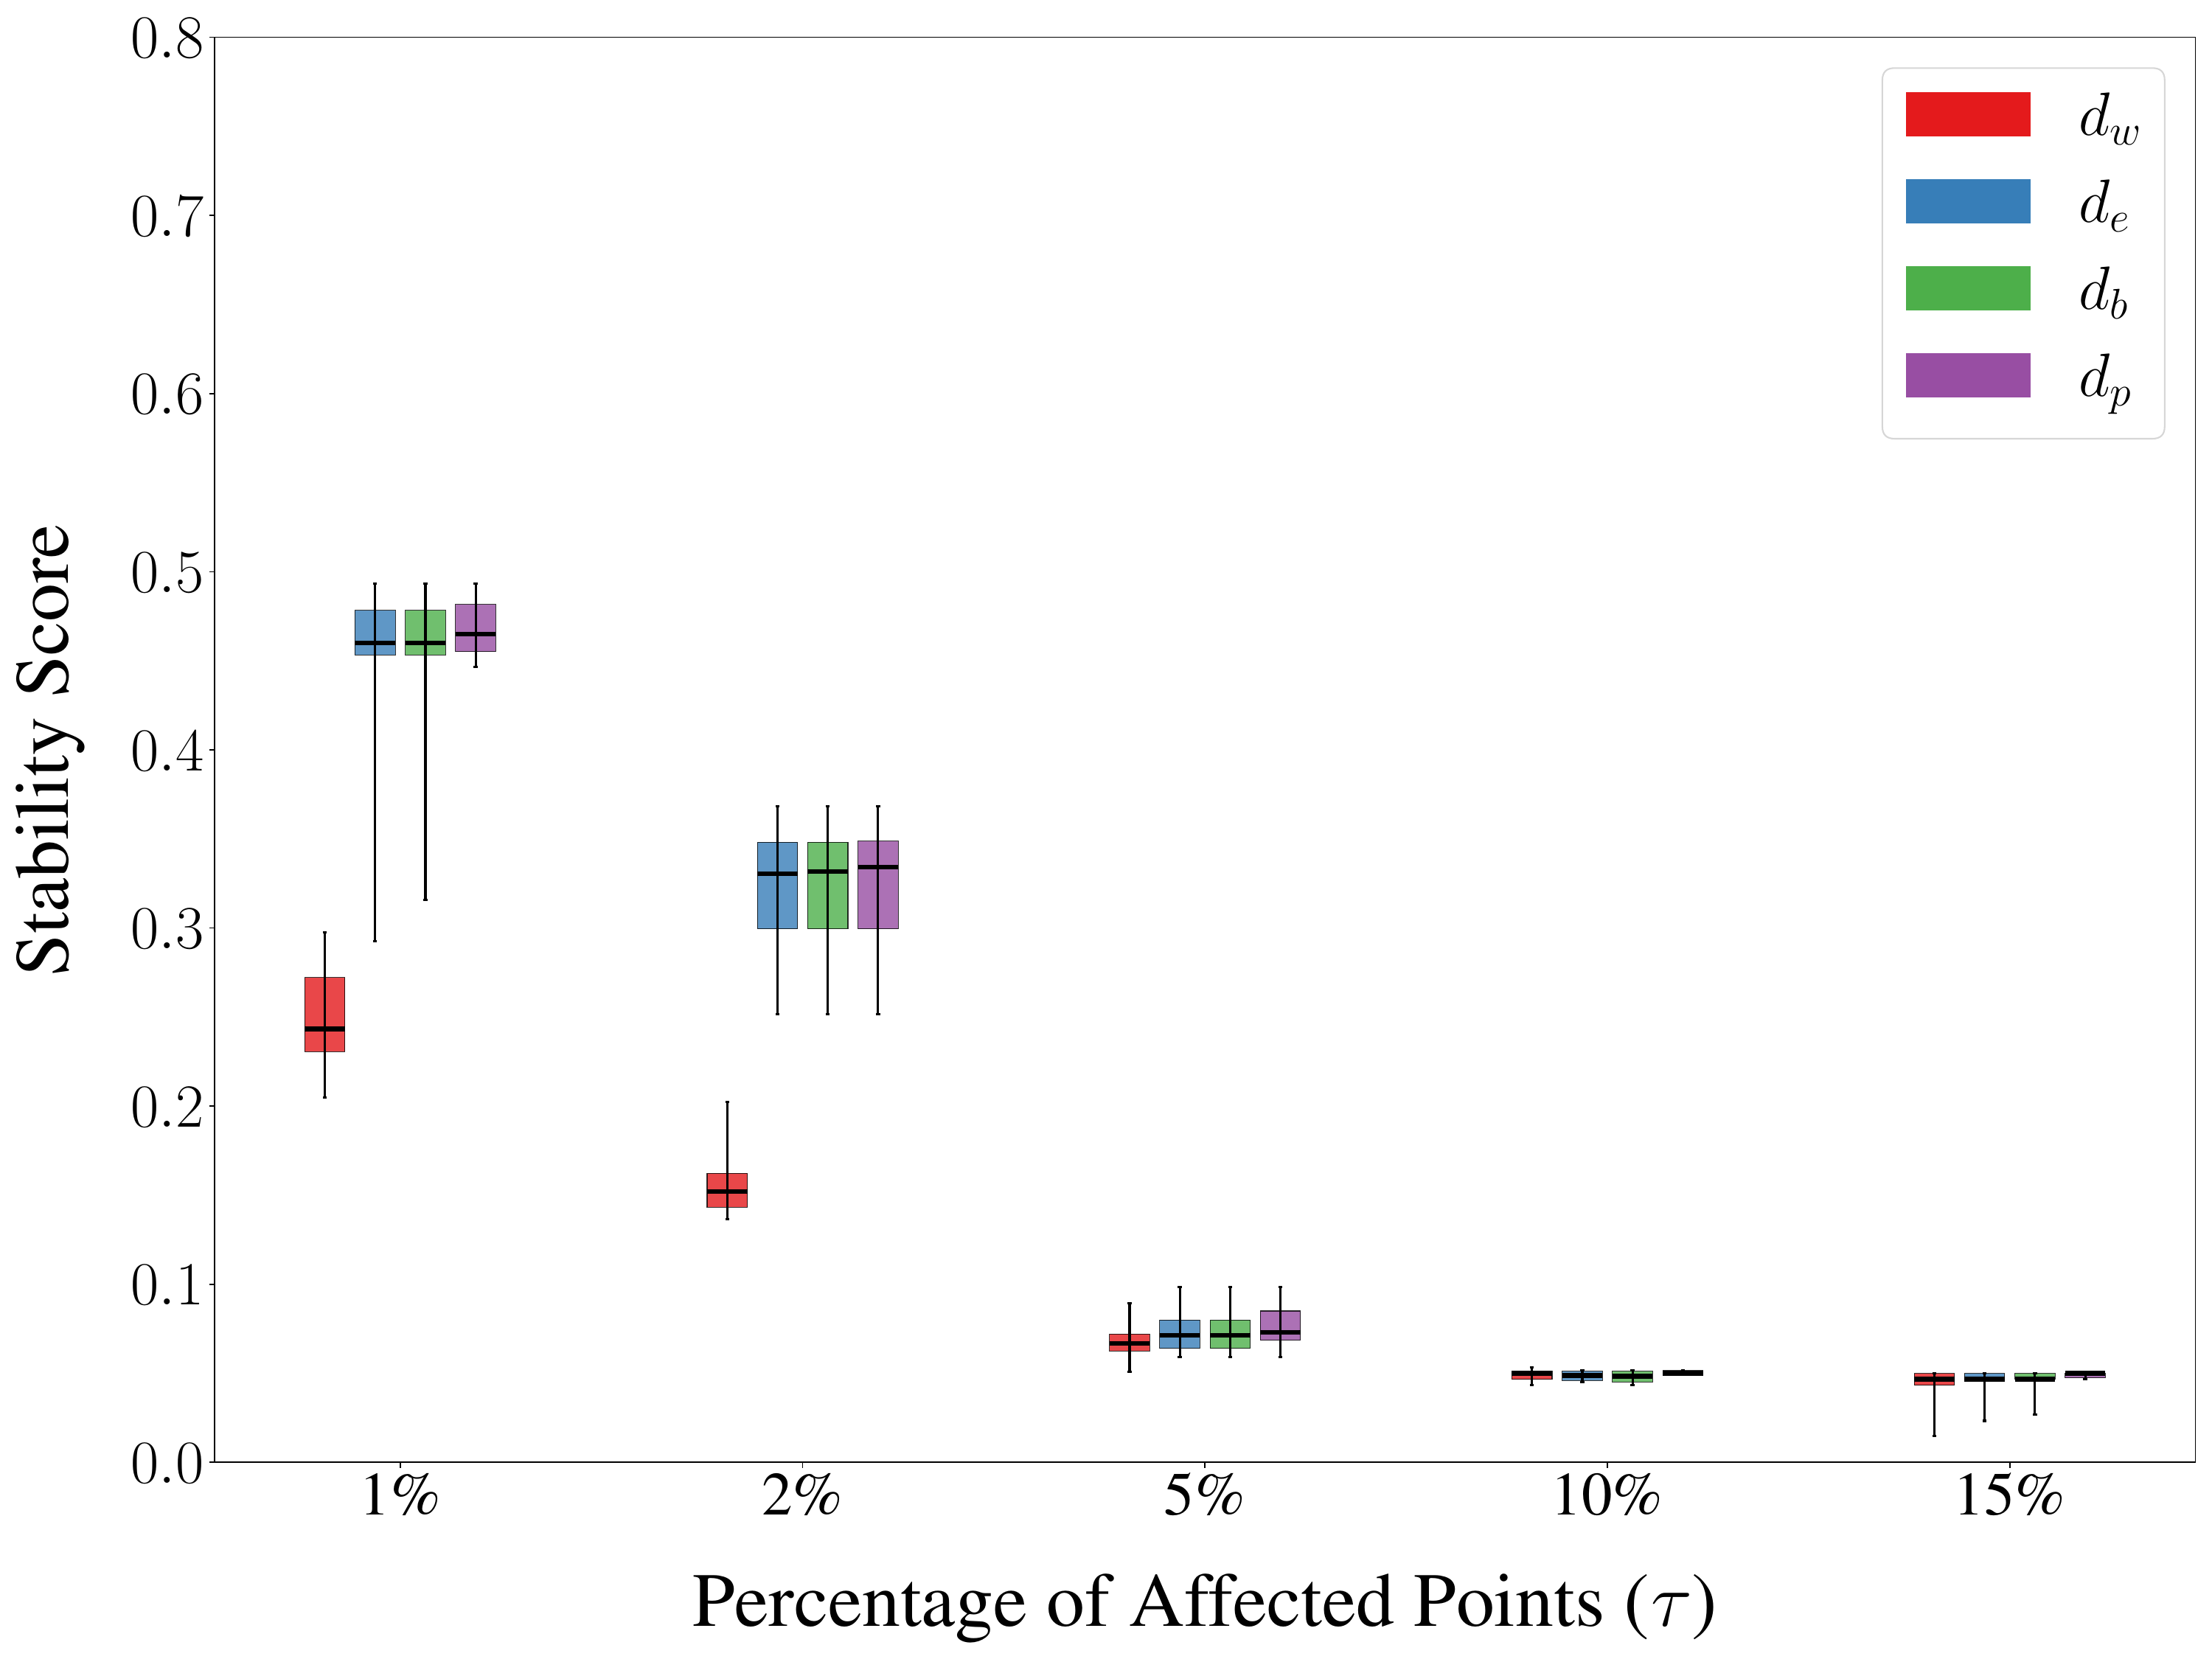}
    \caption{The tracking stability of the extrema of the for methods 
    if we stop at $\epsilon_\text{max}=20\%$.}
    \label{fig-stab20}
\end{figure}
\section*{Extra Results on Real-World Data Set}
We introduce information on the data sets used in this section,
followed by the results for each of them. 

\dataset{IonizationFront2D} is a simulated 2D scalar field 
from 2008 SciVis Contest \cite{whalen2008competition},  
The results 
capture the formation of the first stars in the universe 
through density variations of the so-called ionization front.
We use the first $100$ time steps for our experiment.
The split trees can be used to map the regions with similar density
as the shadow instability progresses.

\dataset{Storms2D} depicts a one-hourly mean sea level pressure 
over the month of December 1999. This data set is available to download at 
\cite{ERA5data}. Similar to K\"opp and Weinkauf \cite{koepp22},
the mean over eight days is computed and a light Gaussian smoothing is applied.
This process creates a time-dependent 2D scalar field with 743 time steps.
The structural changes in join trees over time 
provide insight into the formation and evolution of storms.

\dataset{Boussinesq2D} is a simulation of a flow generated 
by a heated cylinder \cite{Guenther17} over $2001$ time steps
using Gerris flow solver \cite{germer11a}.
It is a time-dependent vector field and 
contains numerous small vortices rotating around each other.
Using the last $1000$ time steps, we compute and 
track the evolution of join trees of the velocity magnitude,
as their nodes associate with the vortex centers.

\dataset{Cylinder3D} originates from a simulation of 3D turbulent flow 
around a half-cylinder. \cite{BaezaRojo19SciVisa} with
the Reynolds number of $640$. 
It contains $151$ time steps.
The split trees are employed to track the temporal evolution of the 
local maxima and saddle points of the velocity magnitude.

\dataset{Tangaroa3D} captures the 3D flow around a research vessel Tangaroa
over $200$ time steps \cite{PopinetEtAl2004_Tangaroa}.
Similar to Cylinder3D, we also compute the magnitude of the velocity
to obtain a scalar field for each time step.
We also track the evolution of split trees of 
resulted from the velocity magnitude.

The three data sets \dataset{Boussinesq2D}, \dataset{Cylinder3D}, and \dataset{Tangaroa3D}
can be found at the
\href{https://cgl.ethz.ch/research/visualization/data.php}{Computer Graphics Laboratory}.
The simplification thresholds for the data sets are:
\dataset{IonizationFront2D} at $5\%$,
\dataset{Storms2D} at $1\%$,
\dataset{Boussinesq2D} at $2\%$,
both \dataset{Cylinder3D} and \dataset{Tangaroa3D} at $8\%$.
We also provide results for with more time steps of \dataset{Cylinder2D}.

\subsection*{Results using IonizationFront2D}
The results of the experiments using \dataset{IonizationFront2D}
are shown from \Cref{fig-IonizationFront2DAllNodes}
to \Cref{fig-IonizationFront2DSimilarities}.

\begin{figure}
\centering
\includegraphics[width=0.8\linewidth]{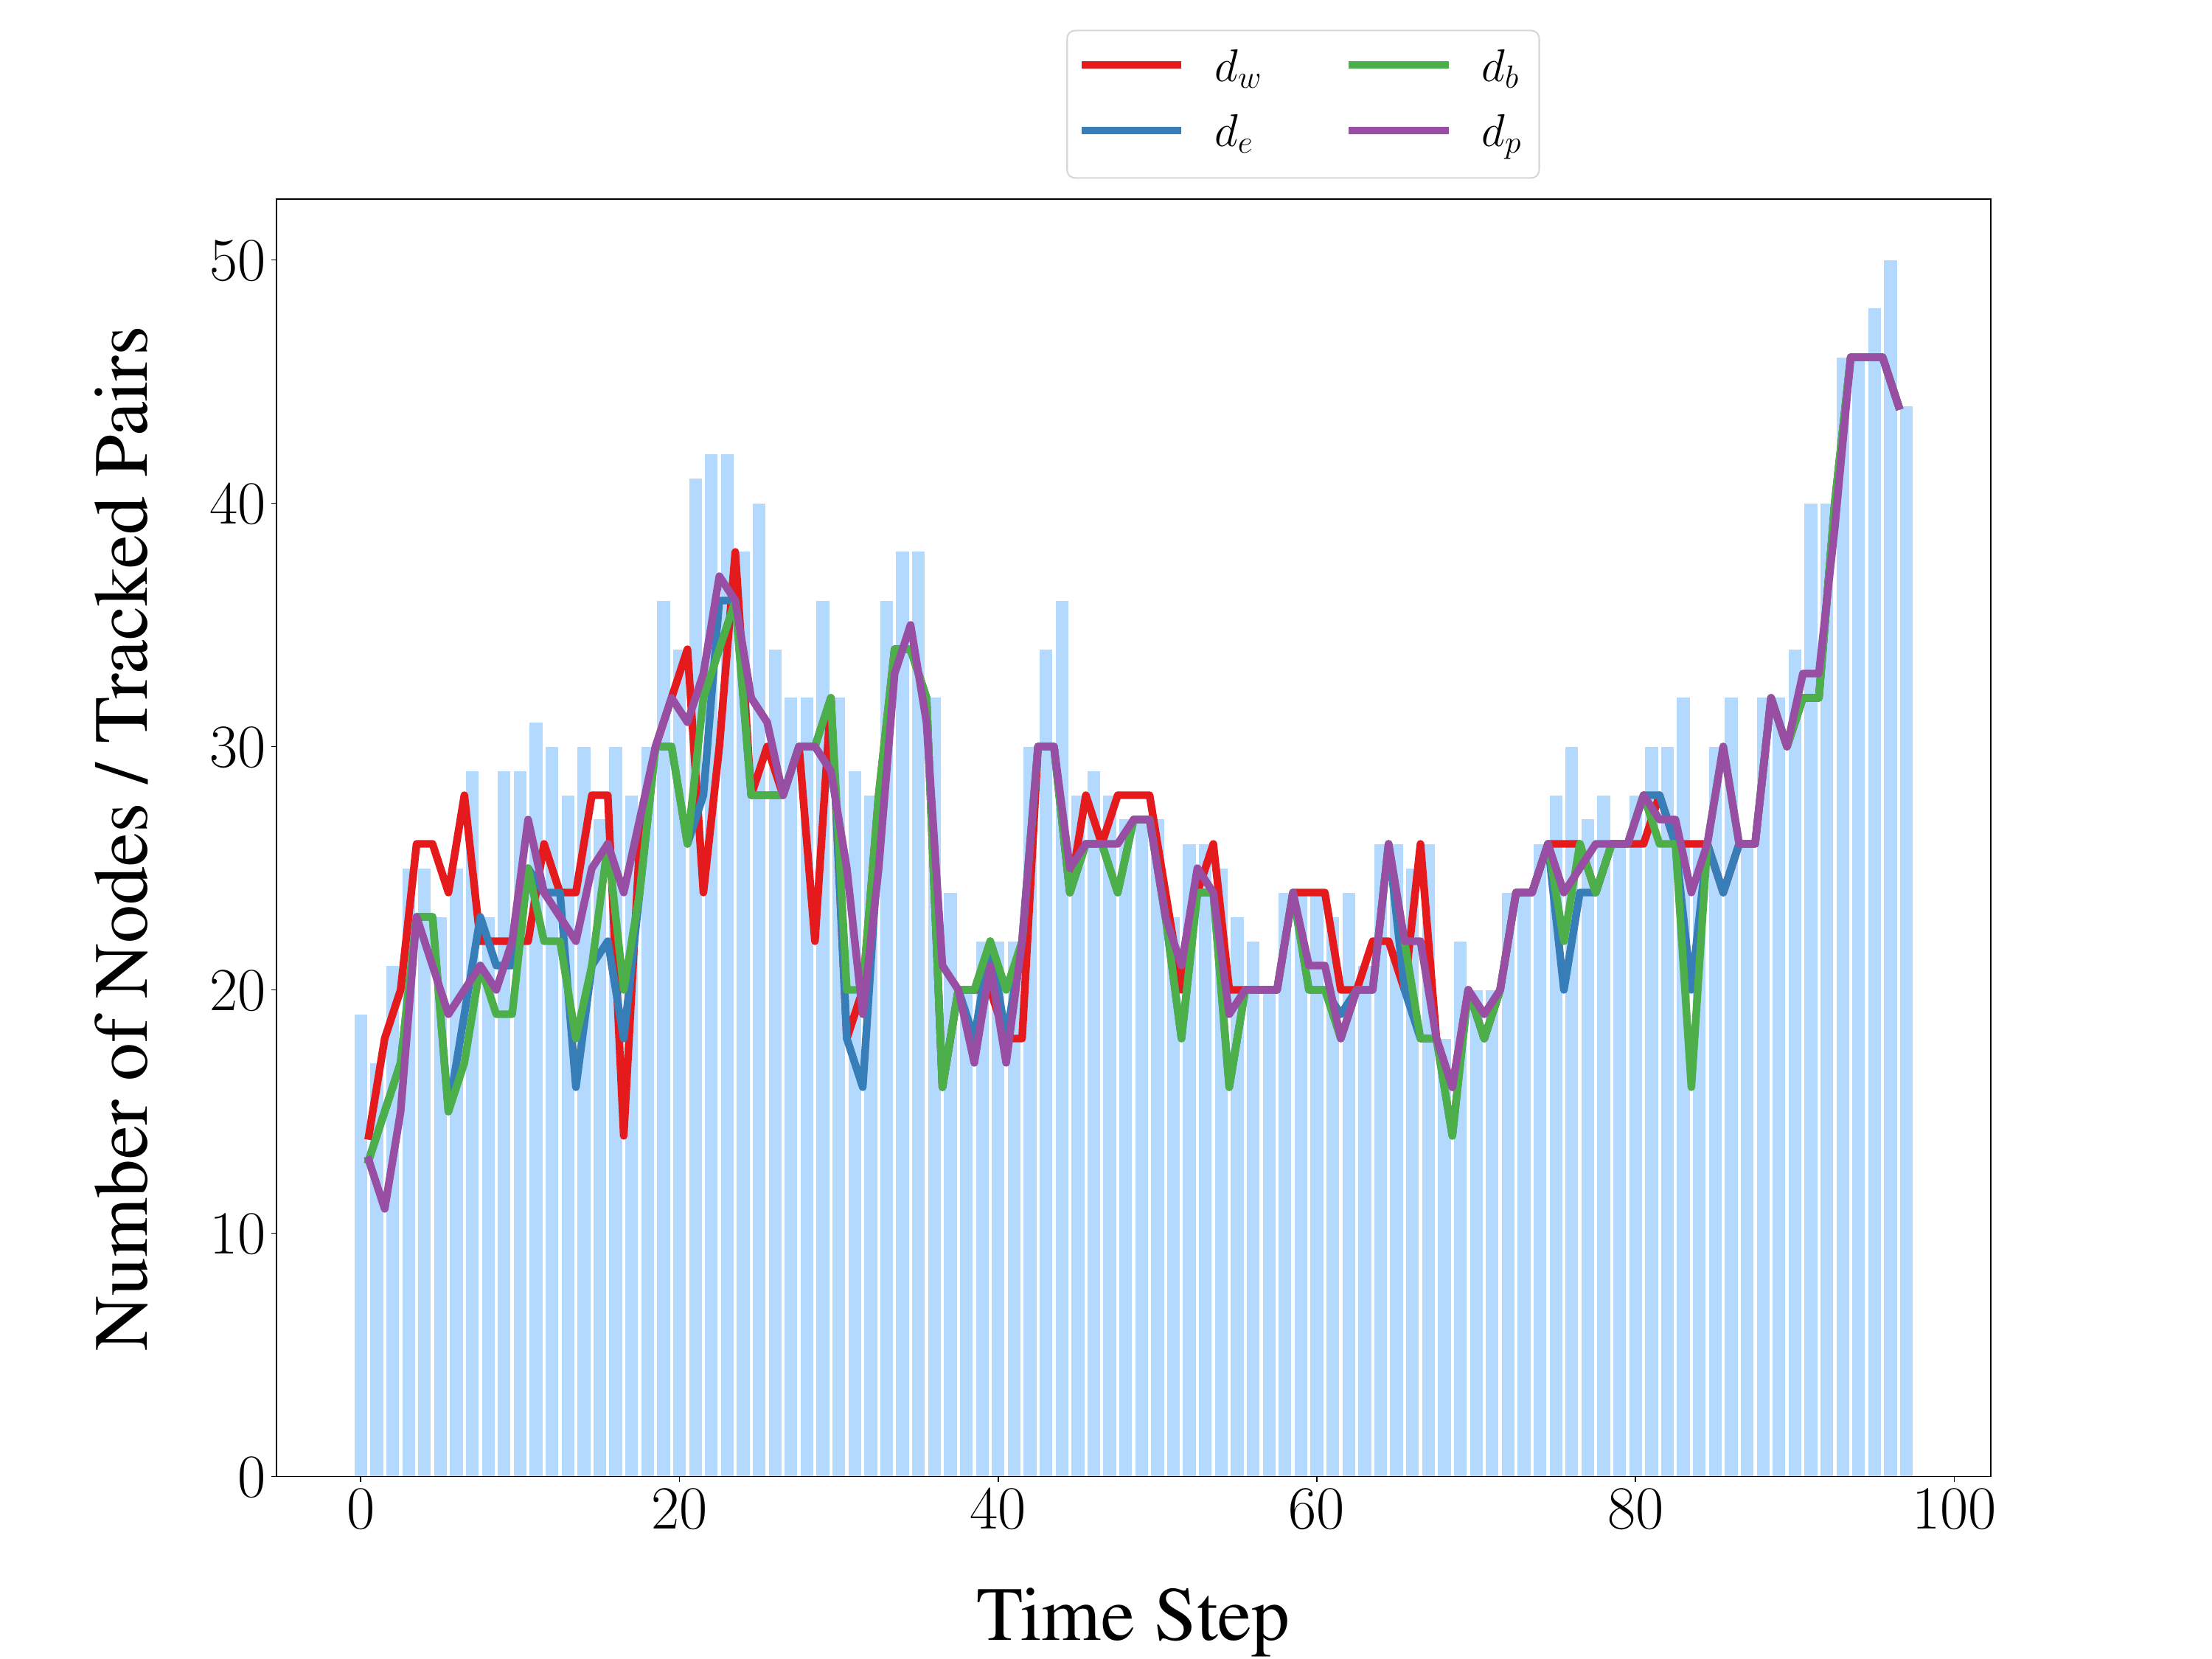}
\caption{
    Number of tracked nodes (colored and labeled) 
    relative to the total nodes of merge trees (light blue bars)
    for \dataset{IonizationFront2D}.
}
\label{fig-IonizationFront2DAllNodes}
\end{figure}

\begin{figure}
\centering
\includegraphics[width=0.8\linewidth]{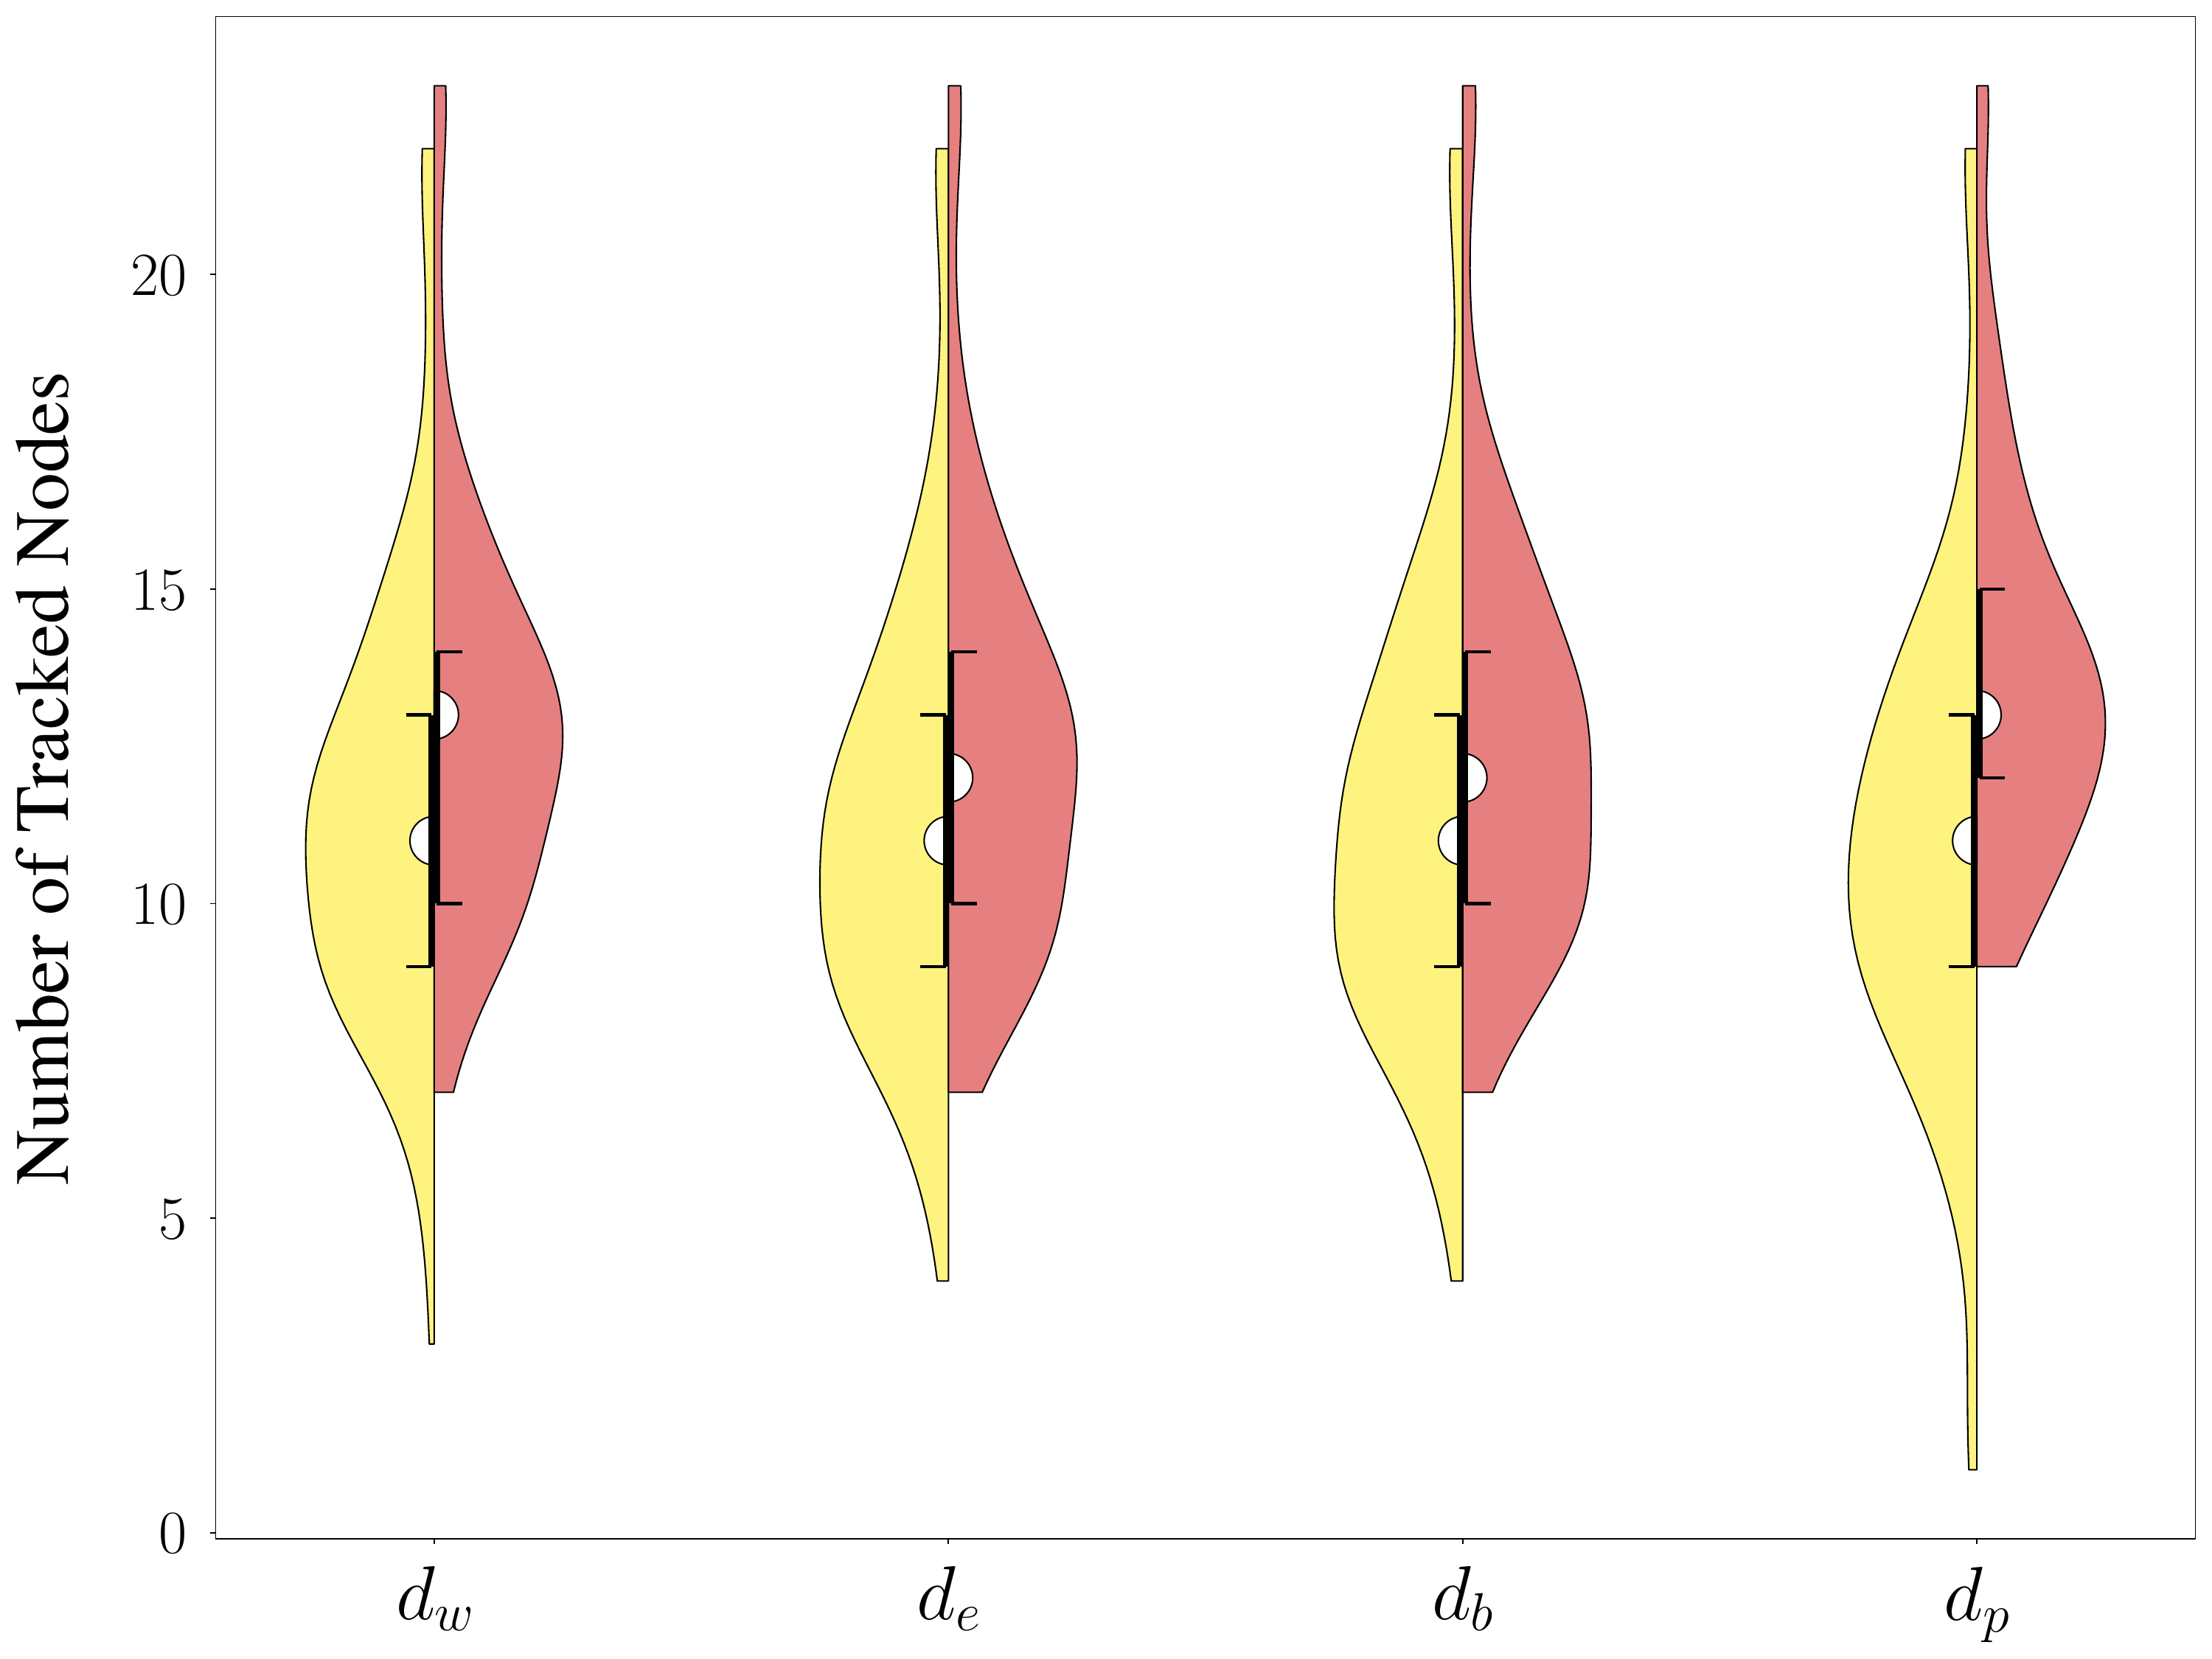}
\caption{
    Distributions of tracked nodes 
    over the chosen time steps of \dataset{IonizationFront2D},  
    divided by types:
    saddle (yellow) and maxima (red).
}
\label{fig-IonizationFront2DViolin}
\end{figure}

% Length histogram
\begin{figure}%
\begin{subfigure}[t]{\ltwopicwidth}%
\includegraphics[width=\ltwopicwidth]{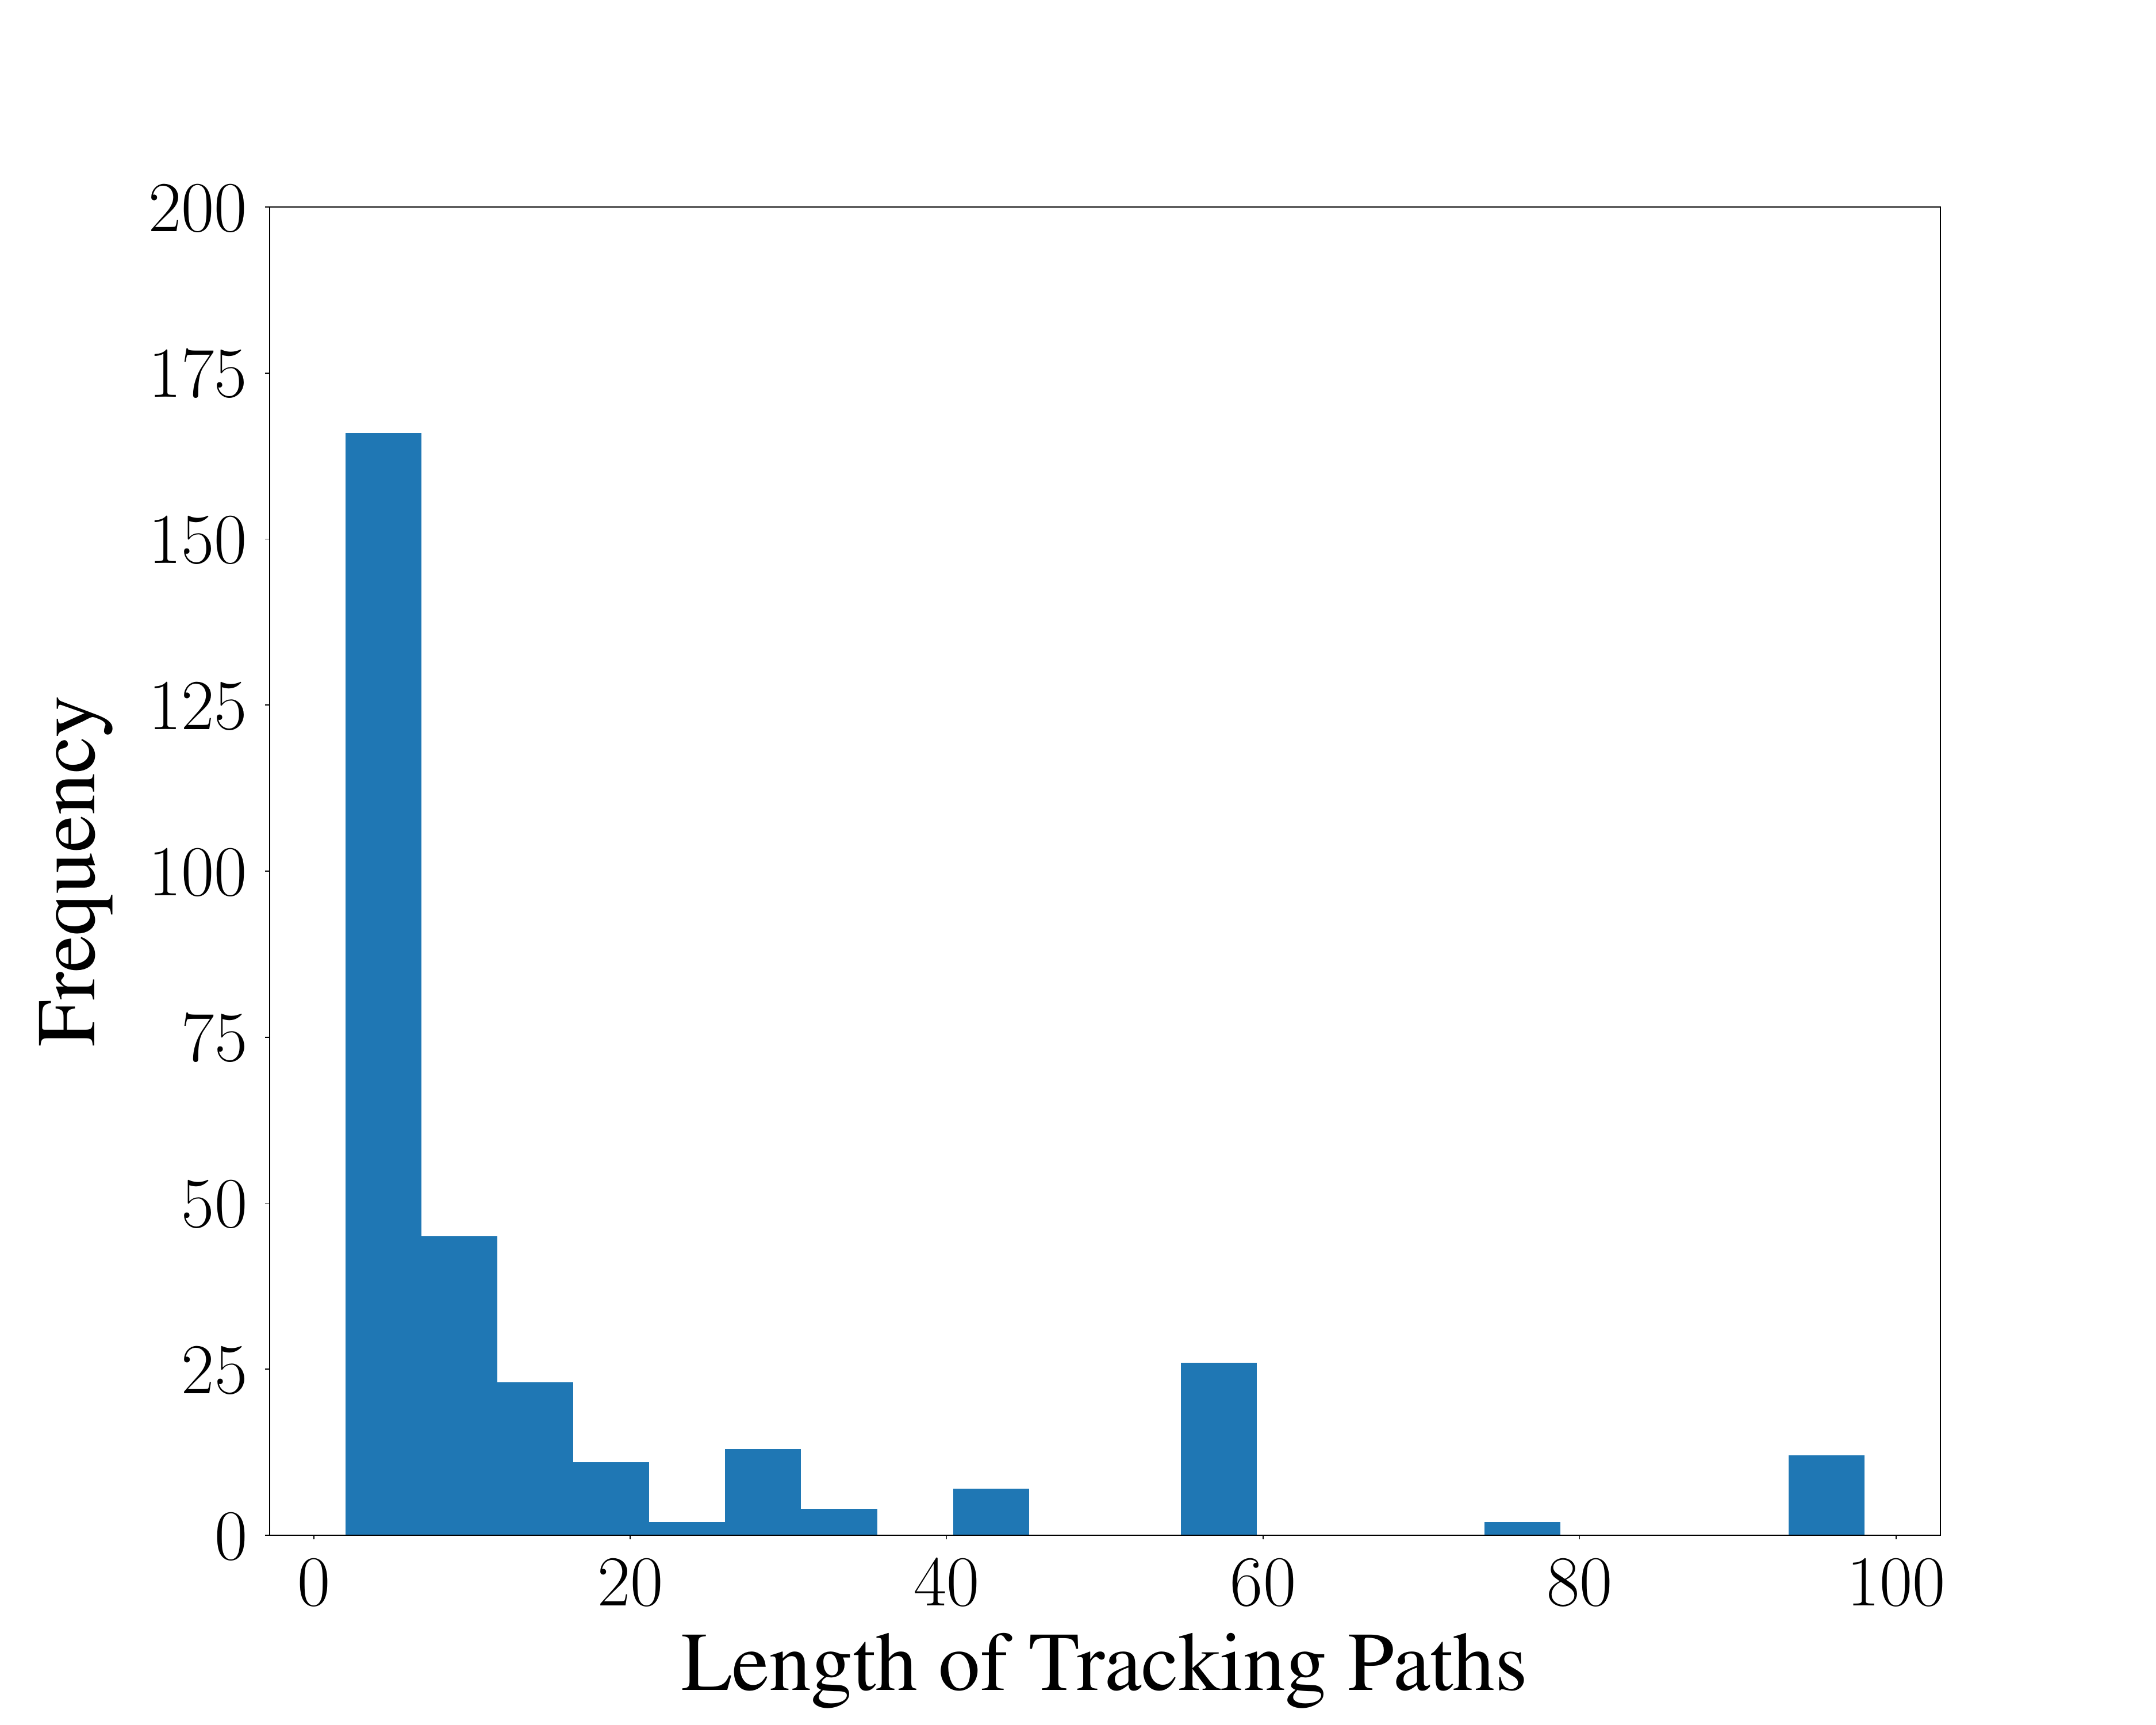}
\caption{$d_w$.}%
\label{fig-LengthHistogramIonizationFront2DW}%
\end{subfigure}
\hfill%
\begin{subfigure}[t]{\ltwopicwidth}%
\includegraphics[width=\ltwopicwidth]{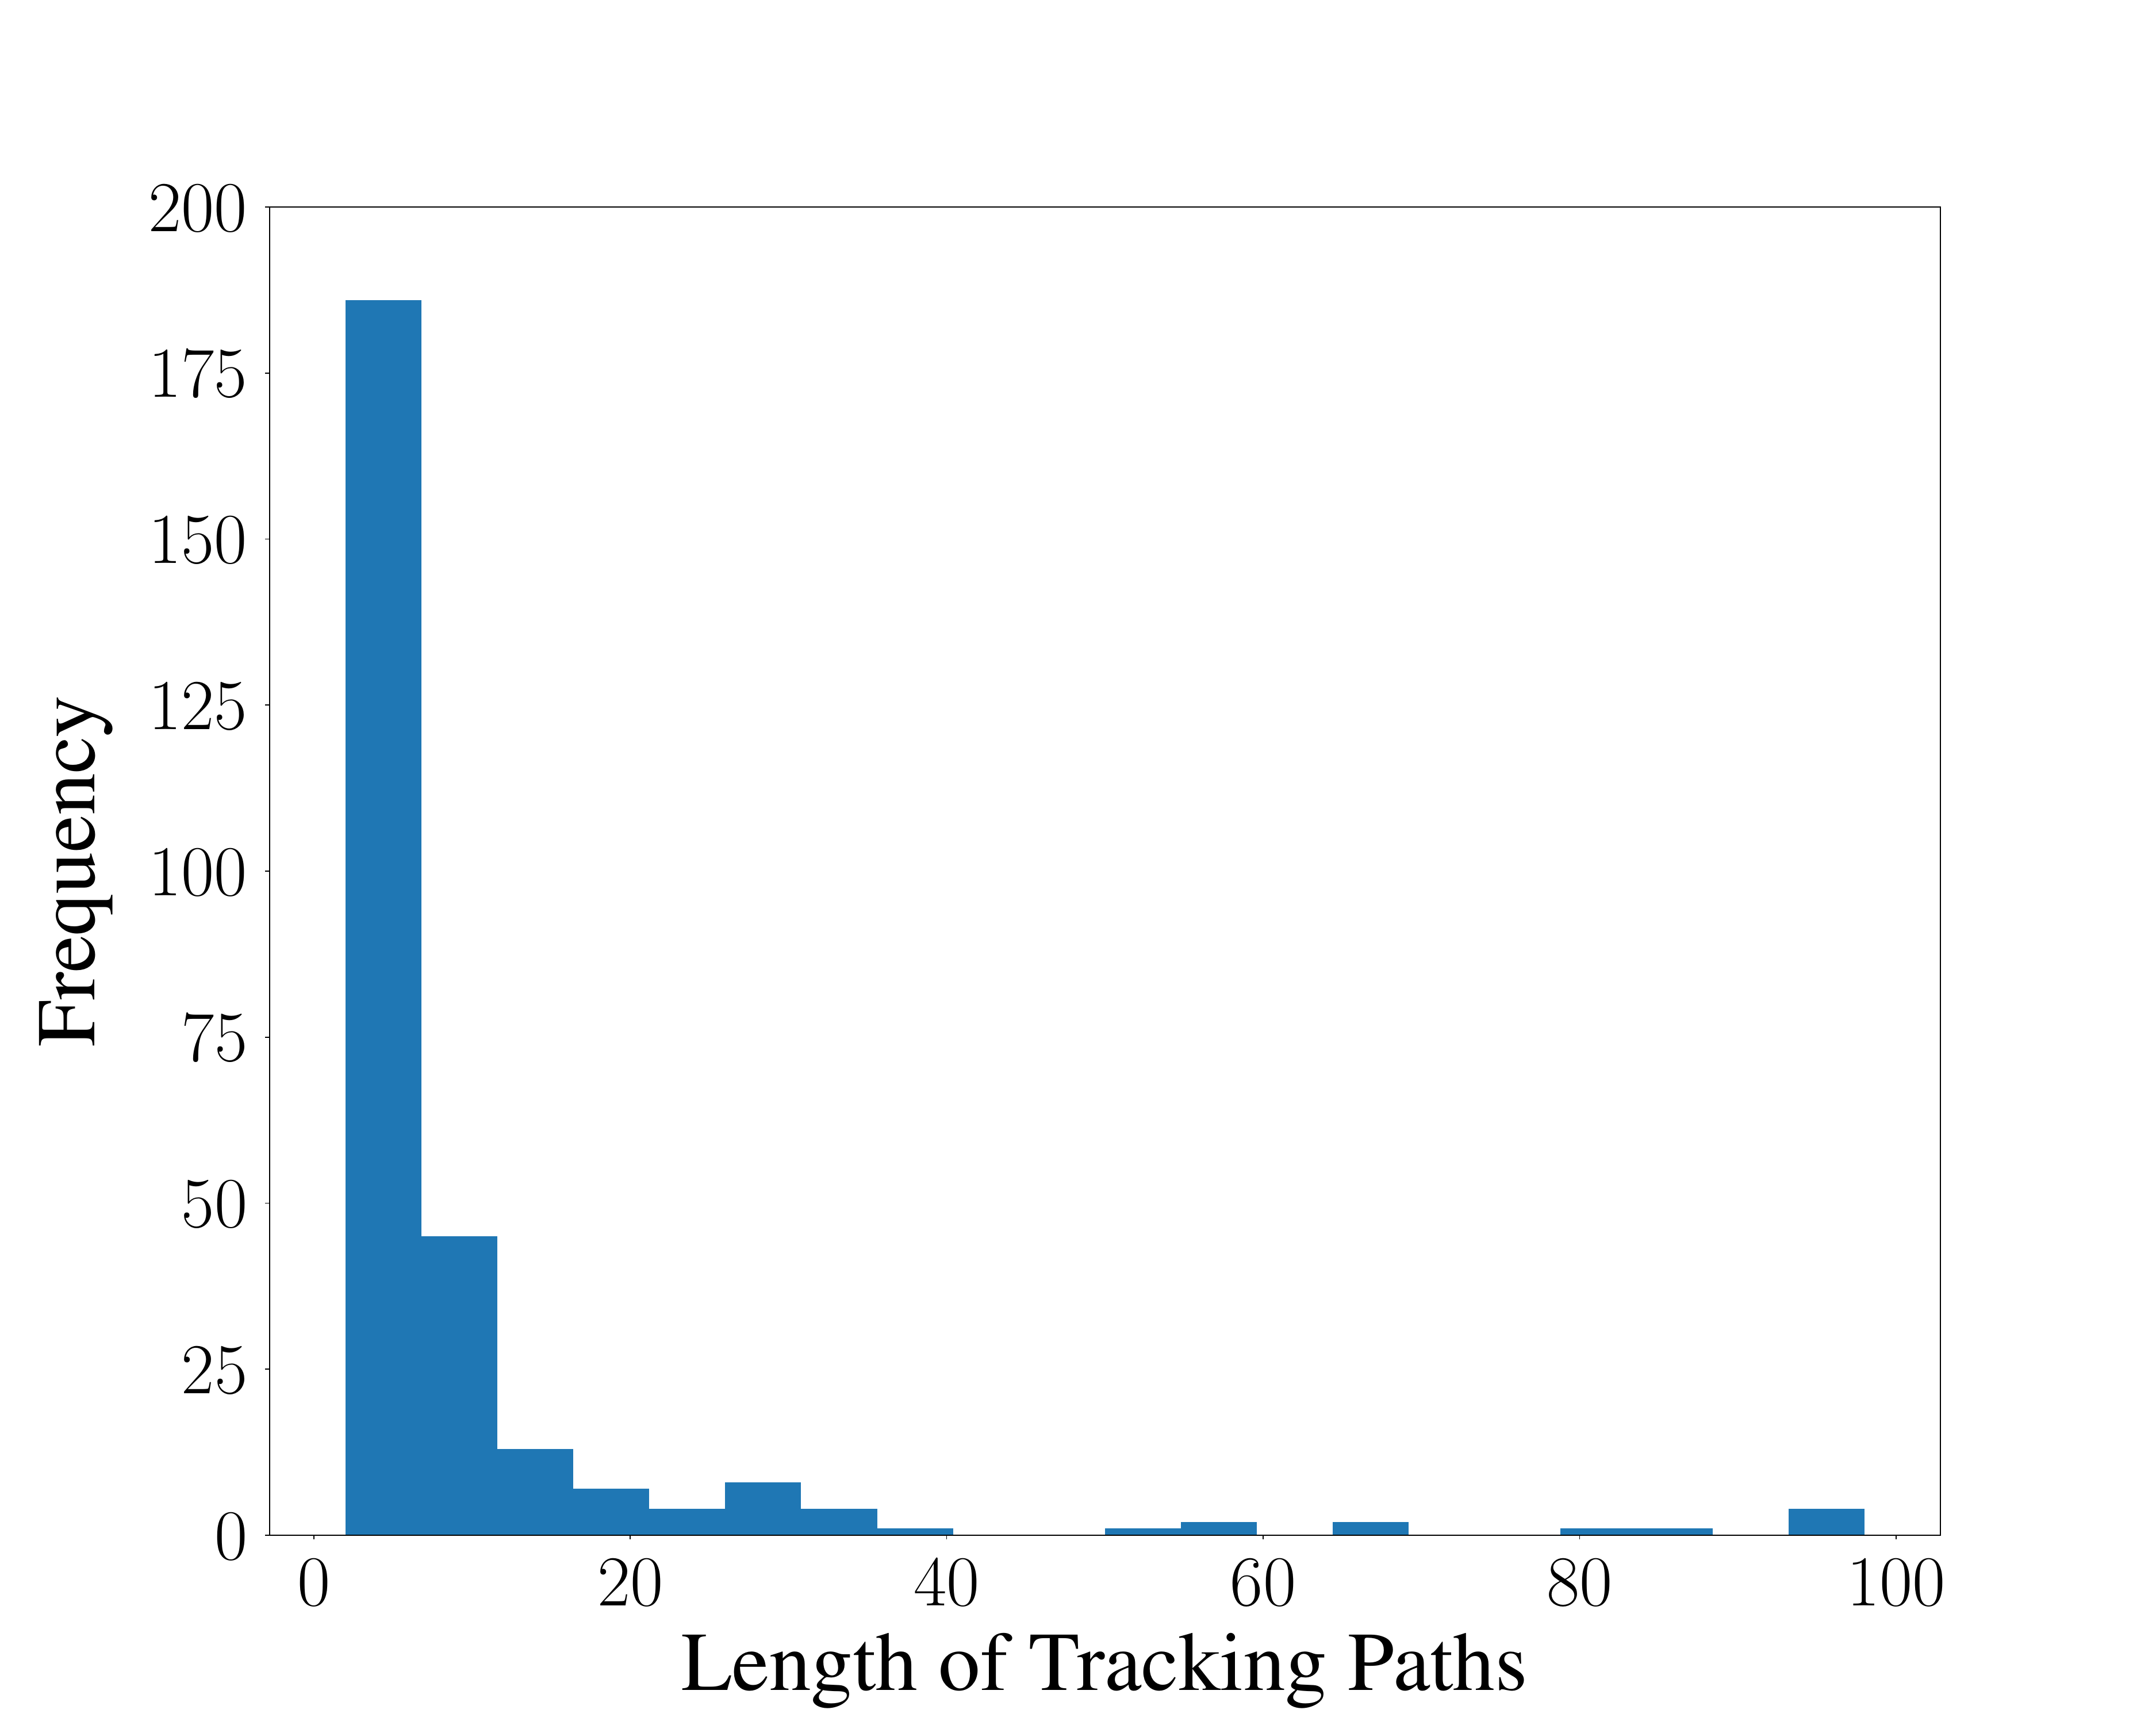}%
\caption{$d_e$.}%
\label{fig-LengthHistogramIonizationFront2DE}%
\end{subfigure}%
\\%
\begin{subfigure}[t]{\ltwopicwidth}%
\includegraphics[width=\ltwopicwidth]{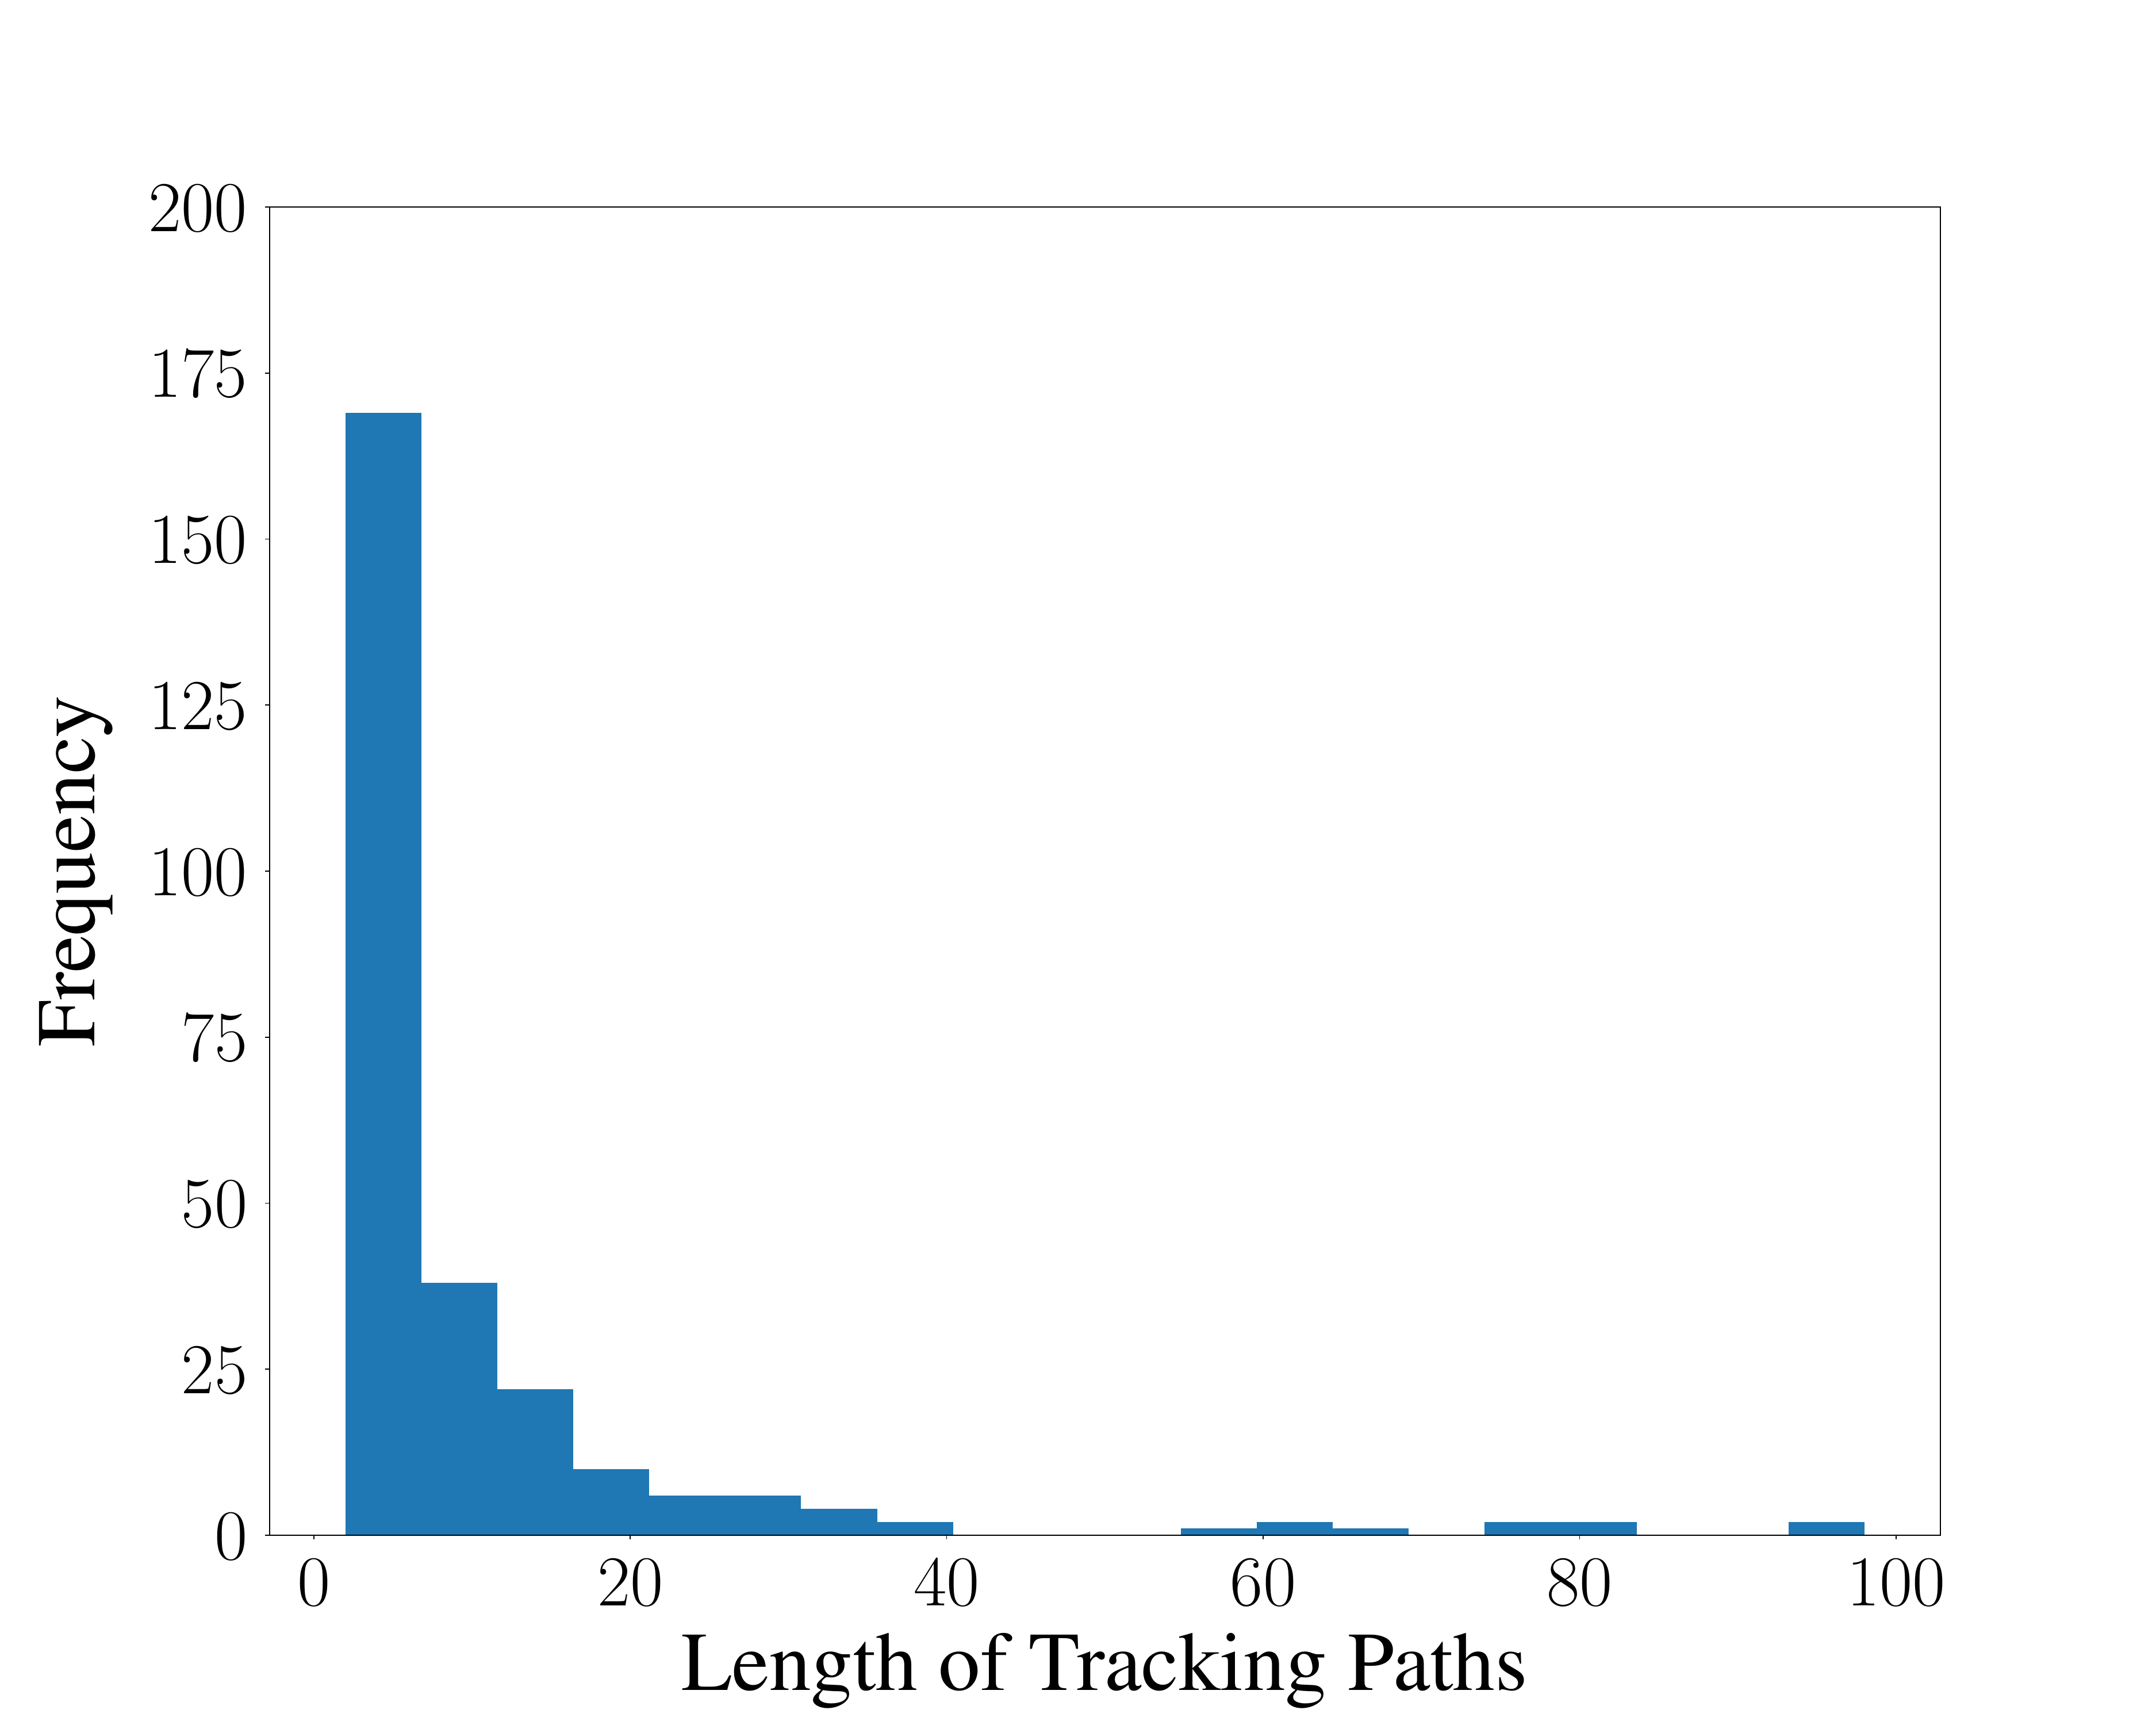}%
\caption{$d_b$.}%
\label{fig-LengthHistogramIonizationFront2DB}%
\end{subfigure}%
\hfill%
\begin{subfigure}[t]{\ltwopicwidth}%
\includegraphics[width=\ltwopicwidth]{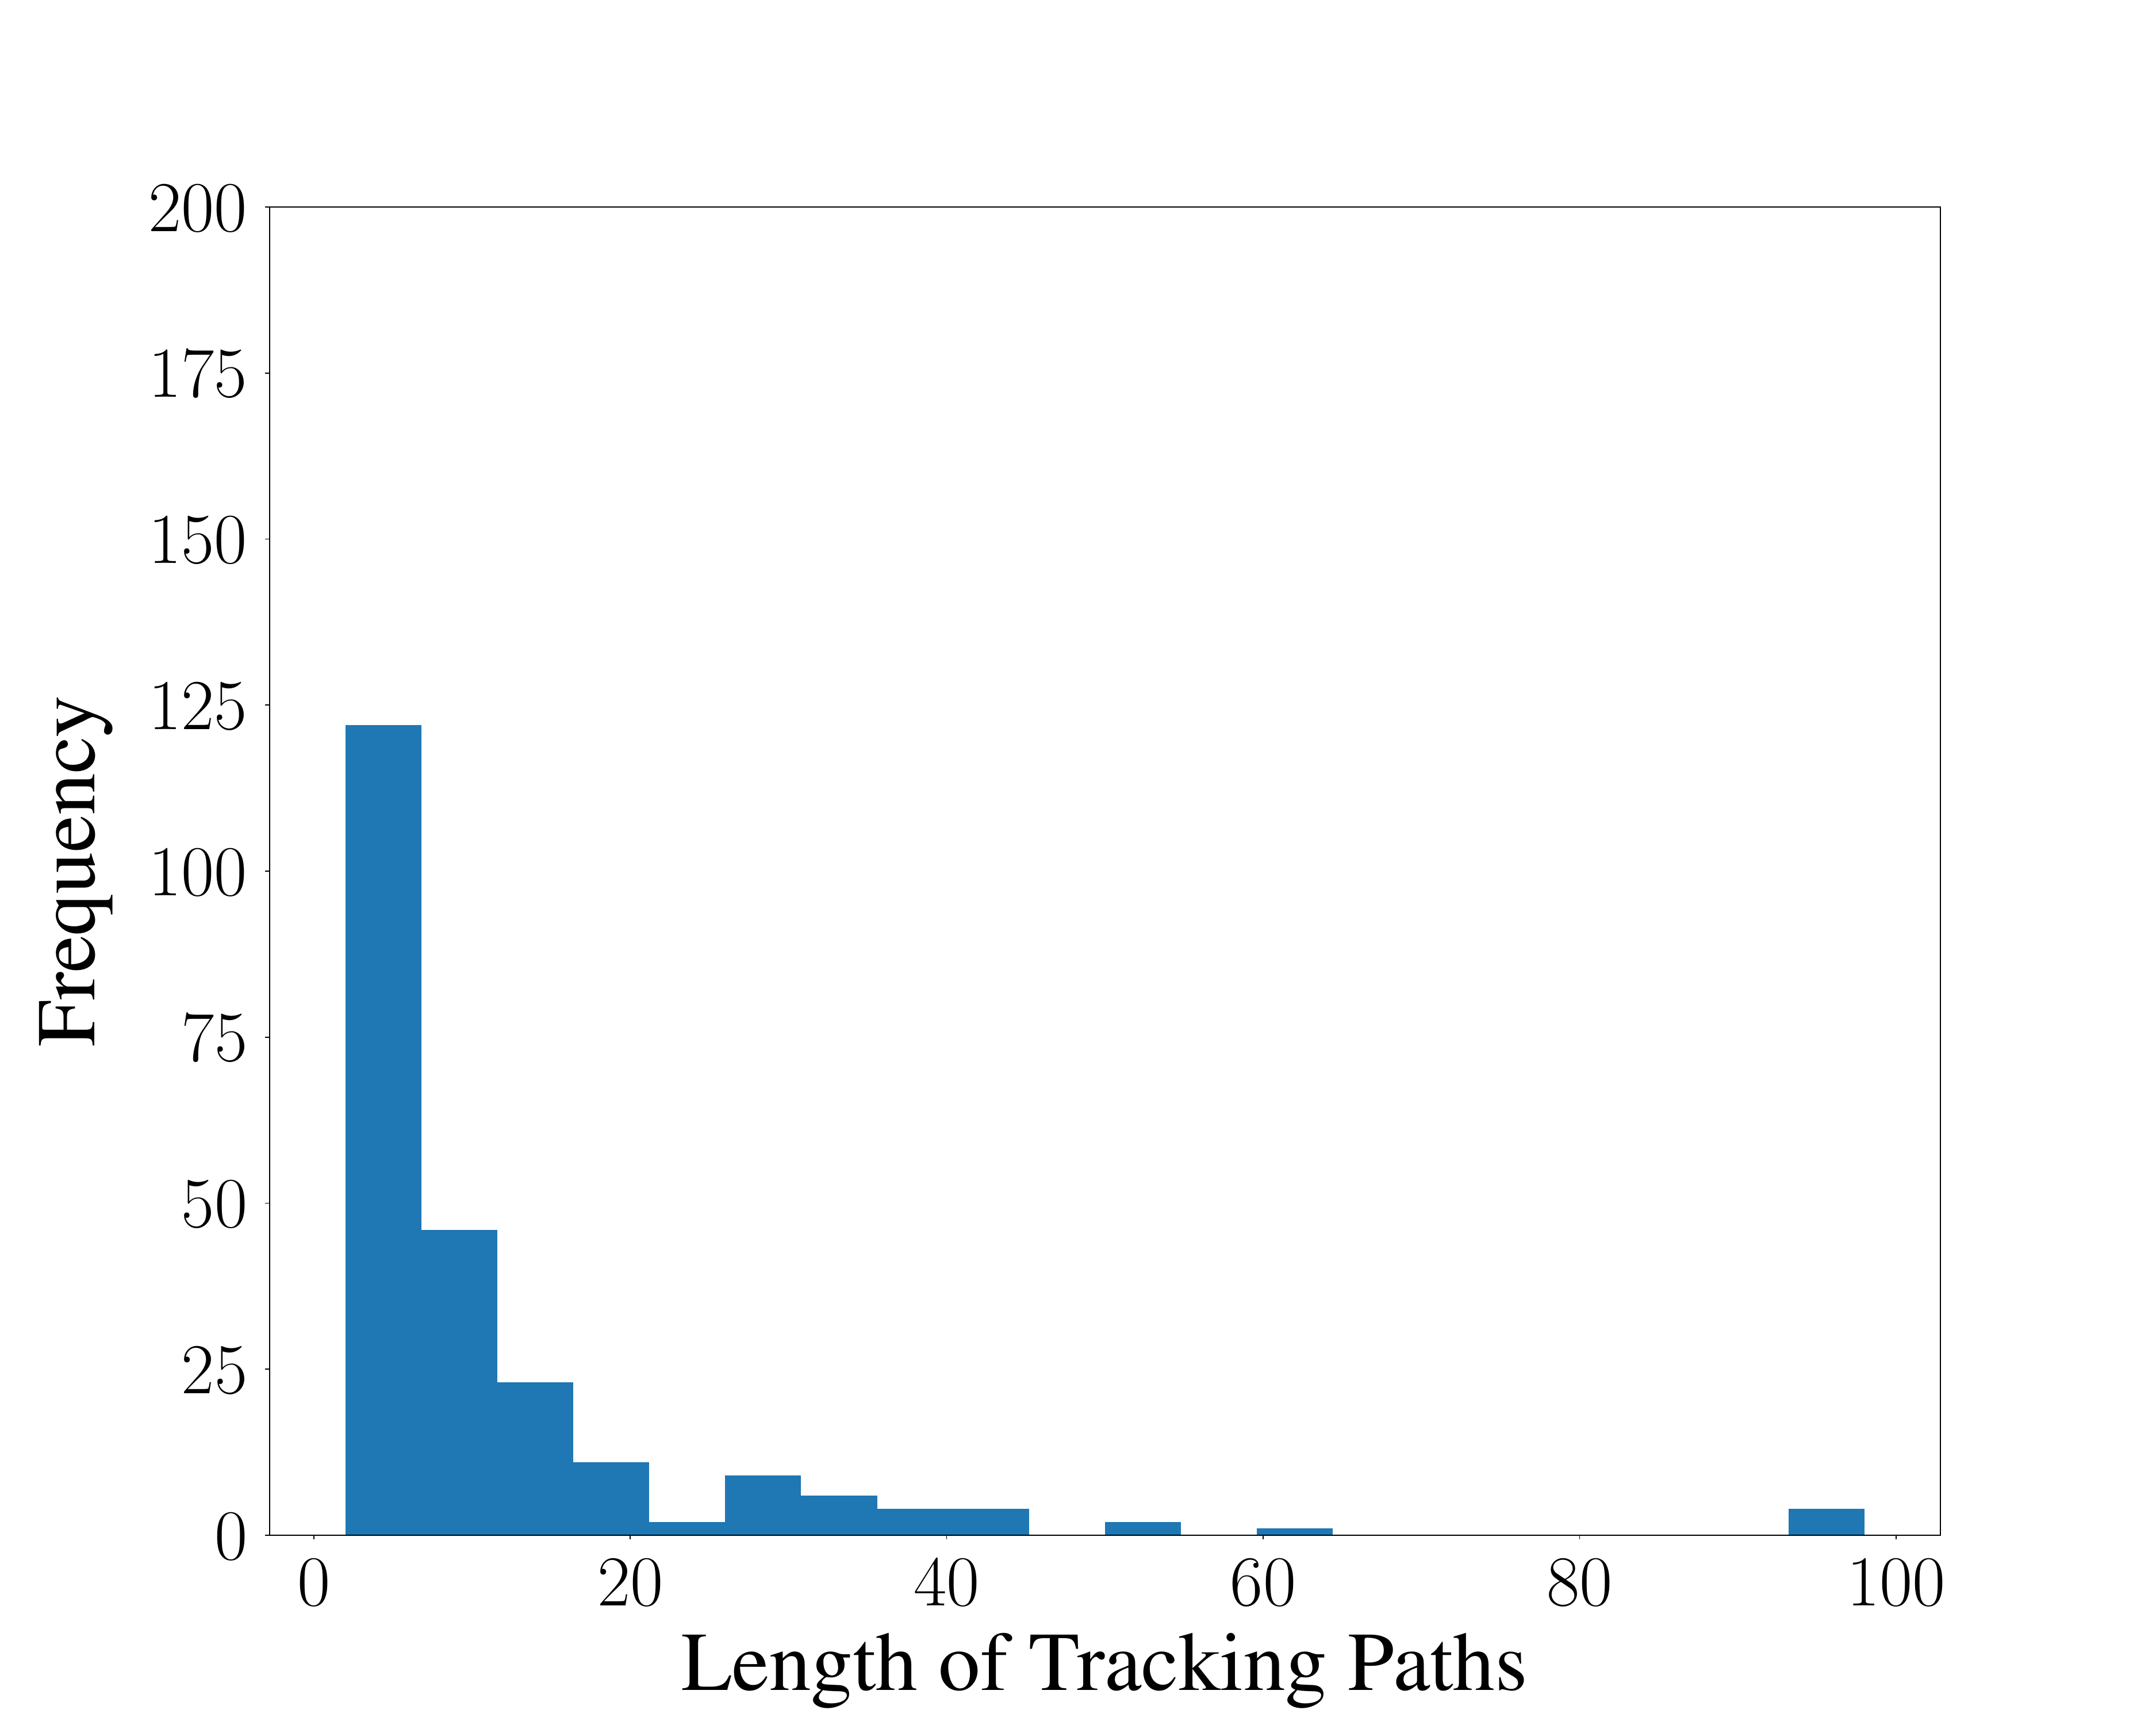}%
\caption{$d_p$.}%
\label{fig-LengthHistogramIonizationFront2DP}%
\end{subfigure}%
\caption{Histograms of the length of the tracking paths of the first $100$ time steps 
    of \dataset{IonizationFront2D}.}%
\label{fig-LengthHisgoramIonizationFront2D}%
\end{figure}

\begin{figure}
\centering
\includegraphics[width=0.8\linewidth]{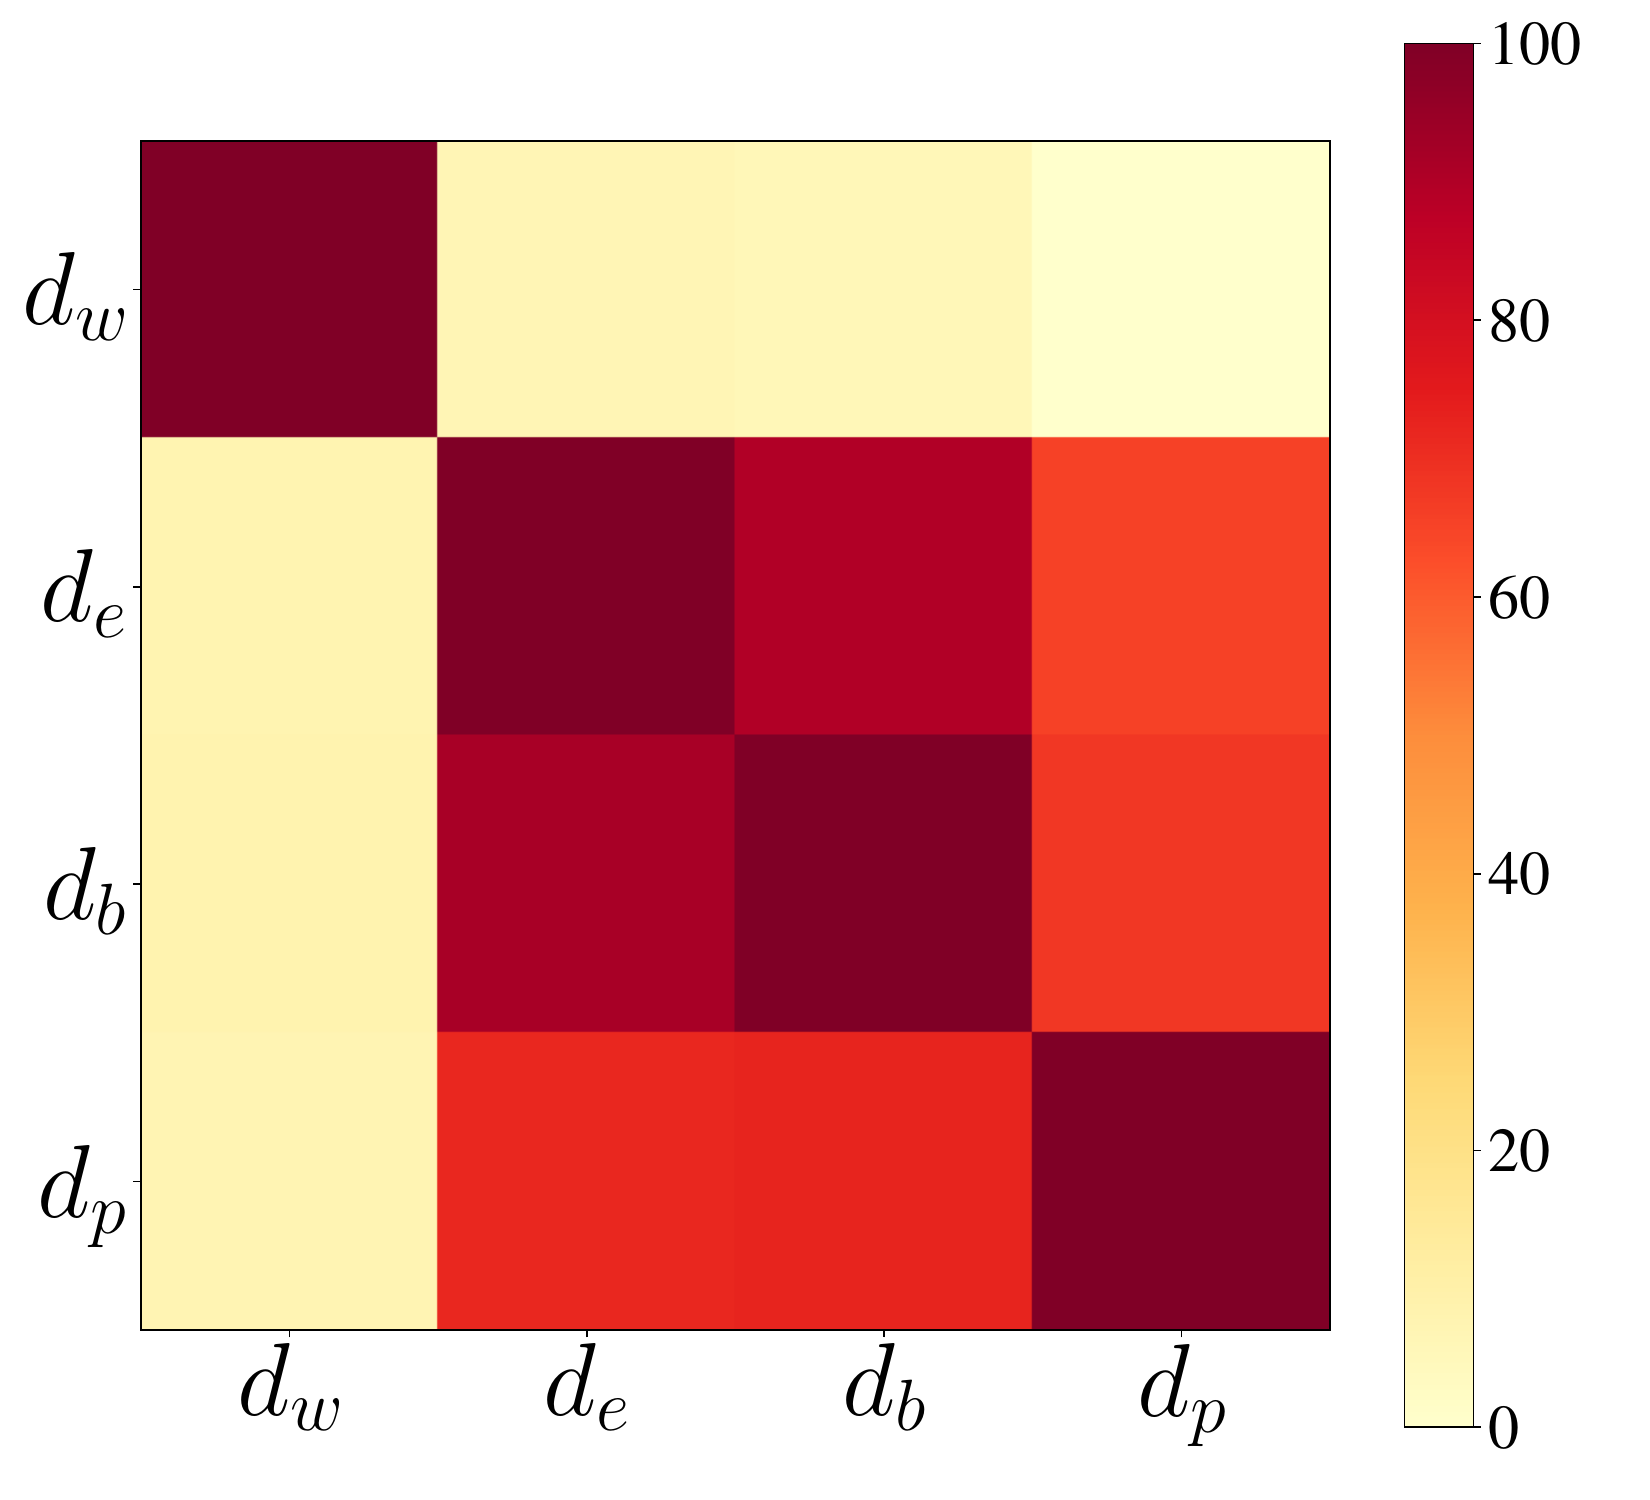}
\caption{
    Pairwise differences between the methods on the columns
    in relation to the methods on the rows
    for \dataset{IonizationFront2D}.
}
\label{fig-IonizationFront2DSimilarities}
\end{figure}

\subsection*{Results using Storms2D}
The results of the experiments using \dataset{Storms2D}
are shown from \Cref{fig-Storms2DAllNodes}
to \Cref{fig-Storms2DSimilarities}.

\begin{figure}
\centering
\includegraphics[width=0.8\linewidth]{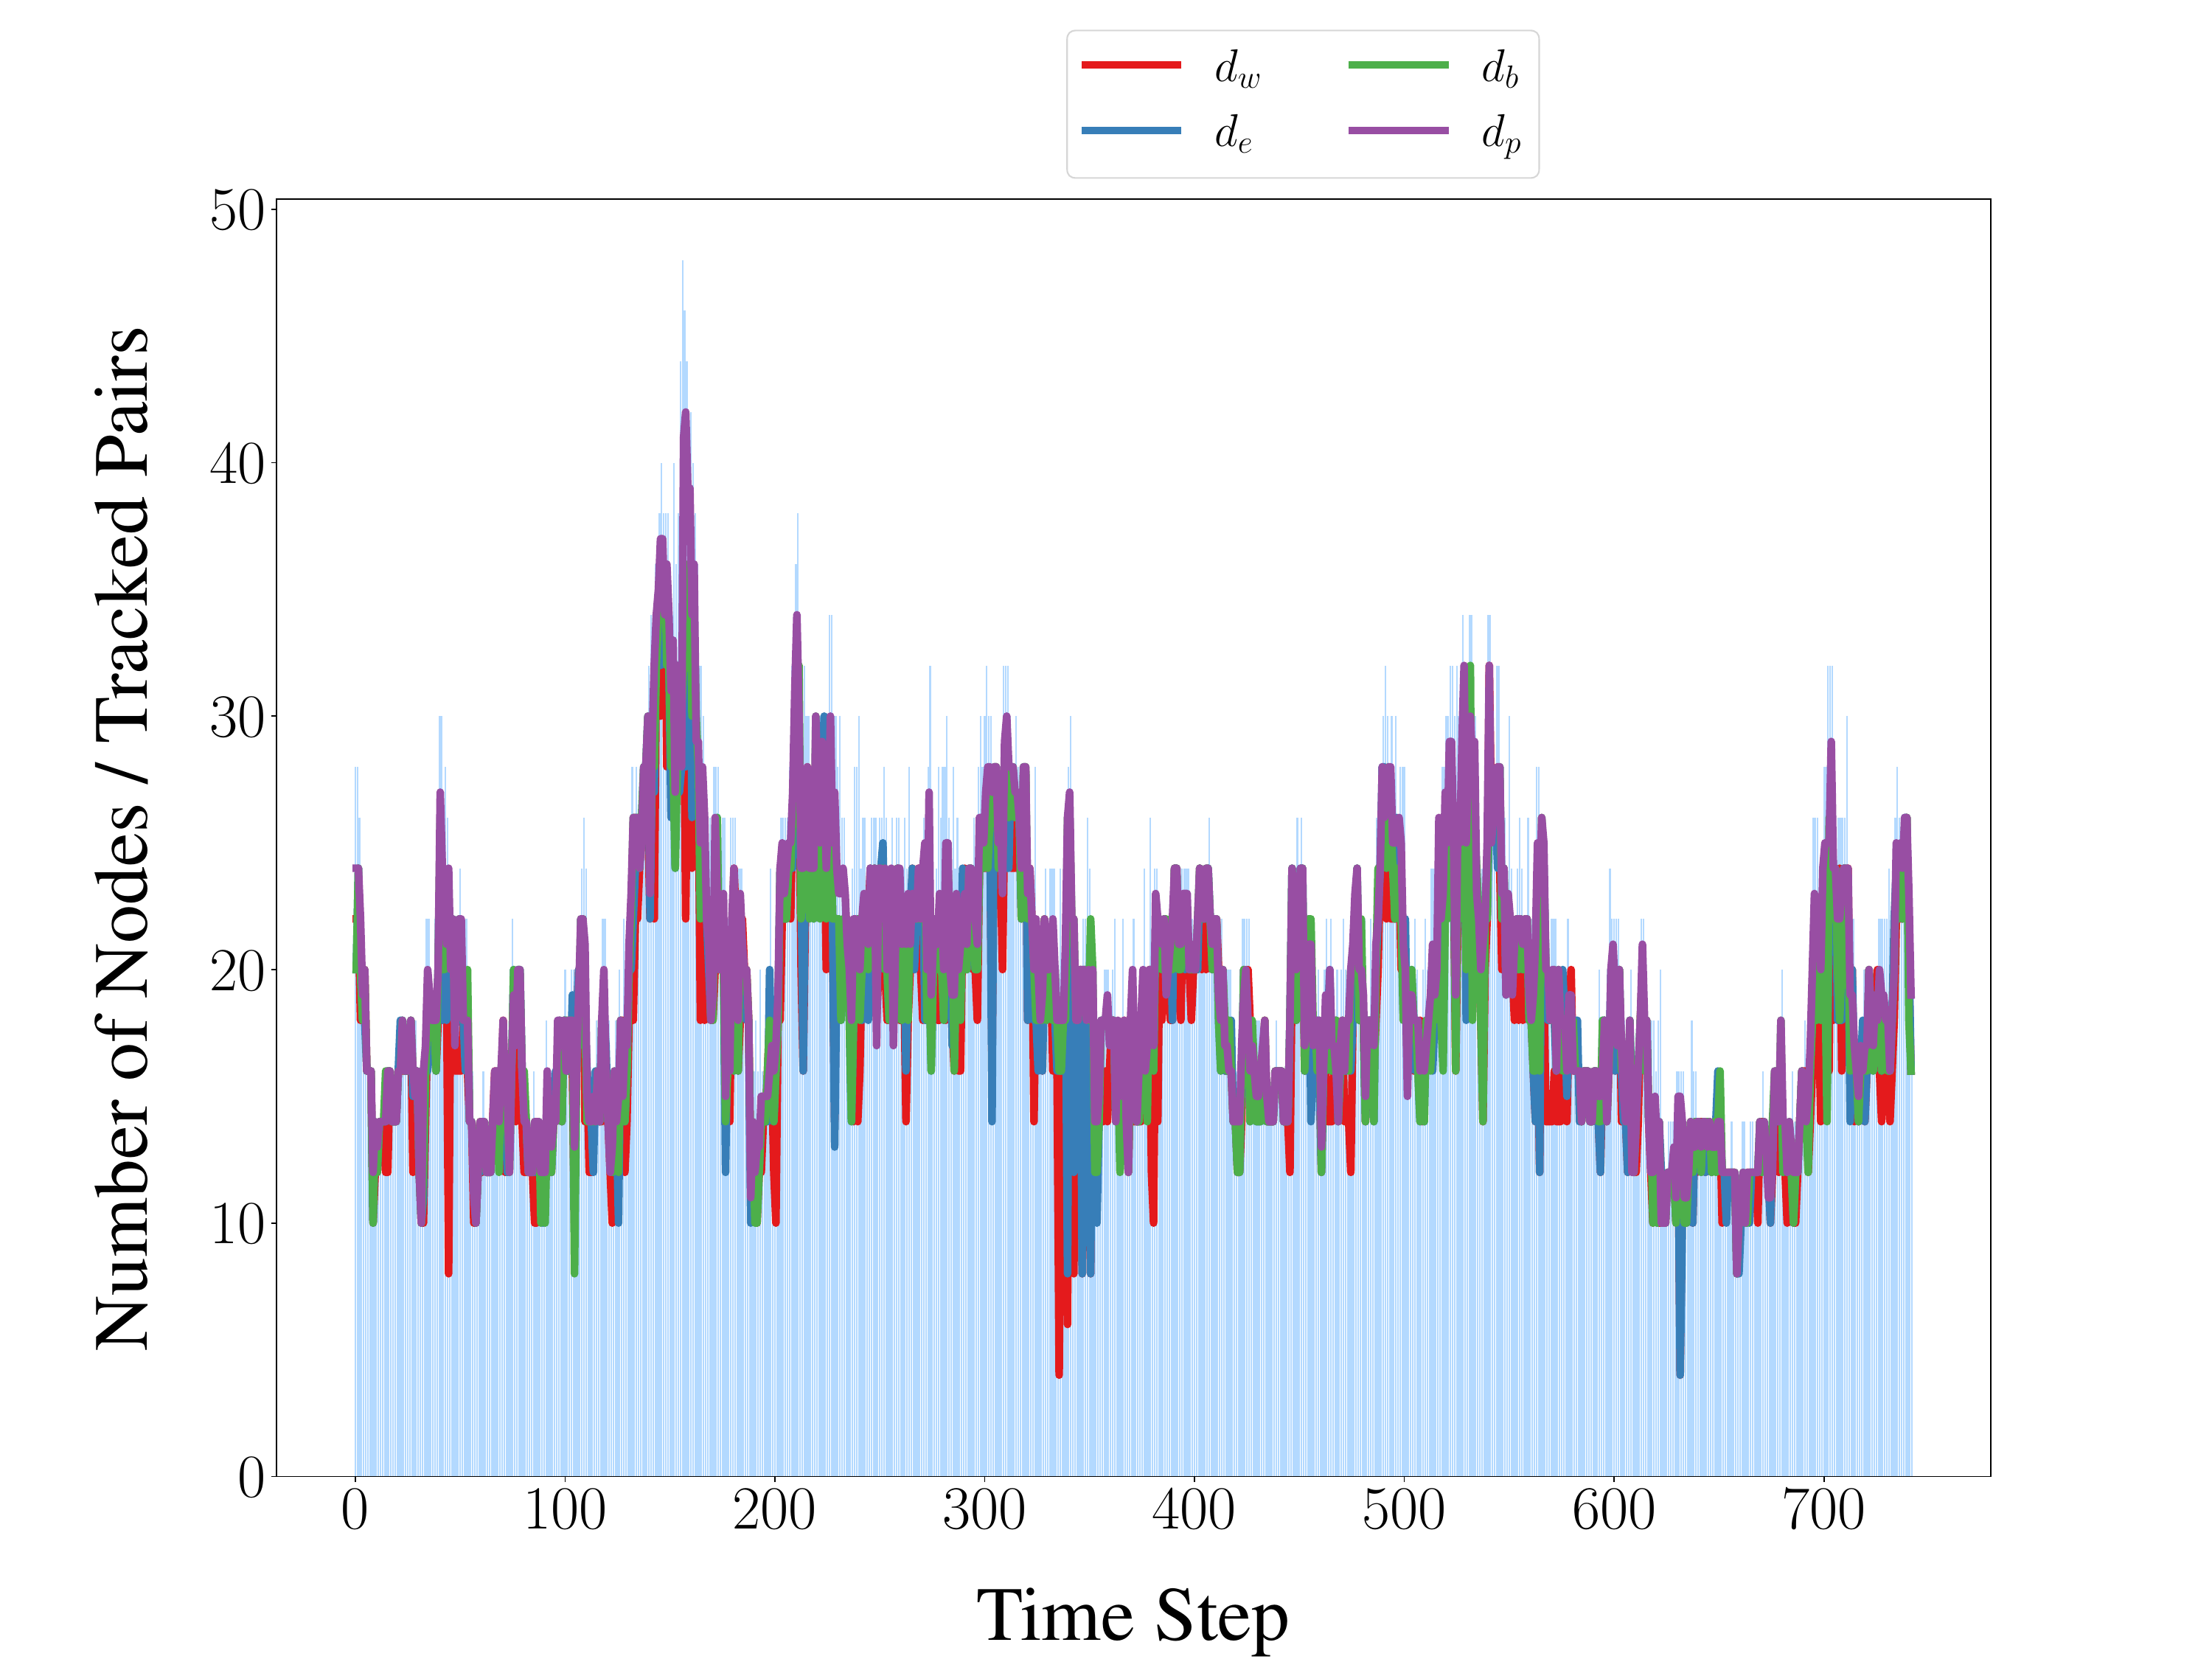}
\caption{
    Number of tracked nodes (colored and labeled) 
    relative to the total nodes of merge trees (light blue bars)
    for \dataset{Storms2D}.
}
\label{fig-Storms2DAllNodes}
\end{figure}

\begin{figure}
\centering
\includegraphics[width=0.8\linewidth]{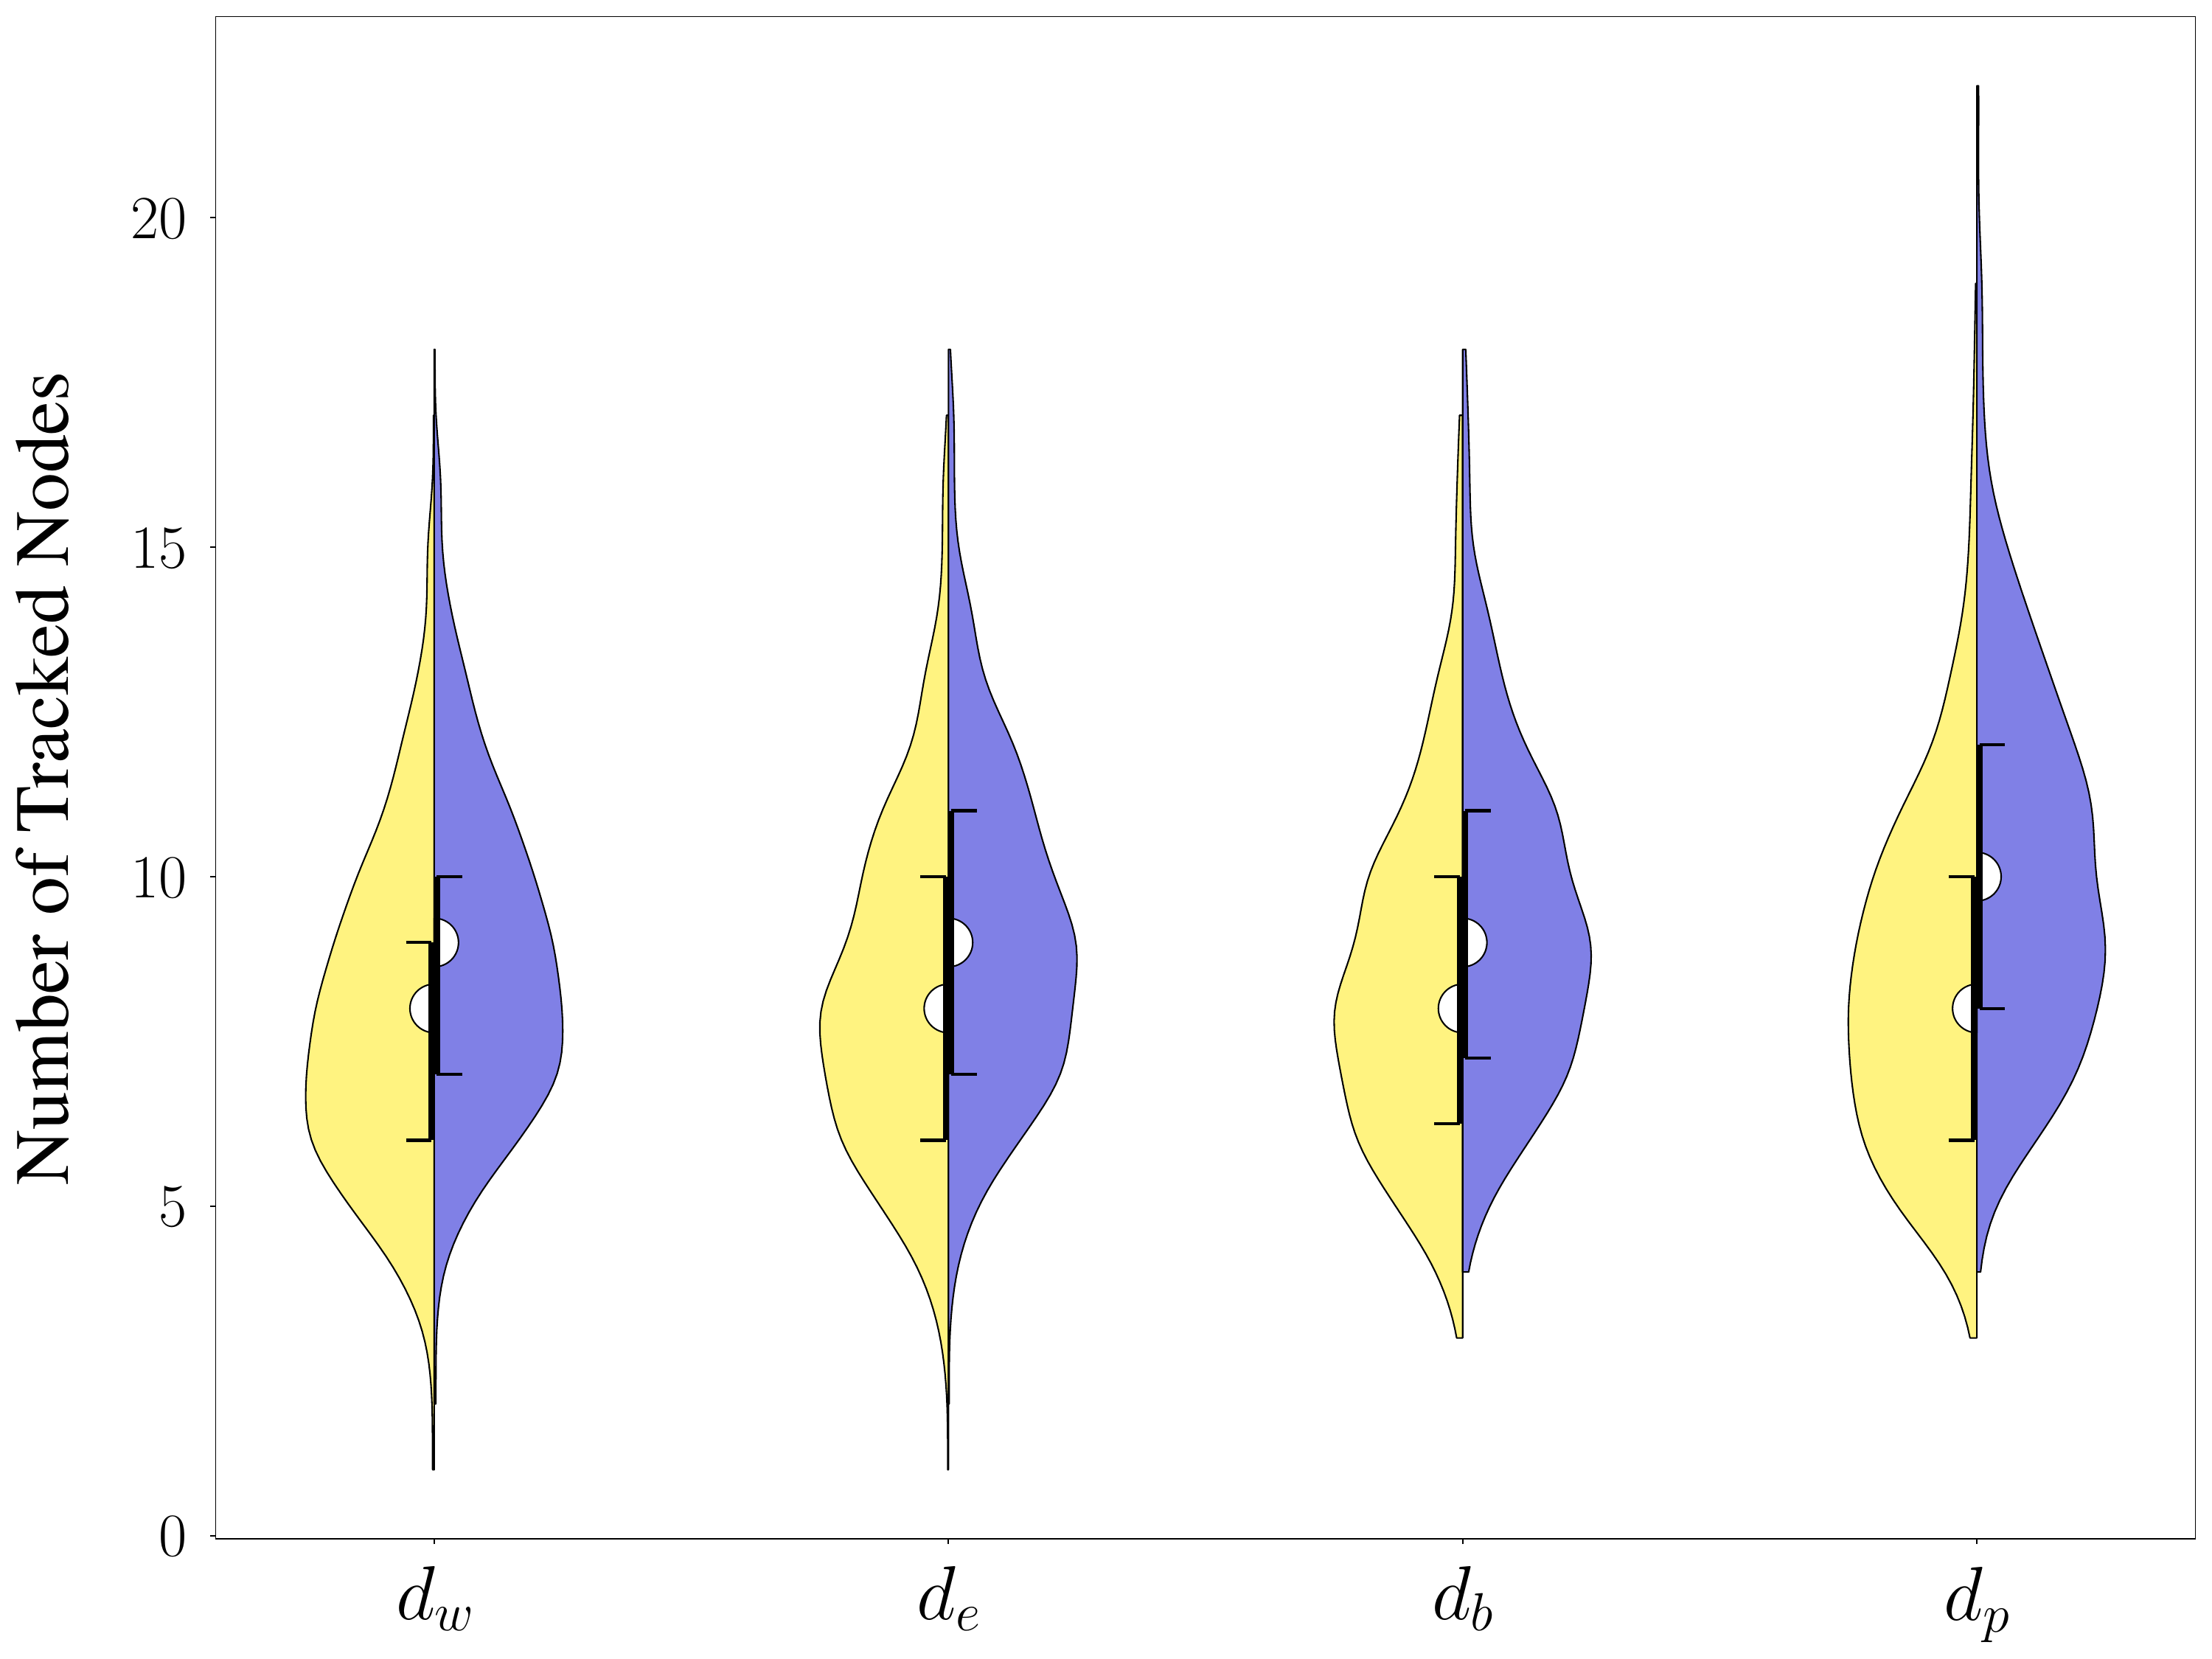}
\caption{
    Distributions of tracked nodes 
    of \dataset{Storms2D},  
    divided by types:
    saddle (yellow) and minima (blue).
}
\label{fig-Storms2DViolin}
\end{figure}

% Length histogram
\begin{figure}%
\begin{subfigure}[t]{\ltwopicwidth}%
\includegraphics[width=\ltwopicwidth]{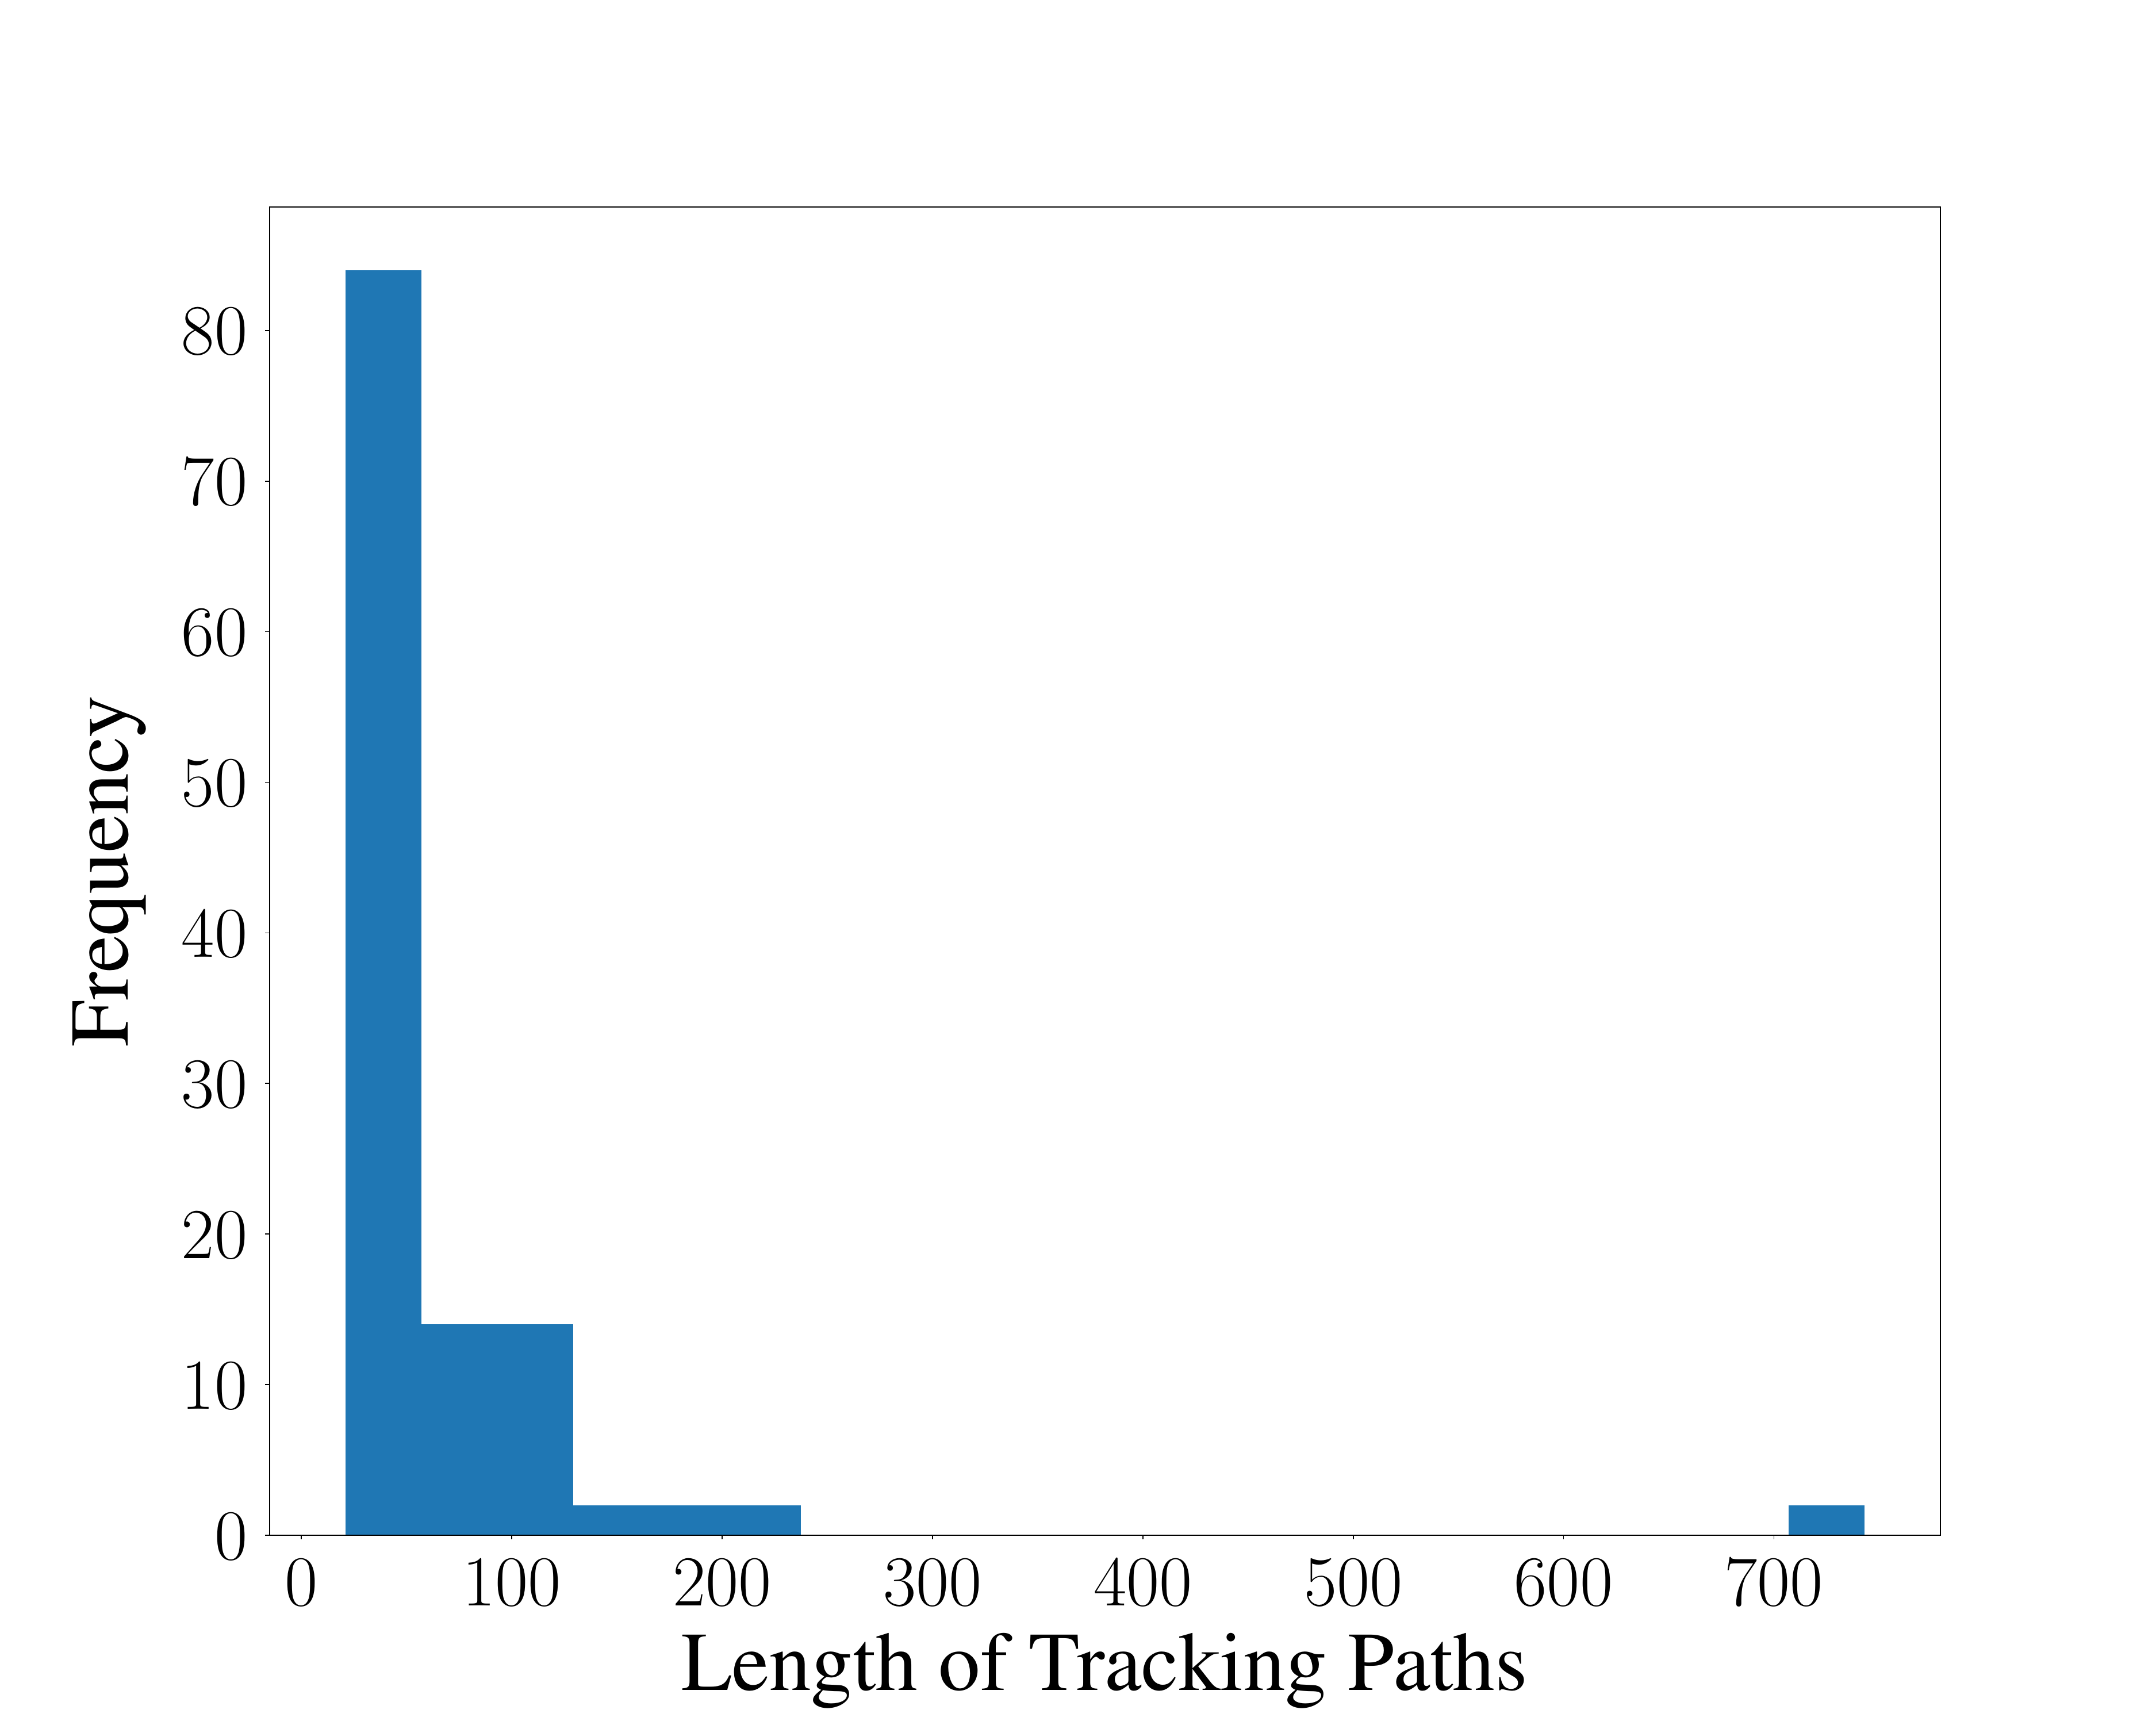}
\caption{$d_w$.}%
\label{fig-LengthHistogramStorms2DW}%
\end{subfigure}
\hfill%
\begin{subfigure}[t]{\ltwopicwidth}%
\includegraphics[width=\ltwopicwidth]{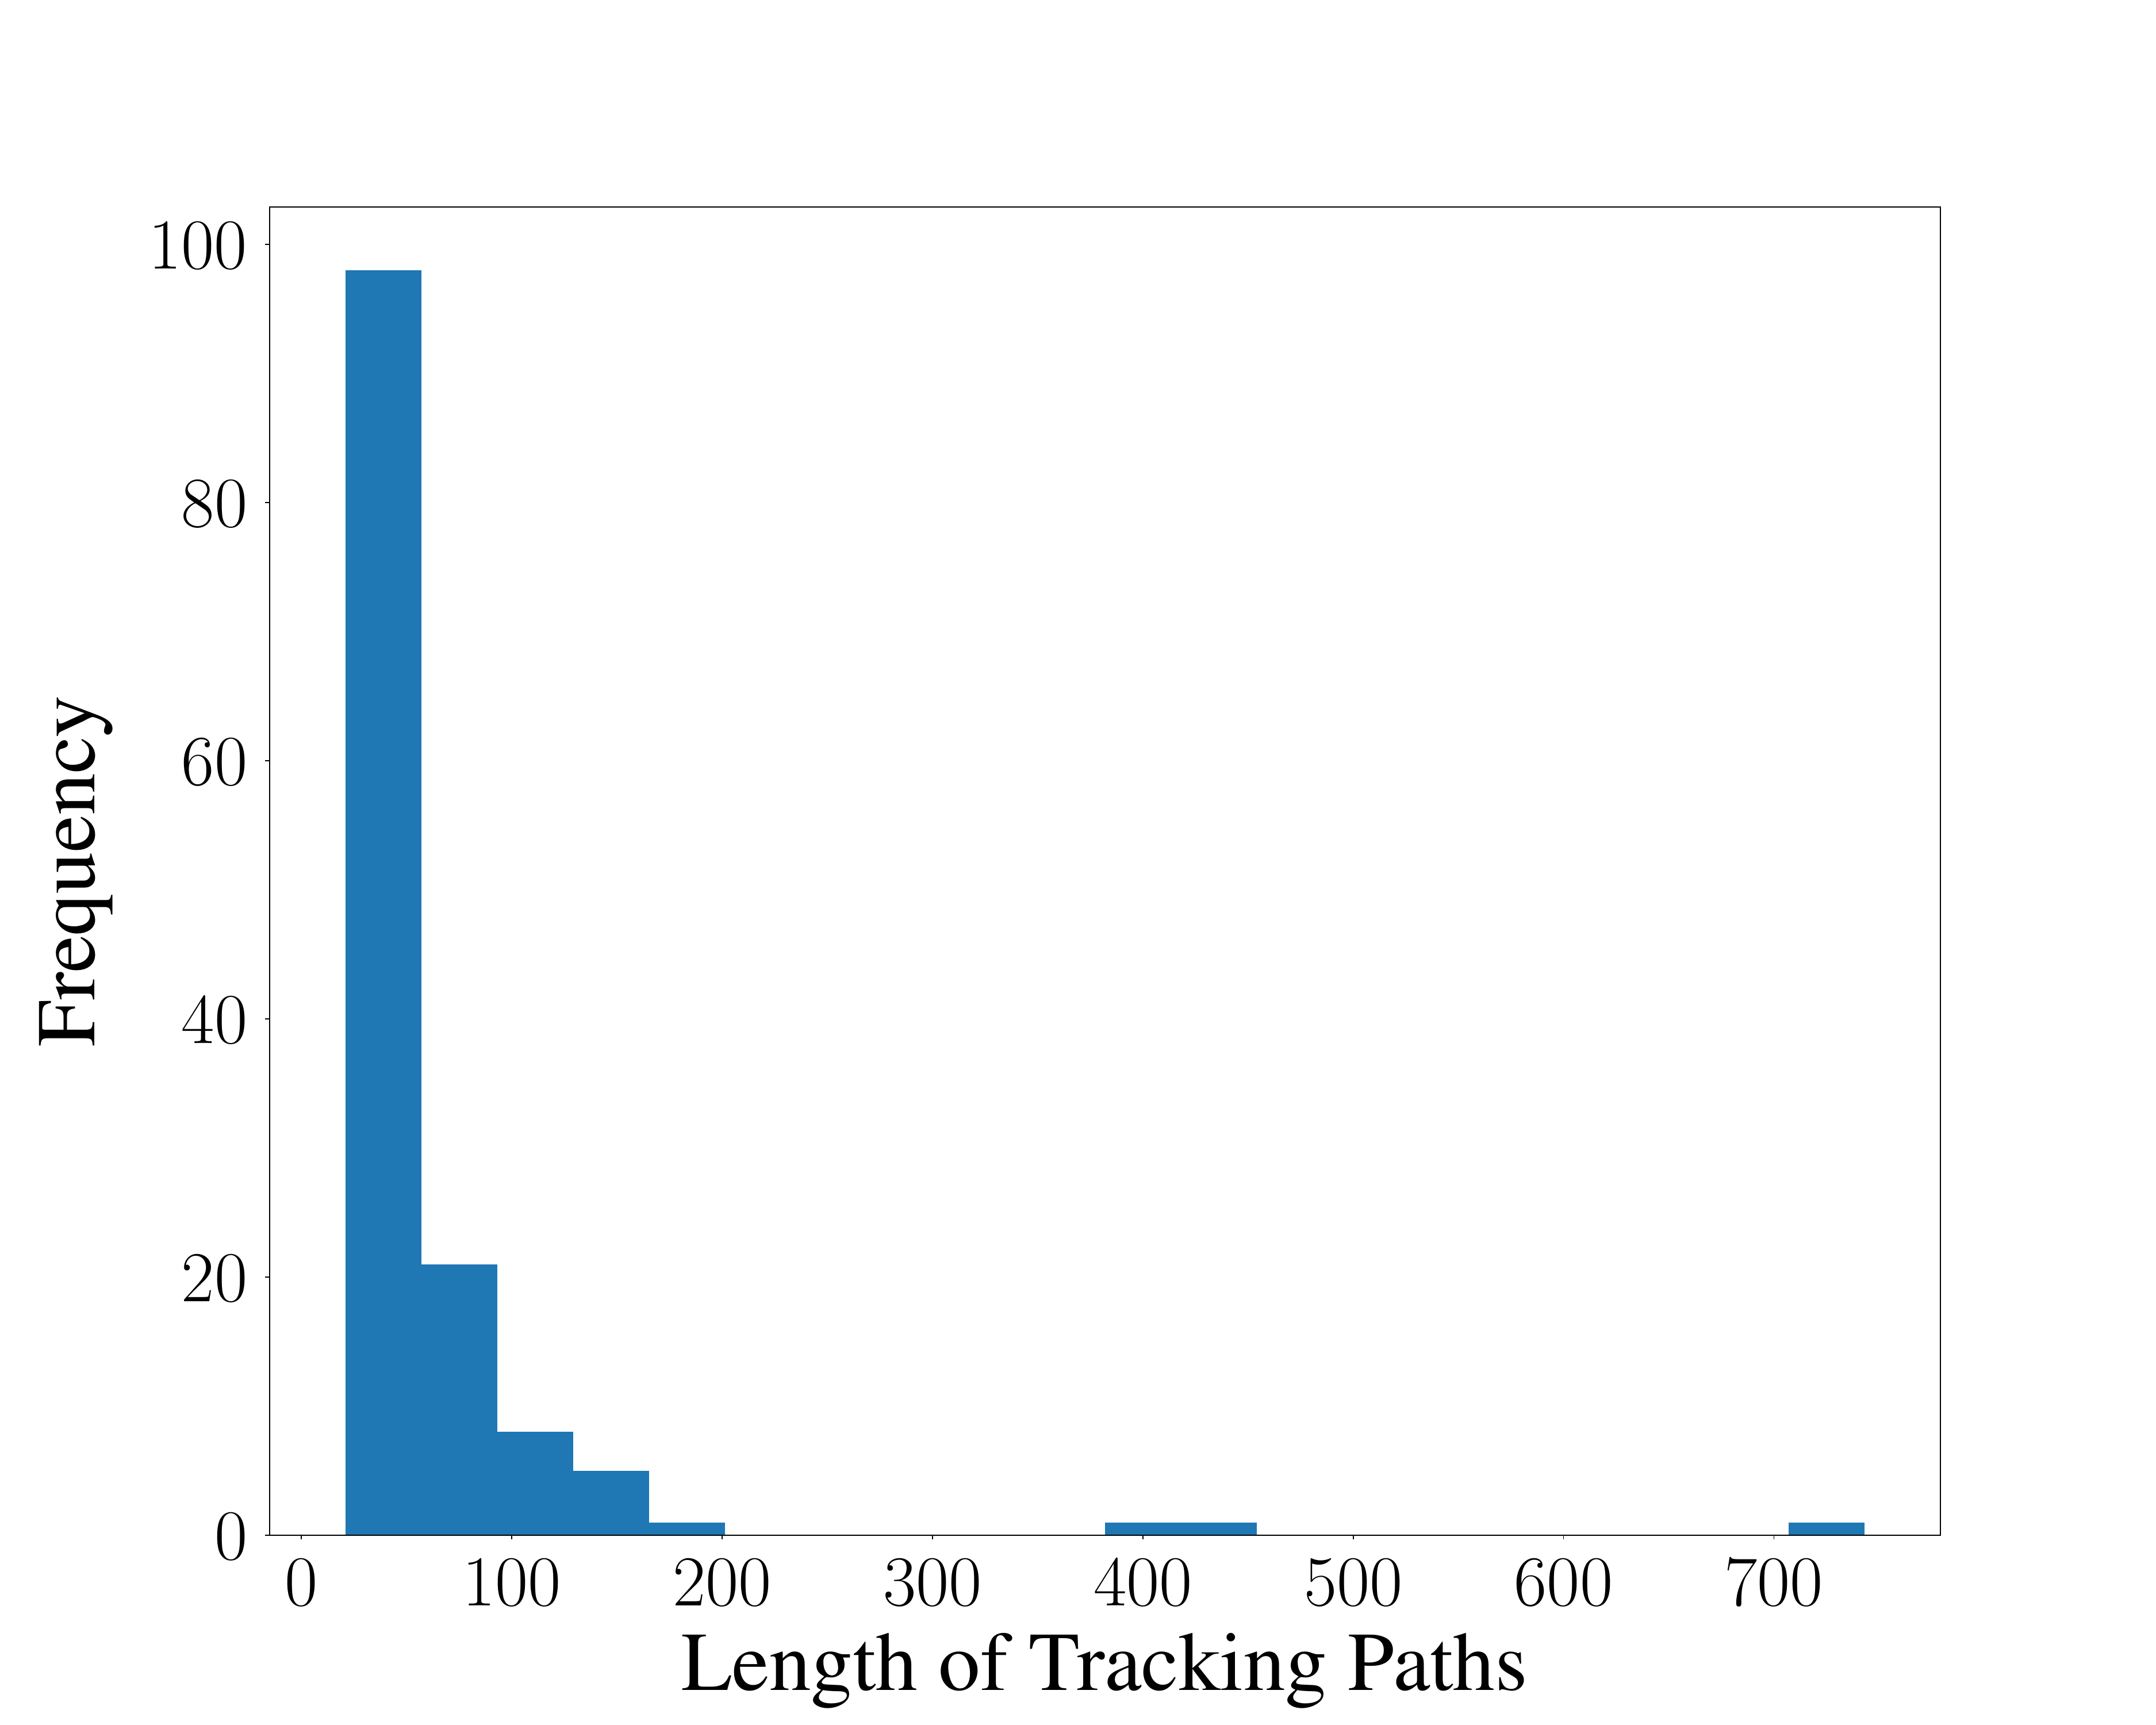}%
\caption{$d_e$.}%
\label{fig-LengthHistogramStorms2DE}%
\end{subfigure}%
\\%
\begin{subfigure}[t]{\ltwopicwidth}%
\includegraphics[width=\ltwopicwidth]{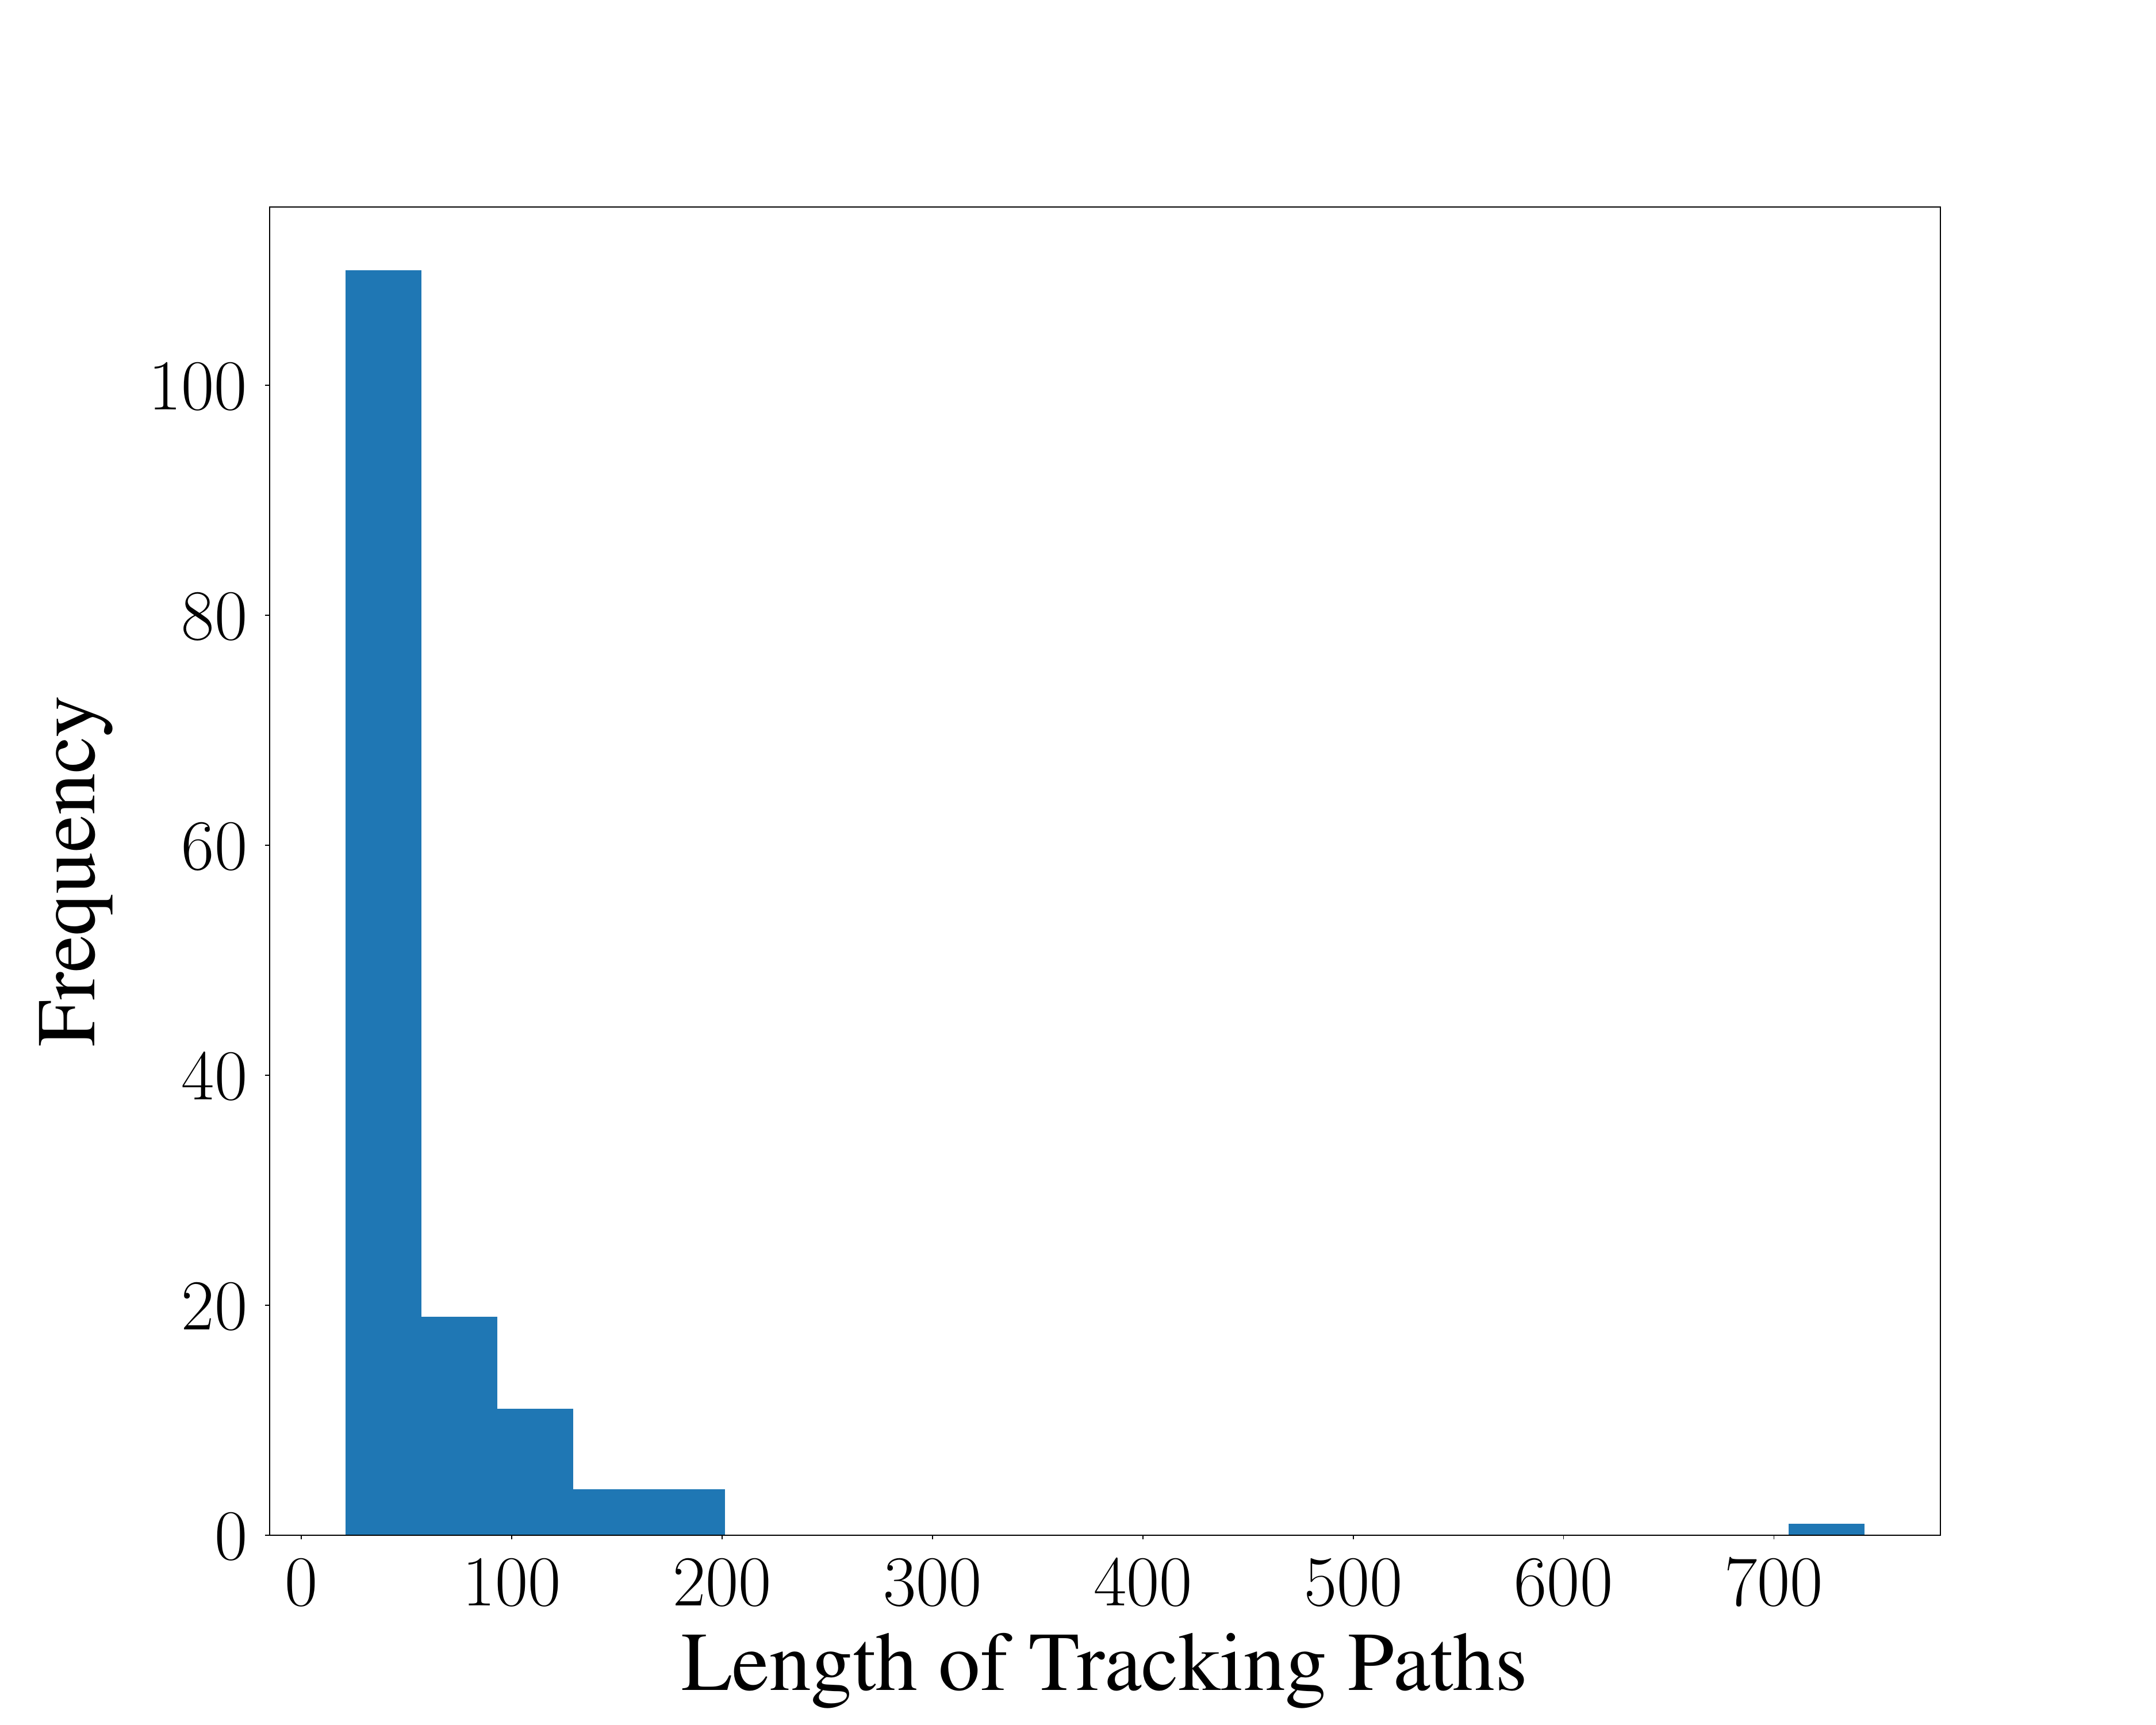}%
\caption{$d_b$.}%
\label{fig-LengthHistogramStorms2DB}%
\end{subfigure}%
\hfill%
\begin{subfigure}[t]{\ltwopicwidth}%
\includegraphics[width=\ltwopicwidth]{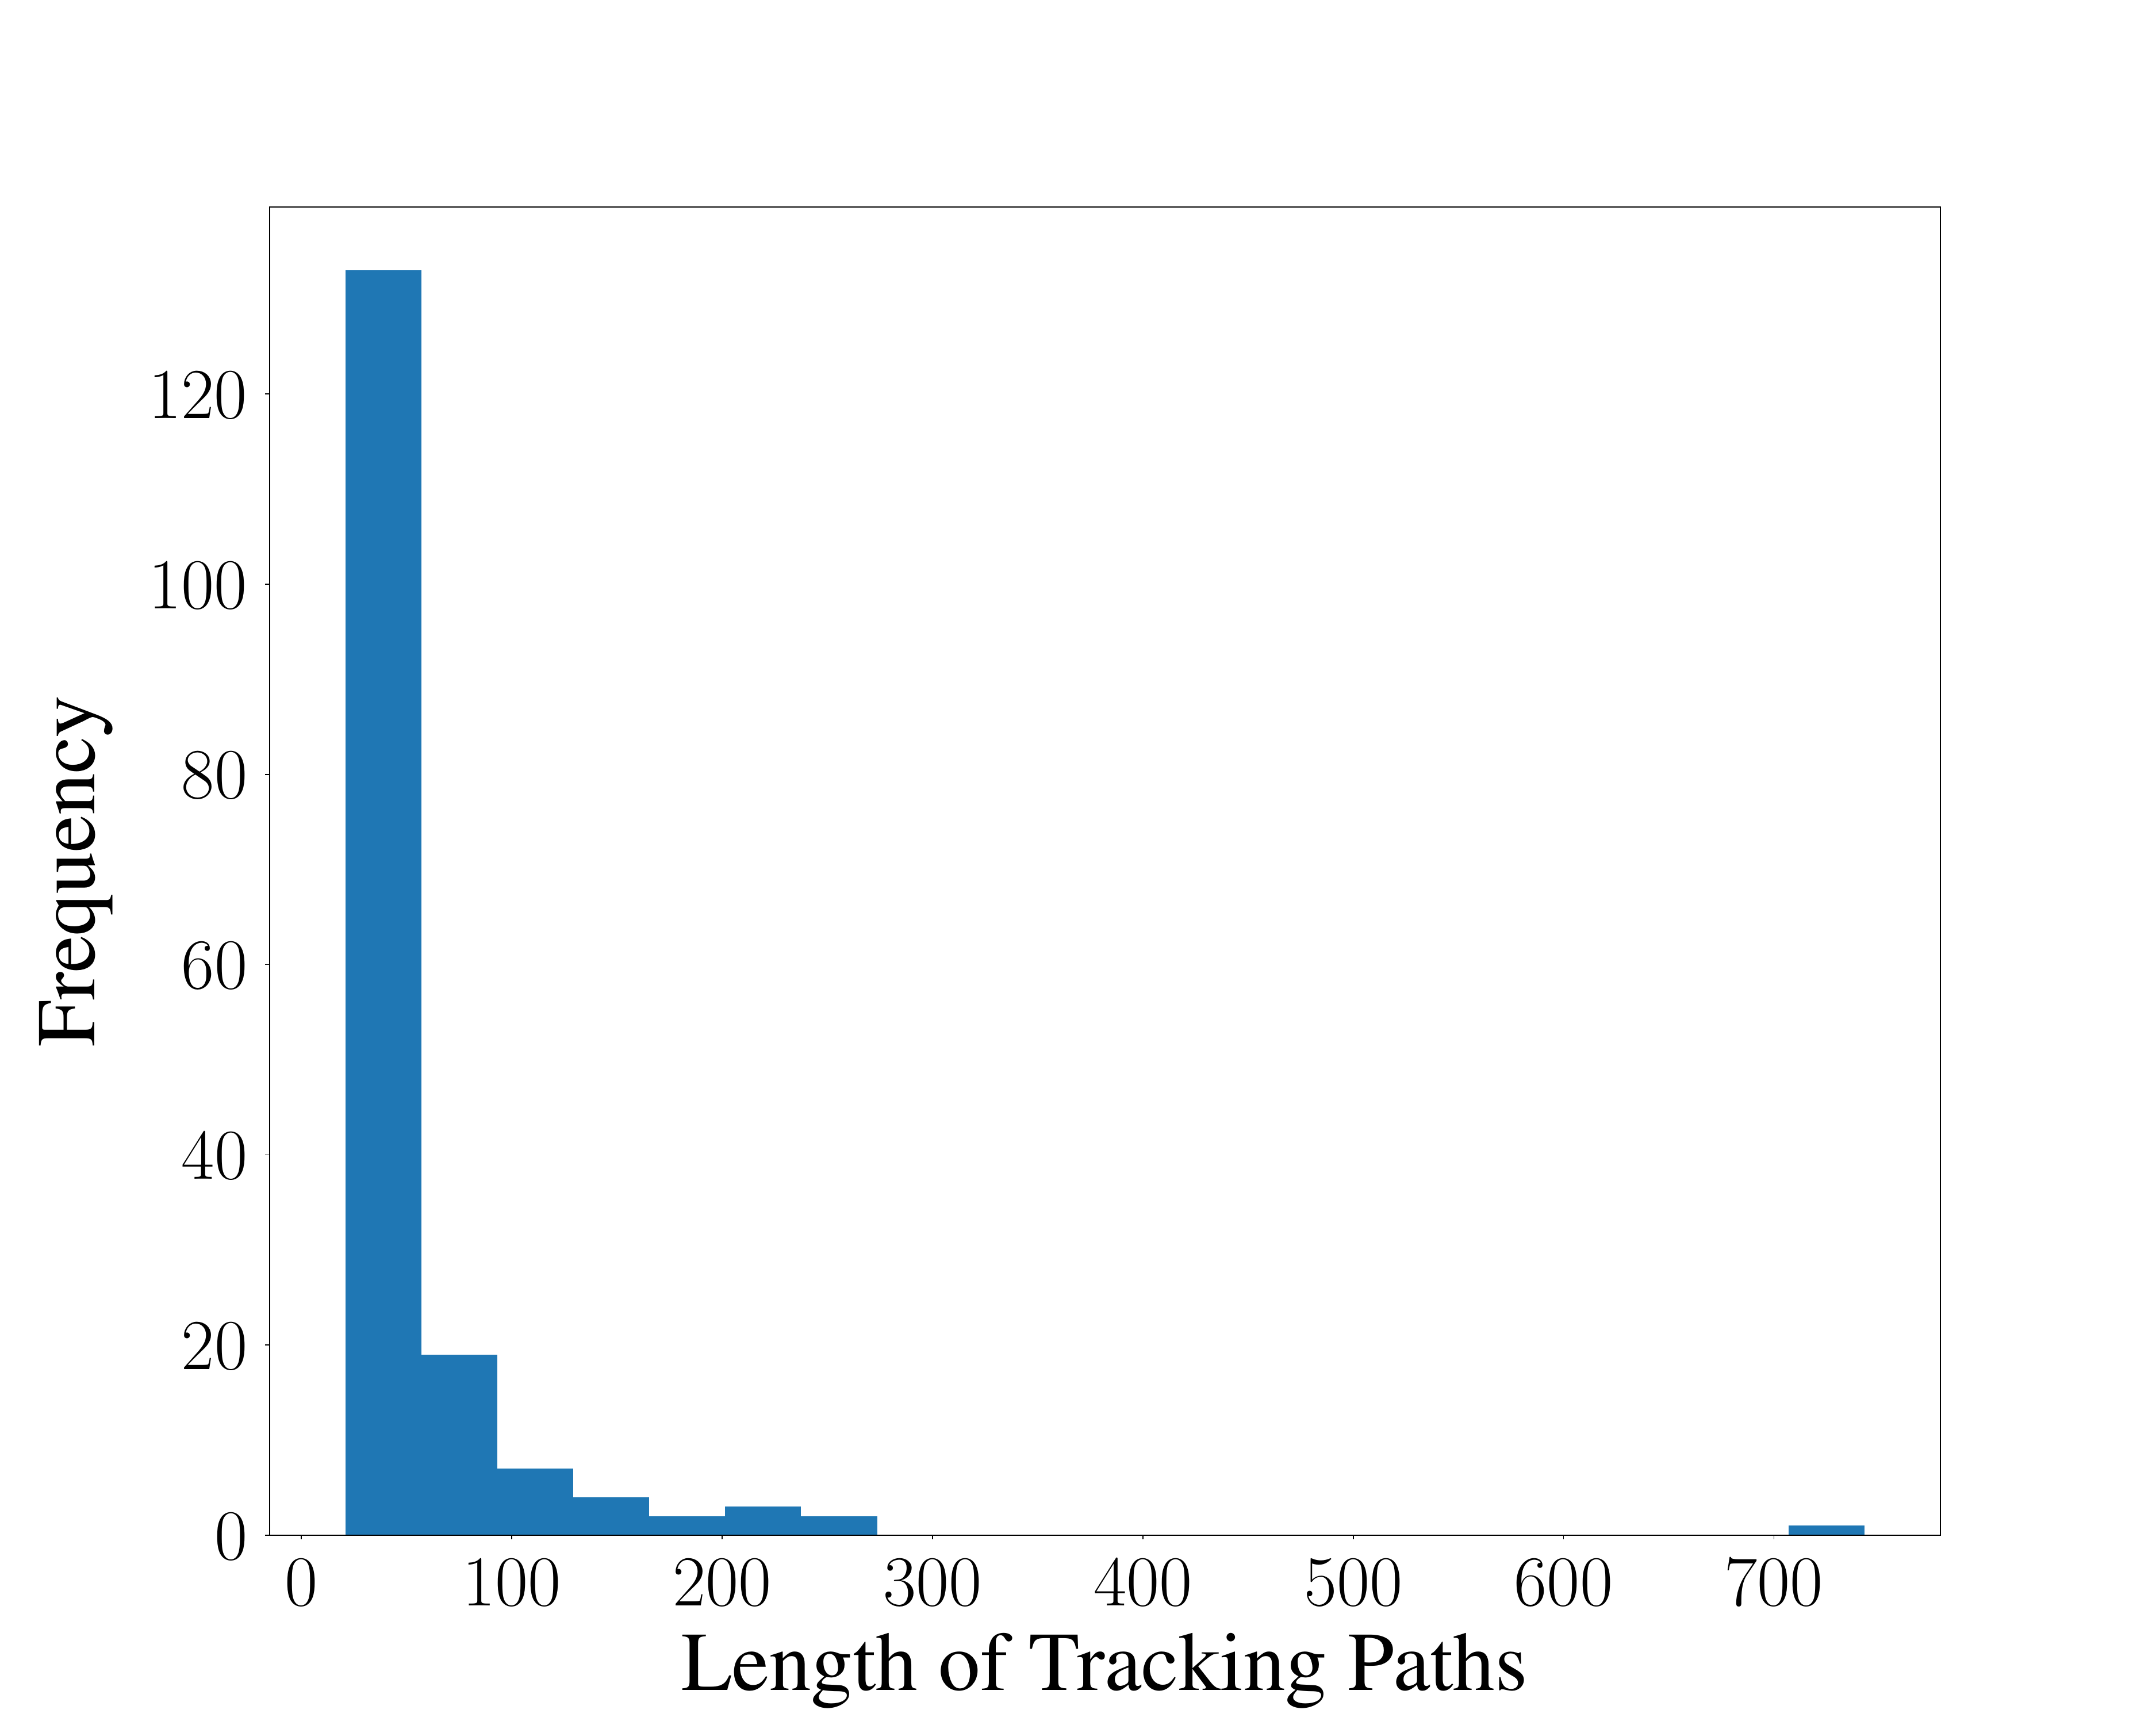}%
\caption{$d_p$.}%
\label{fig-LengthHistogramStorms2DP}%
\end{subfigure}%
\caption{Histograms of the length of the tracking paths 
    of \dataset{Storms2D}.}%
\label{fig-LengthHisgoramStorms2D}%
\end{figure}

\begin{figure}
\centering
\includegraphics[width=0.8\linewidth]{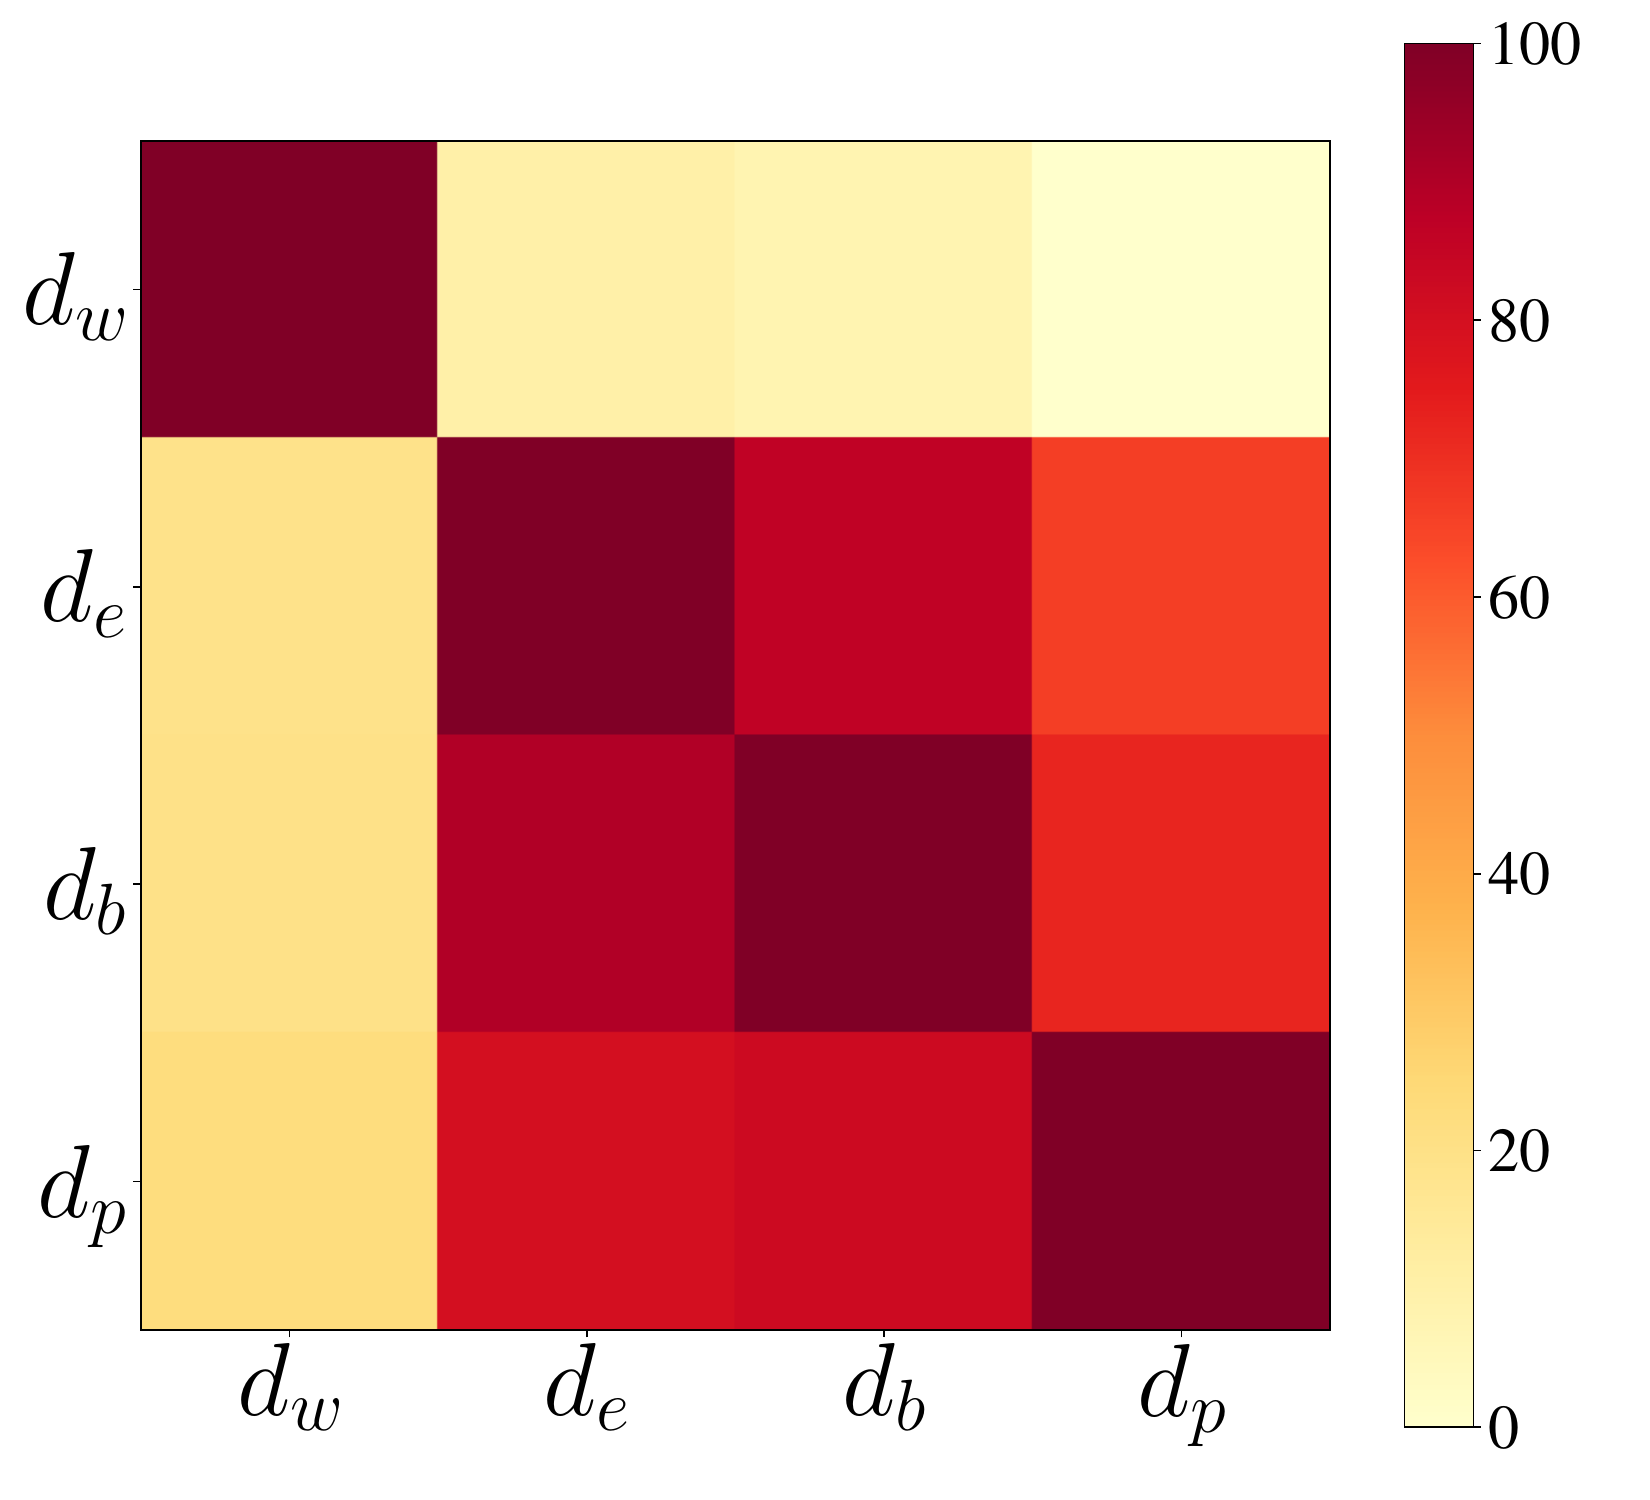}
\caption{
    Pairwise differences between the methods on the columns
    in relation to the methods on the rows
    for \dataset{Storms2D}.
}
\label{fig-Storms2DSimilarities}
\end{figure}

\subsection*{Results using Boussinesq2D}
The results of the experiments using \dataset{Boussinesq2D}
are shown from \Cref{fig-Boussinesq2DAllNodes}
to \Cref{fig-Boussinesq2DSimilarities}.

\begin{figure}
\centering
\includegraphics[width=0.8\linewidth]{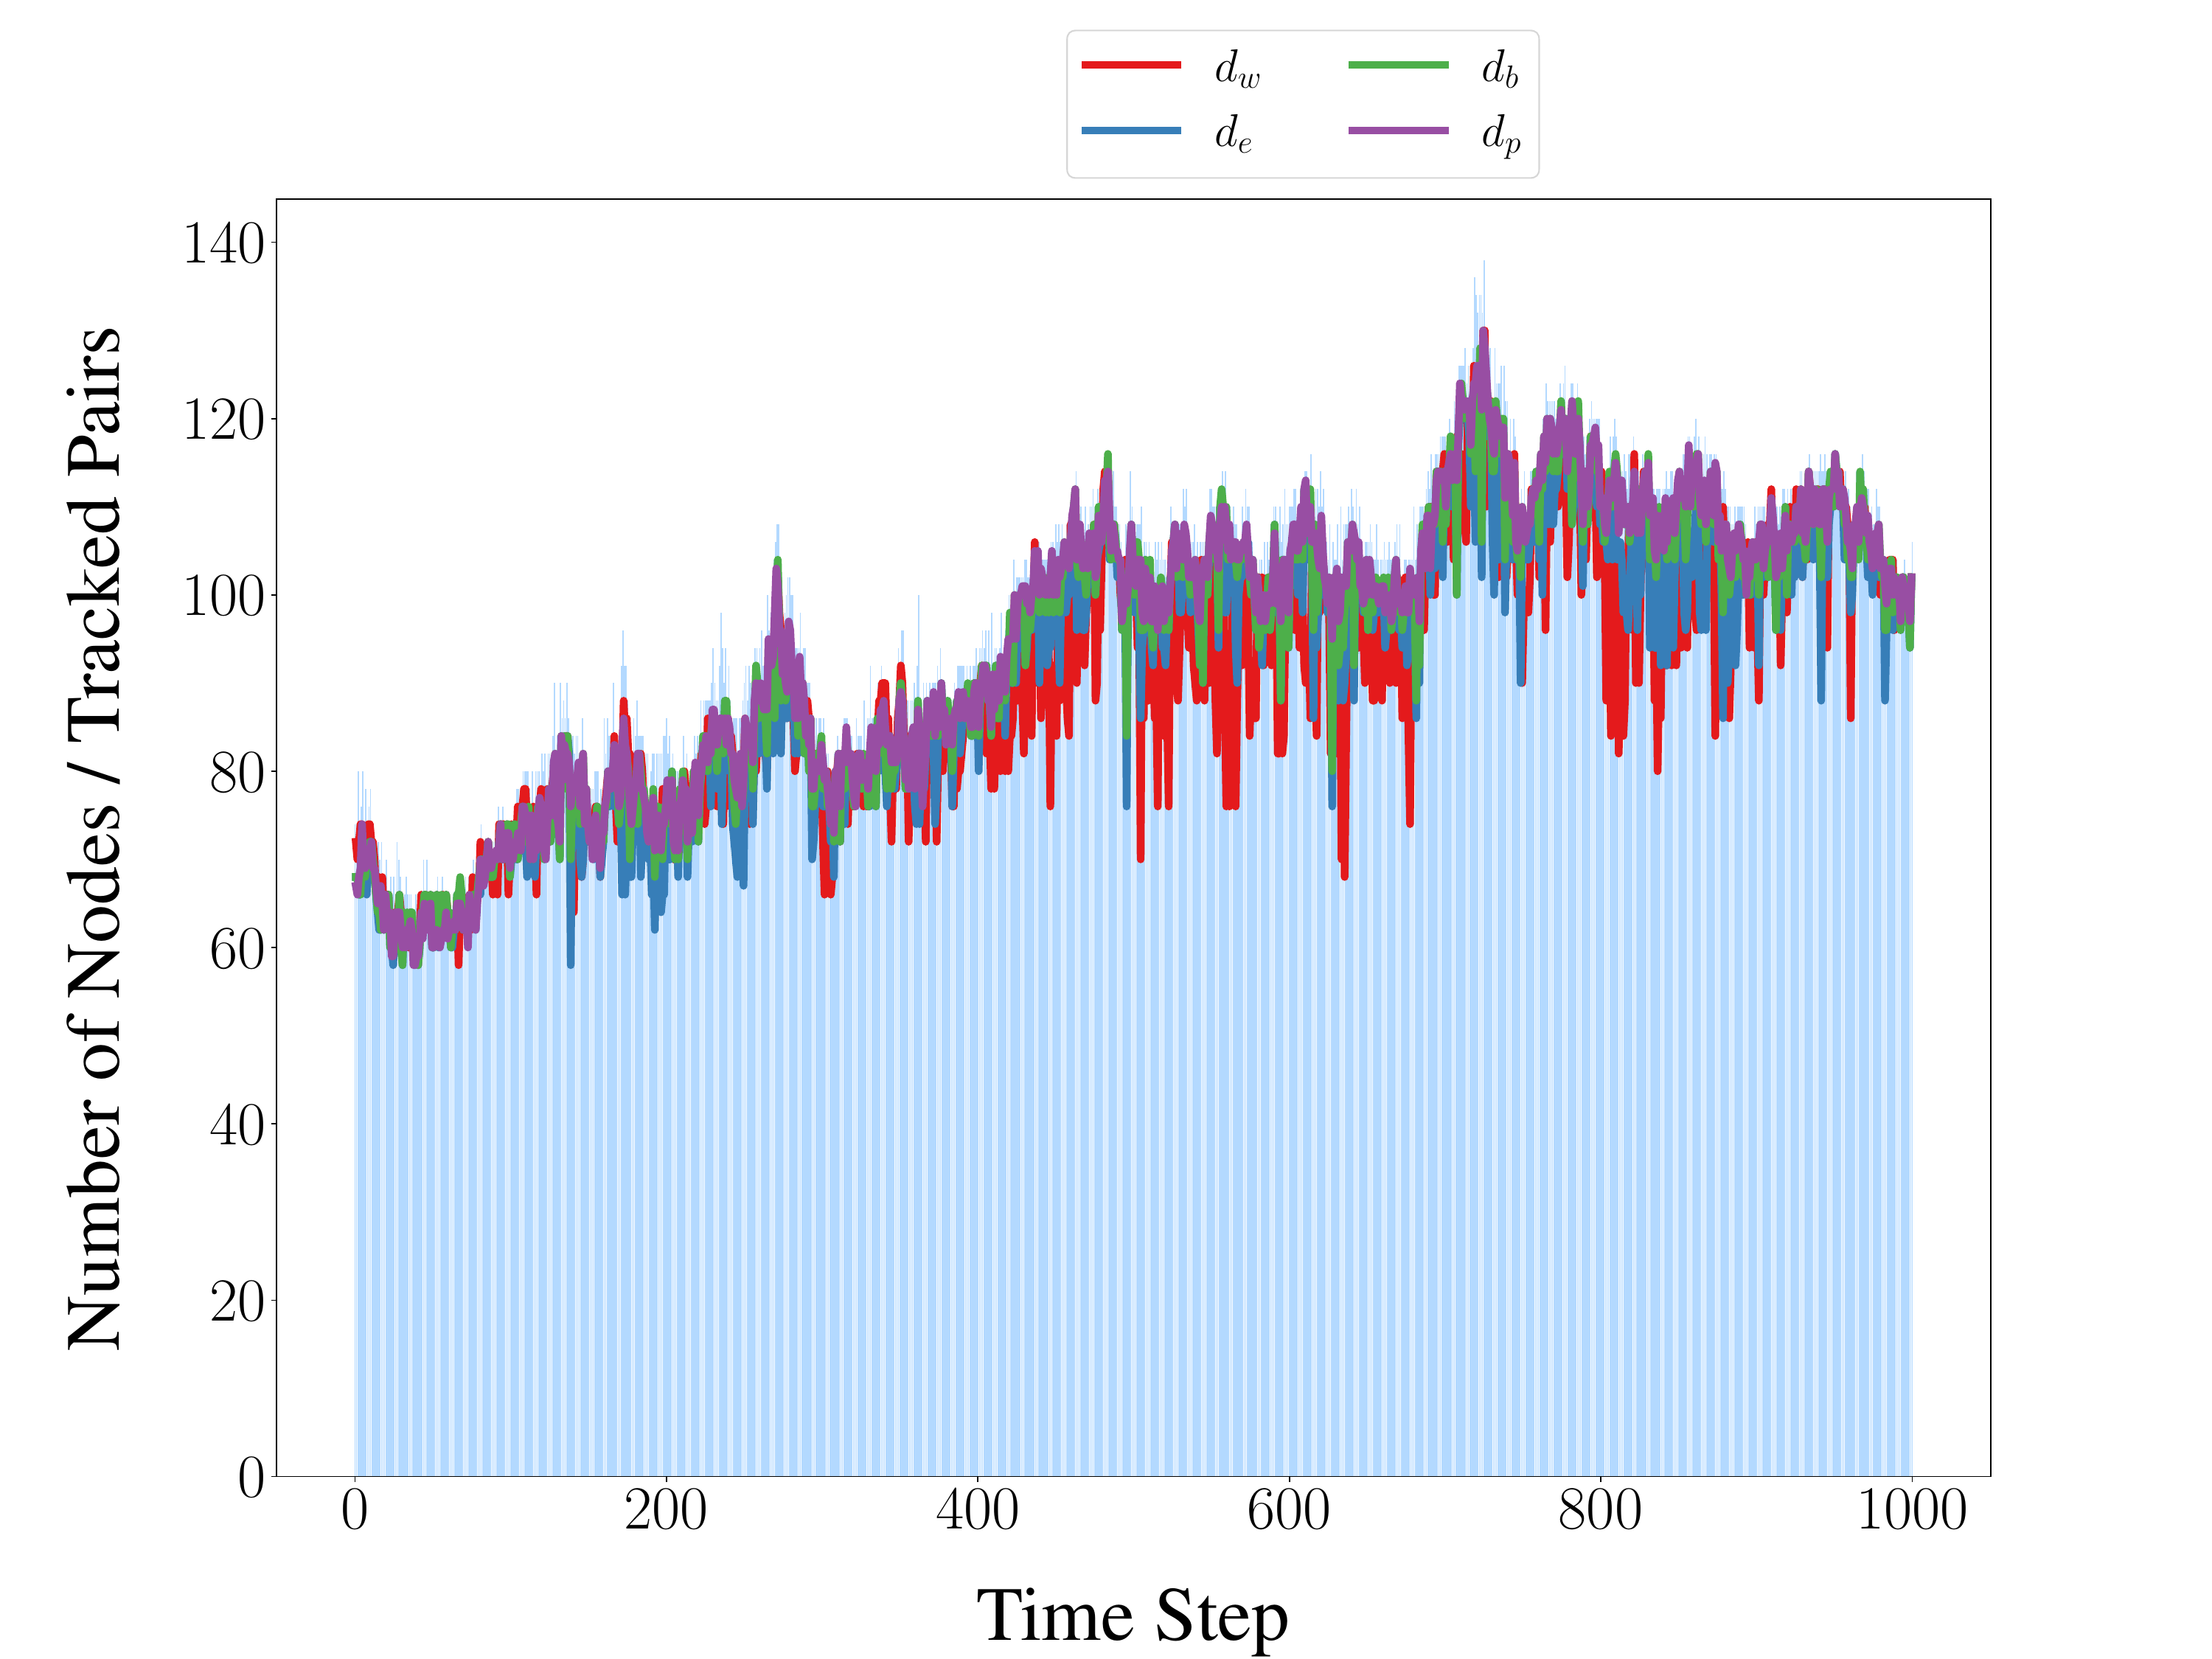}
\caption{
    Number of tracked nodes (colored and labeled) 
    relative to the total nodes of merge trees (light blue bars)
    for \dataset{Boussinesq2D}.
}
\label{fig-Boussinesq2DAllNodes}
\end{figure}

\begin{figure}
\centering
\includegraphics[width=0.8\linewidth]{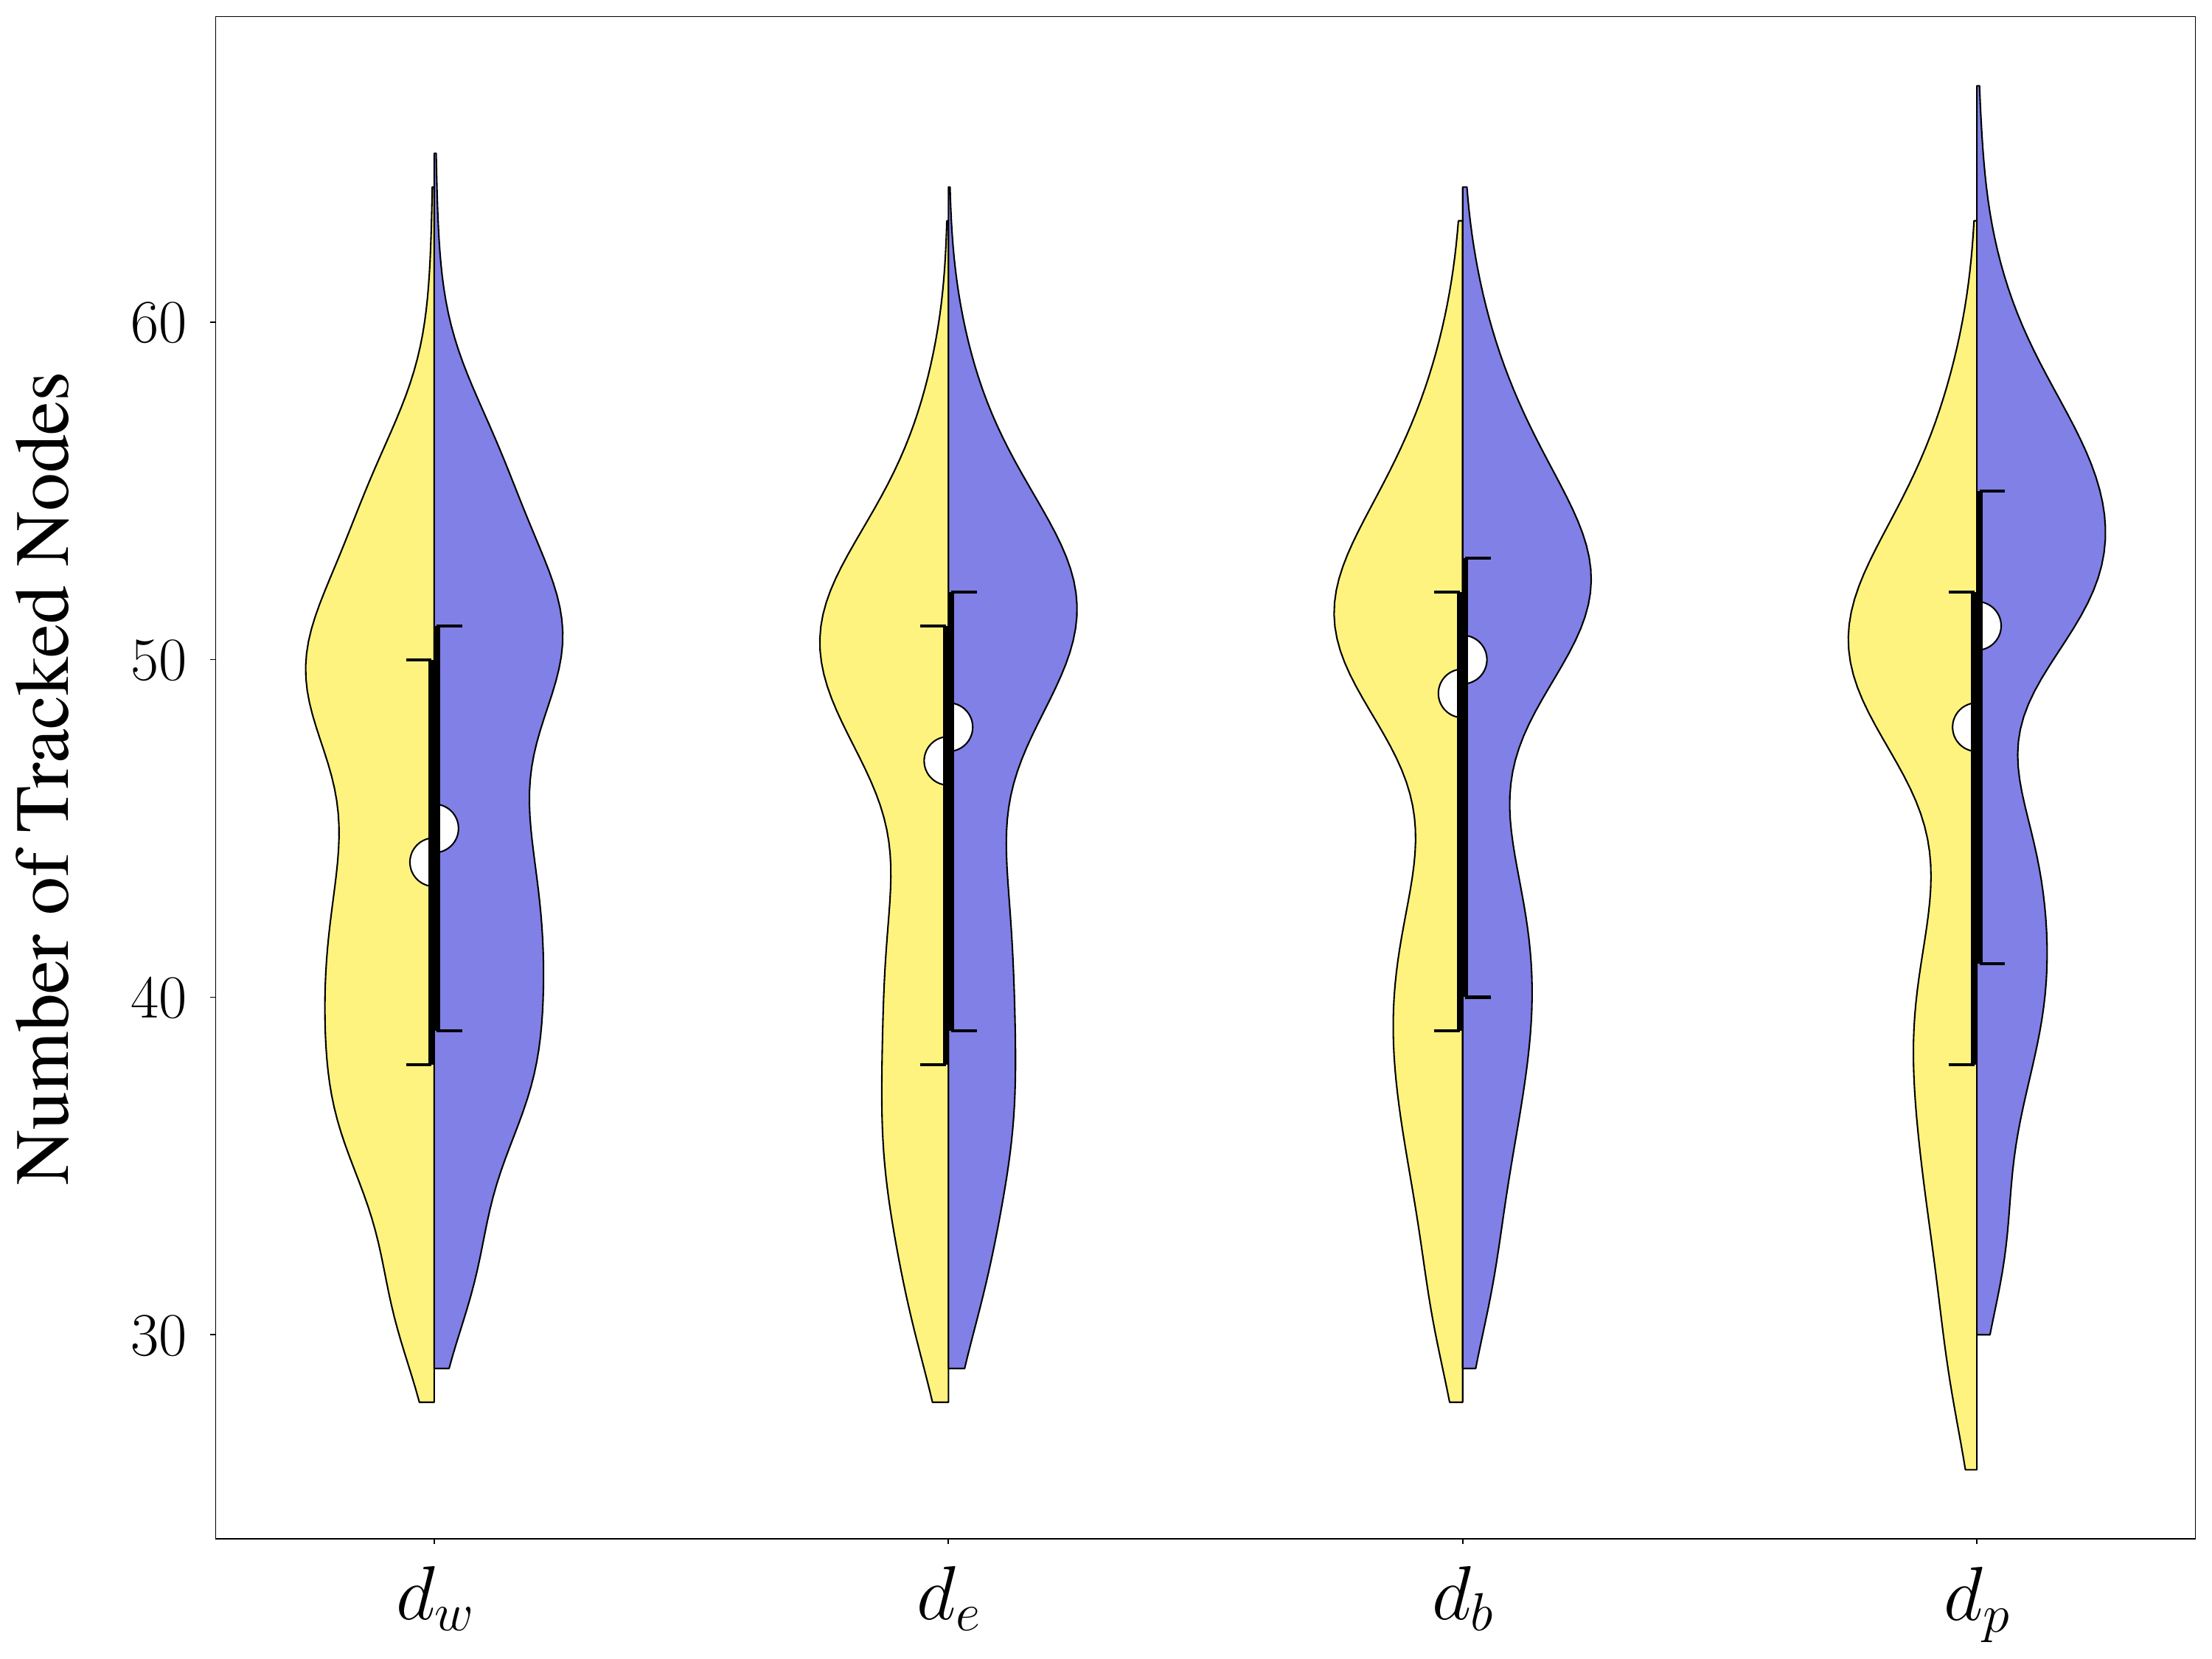}
\caption{
    Distributions of tracked nodes 
    over the chosen time steps of \dataset{Boussinesq2D},  
    divided by types:
    saddle (yellow) and minima (blue).
}
\label{fig-Boussinesq2DViolin}
\end{figure}

% Length histogram
\begin{figure}%
\begin{subfigure}[t]{\ltwopicwidth}%
\includegraphics[width=\ltwopicwidth]{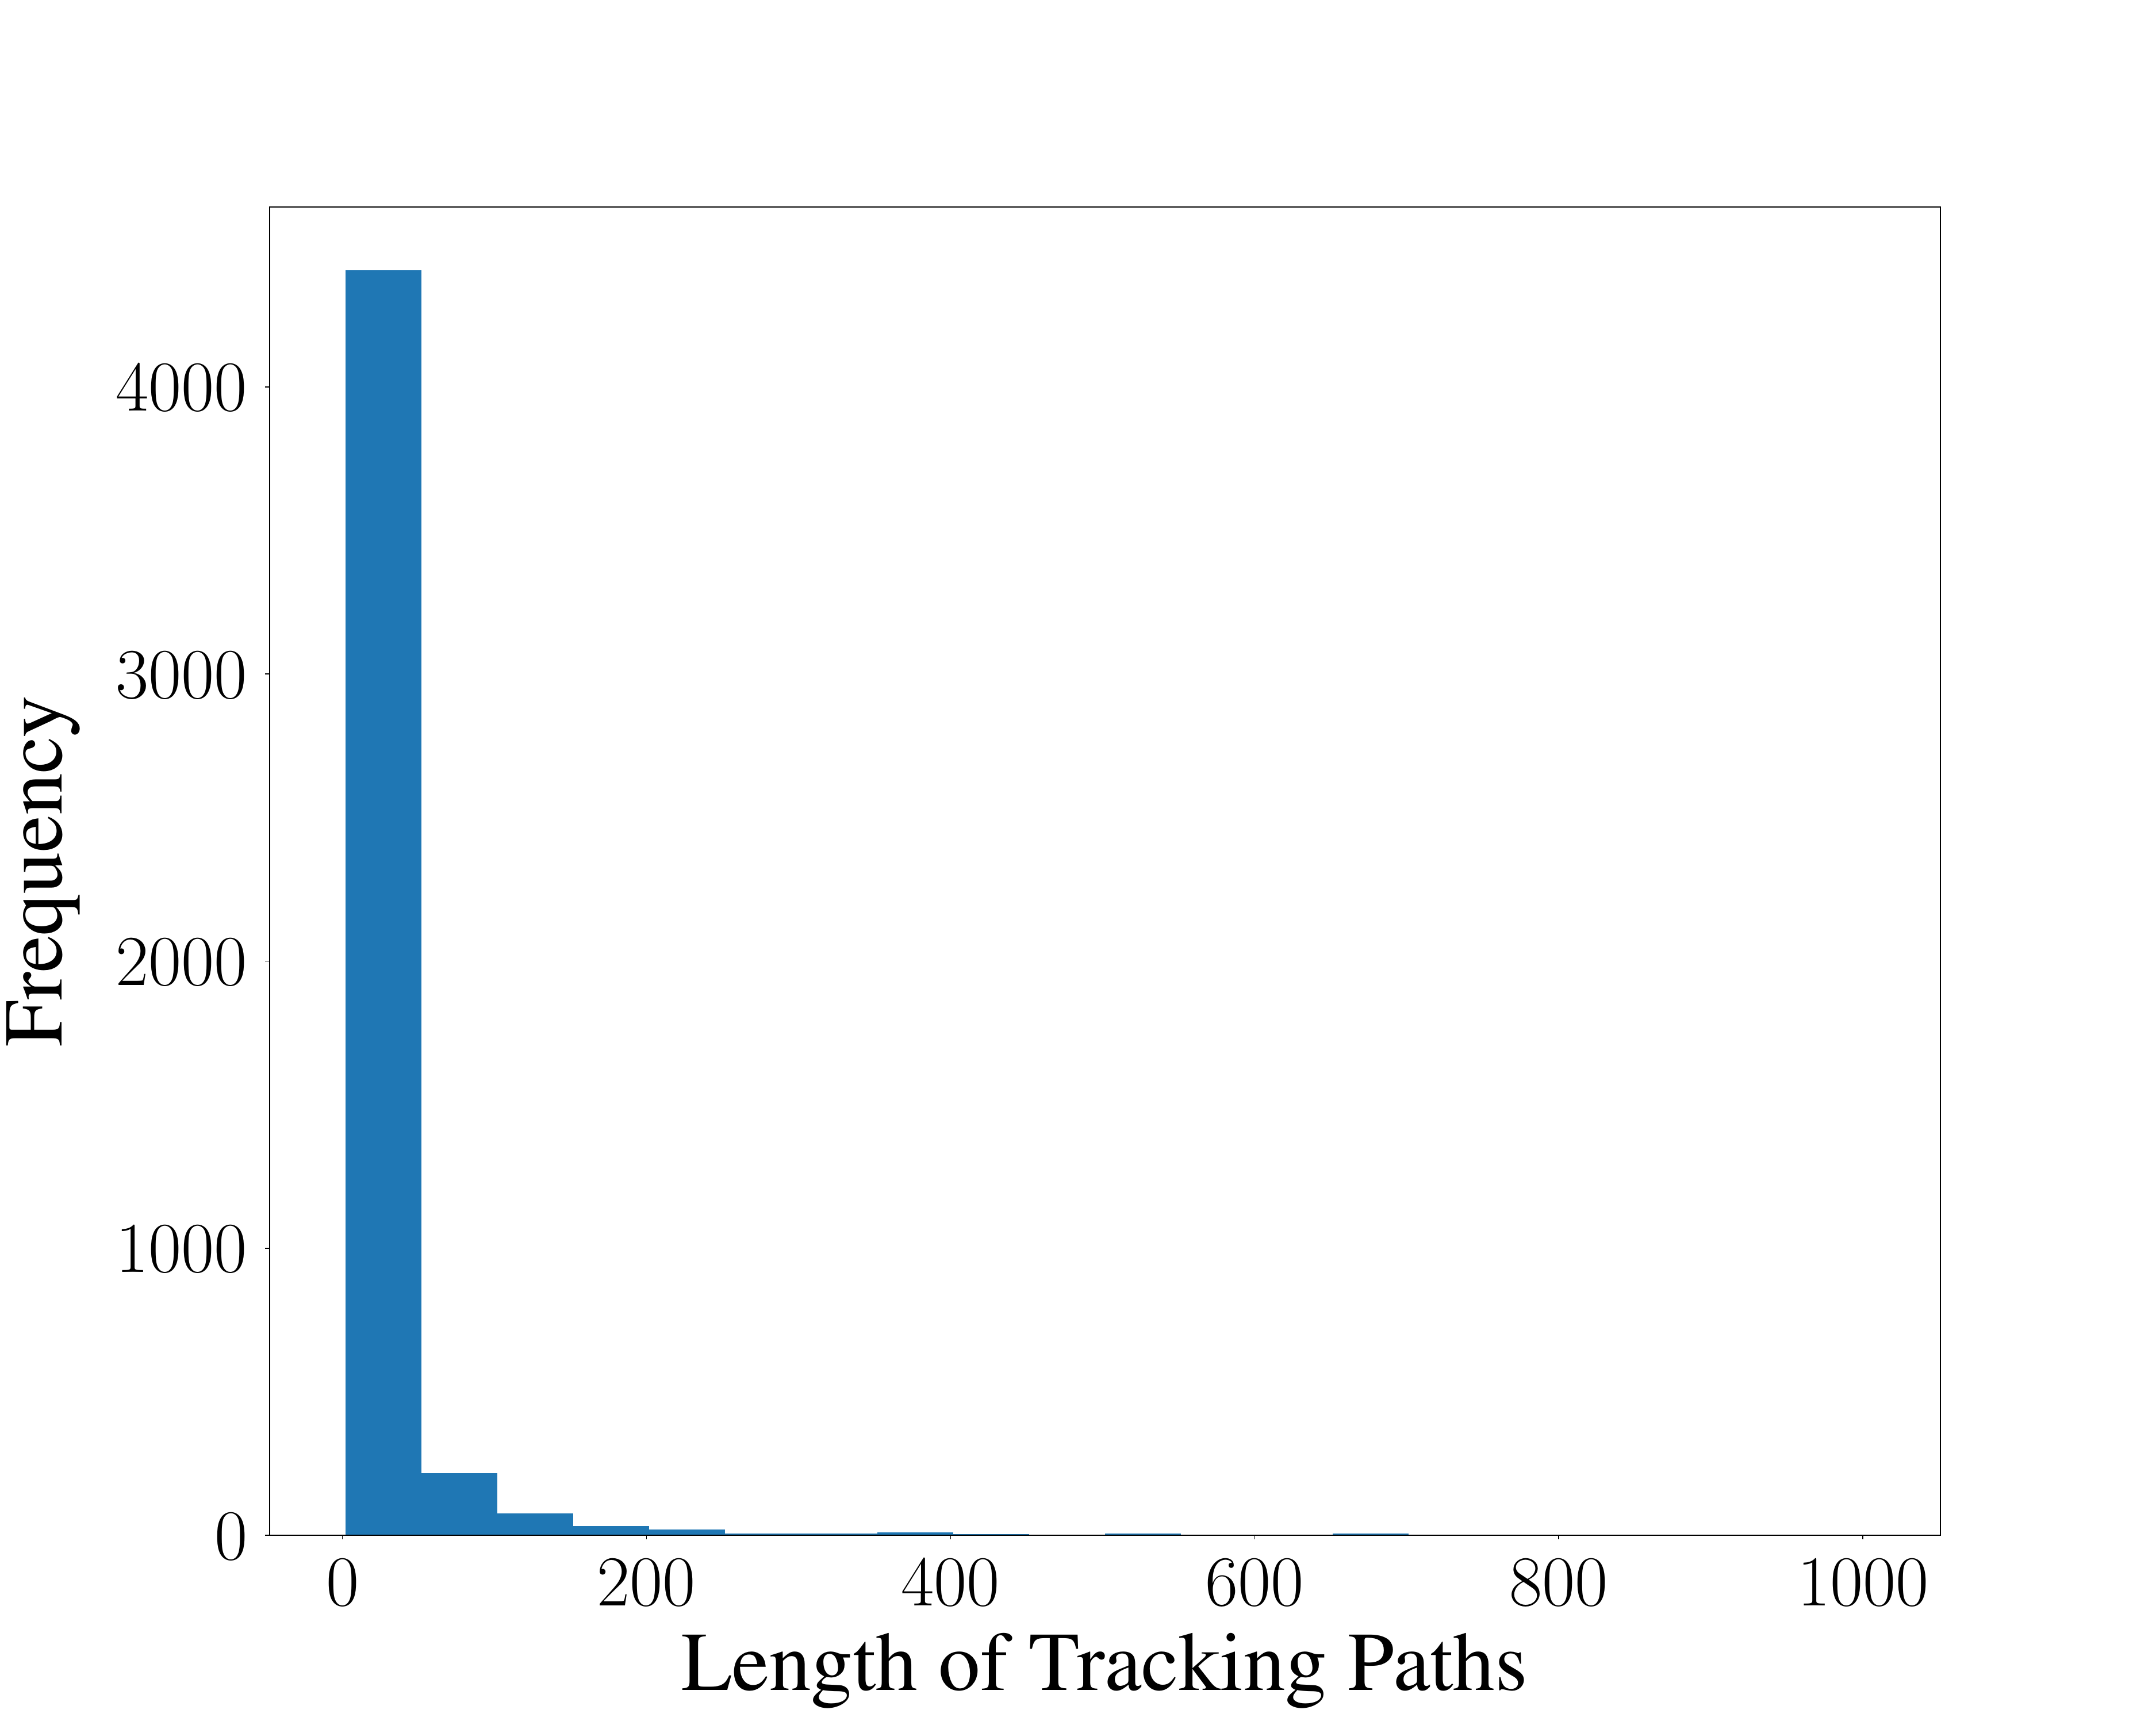}
\caption{$d_w$.}%
\label{fig-LengthHistogramBoussinesq2DW}%
\end{subfigure}
\hfill%
\begin{subfigure}[t]{\ltwopicwidth}%
\includegraphics[width=\ltwopicwidth]{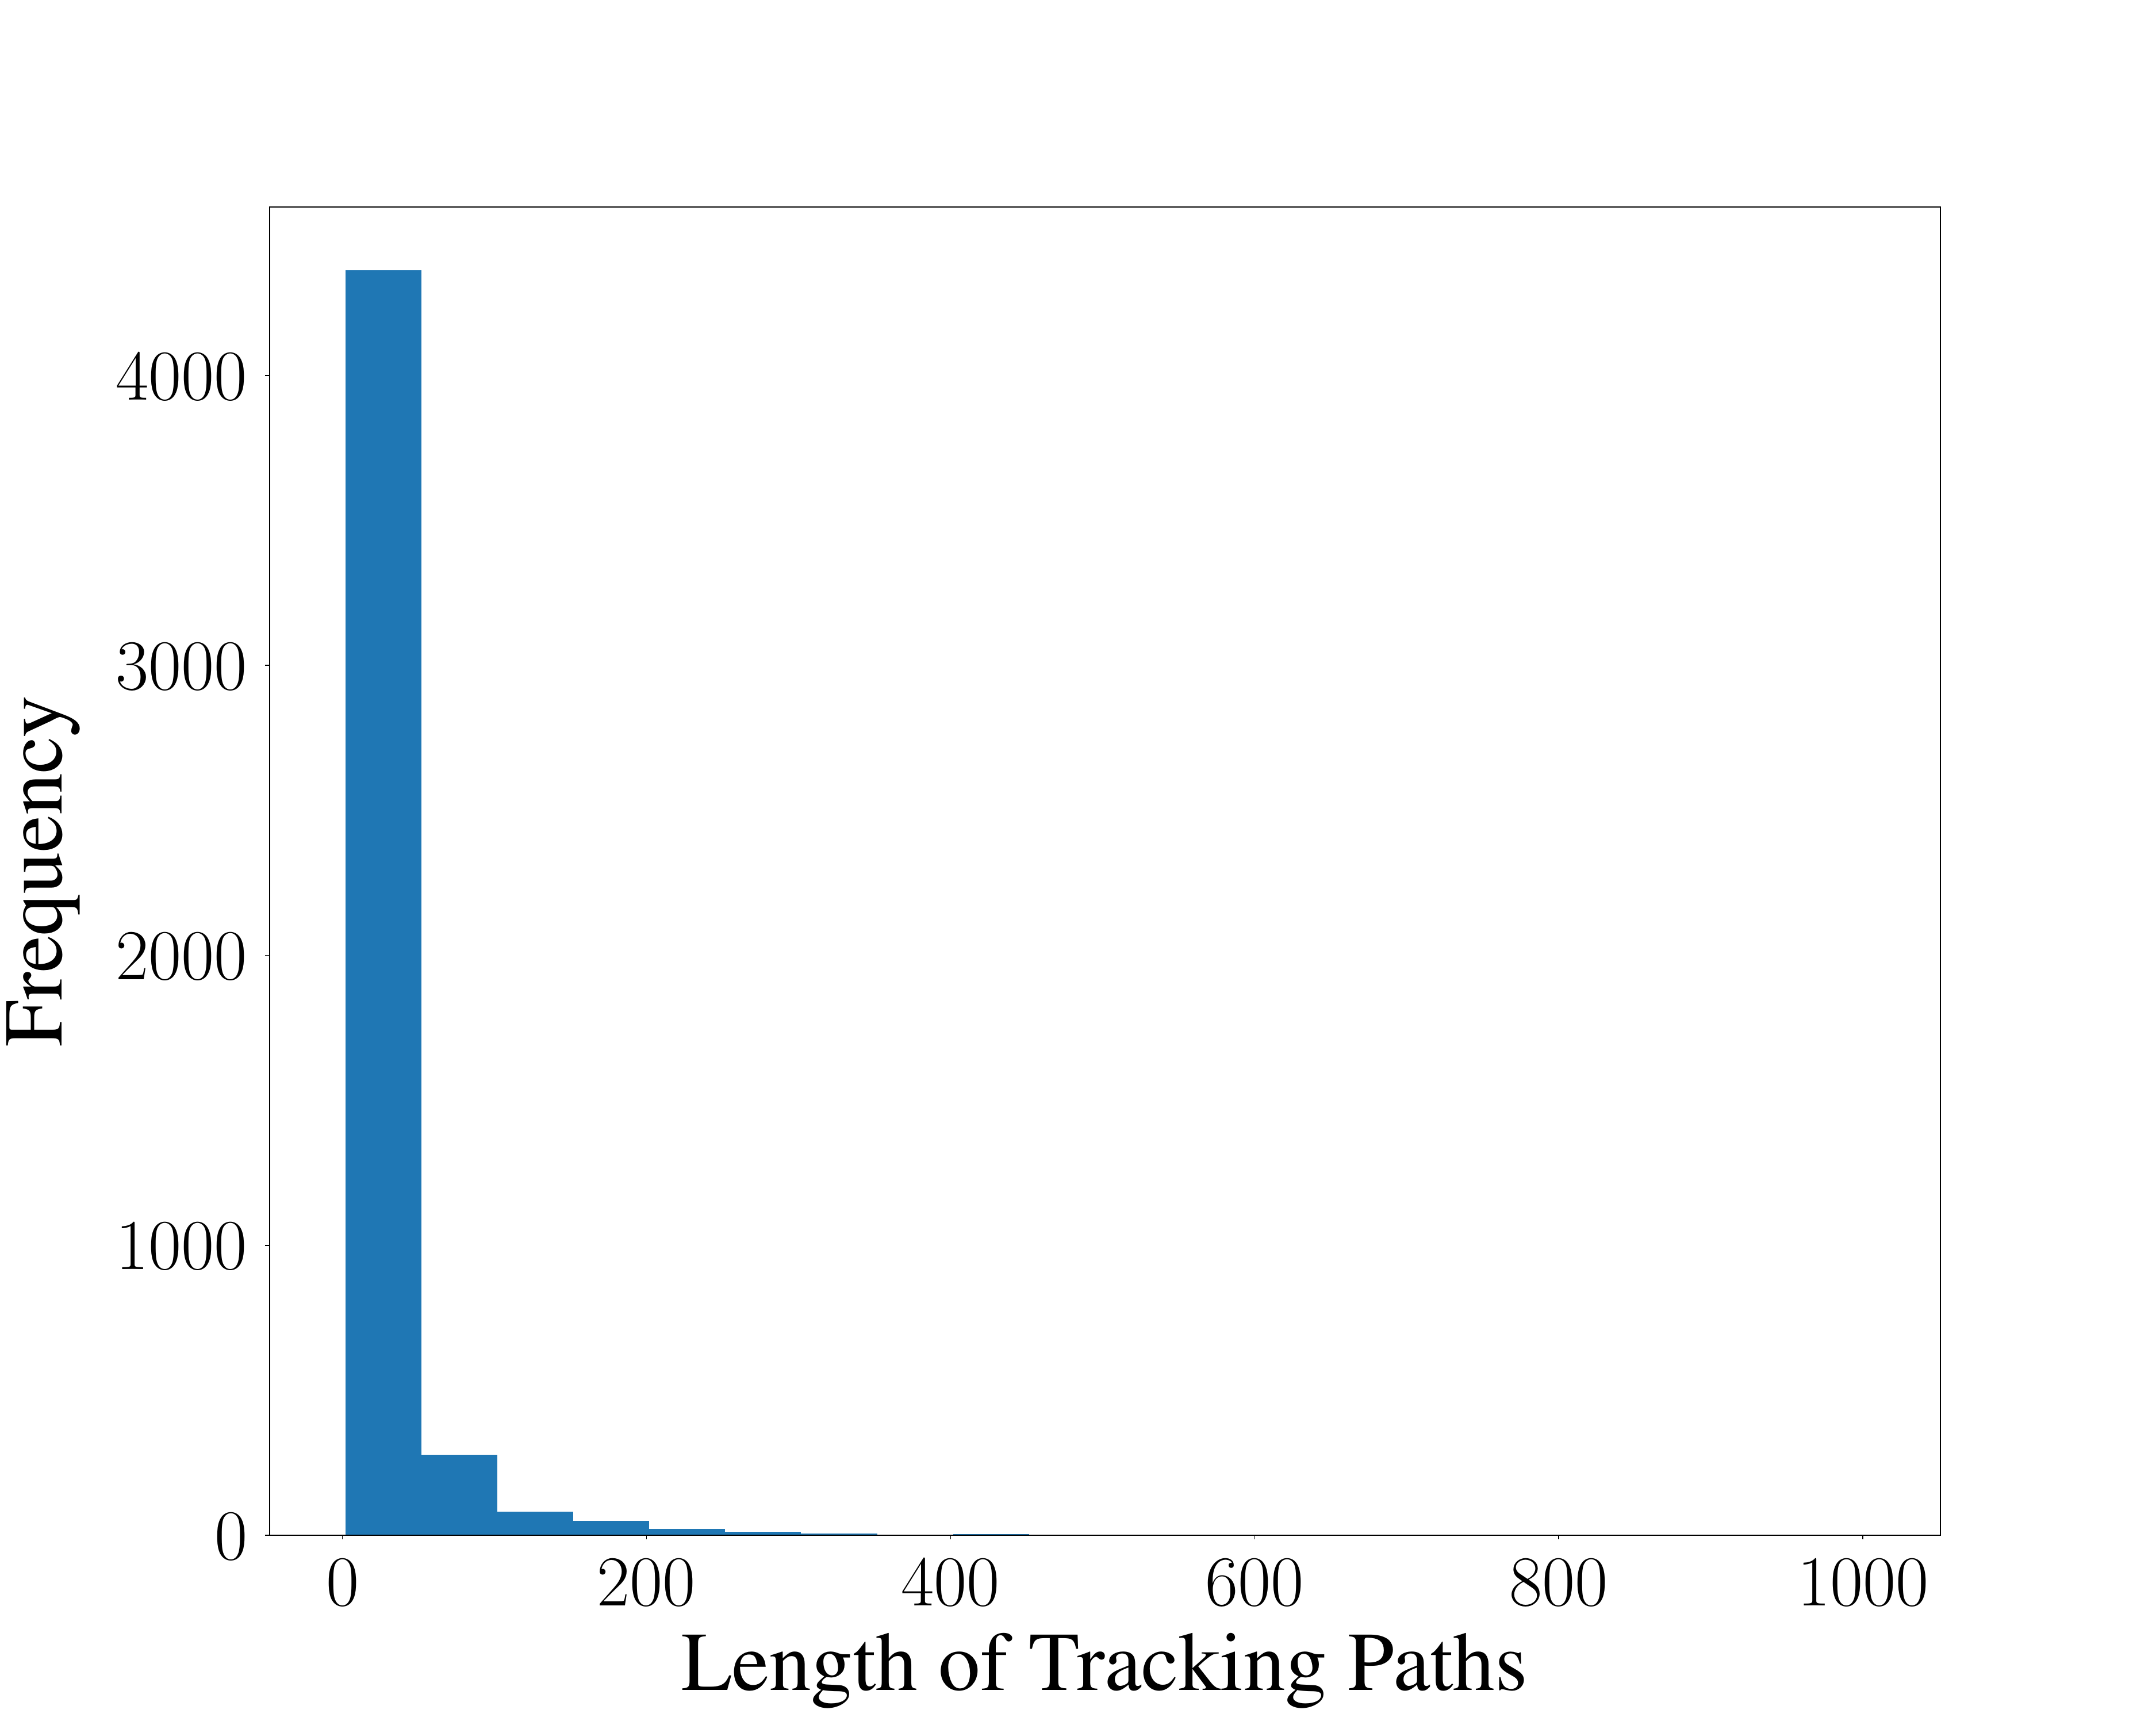}%
\caption{$d_e$.}%
\label{fig-LengthHistogramBoussinesq2DE}%
\end{subfigure}%
\\%
\begin{subfigure}[t]{\ltwopicwidth}%
\includegraphics[width=\ltwopicwidth]{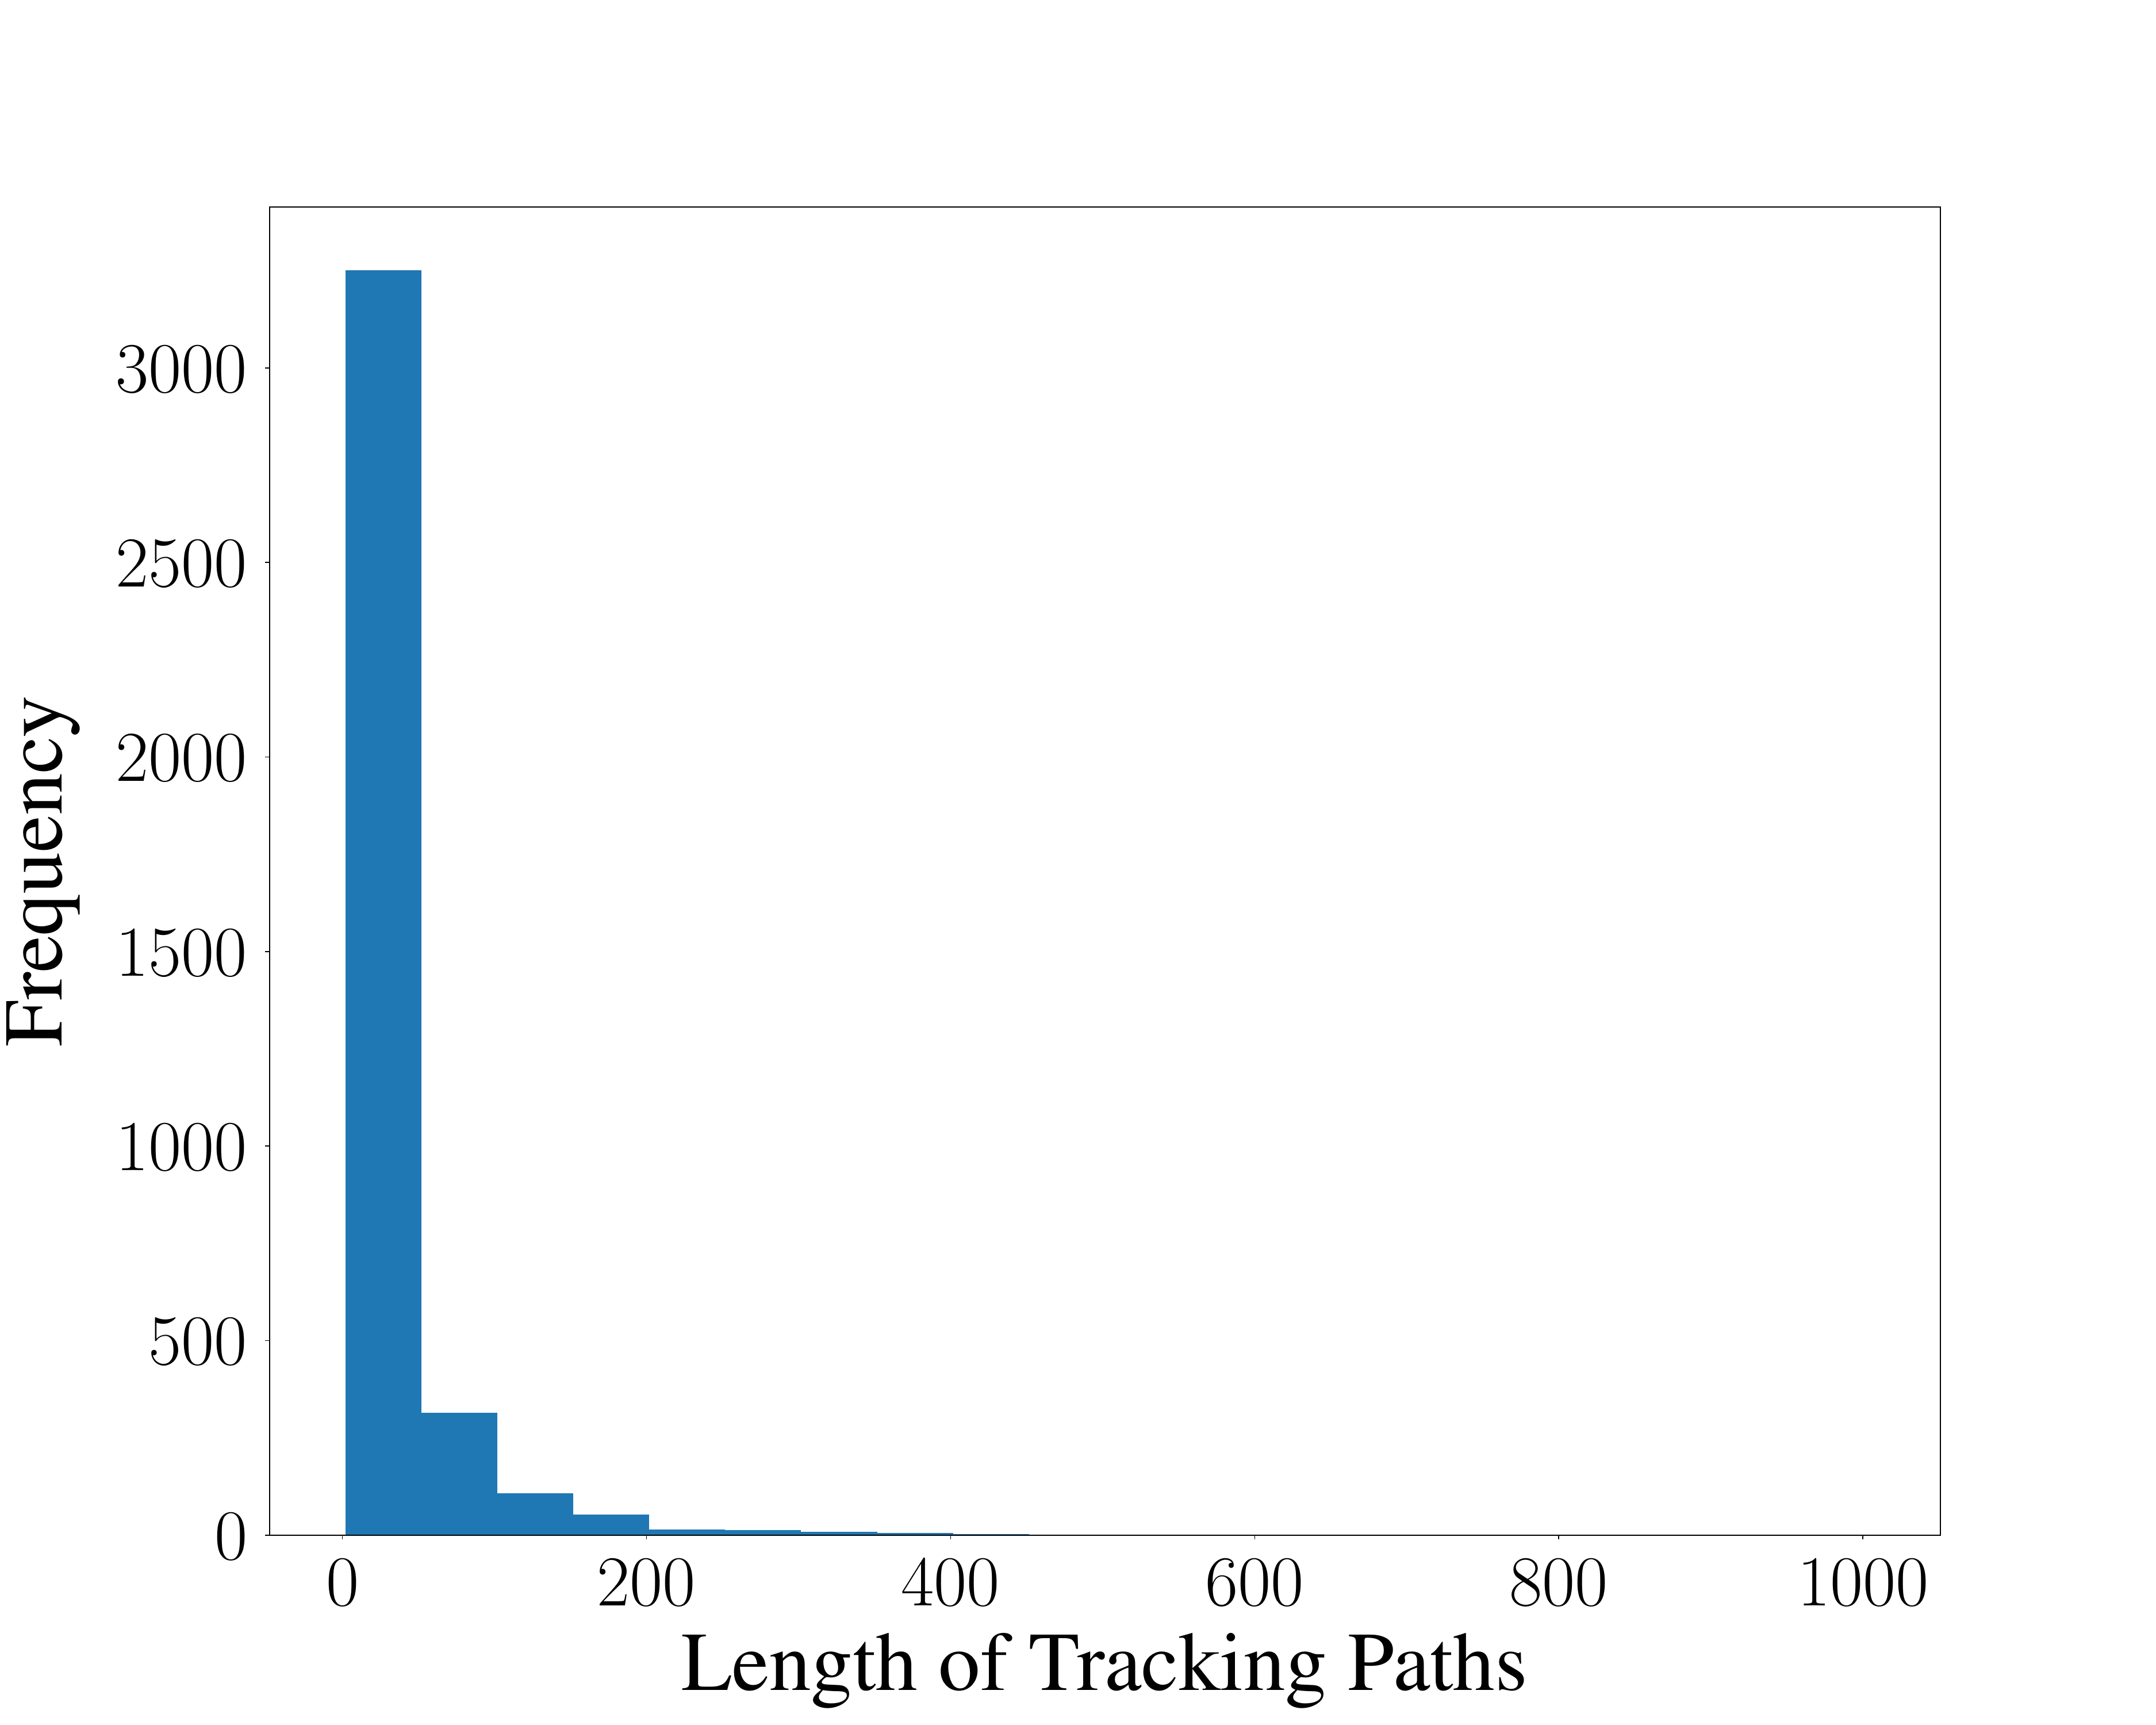}%
\caption{$d_b$.}%
\label{fig-LengthHistogramBoussinesq2DB}%
\end{subfigure}%
\hfill%
\begin{subfigure}[t]{\ltwopicwidth}%
\includegraphics[width=\ltwopicwidth]{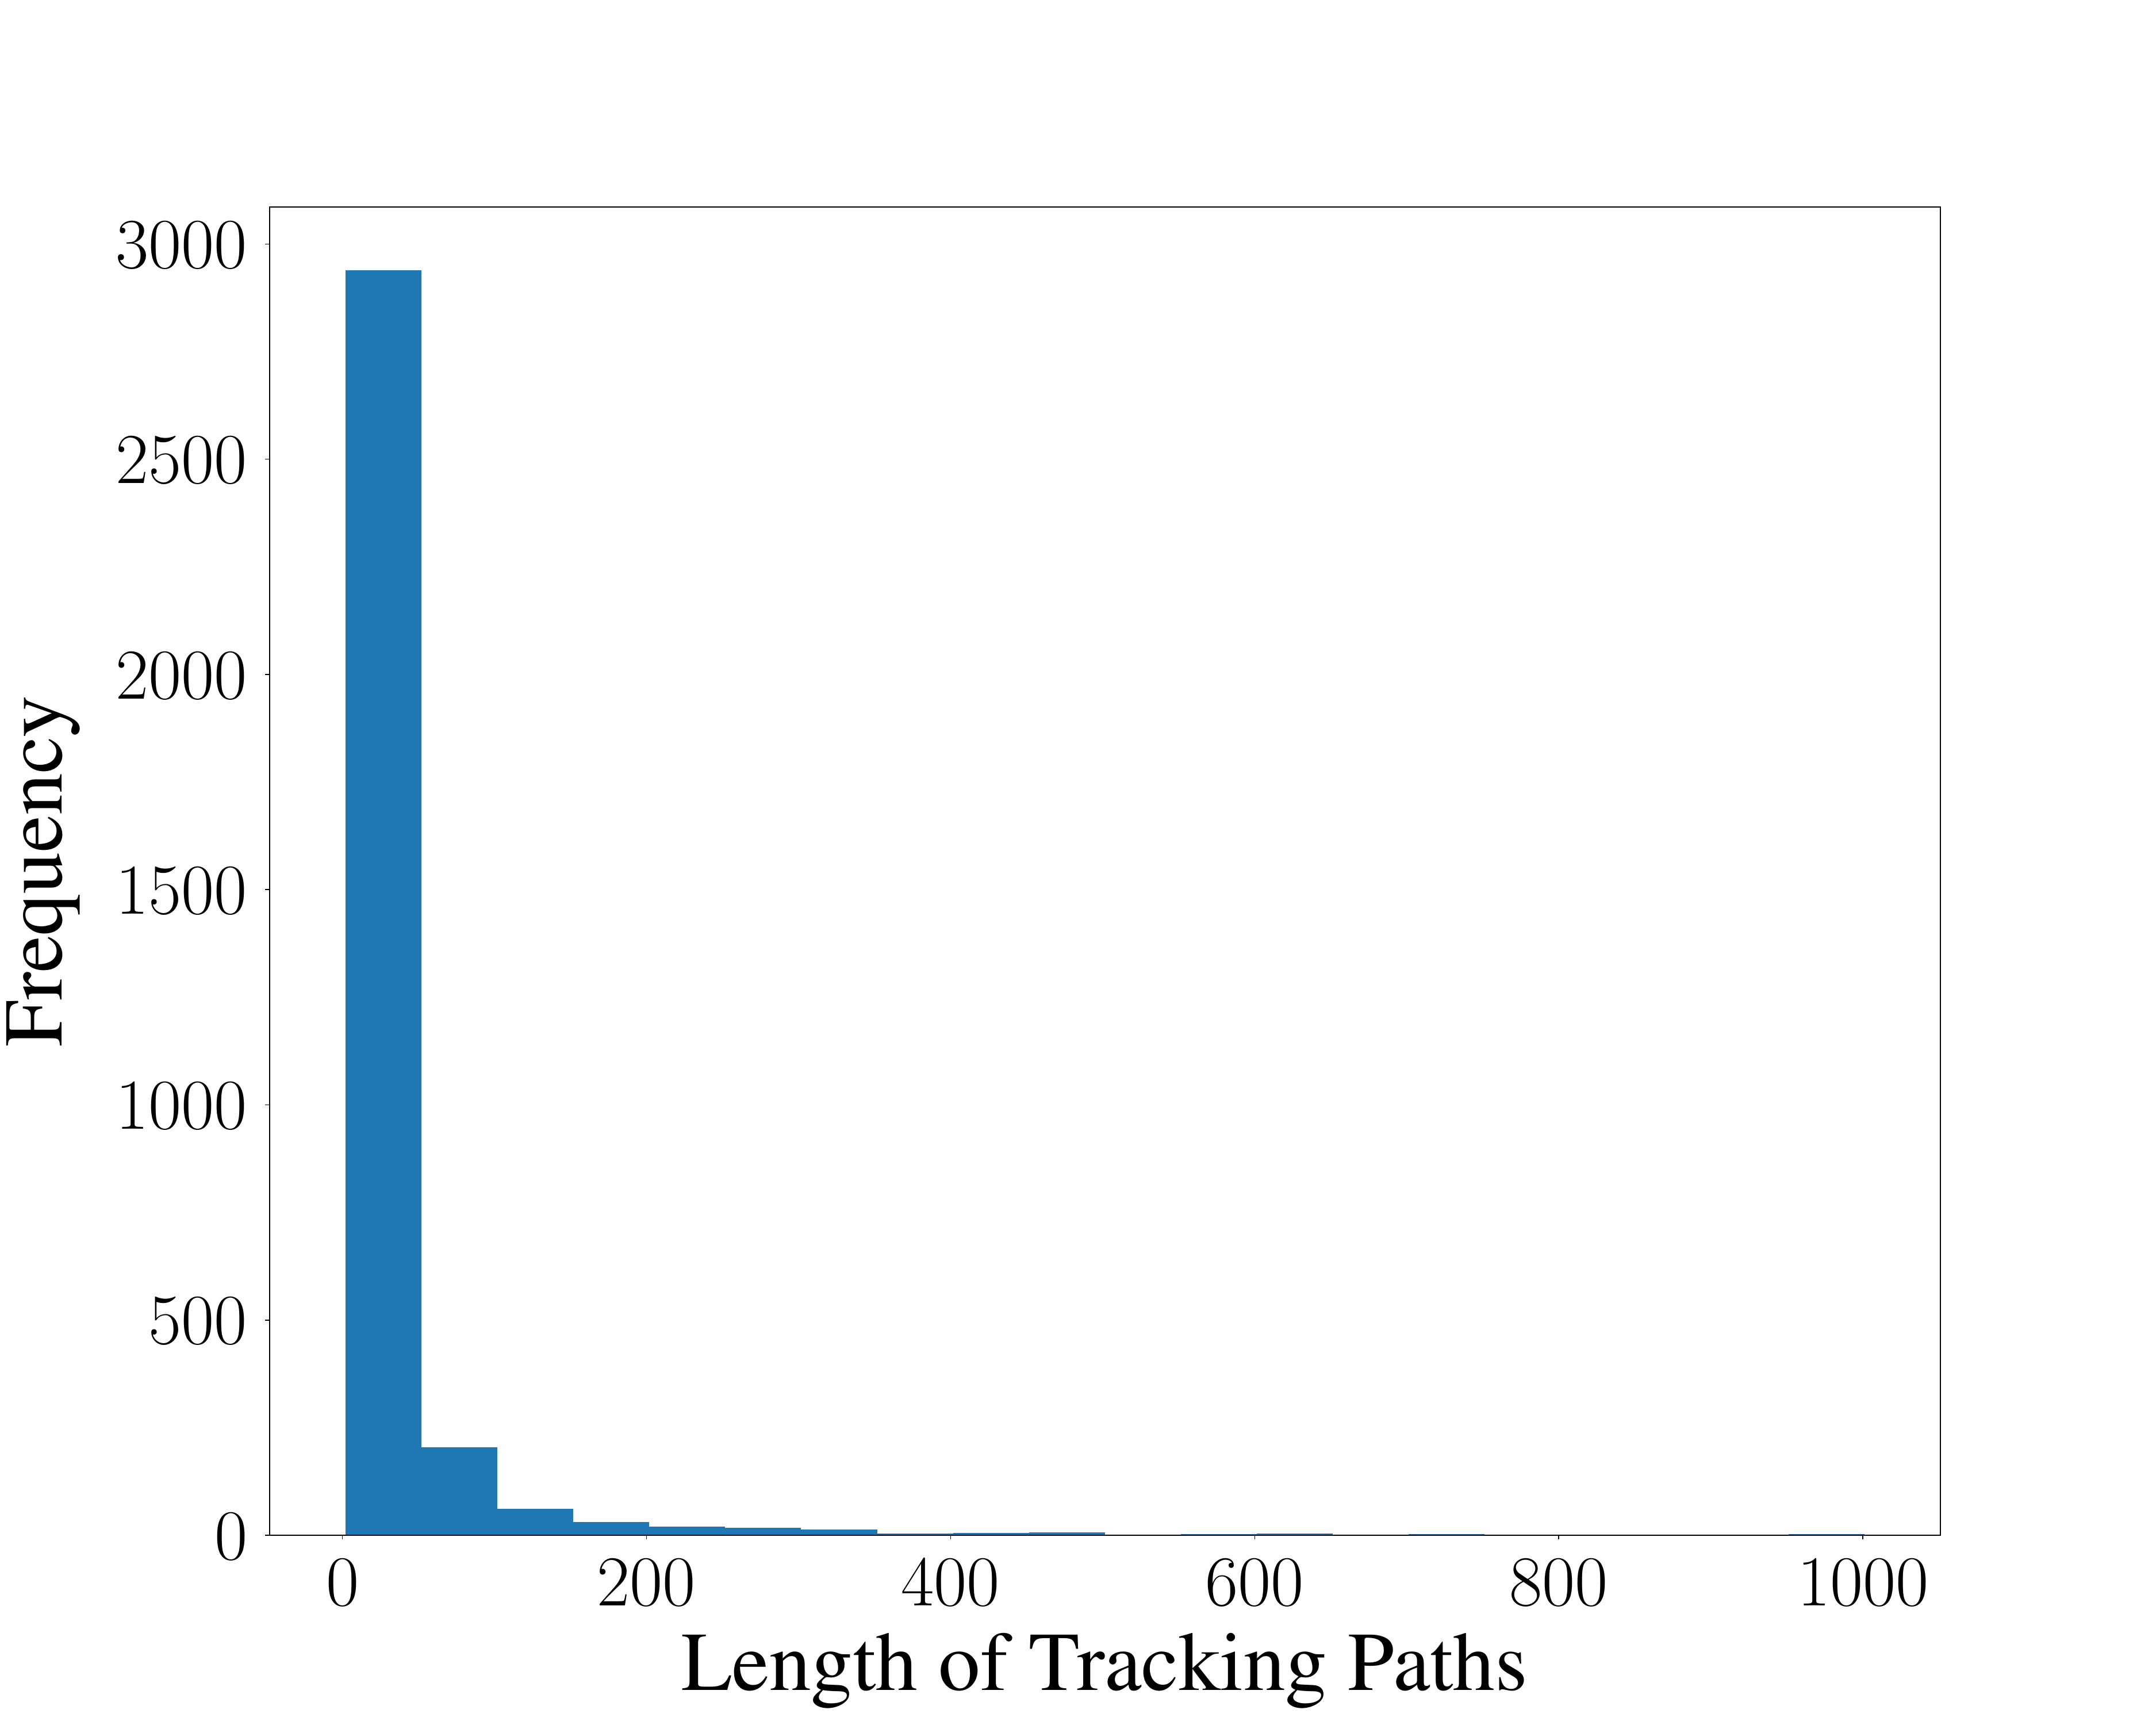}%
\caption{$d_p$.}%
\label{fig-LengthHistogramBoussinesq2DP}%
\end{subfigure}%
\caption{Histograms of the length of the tracking paths 
    using the last $1000$ time steps
    of \dataset{Boussinesq2D}.}%
\label{fig-LengthHisgoramBoussinesq2D}%
\end{figure}

\begin{figure}
\centering
\includegraphics[width=0.8\linewidth]{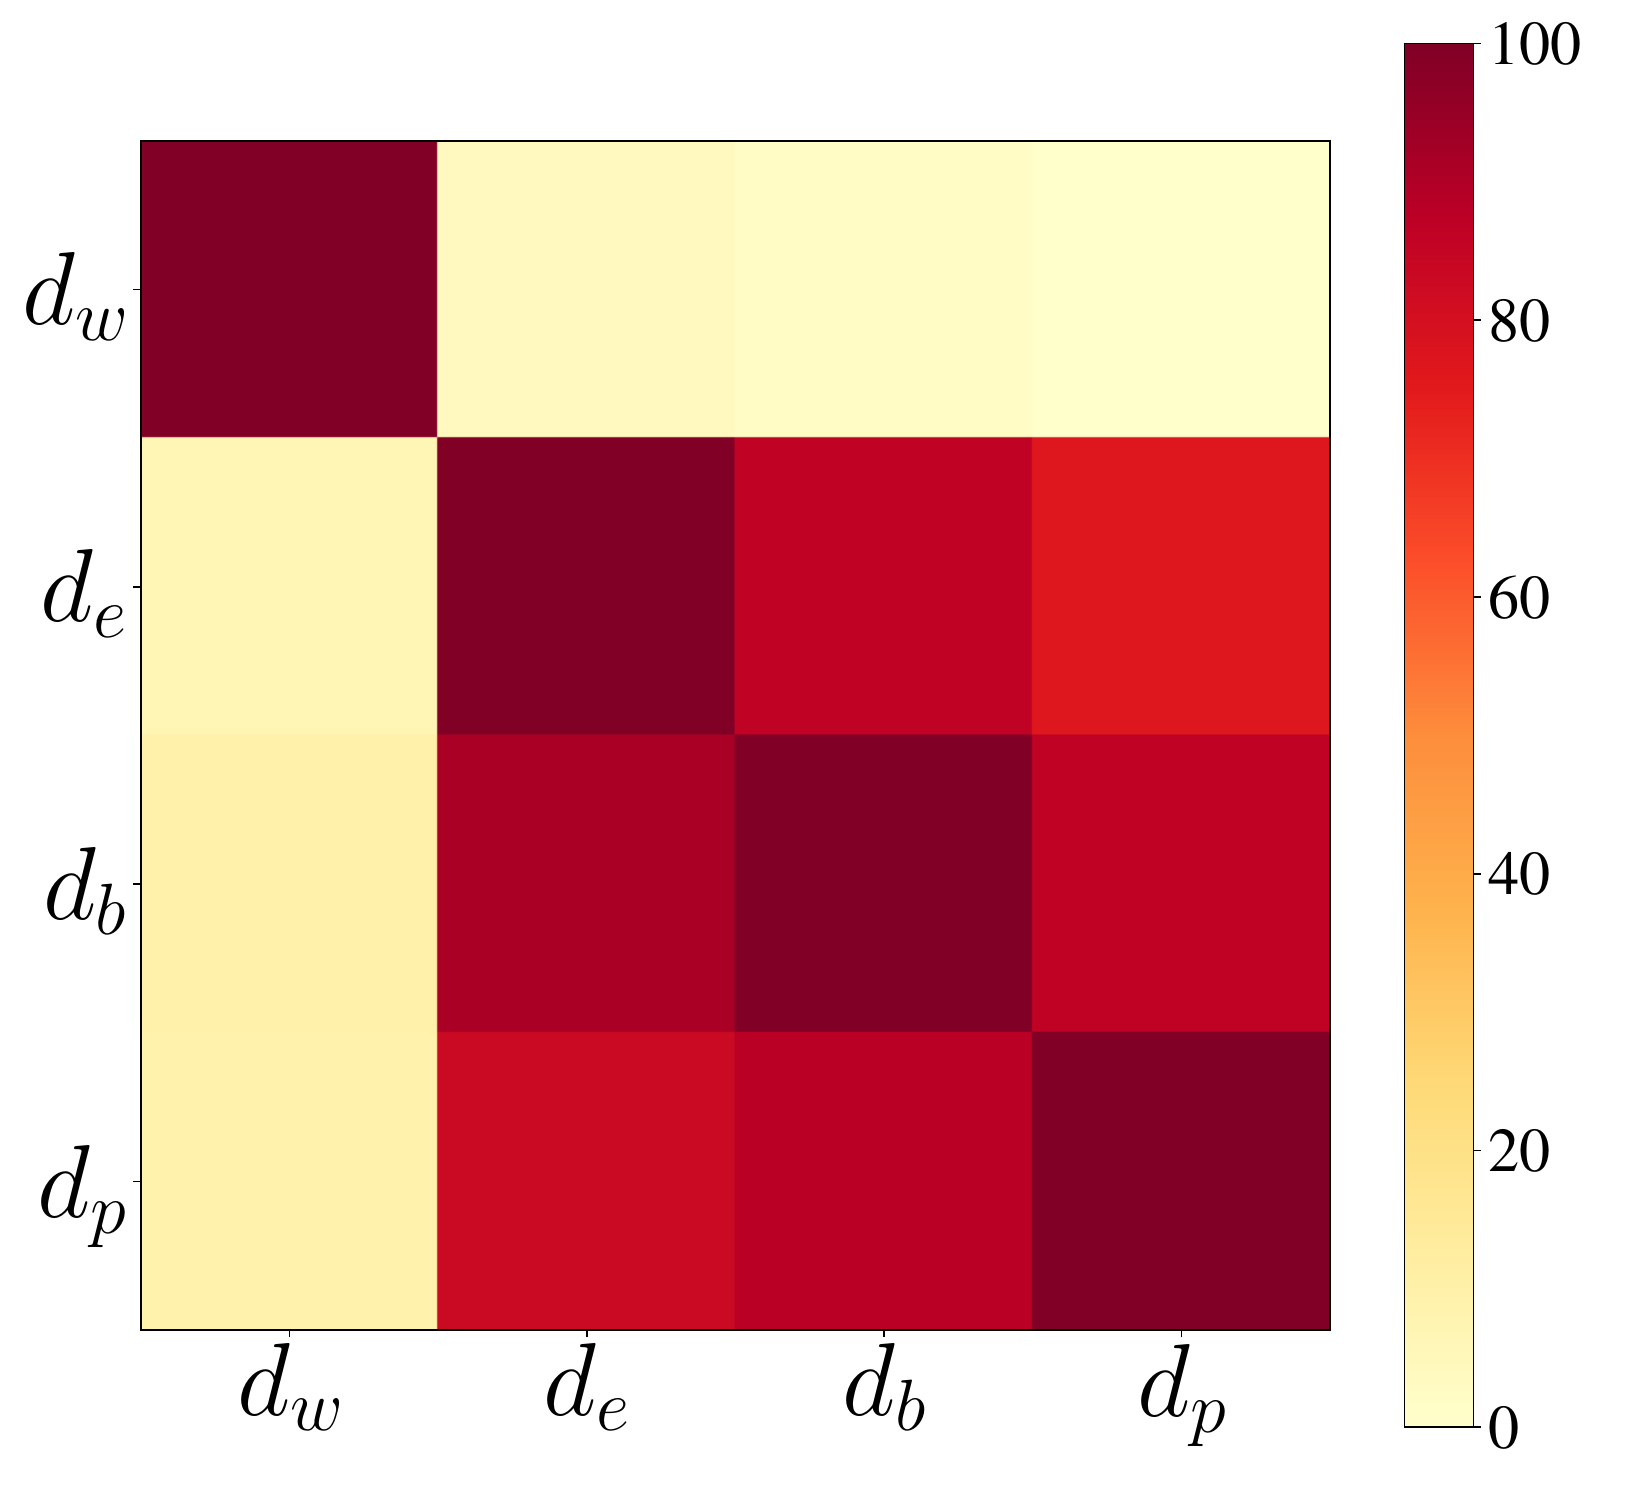}
\caption{
    Pairwise differences between the methods on the columns
    in relation to the methods on the rows
    for \dataset{Boussinesq2D}.
}
\label{fig-Boussinesq2DSimilarities}
\end{figure}

\subsection*{Results using Cylinder3D}
The results of the experiments using \dataset{Cylinder3D}
are shown from \Cref{fig-Cylinder3DAllNodes}
to \Cref{fig-Cylinder3DSimilarities}.

\begin{figure}
\centering
\includegraphics[width=0.8\linewidth]{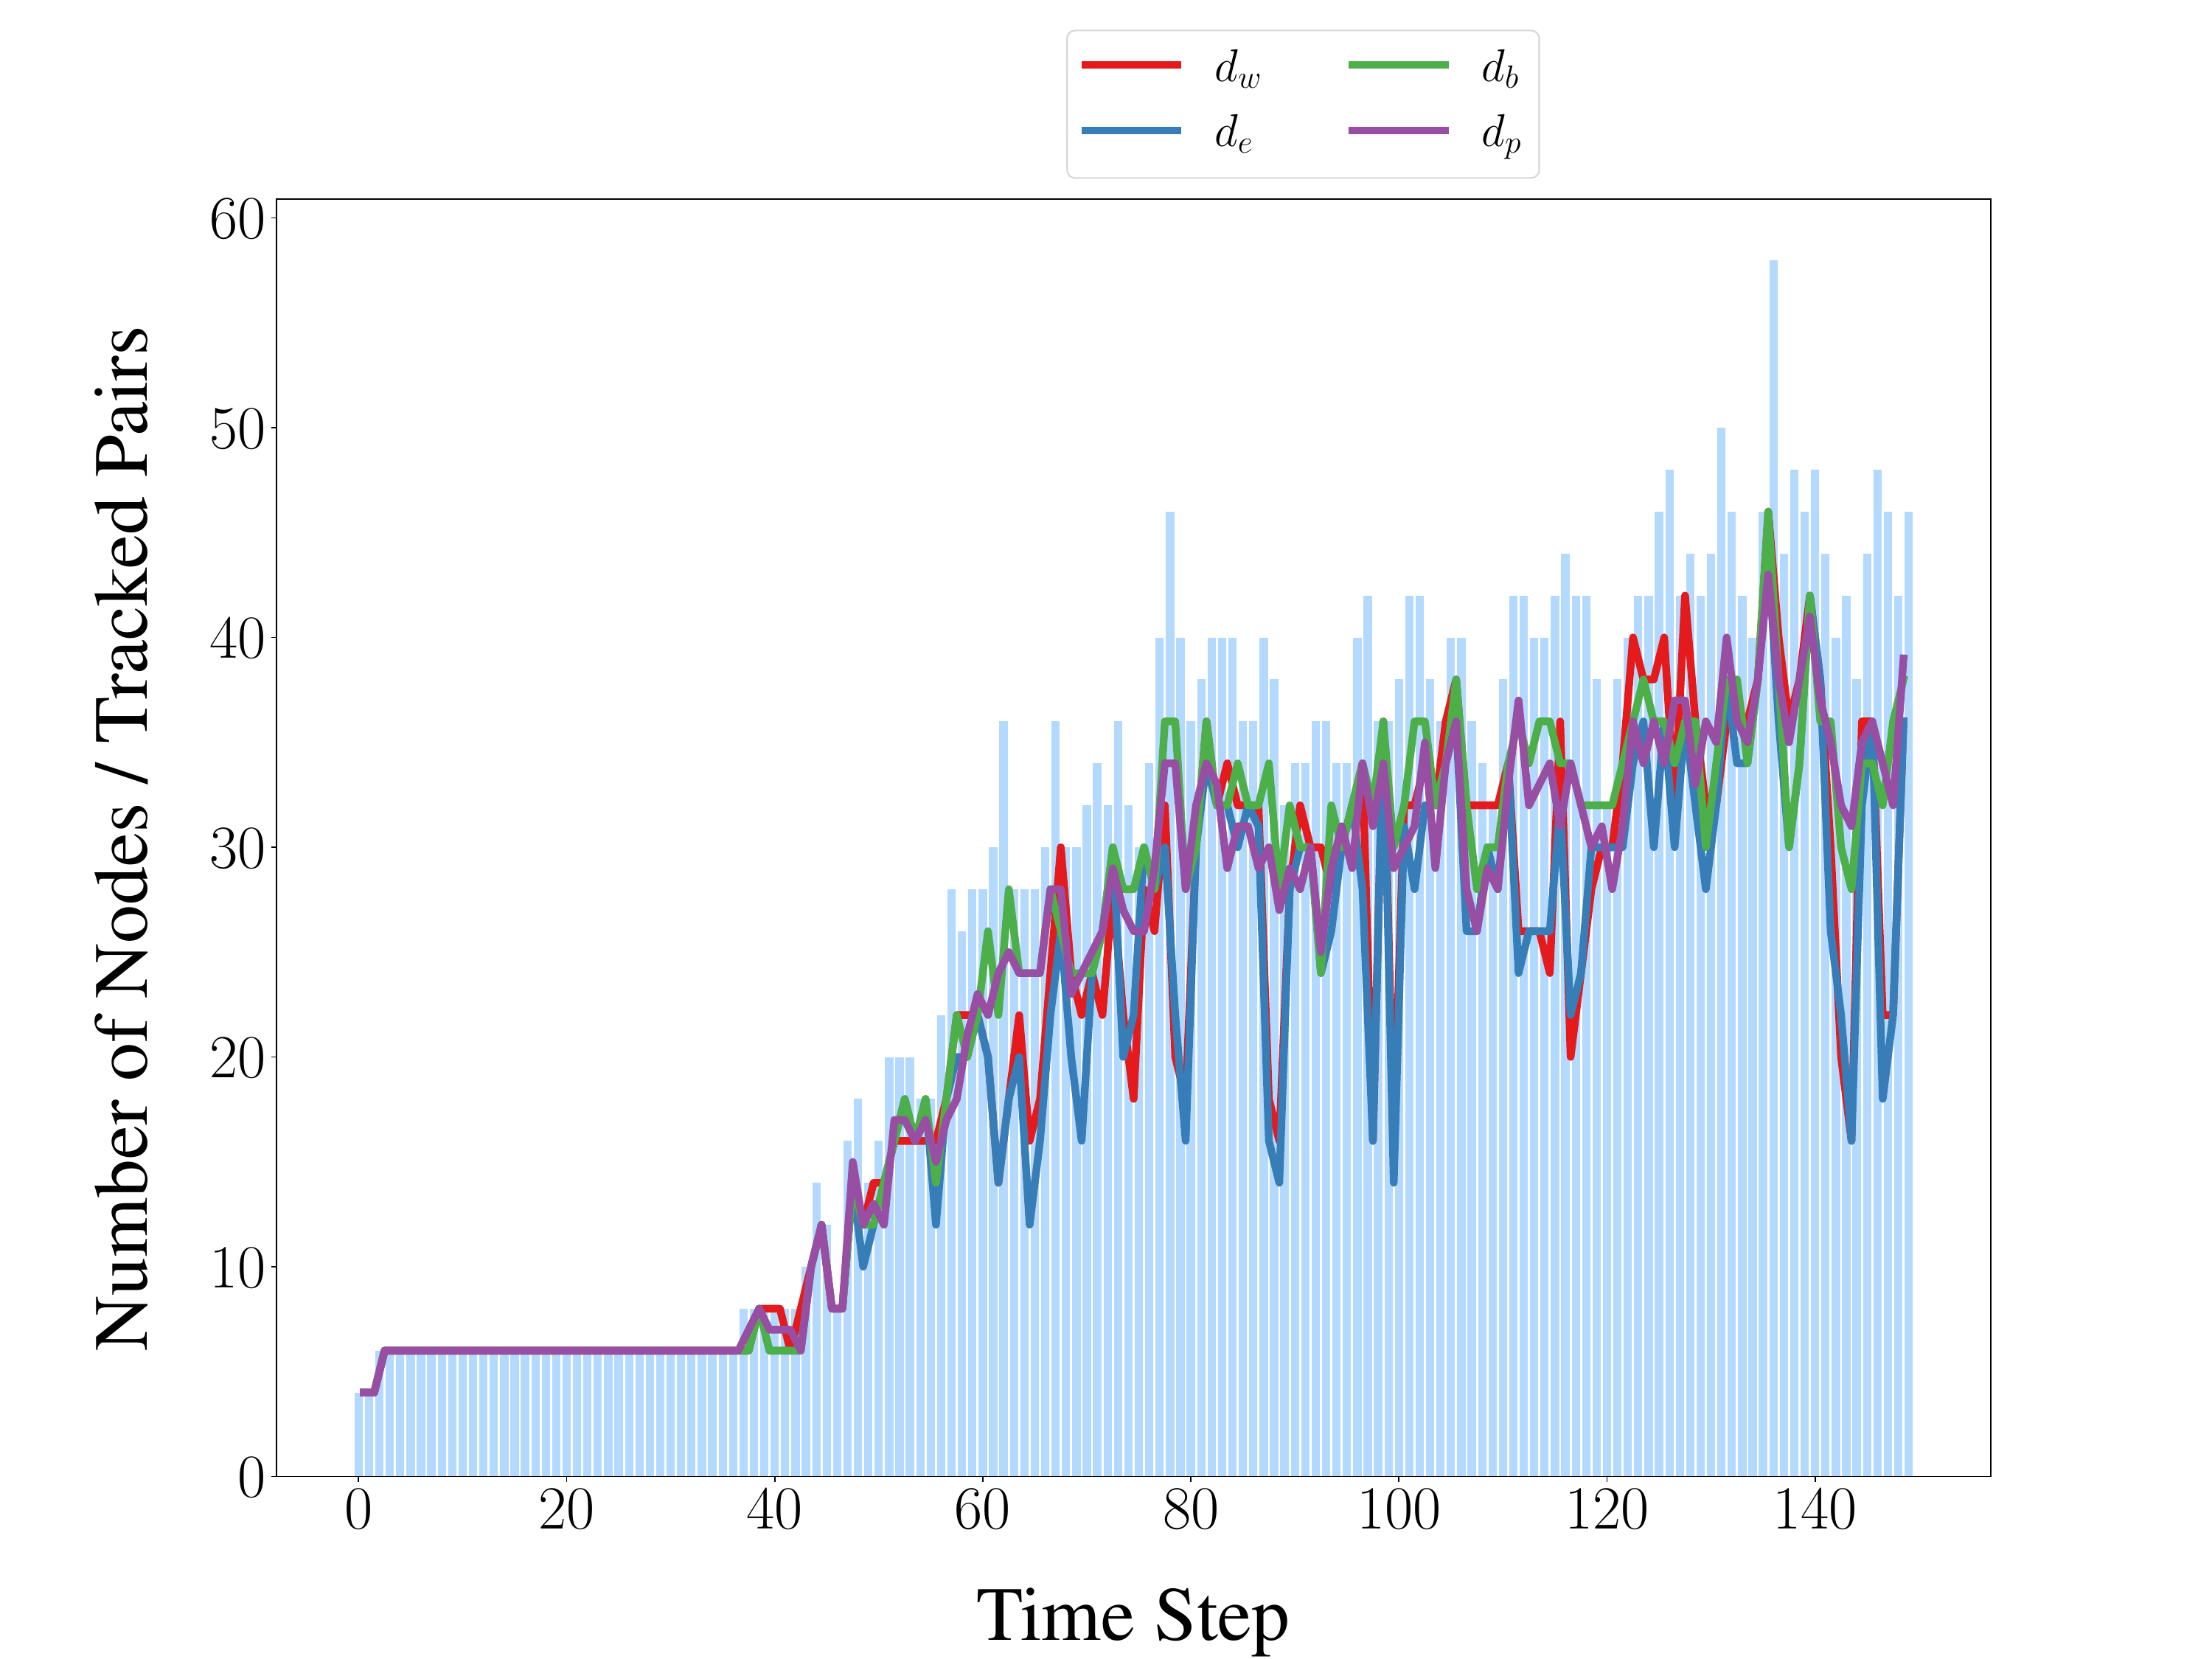}
\caption{
    Number of tracked nodes (colored and labeled) 
    relative to the total nodes of merge trees (light blue bars)
    for \dataset{Cylinder3D}.
}
\label{fig-Cylinder3DAllNodes}
\end{figure}

\begin{figure}
\centering
\includegraphics[width=0.8\linewidth]{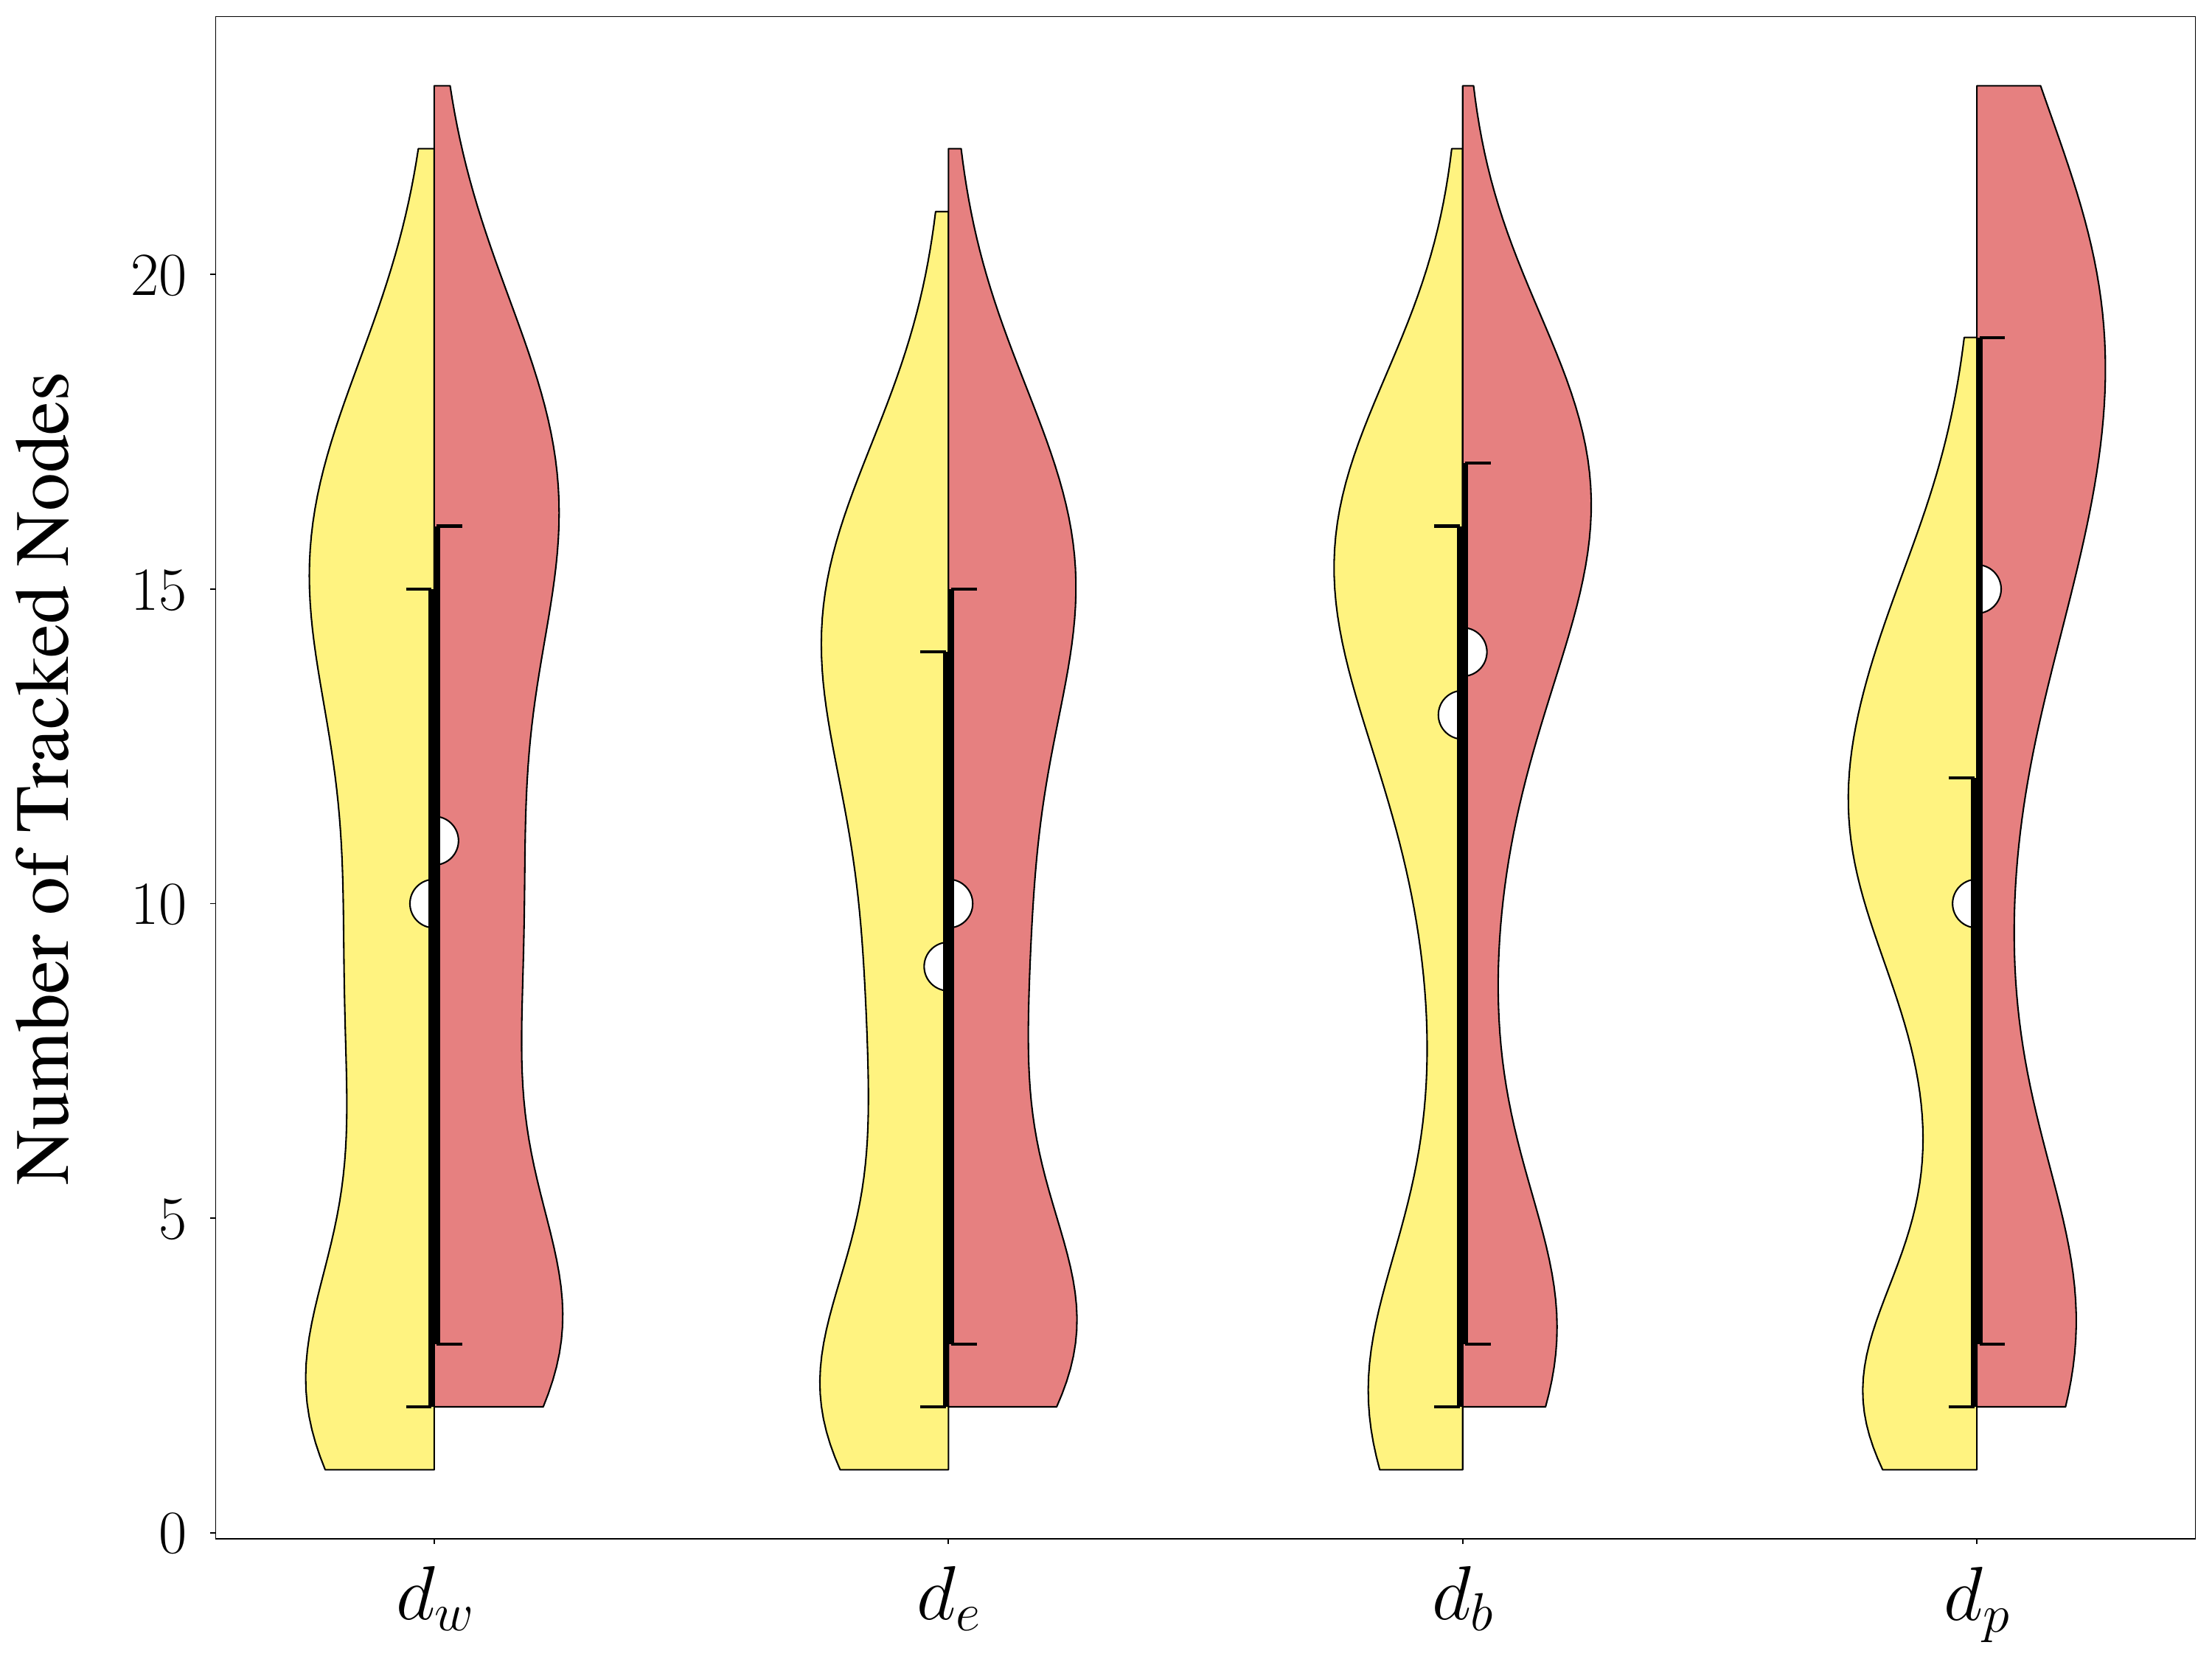}
\caption{
    Distributions of tracked nodes 
    of \dataset{Cylinder3D},  
    divided by types:
    saddle (yellow) and minima (blue).
}
\label{fig-Cylinder3DViolin}
\end{figure}

% Length histogram
\begin{figure}%
\begin{subfigure}[t]{\ltwopicwidth}%
\includegraphics[width=\ltwopicwidth]{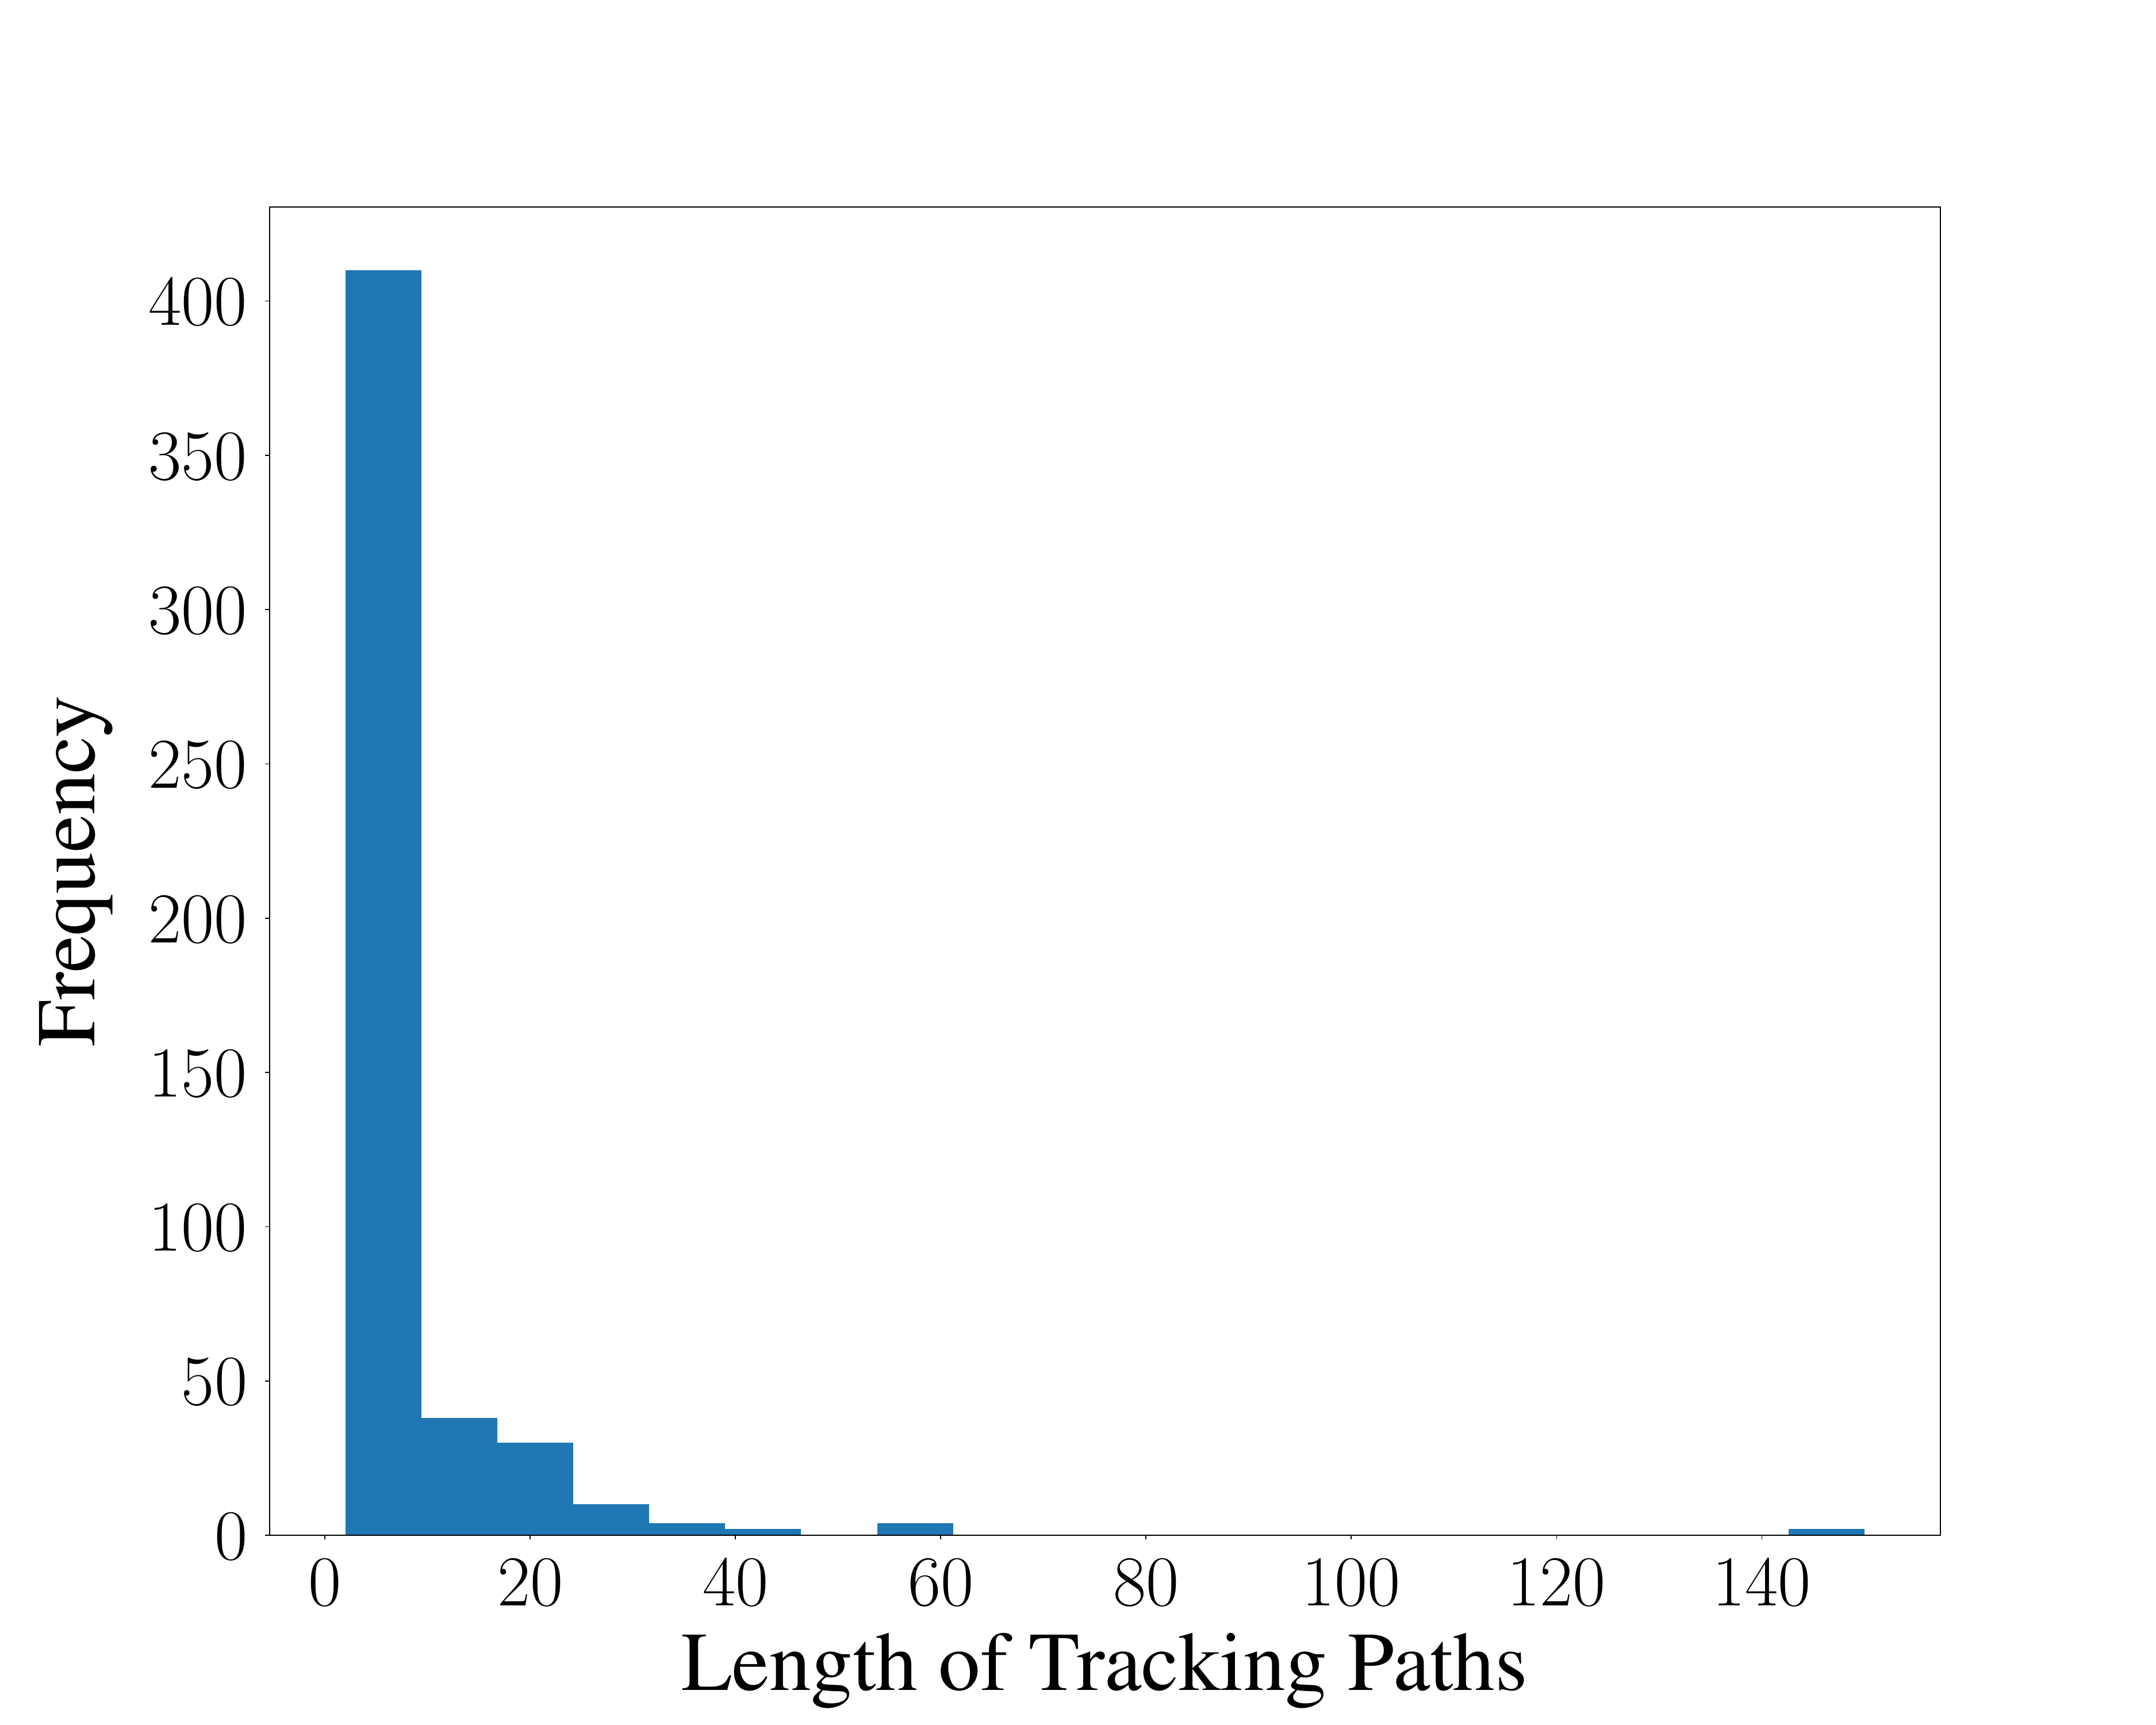}
\caption{$d_w$.}%
\label{fig-LengthHistogramCylinder3DW}%
\end{subfigure}
\hfill%
\begin{subfigure}[t]{\ltwopicwidth}%
\includegraphics[width=\ltwopicwidth]{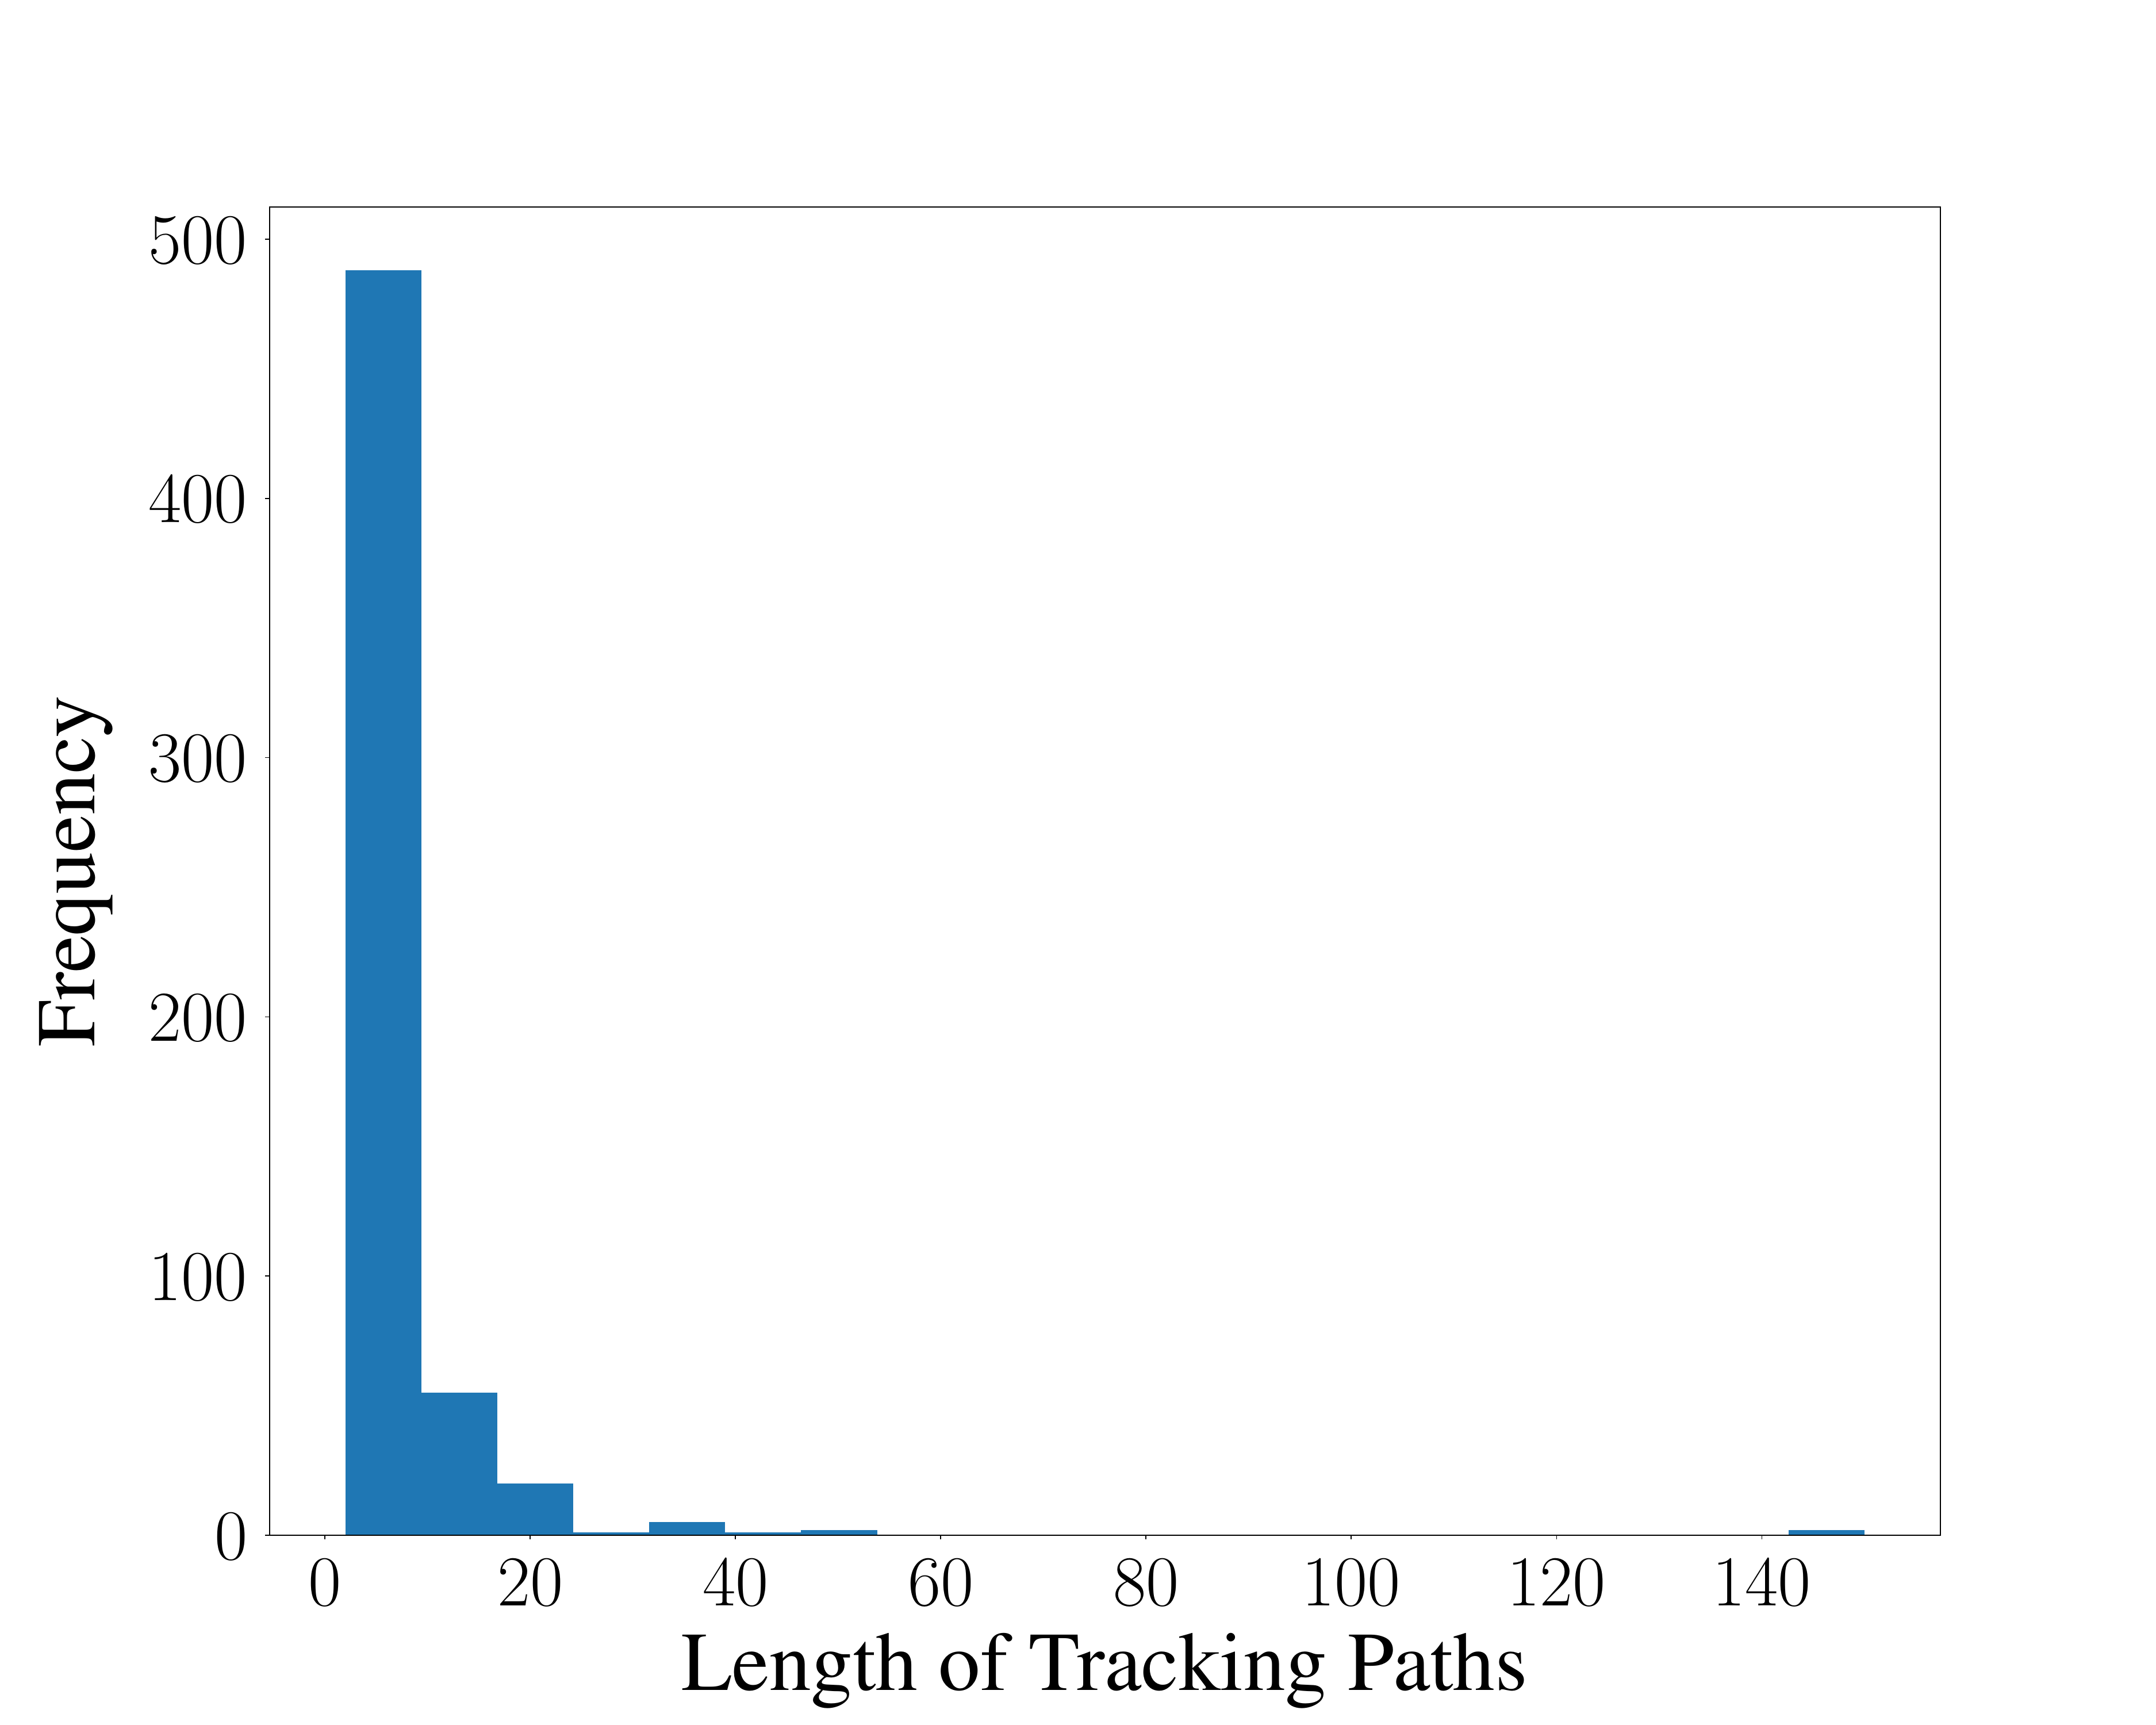}%
\caption{$d_e$.}%
\label{fig-LengthHistogramCylinder3DE}%
\end{subfigure}%
\\%
\begin{subfigure}[t]{\ltwopicwidth}%
\includegraphics[width=\ltwopicwidth]{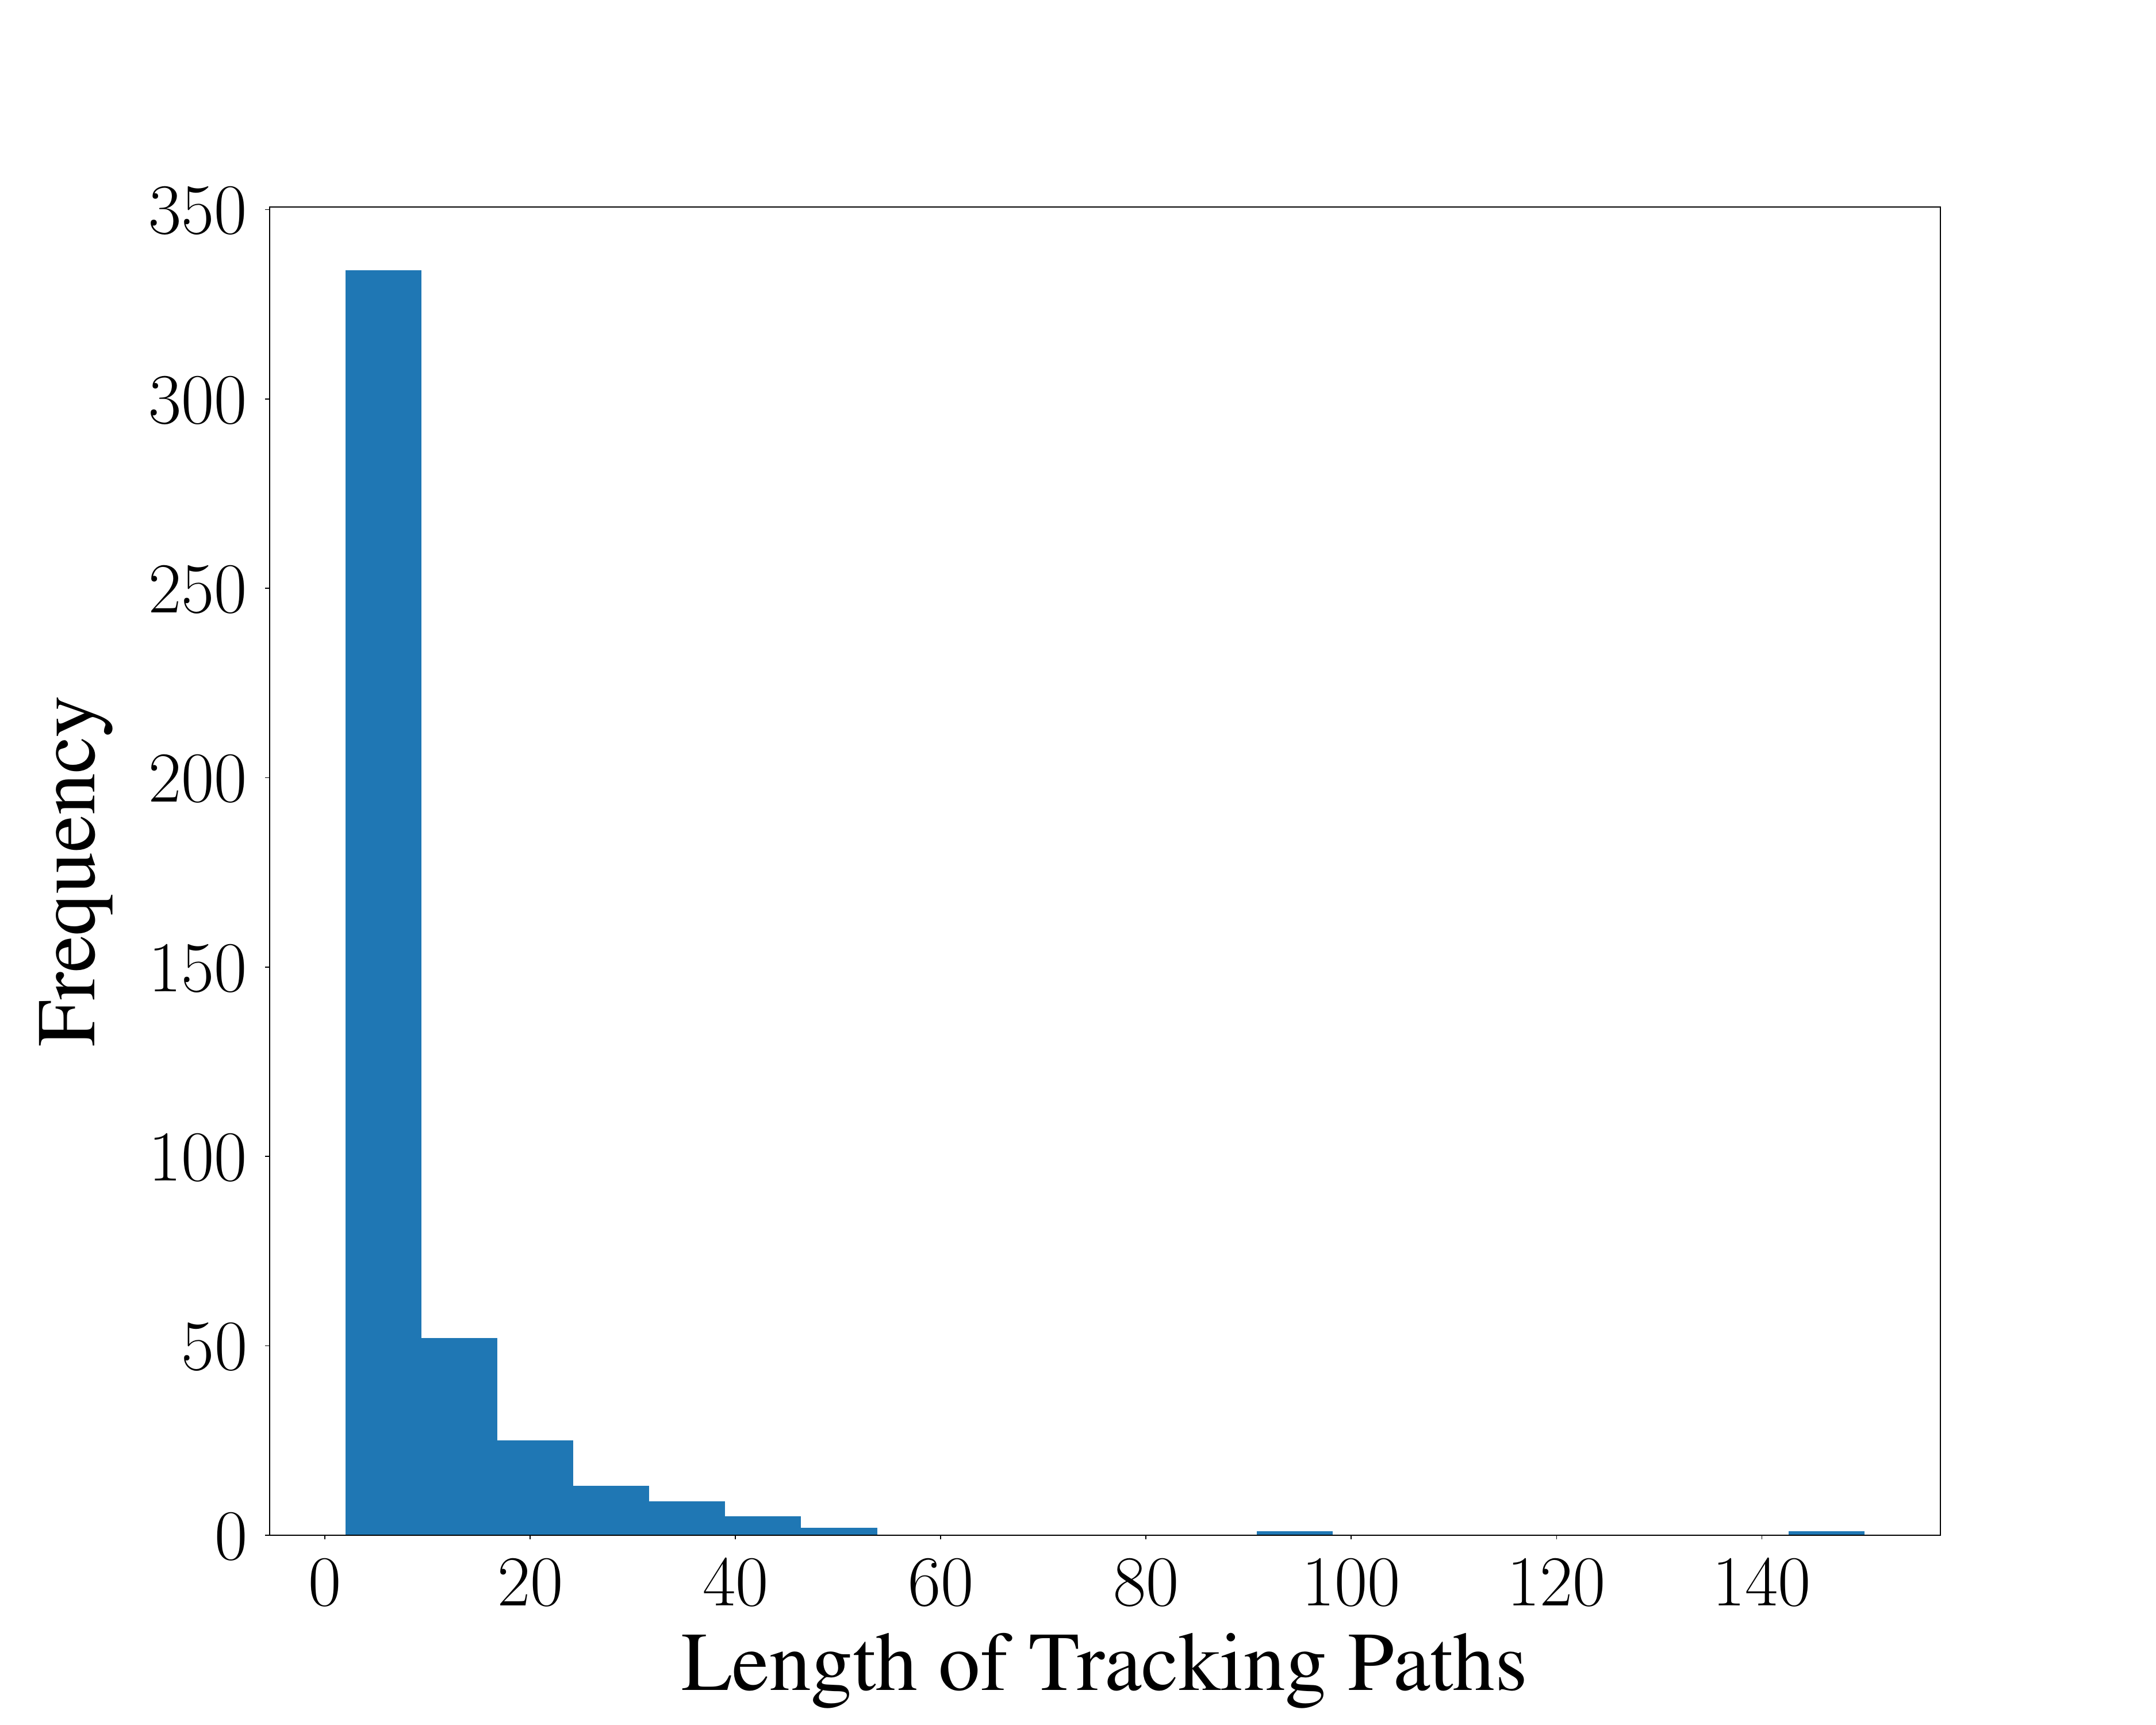}%
\caption{$d_b$.}%
\label{fig-LengthHistogramCylinder3DB}%
\end{subfigure}%
\hfill%
\begin{subfigure}[t]{\ltwopicwidth}%
\includegraphics[width=\ltwopicwidth]{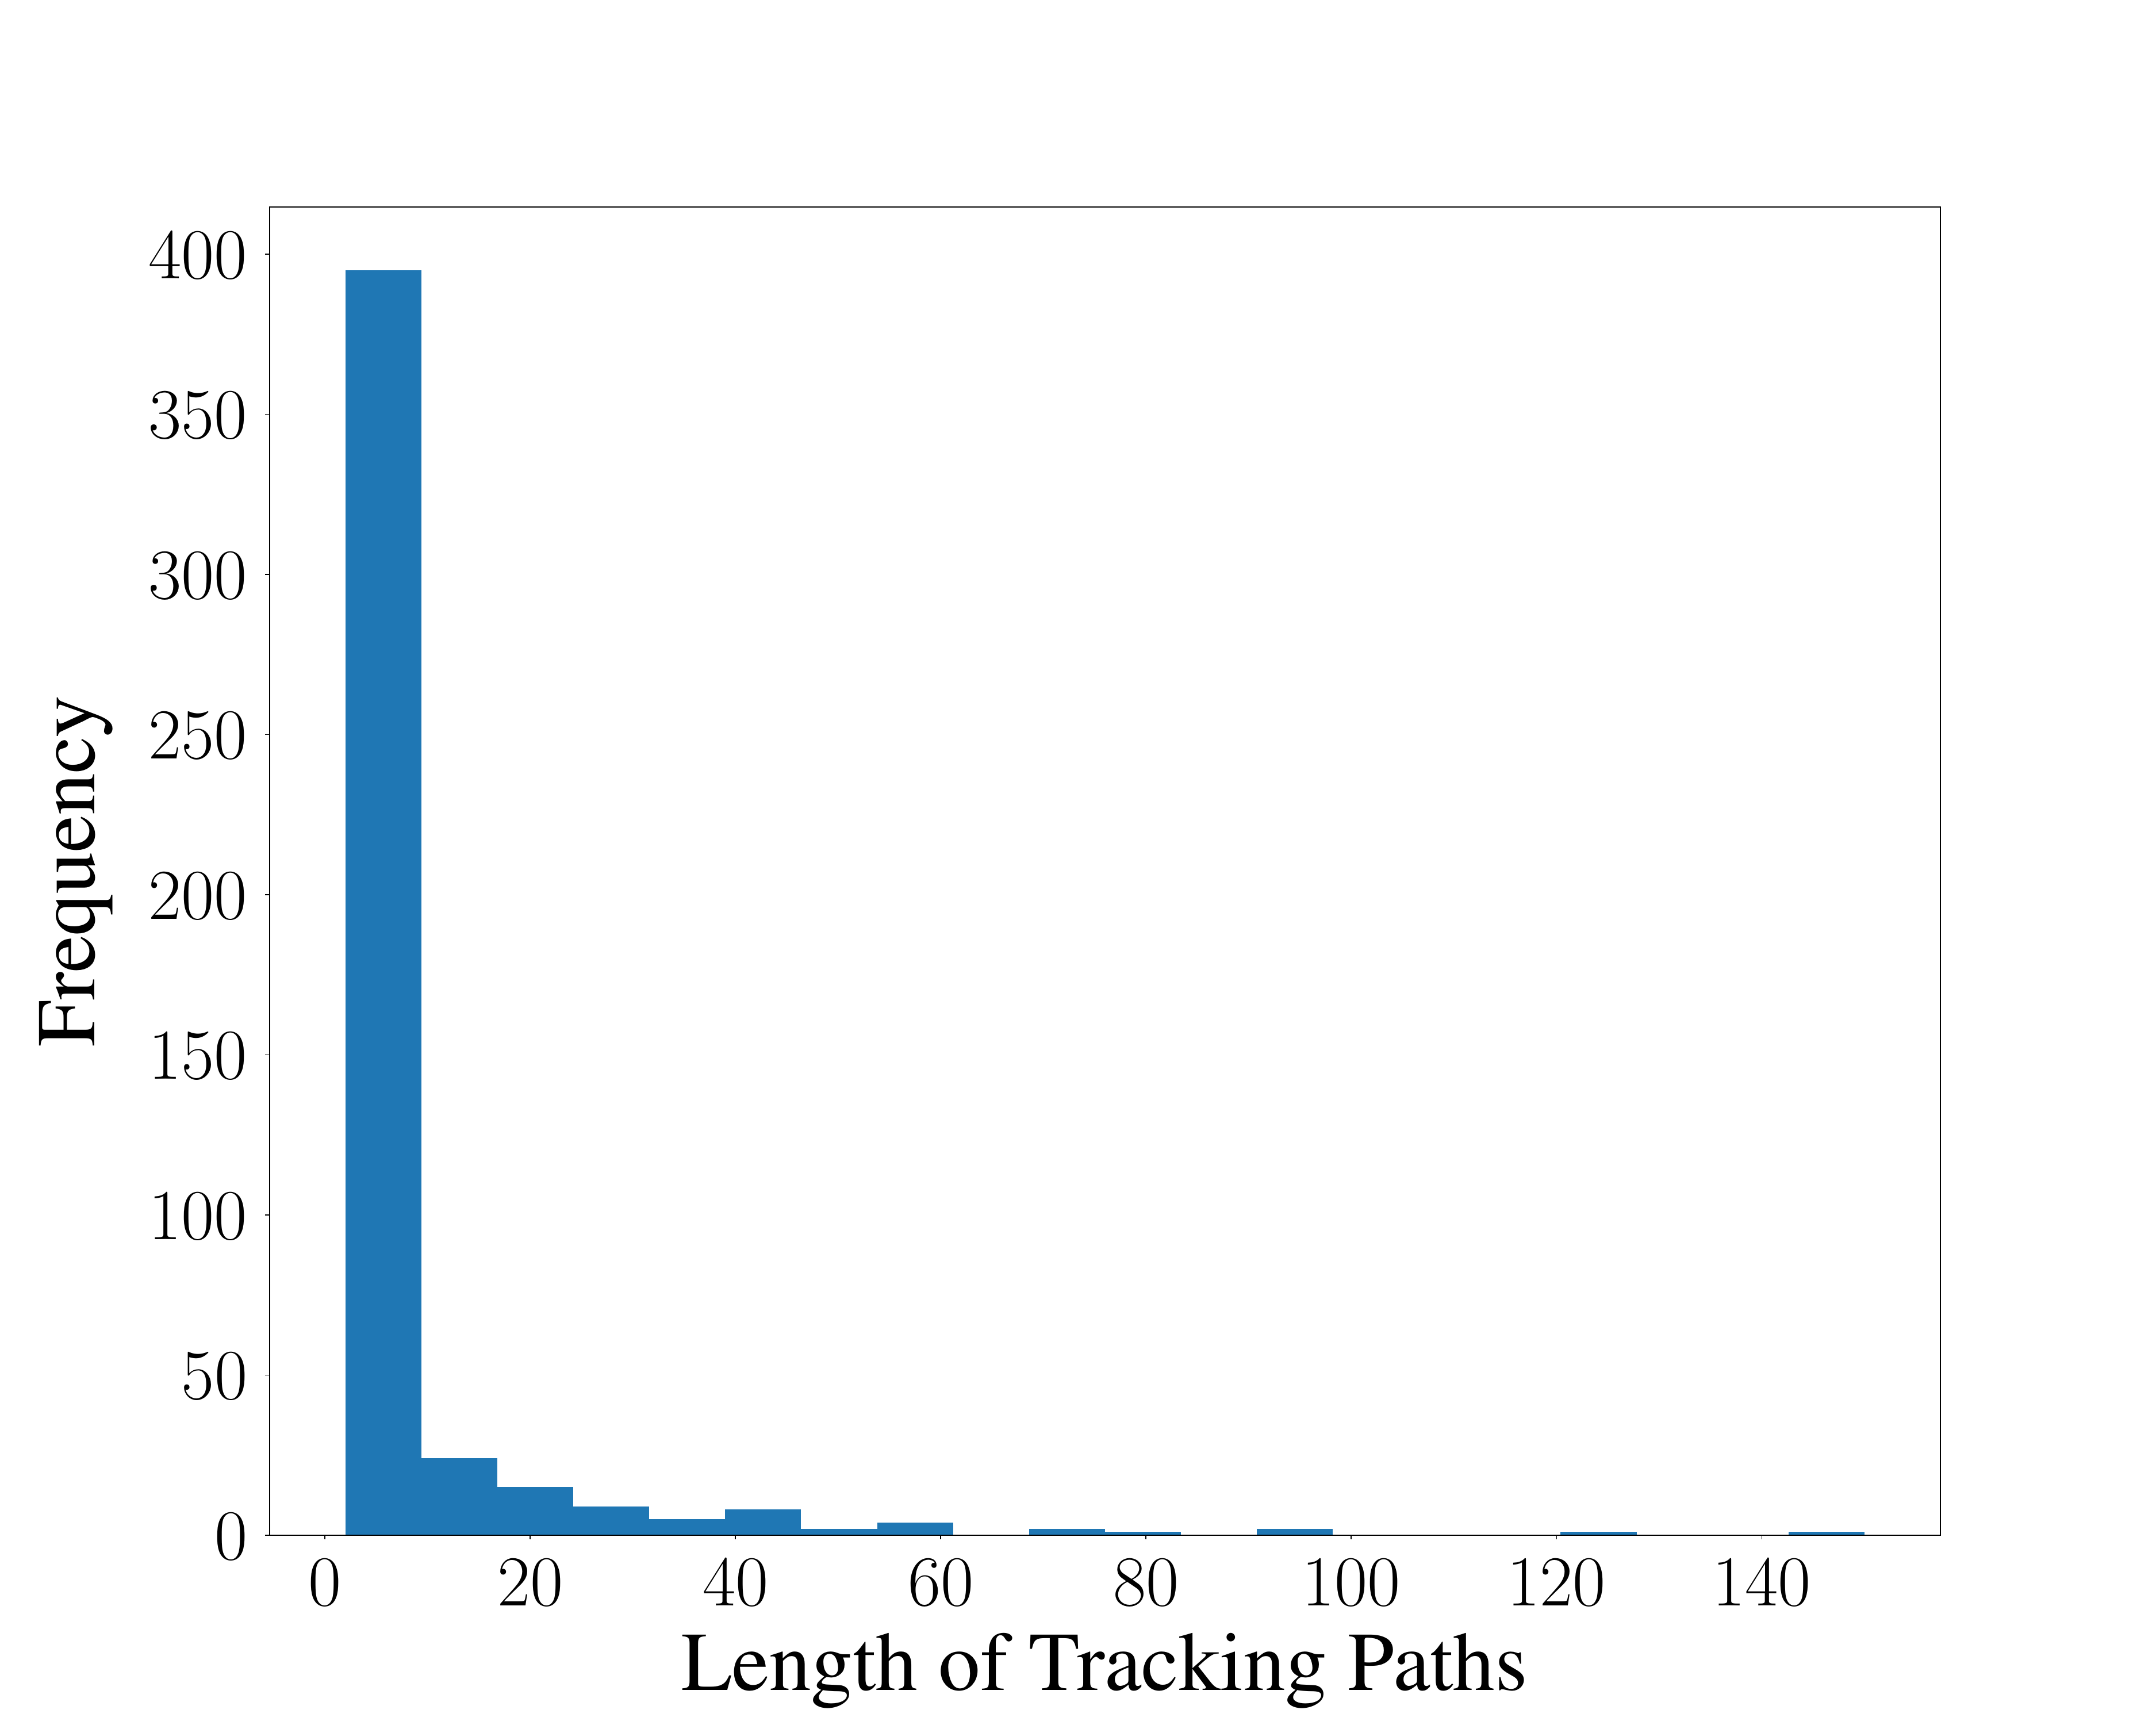}%
\caption{$d_p$.}%
\label{fig-LengthHistogramCylinder3DP}%
\end{subfigure}%
\caption{Histograms of the length of the tracking paths 
    of \dataset{Cylinder3D}.}%
\label{fig-LengthHisgoramCylinder3D}%
\end{figure}

\begin{figure}
\centering
\includegraphics[width=0.8\linewidth]{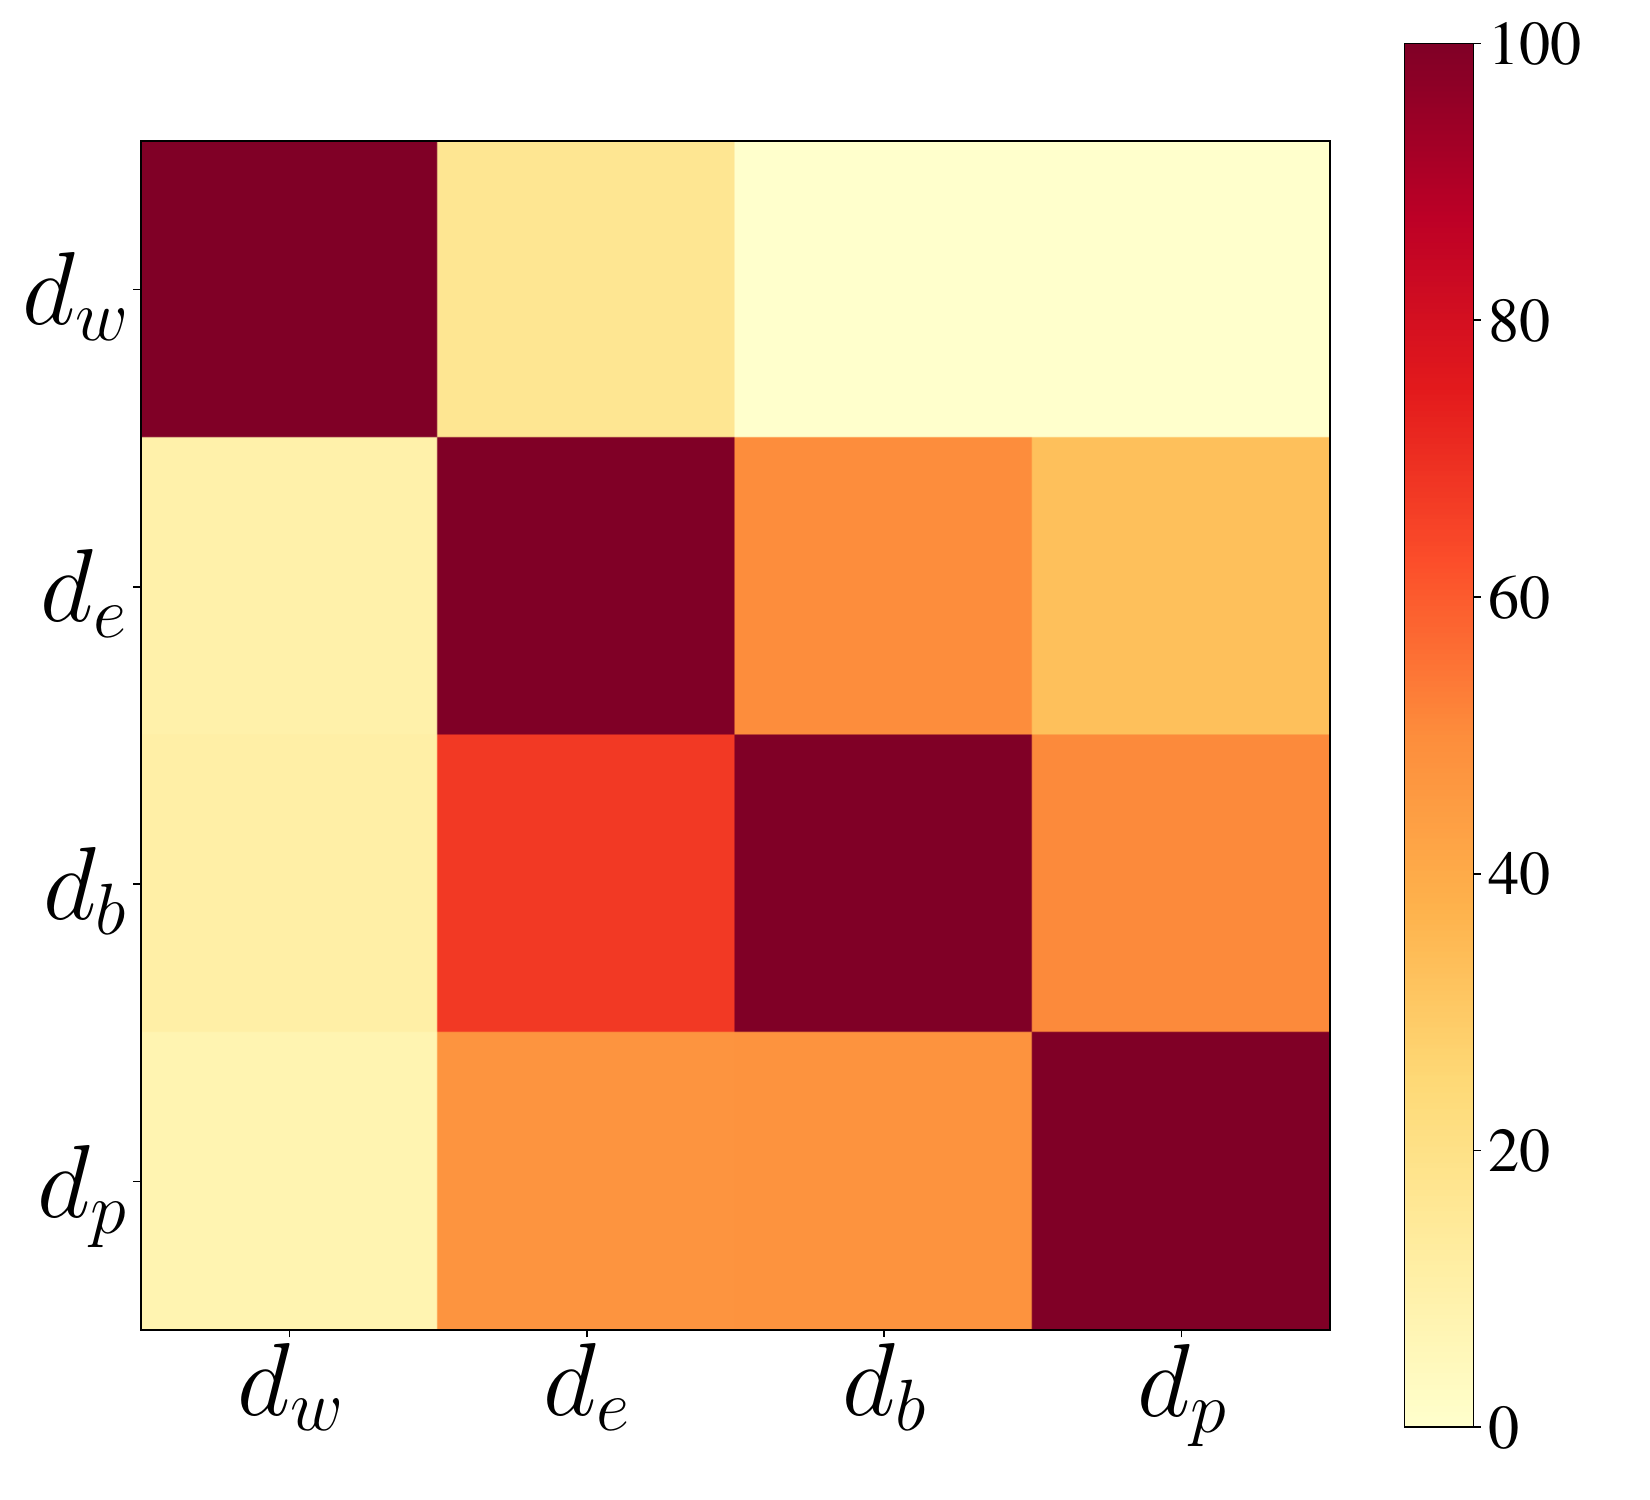}
\caption{
    Pairwise differences between the methods on the columns
    in relation to the methods on the rows
    for \dataset{Cylinder3D}.
}
\label{fig-Cylinder3DSimilarities}
\end{figure}

\subsection*{Results with Tangaroa data set}
The results of the experiments using \dataset{Tangaroa3D}
are shown in \Cref{fig-Tangaroa3DAllNodes}
through \Cref{fig-Tangaroa3DSimilarities}.

\begin{figure}
\centering
\includegraphics[width=0.8\linewidth]{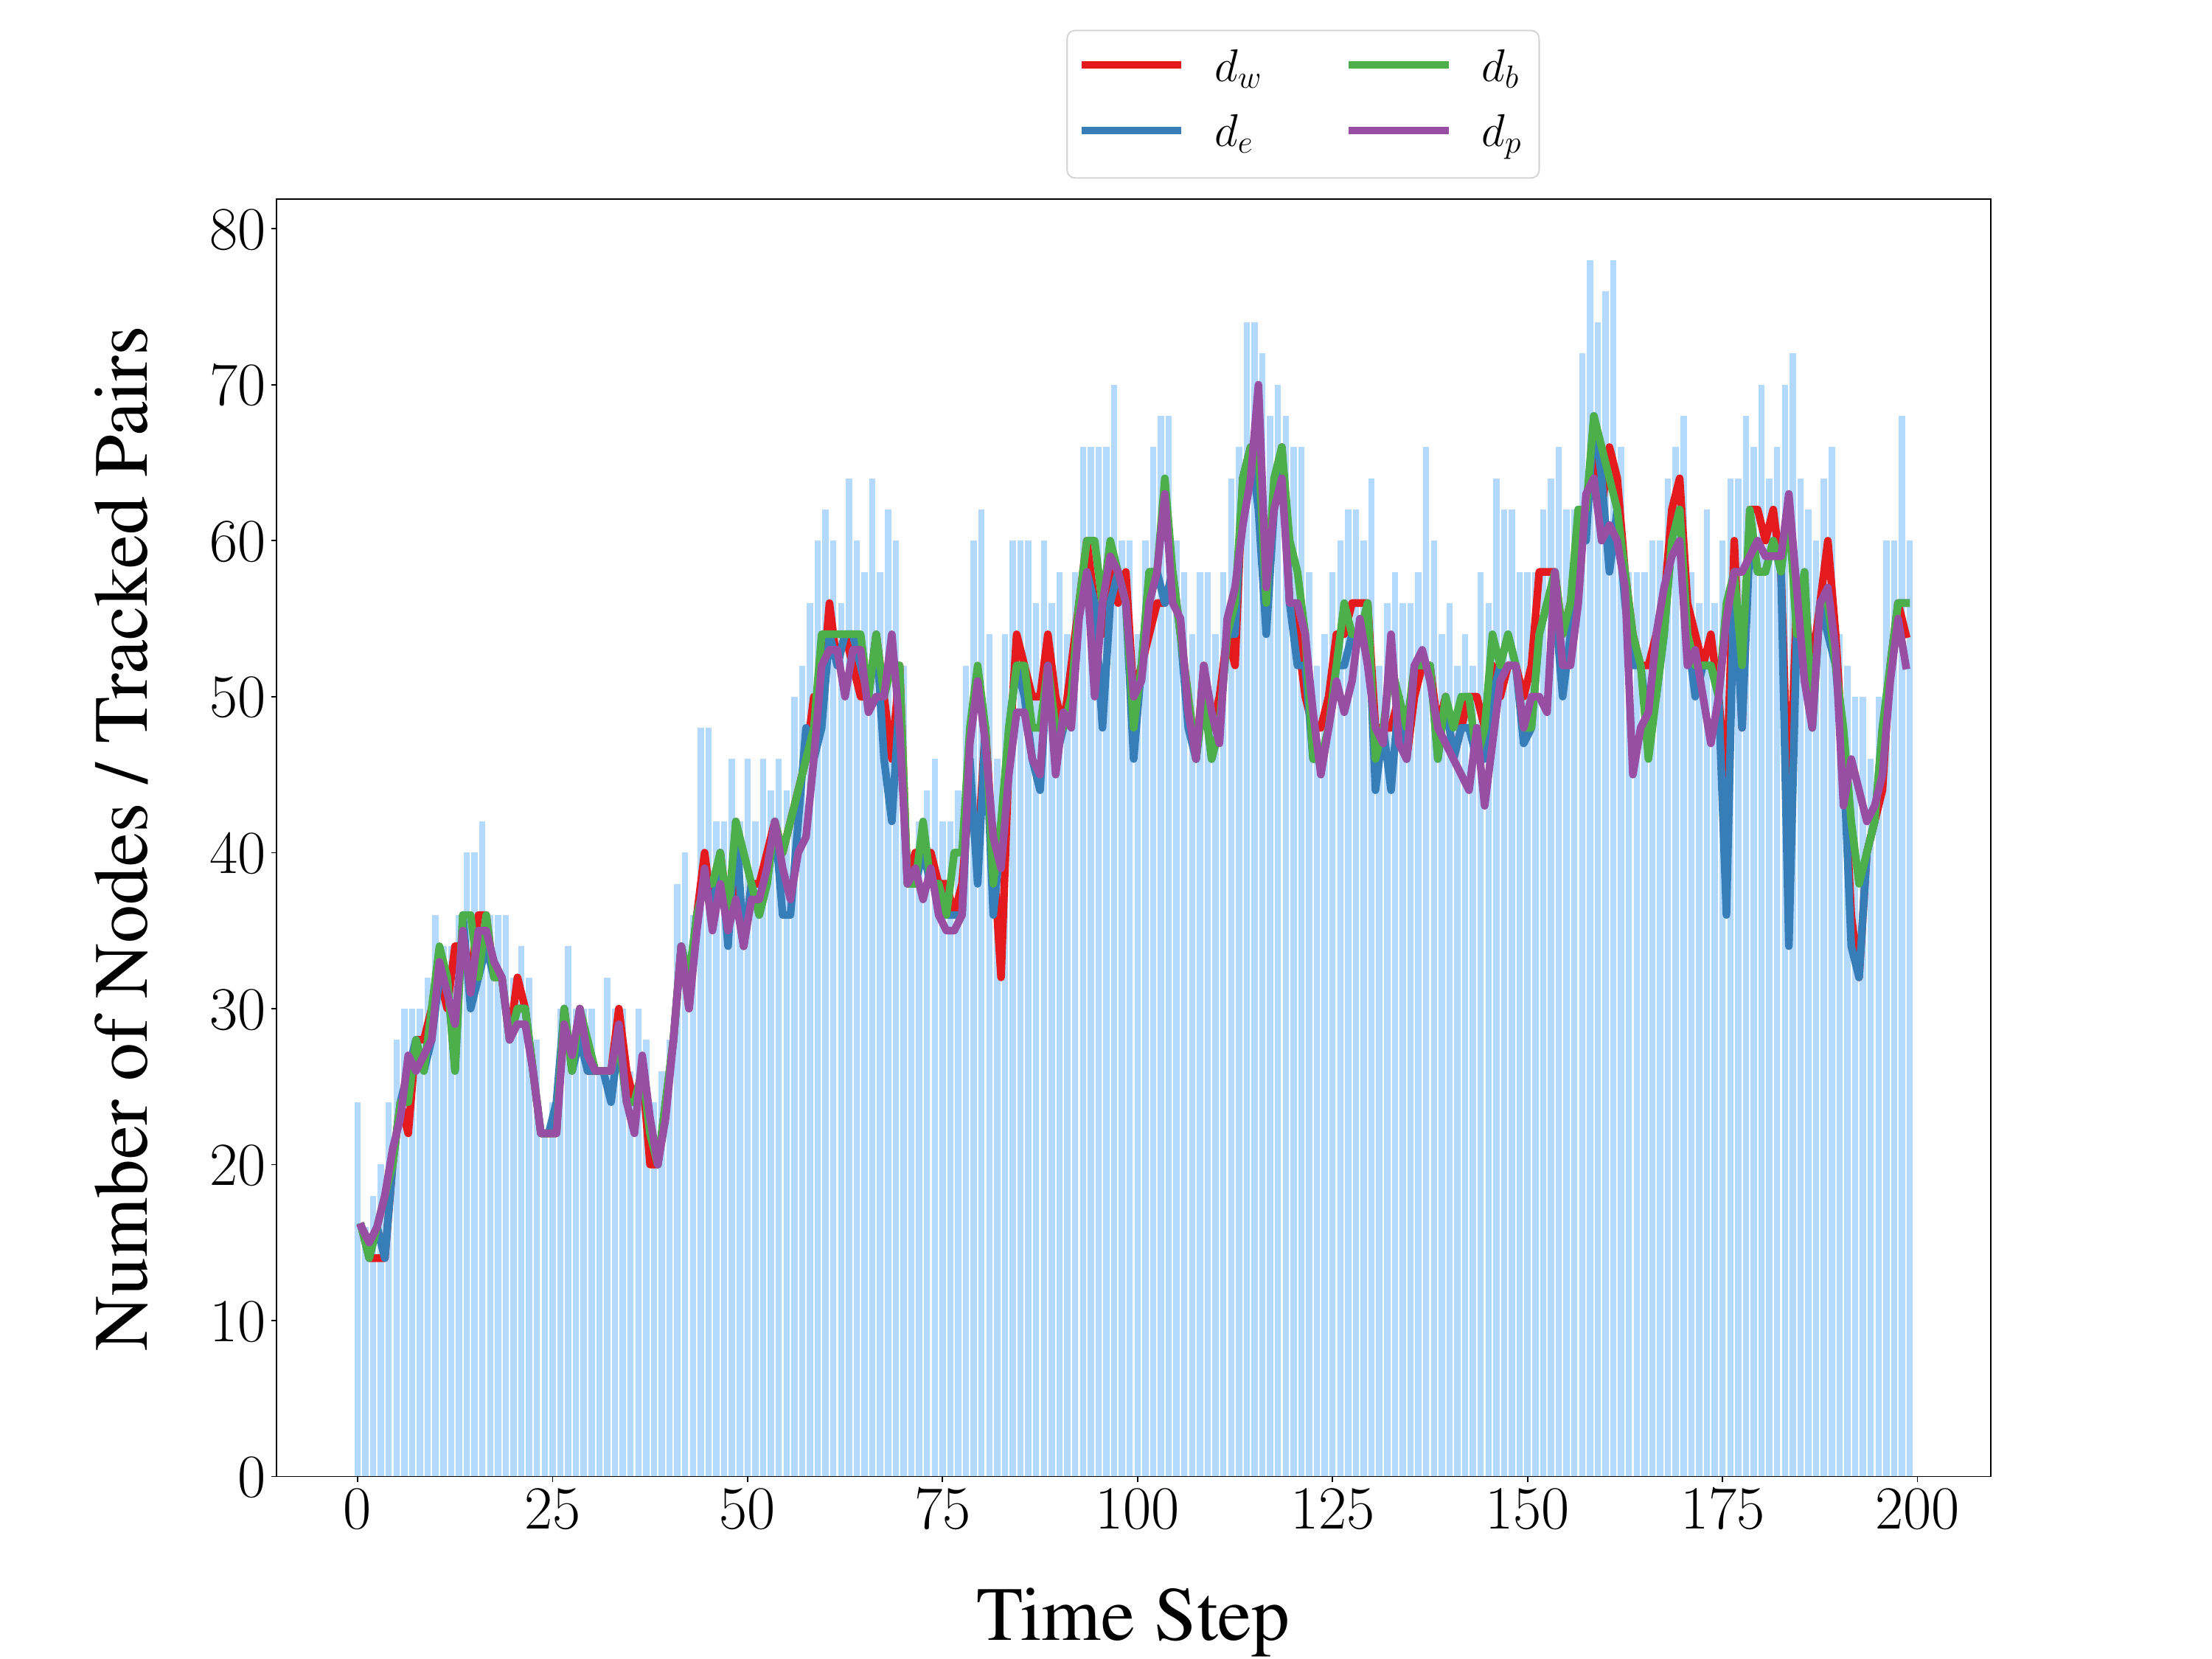}
\caption{
    Number of tracked nodes (colored and labeled) 
    relative to the total nodes of merge trees (light blue bars)
    for \dataset{Tangaroa3D}.
}
\label{fig-Tangaroa3DAllNodes}
\end{figure}

\begin{figure}
\centering
\includegraphics[width=0.8\linewidth]{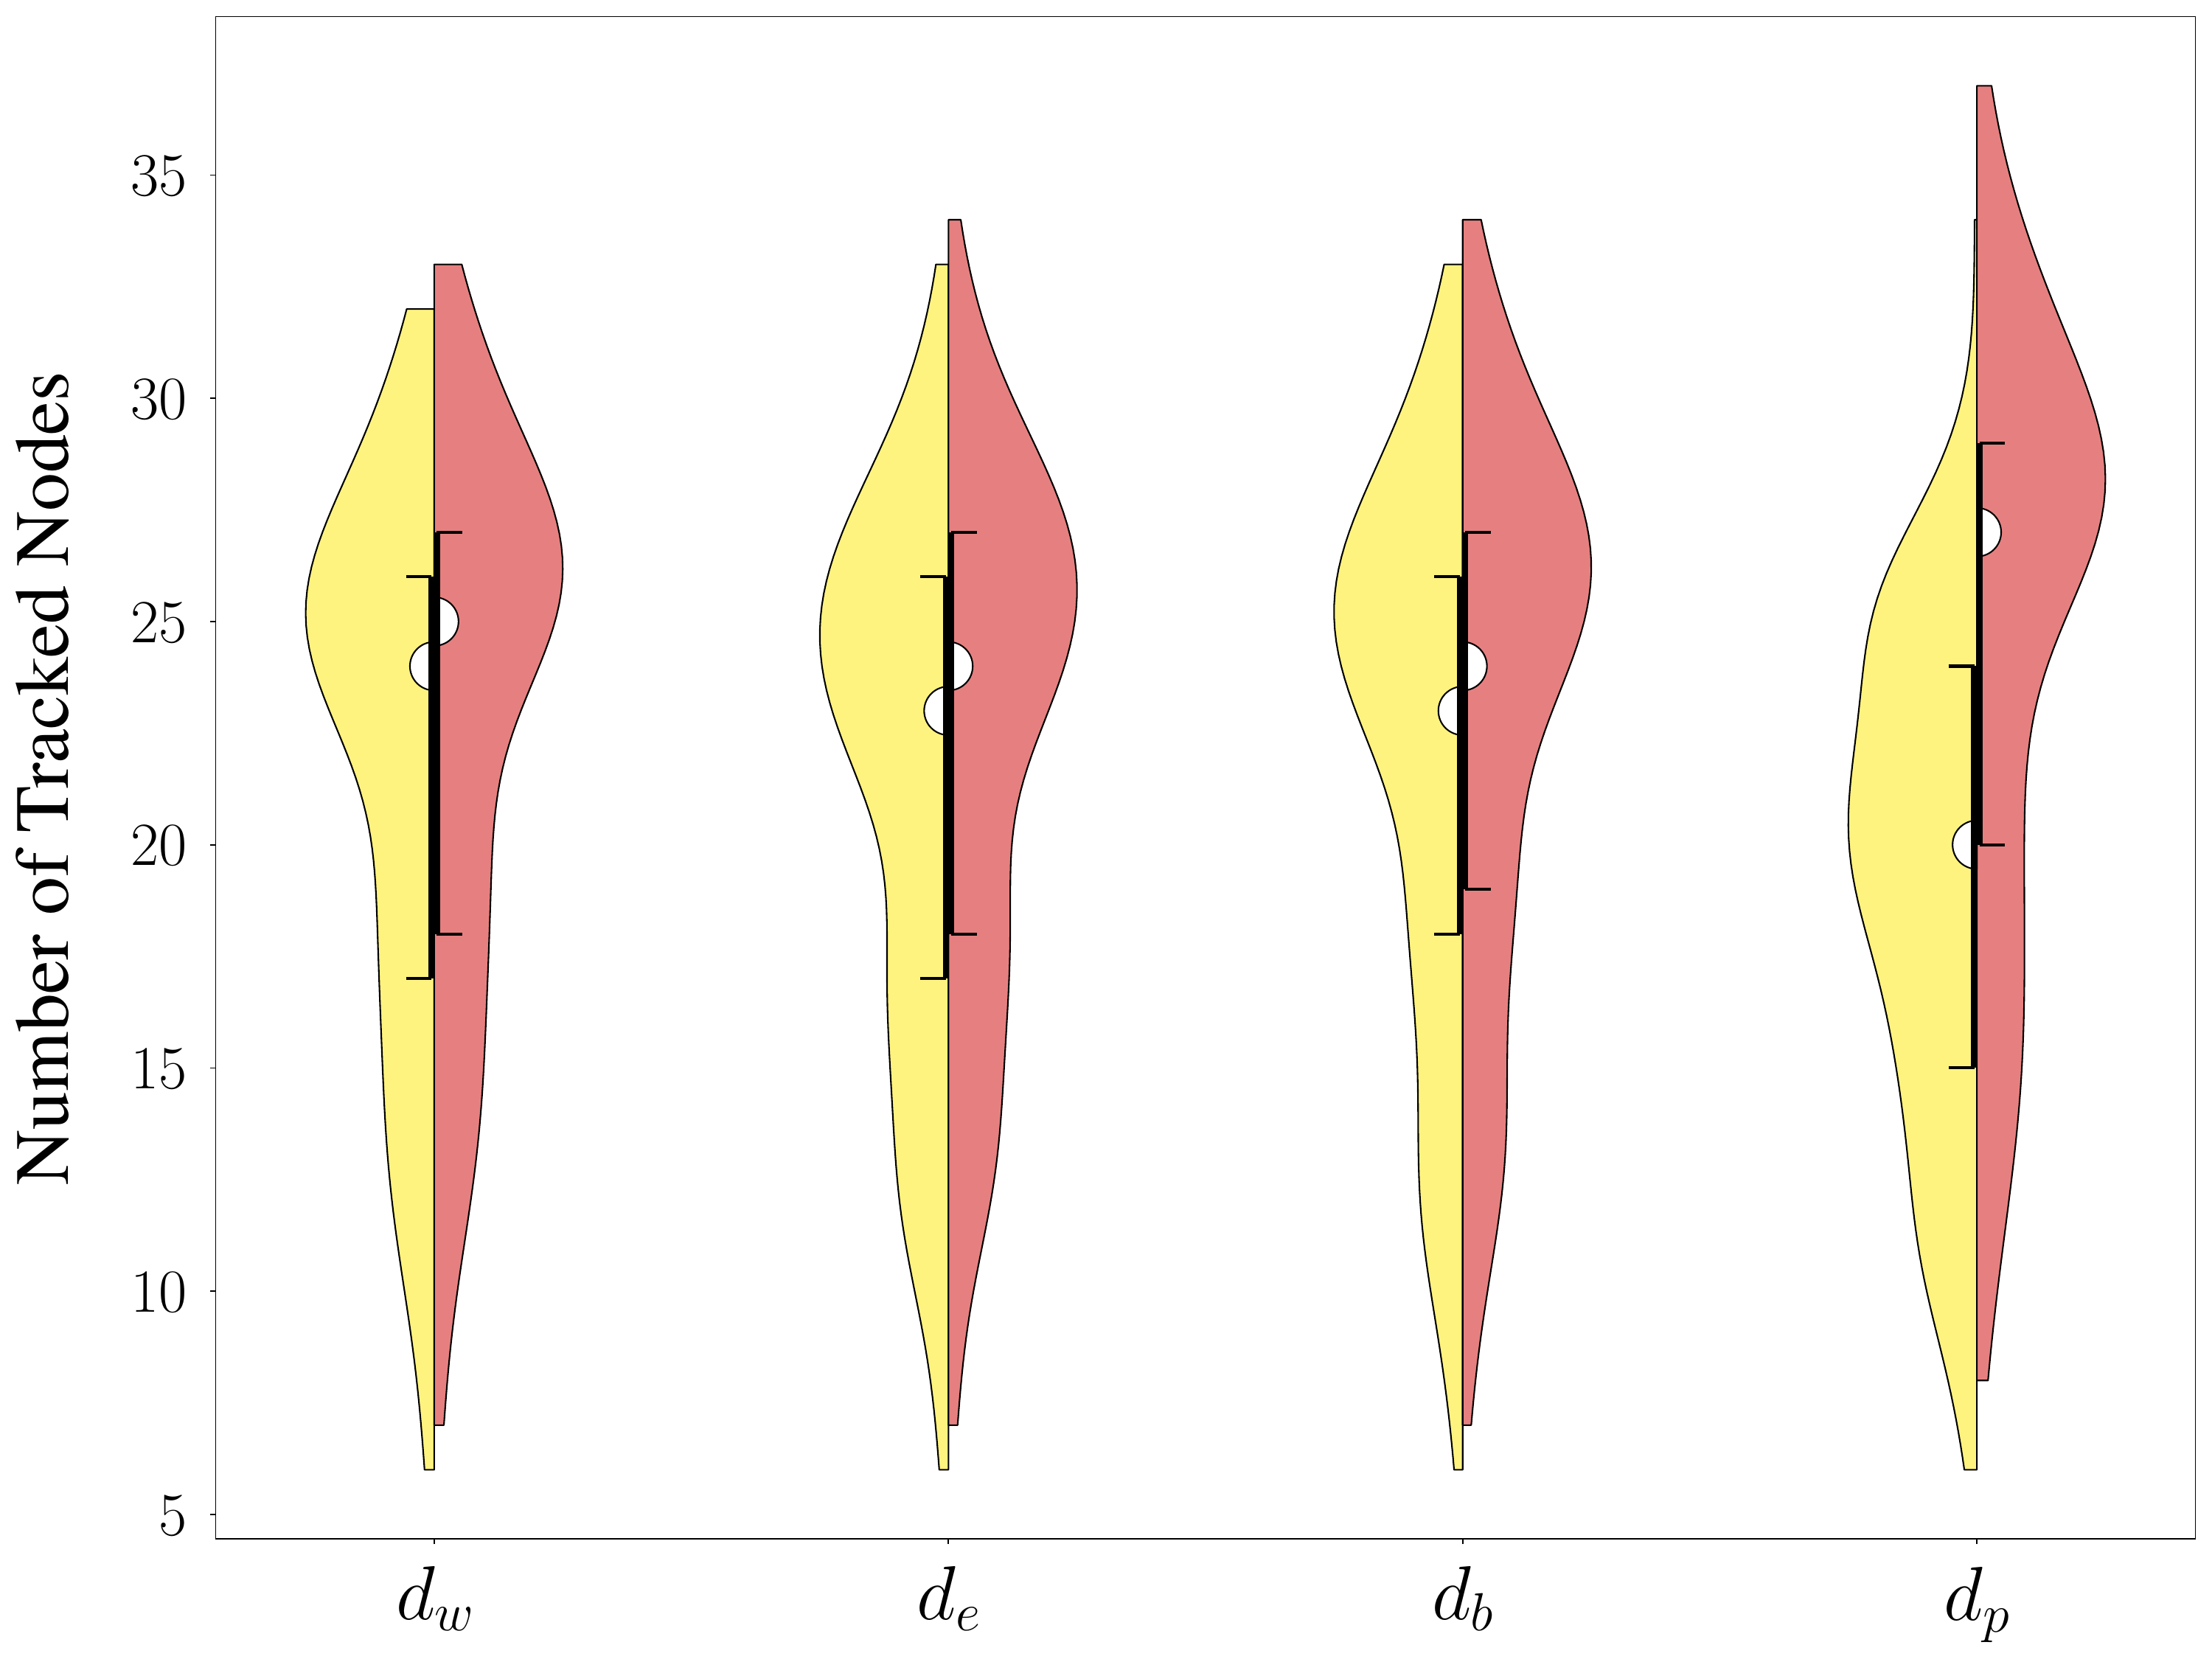}
\caption{
    Distributions of tracked nodes 
    \dataset{Tangaroa3D},  
    divided by types:
    saddle (yellow) and maxima (red).
}
\label{fig-Tangaroa3DViolin}
\end{figure}

% Length histogram
\begin{figure}%
\begin{subfigure}[t]{\ltwopicwidth}%
\includegraphics[width=\ltwopicwidth]{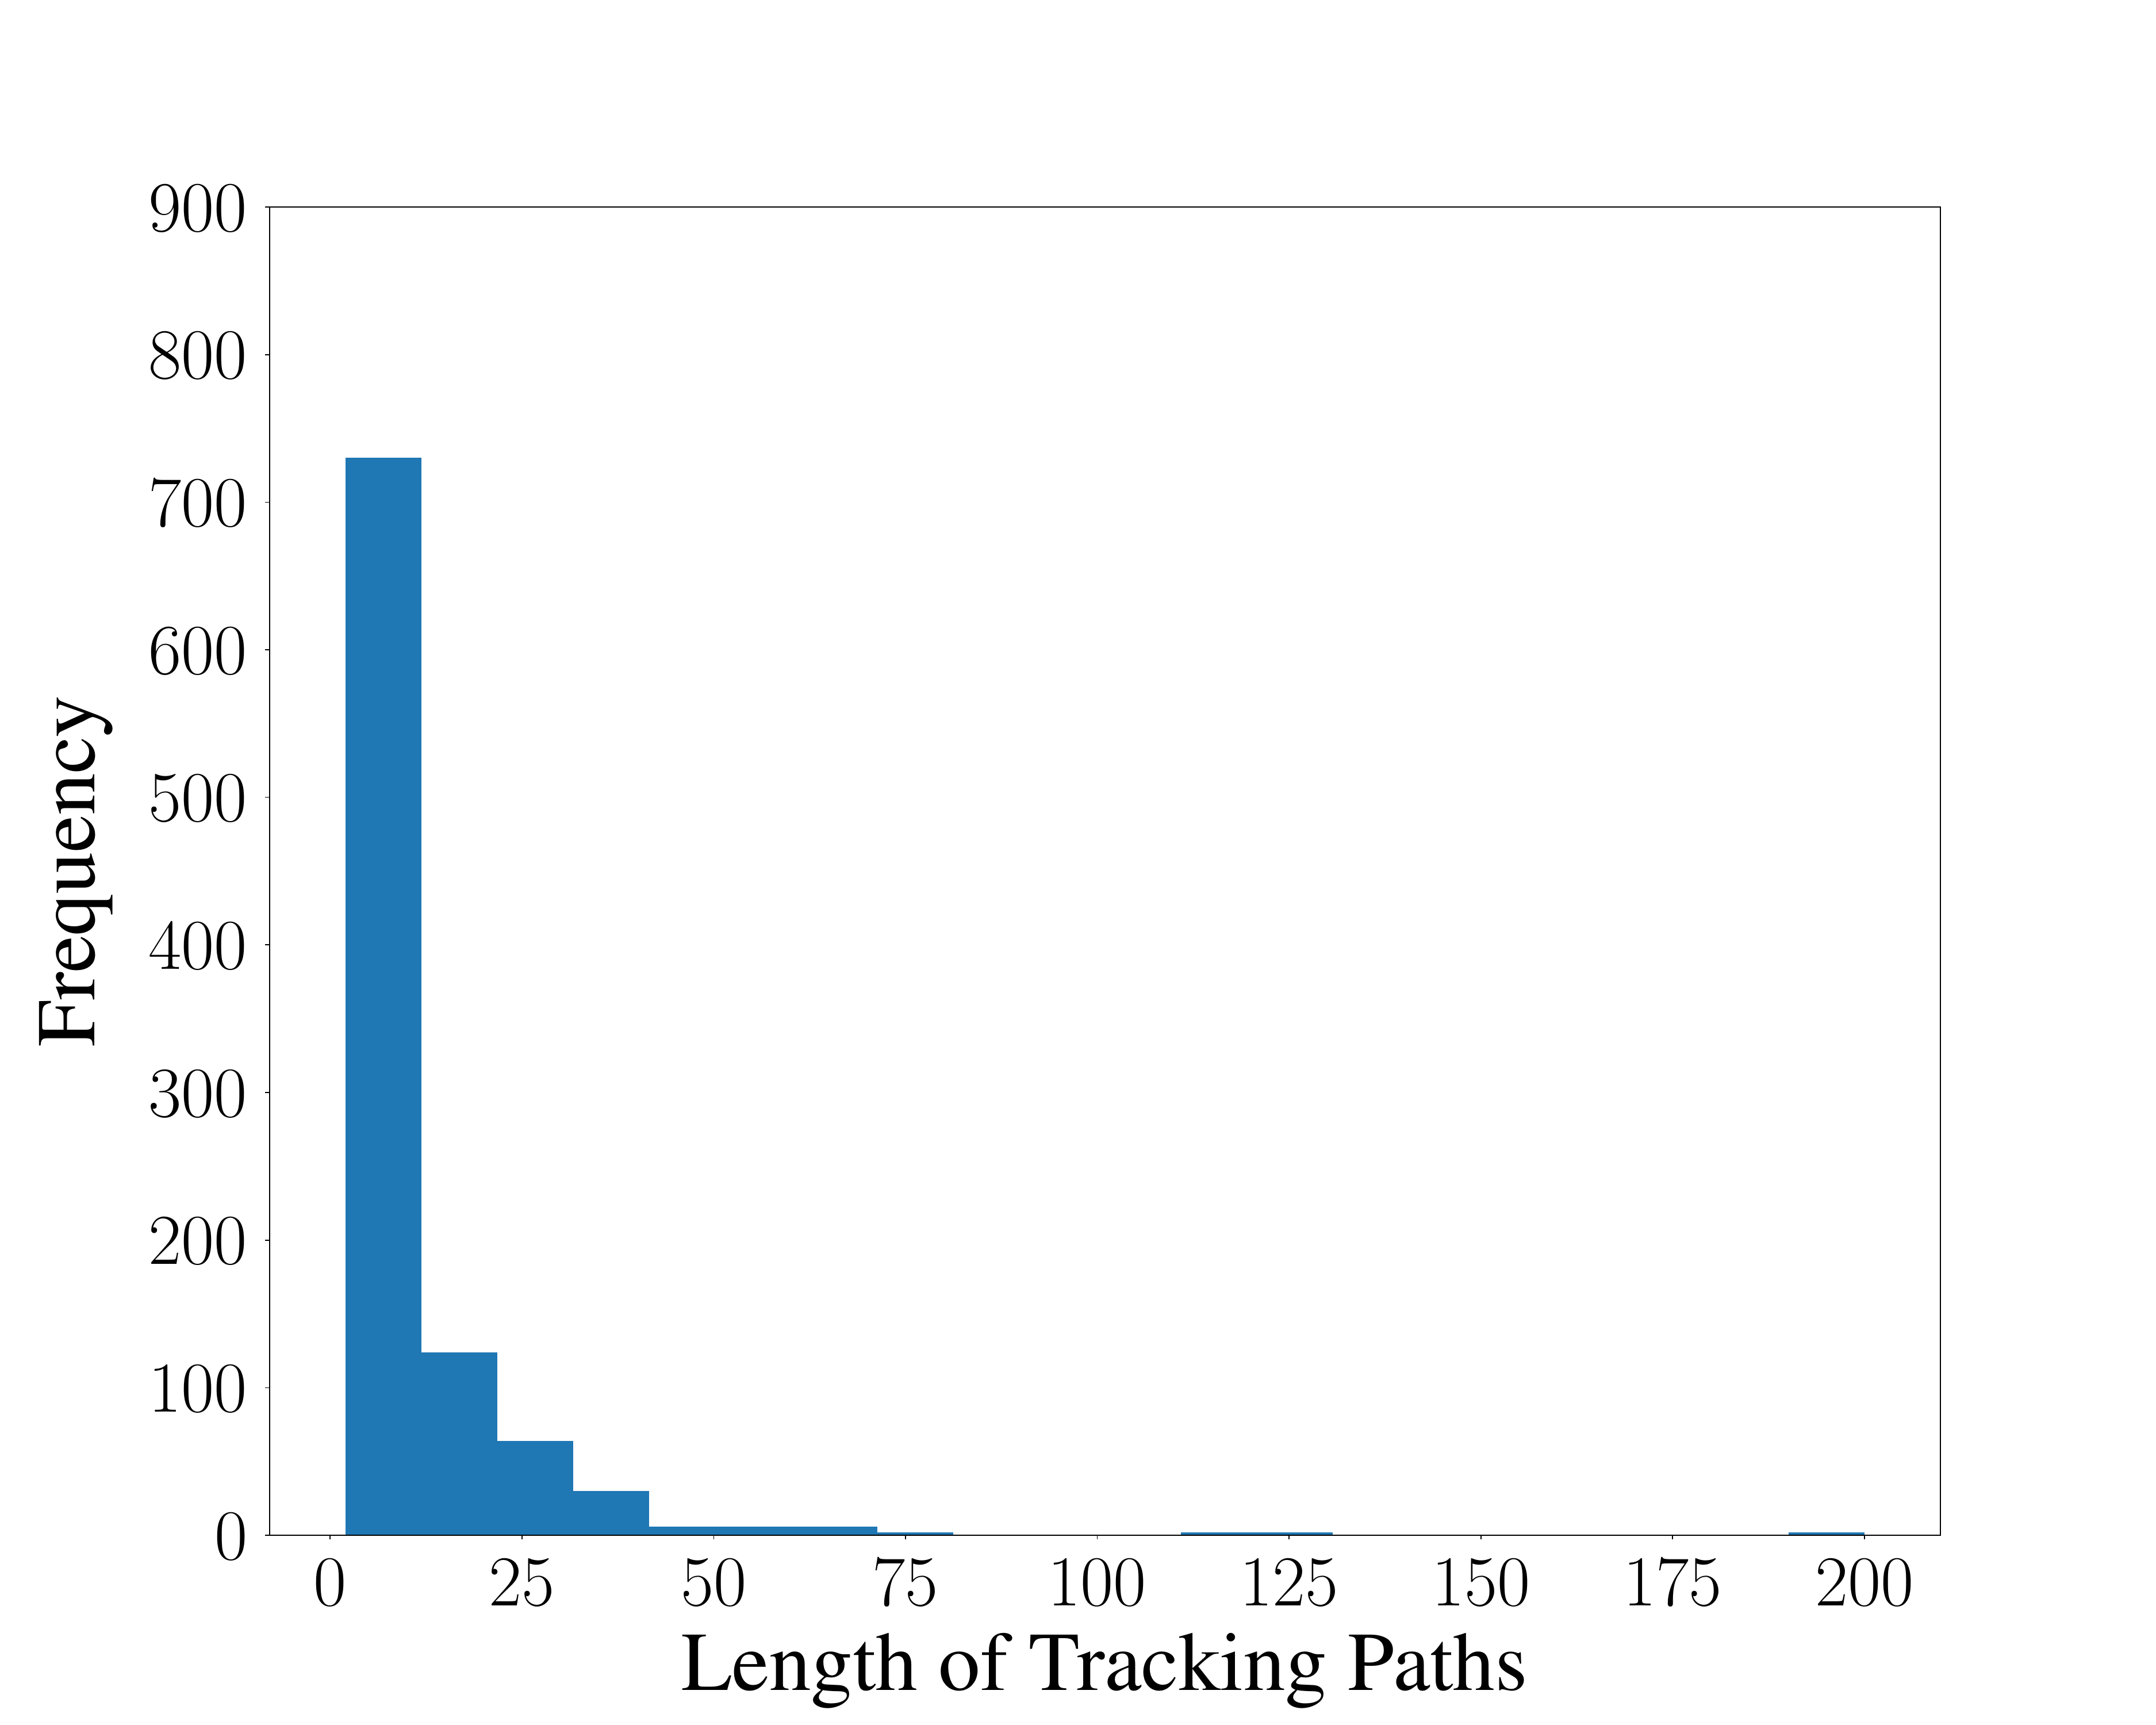}
\caption{$d_w$.}%
\label{fig-LengthHistogramTangaroa3DW}%
\end{subfigure}
\hfill%
\begin{subfigure}[t]{\ltwopicwidth}%
\includegraphics[width=\ltwopicwidth]{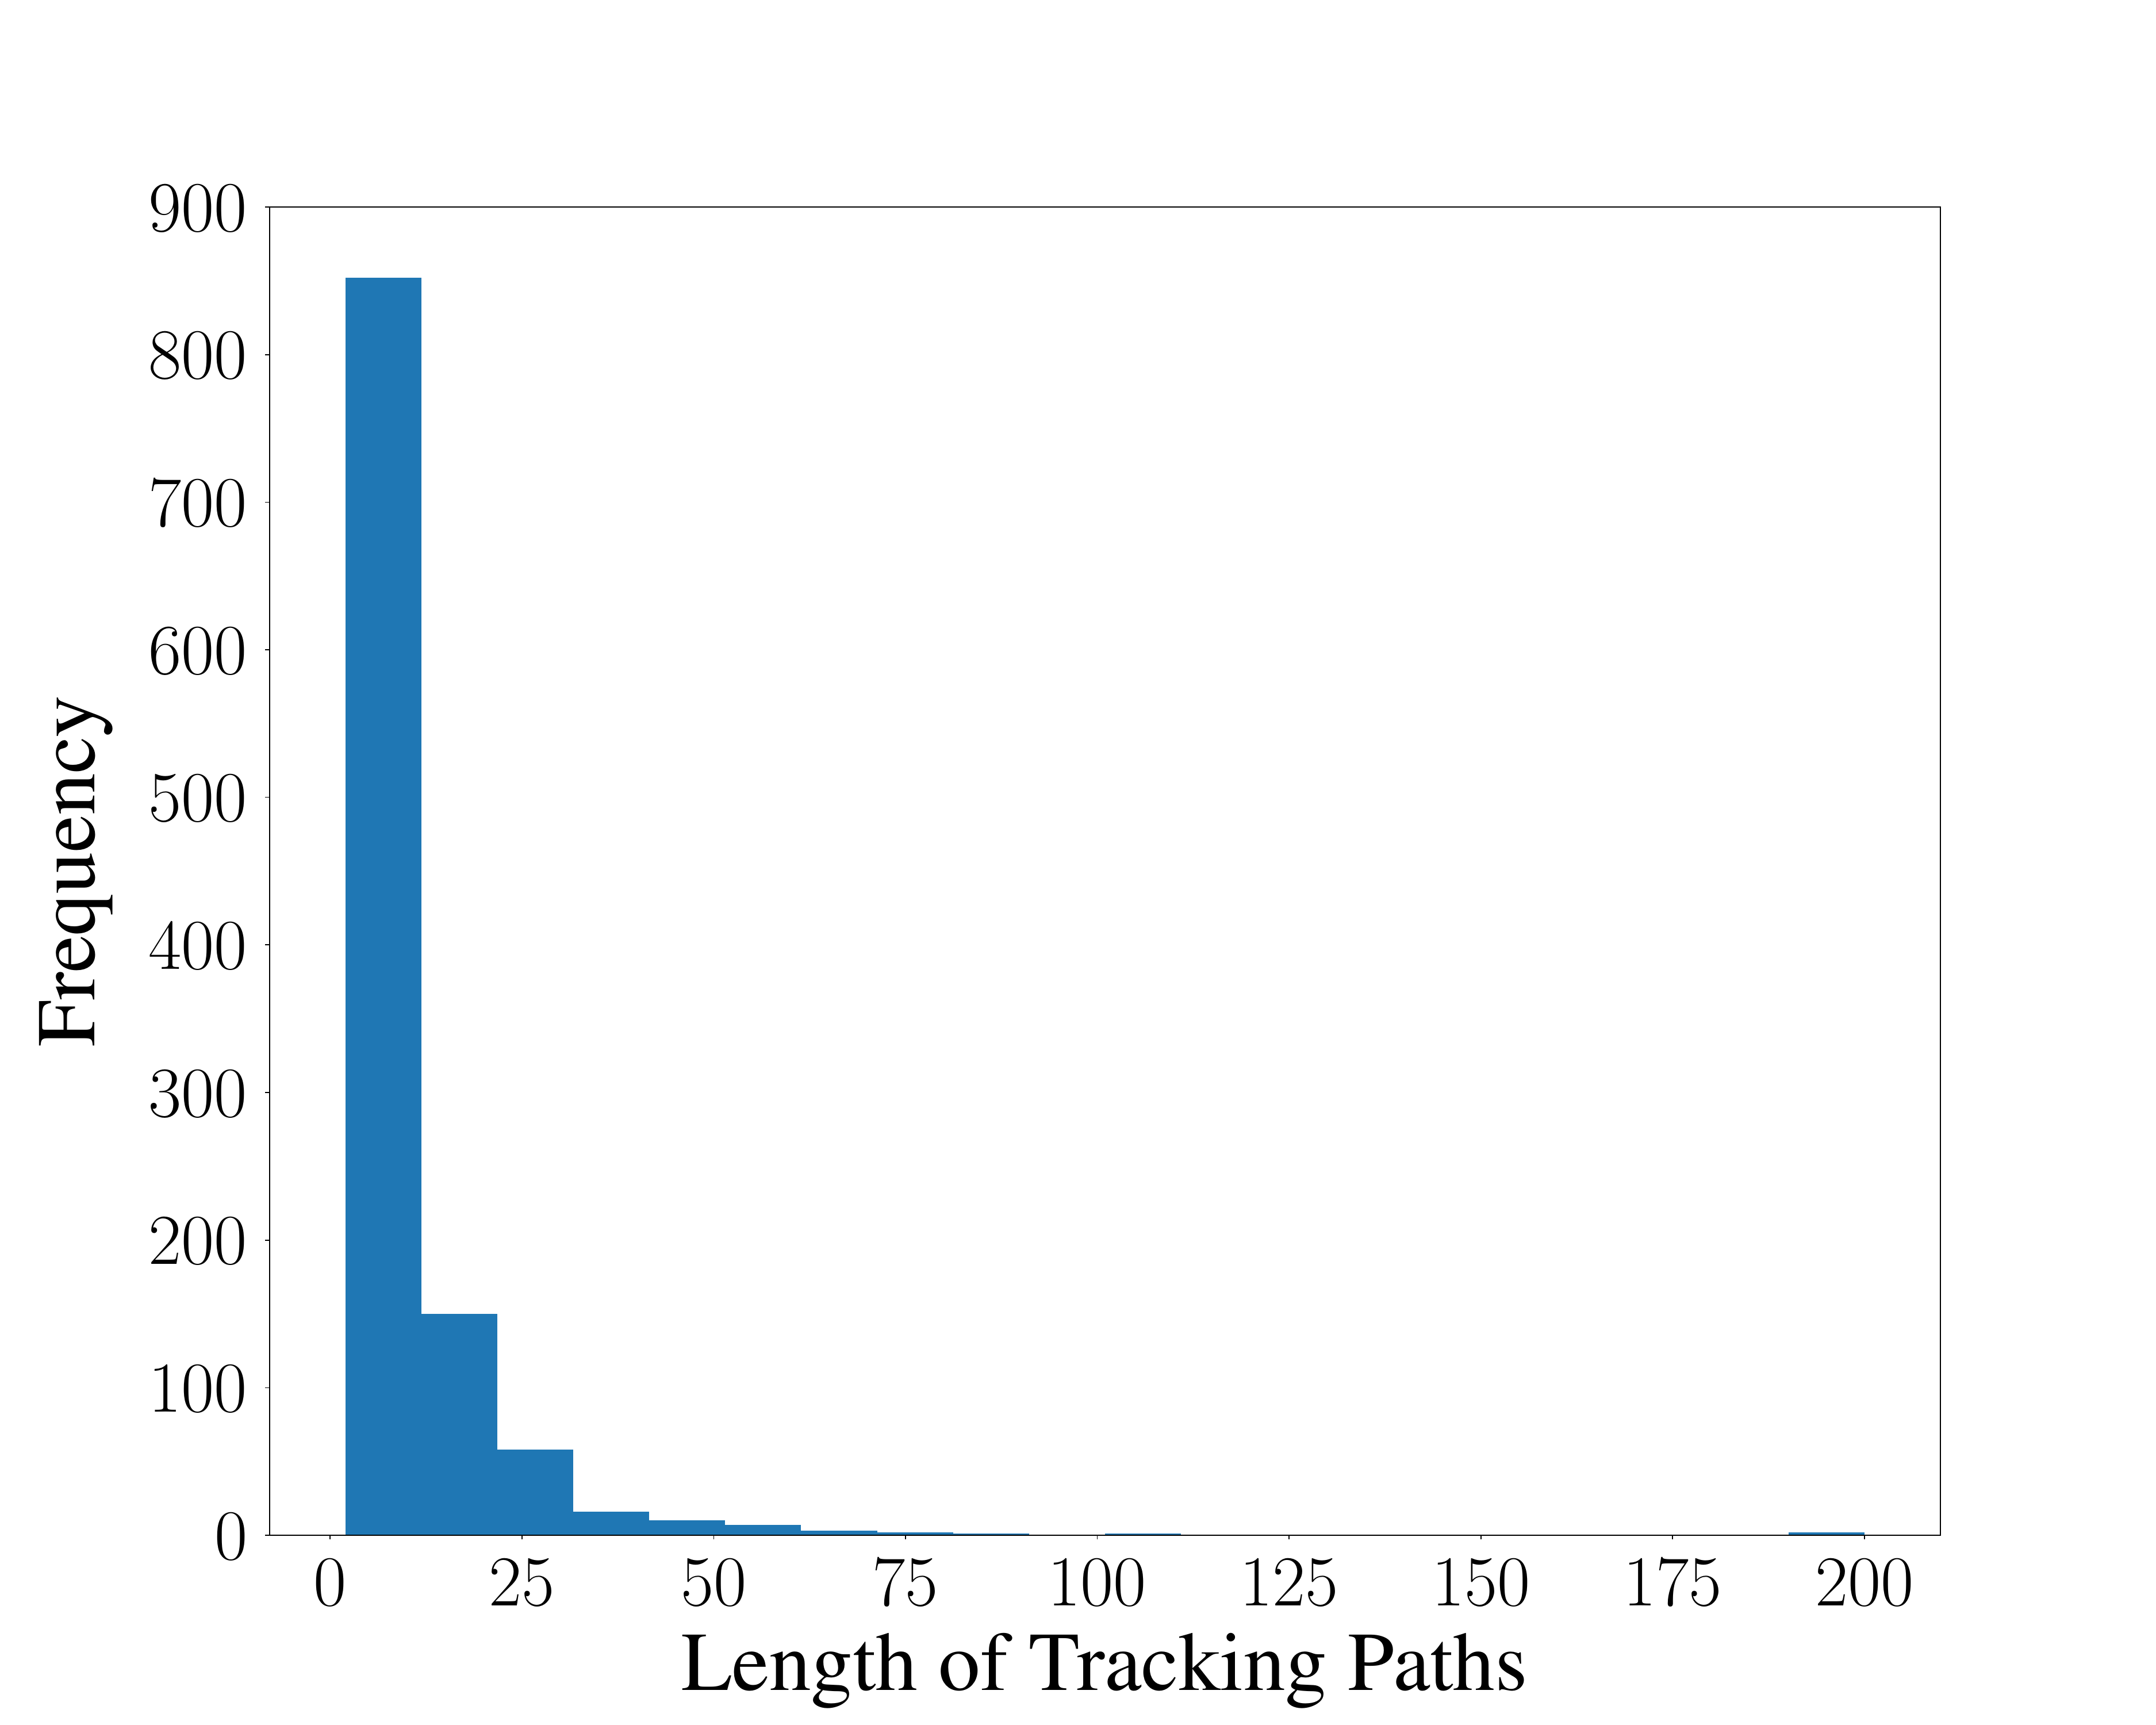}%
\caption{$d_e$.}%
\label{fig-LengthHistogramTangaroa3DE}%
\end{subfigure}%
\\%
\begin{subfigure}[t]{\ltwopicwidth}%
\includegraphics[width=\ltwopicwidth]{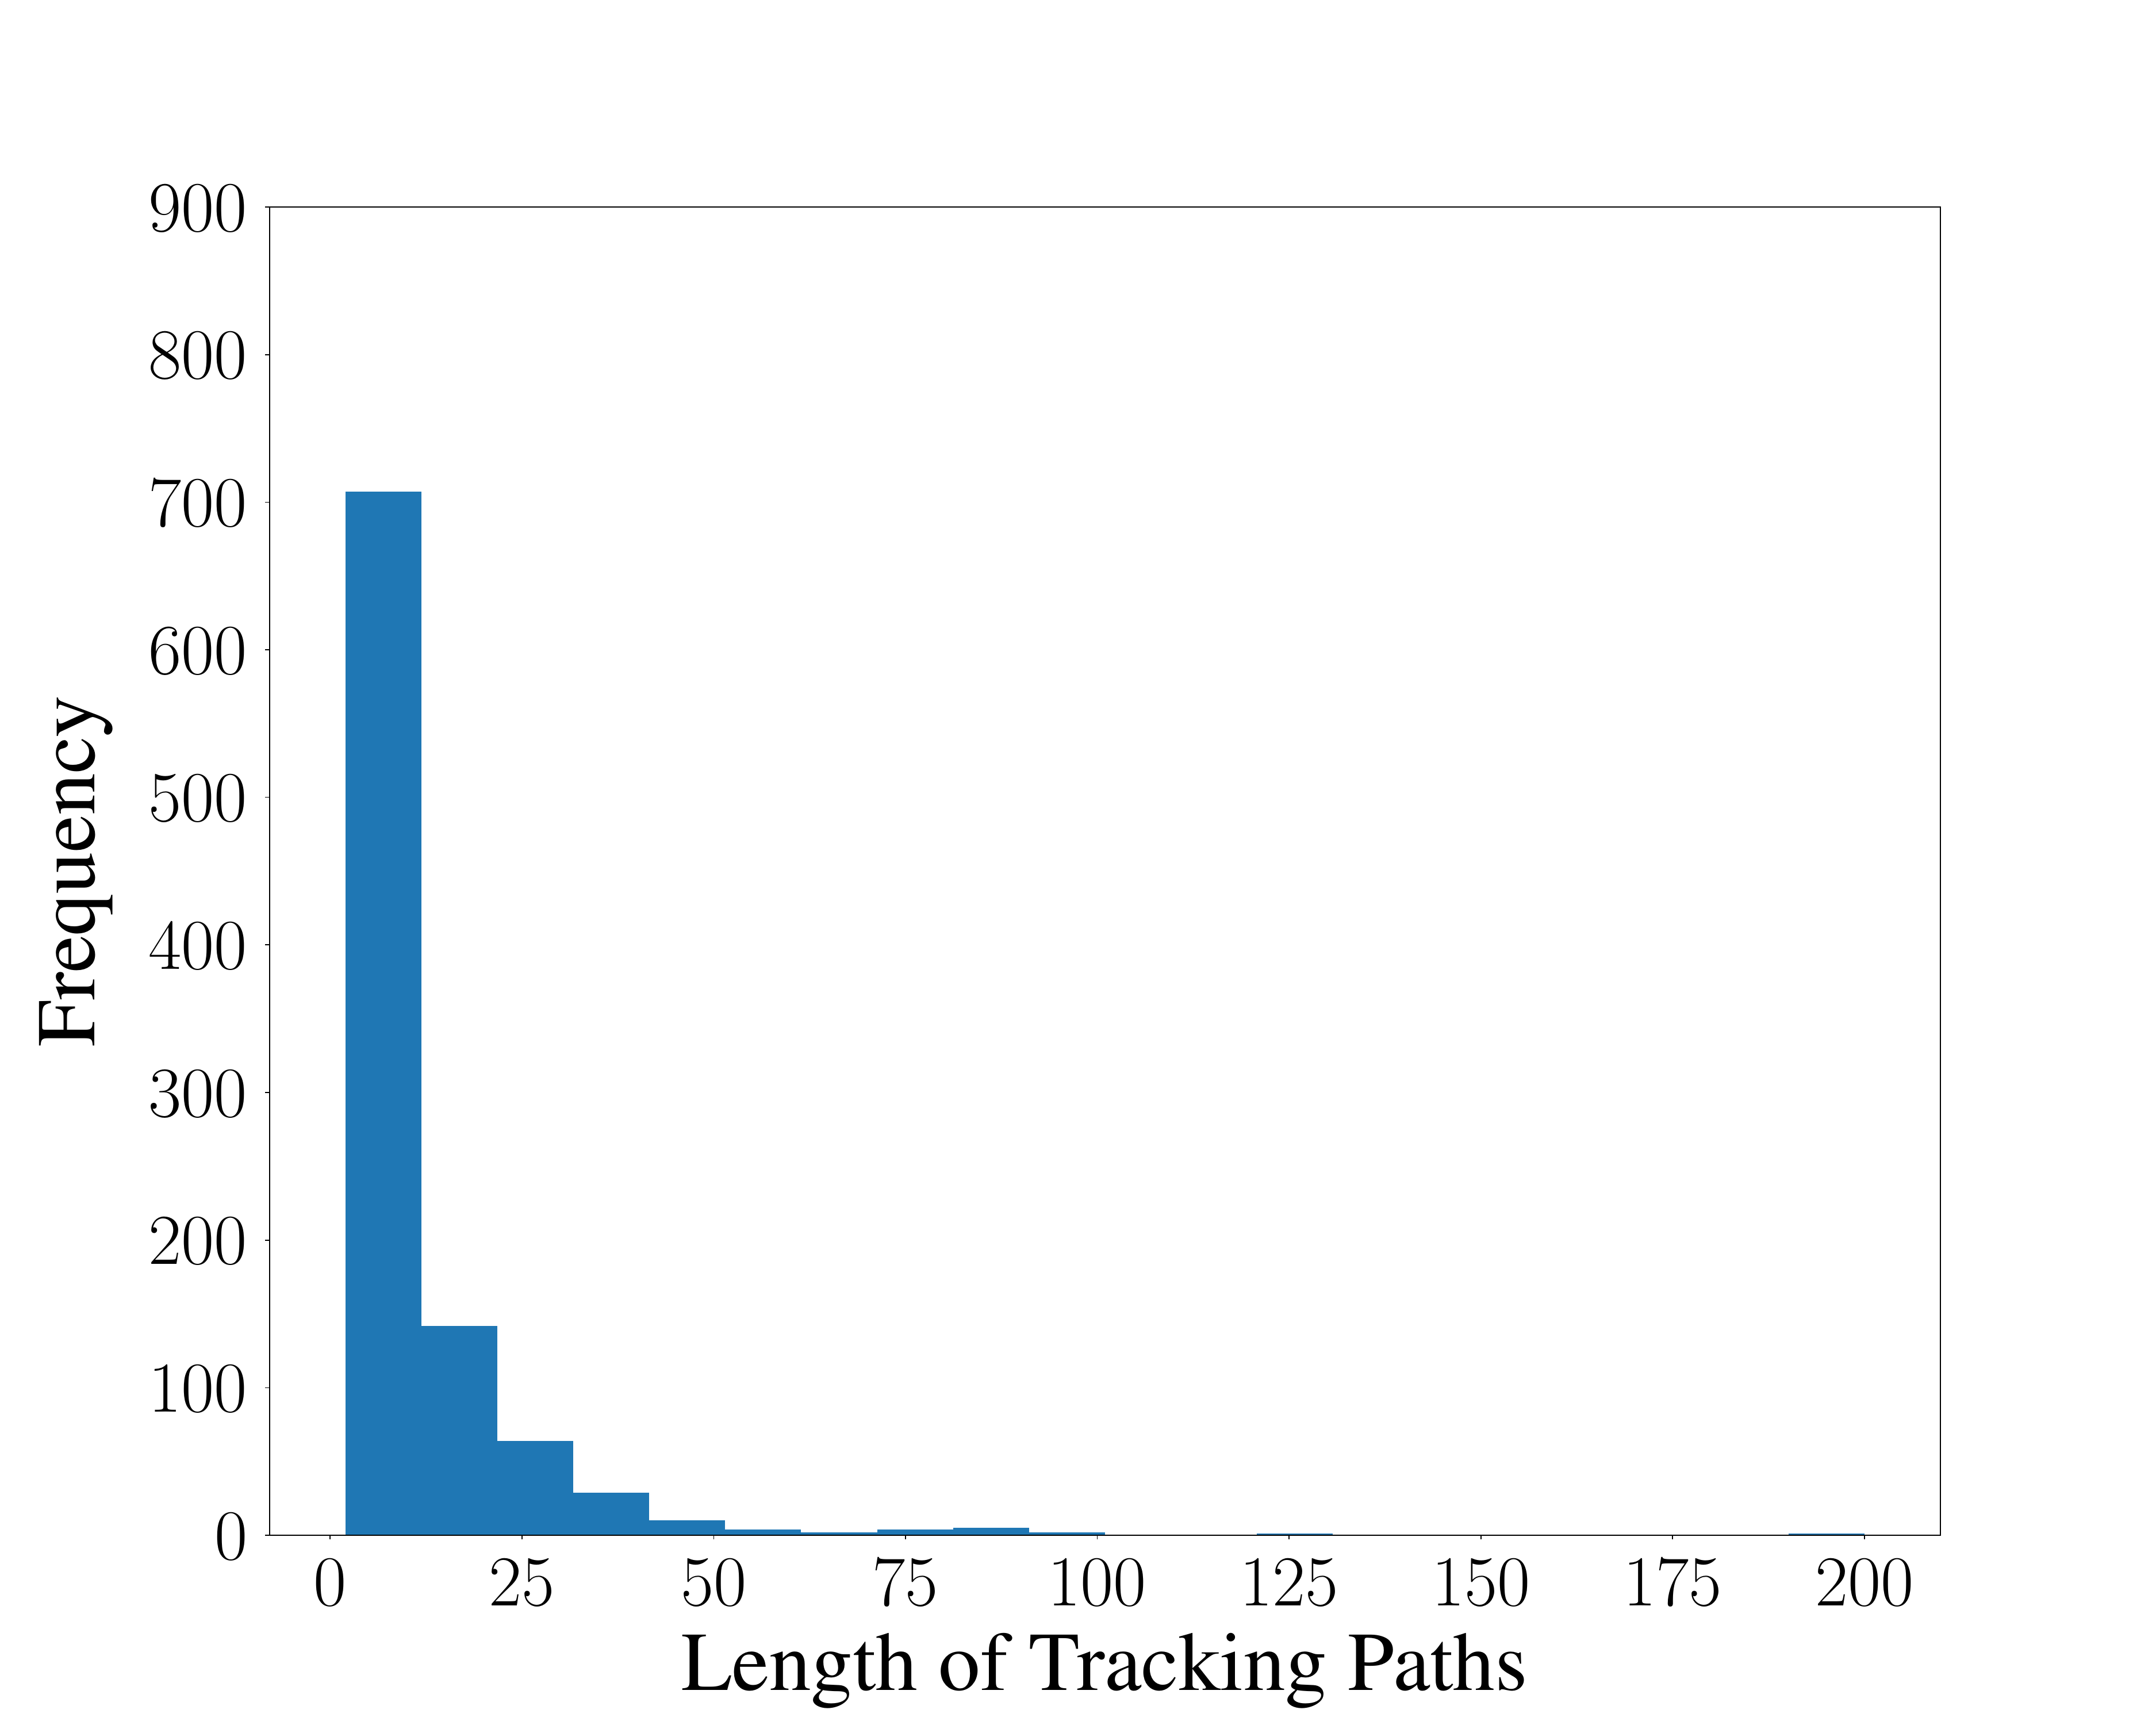}%
\caption{$d_b$.}%
\label{fig-LengthHistogramTangaroa3DB}%
\end{subfigure}%
\hfill%
\begin{subfigure}[t]{\ltwopicwidth}%
\includegraphics[width=\ltwopicwidth]{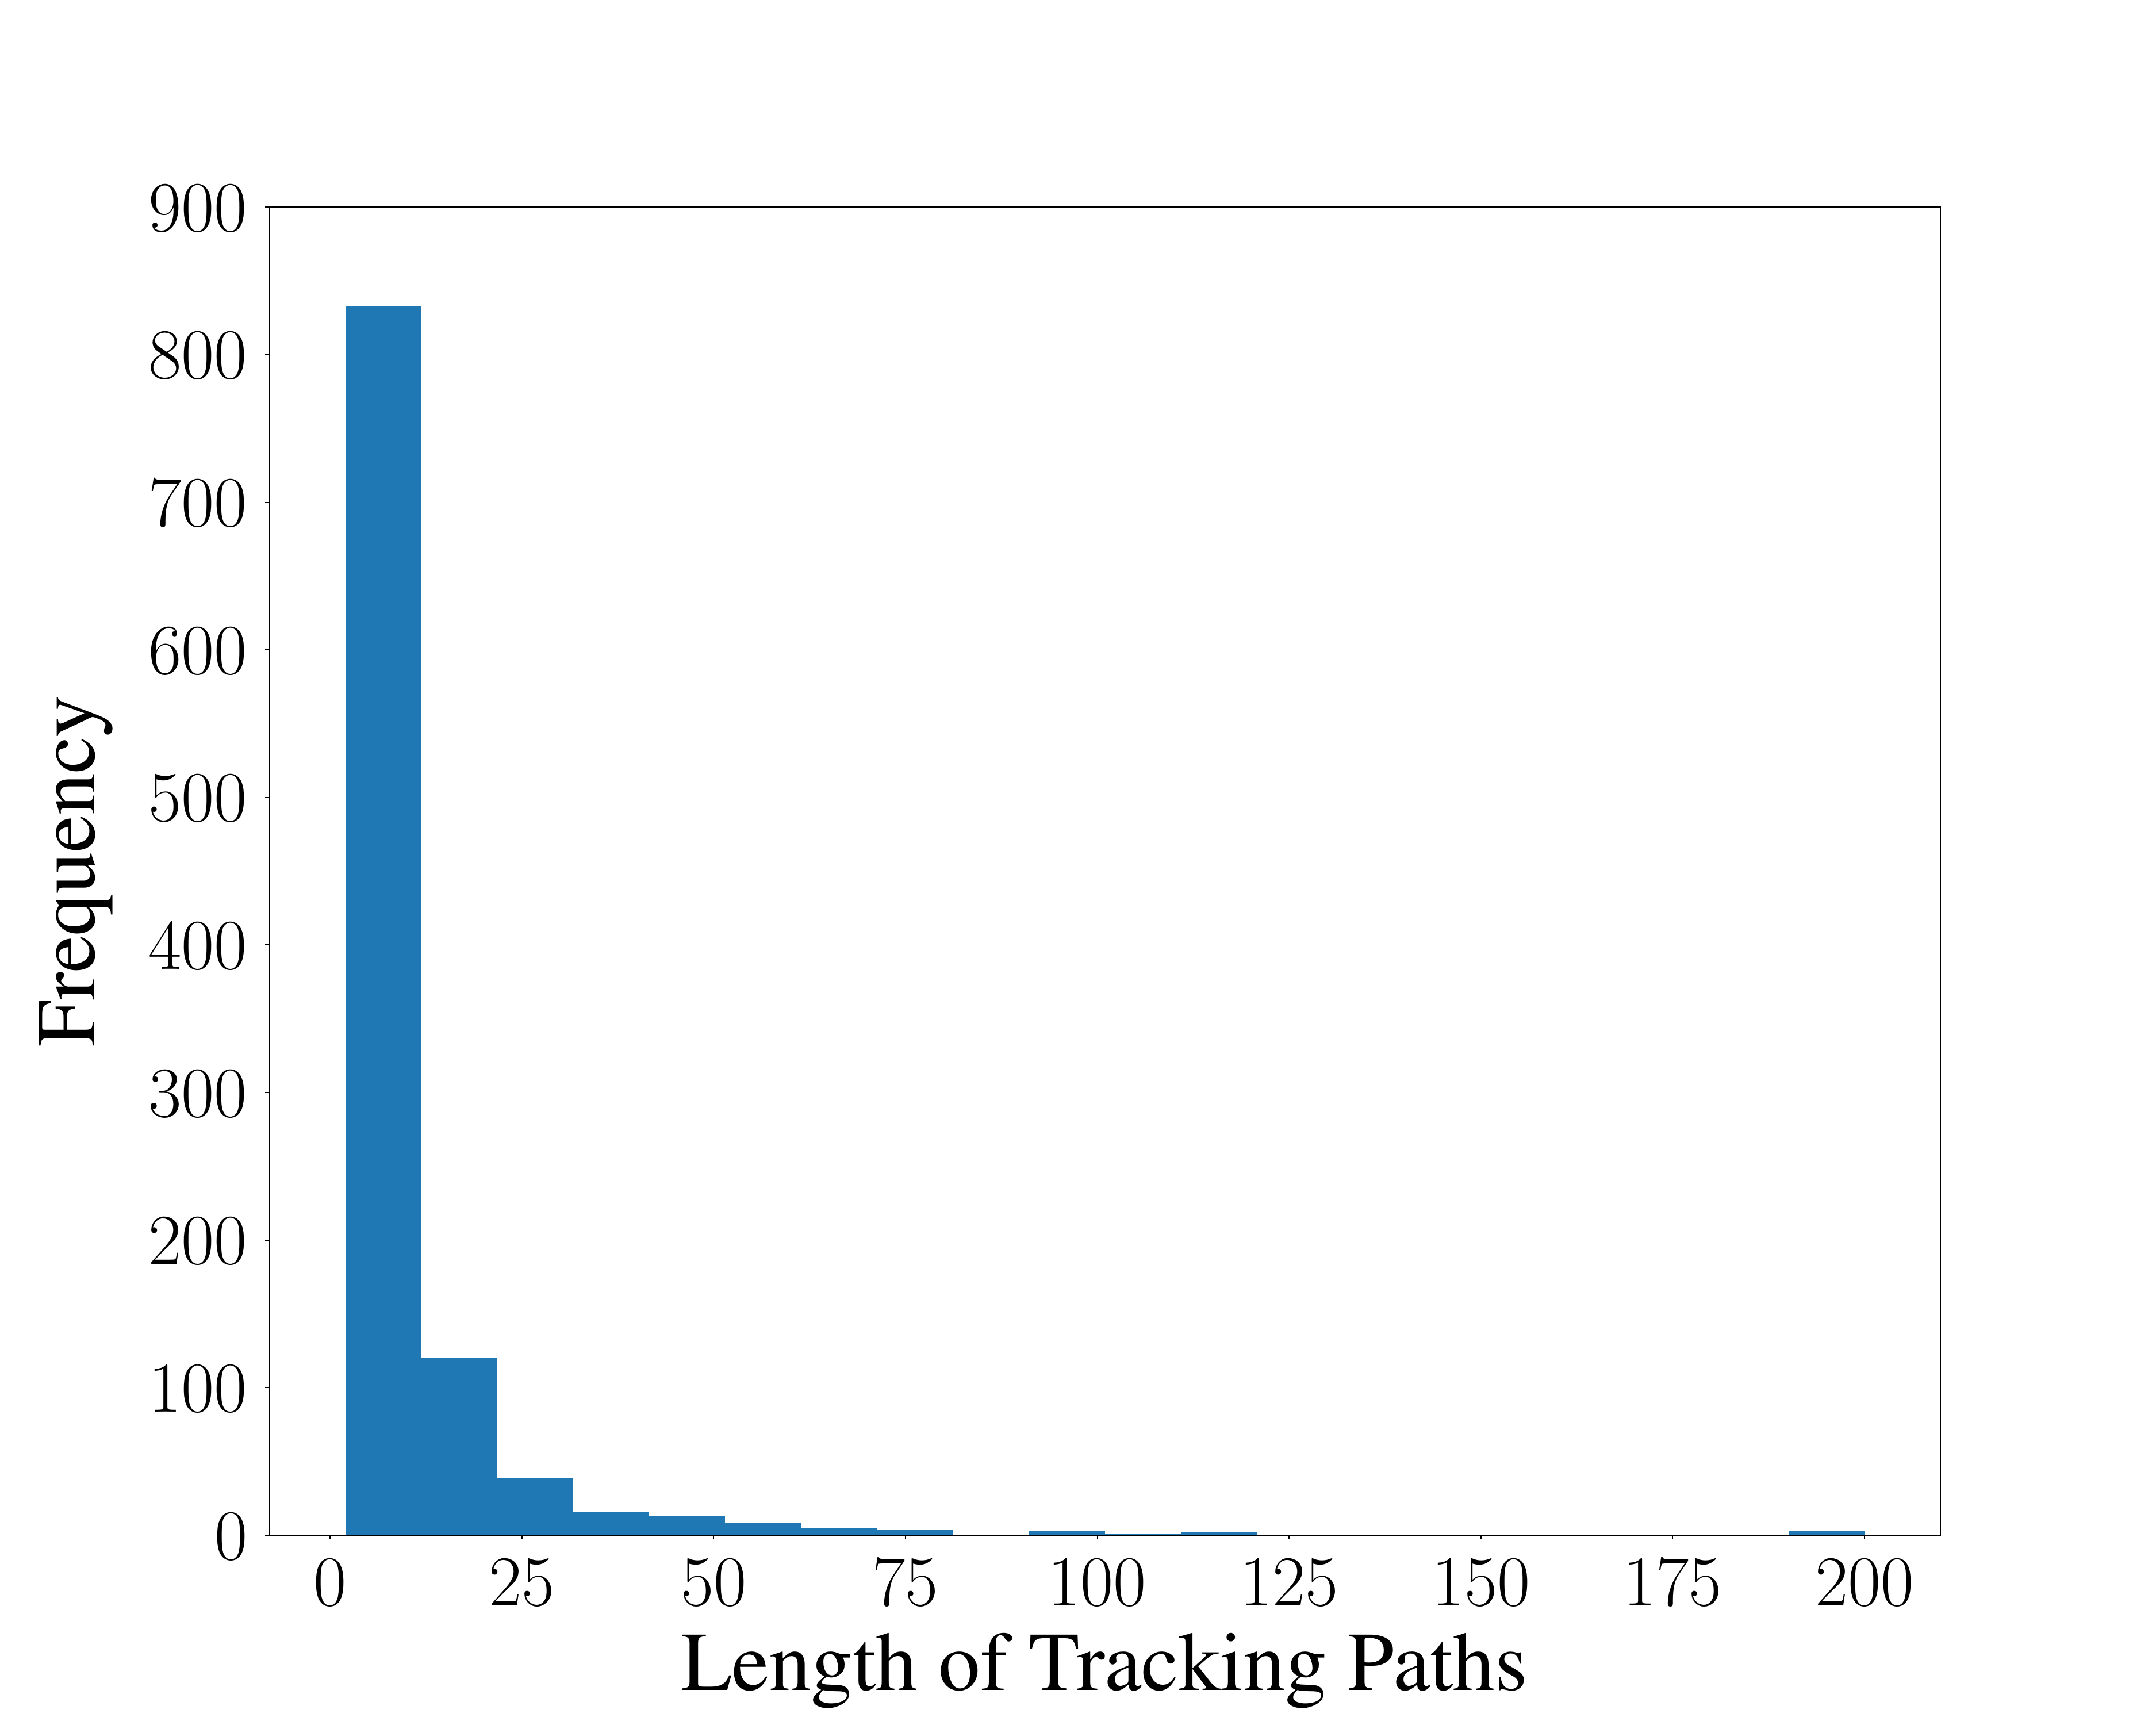}%
\caption{$d_p$.}%
\label{fig-LengthHistogramTangaroa3DP}%
\end{subfigure}%
\caption{Histograms of the length of the tracking paths
    of \dataset{Tangaroa3D}.}%
\label{fig-LengthHisgoramTangaroa3D}%
\end{figure}

\begin{figure}
\centering
\includegraphics[width=0.8\linewidth]{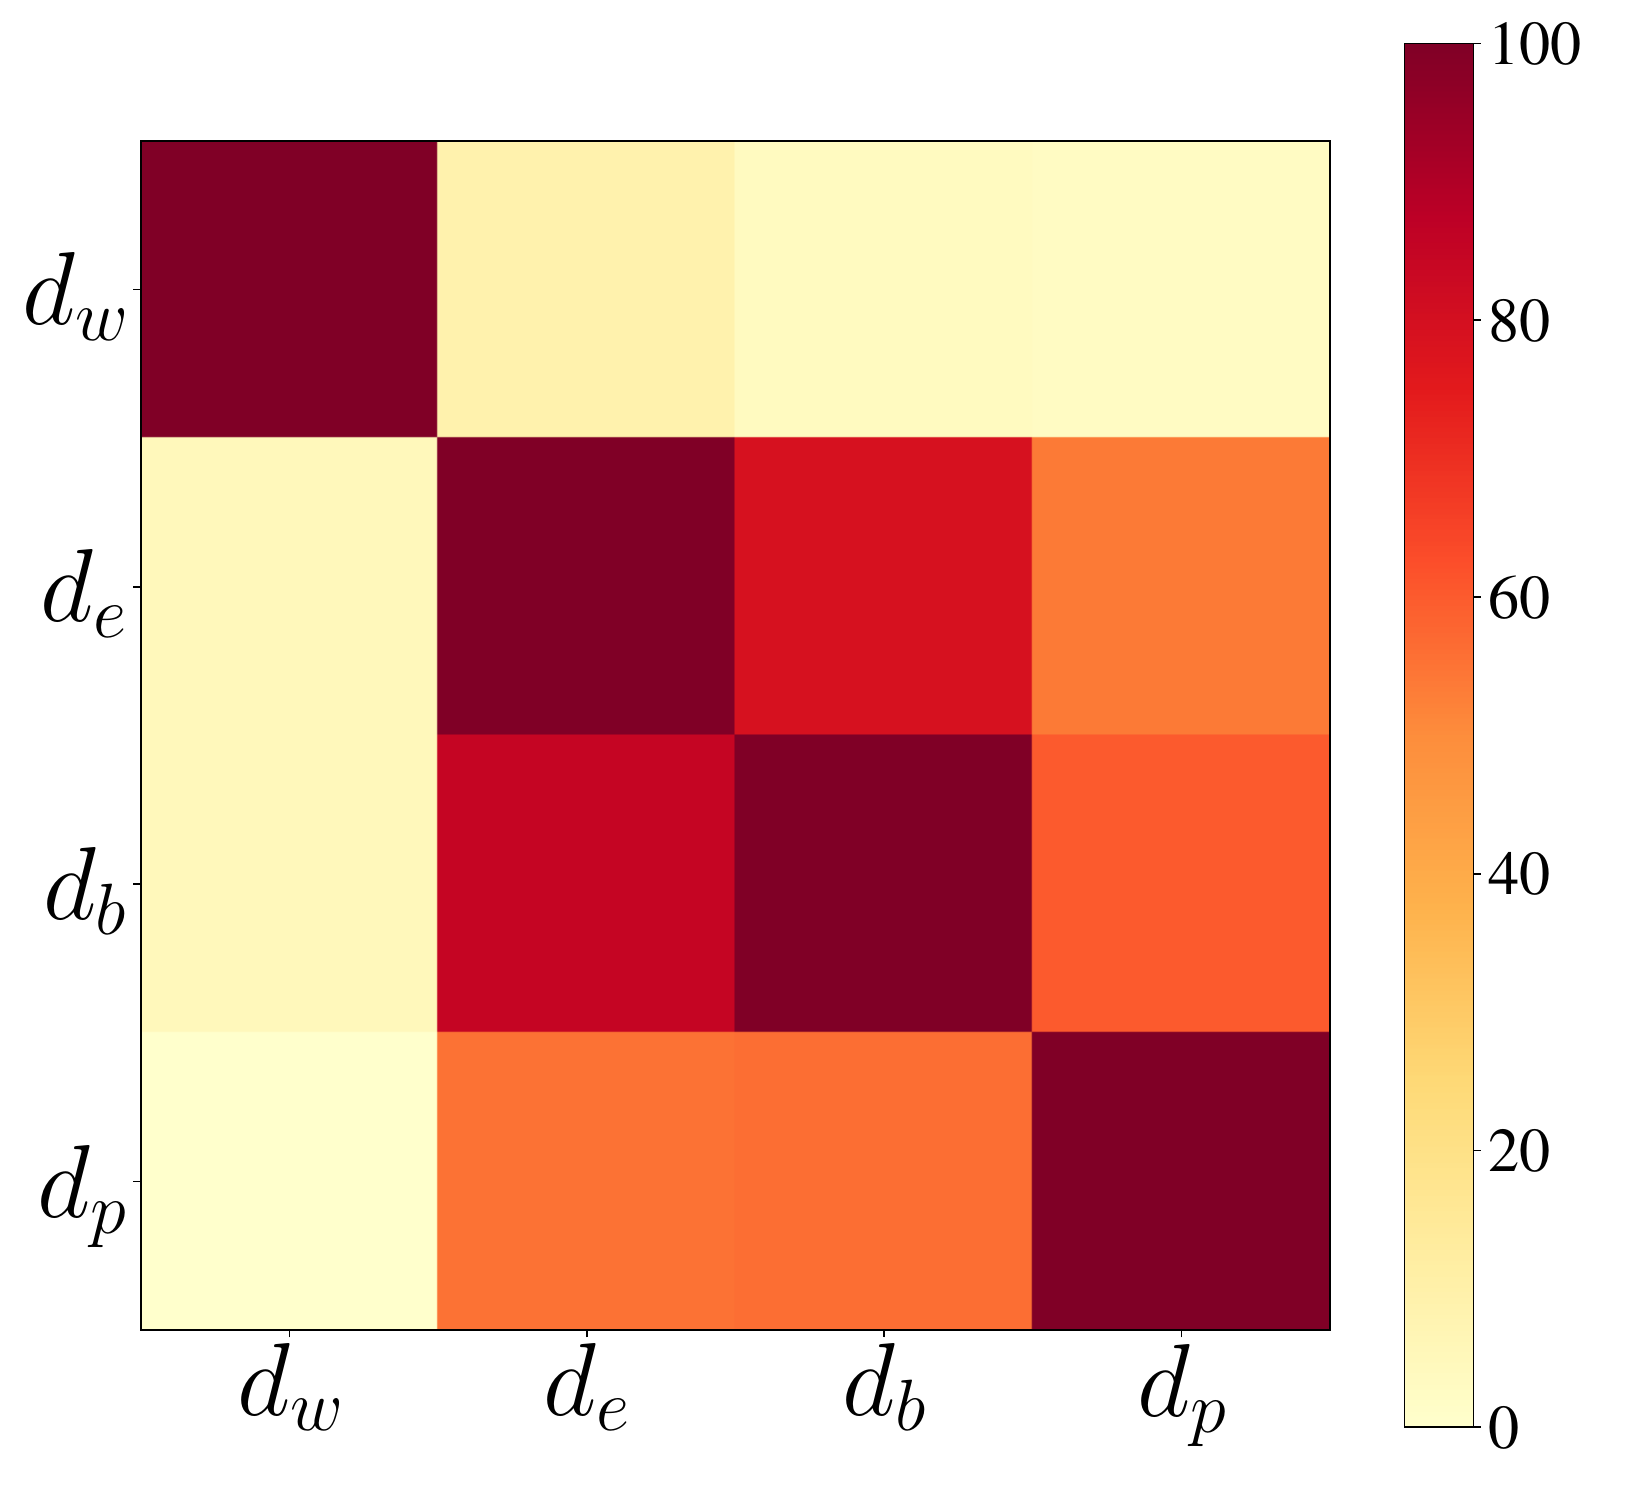}
\caption{
    Pairwise differences between the methods on the columns
    in relation to the methods on the rows
    for \dataset{Tangaroa3D}.
}
\label{fig-Tangaroa3DSimilarities}
\end{figure}

\subsection*{Extra results with Cylinder2D data set}
More results of the experiments using \dataset{Cylinder2D}
are shown in \Cref{fig-Cylinder2DAllNodesLong}
through \Cref{fig-LengthHisgoramCylinder2DLong}.

\begin{figure}
\centering
\includegraphics[width=0.8\linewidth]{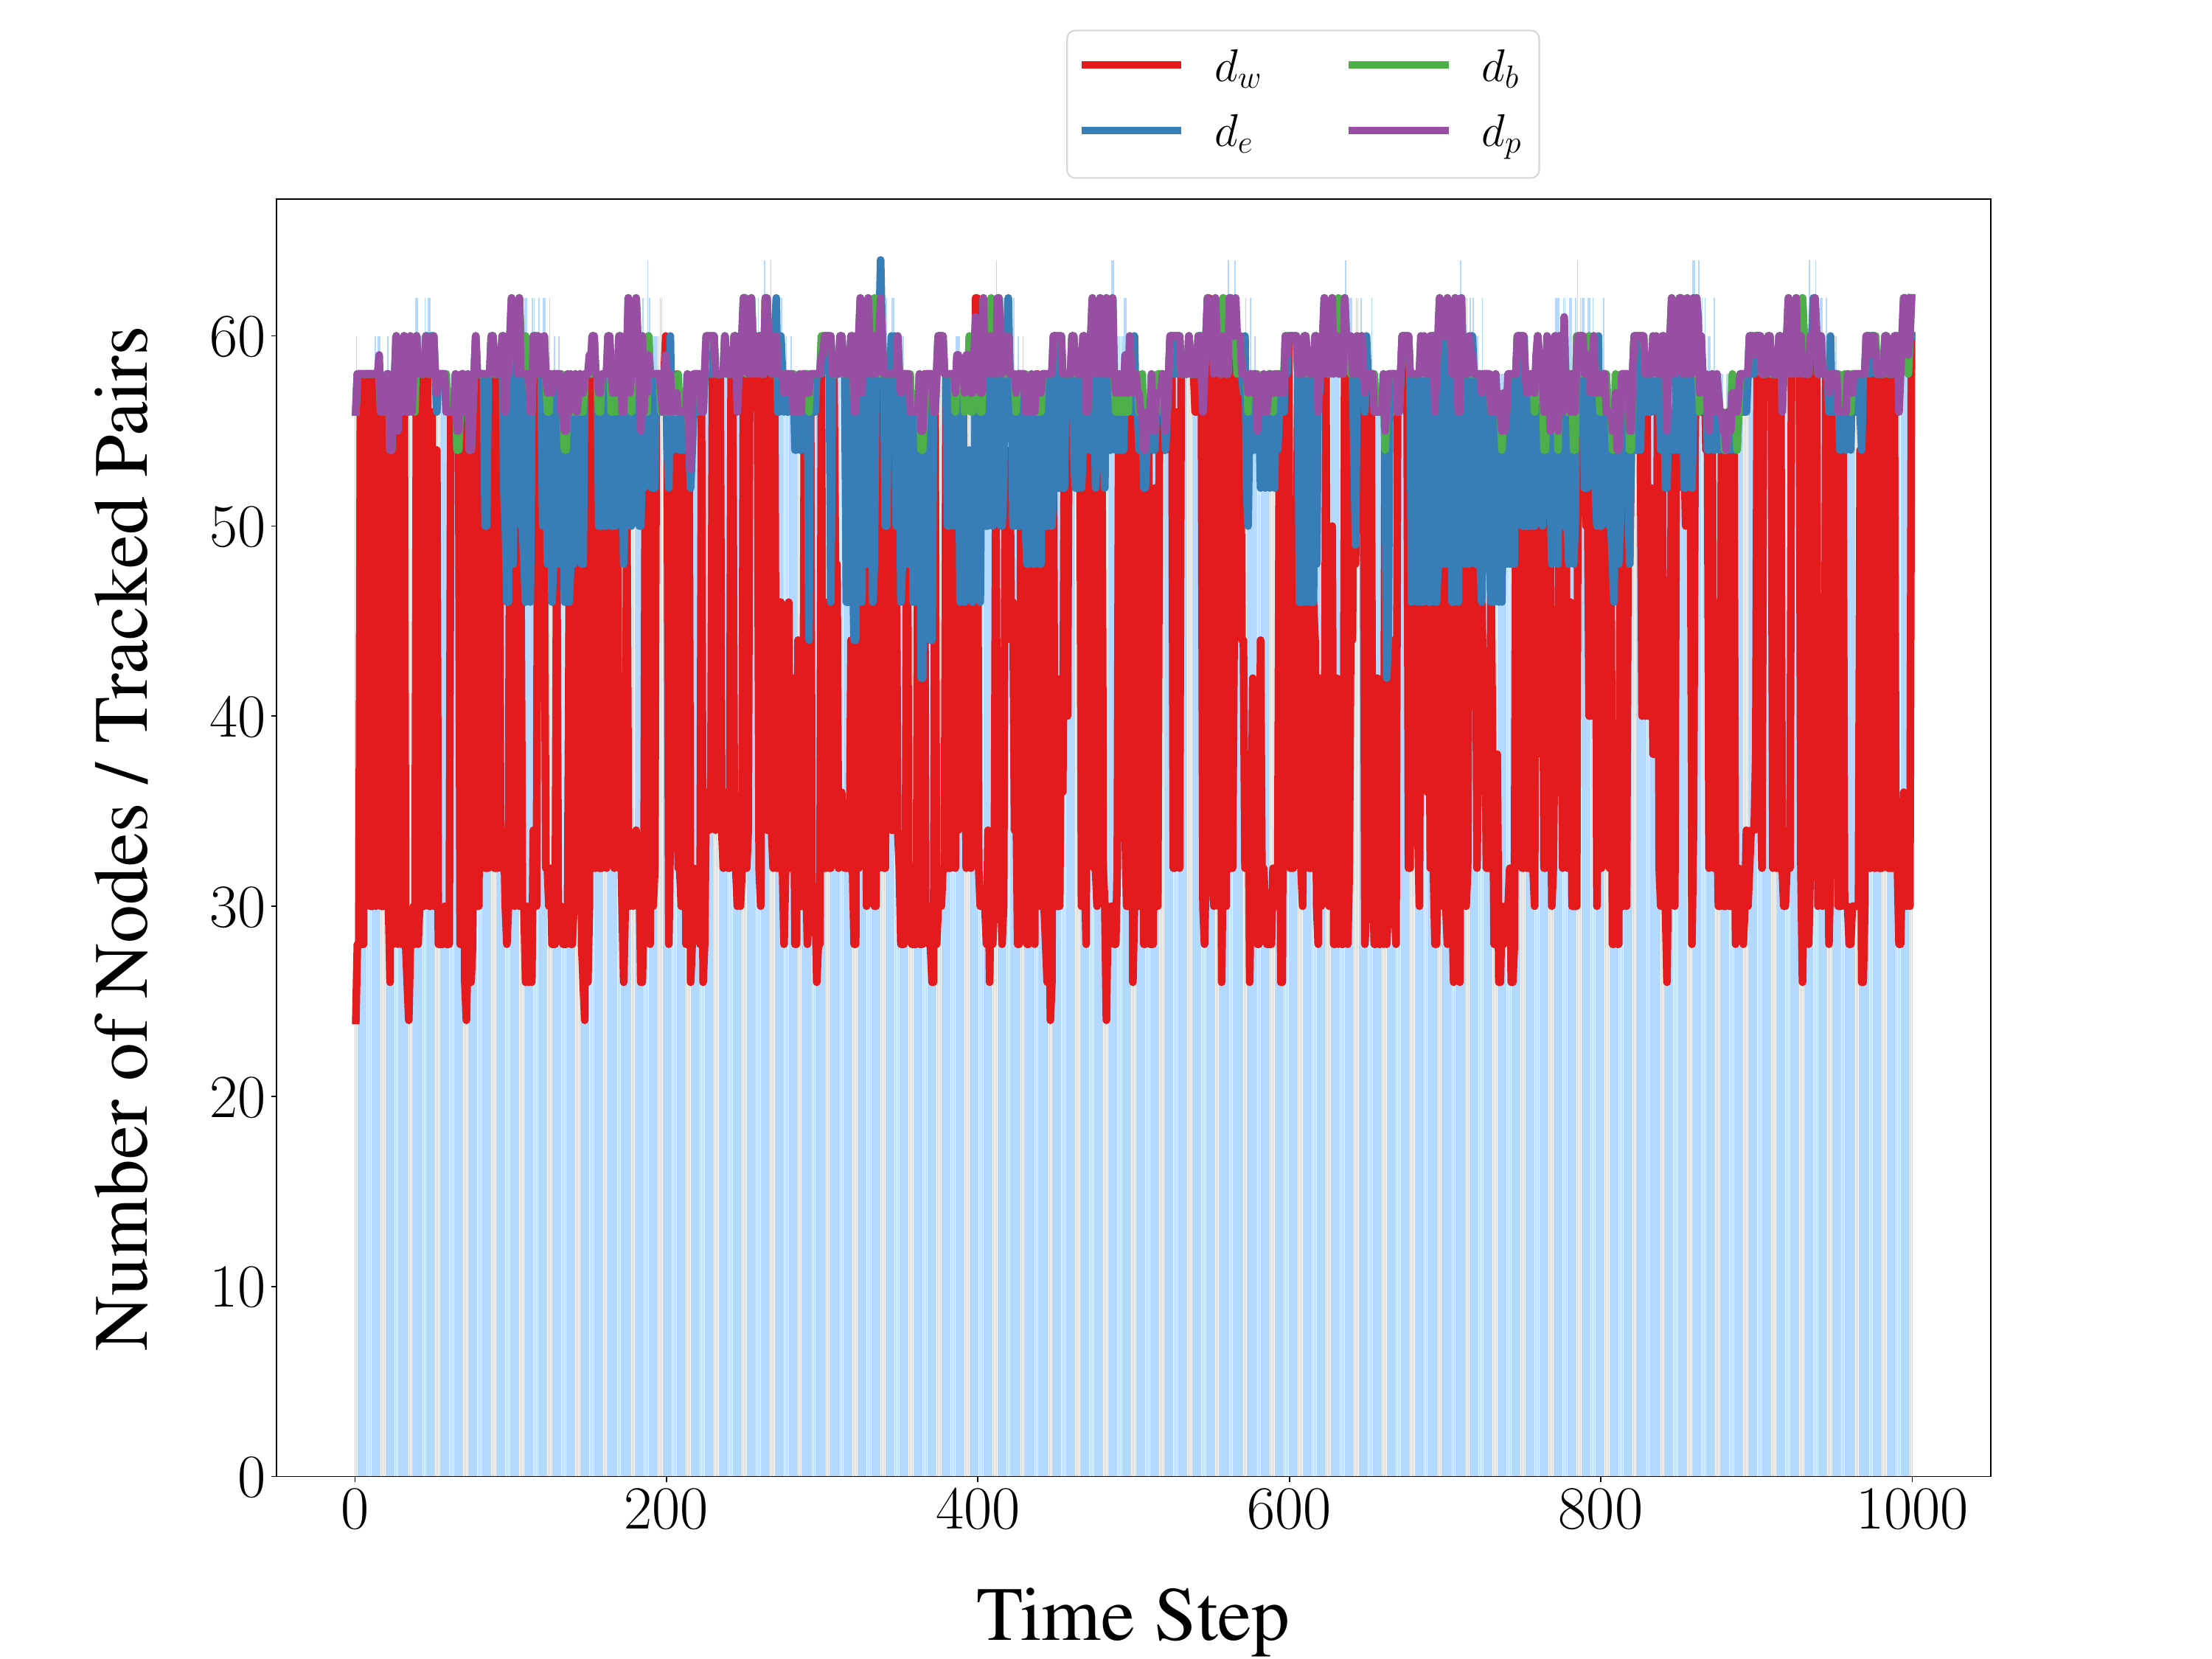}
\caption{
    Number of tracked nodes (colored and labeled) 
    relative to the total nodes of merge trees (light blue bars)
    for \dataset{Cylinder2D}.
}
\label{fig-Cylinder2DAllNodesLong}
\end{figure}

% Length histogram
\begin{figure}%
\begin{subfigure}[t]{\ltwopicwidth}%
\includegraphics[width=\ltwopicwidth]{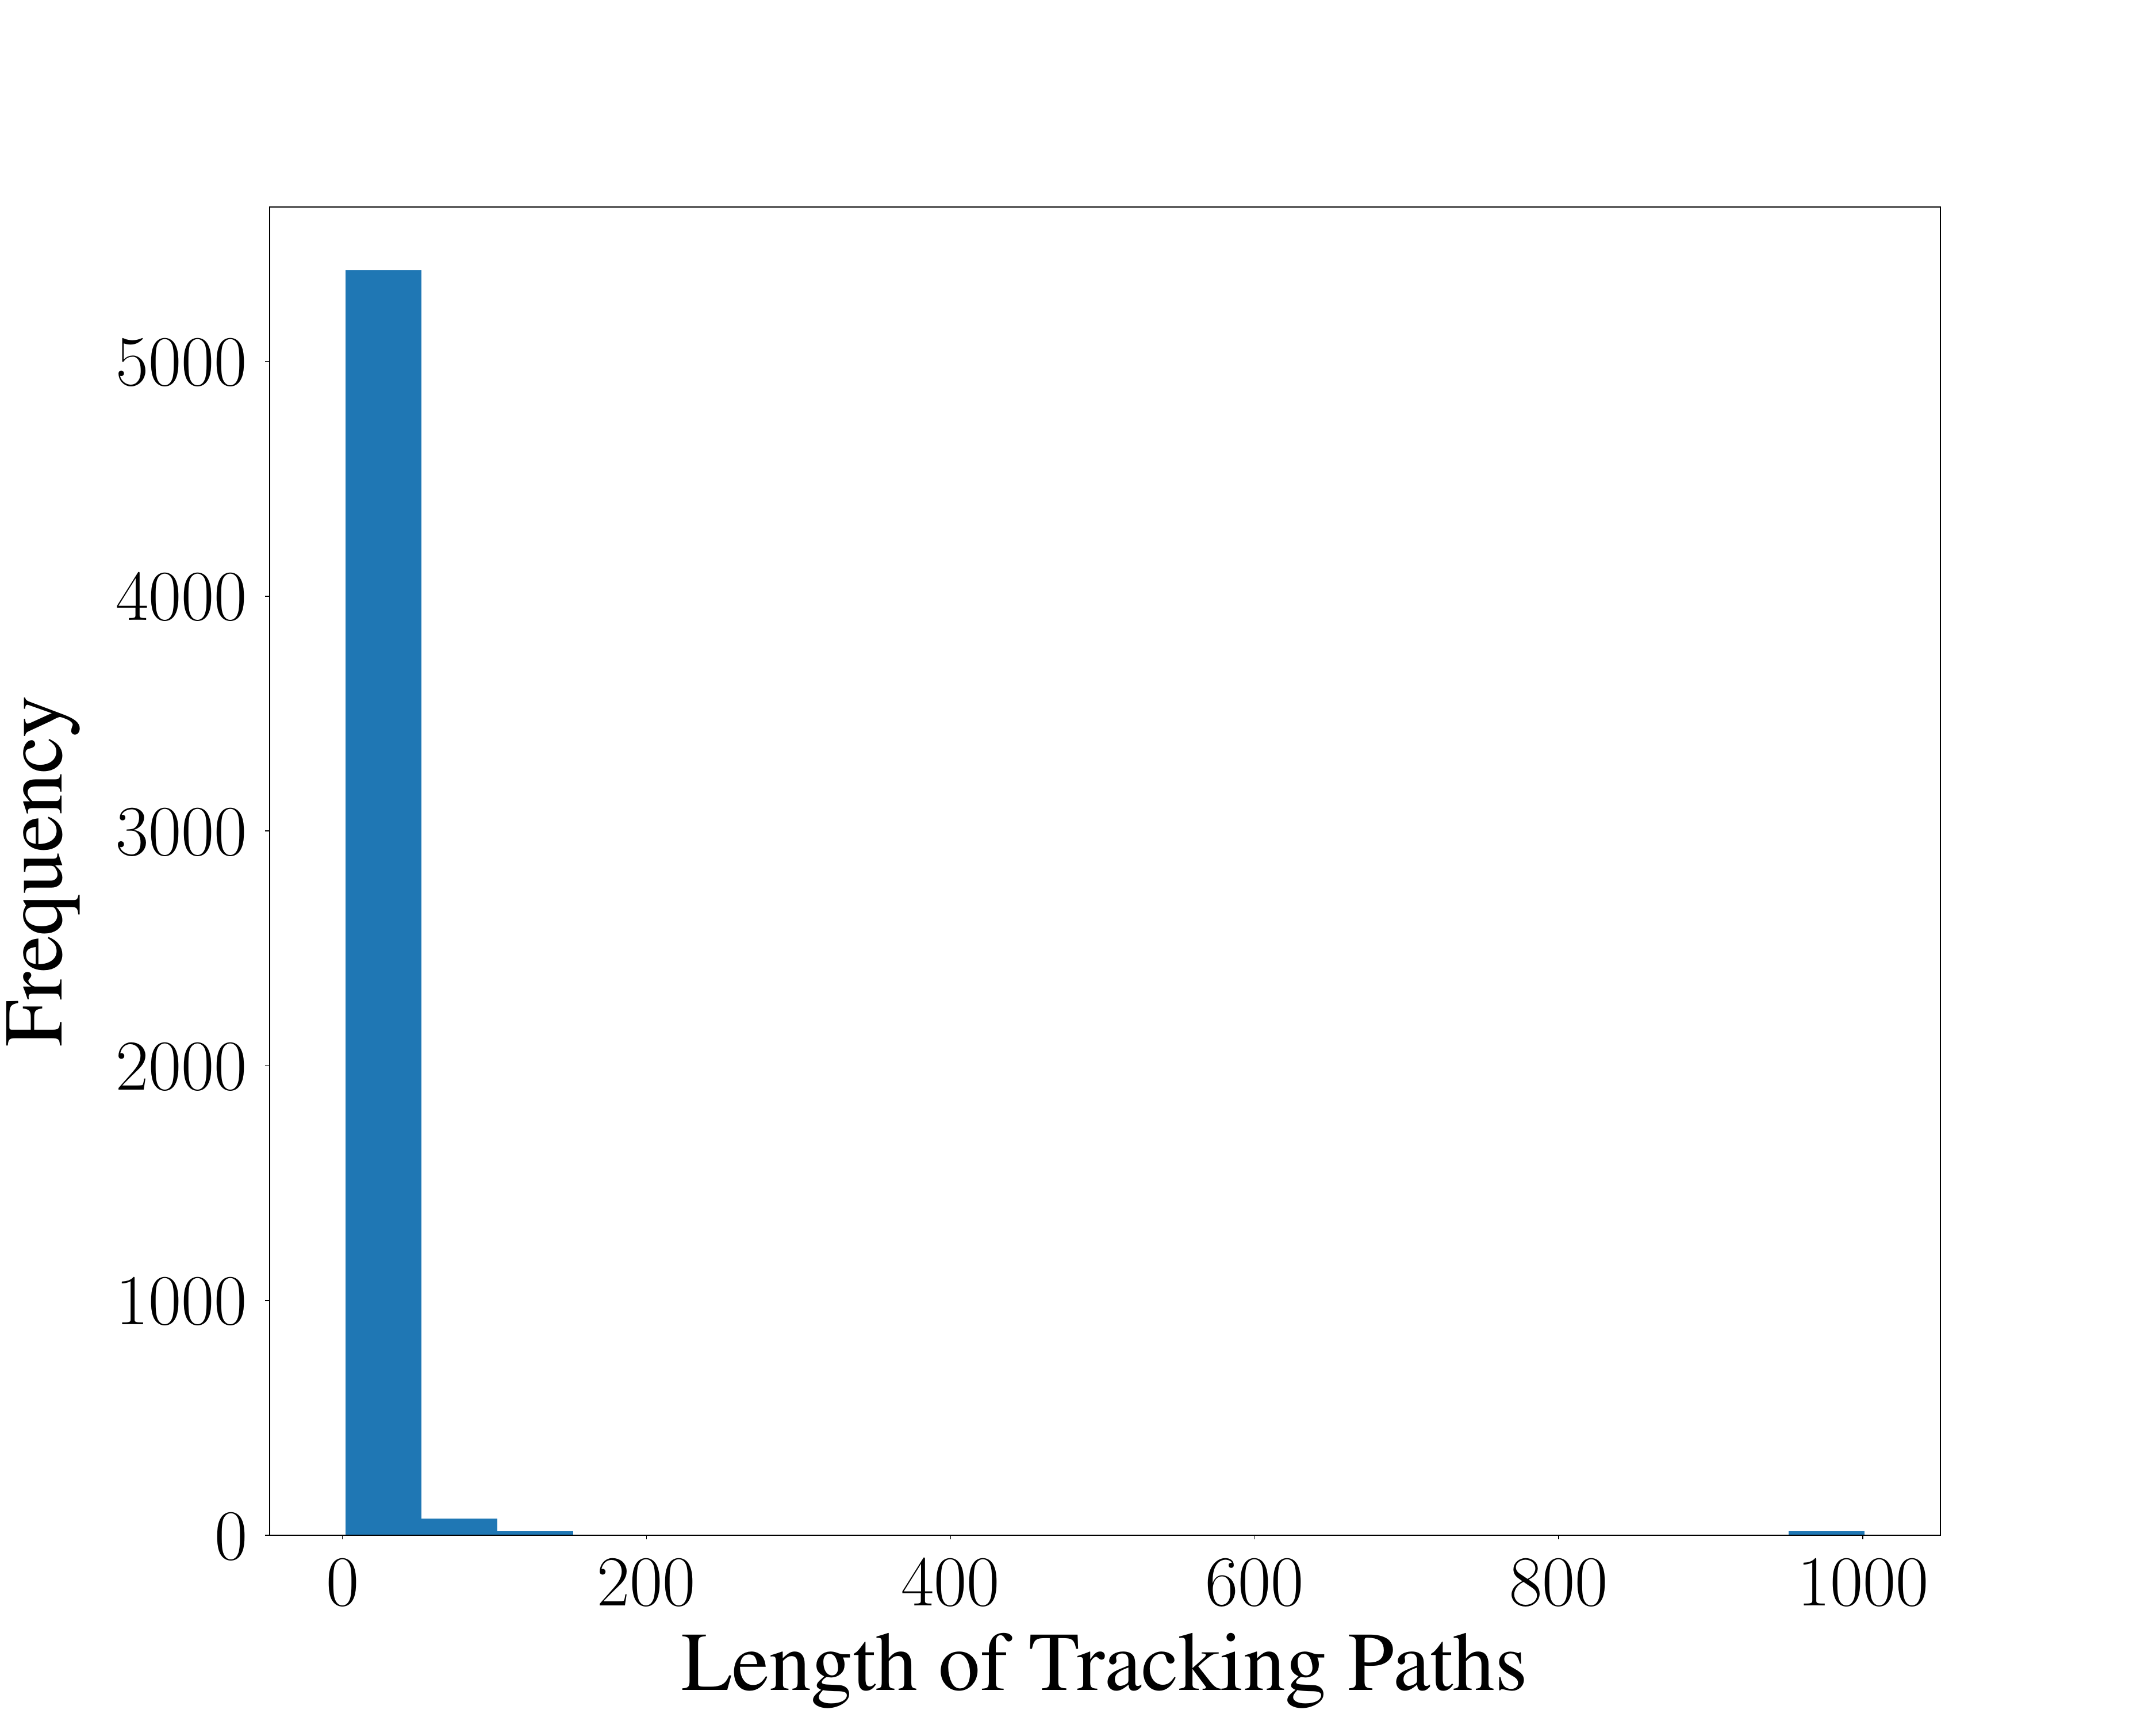}
\caption{$d_w$.}%
\label{fig-LengthHistogramCylinder2DWLong}%
\end{subfigure}
\hfill%
\begin{subfigure}[t]{\ltwopicwidth}%
\includegraphics[width=\ltwopicwidth]{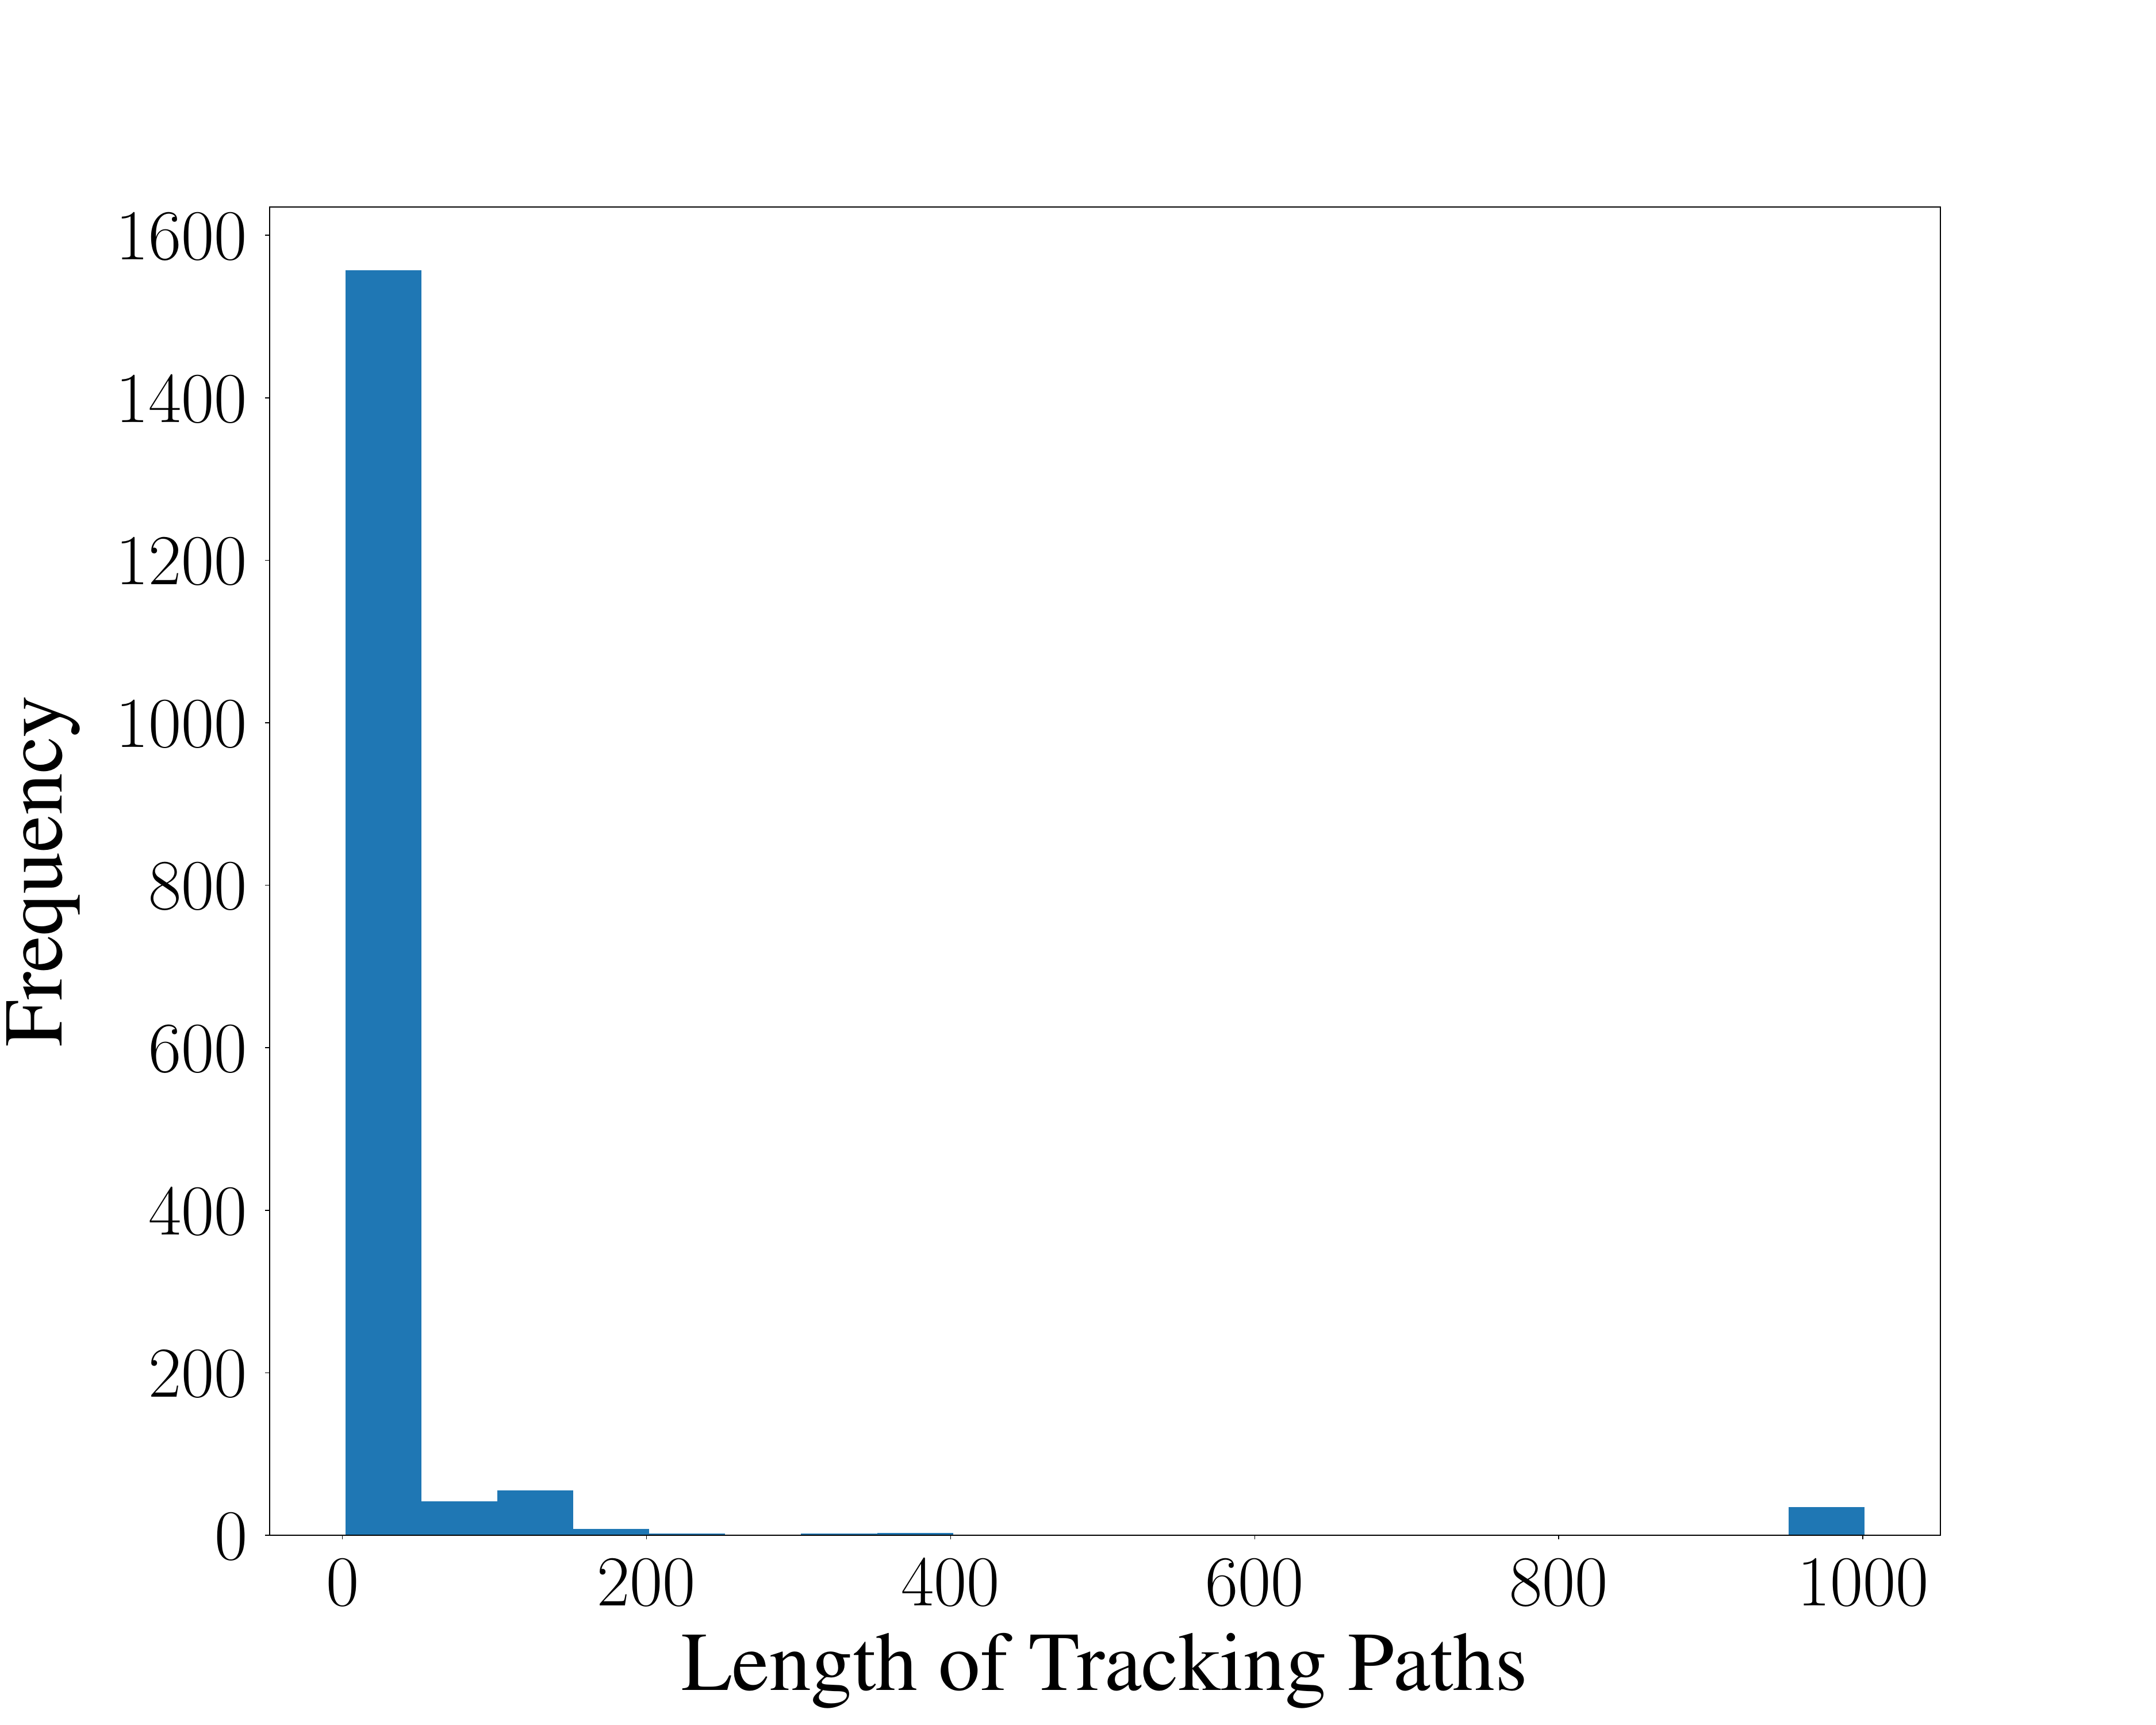}%
\caption{$d_e$.}%`'
\label{fig-LengthHistogramCylinder2DELong}%
\end{subfigure}%
\\%
\begin{subfigure}[t]{\ltwopicwidth}%
\includegraphics[width=\ltwopicwidth]{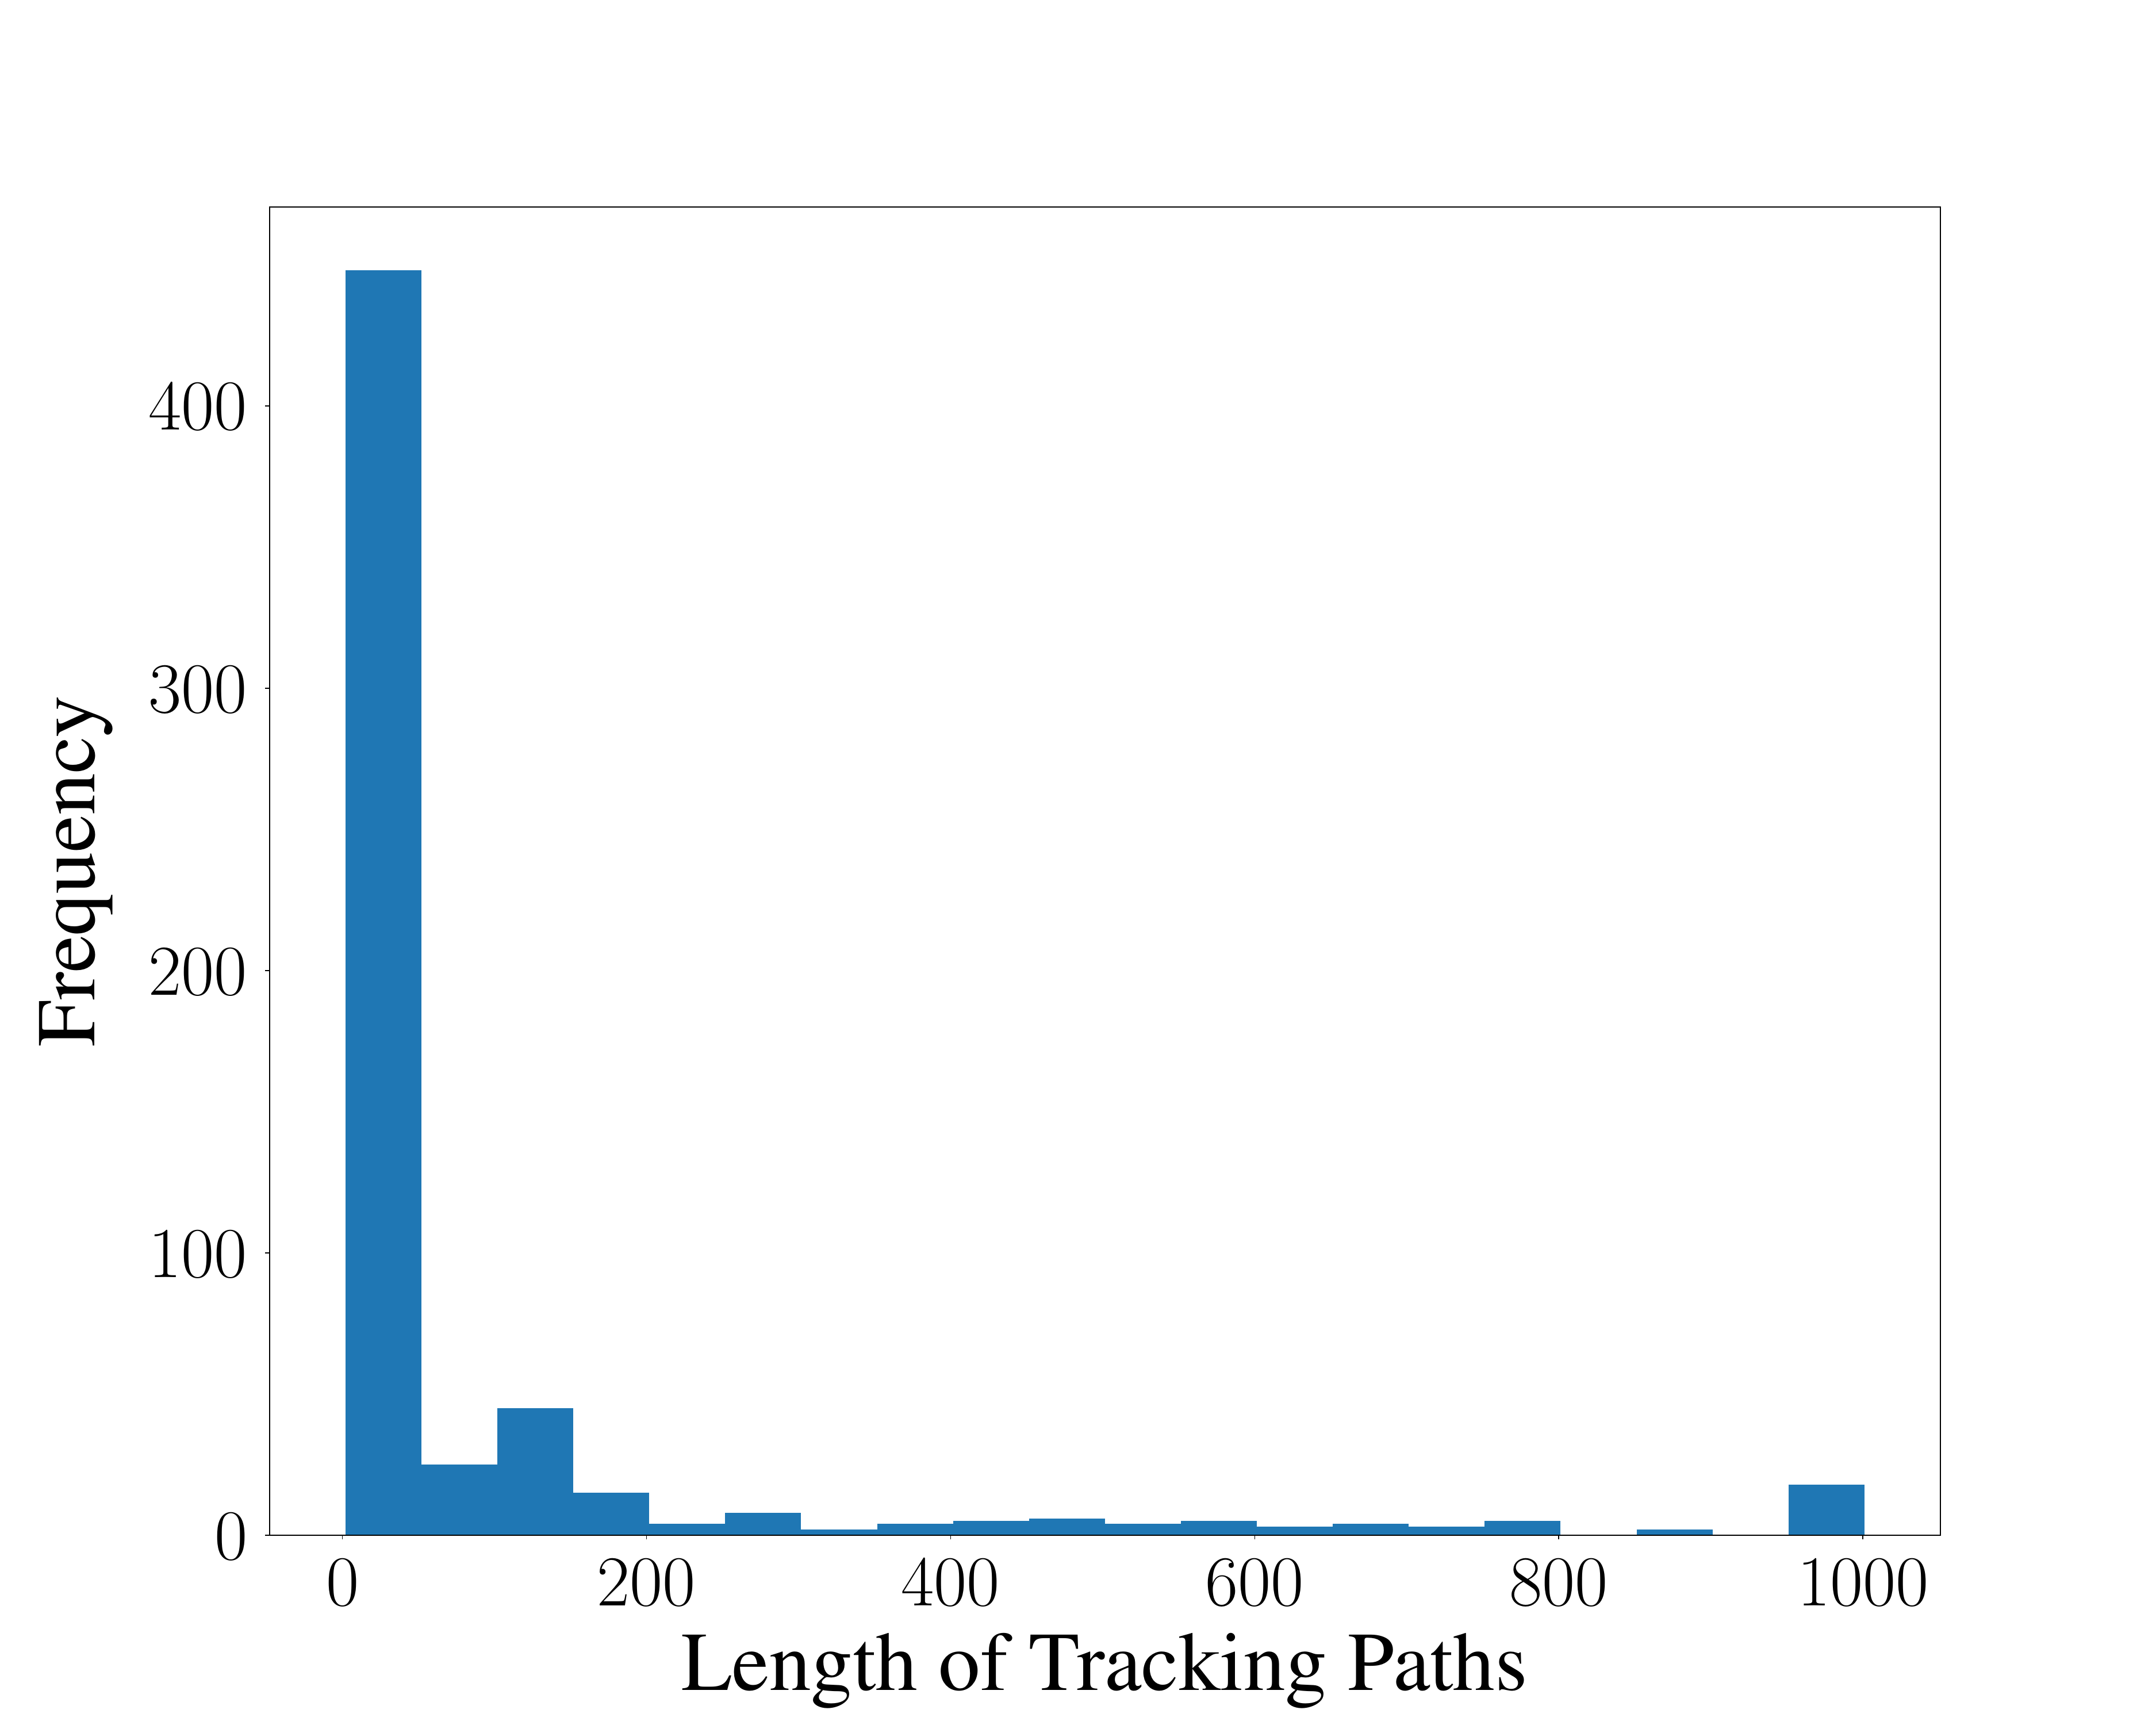}%
\caption{$d_b$.}%
\label{fig-LengthHistogramCylinder2DBLong}%
\end{subfigure}%
\hfill%
\begin{subfigure}[t]{\ltwopicwidth}%
\includegraphics[width=\ltwopicwidth]{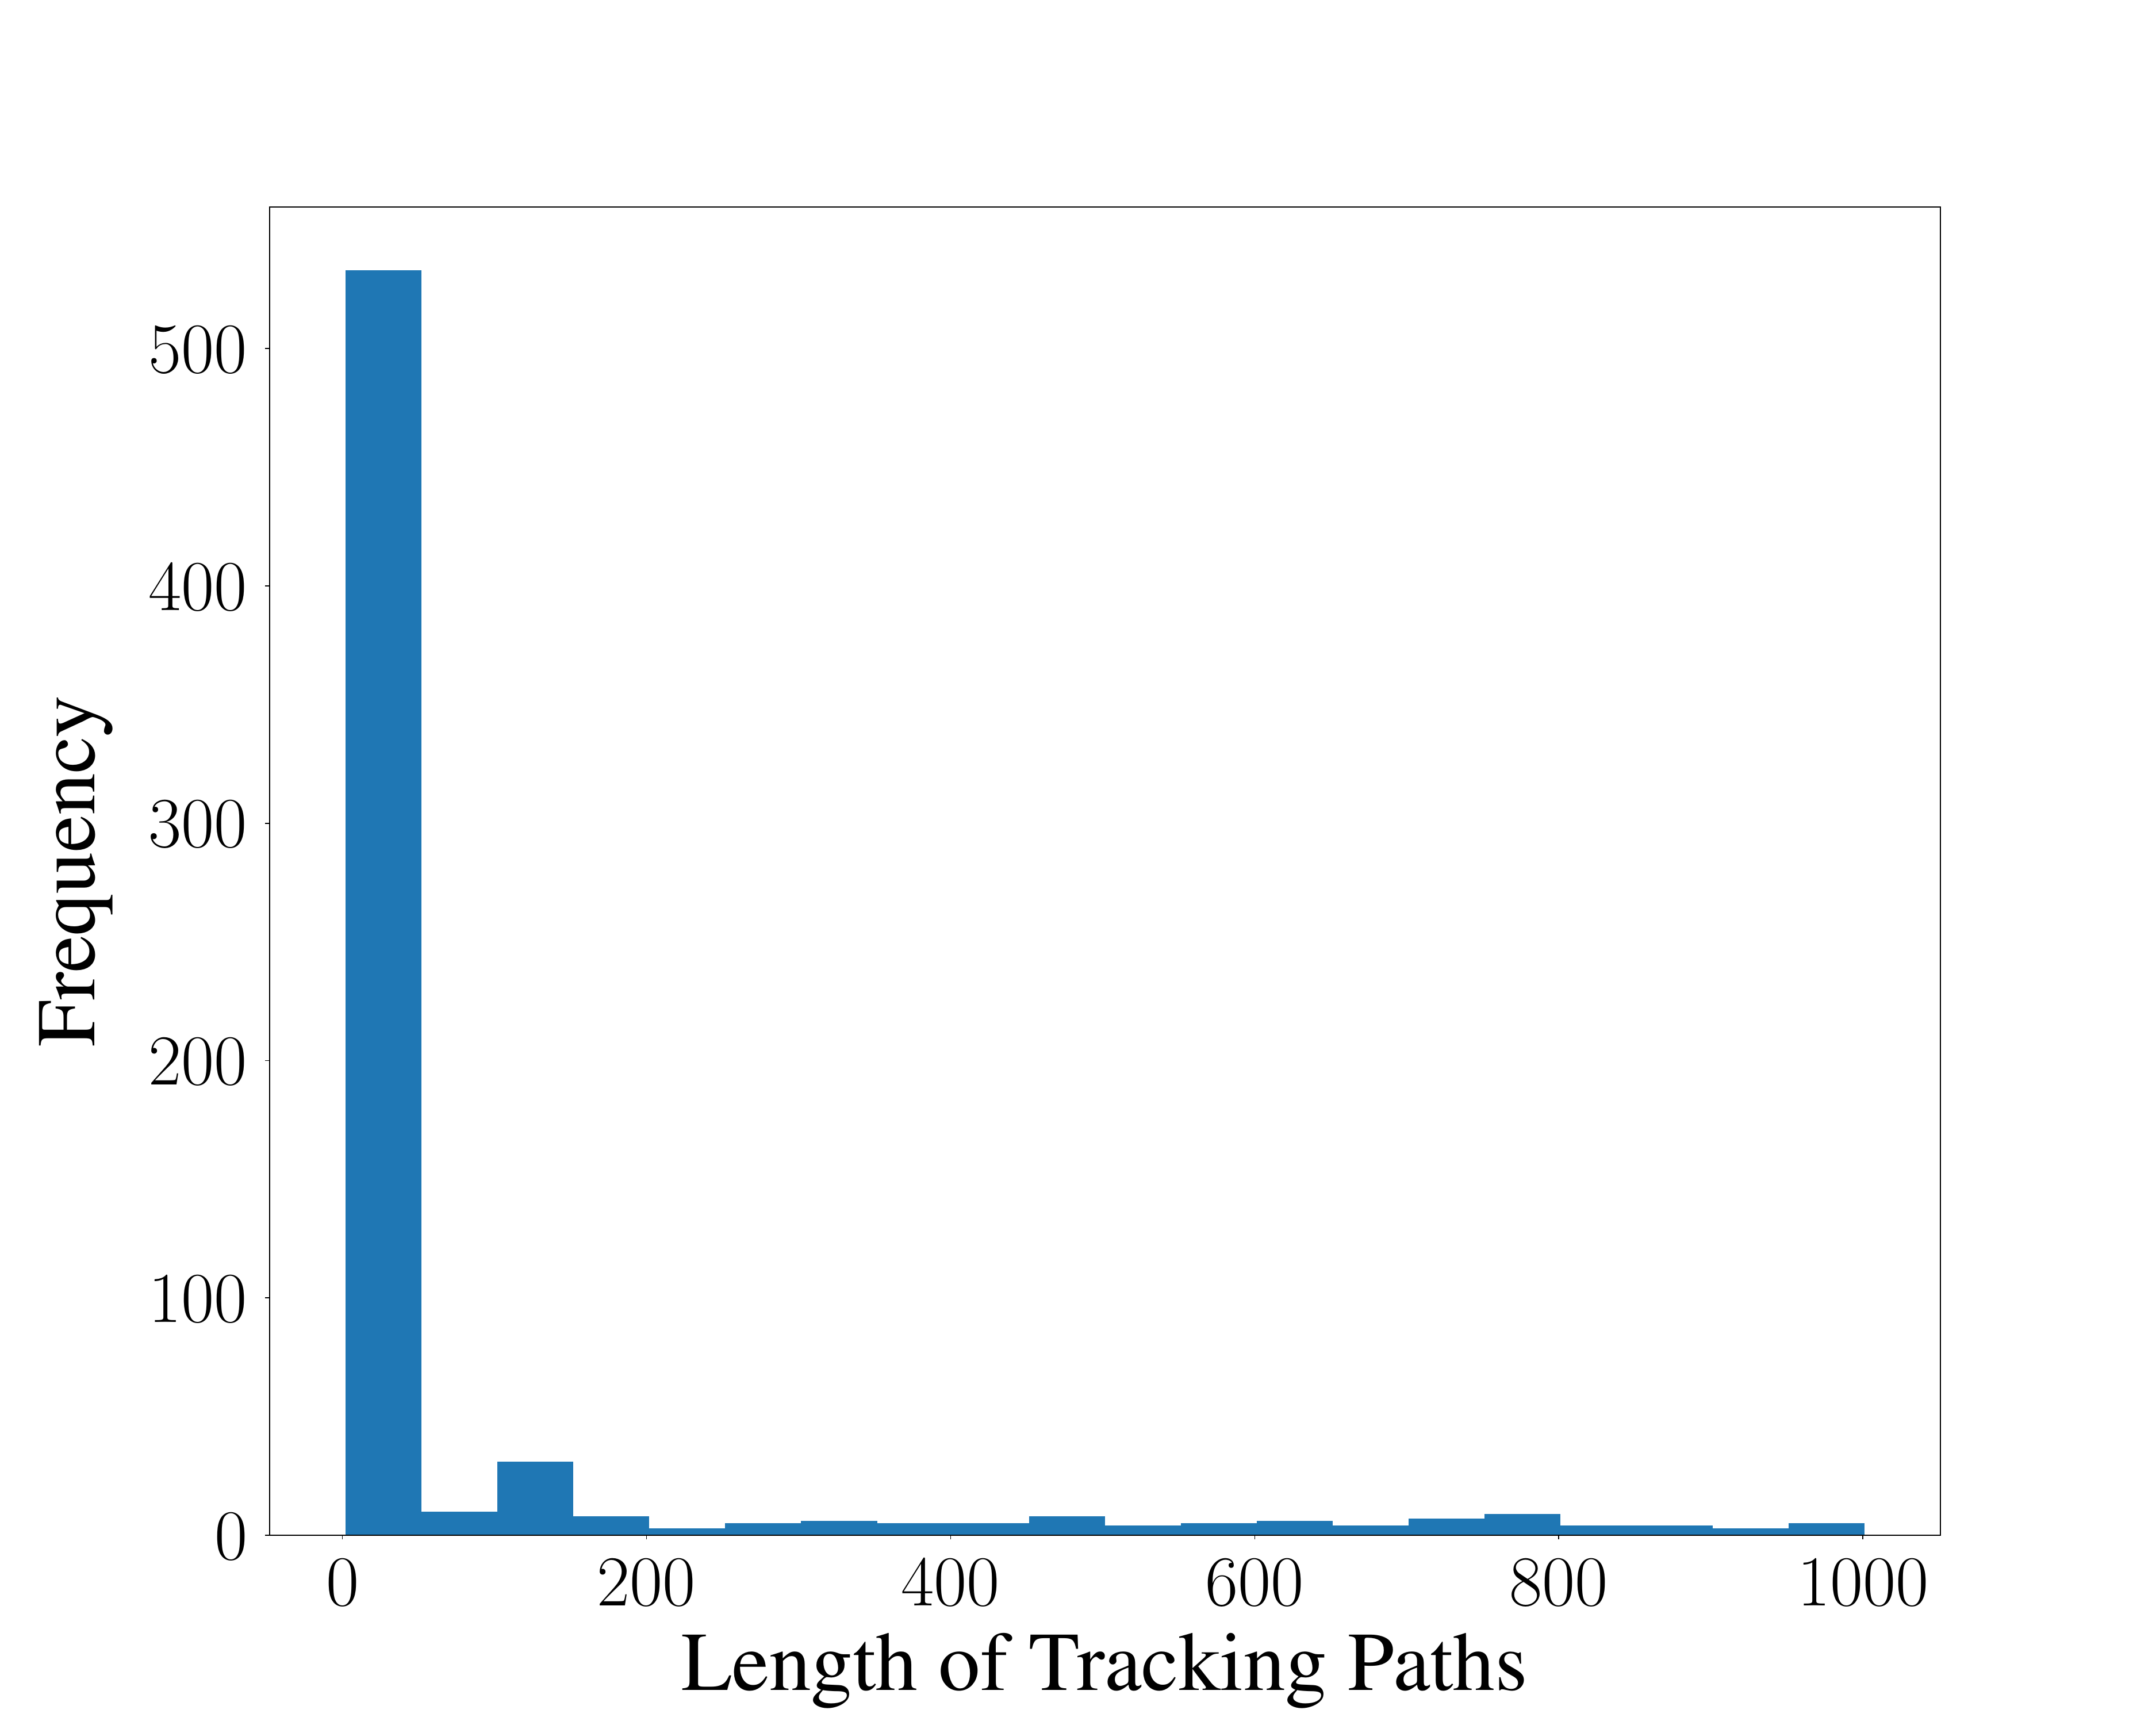}%
\caption{$d_p$.}%
\label{fig-LengthHistogramCylinder2DPLong}%
\end{subfigure}%
\caption{Histograms of the length of the tracking paths
    of \dataset{Cylinder2D}.}%
\label{fig-LengthHisgoramCylinder2DLong}%
\end{figure}

%% if specified like this the section will be committed in review mode
\acknowledgments{
This work was supported through grants from The Swedish Research Council (Vetenskapsrådet, project 2020-05461), and the Swedish e-Science Research Centre (SeRC).
We would like to thank the anonymous reviewers for their valuable feedback.
}

\bibliographystyle{abbrv-doi}

\bibliography{Literature}
\end{document}
