# Supplementary material for: A Comparative Study of Different Edit Distance-Based Methods for Feature Tracking using Merge Trees on Time-Varying Scalar Fields
Source: arXiv:2509.17974 source file (2025-10-12)
Supplement: Supplementary file 3 [file supp_Cylinder2D.tex]

\subsection*{Extra results with Cylinder2D data set}
More results of the experiments using \dataset{Cylinder2D}
are shown in \Cref{fig-Cylinder2DAllNodesLong}
through \Cref{fig-LengthHisgoramCylinder2DLong}.

\begin{figure}
\centering
\includegraphics[width=0.8\linewidth]{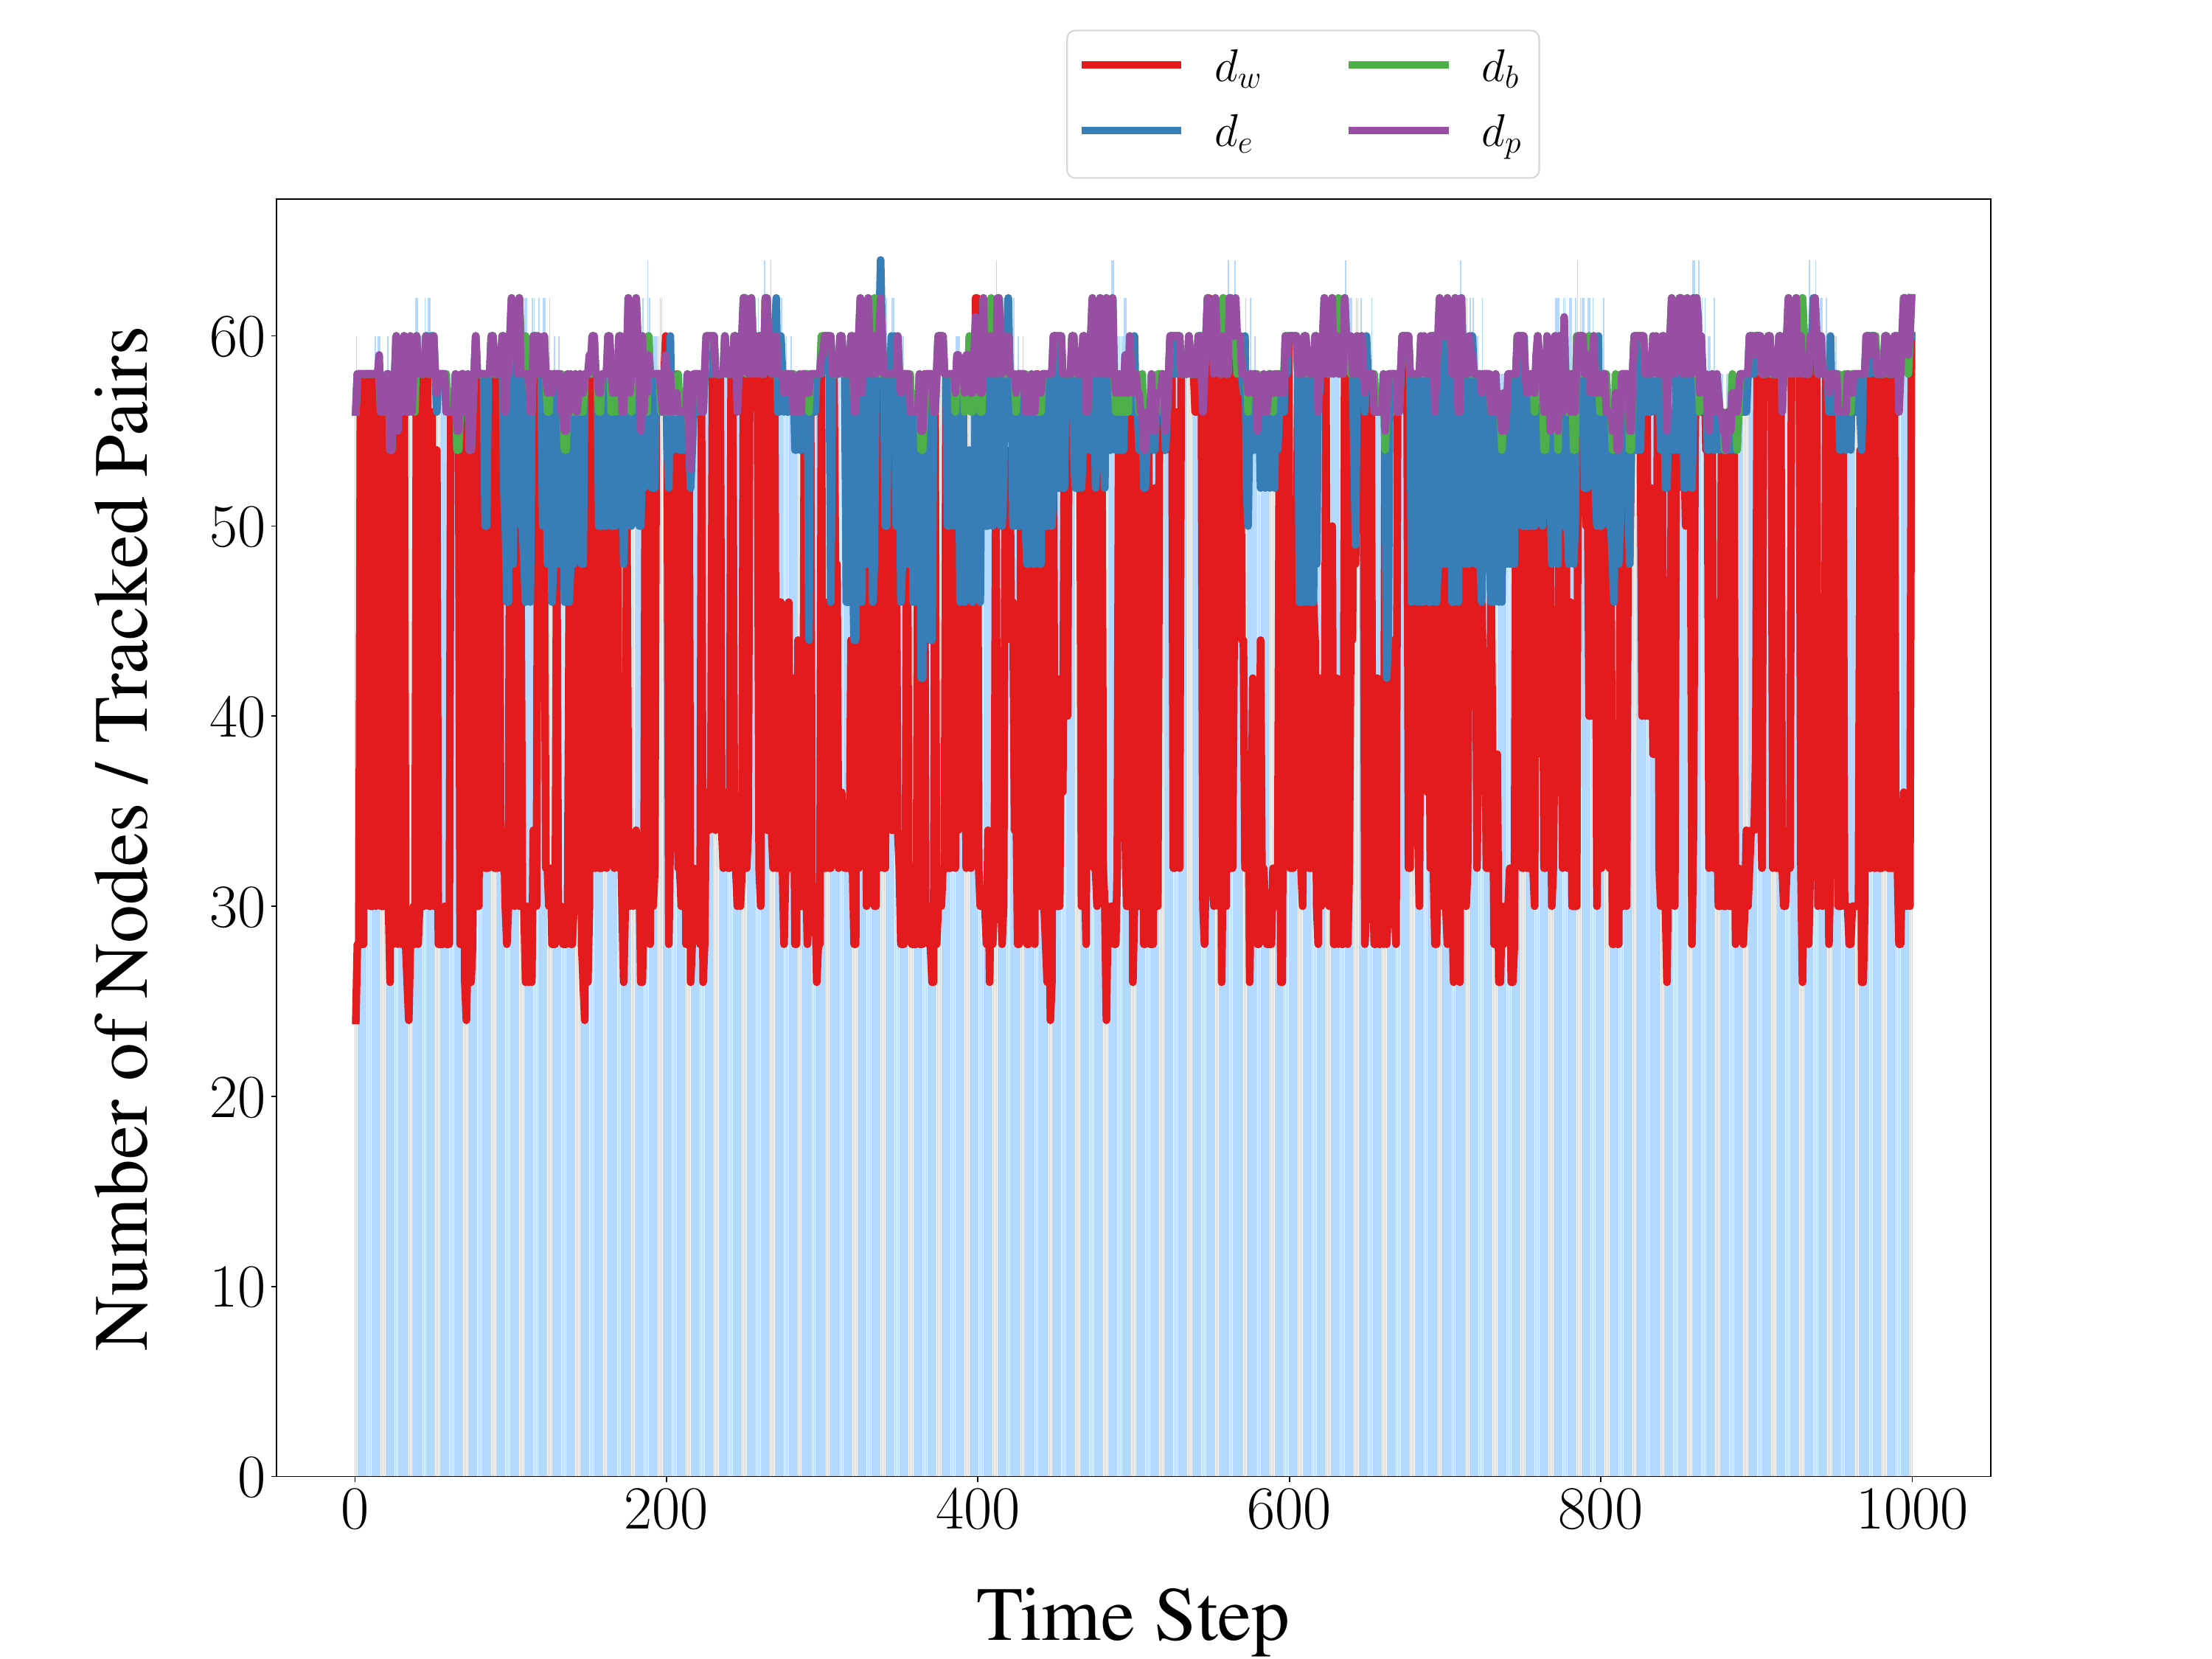}
\caption{
    Number of tracked nodes (colored and labeled) 
    relative to the total nodes of merge trees (light blue bars)
    for \dataset{Cylinder2D}.
}
\label{fig-Cylinder2DAllNodesLong}
\end{figure}

% Length histogram
\begin{figure}%
\begin{subfigure}[t]{\ltwopicwidth}%
\includegraphics[width=\ltwopicwidth]{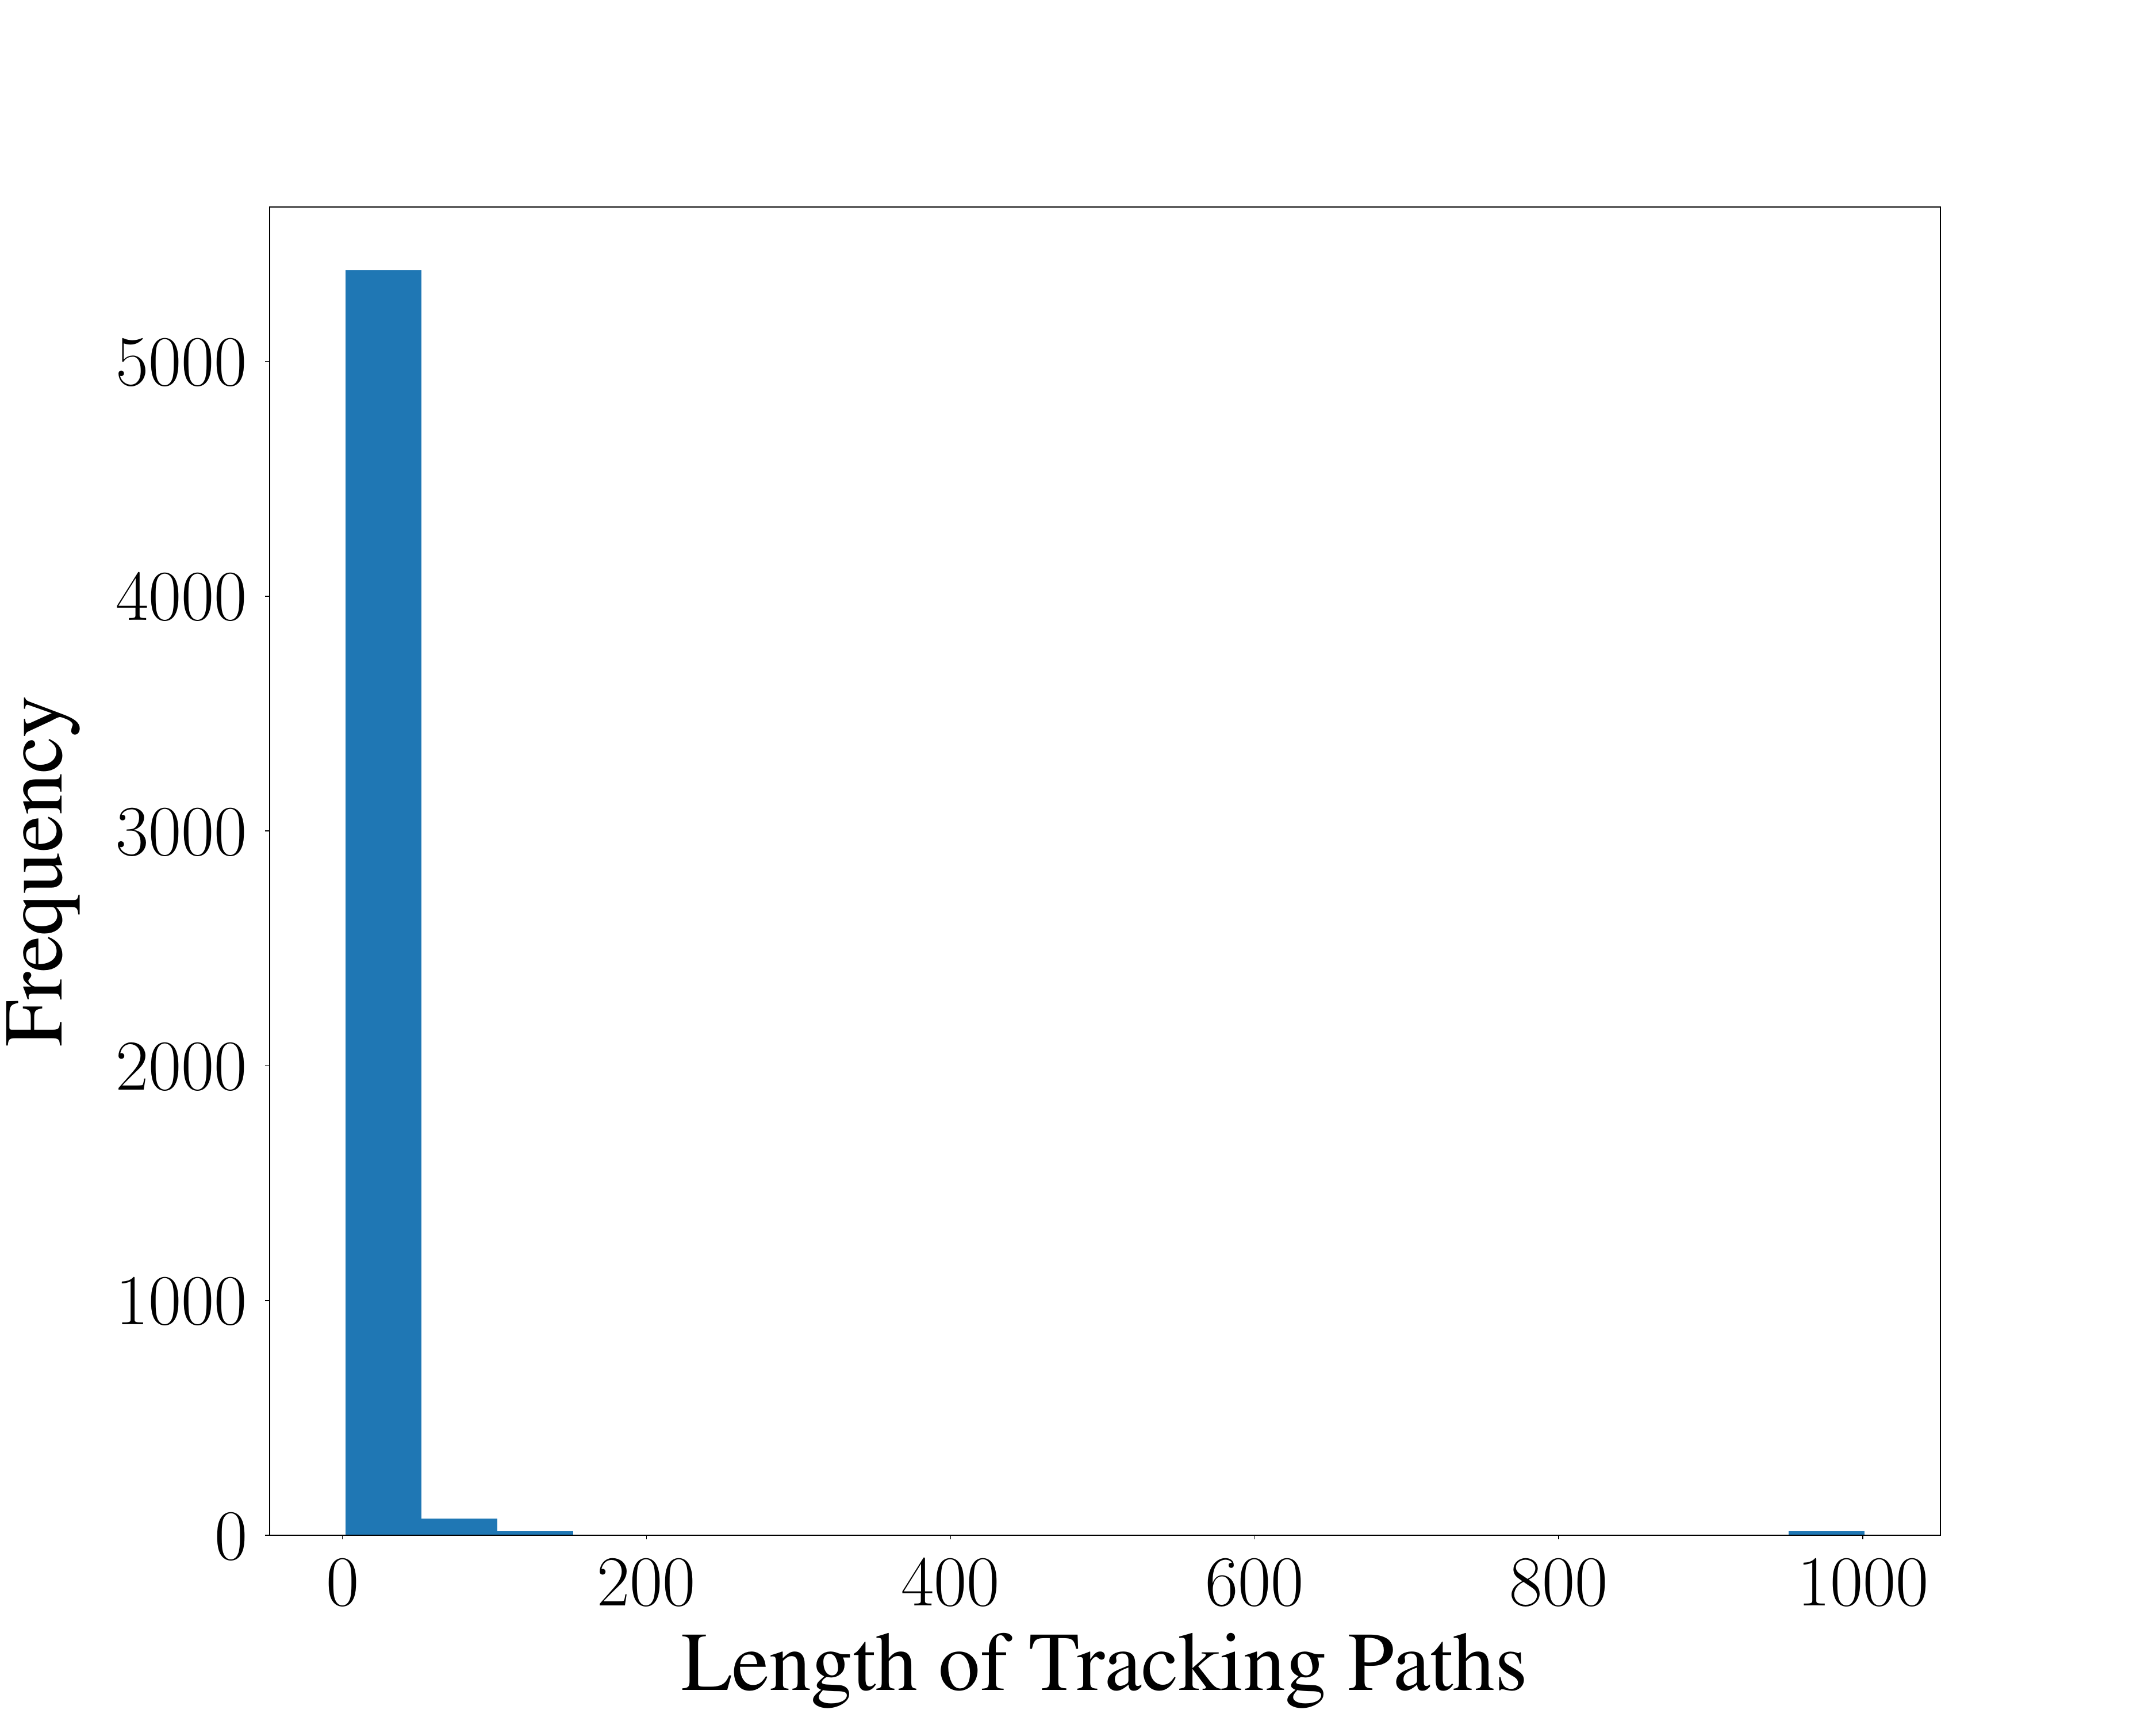}
\caption{$d_w$.}%
\label{fig-LengthHistogramCylinder2DWLong}%
\end{subfigure}
\hfill%
\begin{subfigure}[t]{\ltwopicwidth}%
\includegraphics[width=\ltwopicwidth]{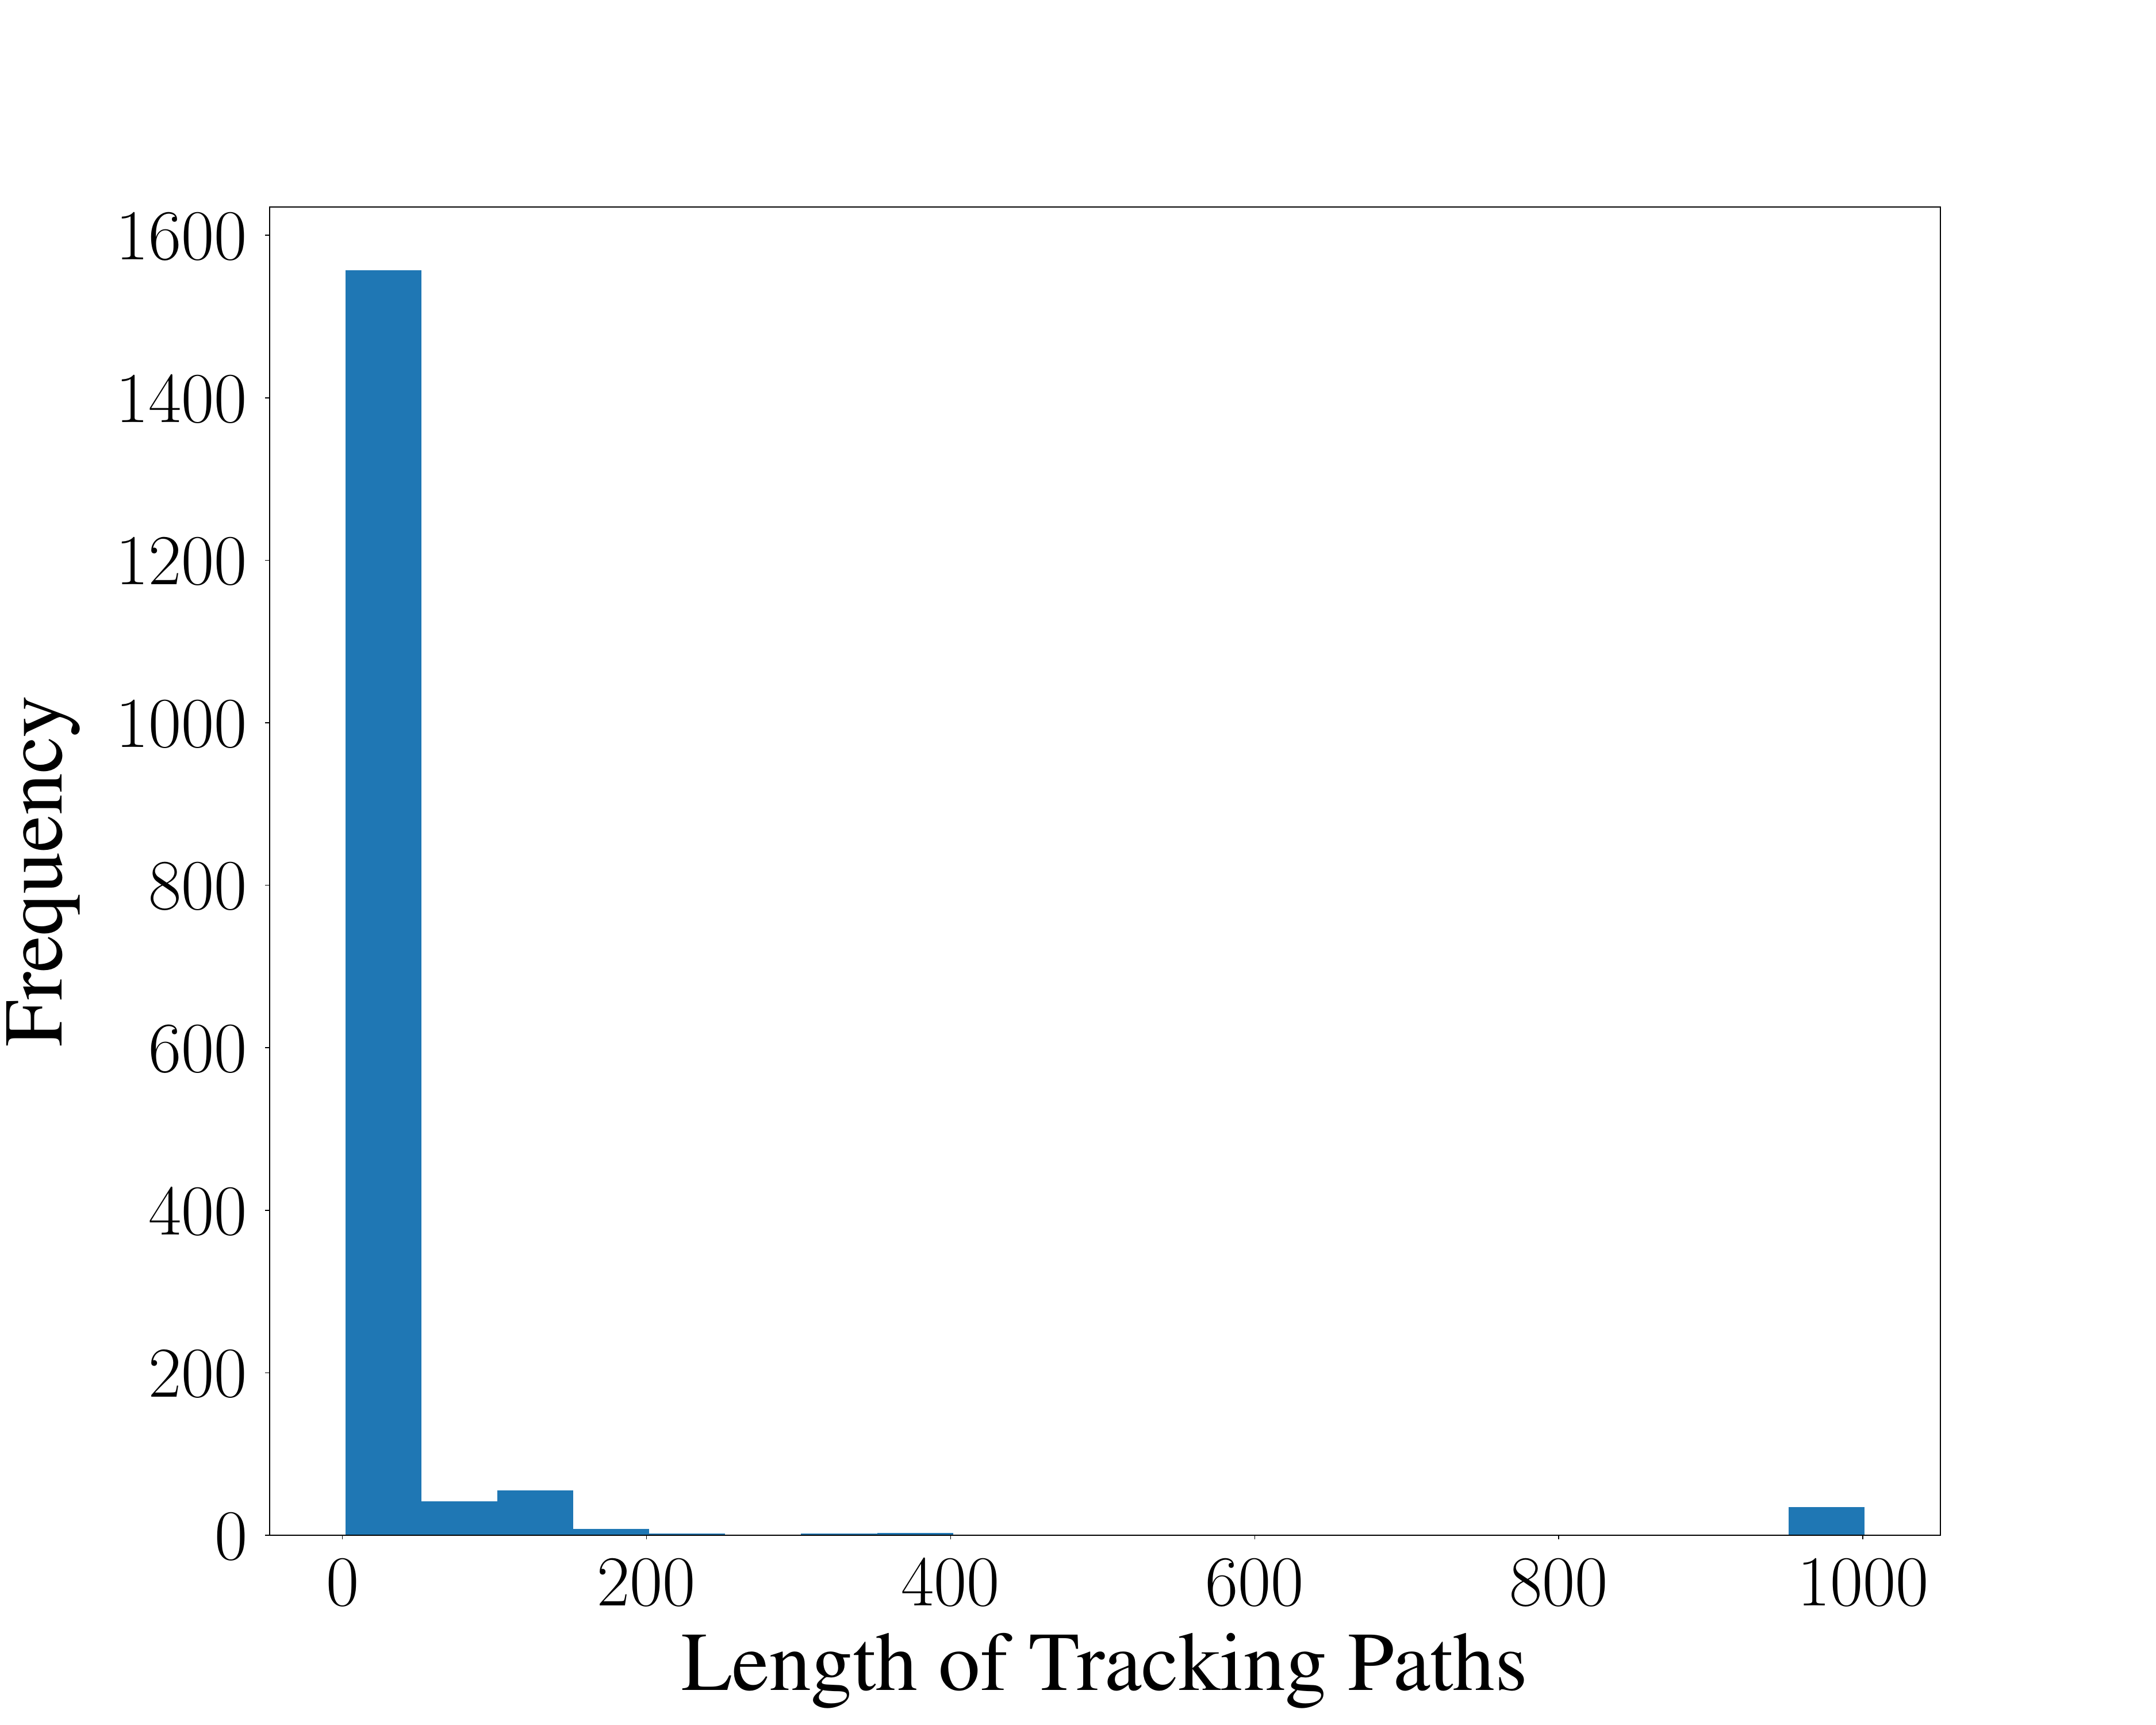}%
\caption{$d_e$.}%`'
\label{fig-LengthHistogramCylinder2DELong}%
\end{subfigure}%
\\%
\begin{subfigure}[t]{\ltwopicwidth}%
\includegraphics[width=\ltwopicwidth]{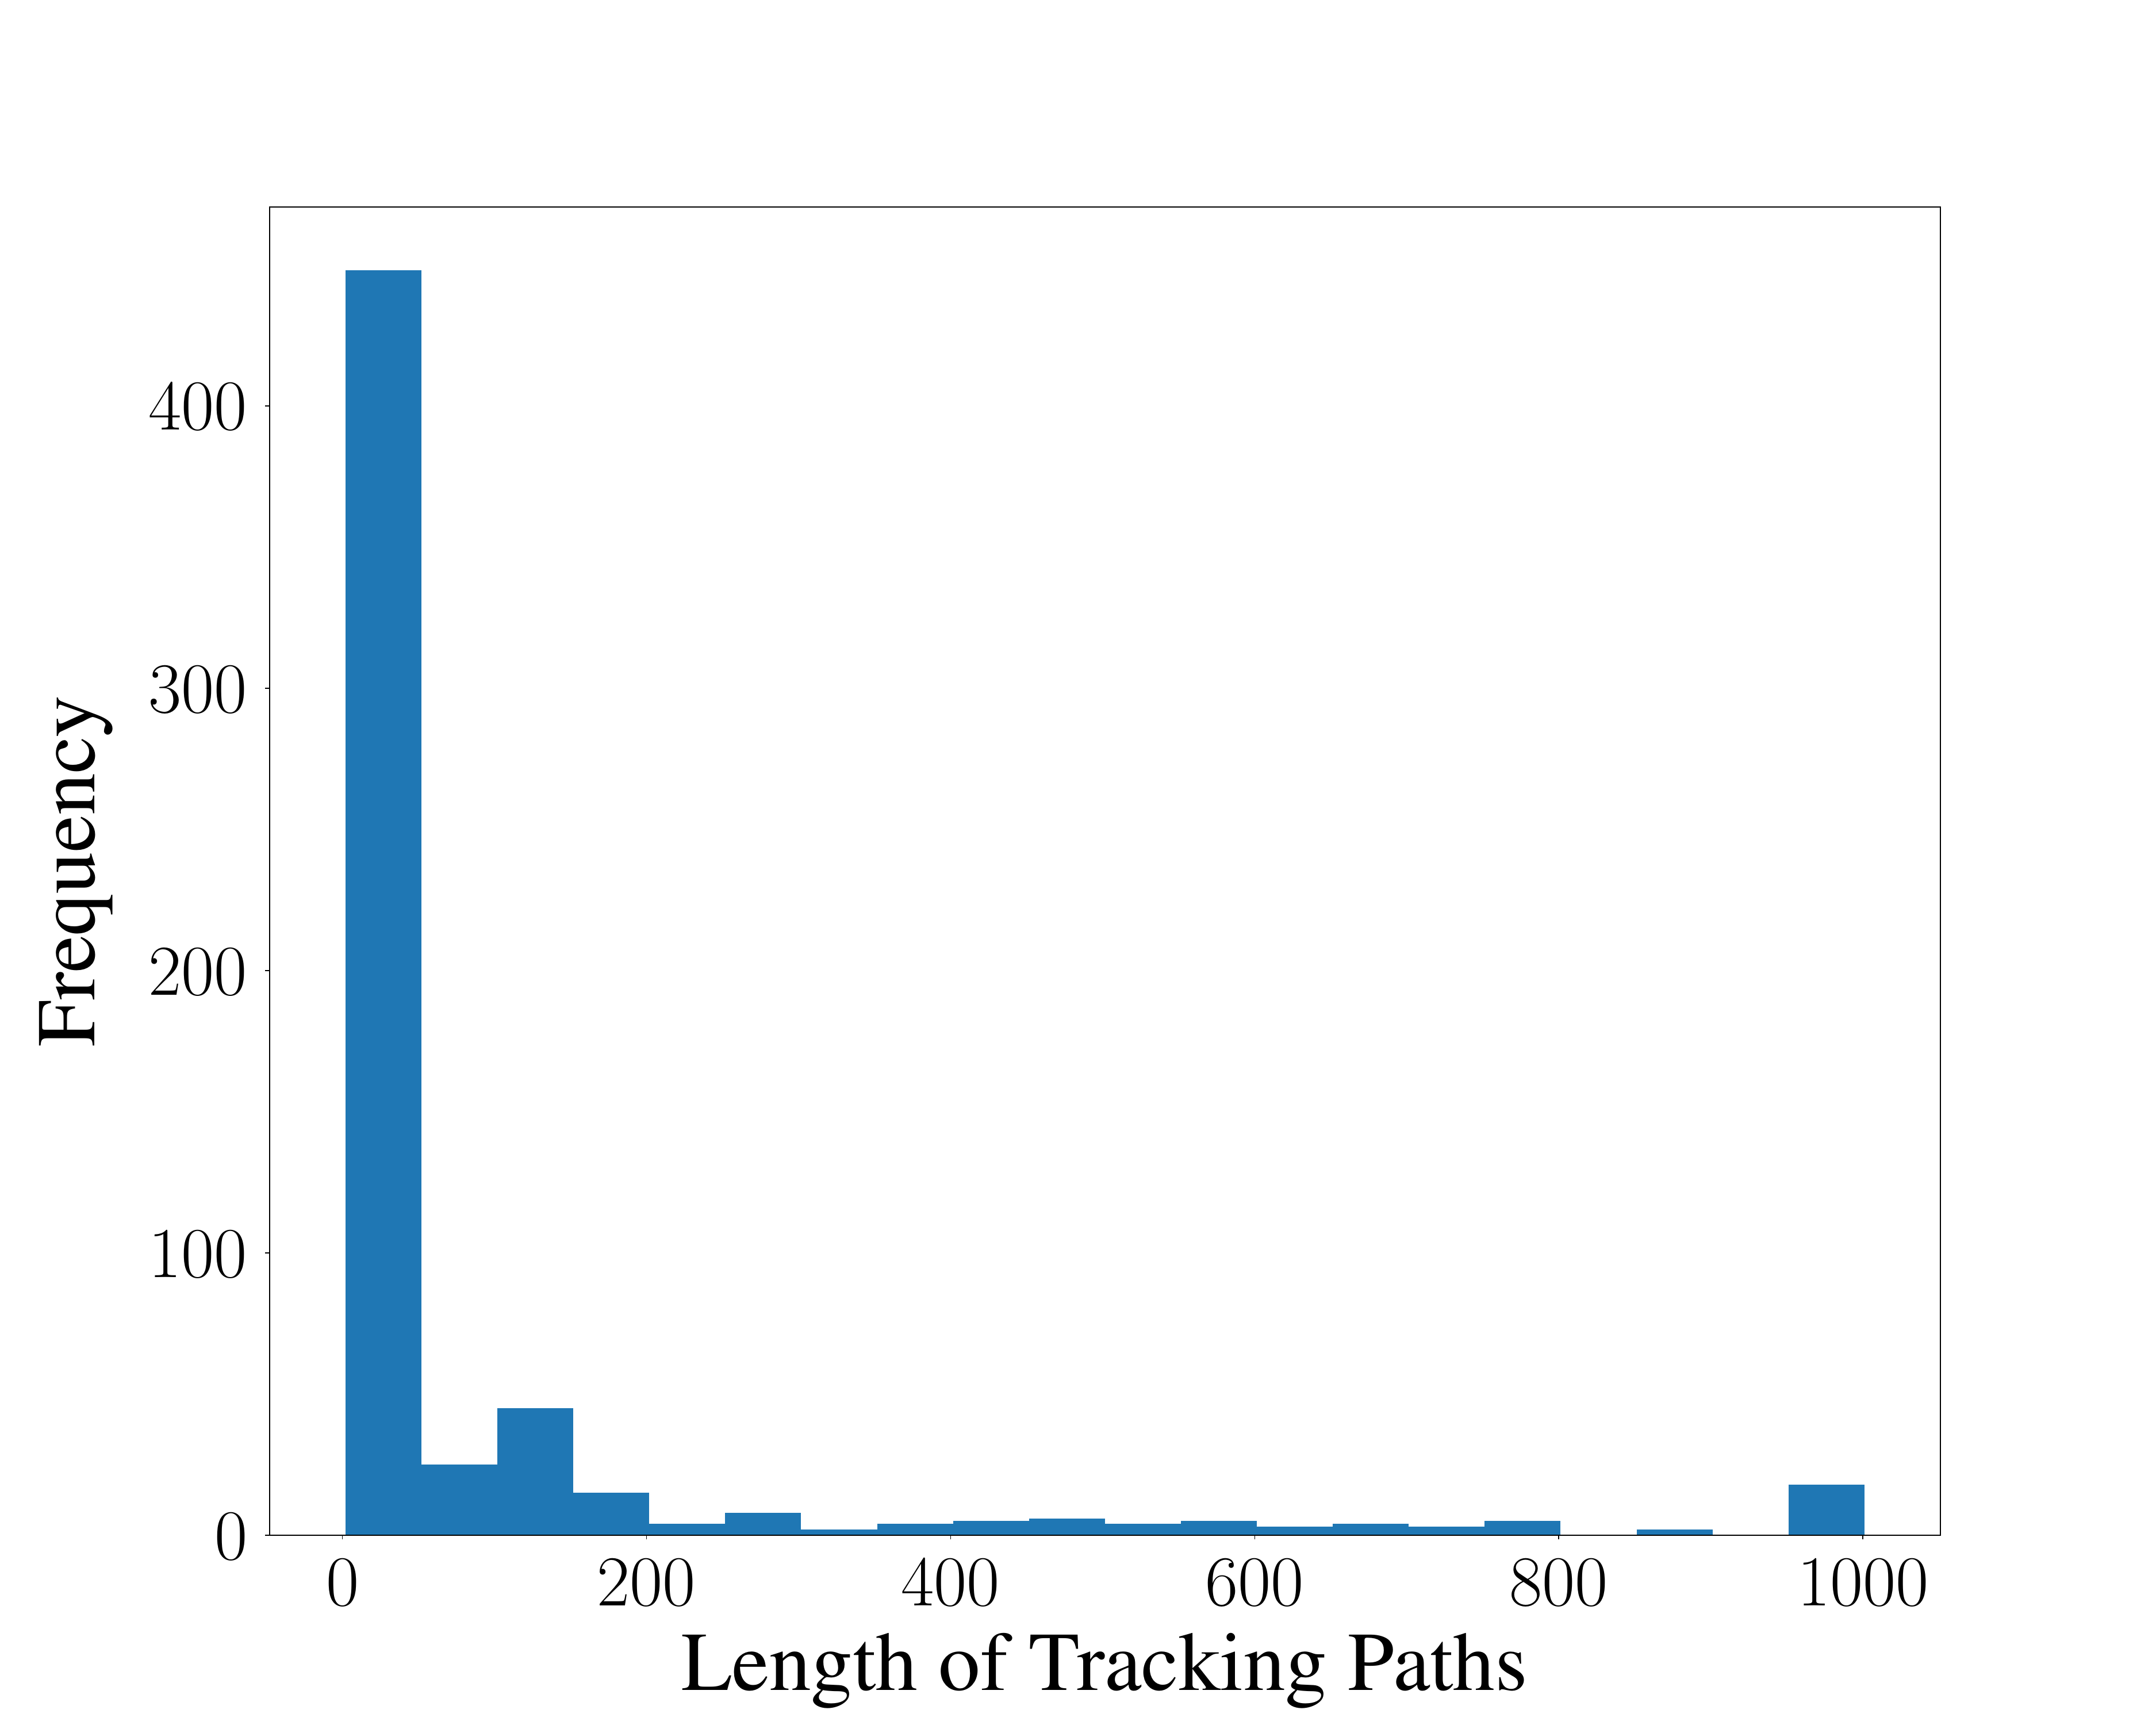}%
\caption{$d_b$.}%
\label{fig-LengthHistogramCylinder2DBLong}%
\end{subfigure}%
\hfill%
\begin{subfigure}[t]{\ltwopicwidth}%
\includegraphics[width=\ltwopicwidth]{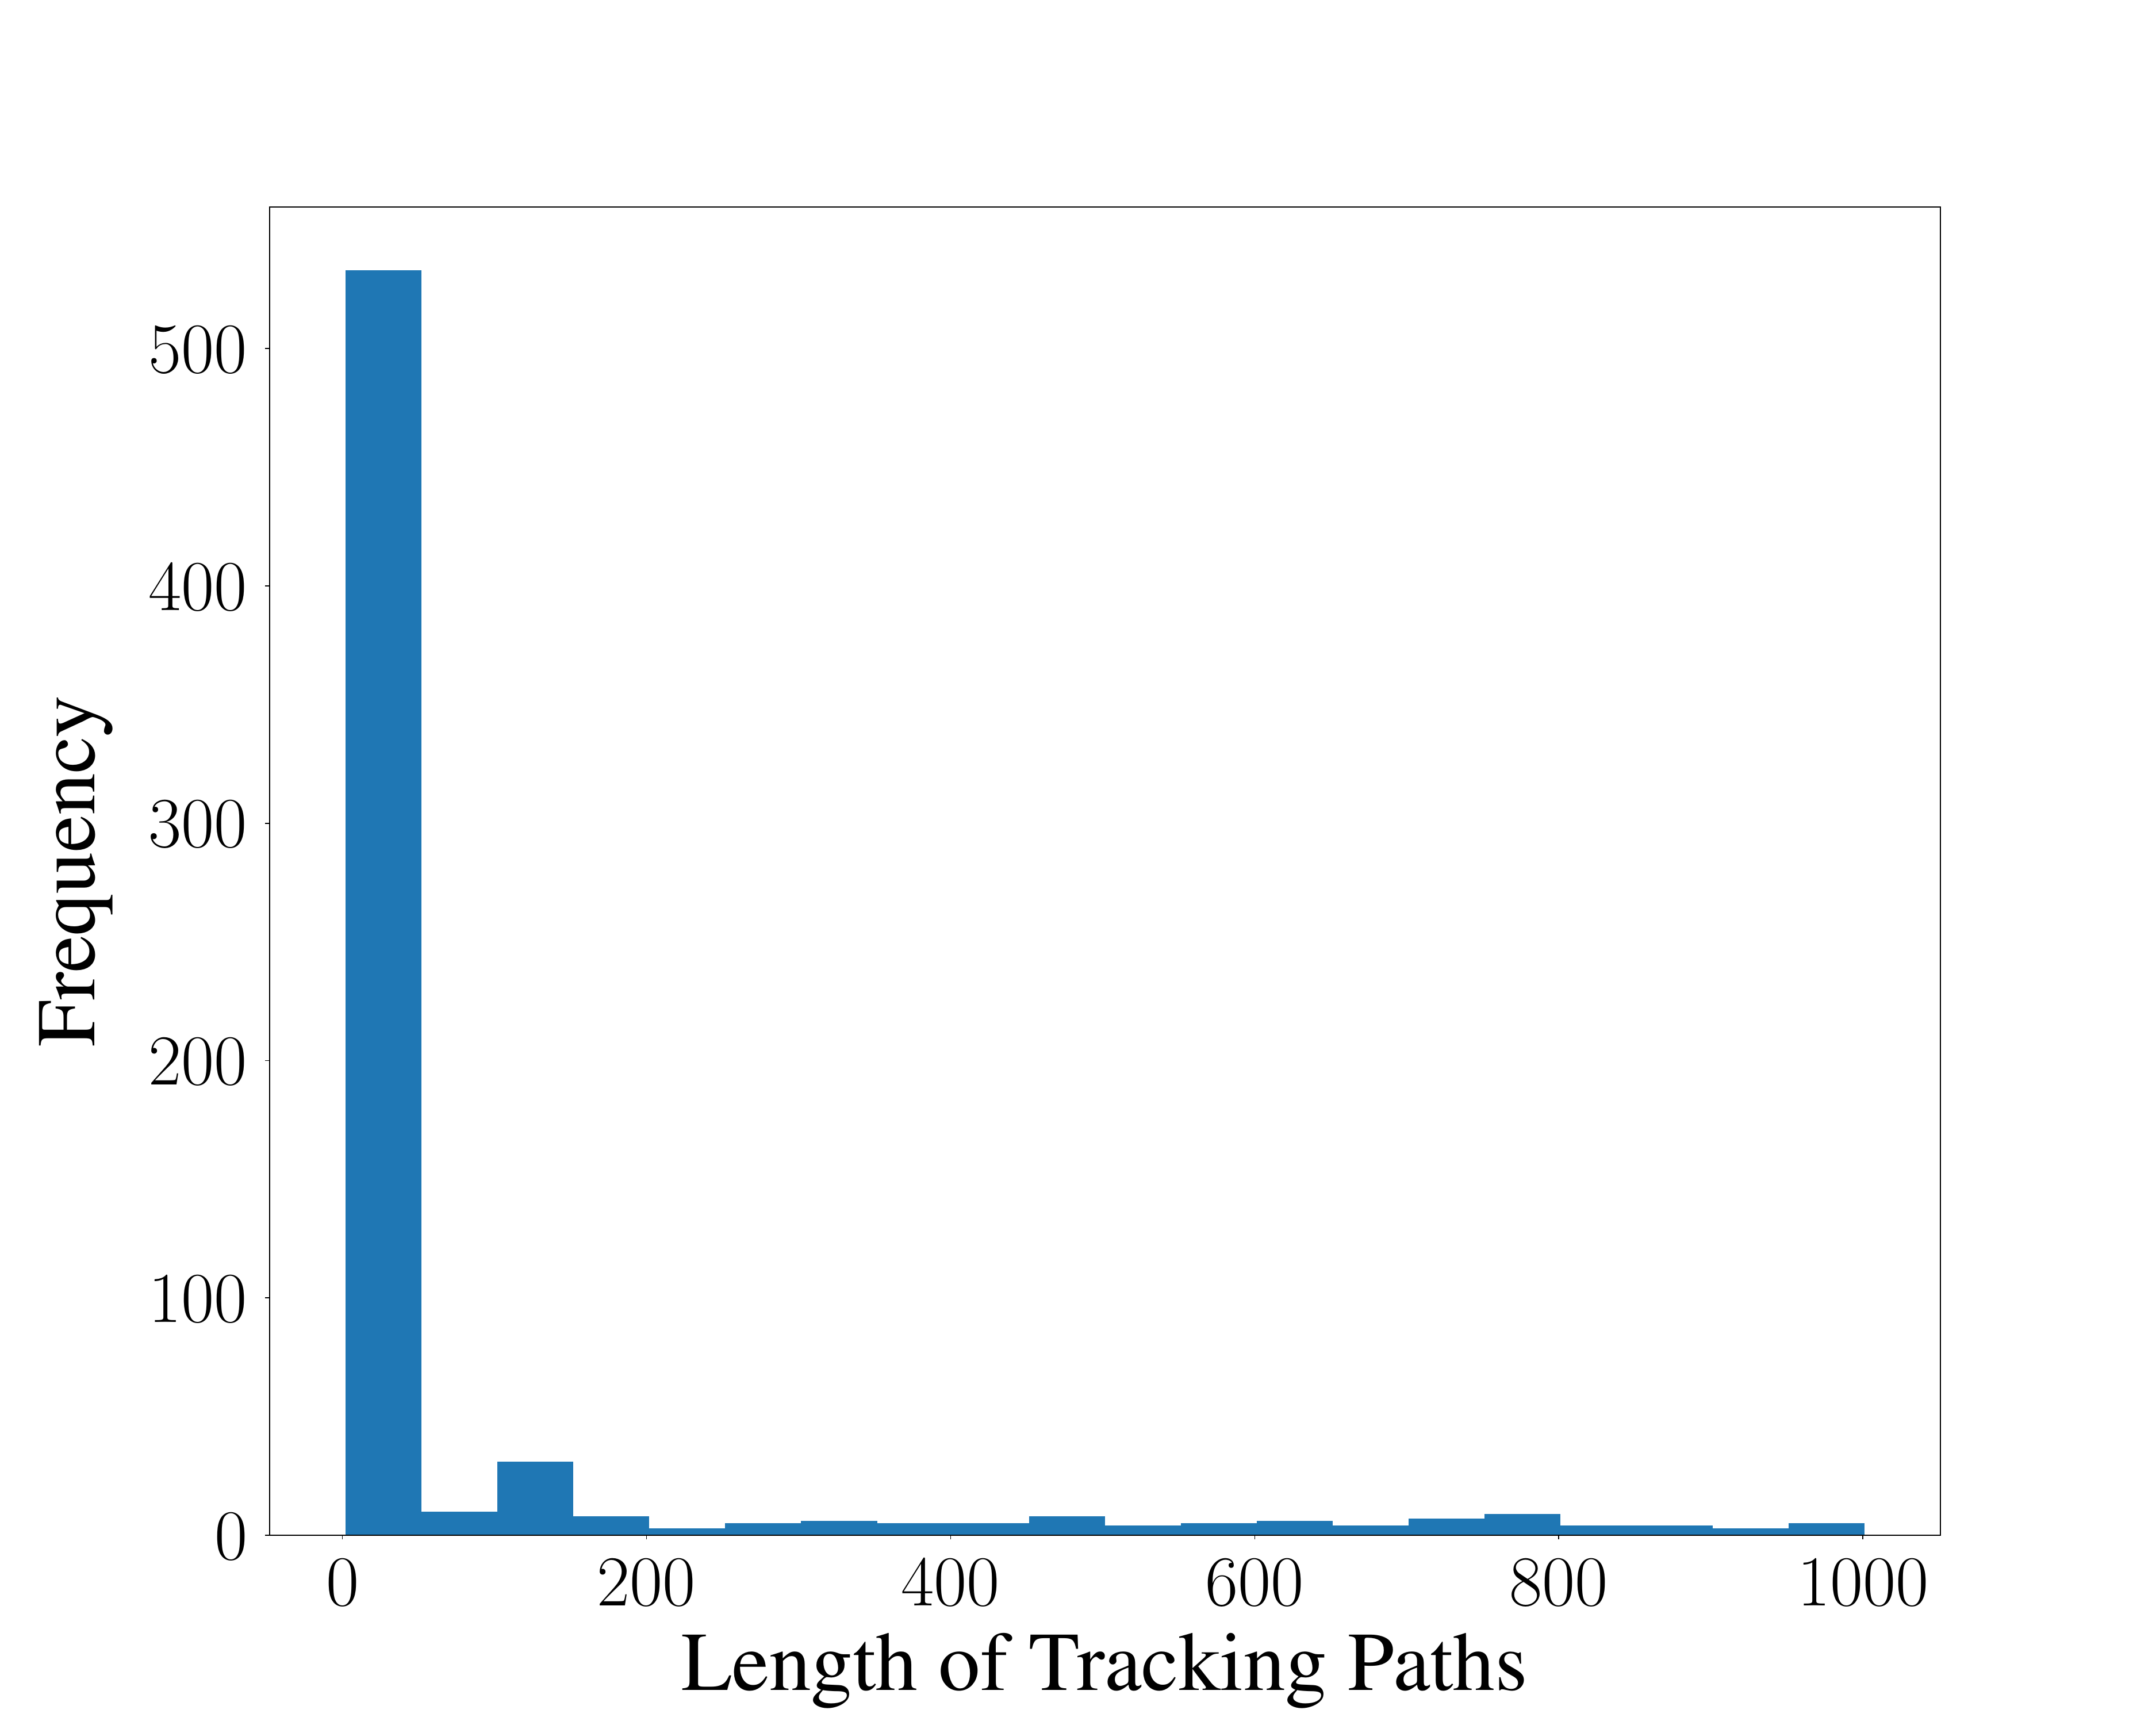}%
\caption{$d_p$.}%
\label{fig-LengthHistogramCylinder2DPLong}%
\end{subfigure}%
\caption{Histograms of the length of the tracking paths
    of \dataset{Cylinder2D}.}%
\label{fig-LengthHisgoramCylinder2DLong}%
\end{figure}
