# Supplementary material for: A Comparative Study of Different Edit Distance-Based Methods for Feature Tracking using Merge Trees on Time-Varying Scalar Fields
Source: arXiv:2509.17974 source file (2025-10-12)
Supplement: Supplementary file 5 [file supp_IonizationFront.tex]

\subsection*{Results using IonizationFront2D}
The results of the experiments using \dataset{IonizationFront2D}
are shown from \Cref{fig-IonizationFront2DAllNodes}
to \Cref{fig-IonizationFront2DSimilarities}.

\begin{figure}
\centering
\includegraphics[width=0.8\linewidth]{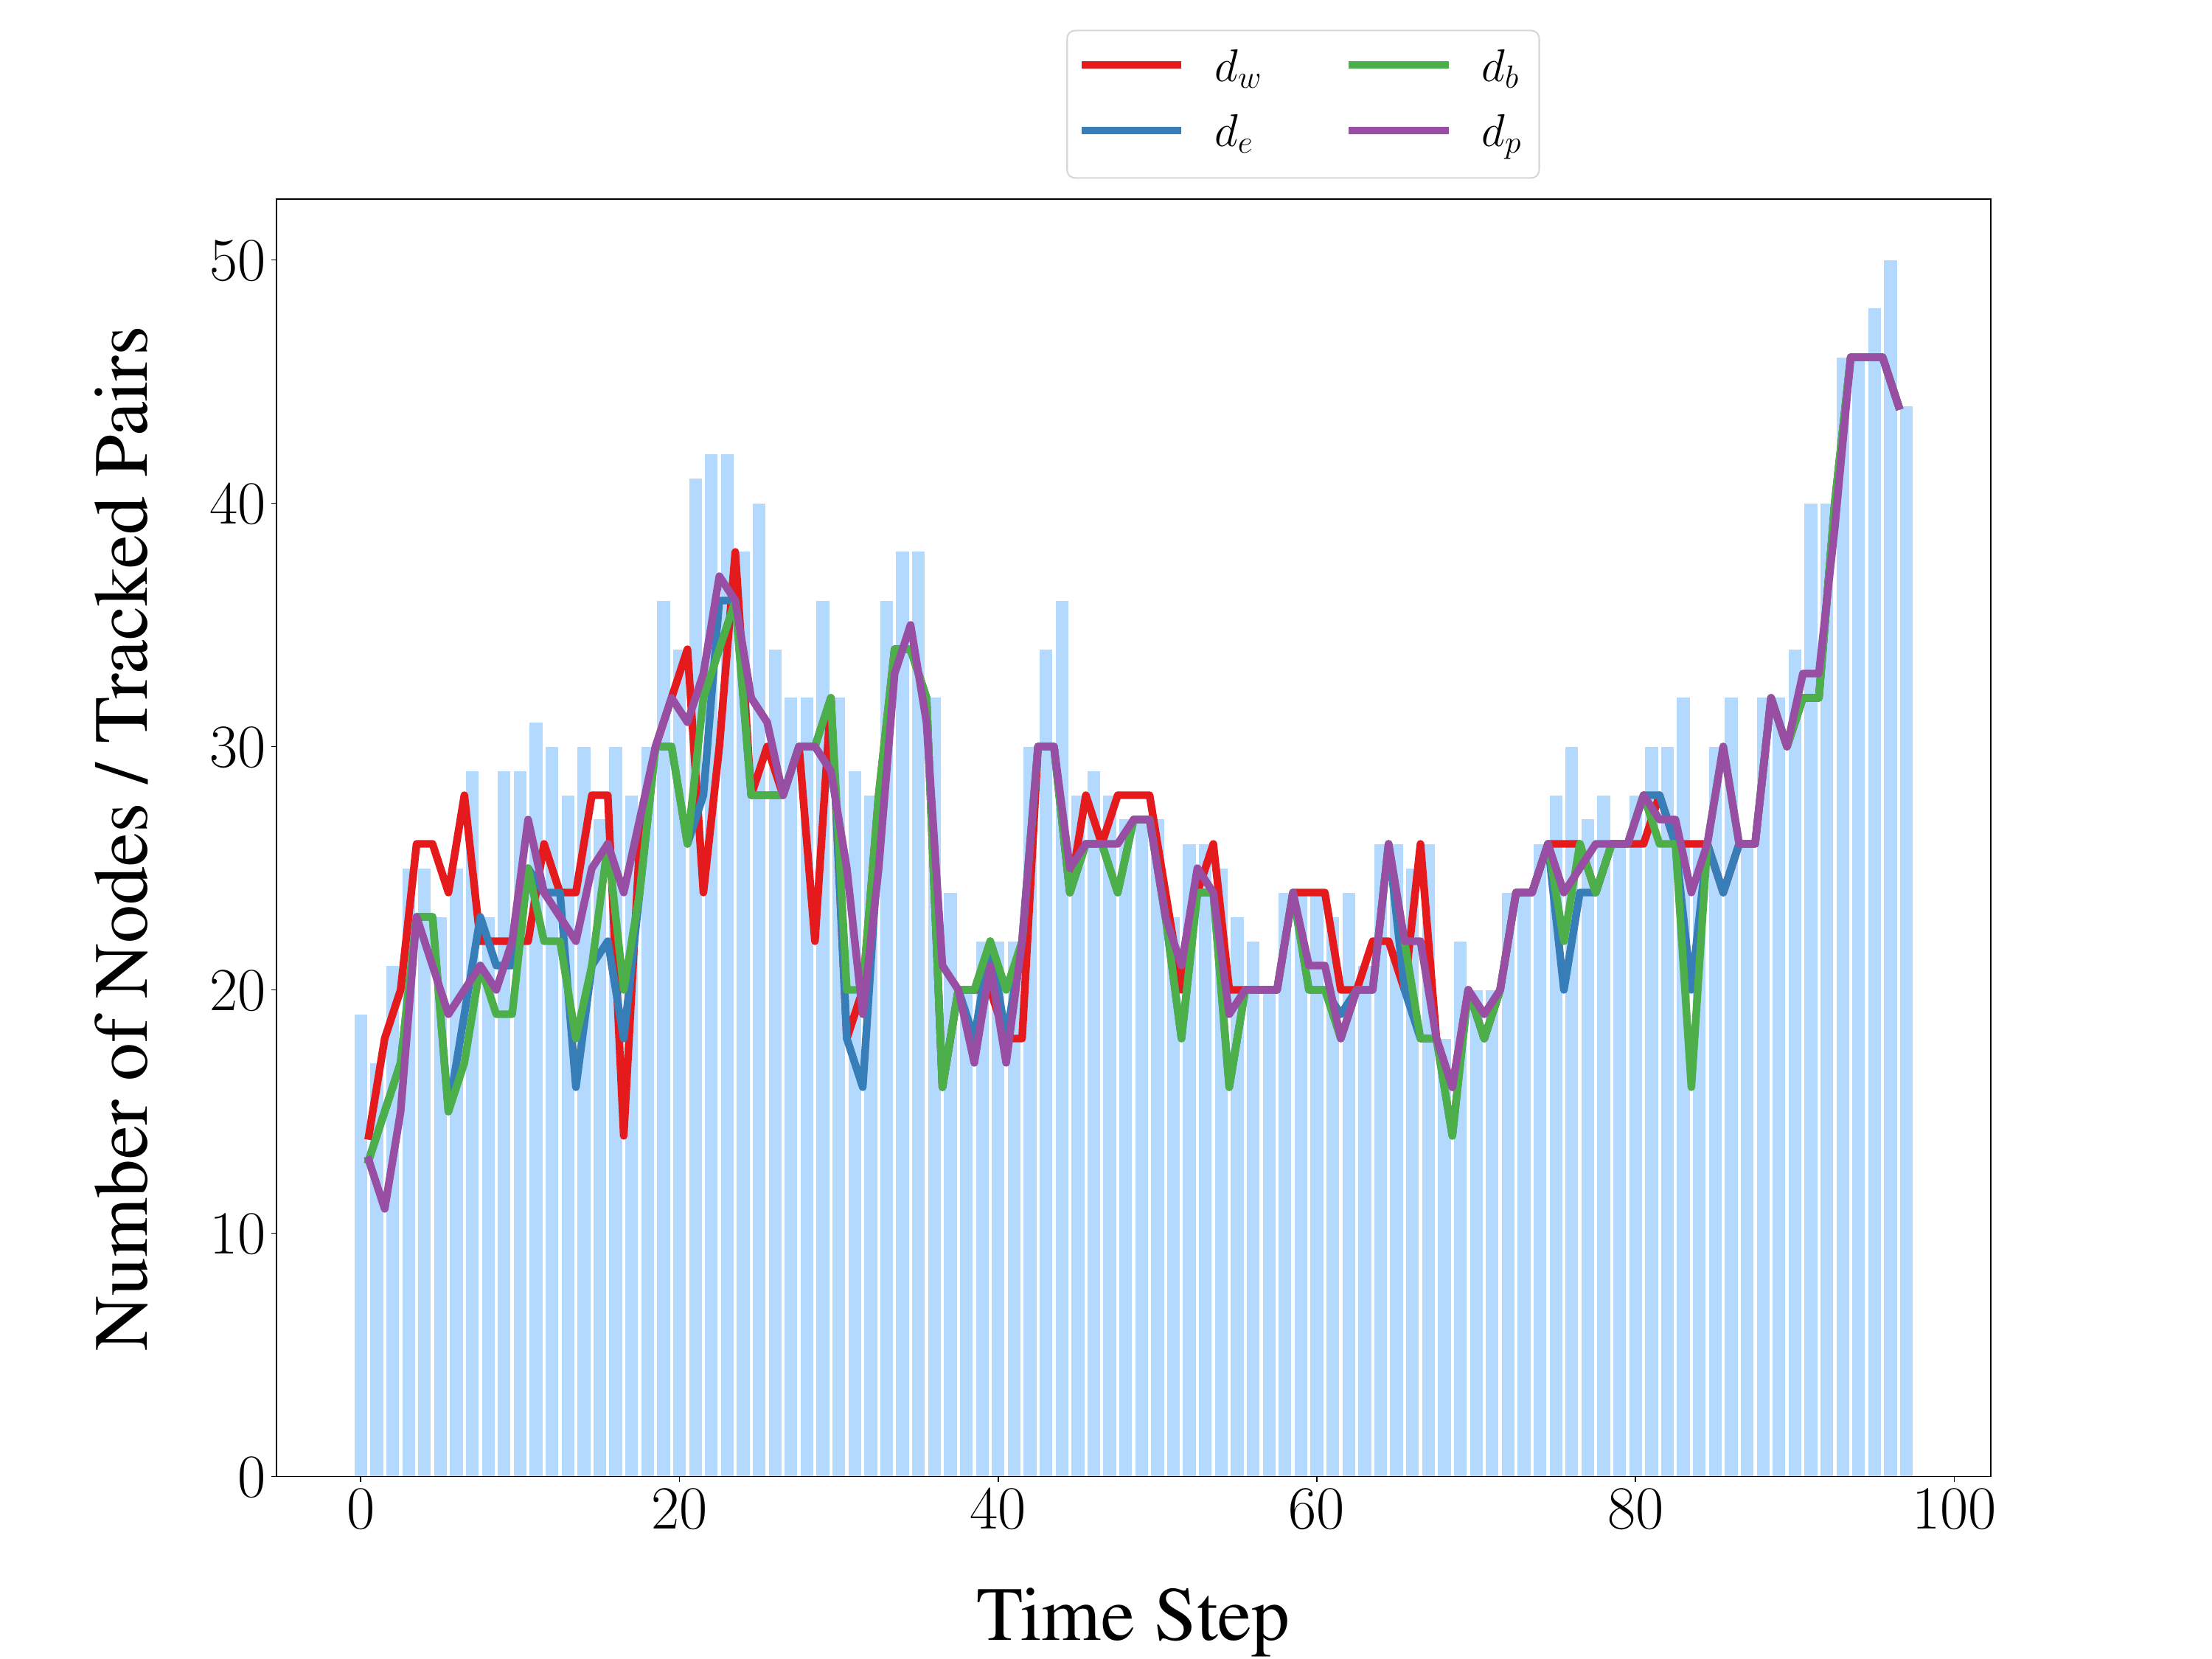}
\caption{
    Number of tracked nodes (colored and labeled) 
    relative to the total nodes of merge trees (light blue bars)
    for \dataset{IonizationFront2D}.
}
\label{fig-IonizationFront2DAllNodes}
\end{figure}

\begin{figure}
\centering
\includegraphics[width=0.8\linewidth]{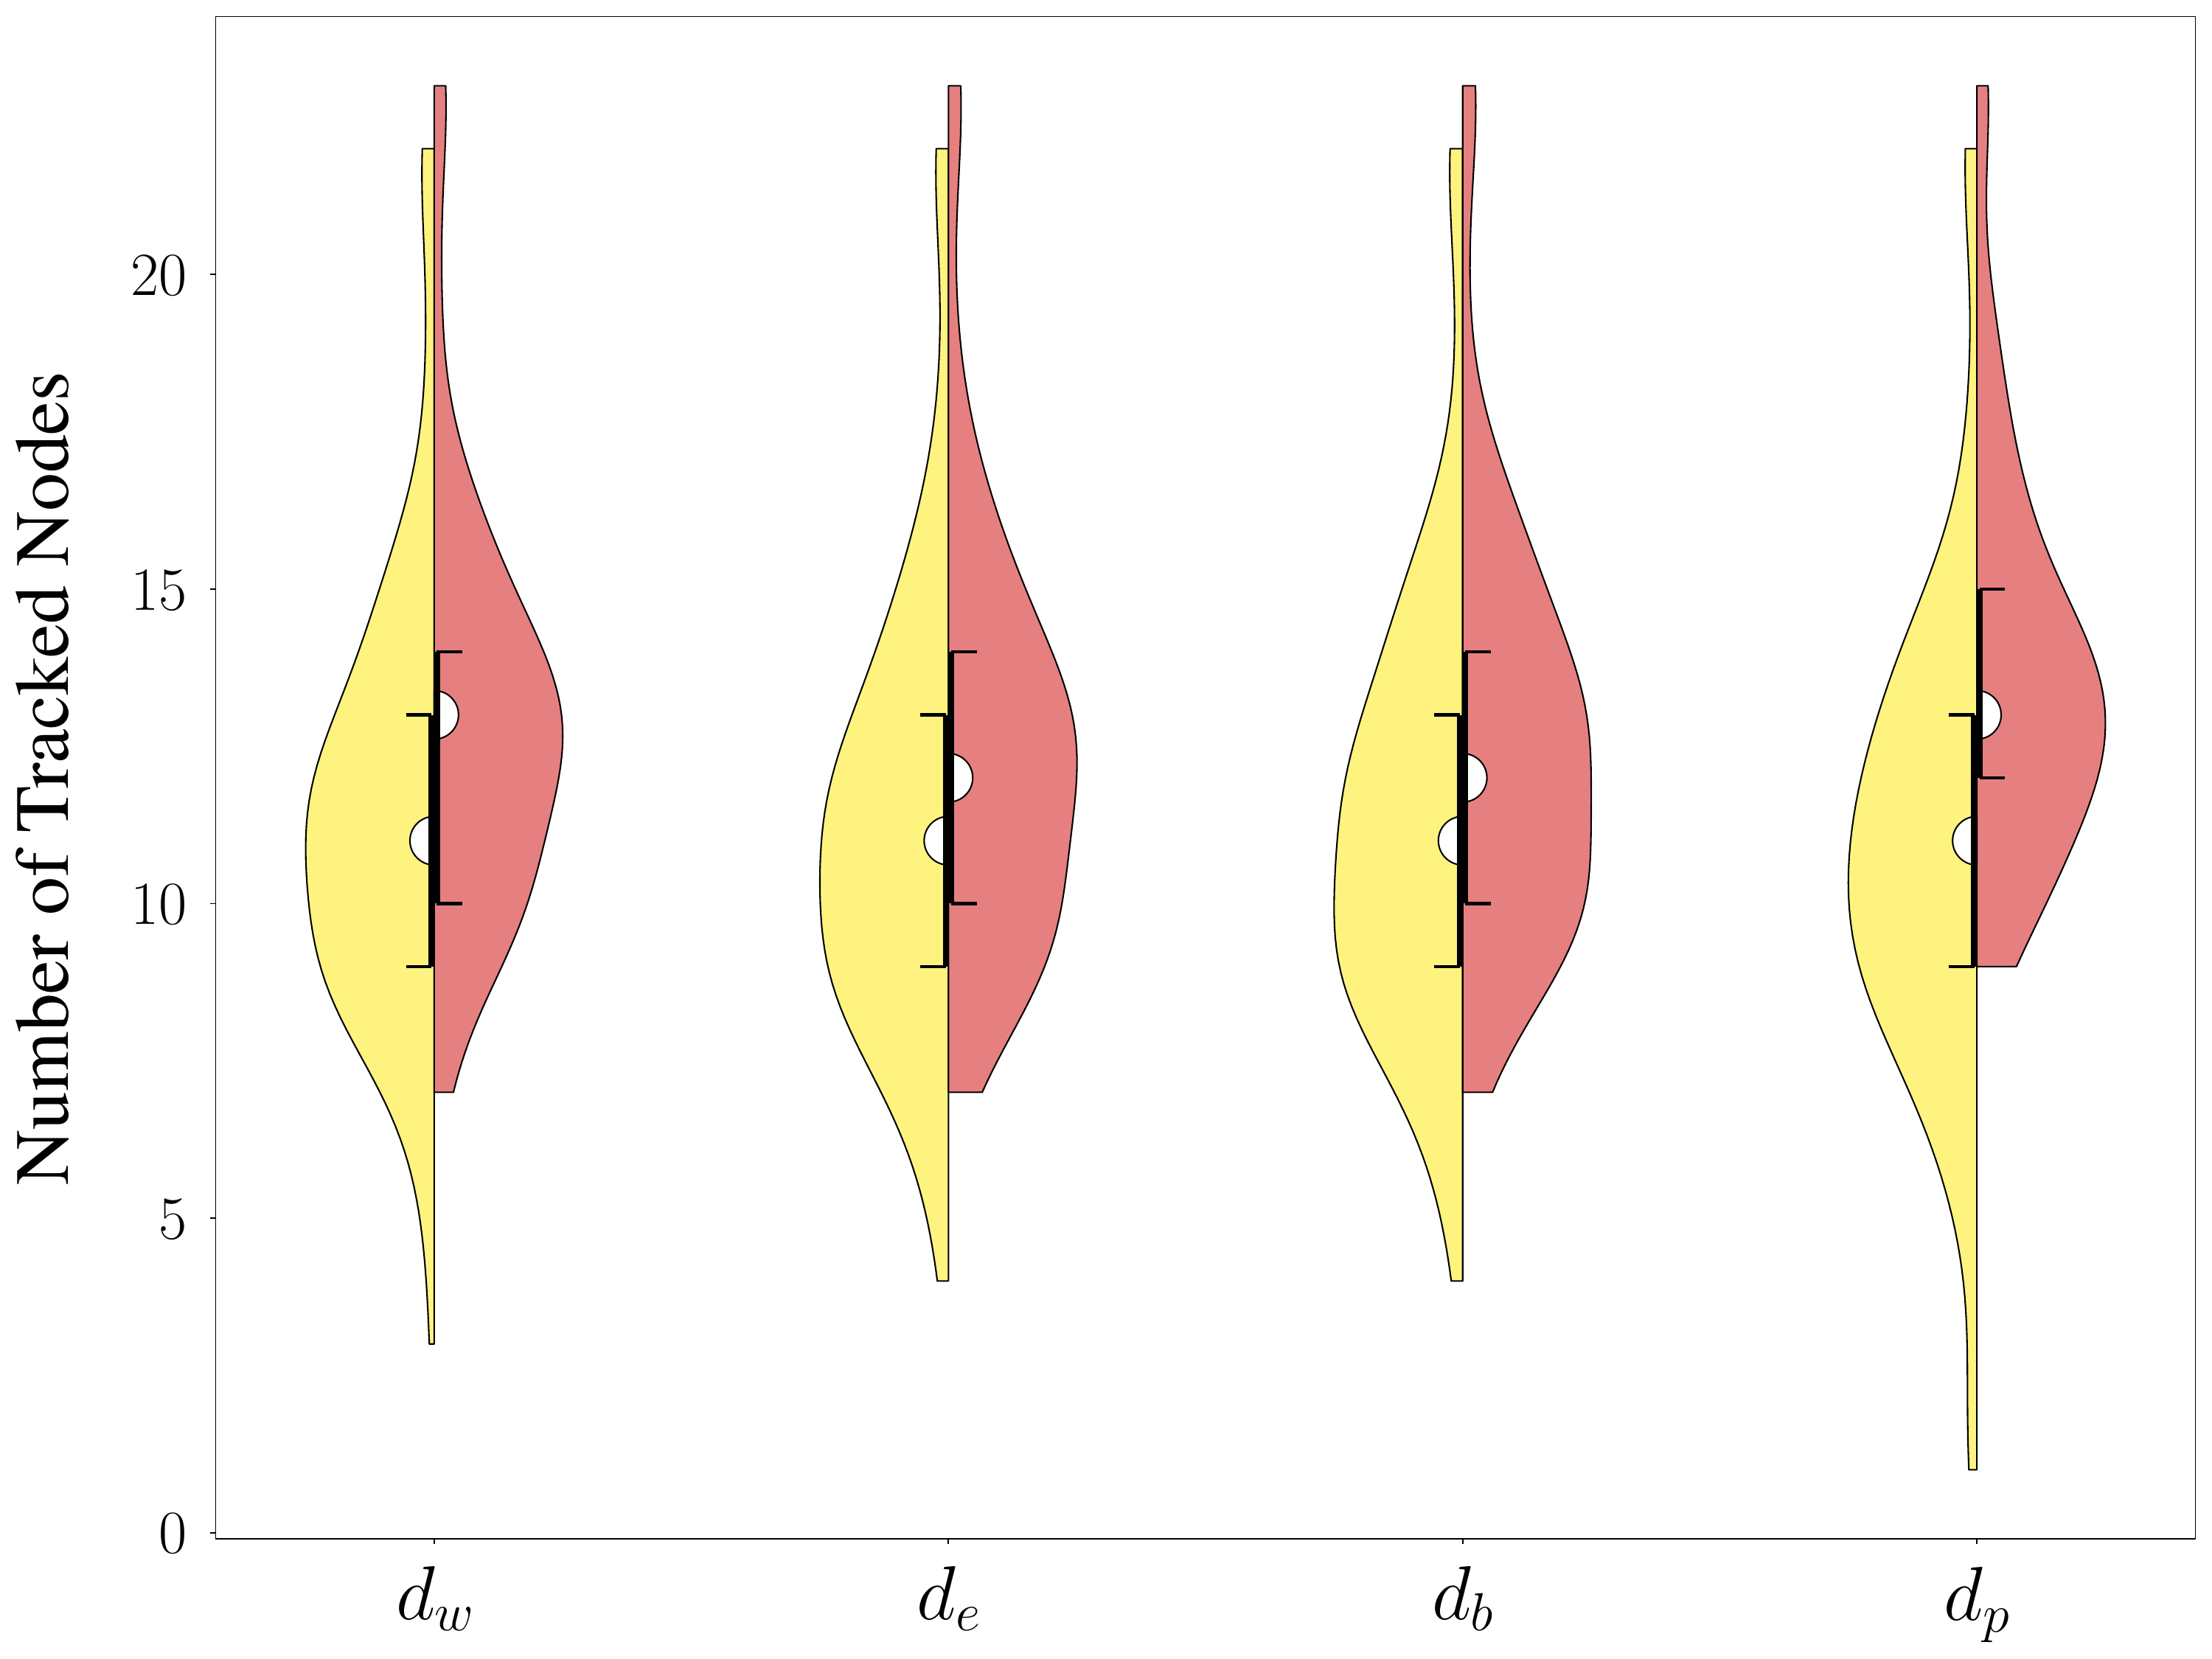}
\caption{
    Distributions of tracked nodes 
    over the chosen time steps of \dataset{IonizationFront2D},  
    divided by types:
    saddle (yellow) and maxima (red).
}
\label{fig-IonizationFront2DViolin}
\end{figure}

% Length histogram
\begin{figure}%
\begin{subfigure}[t]{\ltwopicwidth}%
\includegraphics[width=\ltwopicwidth]{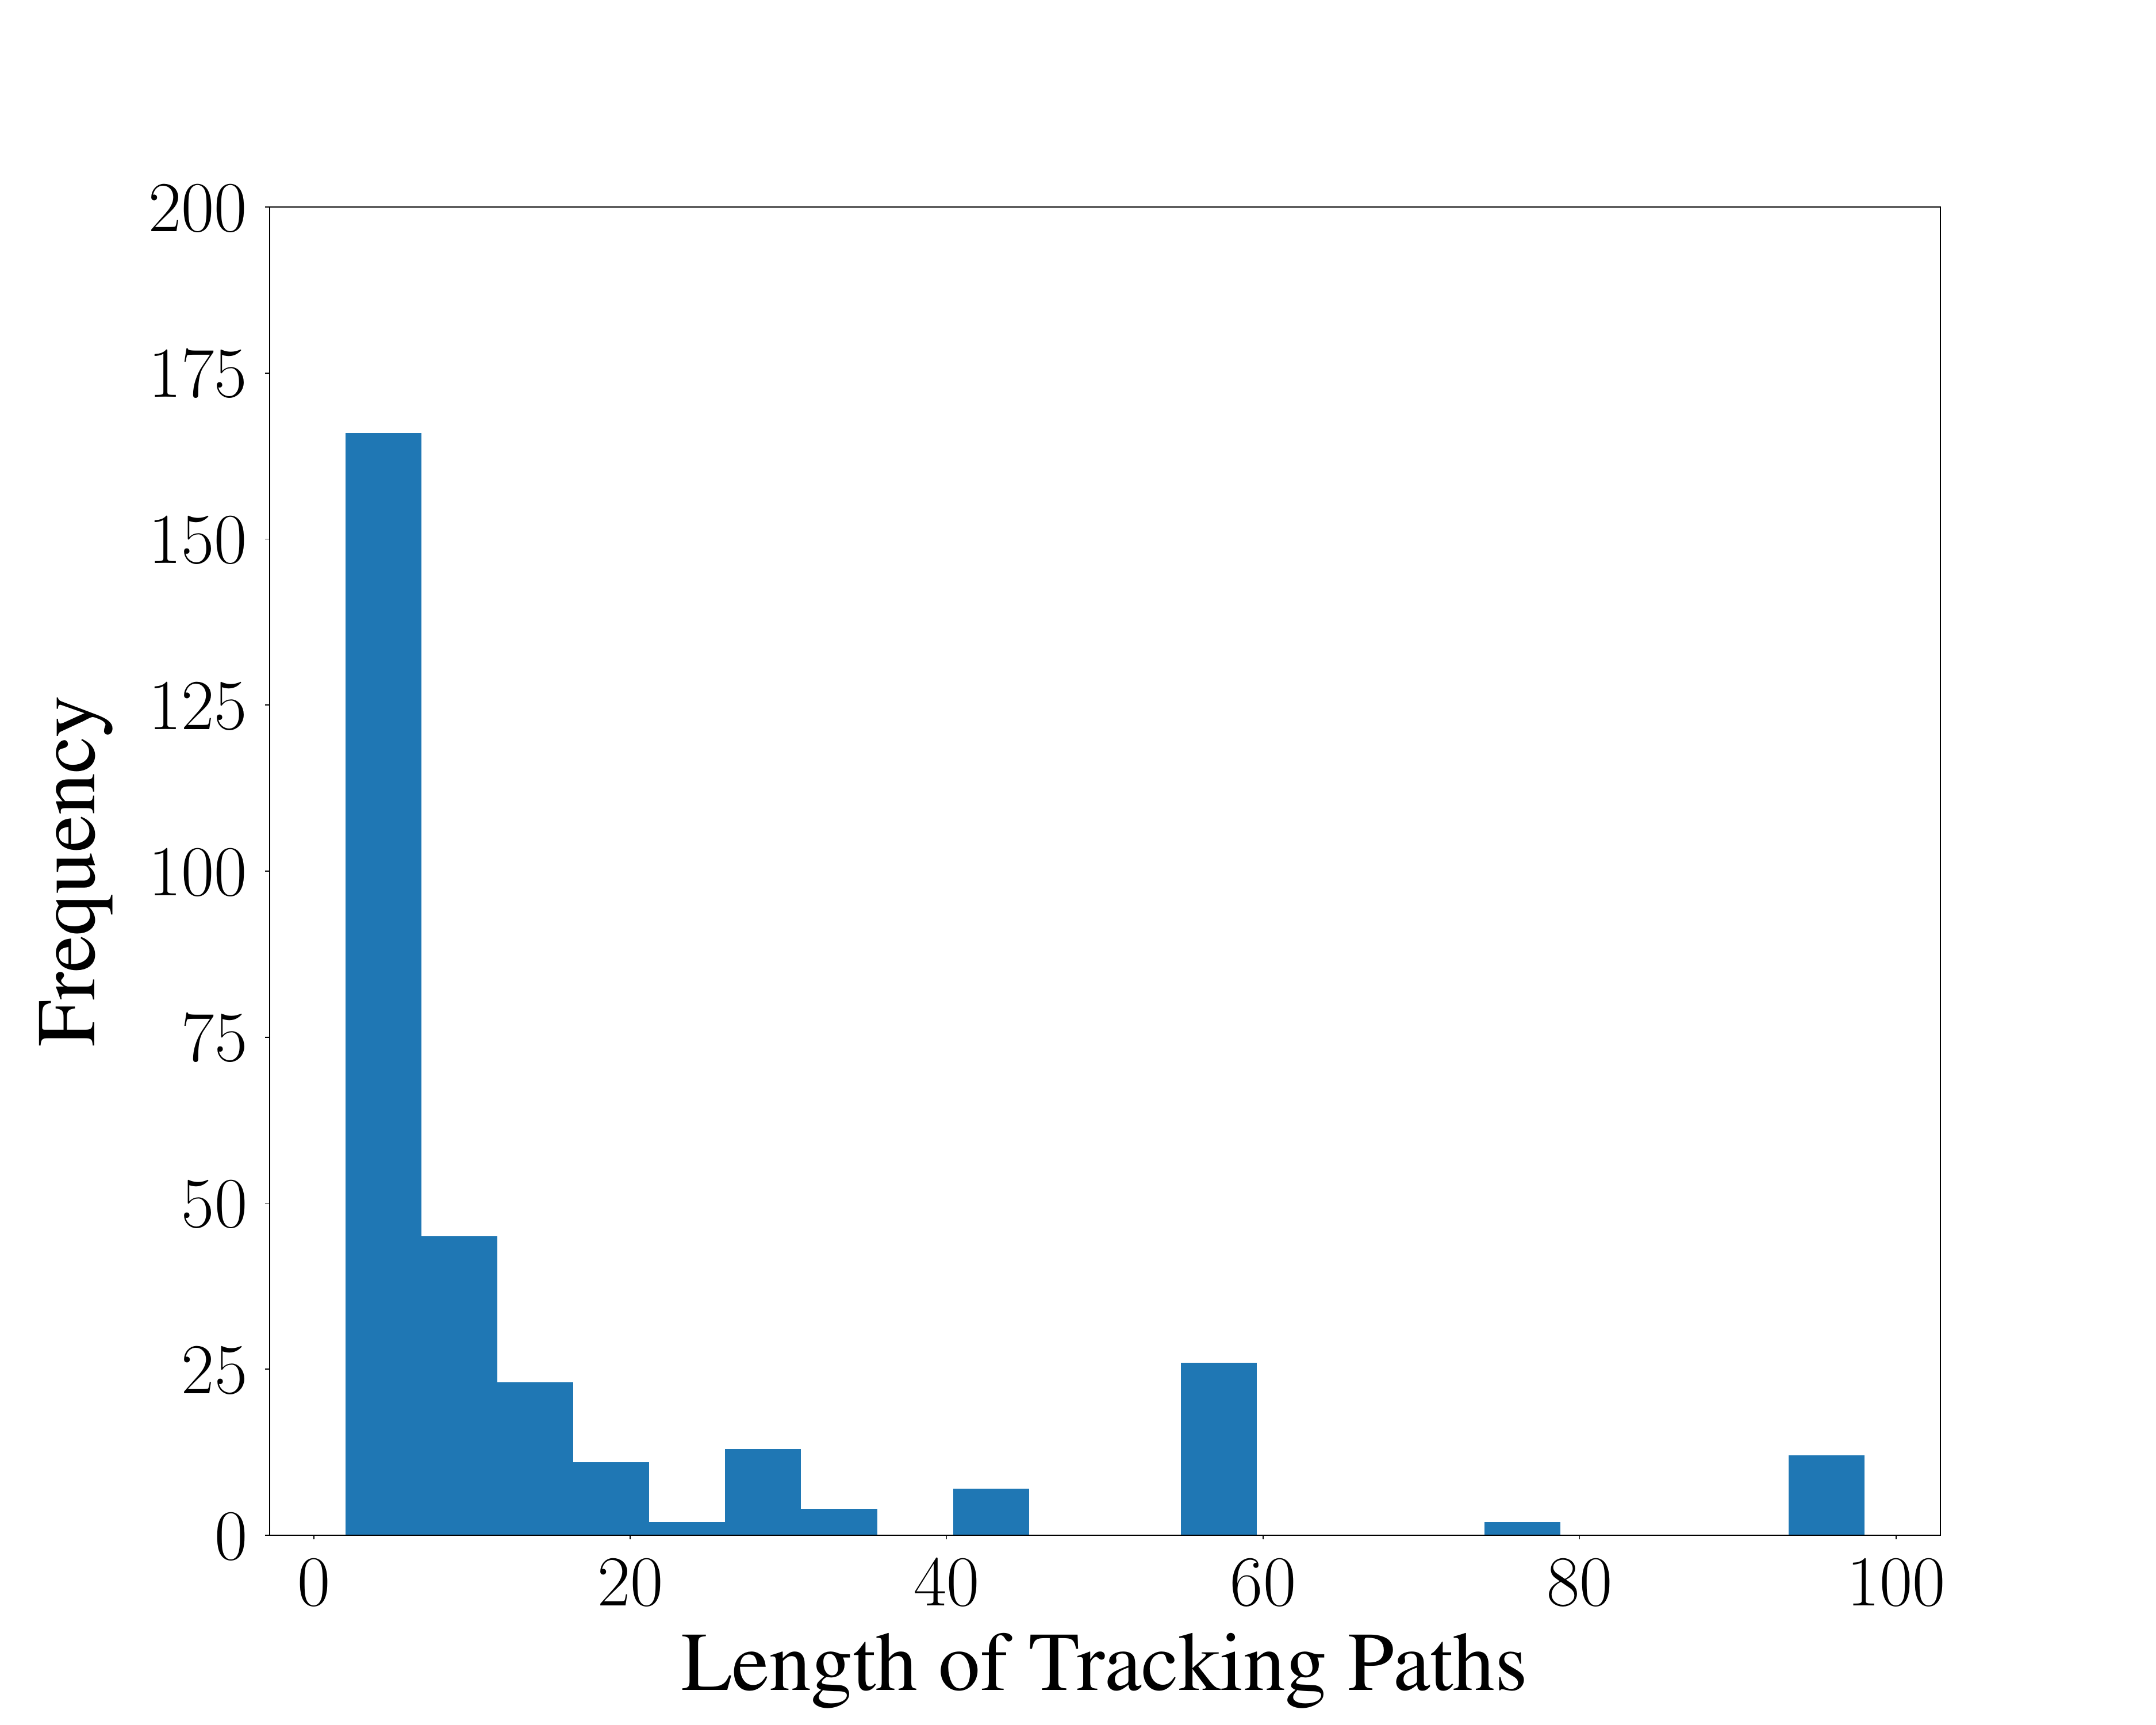}
\caption{$d_w$.}%
\label{fig-LengthHistogramIonizationFront2DW}%
\end{subfigure}
\hfill%
\begin{subfigure}[t]{\ltwopicwidth}%
\includegraphics[width=\ltwopicwidth]{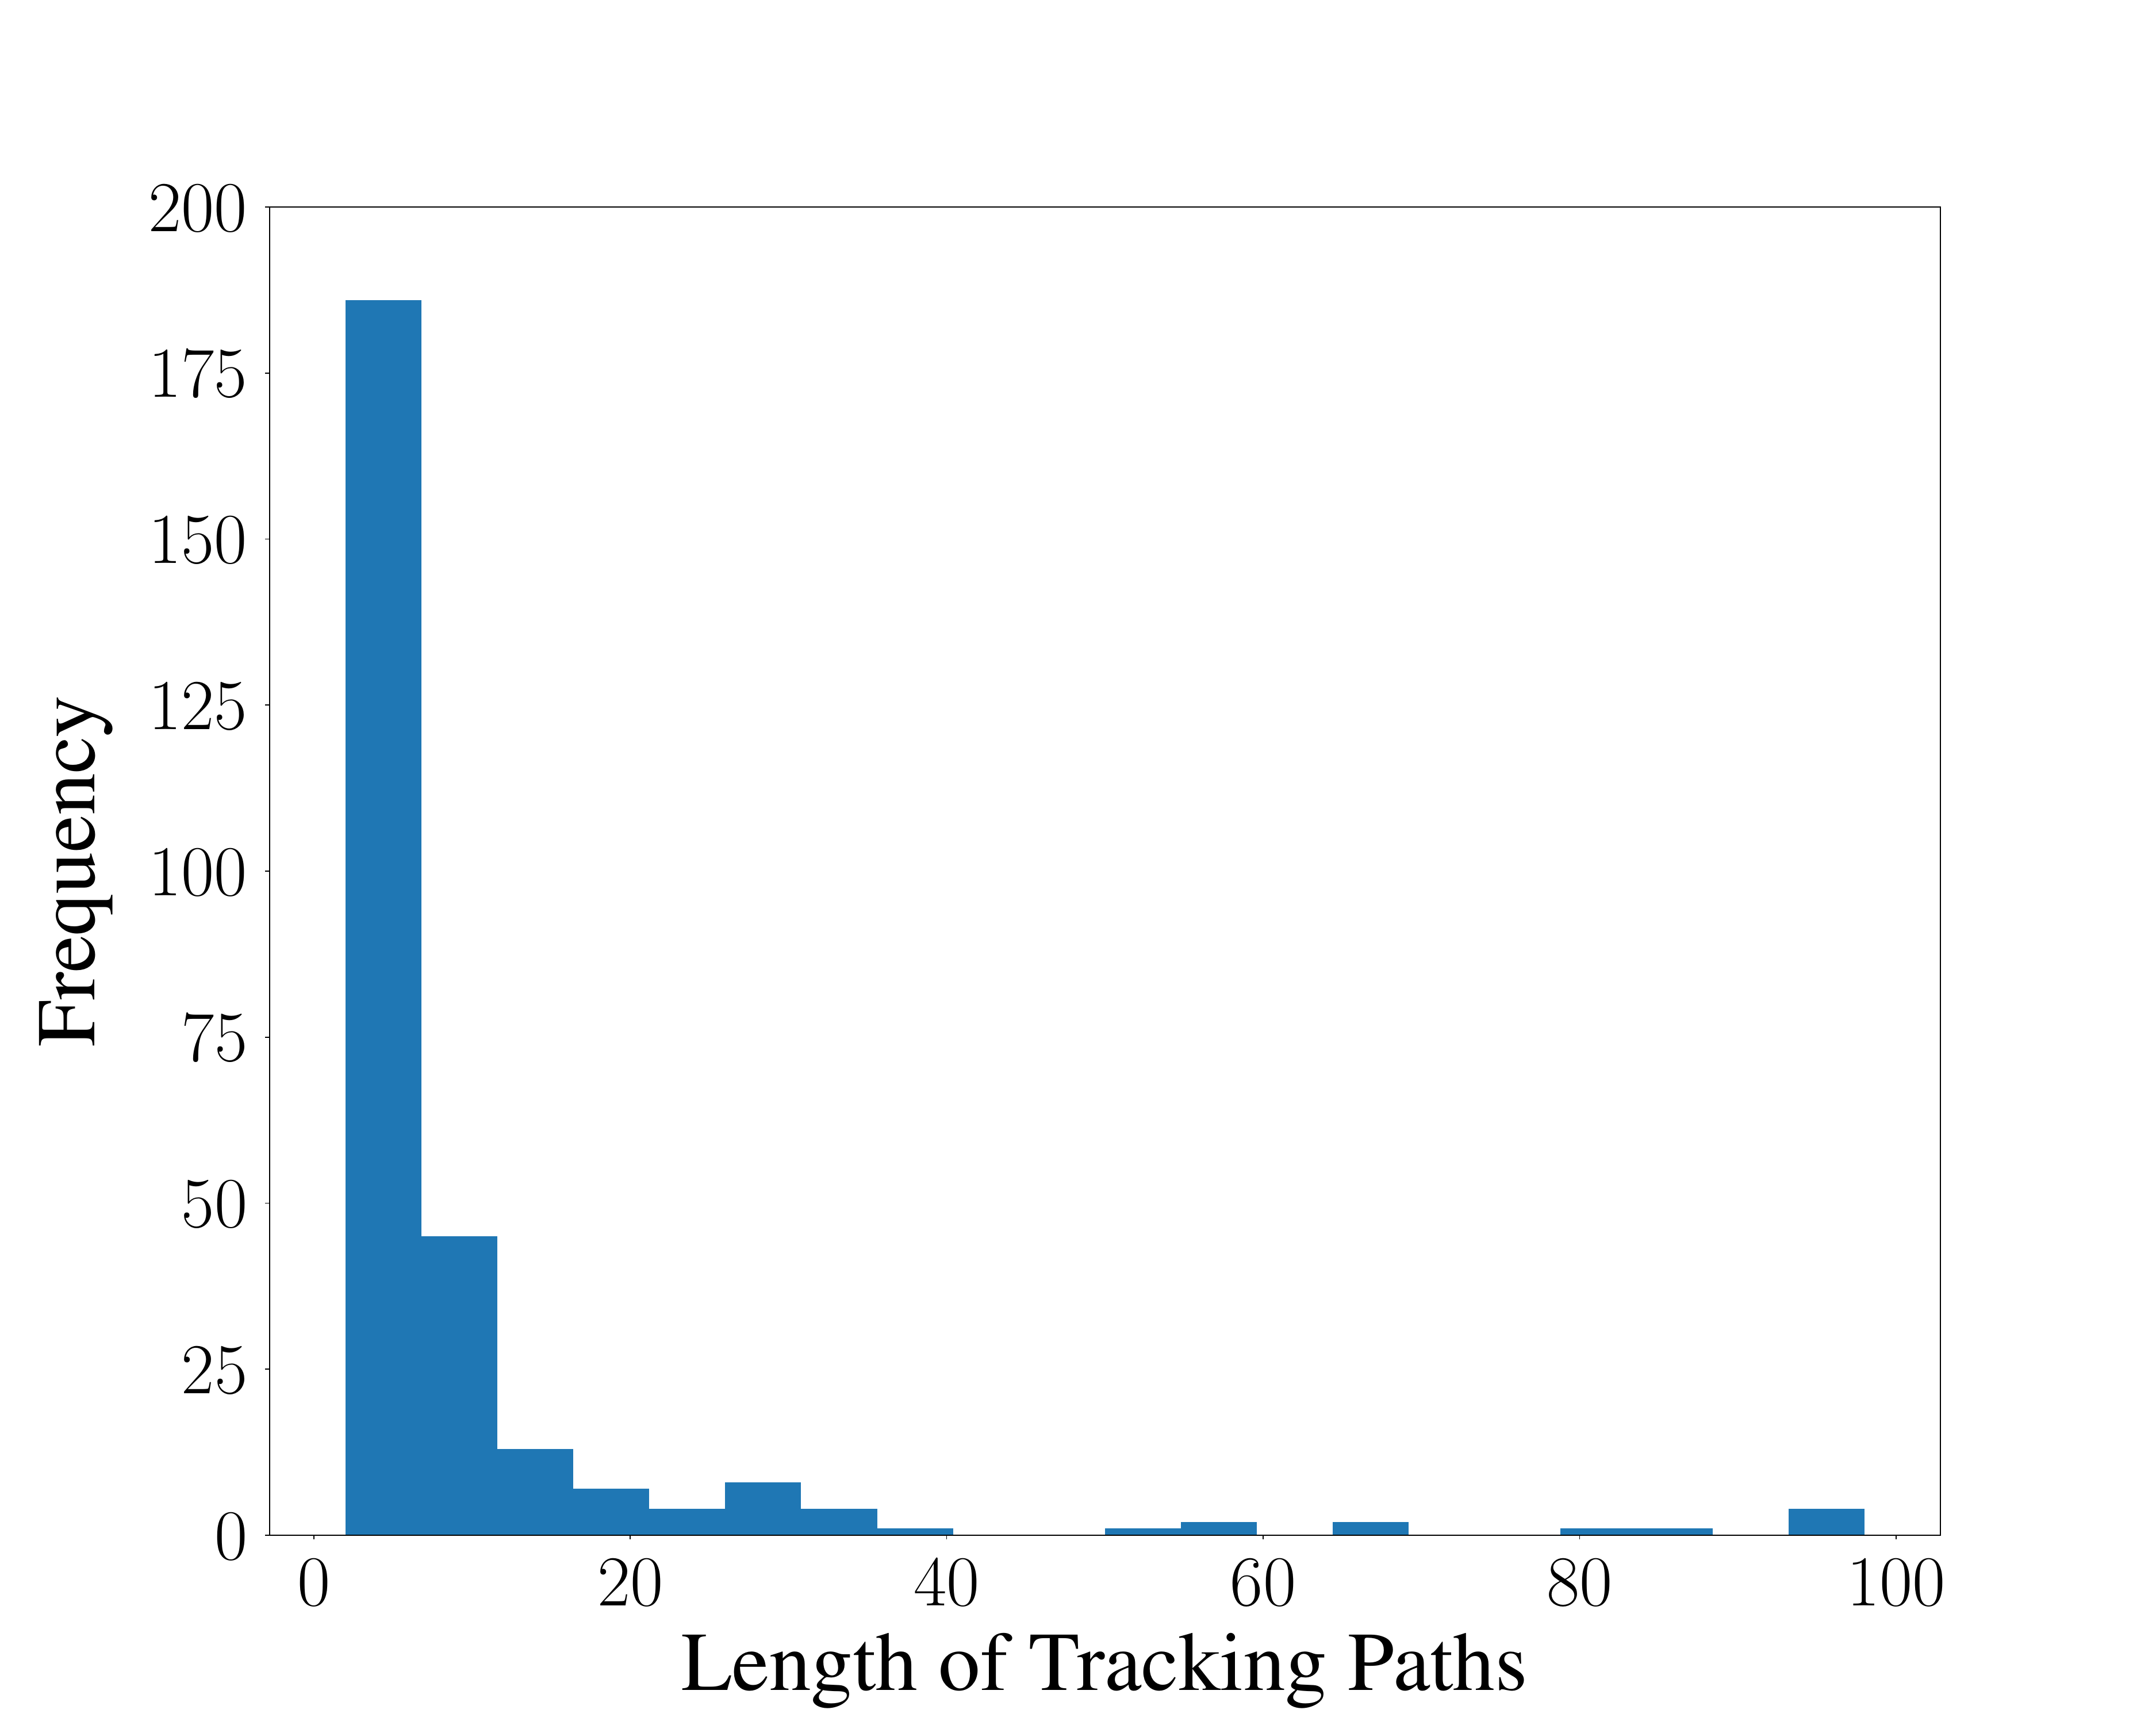}%
\caption{$d_e$.}%
\label{fig-LengthHistogramIonizationFront2DE}%
\end{subfigure}%
\\%
\begin{subfigure}[t]{\ltwopicwidth}%
\includegraphics[width=\ltwopicwidth]{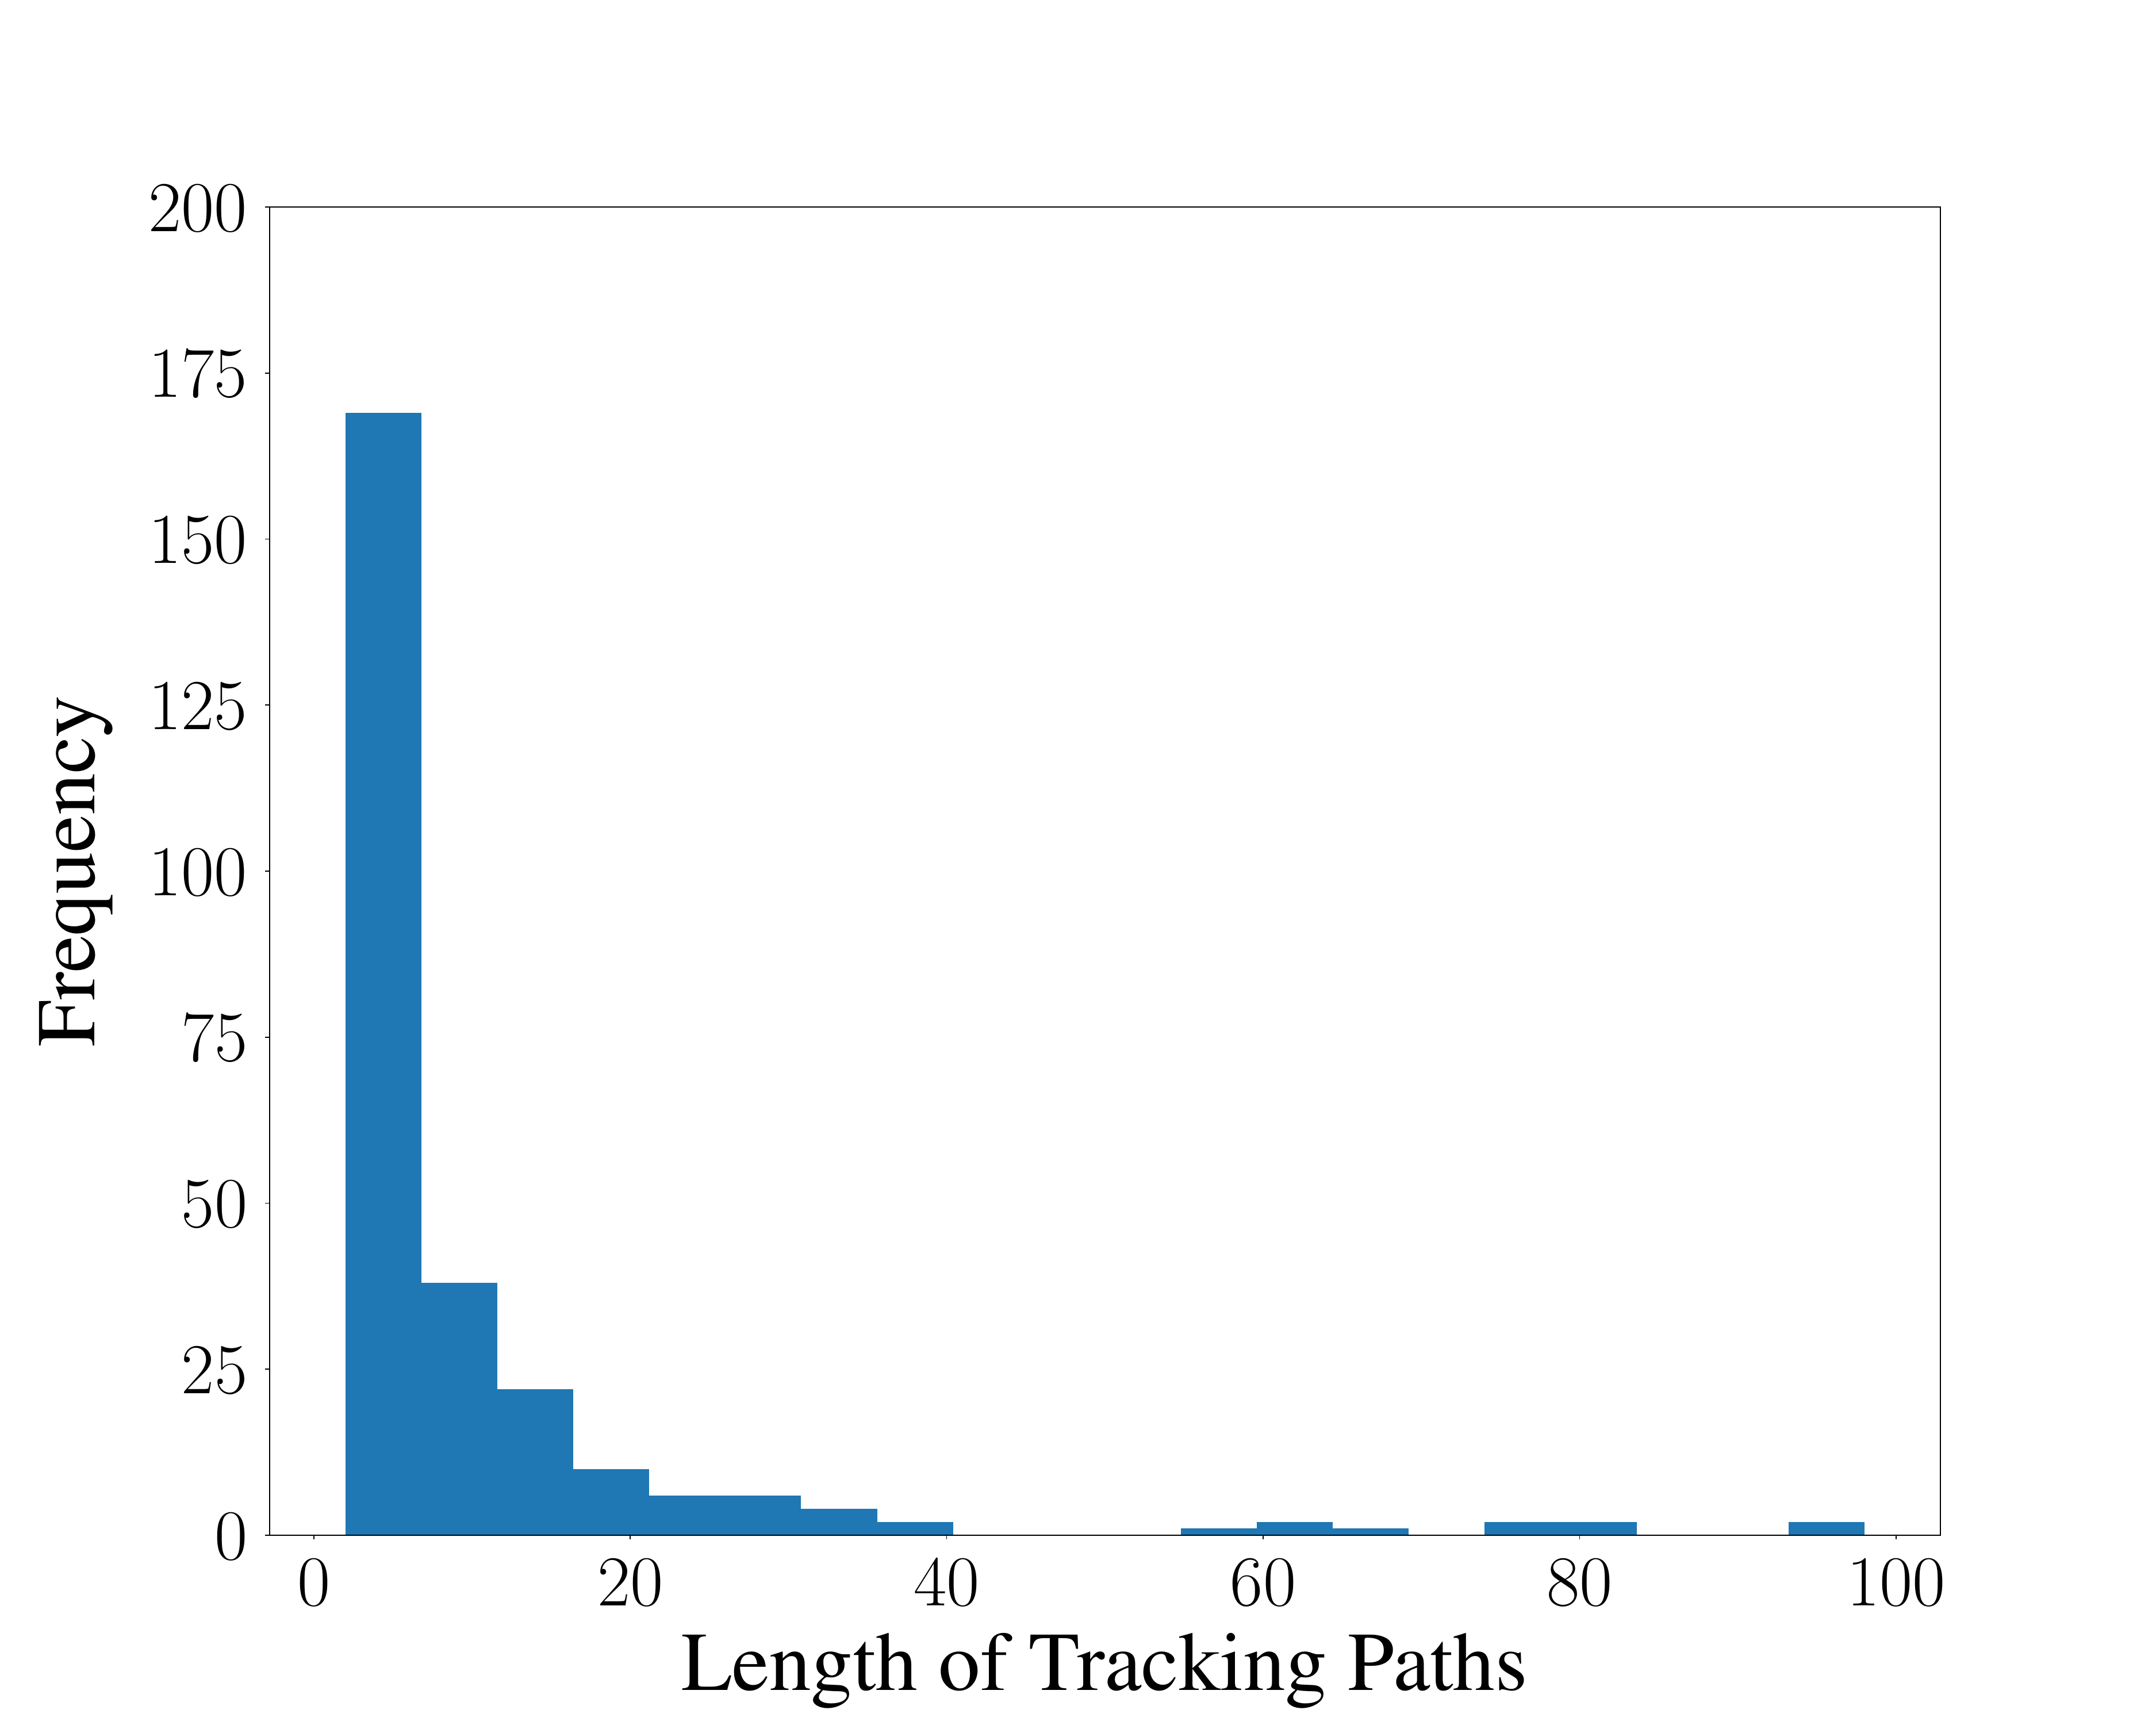}%
\caption{$d_b$.}%
\label{fig-LengthHistogramIonizationFront2DB}%
\end{subfigure}%
\hfill%
\begin{subfigure}[t]{\ltwopicwidth}%
\includegraphics[width=\ltwopicwidth]{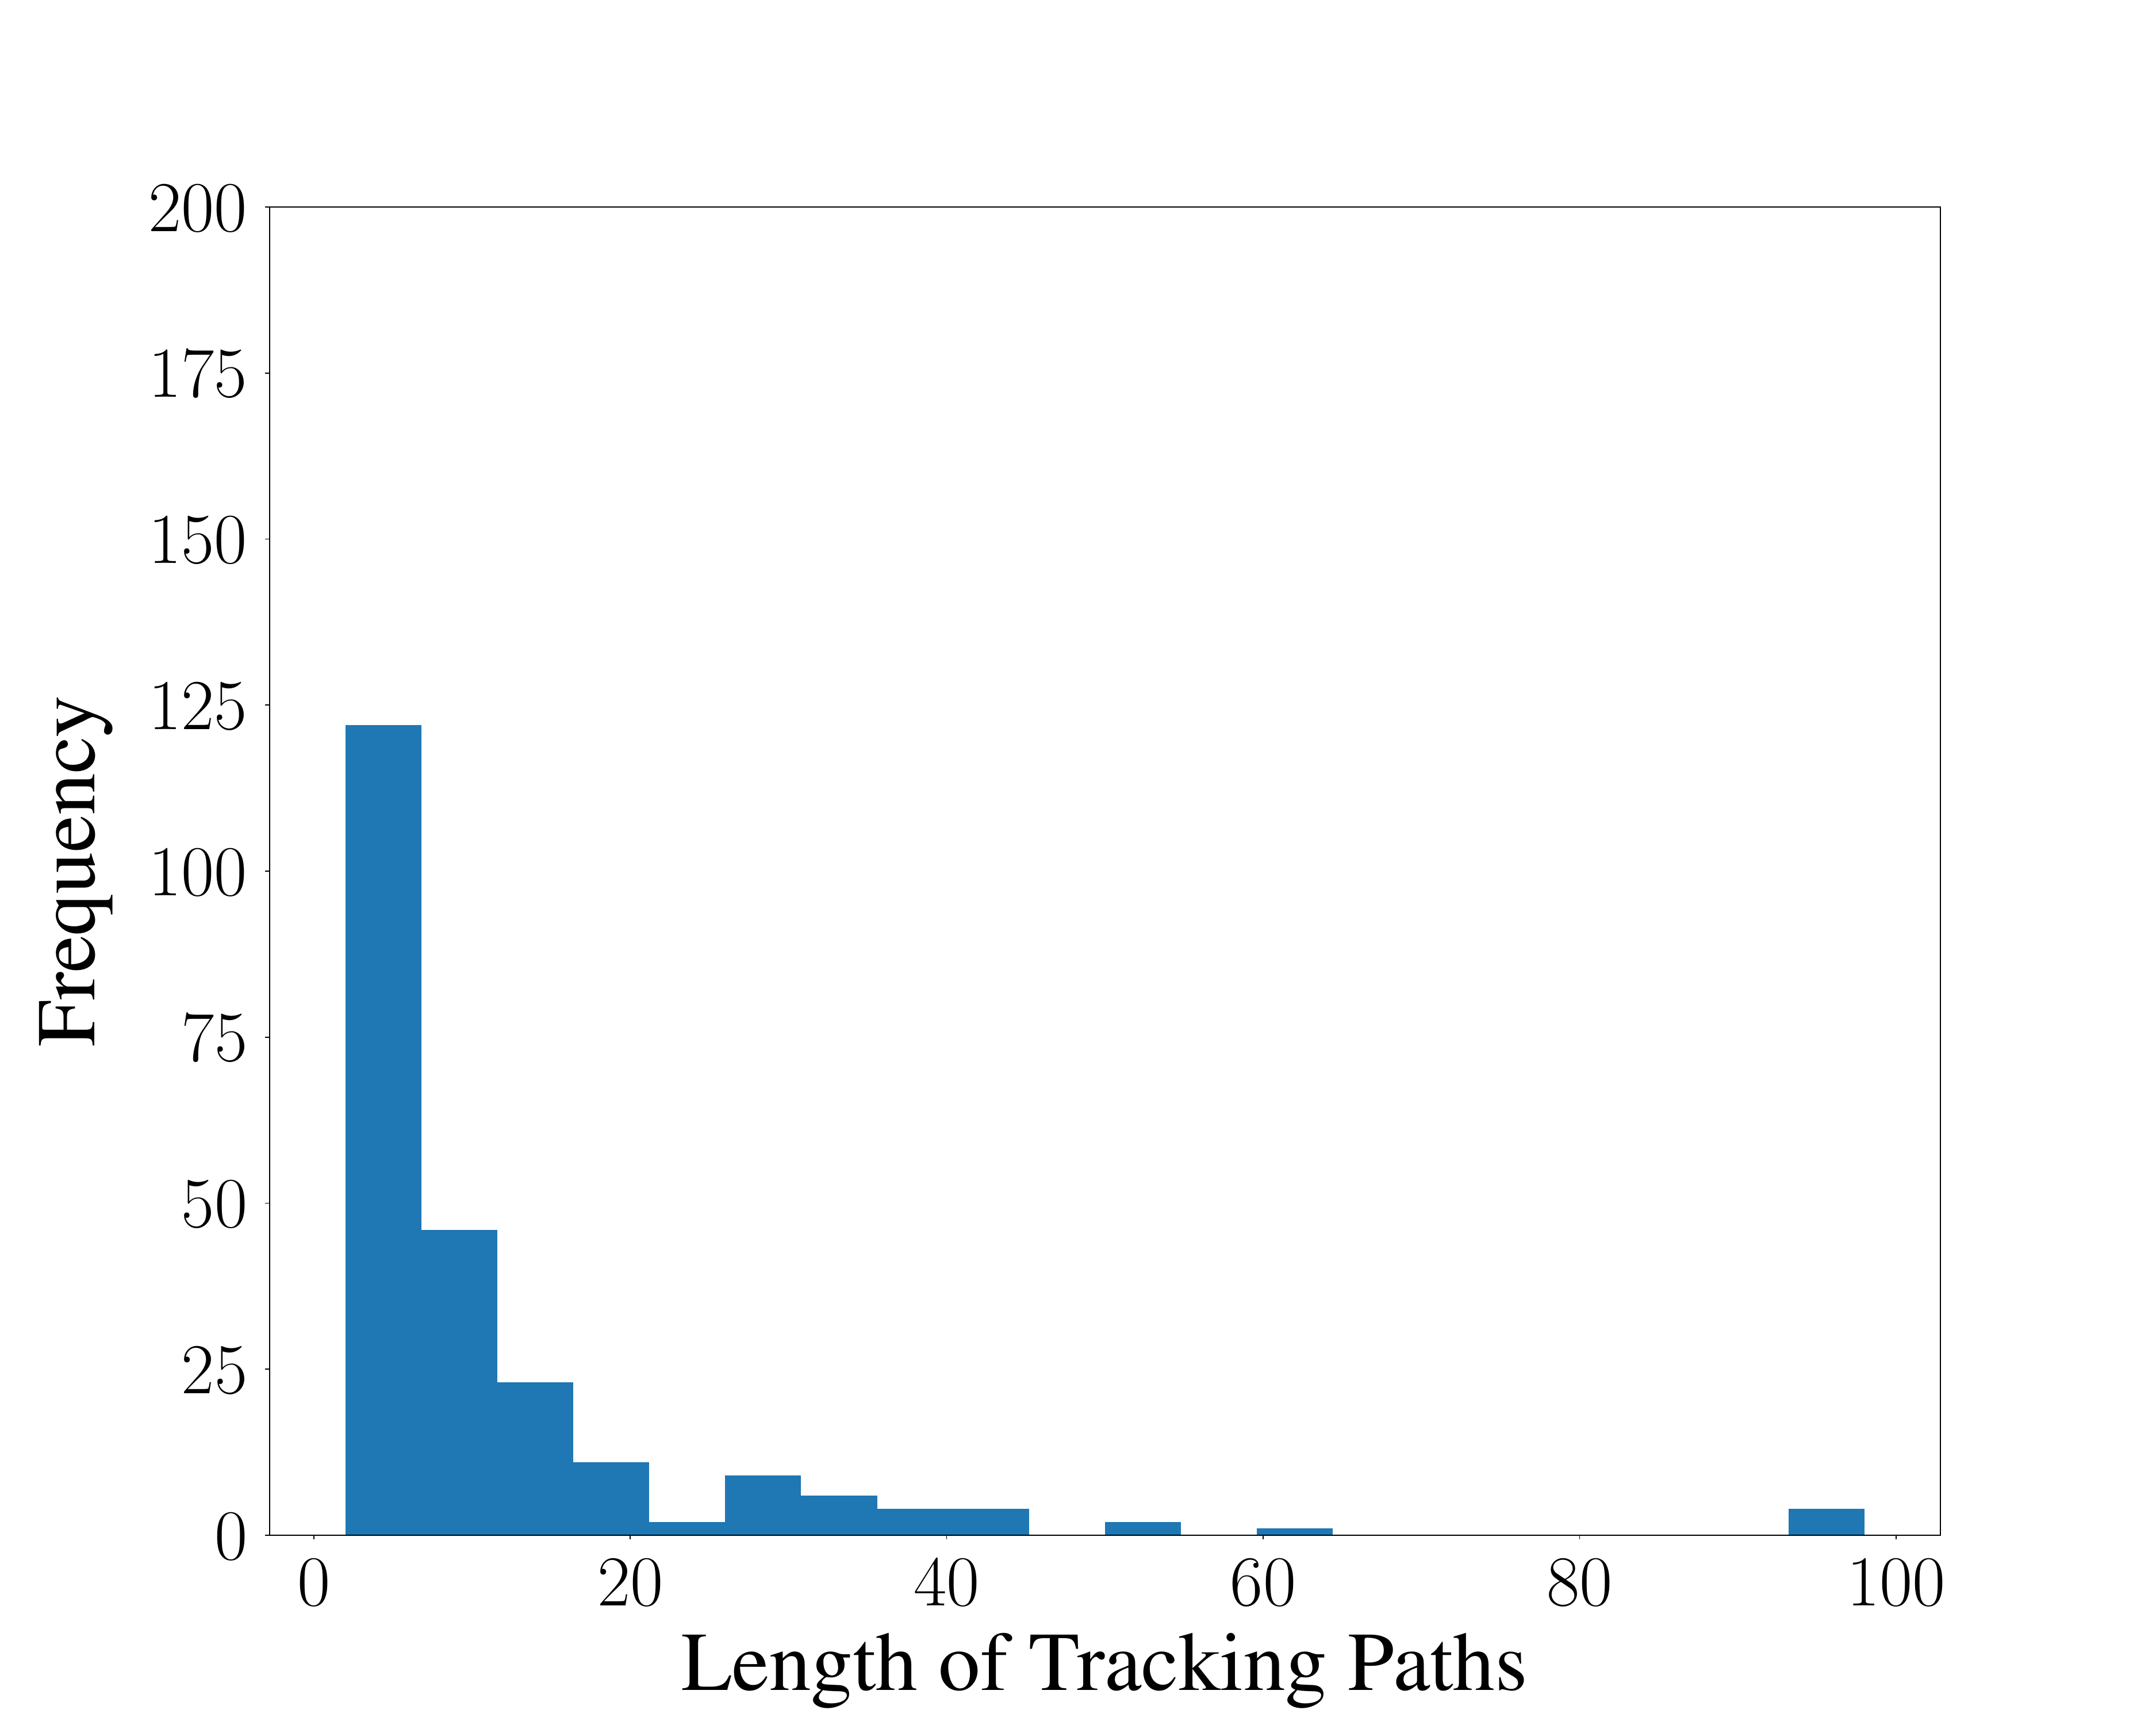}%
\caption{$d_p$.}%
\label{fig-LengthHistogramIonizationFront2DP}%
\end{subfigure}%
\caption{Histograms of the length of the tracking paths of the first $100$ time steps 
    of \dataset{IonizationFront2D}.}%
\label{fig-LengthHisgoramIonizationFront2D}%
\end{figure}

\begin{figure}
\centering
\includegraphics[width=0.8\linewidth]{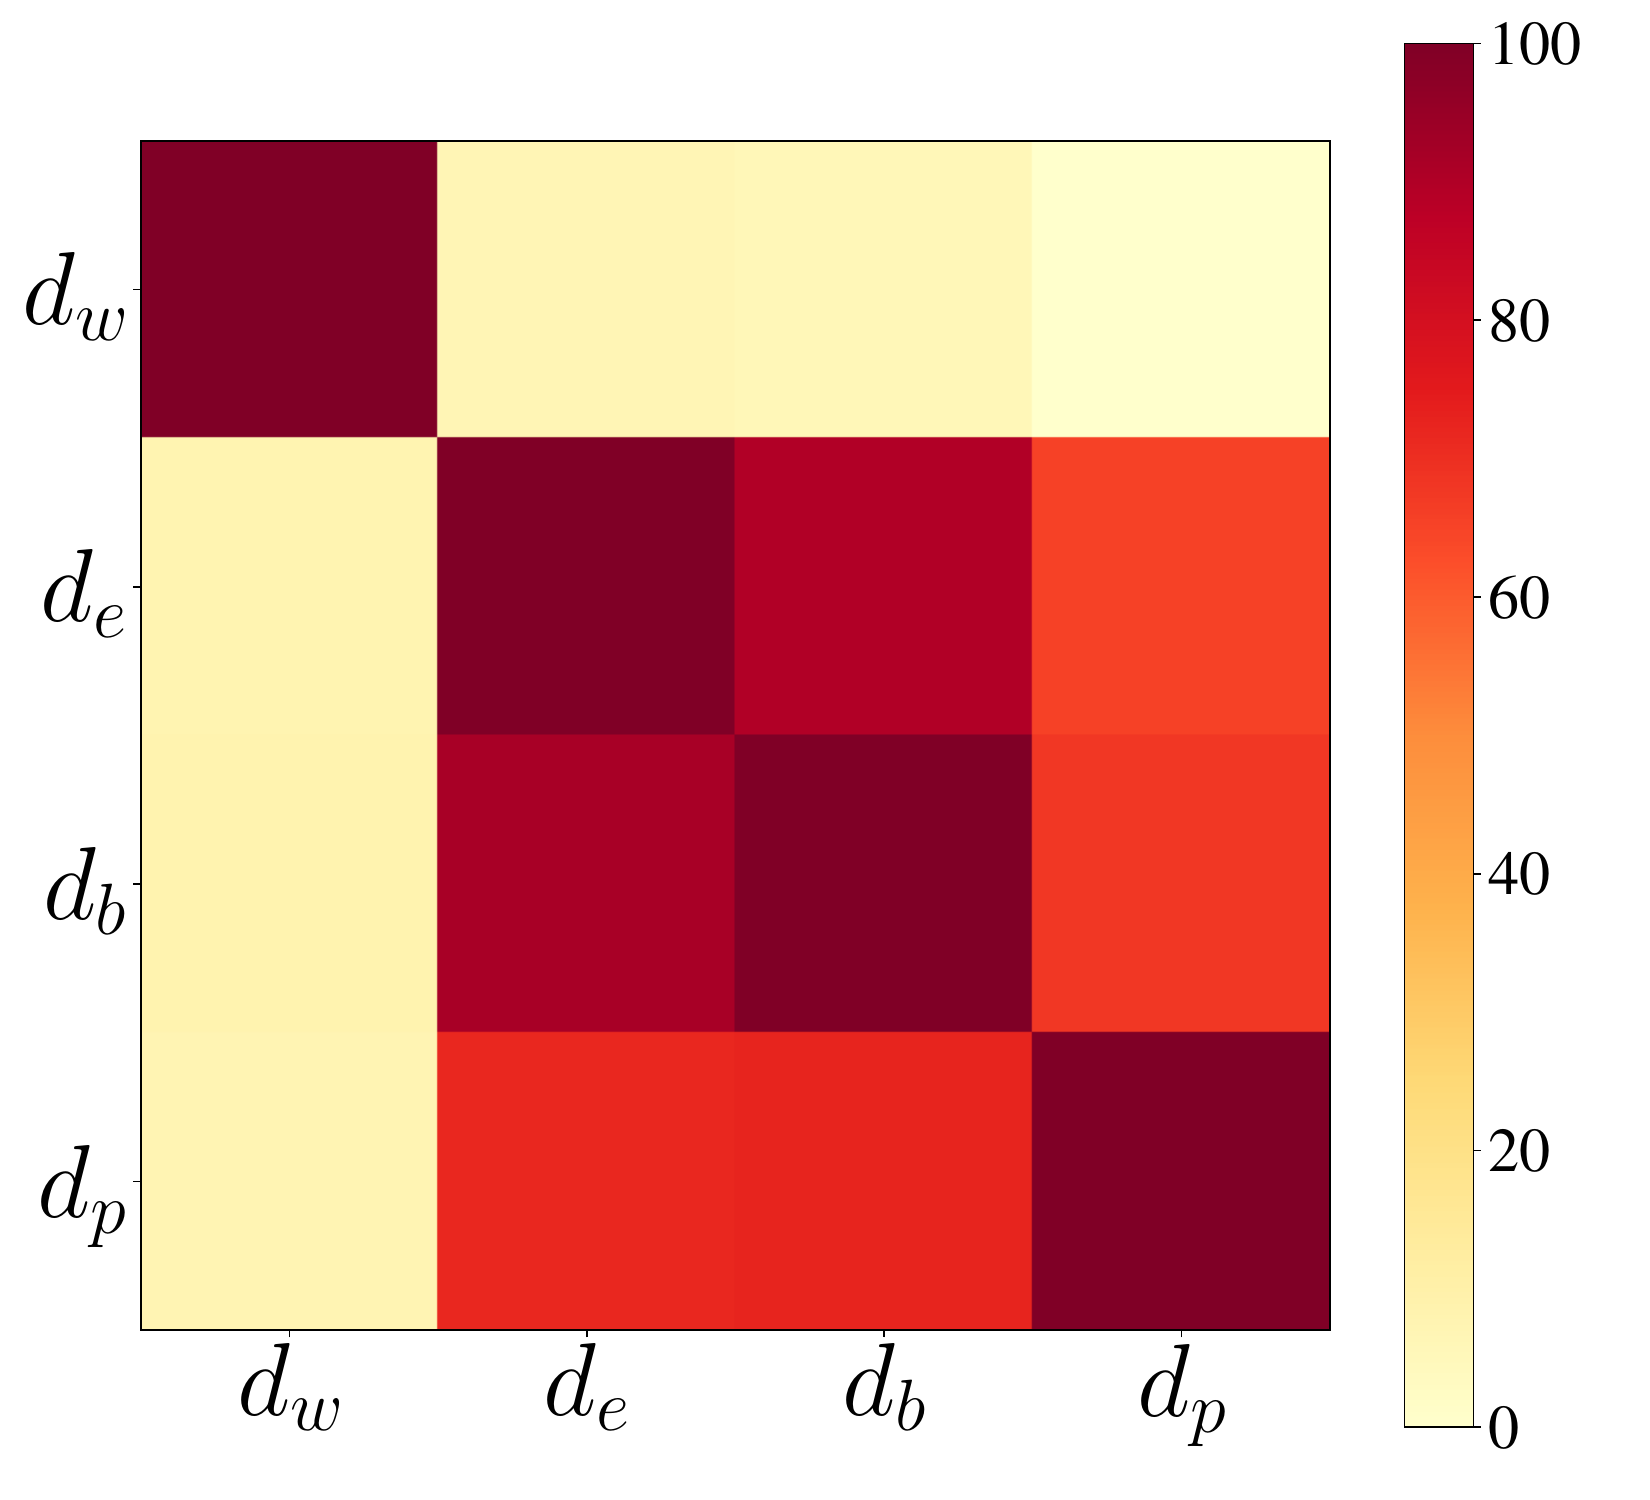}
\caption{
    Pairwise differences between the methods on the columns
    in relation to the methods on the rows
    for \dataset{IonizationFront2D}.
}
\label{fig-IonizationFront2DSimilarities}
\end{figure}
