# Supplementary material for: A Comparative Study of Different Edit Distance-Based Methods for Feature Tracking using Merge Trees on Time-Varying Scalar Fields
Source: arXiv:2509.17974 source file (2025-10-12)
Supplement: Supplementary file 8 [file supp_extraData.tex]

\section*{Extra Results on Real-World Data Set}
We introduce information on the data sets used in this section,
followed by the results for each of them. 

\dataset{IonizationFront2D} is a simulated 2D scalar field 
from 2008 SciVis Contest \cite{whalen2008competition},  
The results 
capture the formation of the first stars in the universe 
through density variations of the so-called ionization front.
We use the first $100$ time steps for our experiment.
The split trees can be used to map the regions with similar density
as the shadow instability progresses.

\dataset{Storms2D} depicts a one-hourly mean sea level pressure 
over the month of December 1999. This data set is available to download at 
\cite{ERA5data}. Similar to K\"opp and Weinkauf \cite{koepp22},
the mean over eight days is computed and a light Gaussian smoothing is applied.
This process creates a time-dependent 2D scalar field with 743 time steps.
The structural changes in join trees over time 
provide insight into the formation and evolution of storms.

\dataset{Boussinesq2D} is a simulation of a flow generated 
by a heated cylinder \cite{Guenther17} over $2001$ time steps
using Gerris flow solver \cite{germer11a}.
It is a time-dependent vector field and 
contains numerous small vortices rotating around each other.
Using the last $1000$ time steps, we compute and 
track the evolution of join trees of the velocity magnitude,
as their nodes associate with the vortex centers.

\dataset{Cylinder3D} originates from a simulation of 3D turbulent flow 
around a half-cylinder. \cite{BaezaRojo19SciVisa} with
the Reynolds number of $640$. 
It contains $151$ time steps.
The split trees are employed to track the temporal evolution of the 
local maxima and saddle points of the velocity magnitude.

\dataset{Tangaroa3D} captures the 3D flow around a research vessel Tangaroa
over $200$ time steps \cite{PopinetEtAl2004_Tangaroa}.
Similar to Cylinder3D, we also compute the magnitude of the velocity
to obtain a scalar field for each time step.
We also track the evolution of split trees of 
resulted from the velocity magnitude.

The three data sets \dataset{Boussinesq2D}, \dataset{Cylinder3D}, and \dataset{Tangaroa3D}
can be found at the
\href{https://cgl.ethz.ch/research/visualization/data.php}{Computer Graphics Laboratory}.
The simplification thresholds for the data sets are:
\dataset{IonizationFront2D} at $5\%$,
\dataset{Storms2D} at $1\%$,
\dataset{Boussinesq2D} at $2\%$,
both \dataset{Cylinder3D} and \dataset{Tangaroa3D} at $8\%$.
We also provide results for with more time steps of \dataset{Cylinder2D}.

\subsection*{Results using IonizationFront2D}
The results of the experiments using \dataset{IonizationFront2D}
are shown from \Cref{fig-IonizationFront2DAllNodes}
to \Cref{fig-IonizationFront2DSimilarities}.

\begin{figure}
\centering
\includegraphics[width=0.8\linewidth]{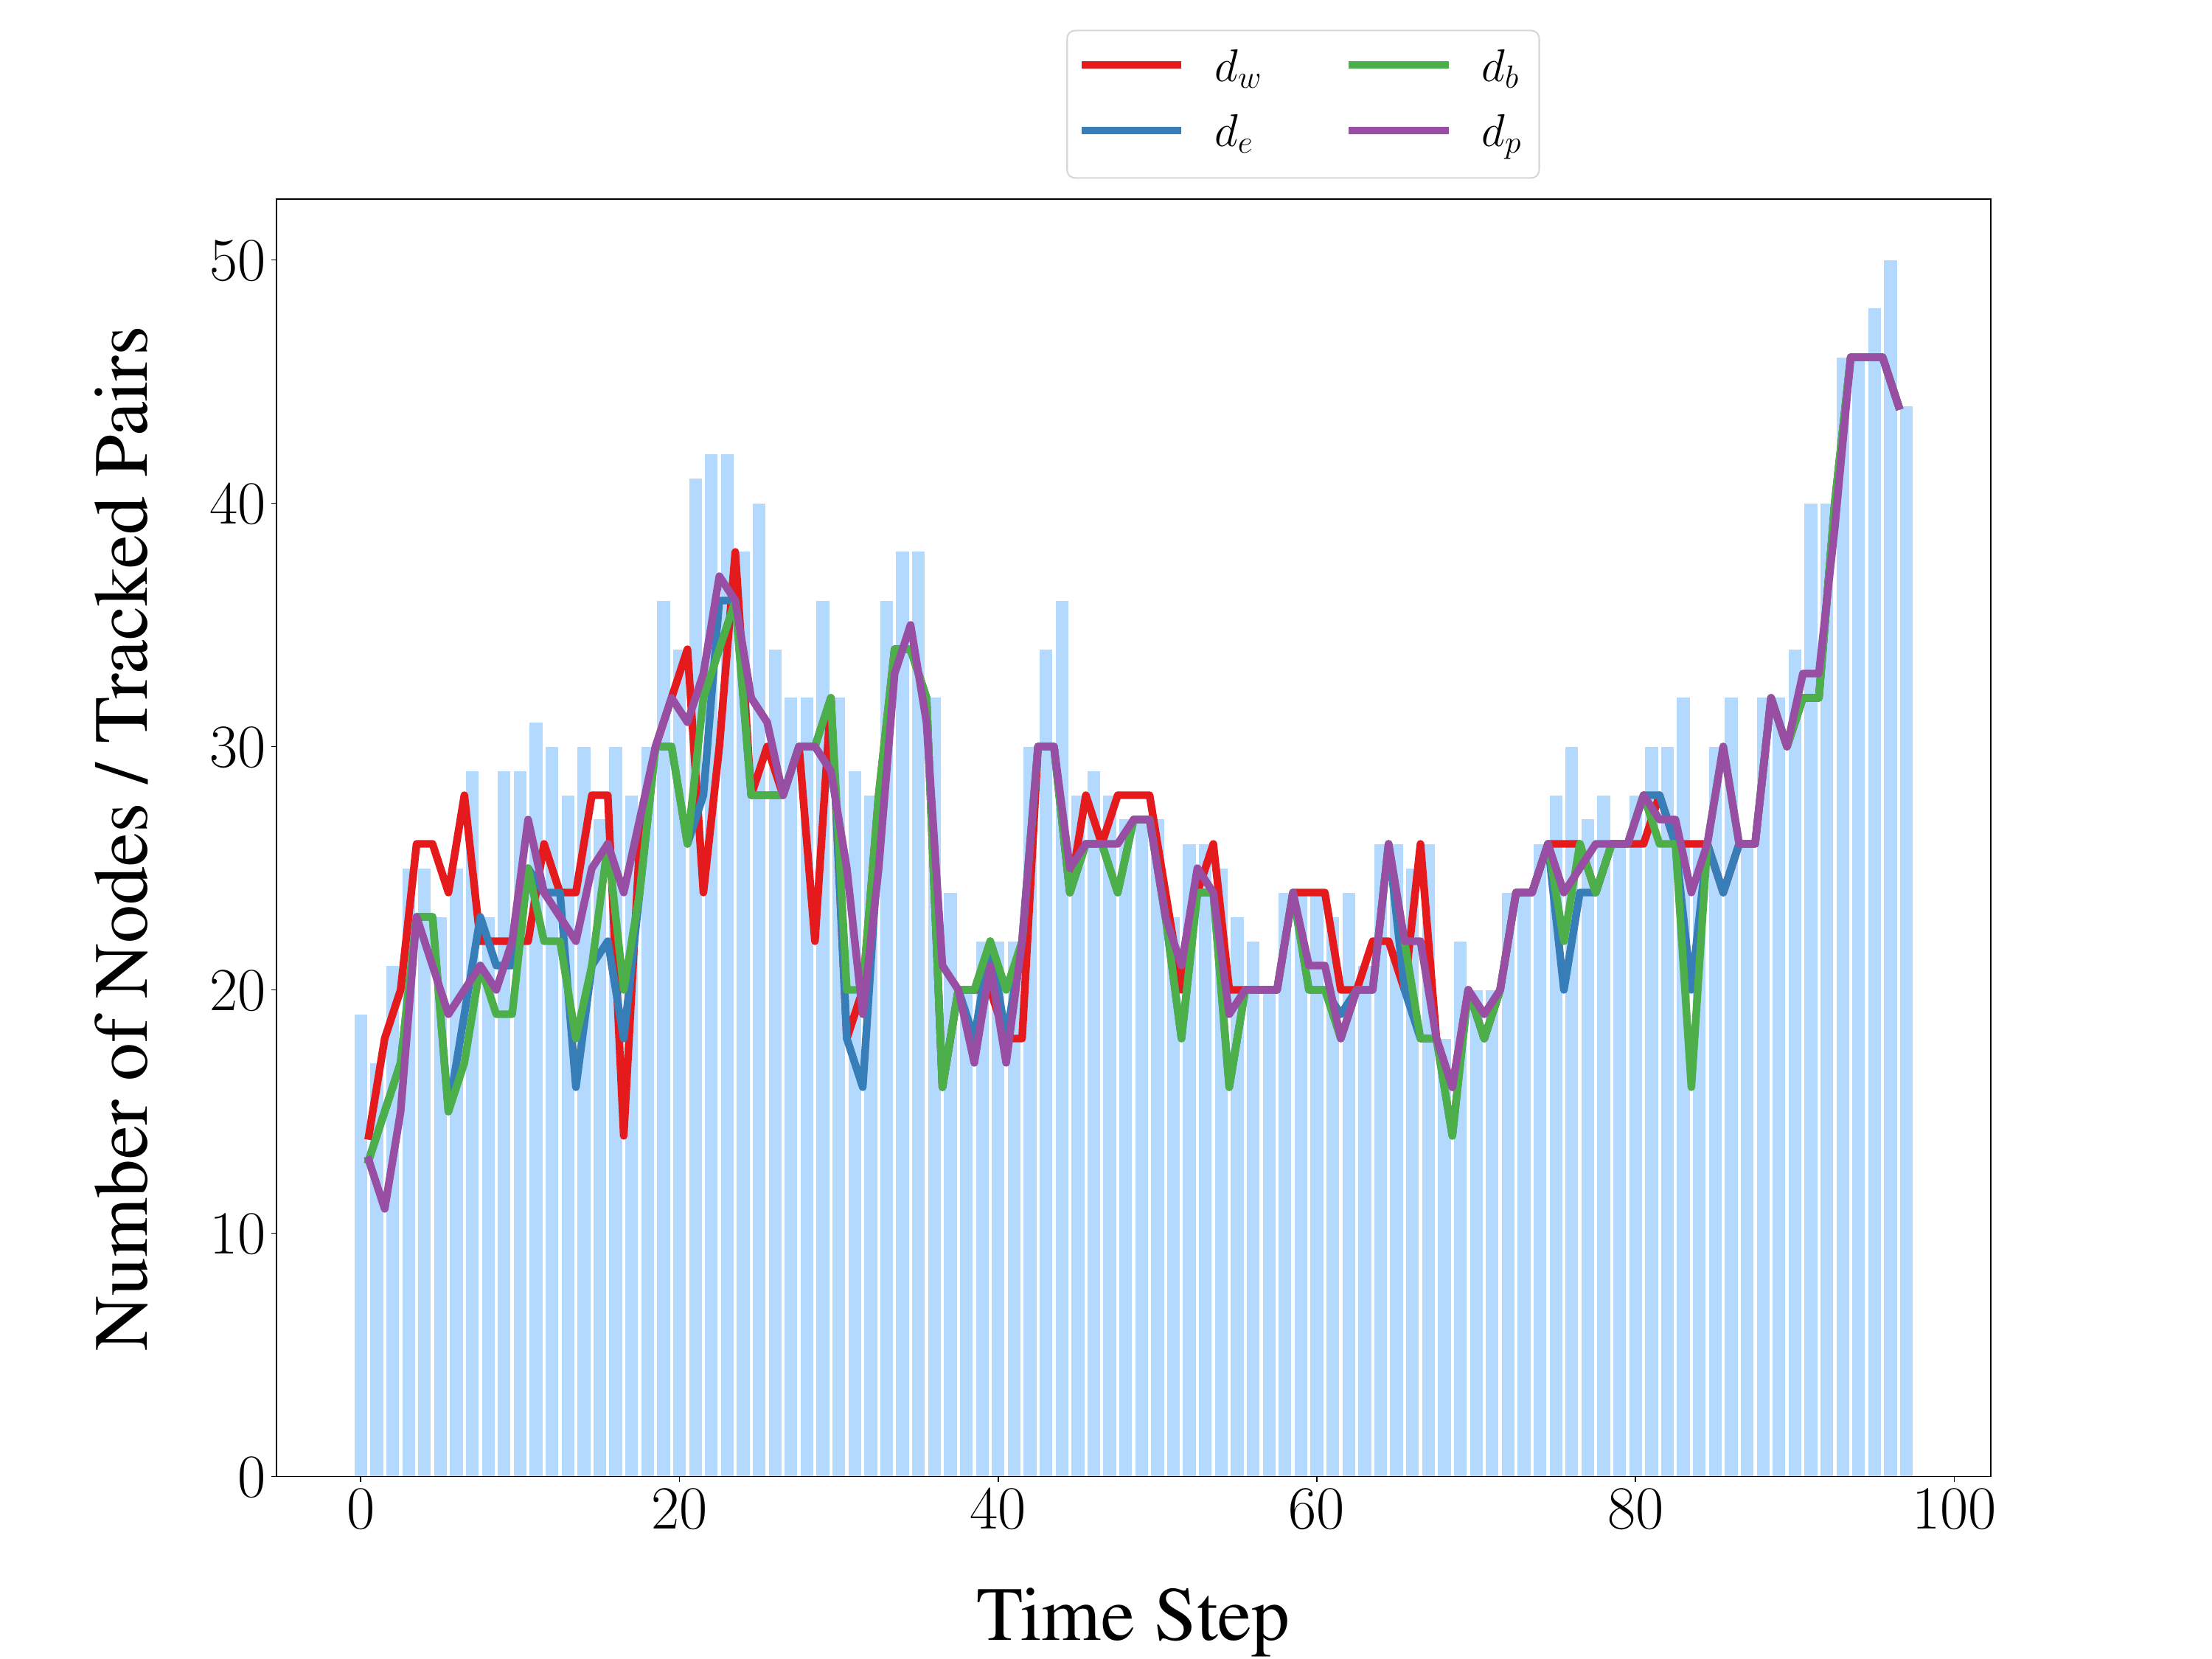}
\caption{
    Number of tracked nodes (colored and labeled) 
    relative to the total nodes of merge trees (light blue bars)
    for \dataset{IonizationFront2D}.
}
\label{fig-IonizationFront2DAllNodes}
\end{figure}

\begin{figure}
\centering
\includegraphics[width=0.8\linewidth]{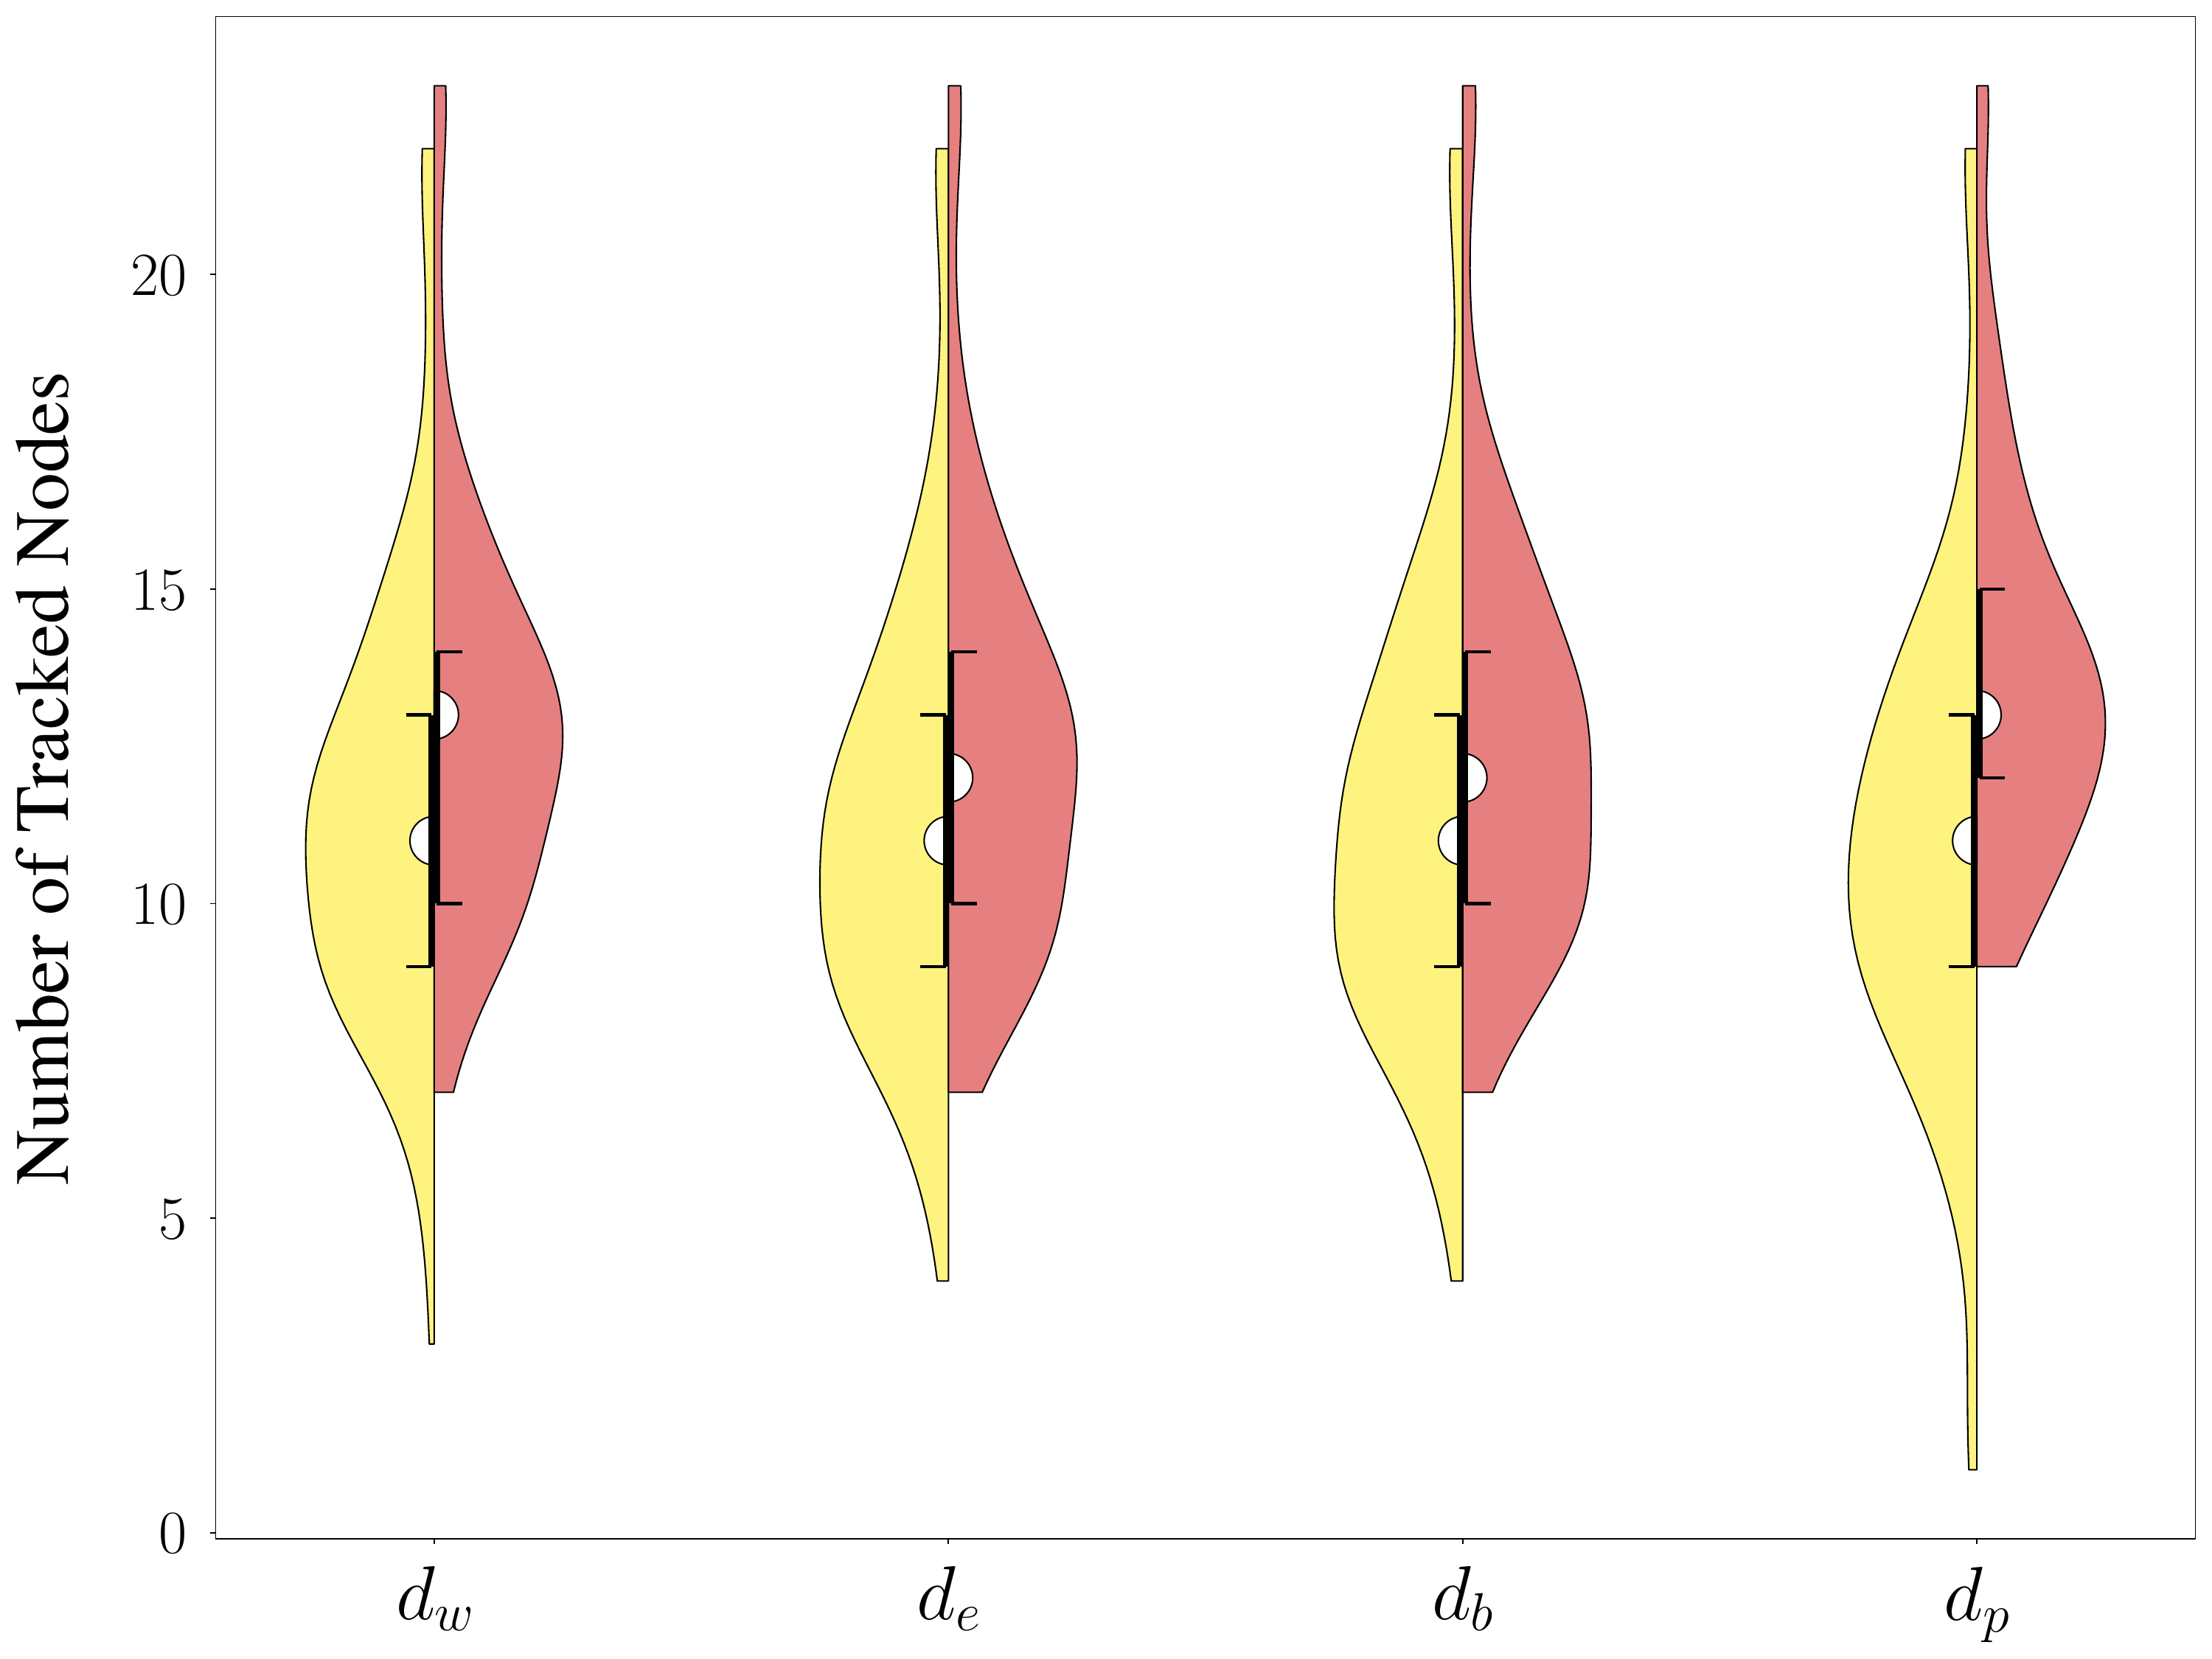}
\caption{
    Distributions of tracked nodes 
    over the chosen time steps of \dataset{IonizationFront2D},  
    divided by types:
    saddle (yellow) and maxima (red).
}
\label{fig-IonizationFront2DViolin}
\end{figure}

% Length histogram
\begin{figure}%
\begin{subfigure}[t]{\ltwopicwidth}%
\includegraphics[width=\ltwopicwidth]{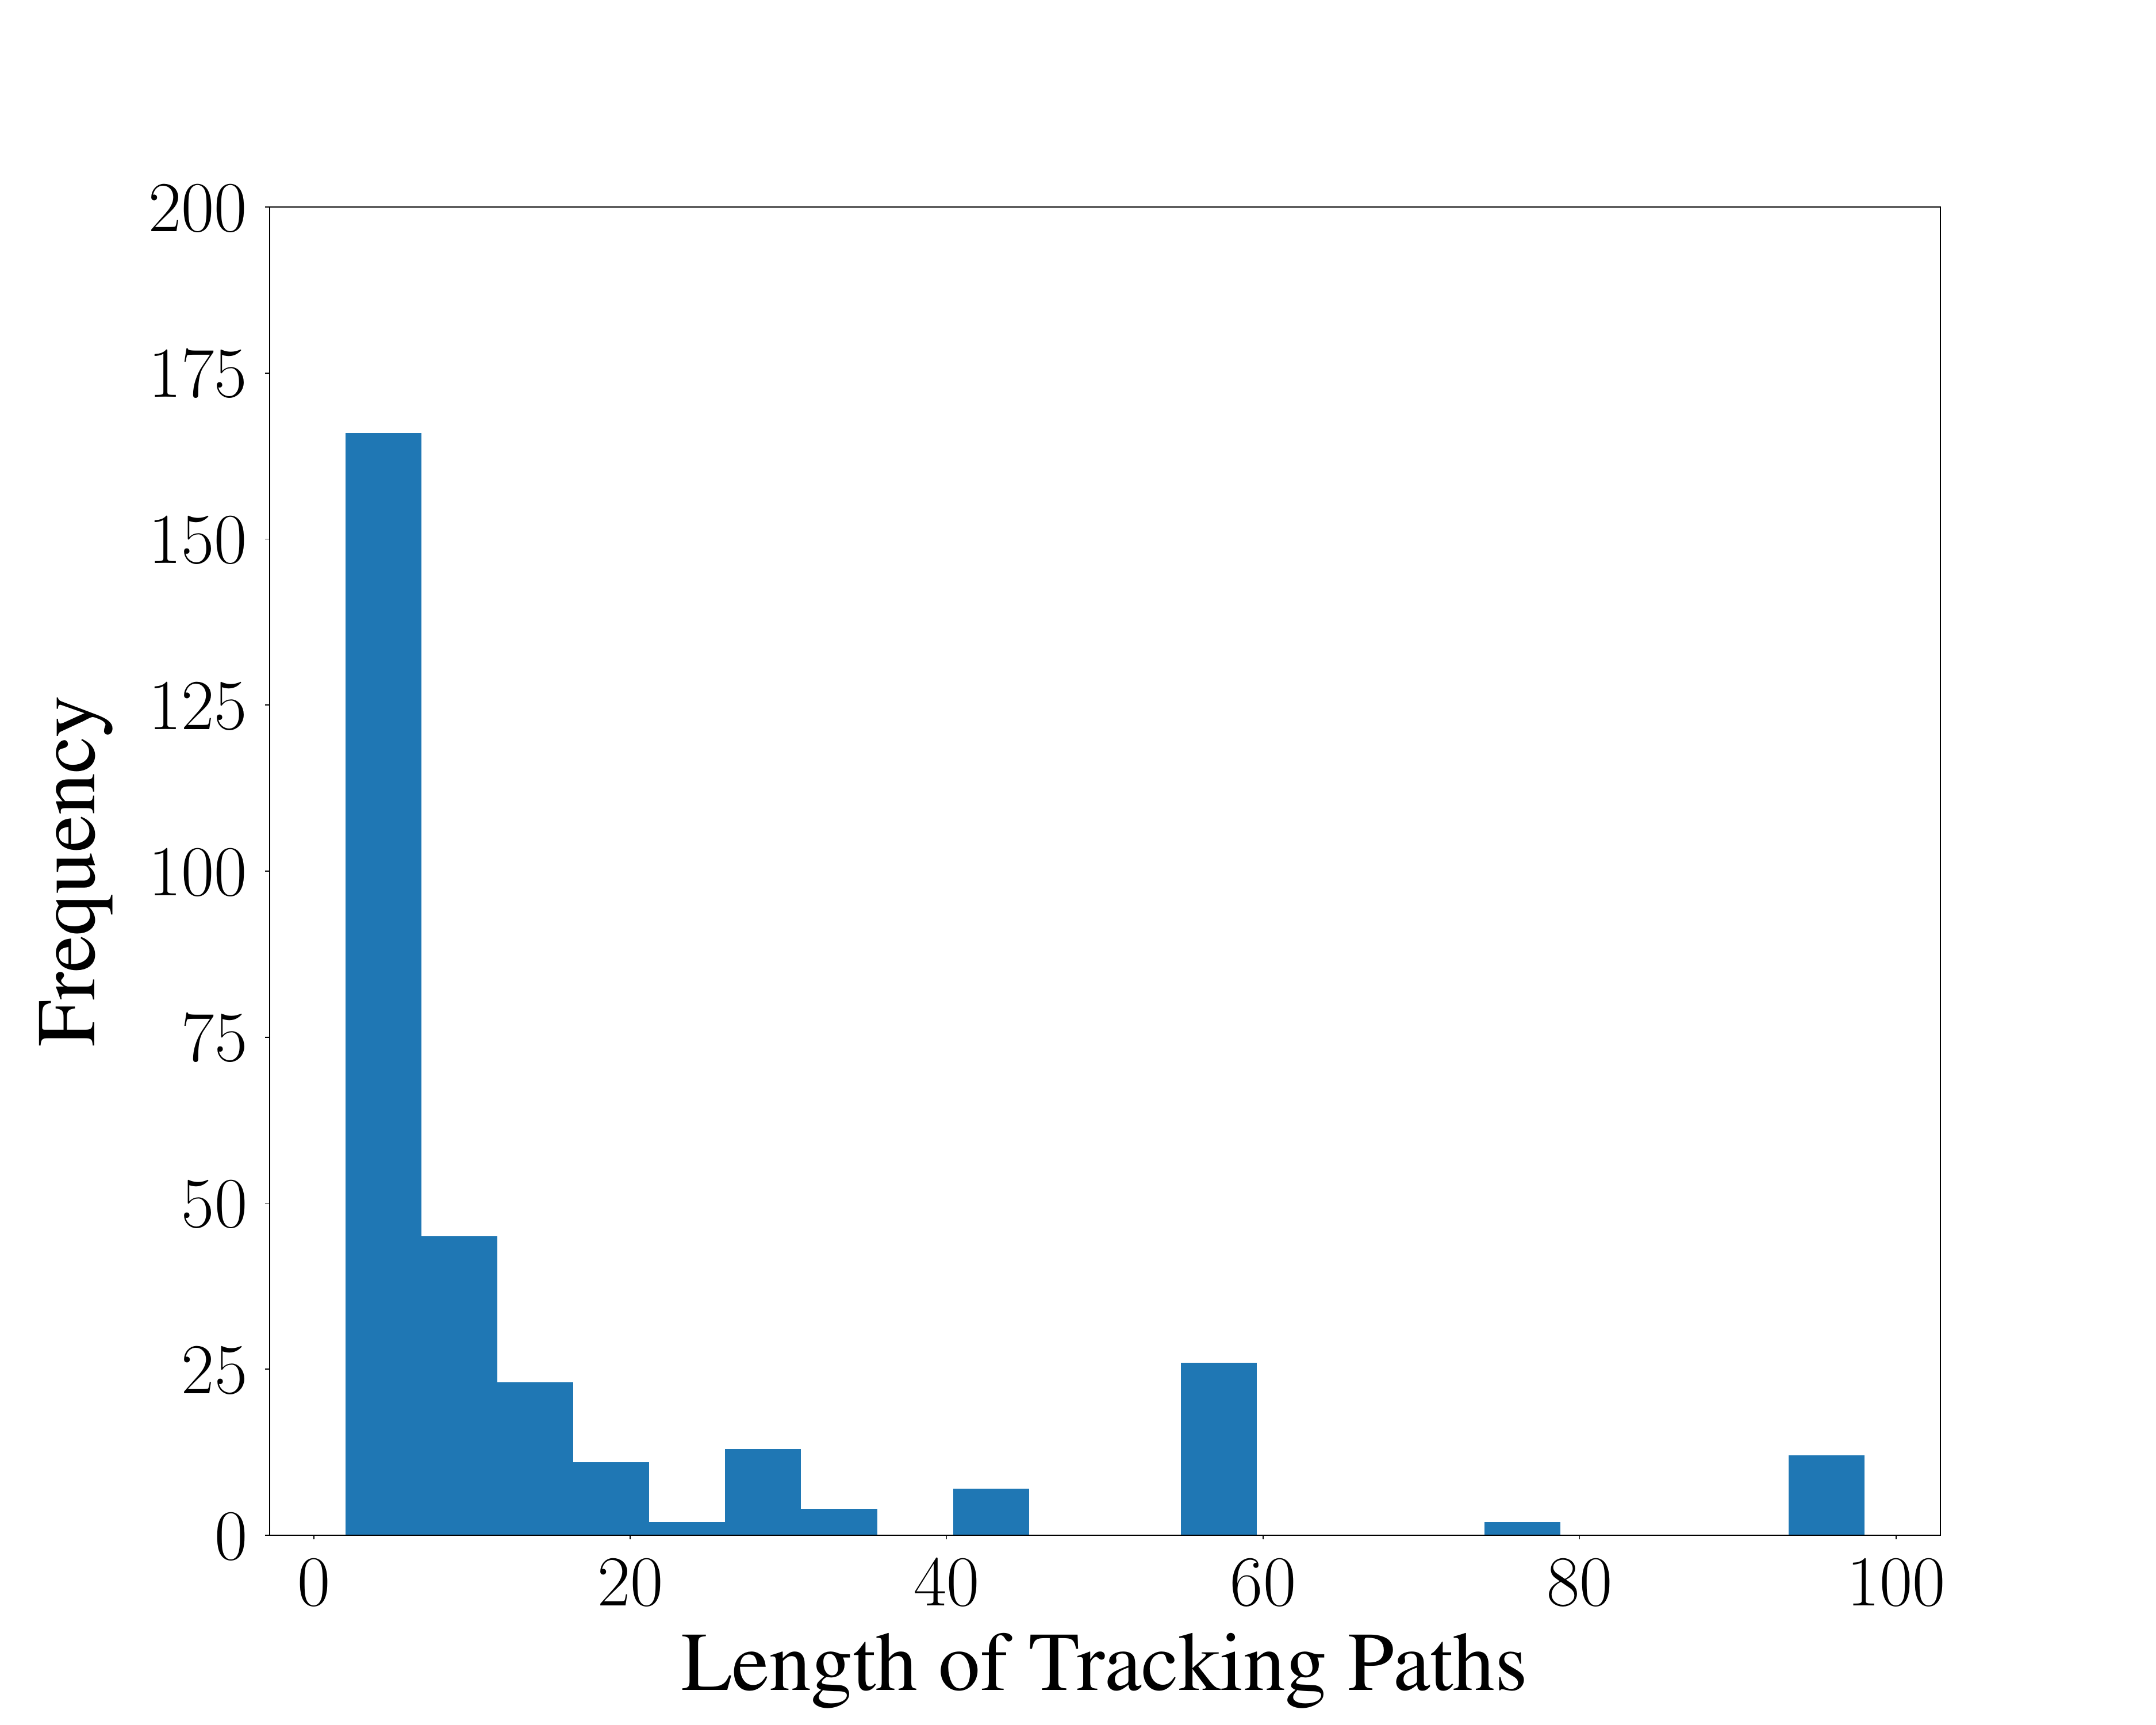}
\caption{$d_w$.}%
\label{fig-LengthHistogramIonizationFront2DW}%
\end{subfigure}
\hfill%
\begin{subfigure}[t]{\ltwopicwidth}%
\includegraphics[width=\ltwopicwidth]{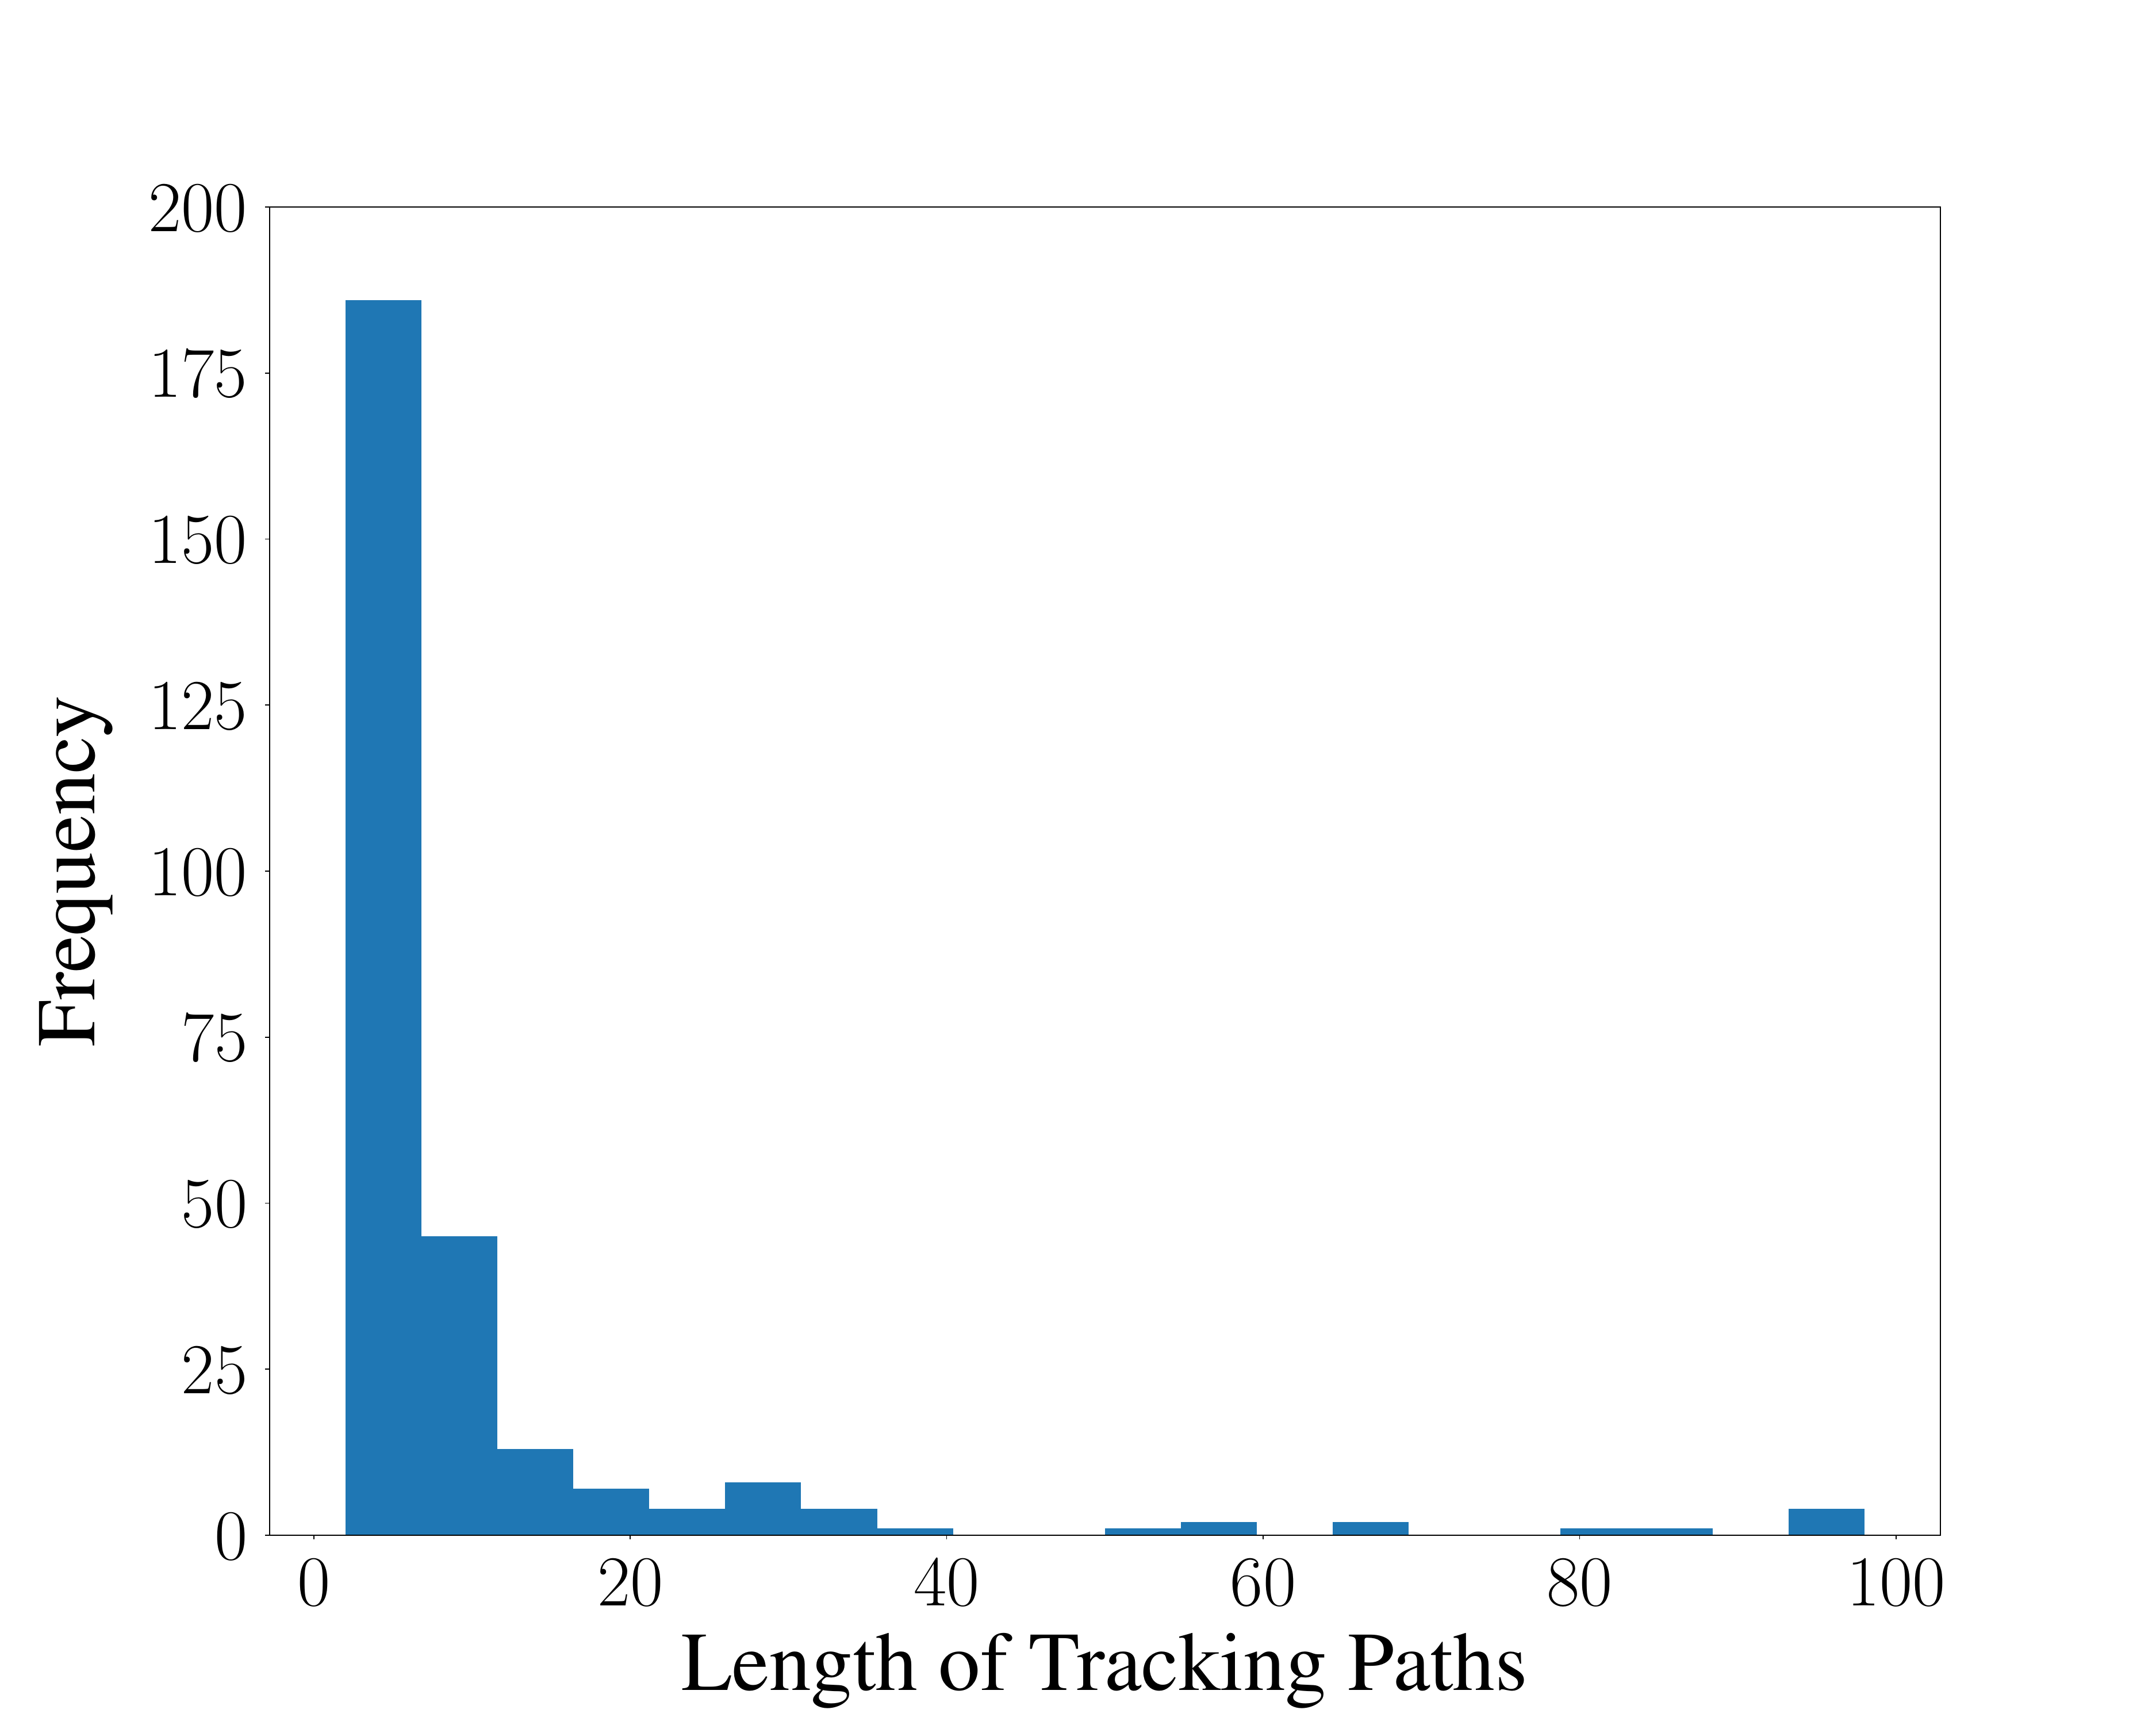}%
\caption{$d_e$.}%
\label{fig-LengthHistogramIonizationFront2DE}%
\end{subfigure}%
\\%
\begin{subfigure}[t]{\ltwopicwidth}%
\includegraphics[width=\ltwopicwidth]{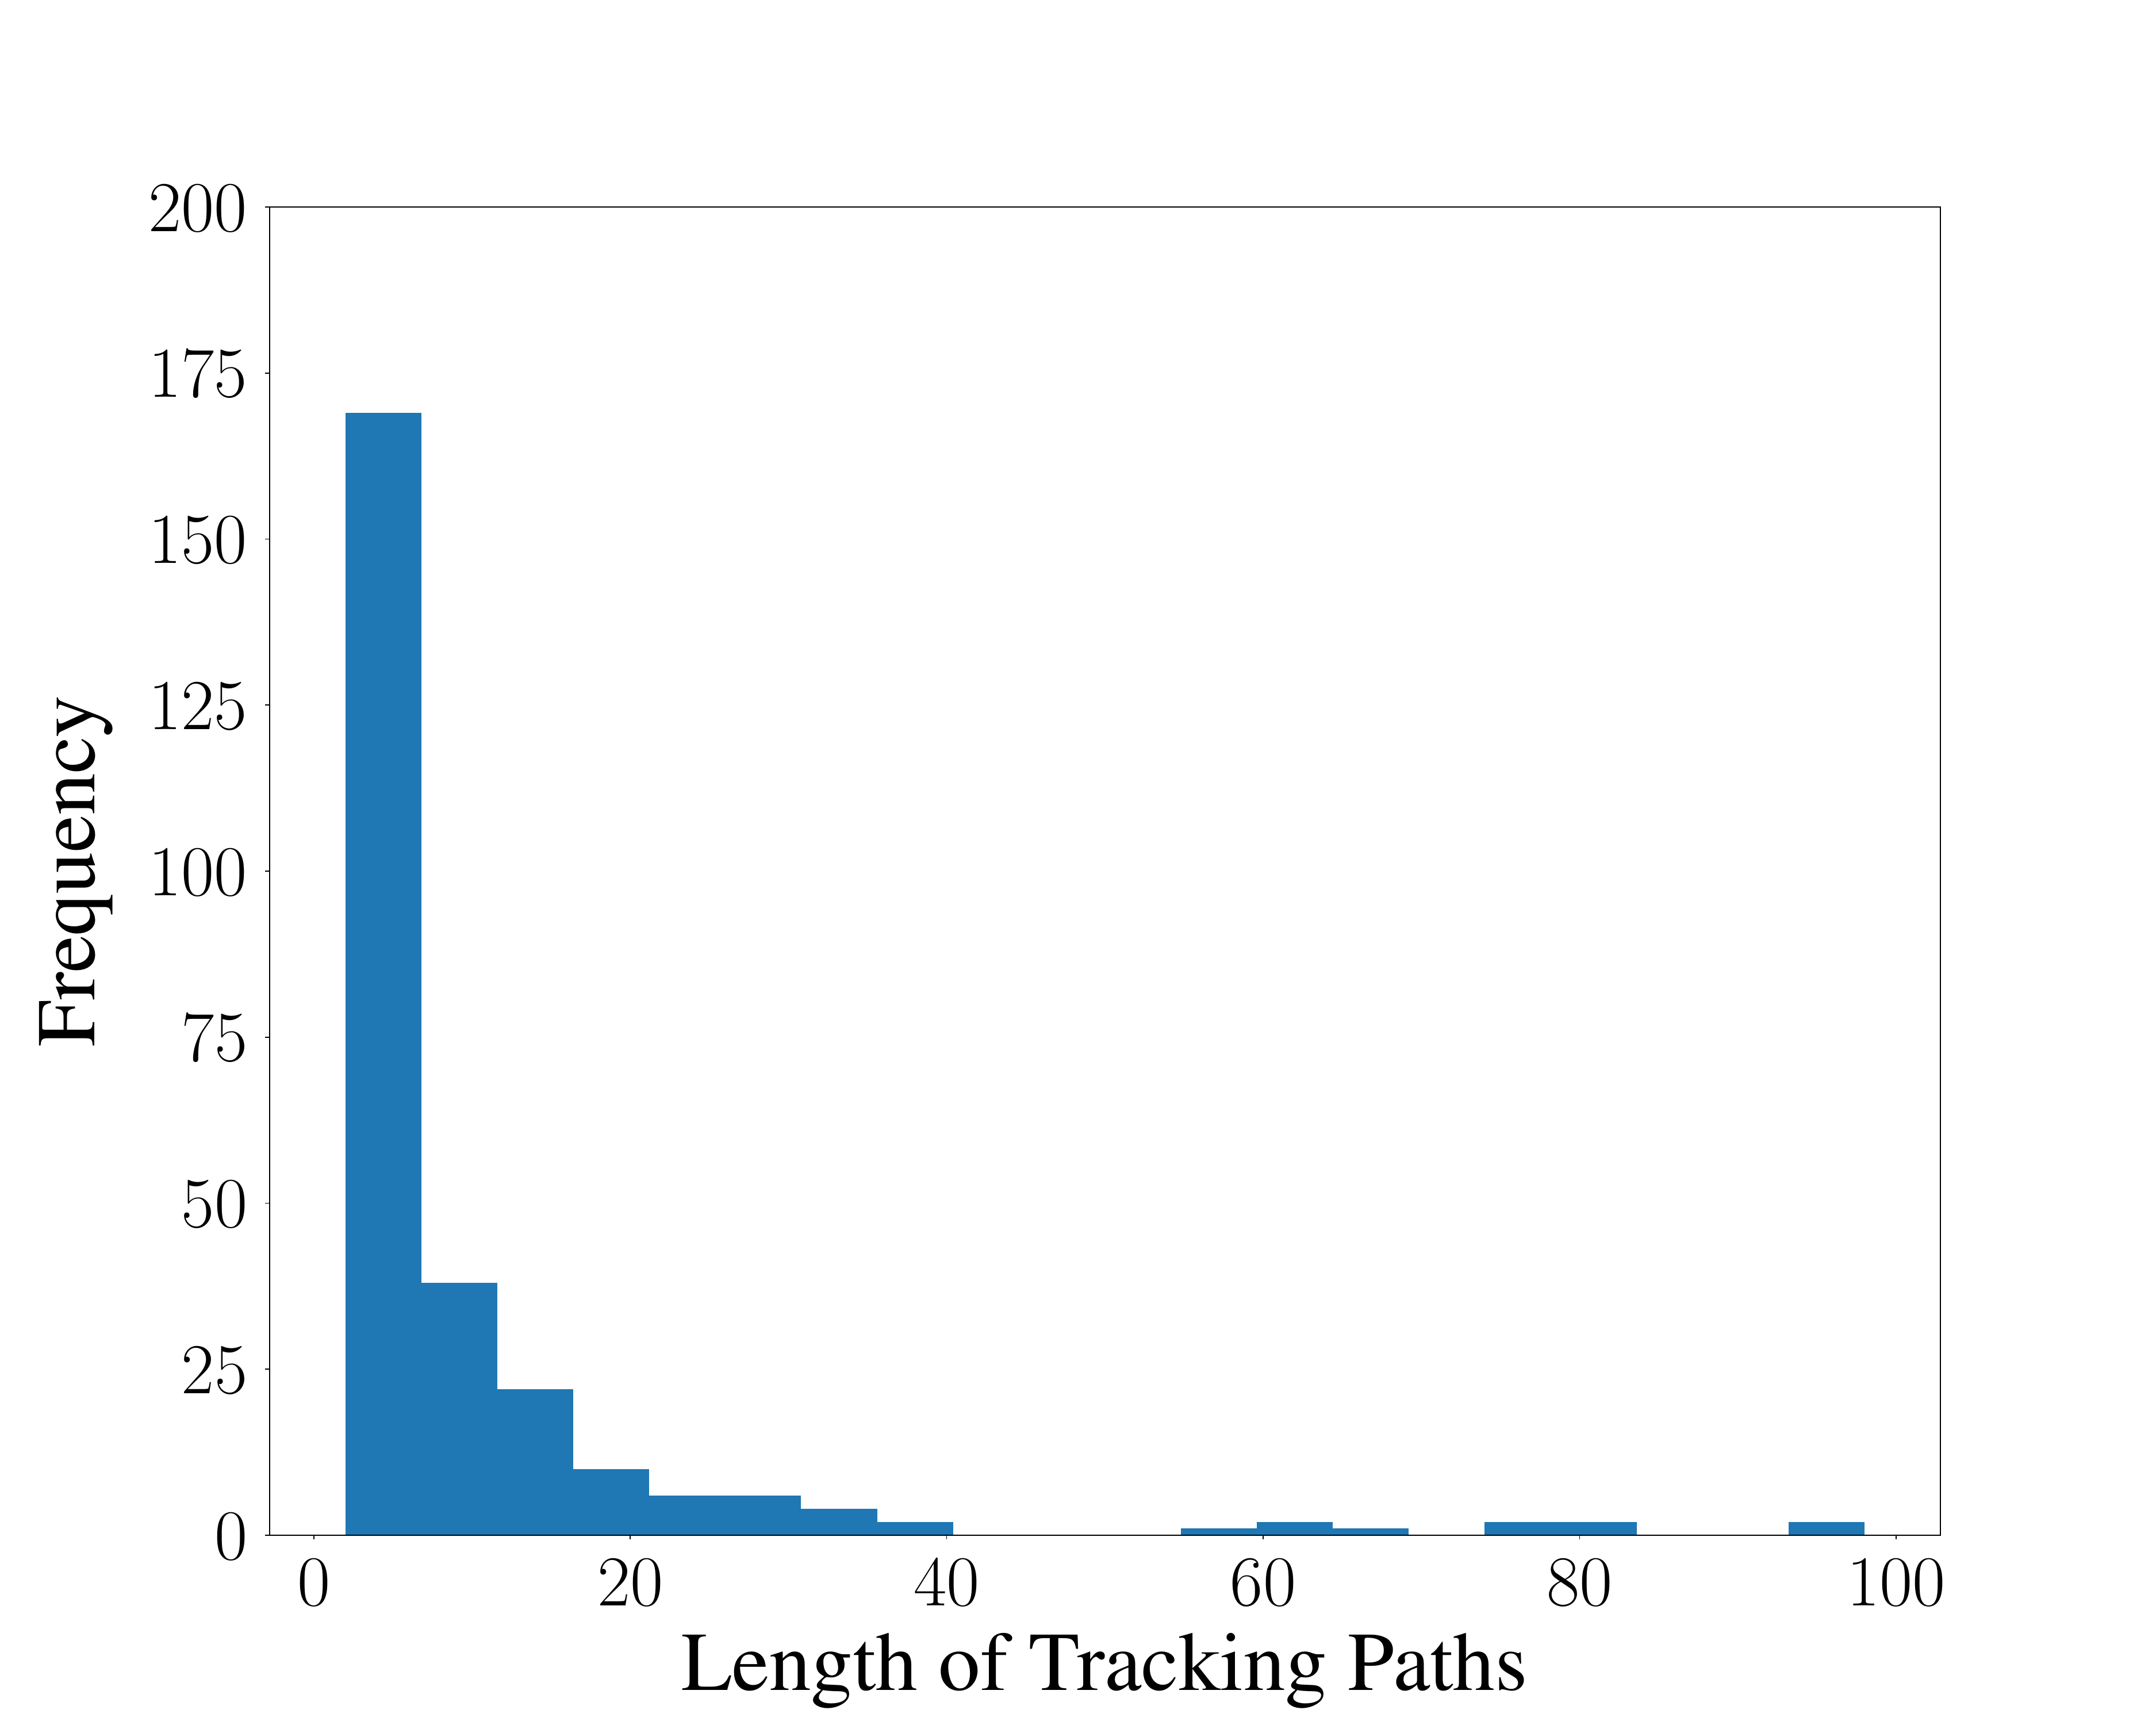}%
\caption{$d_b$.}%
\label{fig-LengthHistogramIonizationFront2DB}%
\end{subfigure}%
\hfill%
\begin{subfigure}[t]{\ltwopicwidth}%
\includegraphics[width=\ltwopicwidth]{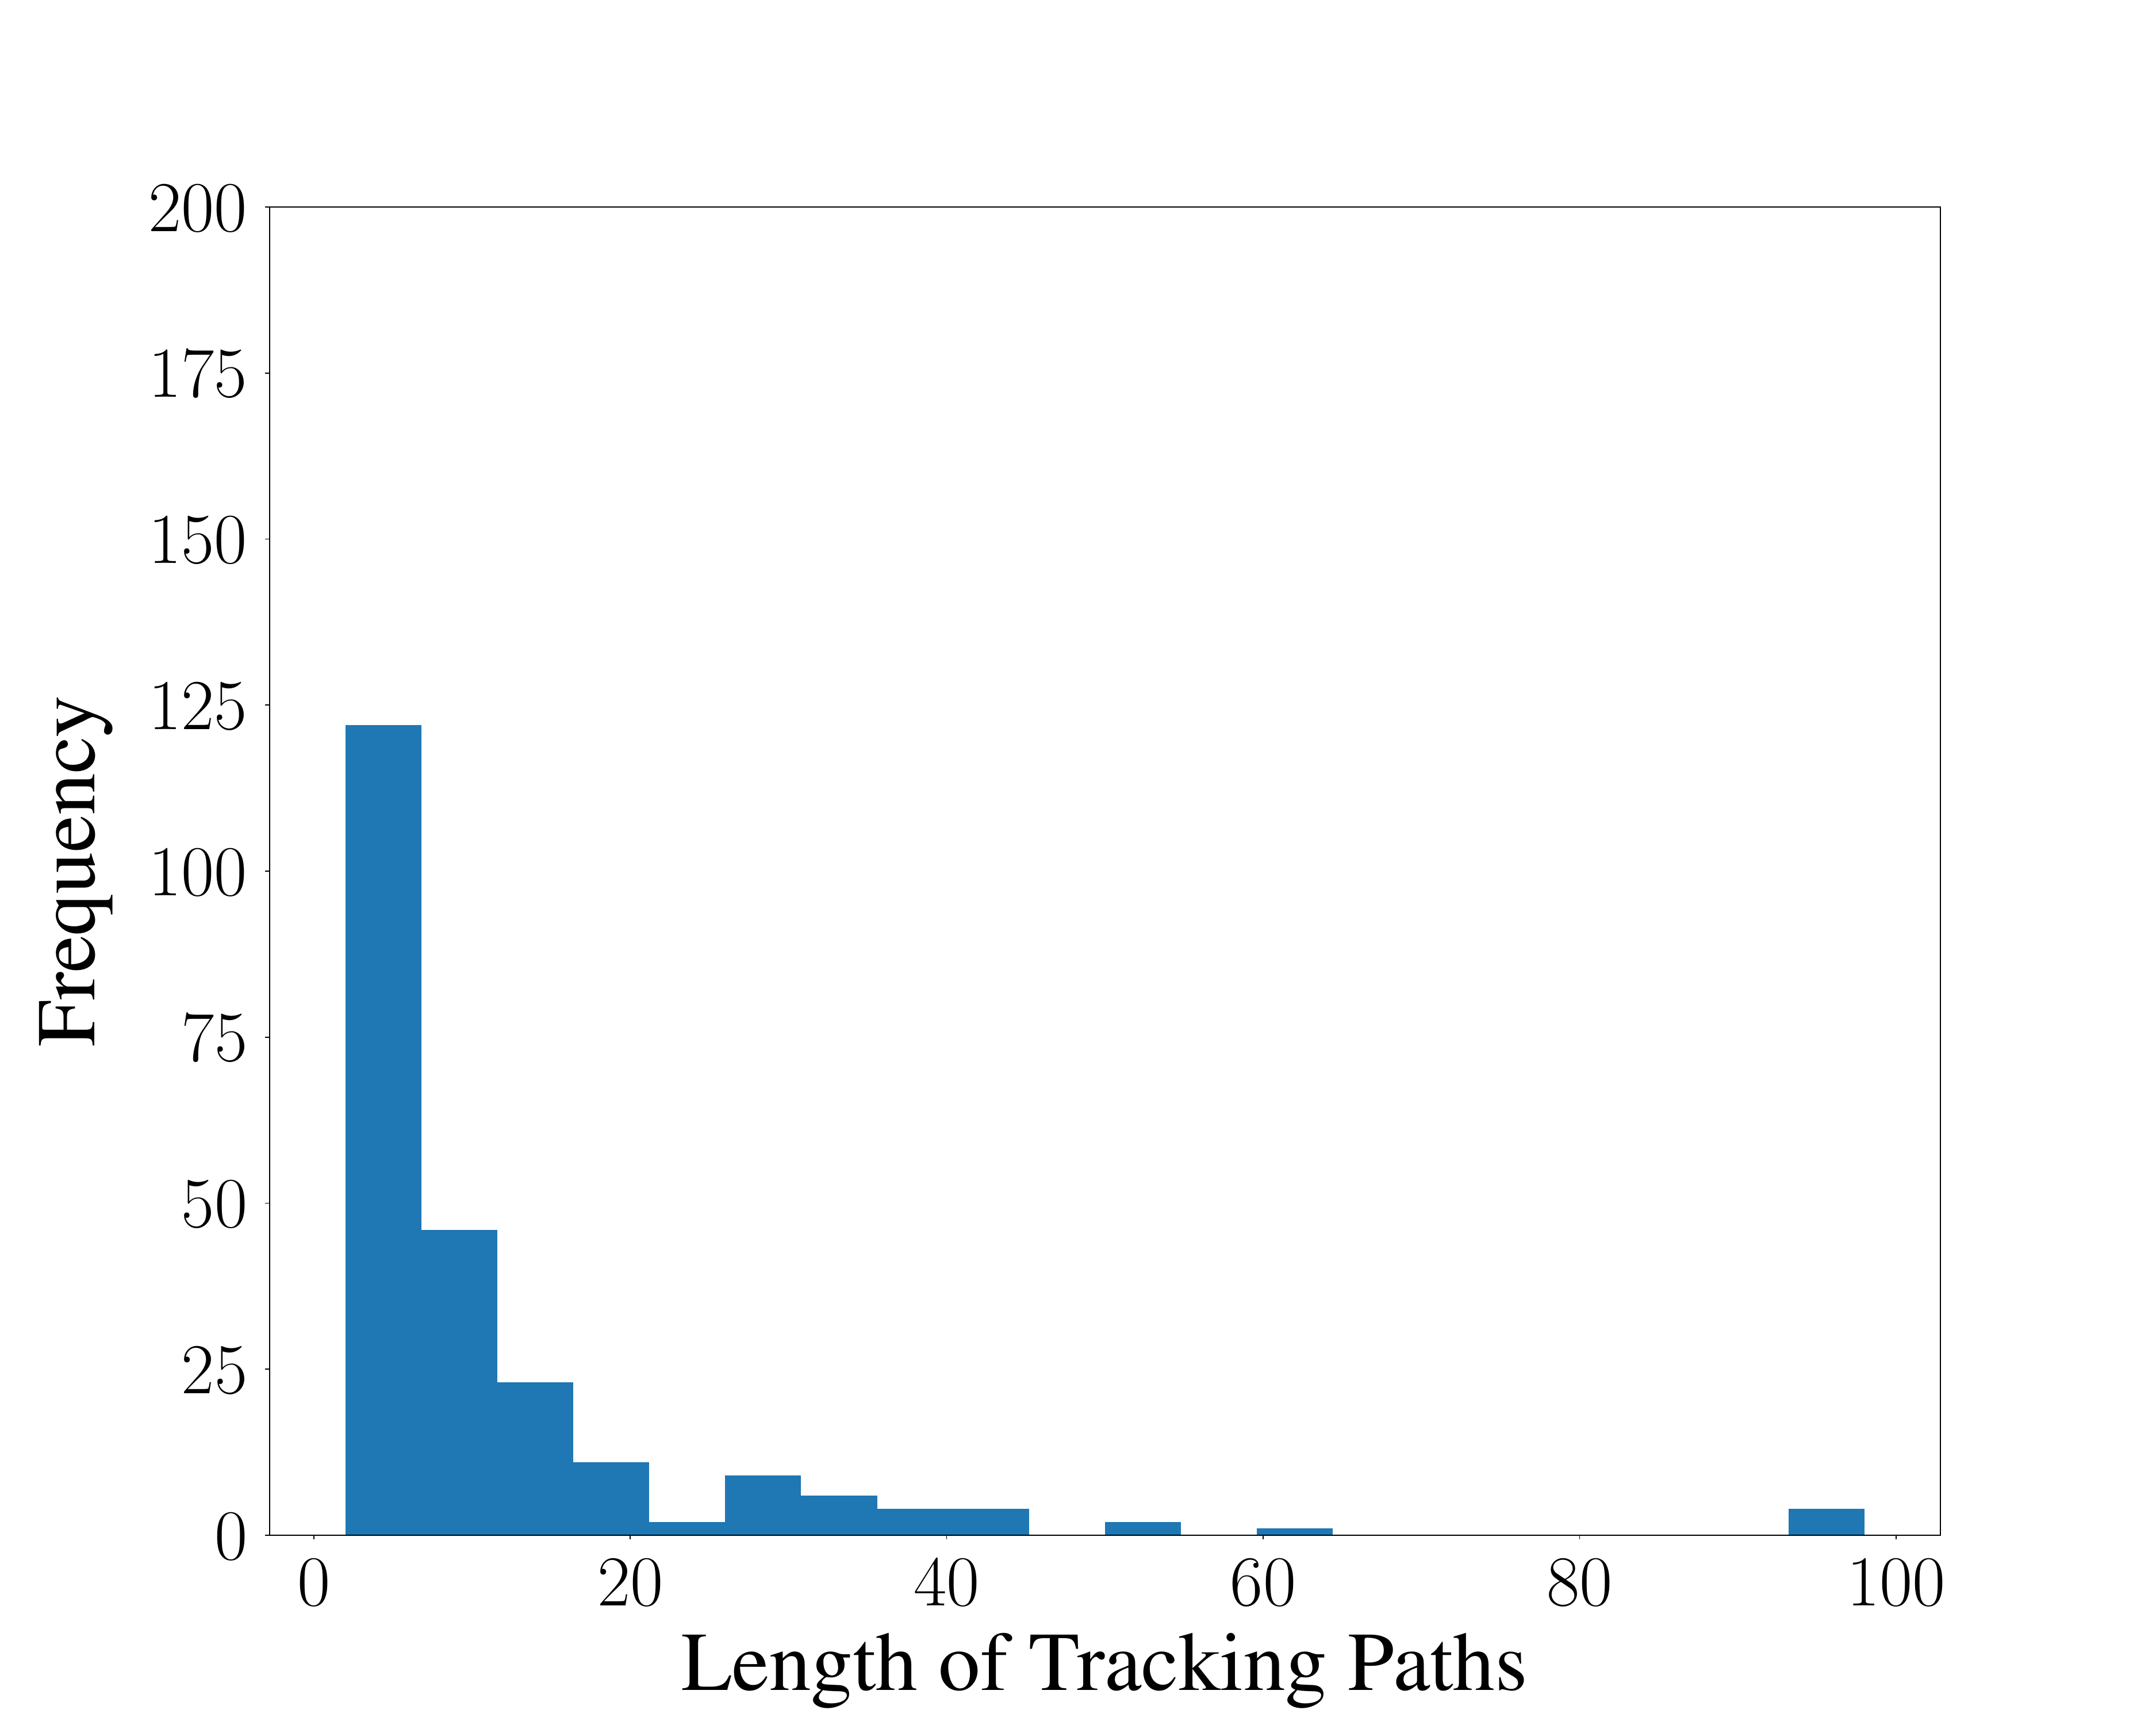}%
\caption{$d_p$.}%
\label{fig-LengthHistogramIonizationFront2DP}%
\end{subfigure}%
\caption{Histograms of the length of the tracking paths of the first $100$ time steps 
    of \dataset{IonizationFront2D}.}%
\label{fig-LengthHisgoramIonizationFront2D}%
\end{figure}

\begin{figure}
\centering
\includegraphics[width=0.8\linewidth]{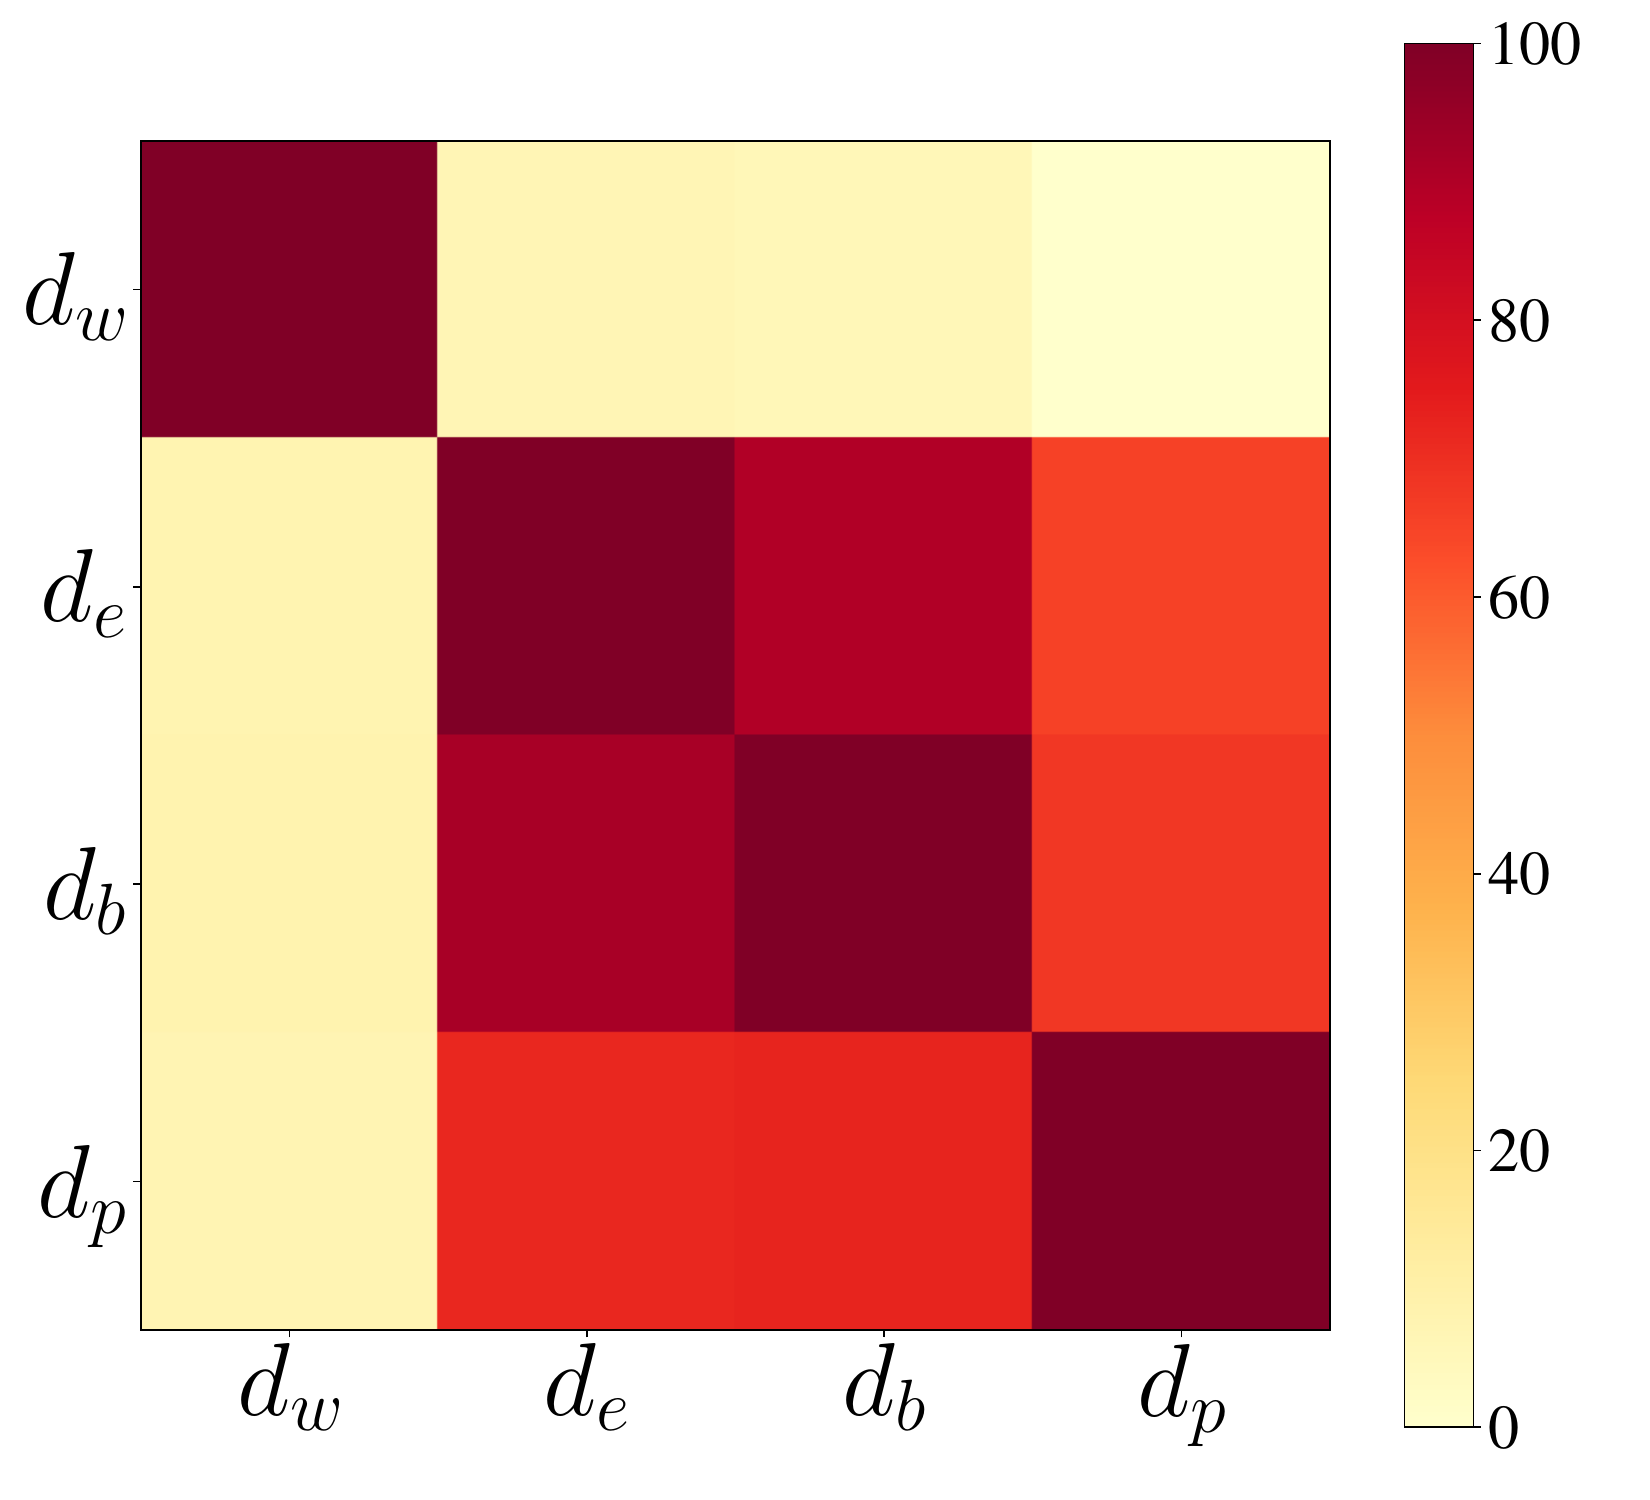}
\caption{
    Pairwise differences between the methods on the columns
    in relation to the methods on the rows
    for \dataset{IonizationFront2D}.
}
\label{fig-IonizationFront2DSimilarities}
\end{figure}

\subsection*{Results using Storms2D}
The results of the experiments using \dataset{Storms2D}
are shown from \Cref{fig-Storms2DAllNodes}
to \Cref{fig-Storms2DSimilarities}.

\begin{figure}
\centering
\includegraphics[width=0.8\linewidth]{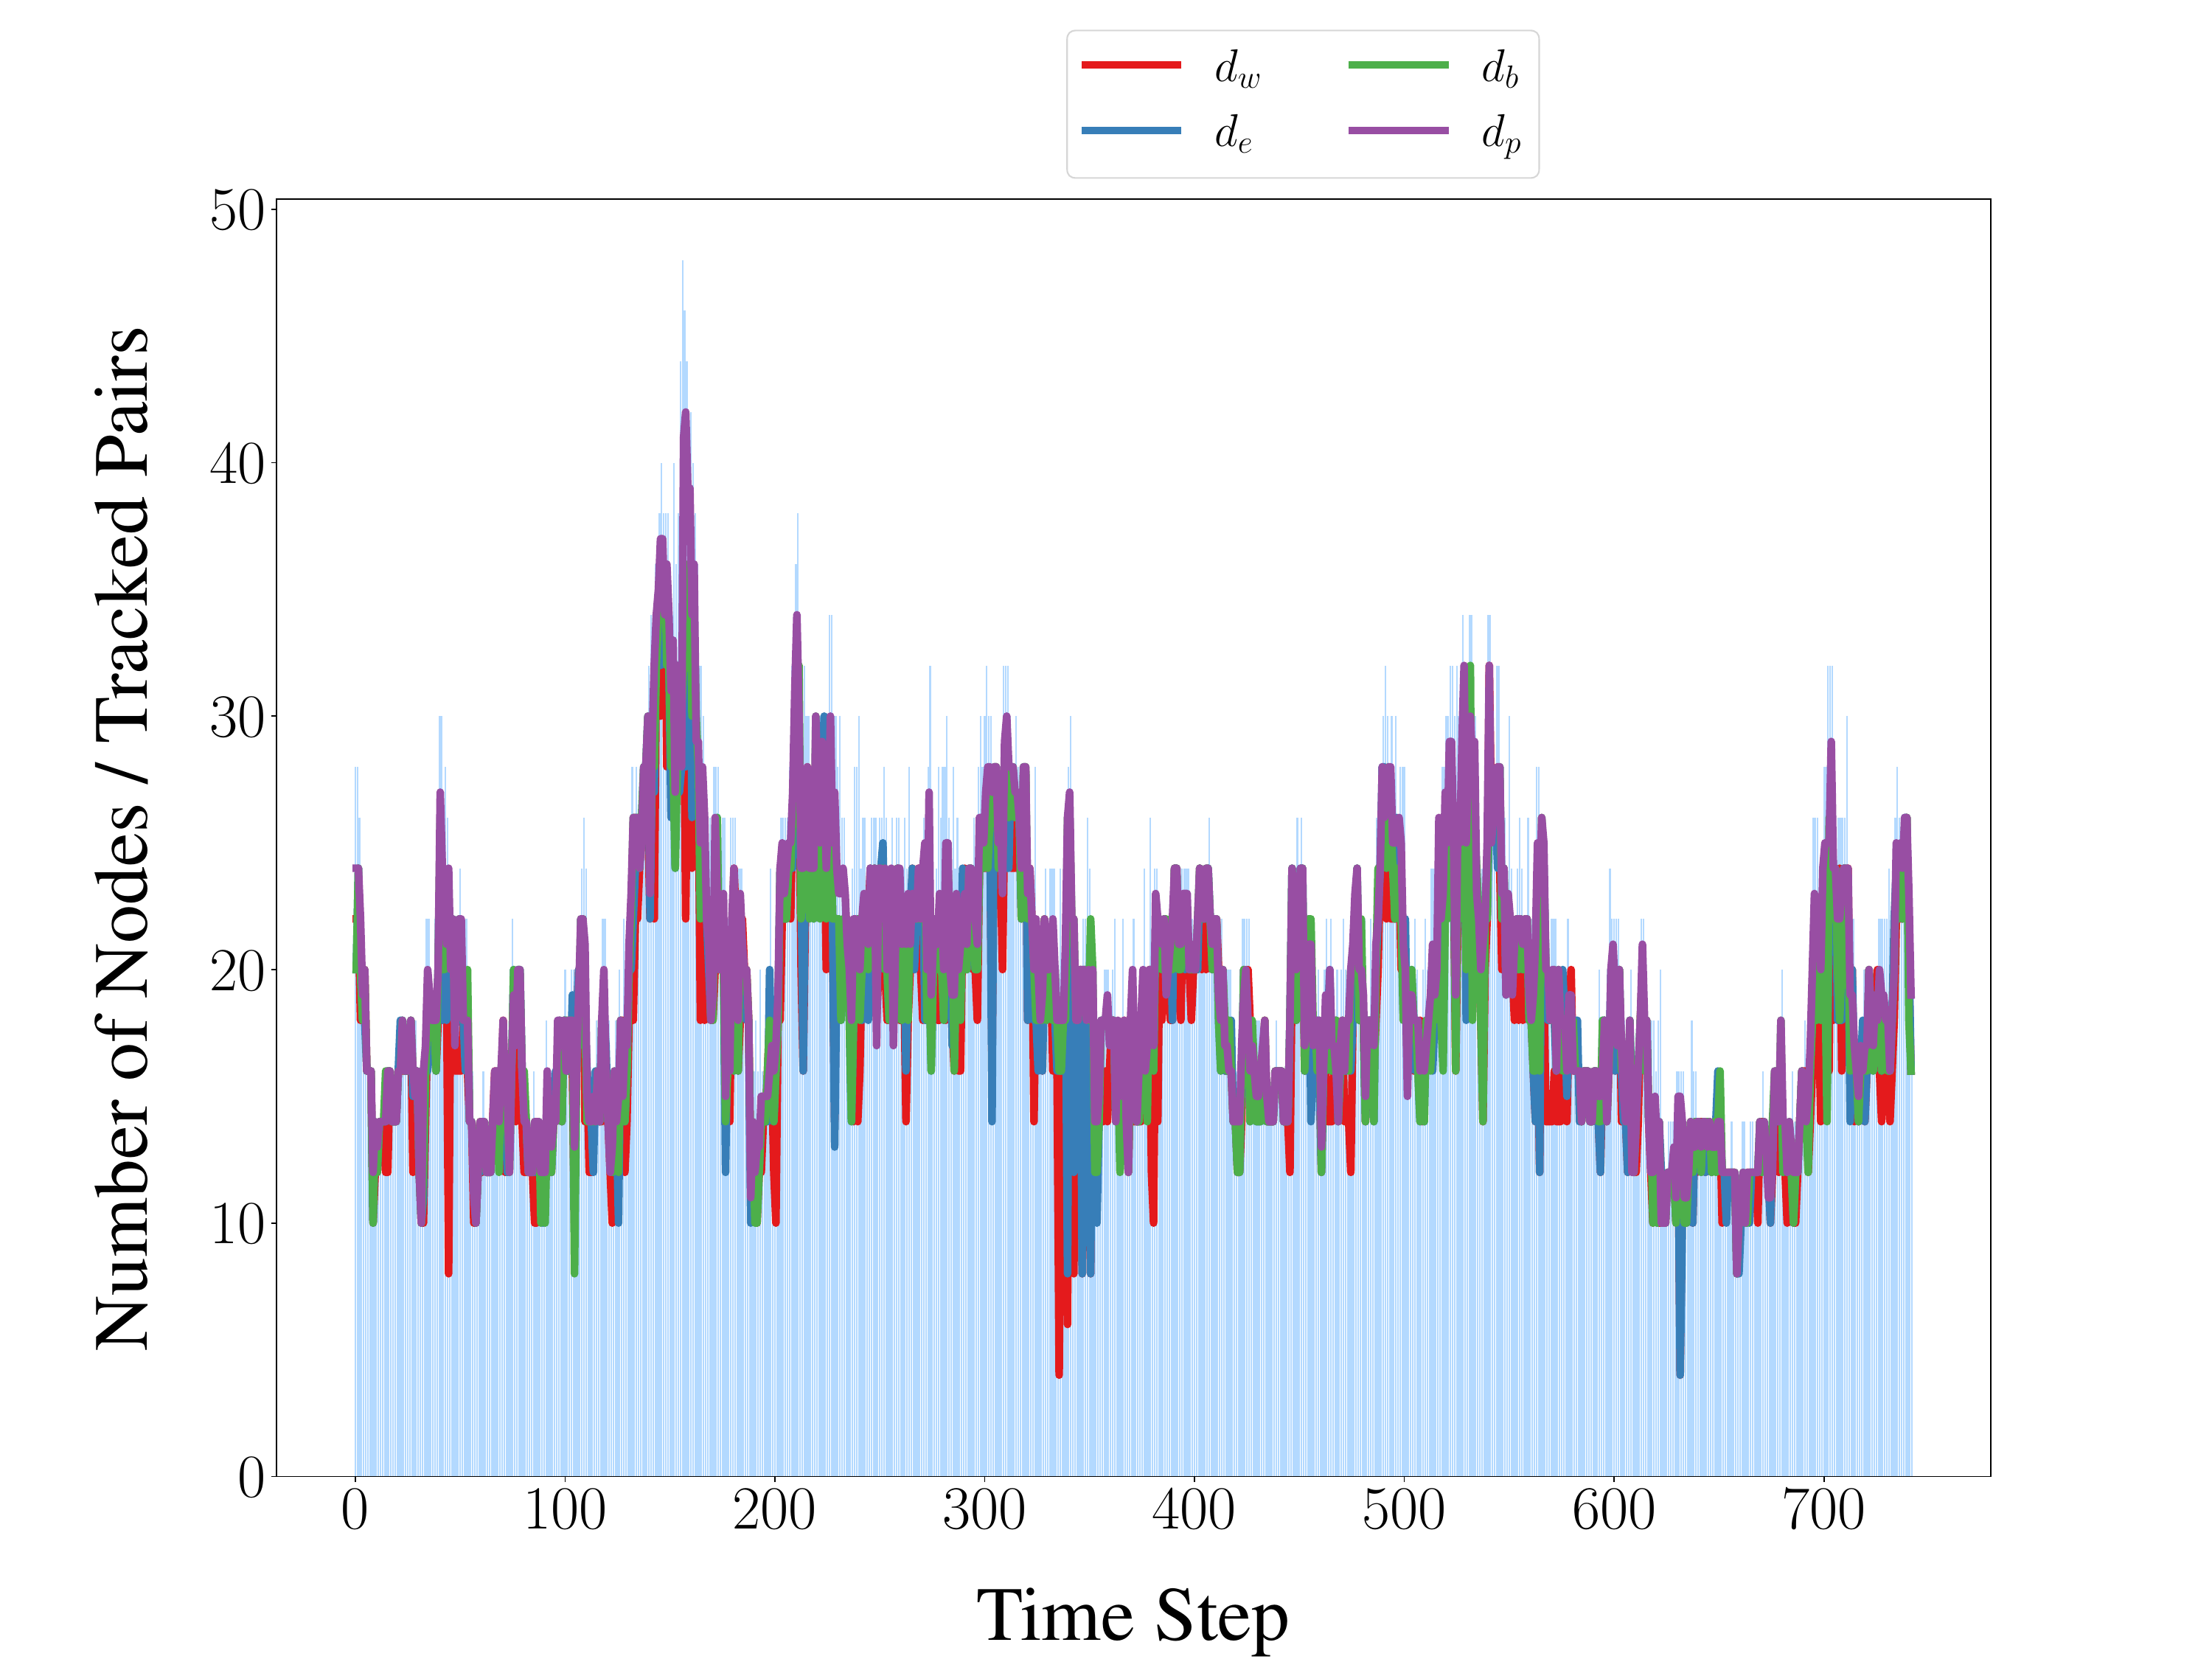}
\caption{
    Number of tracked nodes (colored and labeled) 
    relative to the total nodes of merge trees (light blue bars)
    for \dataset{Storms2D}.
}
\label{fig-Storms2DAllNodes}
\end{figure}

\begin{figure}
\centering
\includegraphics[width=0.8\linewidth]{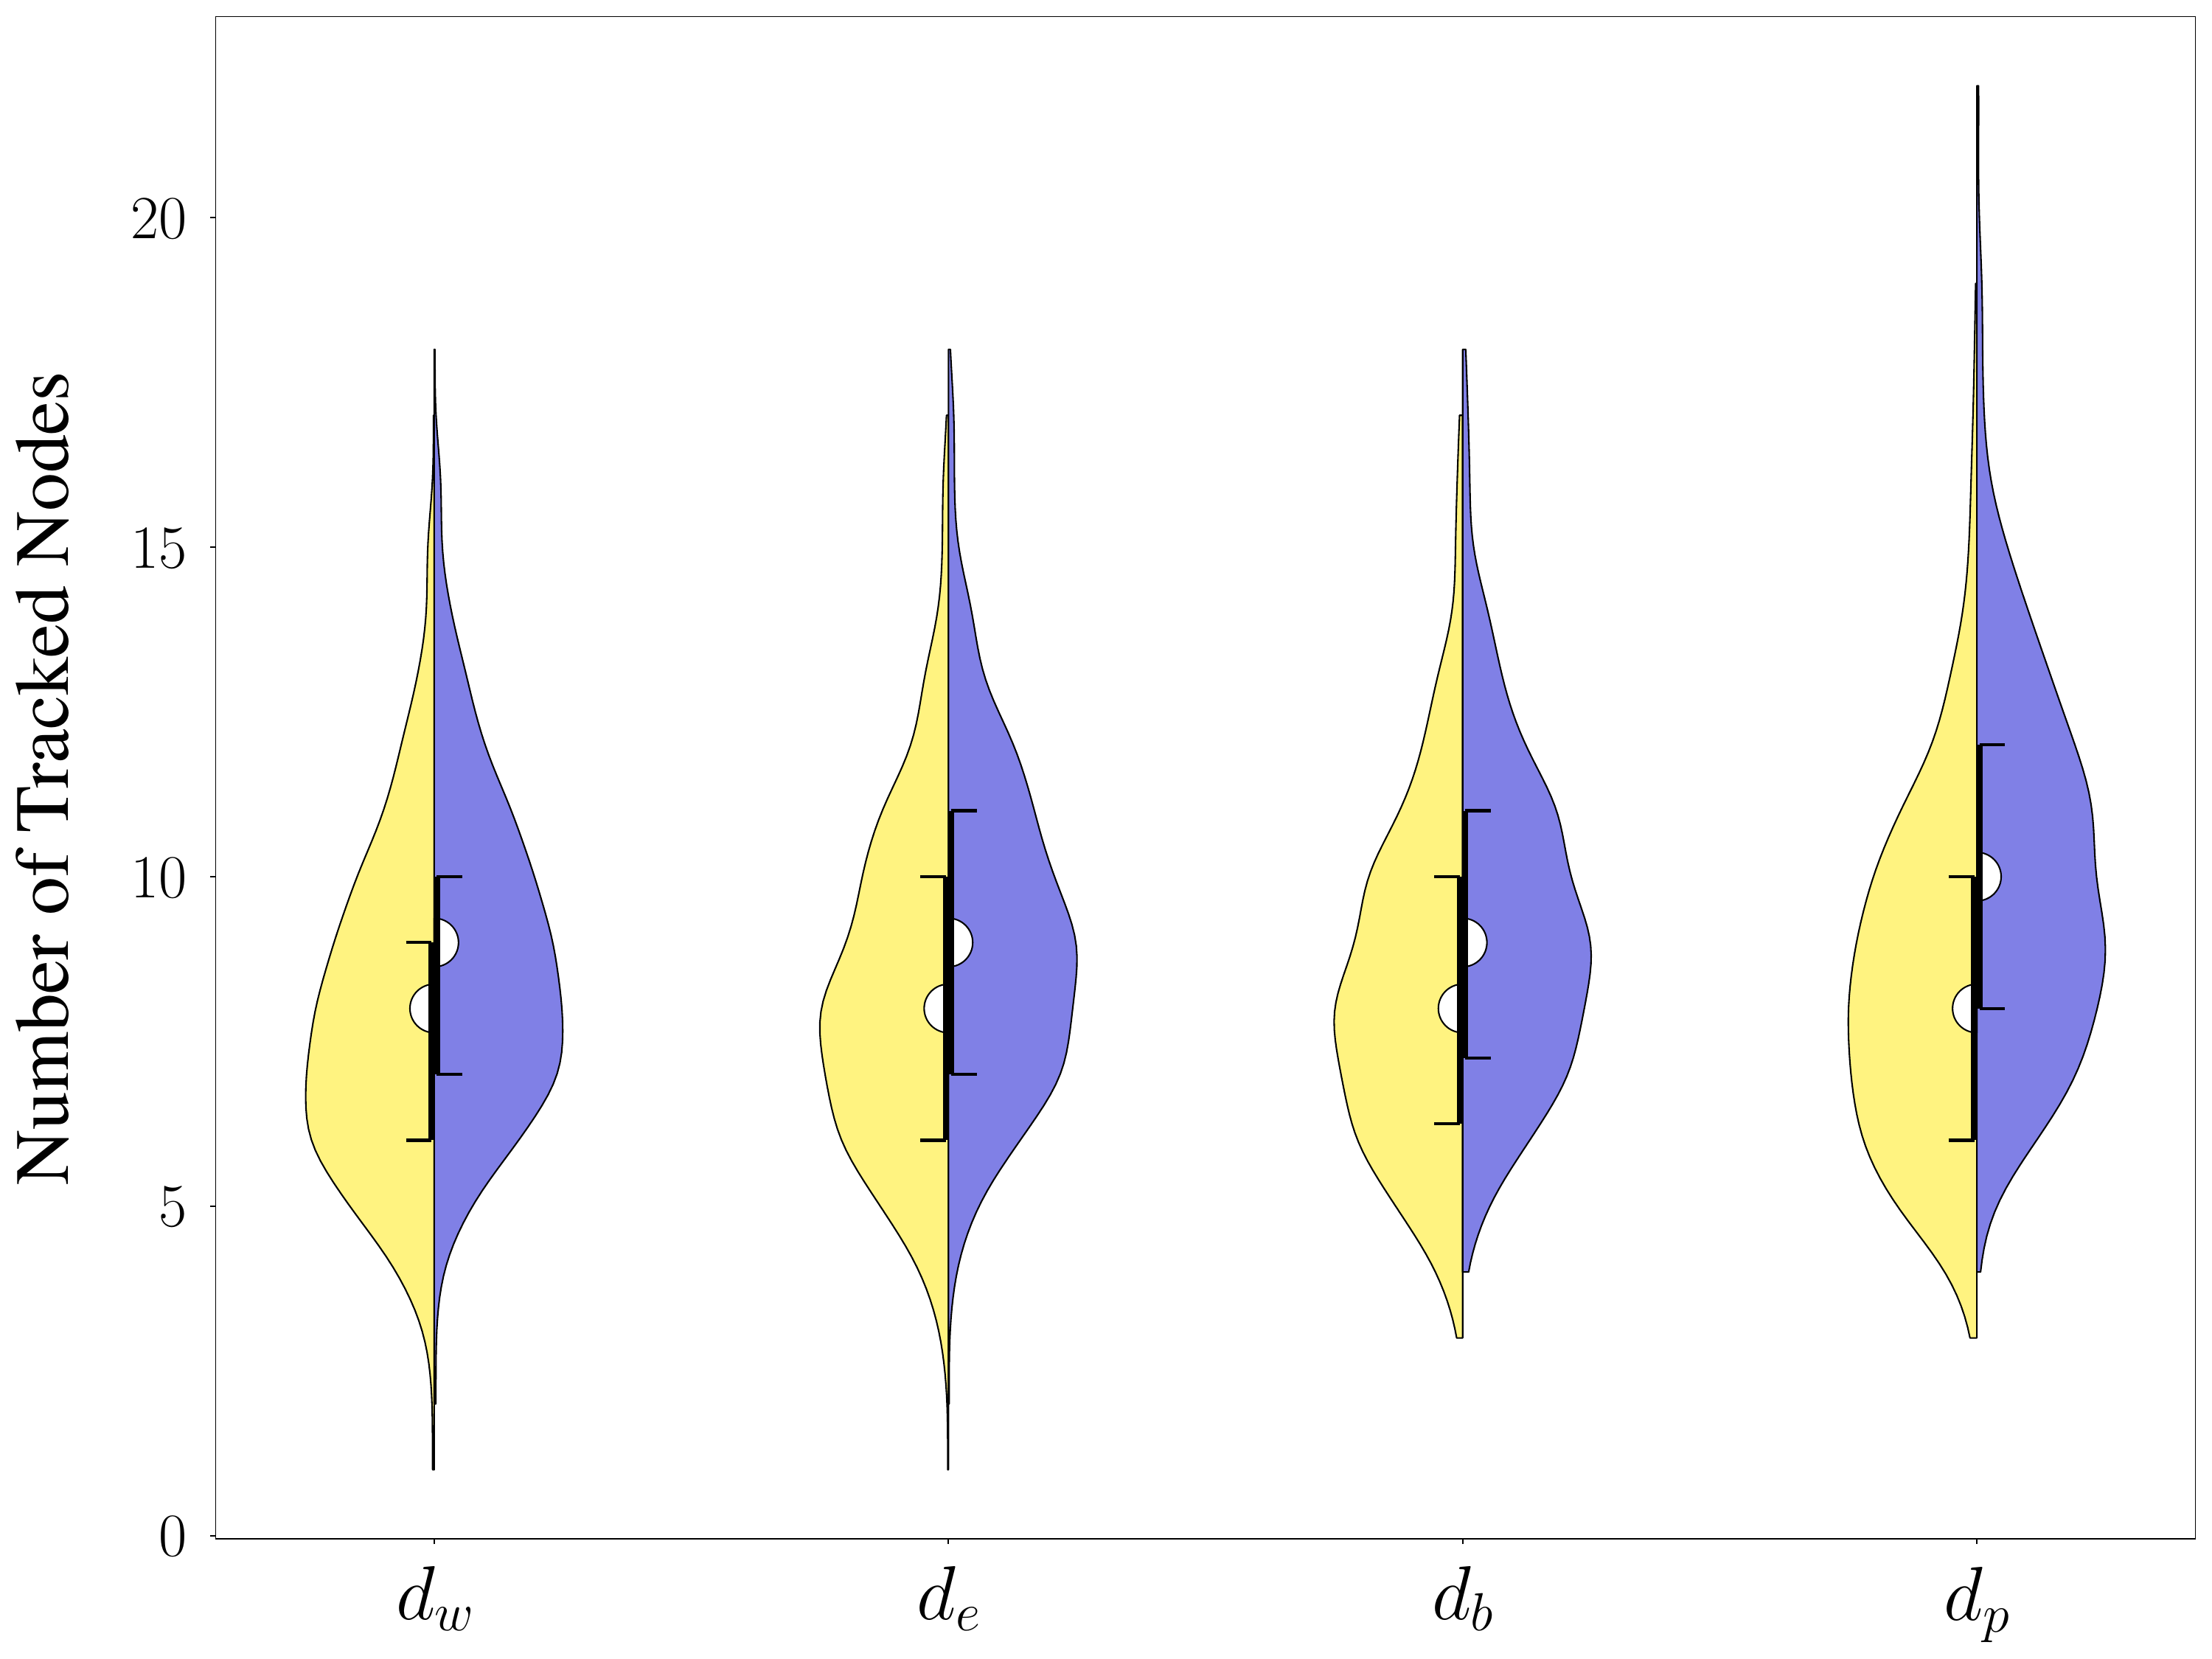}
\caption{
    Distributions of tracked nodes 
    of \dataset{Storms2D},  
    divided by types:
    saddle (yellow) and minima (blue).
}
\label{fig-Storms2DViolin}
\end{figure}

% Length histogram
\begin{figure}%
\begin{subfigure}[t]{\ltwopicwidth}%
\includegraphics[width=\ltwopicwidth]{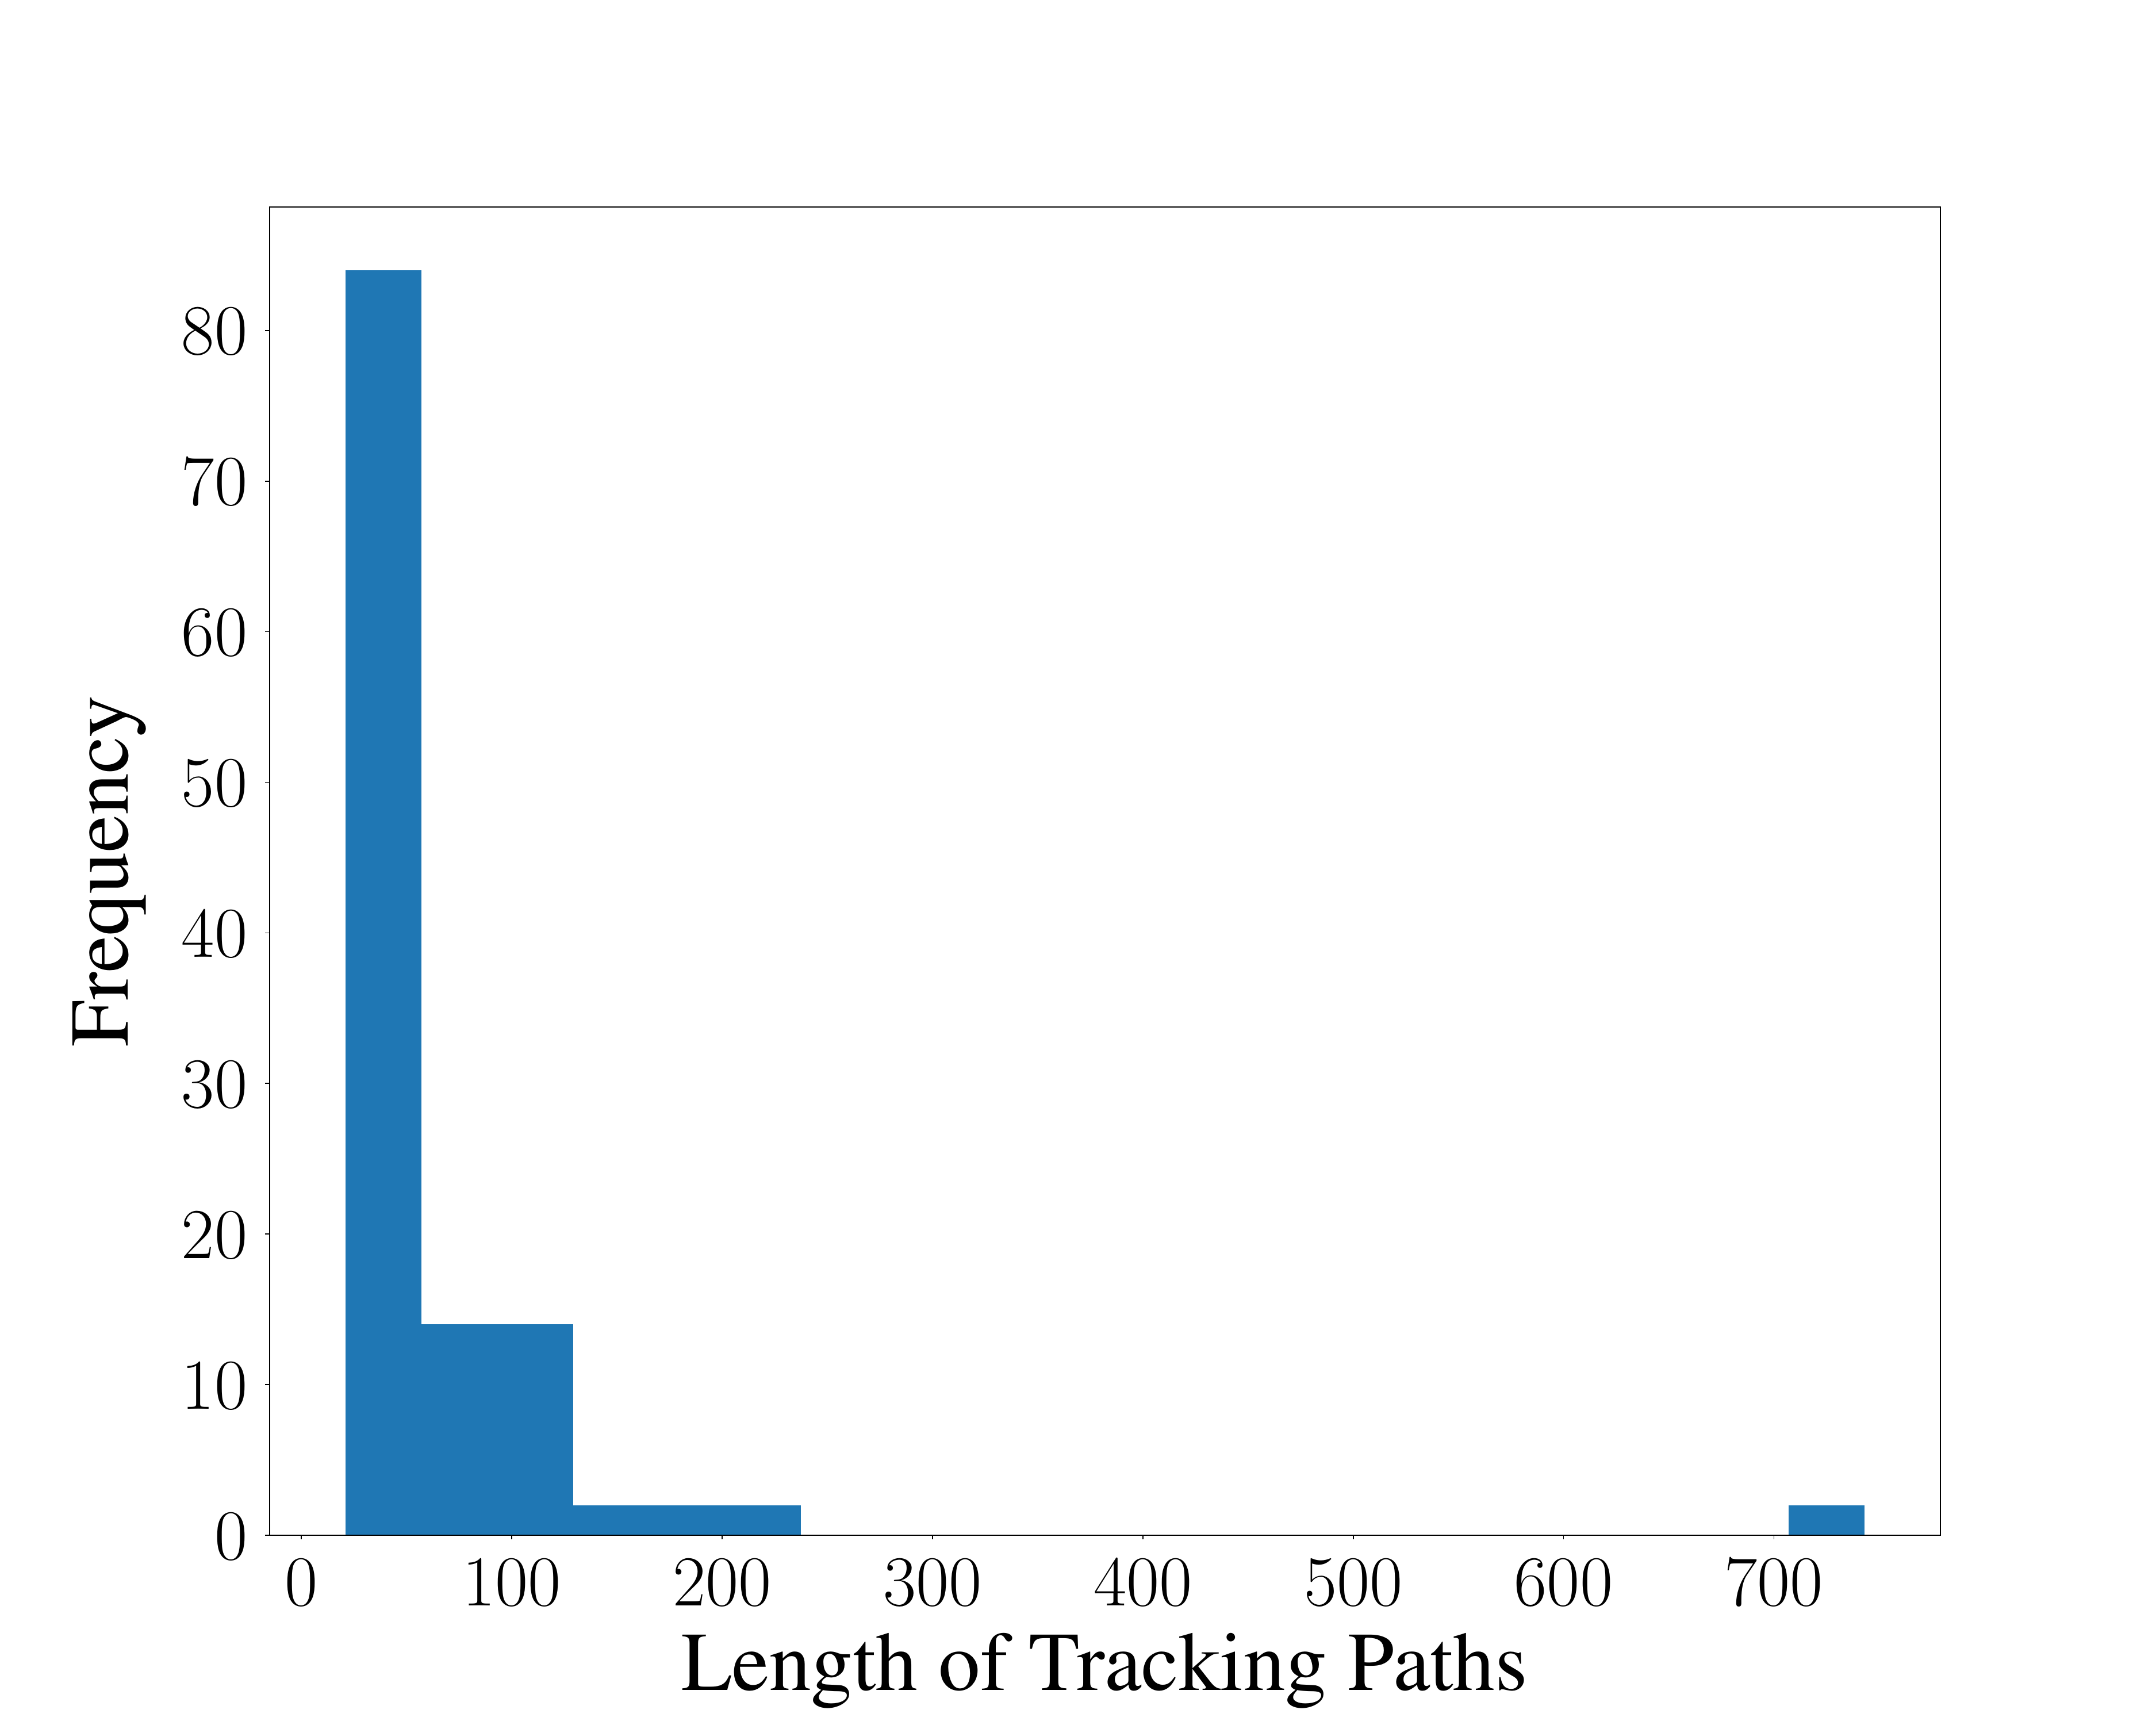}
\caption{$d_w$.}%
\label{fig-LengthHistogramStorms2DW}%
\end{subfigure}
\hfill%
\begin{subfigure}[t]{\ltwopicwidth}%
\includegraphics[width=\ltwopicwidth]{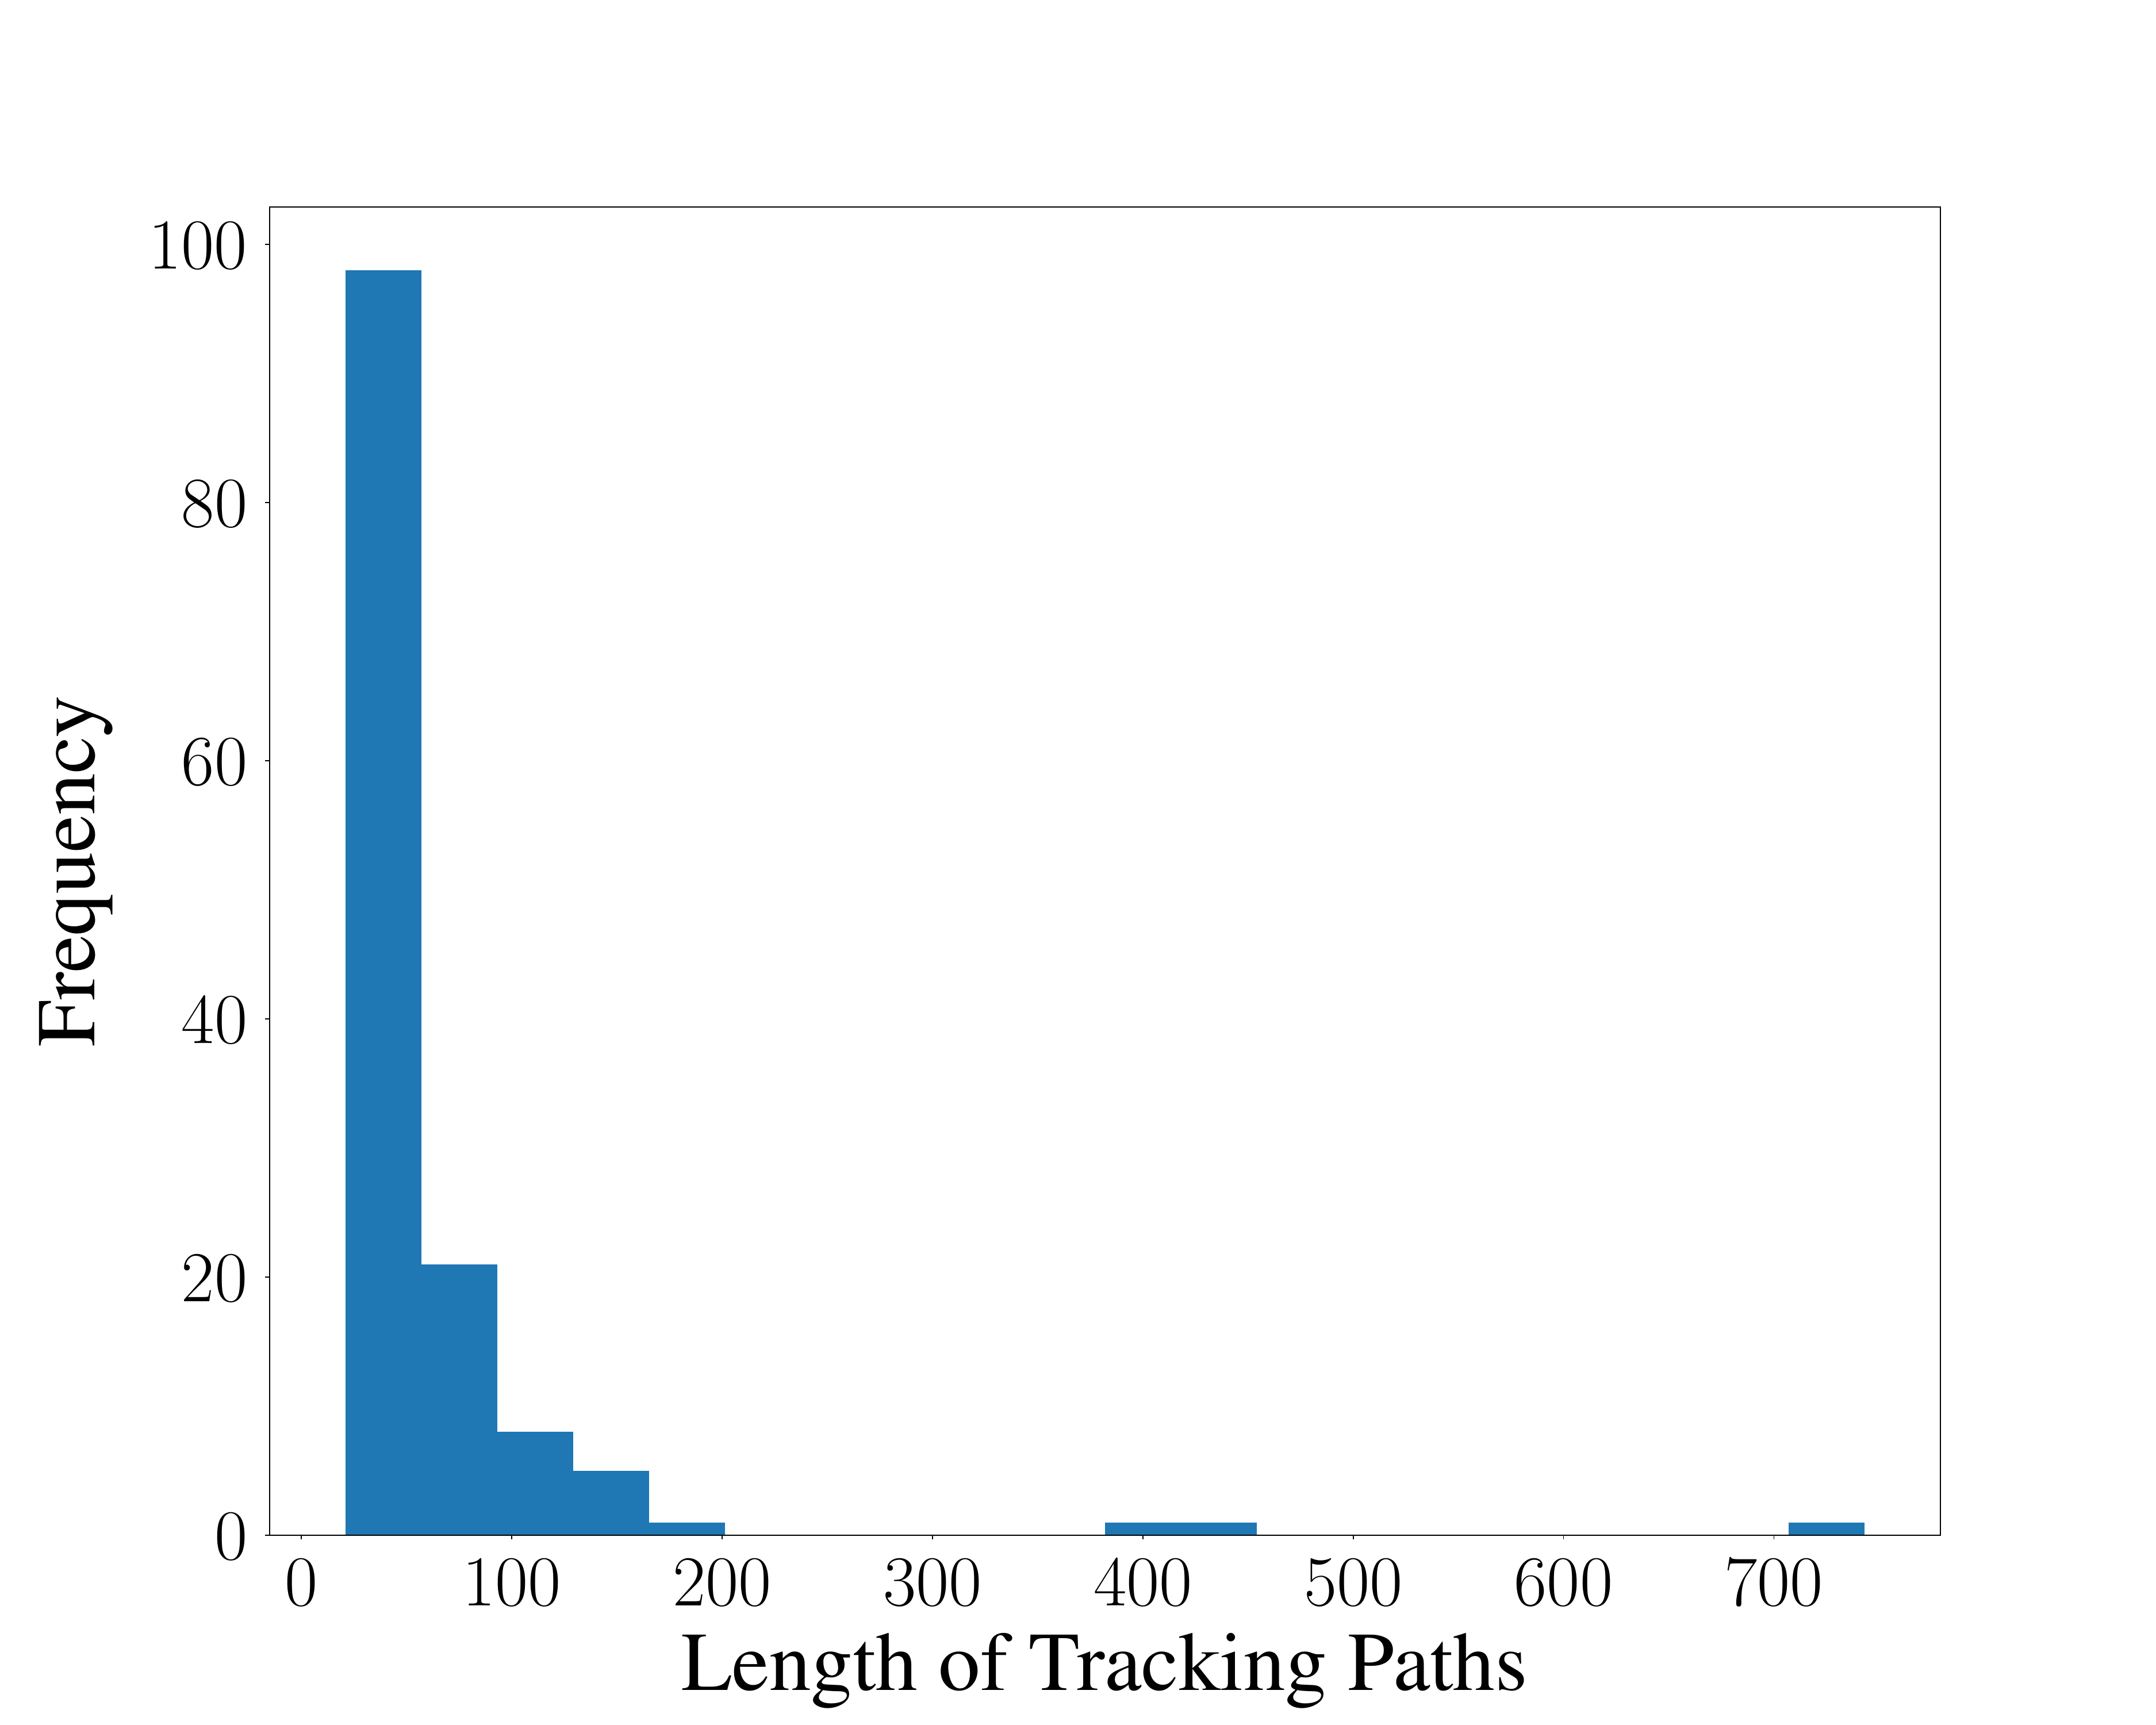}%
\caption{$d_e$.}%
\label{fig-LengthHistogramStorms2DE}%
\end{subfigure}%
\\%
\begin{subfigure}[t]{\ltwopicwidth}%
\includegraphics[width=\ltwopicwidth]{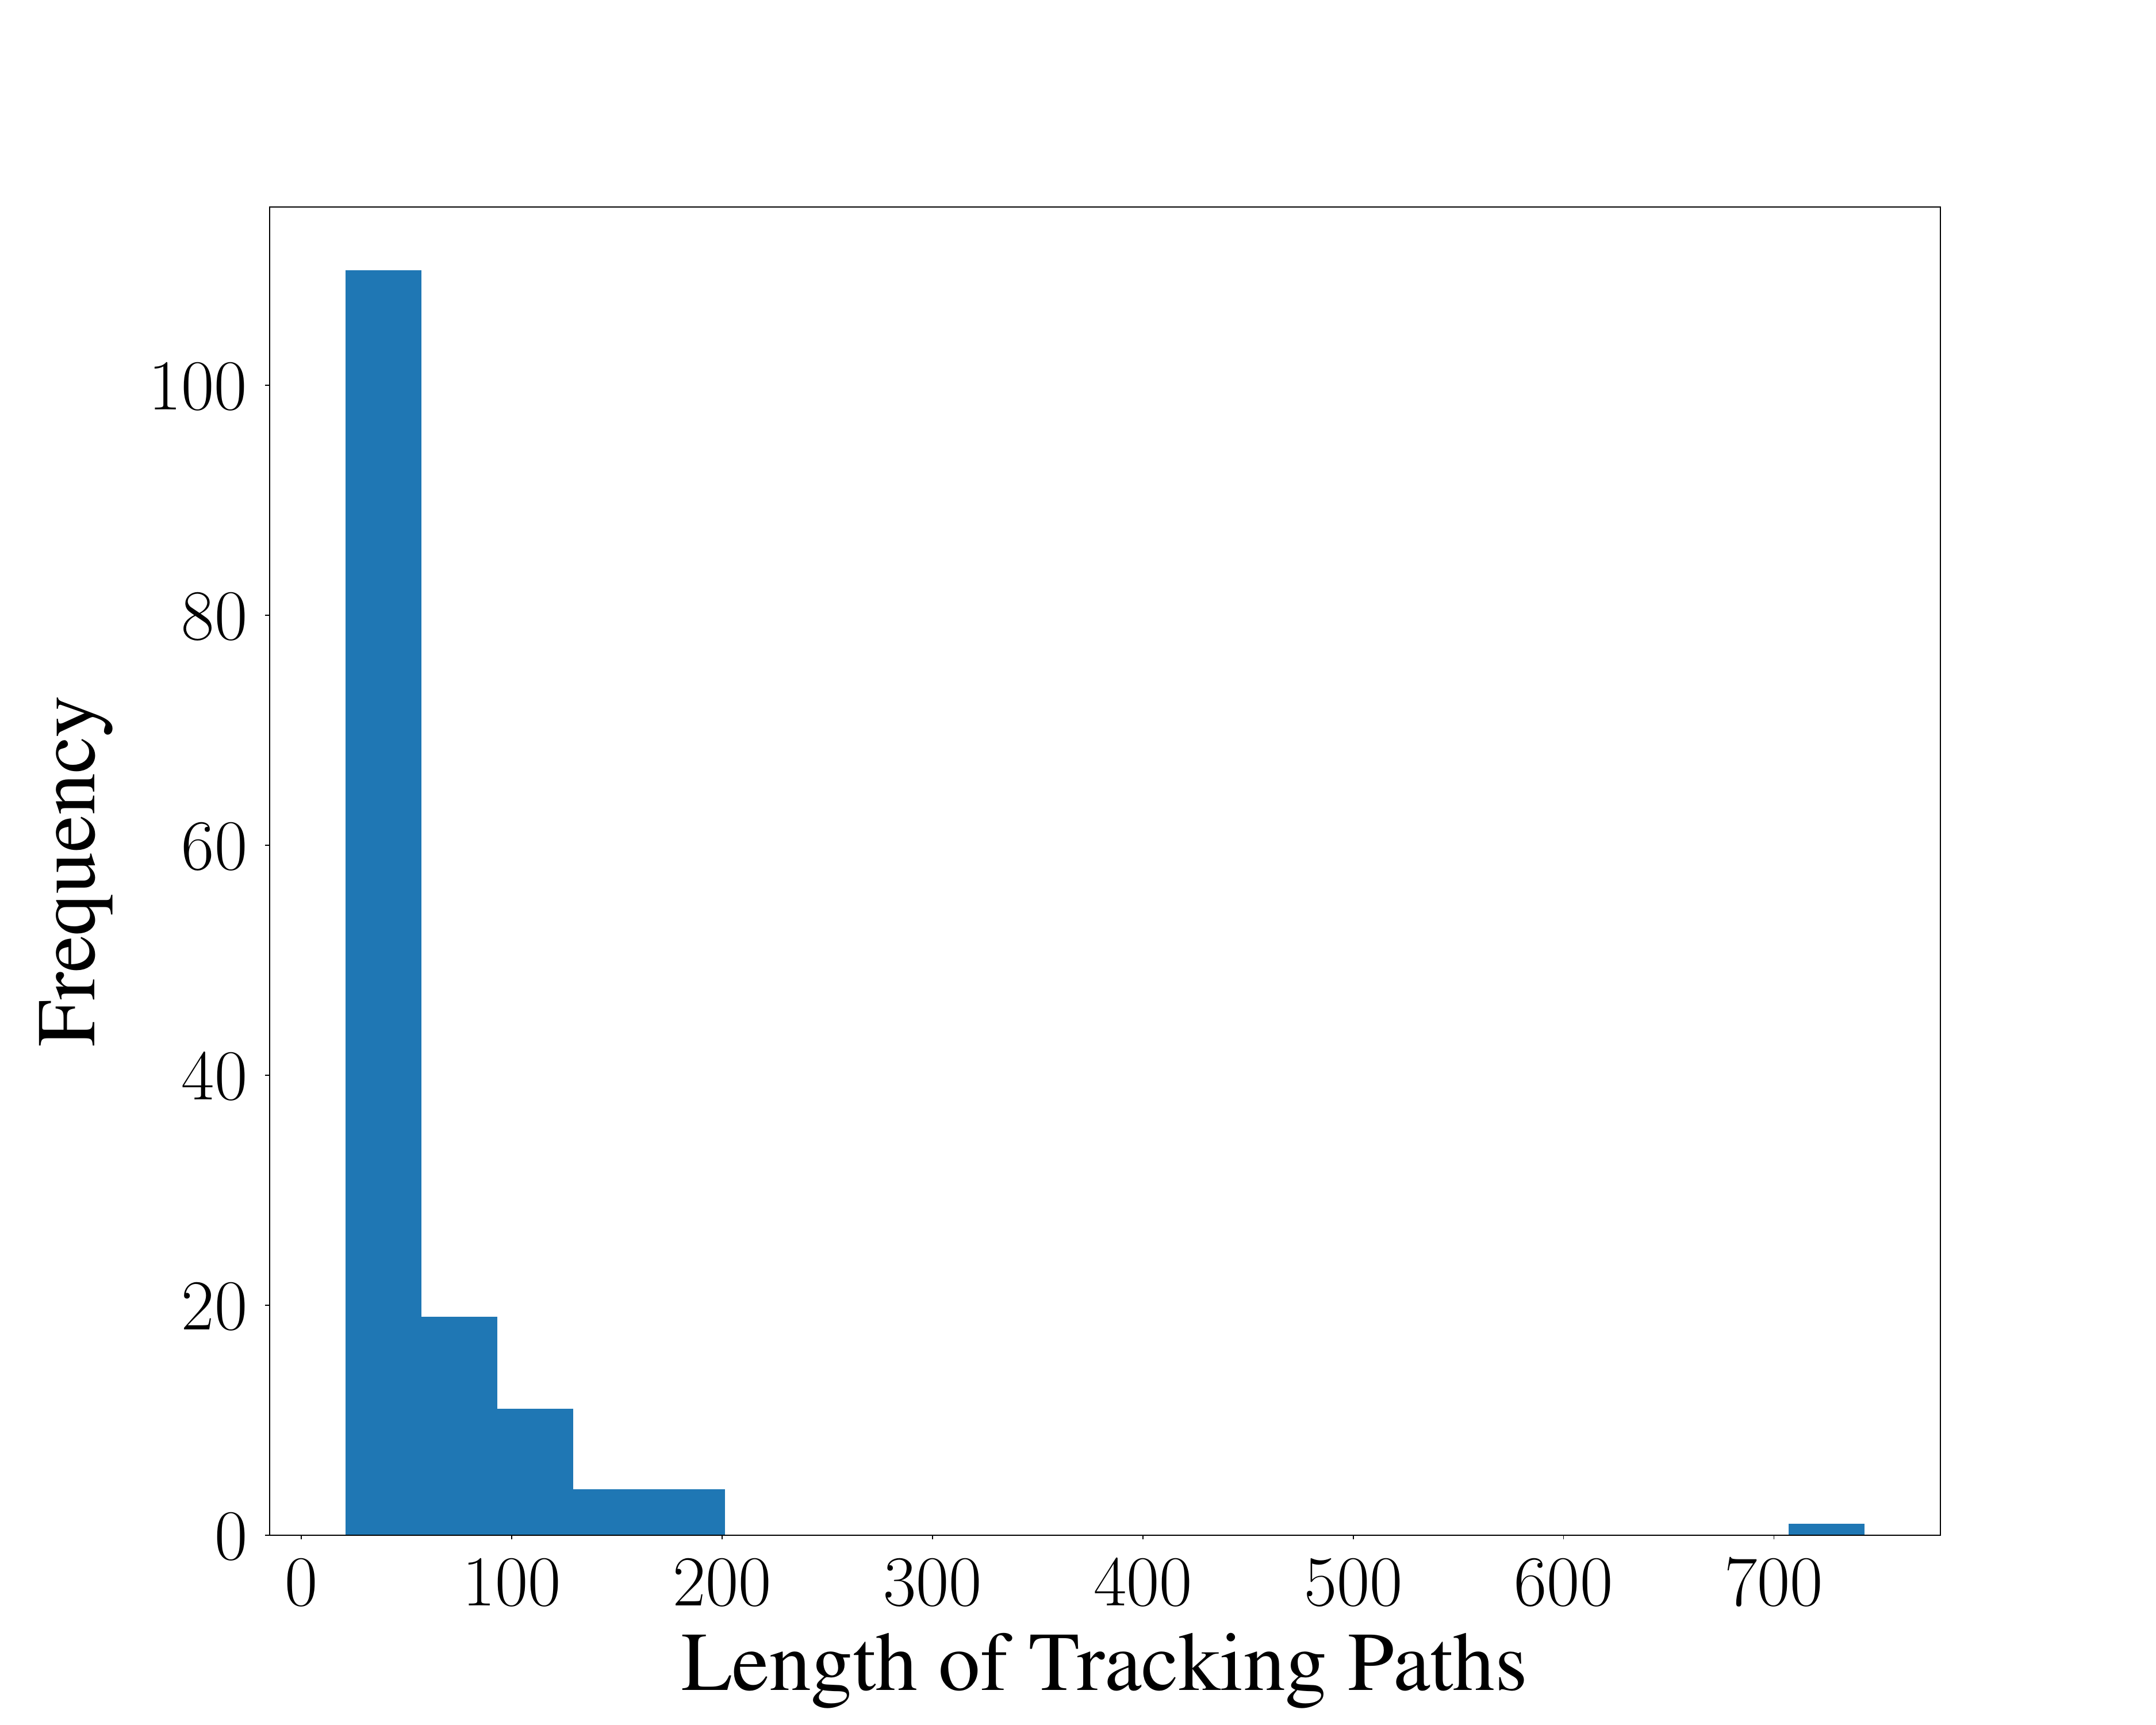}%
\caption{$d_b$.}%
\label{fig-LengthHistogramStorms2DB}%
\end{subfigure}%
\hfill%
\begin{subfigure}[t]{\ltwopicwidth}%
\includegraphics[width=\ltwopicwidth]{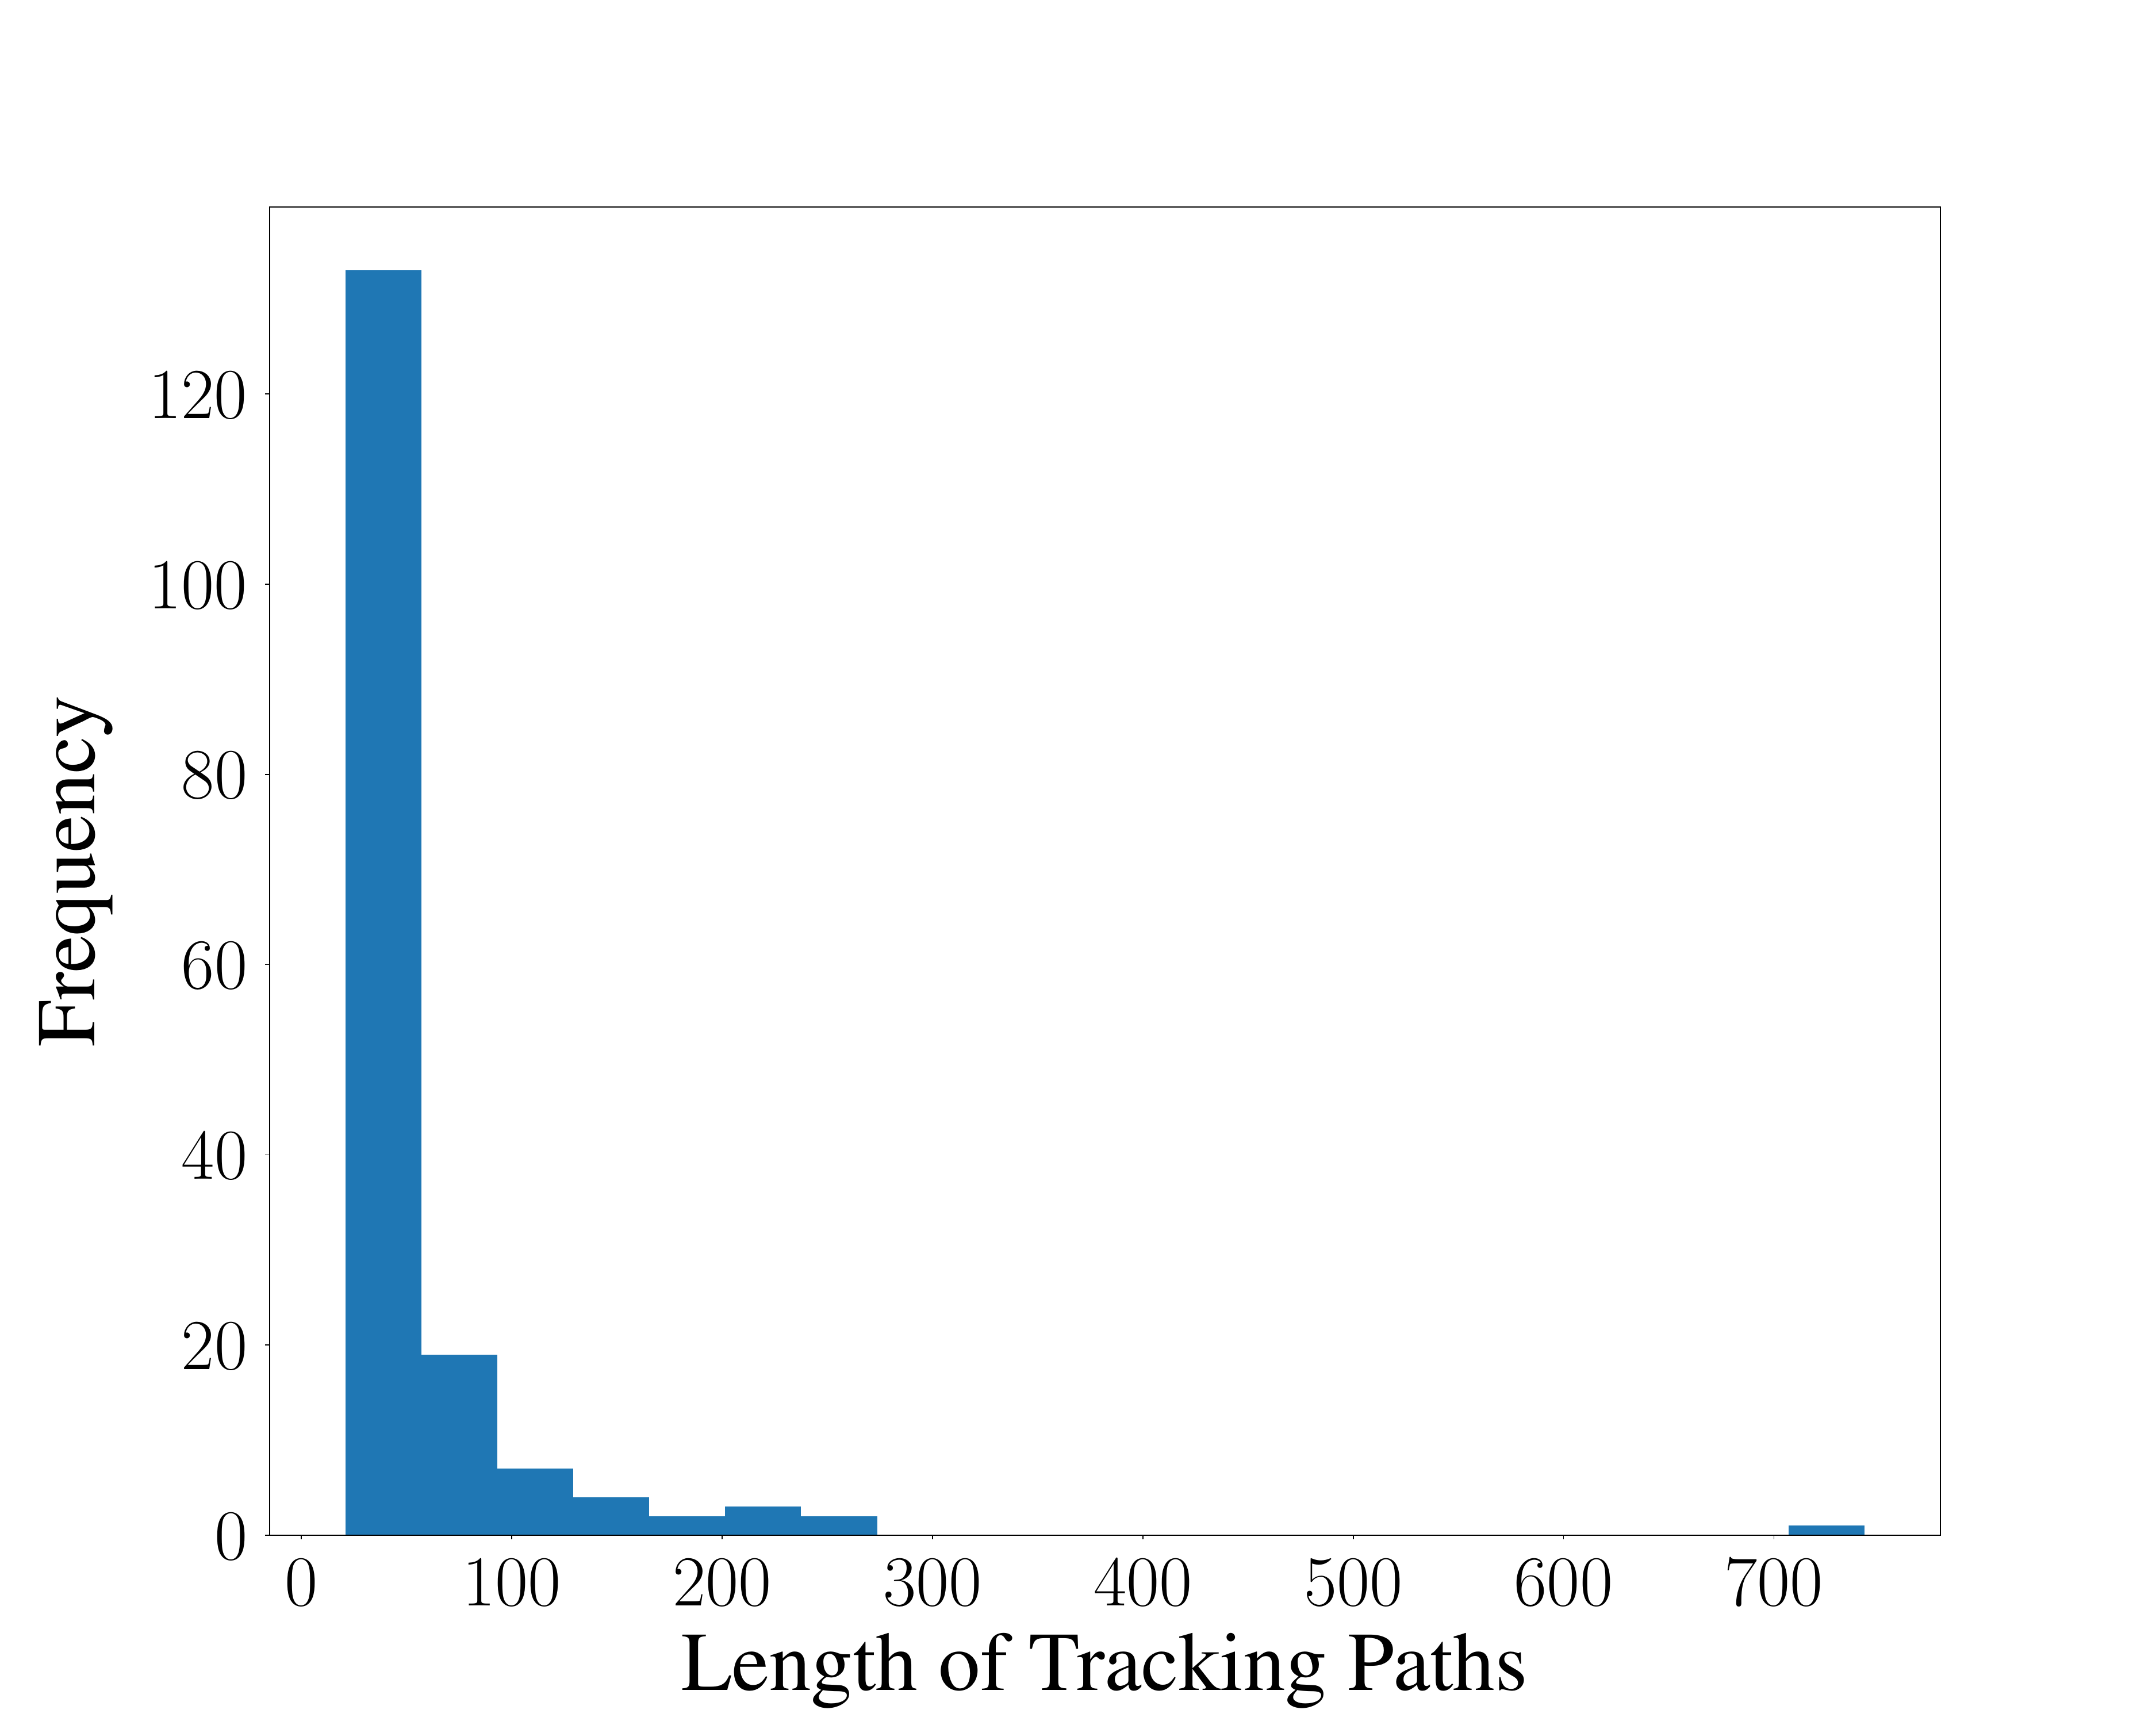}%
\caption{$d_p$.}%
\label{fig-LengthHistogramStorms2DP}%
\end{subfigure}%
\caption{Histograms of the length of the tracking paths 
    of \dataset{Storms2D}.}%
\label{fig-LengthHisgoramStorms2D}%
\end{figure}

\begin{figure}
\centering
\includegraphics[width=0.8\linewidth]{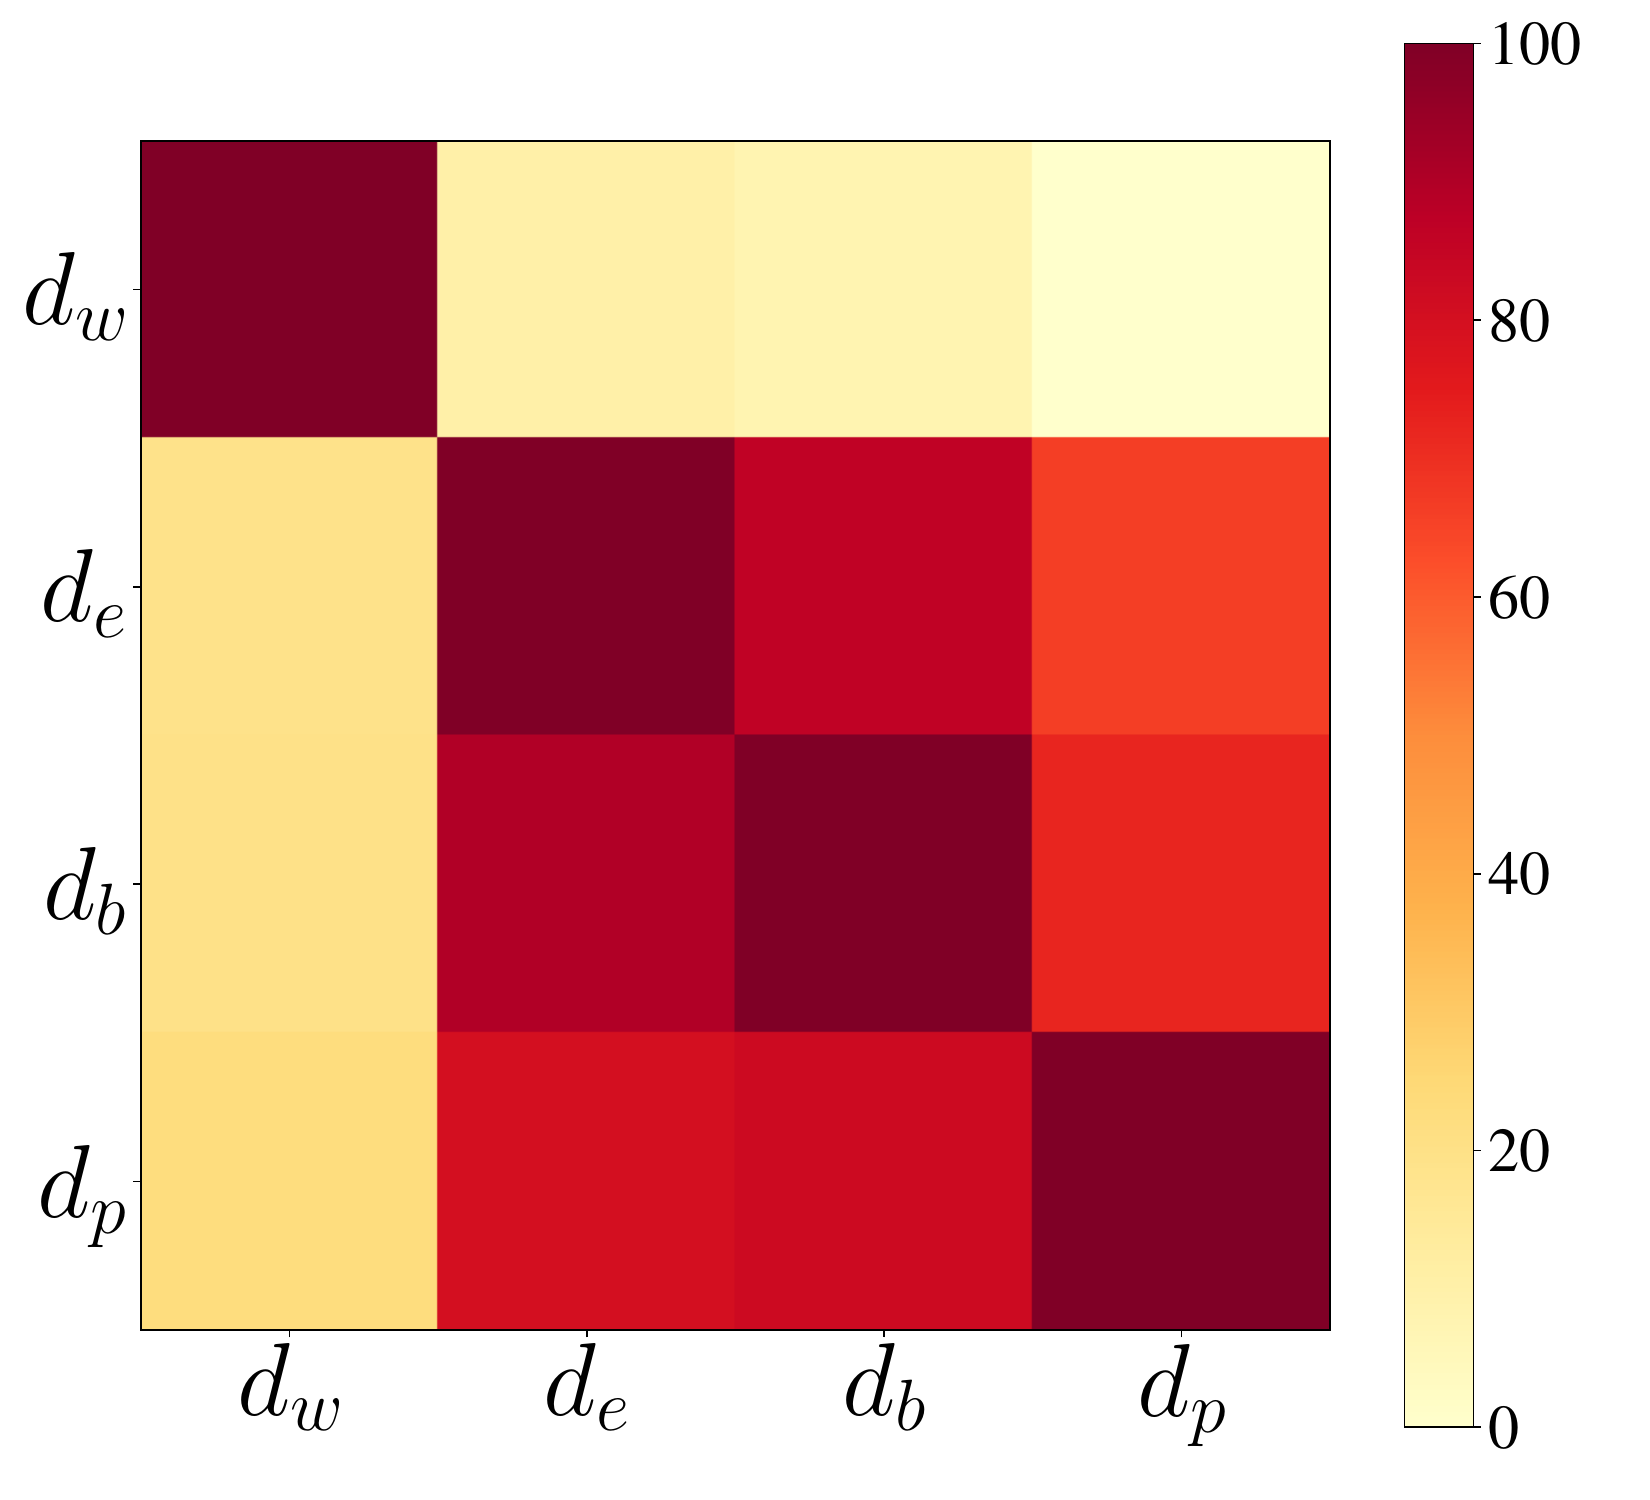}
\caption{
    Pairwise differences between the methods on the columns
    in relation to the methods on the rows
    for \dataset{Storms2D}.
}
\label{fig-Storms2DSimilarities}
\end{figure}

\subsection*{Results using Boussinesq2D}
The results of the experiments using \dataset{Boussinesq2D}
are shown from \Cref{fig-Boussinesq2DAllNodes}
to \Cref{fig-Boussinesq2DSimilarities}.

\begin{figure}
\centering
\includegraphics[width=0.8\linewidth]{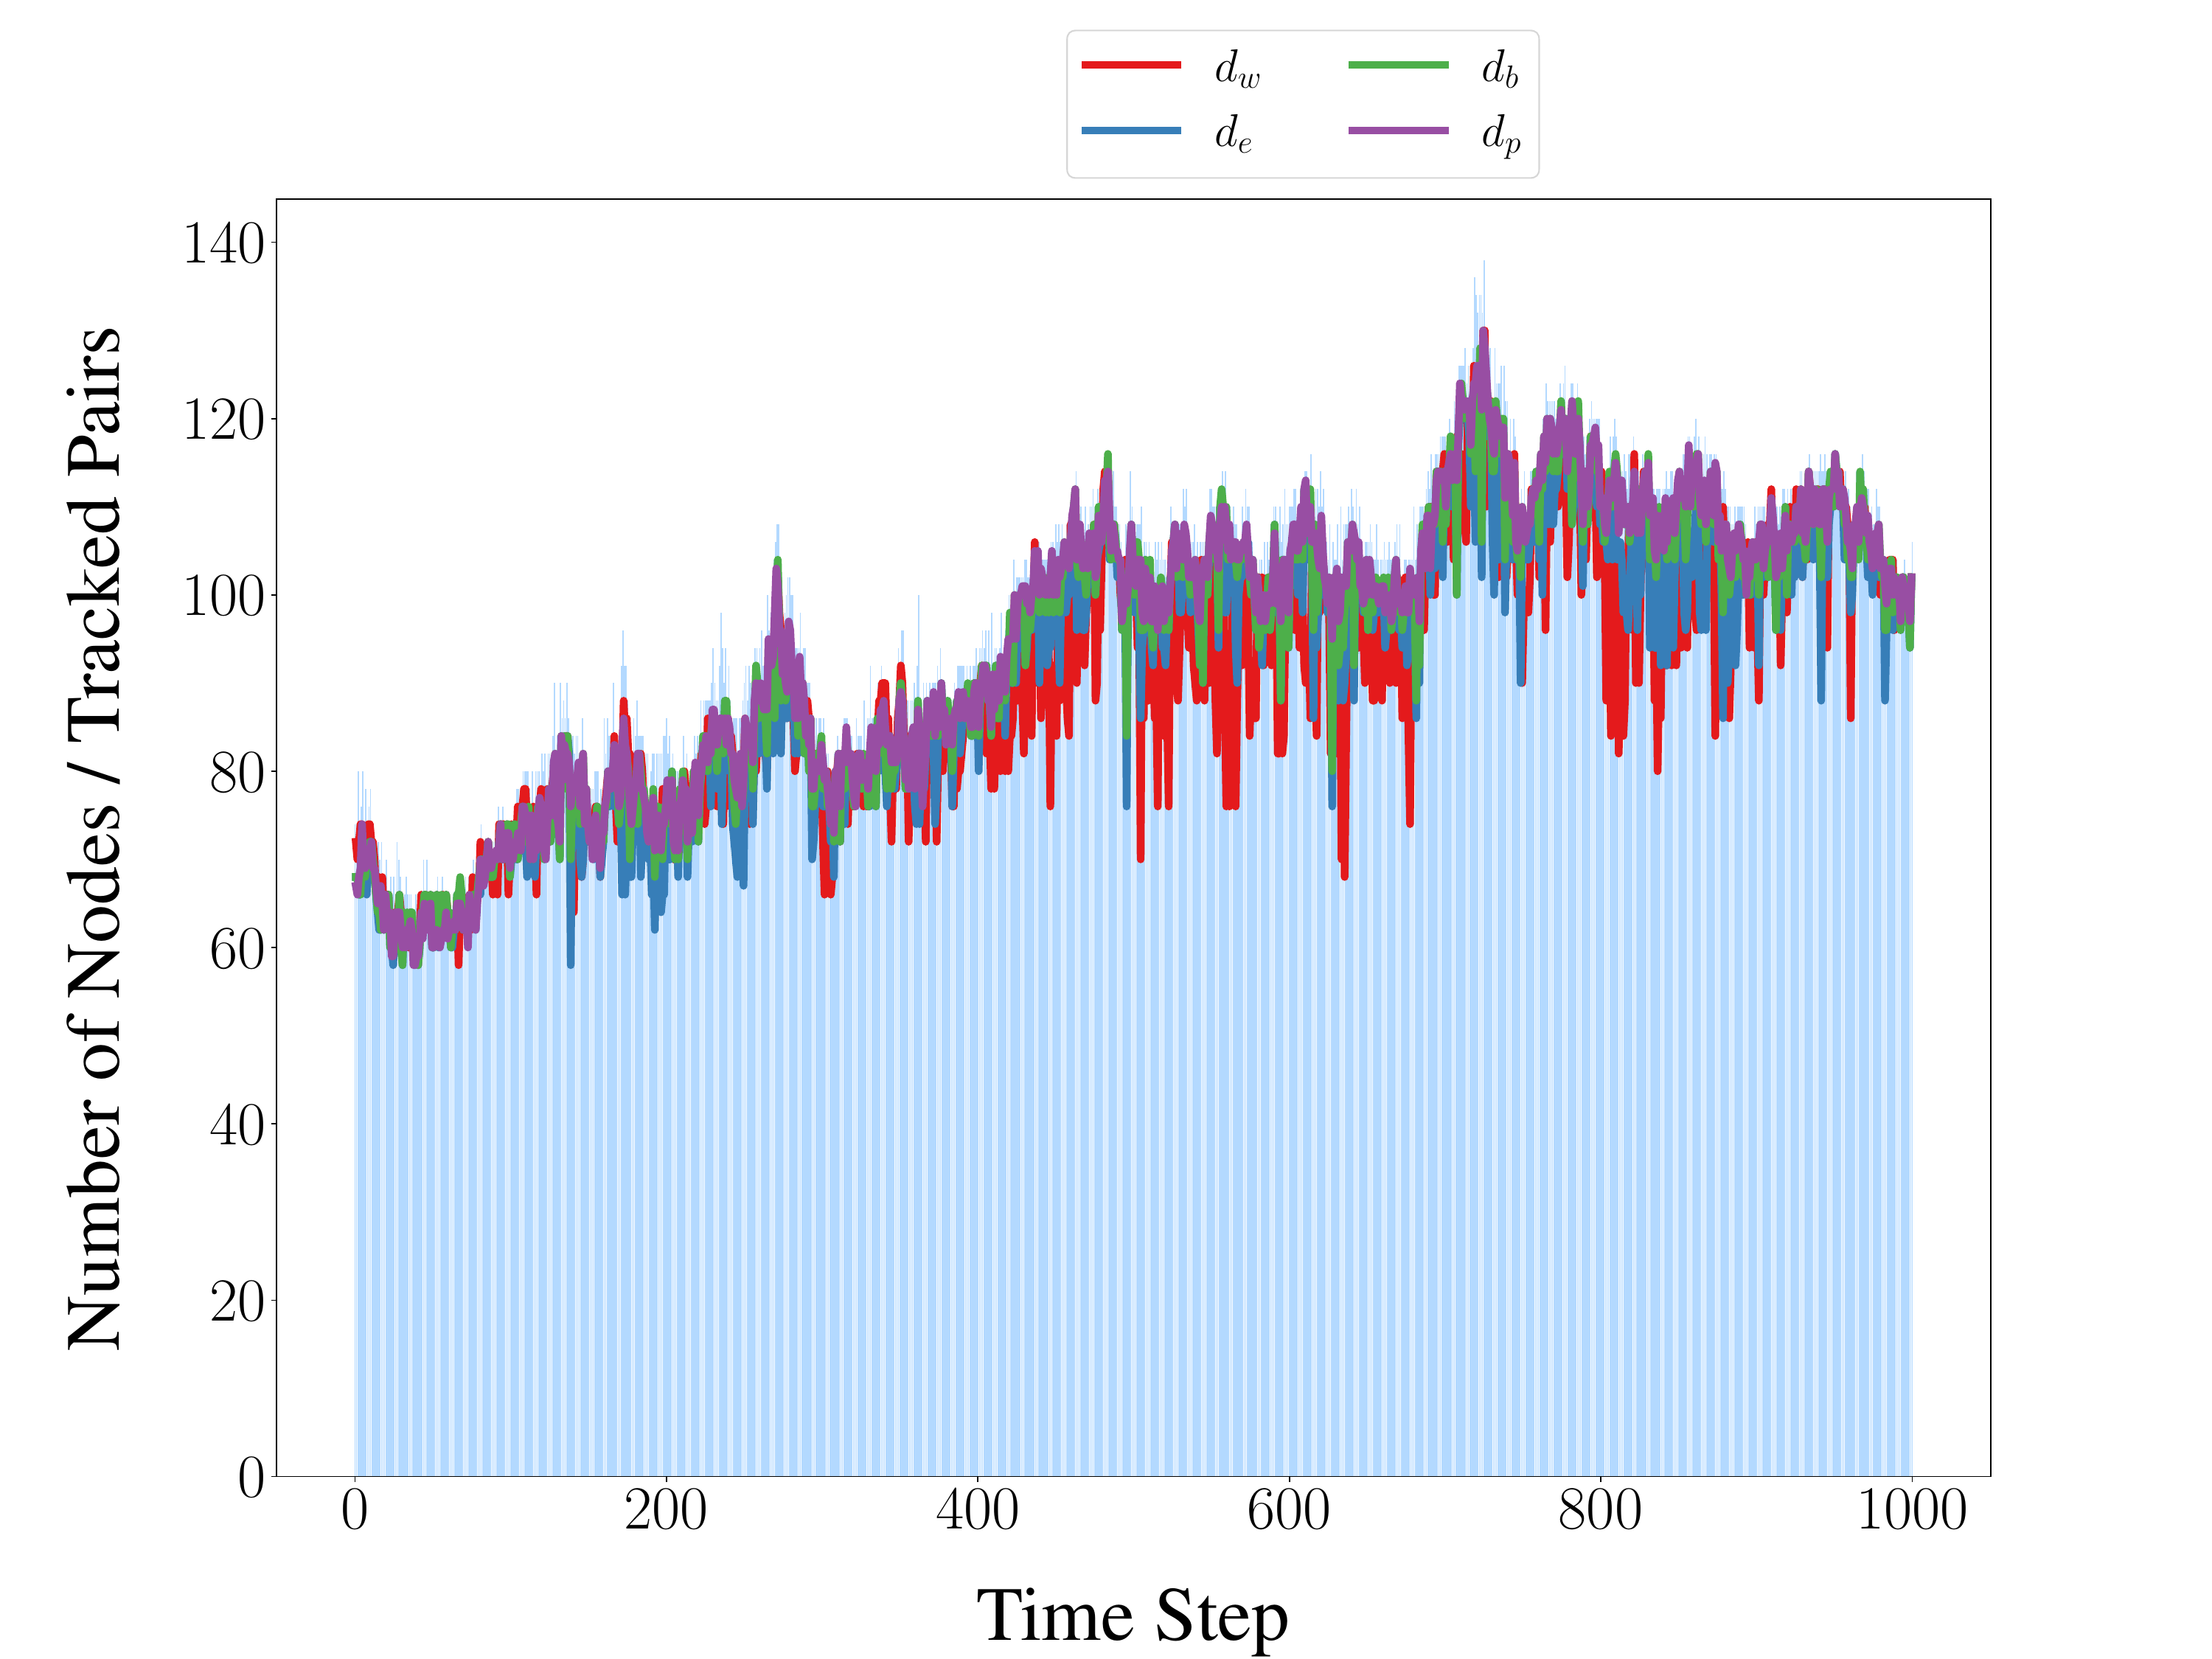}
\caption{
    Number of tracked nodes (colored and labeled) 
    relative to the total nodes of merge trees (light blue bars)
    for \dataset{Boussinesq2D}.
}
\label{fig-Boussinesq2DAllNodes}
\end{figure}

\begin{figure}
\centering
\includegraphics[width=0.8\linewidth]{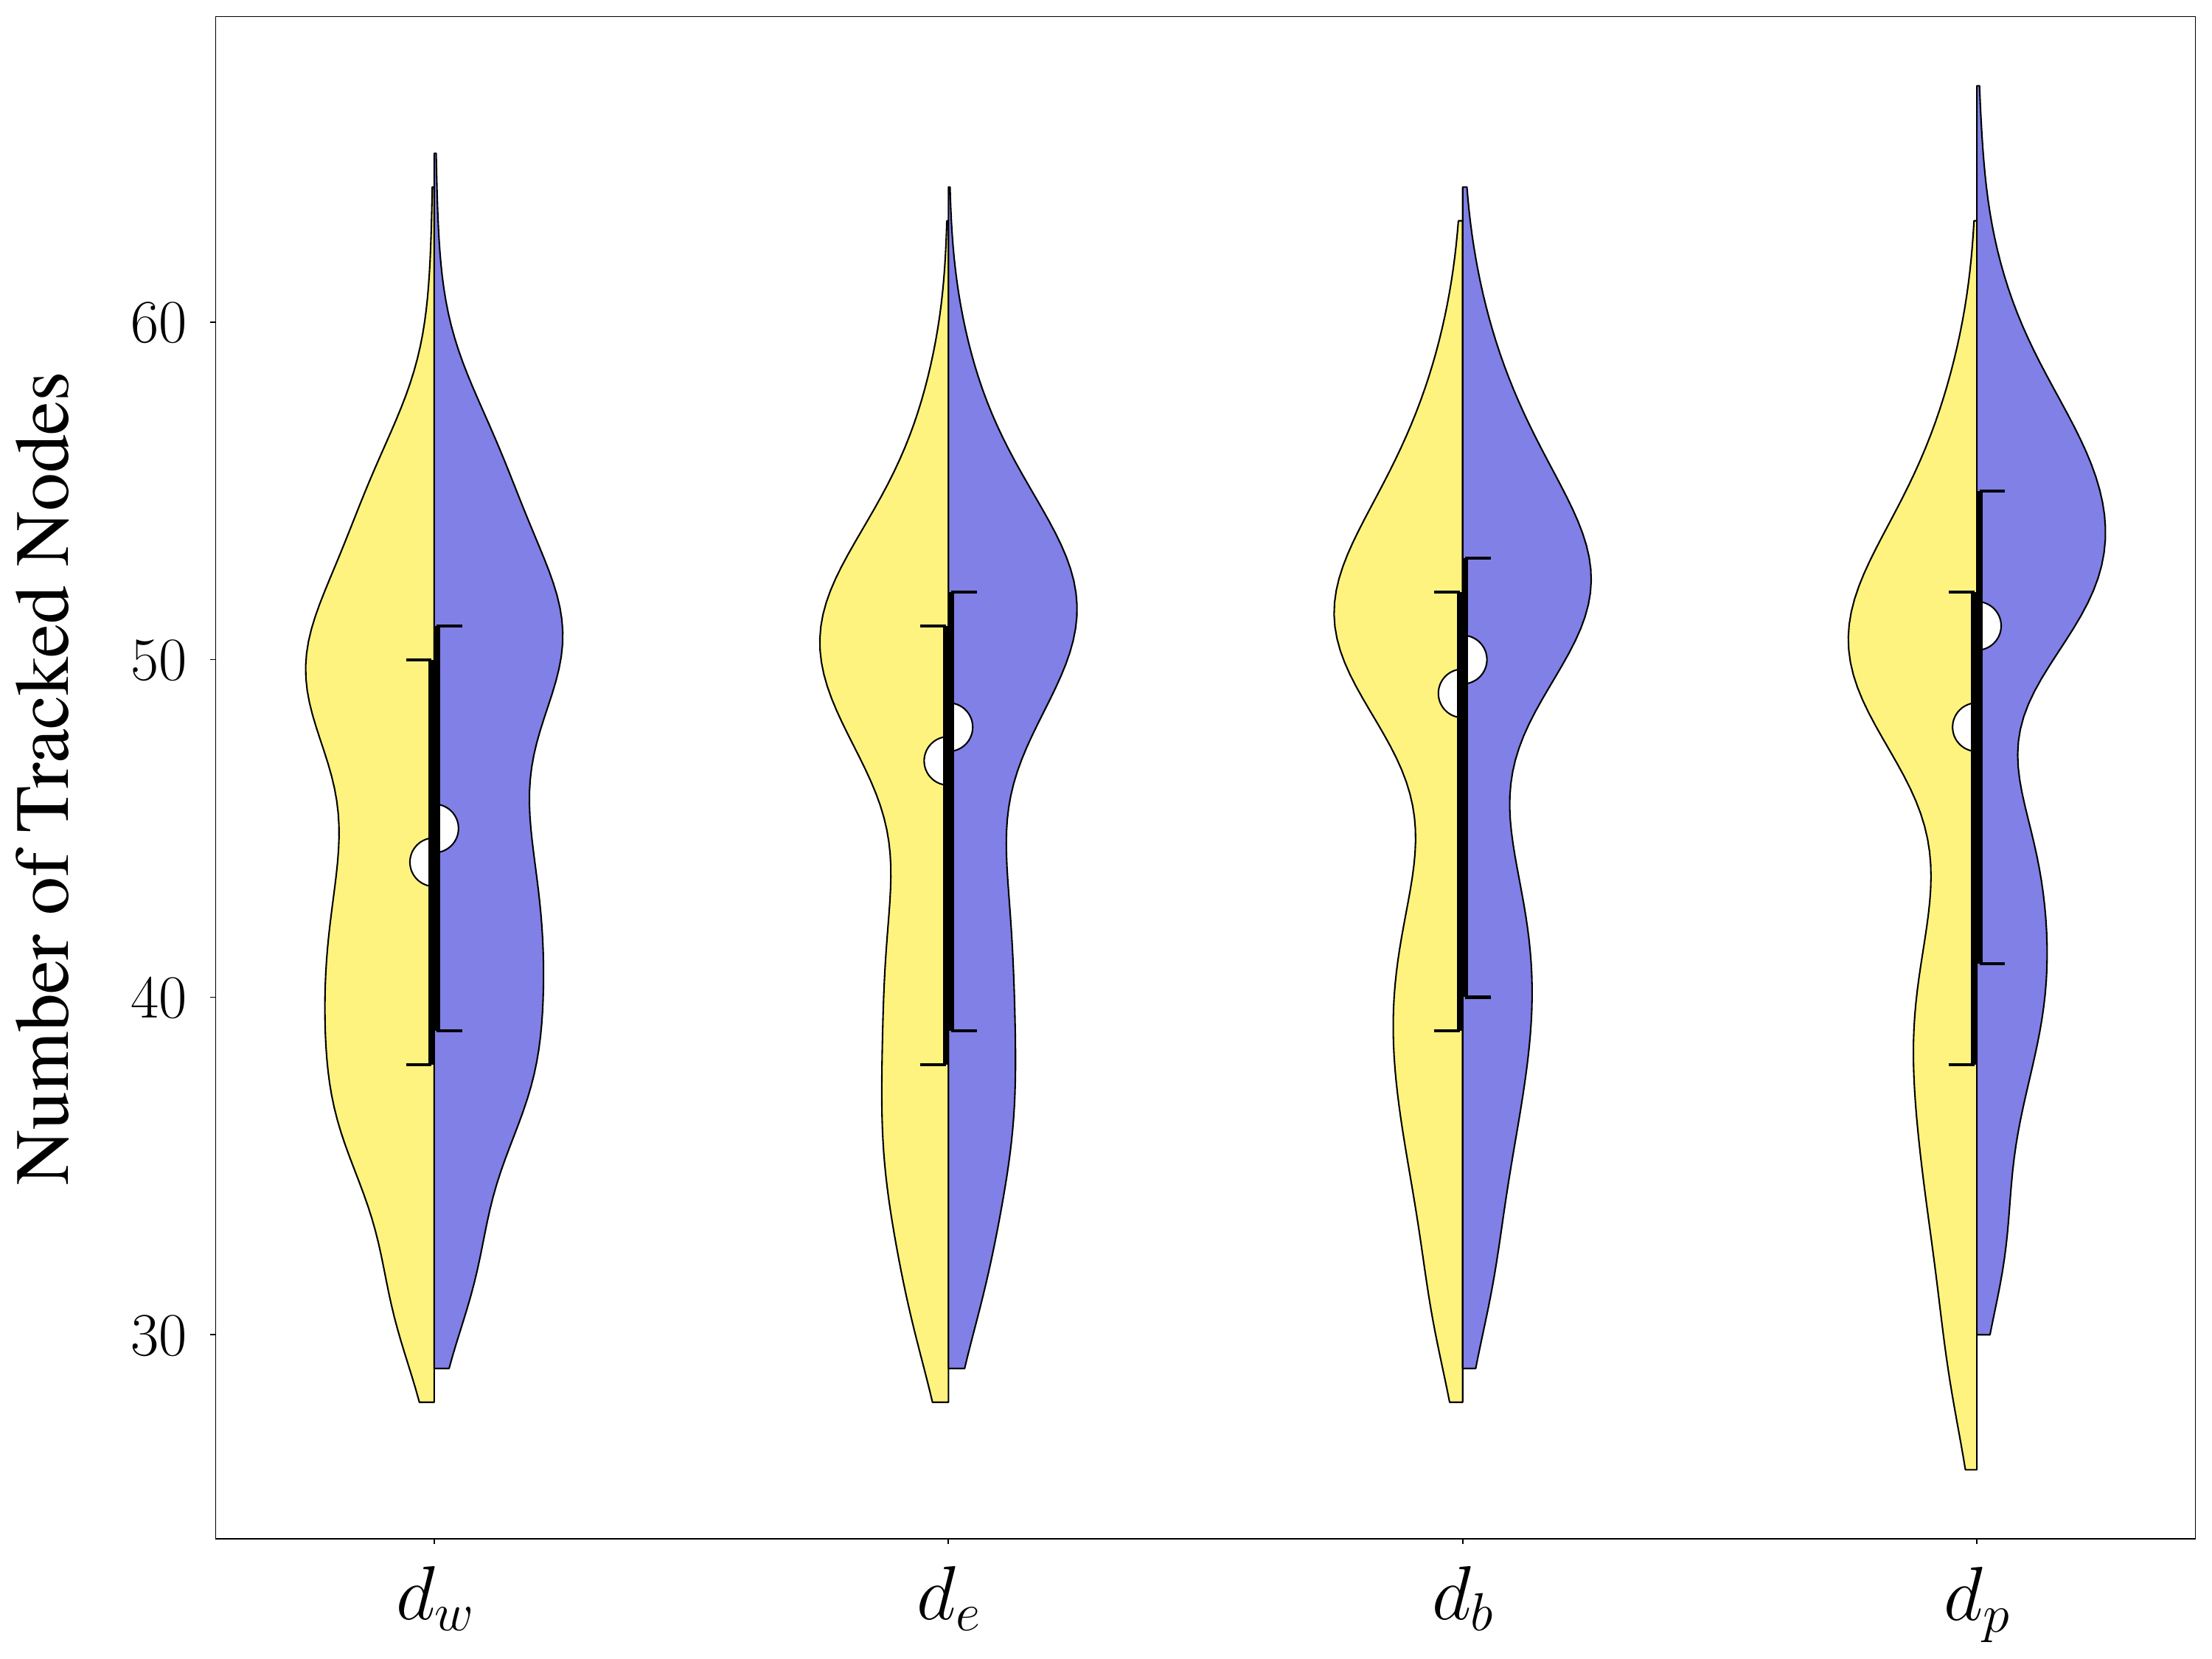}
\caption{
    Distributions of tracked nodes 
    over the chosen time steps of \dataset{Boussinesq2D},  
    divided by types:
    saddle (yellow) and minima (blue).
}
\label{fig-Boussinesq2DViolin}
\end{figure}

% Length histogram
\begin{figure}%
\begin{subfigure}[t]{\ltwopicwidth}%
\includegraphics[width=\ltwopicwidth]{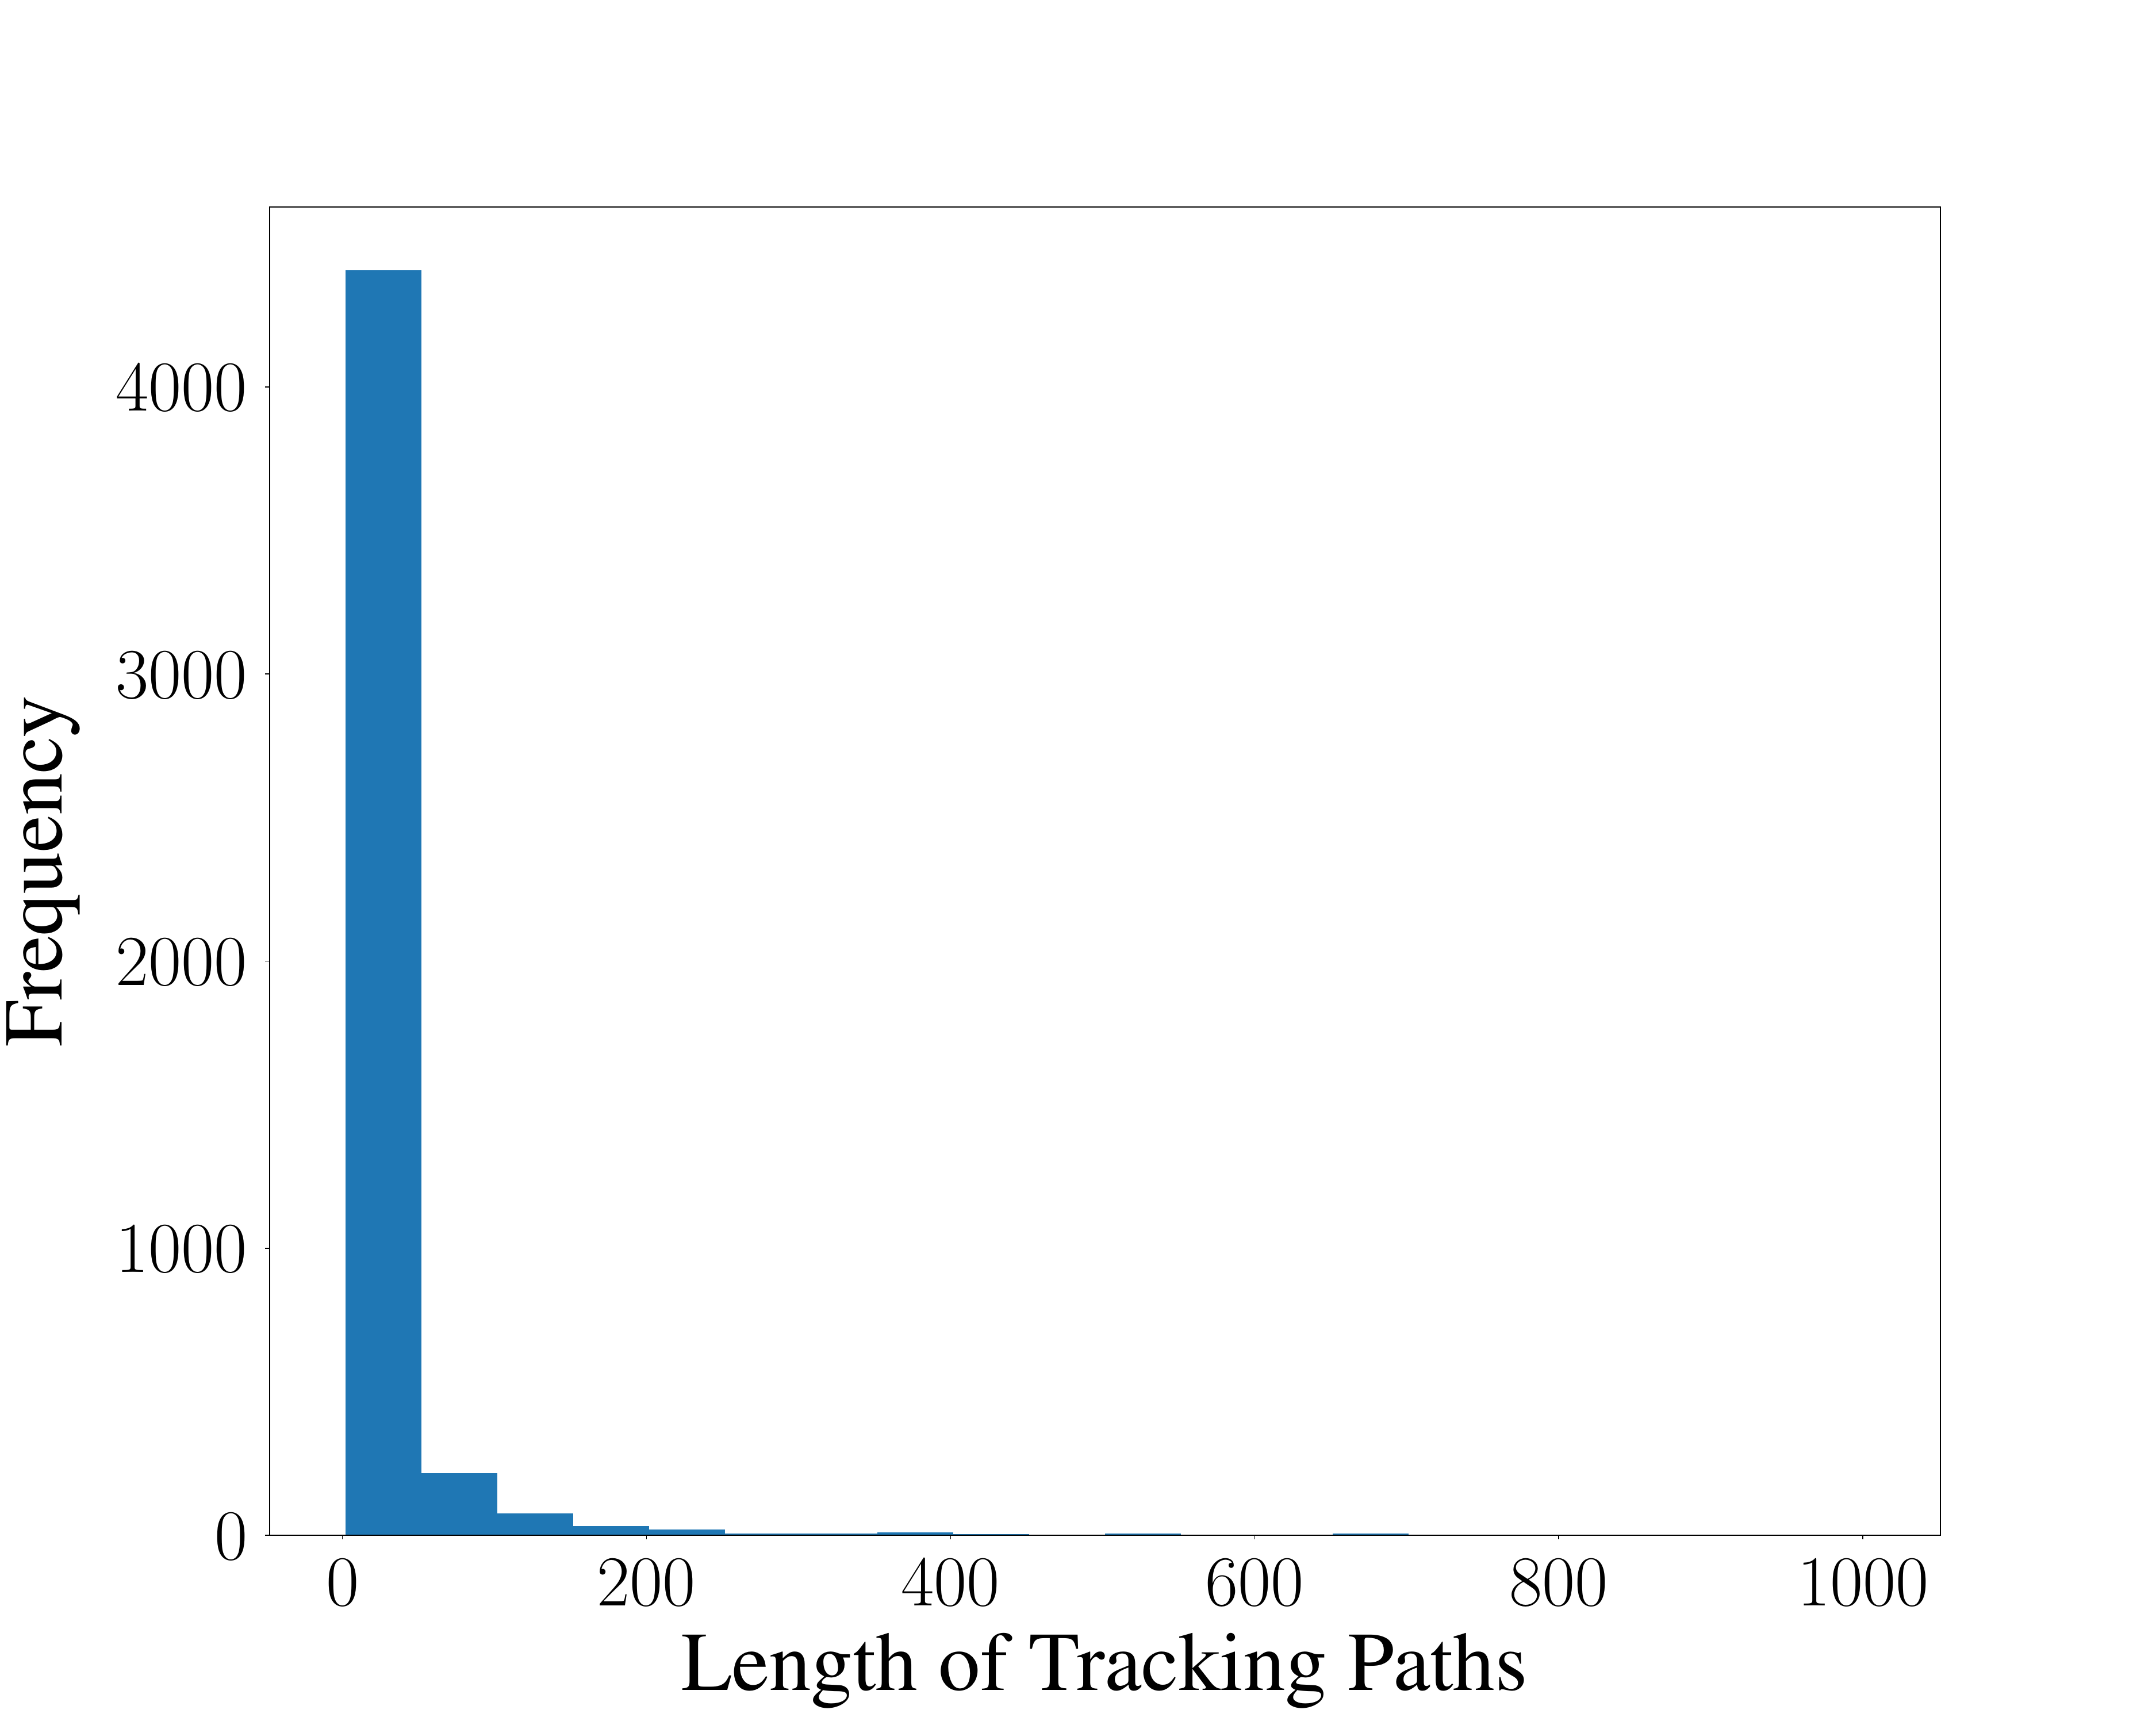}
\caption{$d_w$.}%
\label{fig-LengthHistogramBoussinesq2DW}%
\end{subfigure}
\hfill%
\begin{subfigure}[t]{\ltwopicwidth}%
\includegraphics[width=\ltwopicwidth]{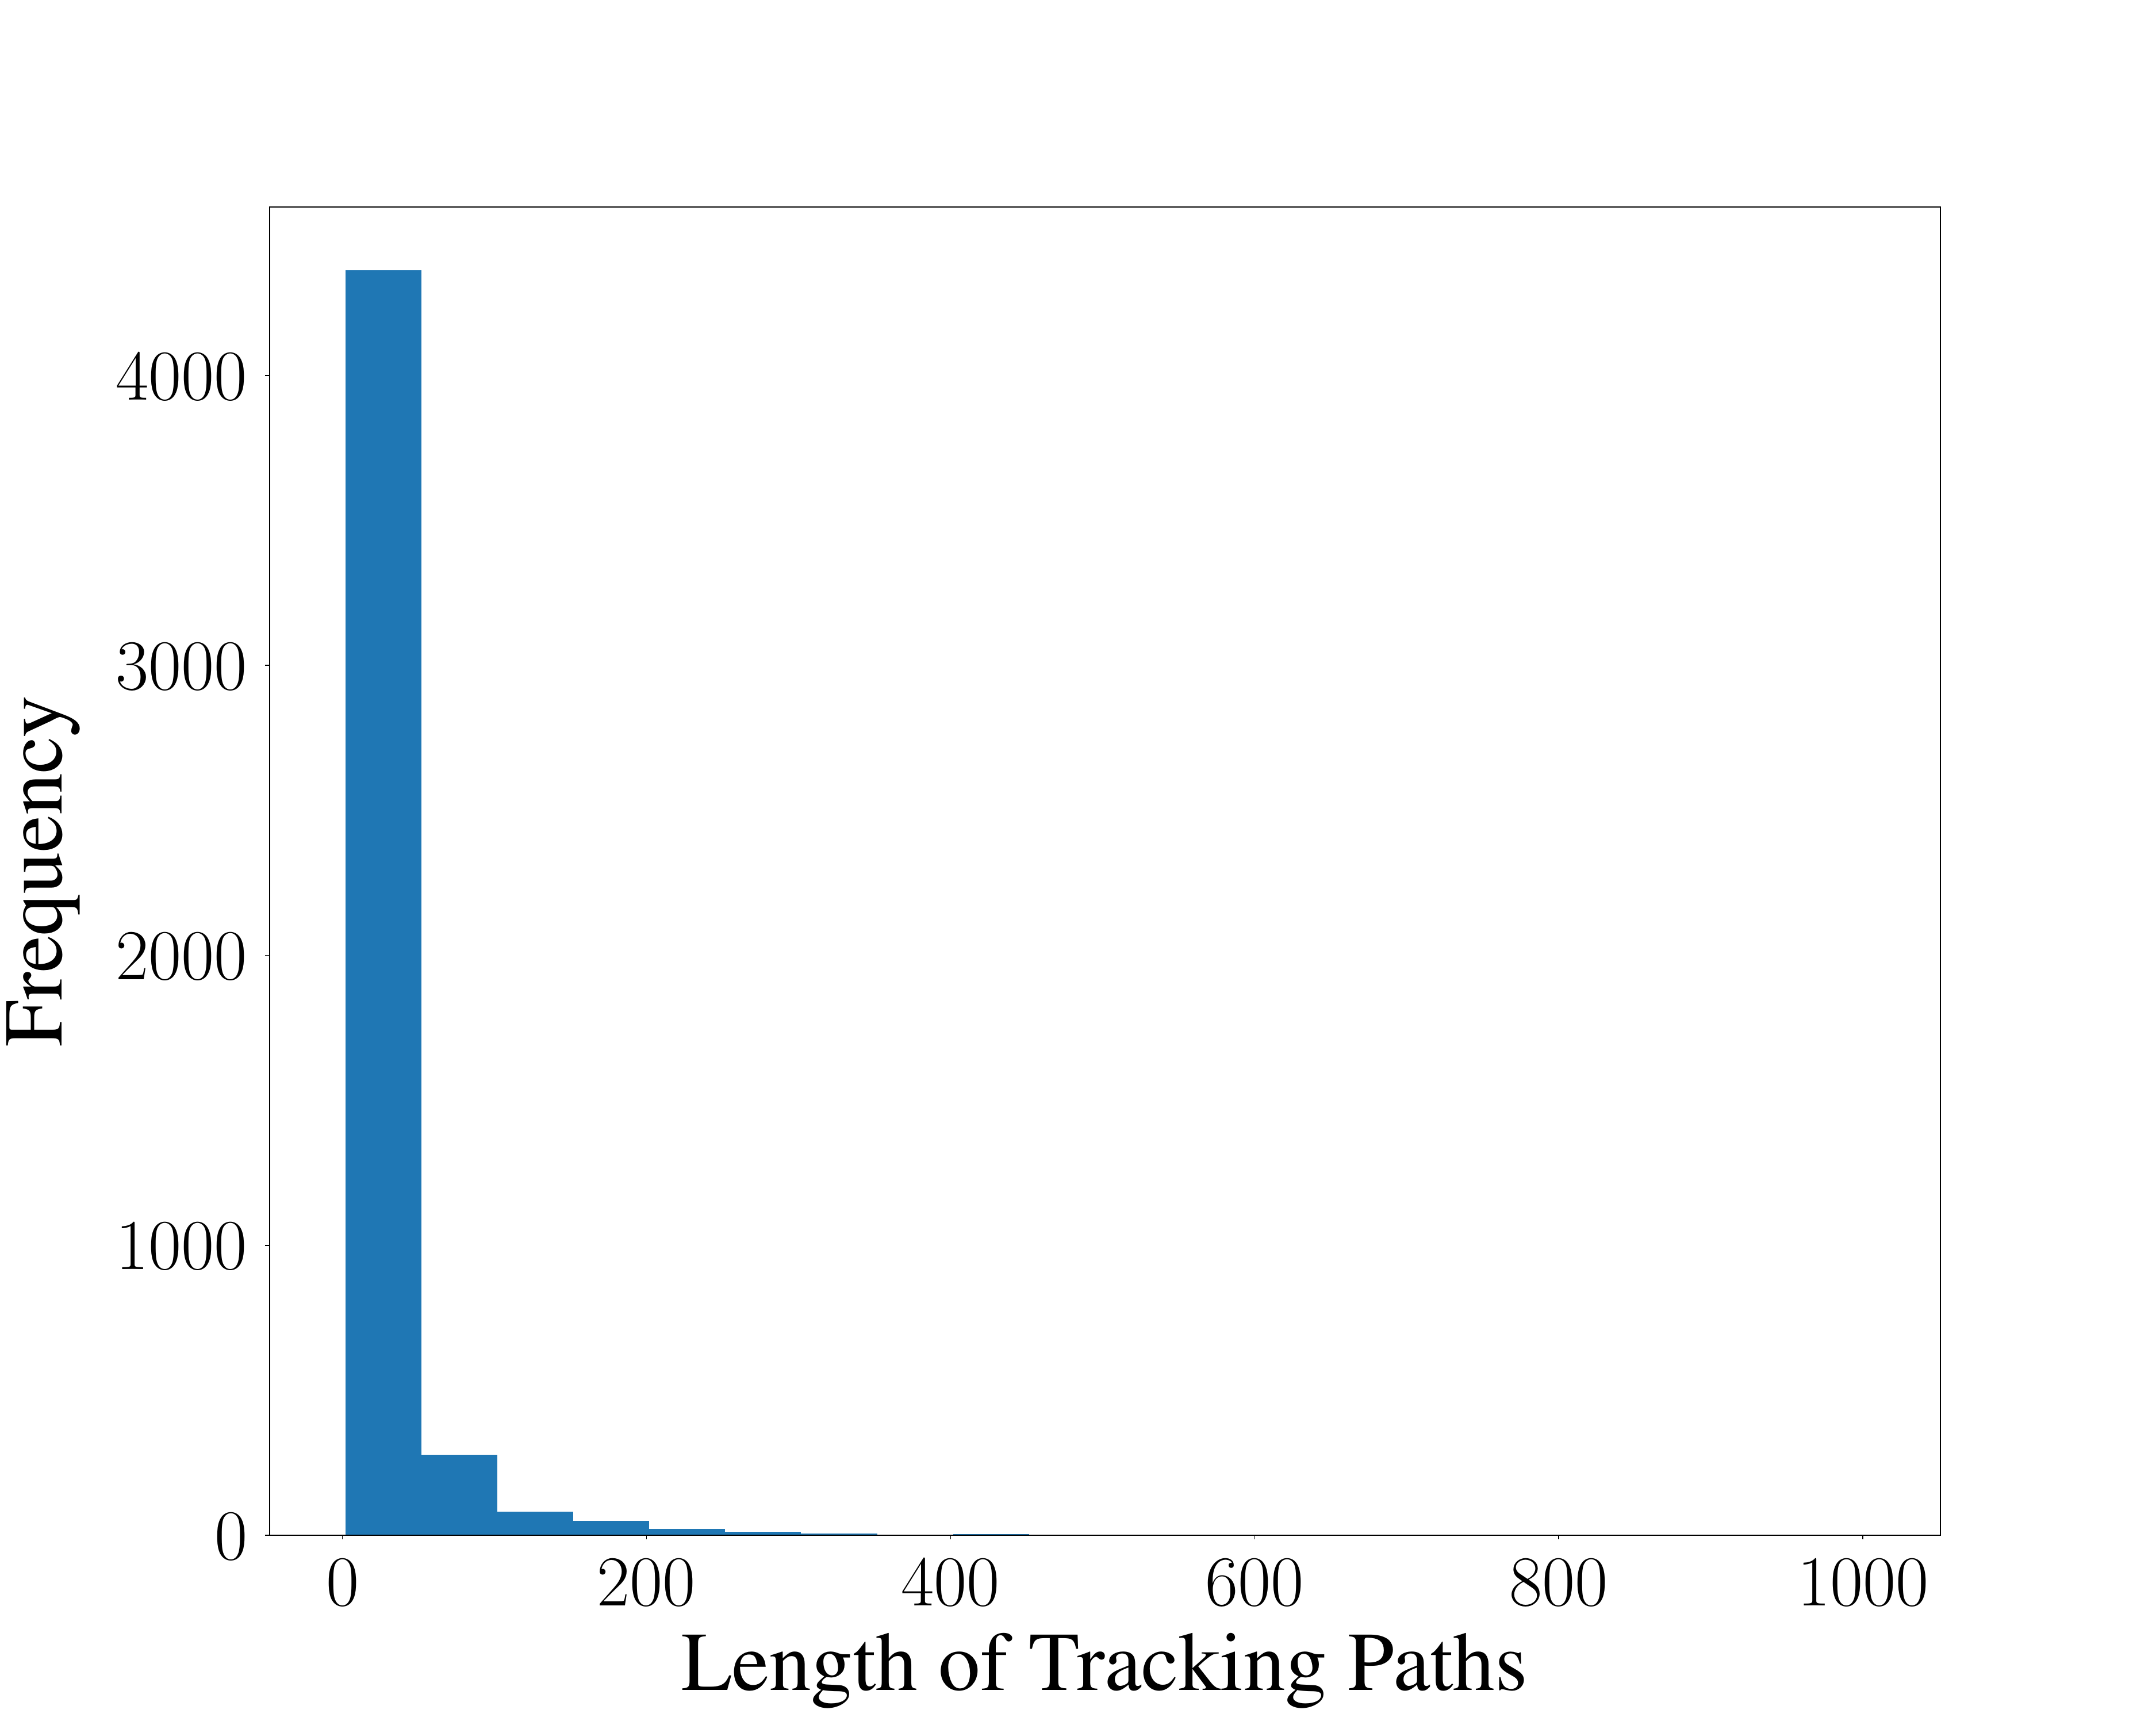}%
\caption{$d_e$.}%
\label{fig-LengthHistogramBoussinesq2DE}%
\end{subfigure}%
\\%
\begin{subfigure}[t]{\ltwopicwidth}%
\includegraphics[width=\ltwopicwidth]{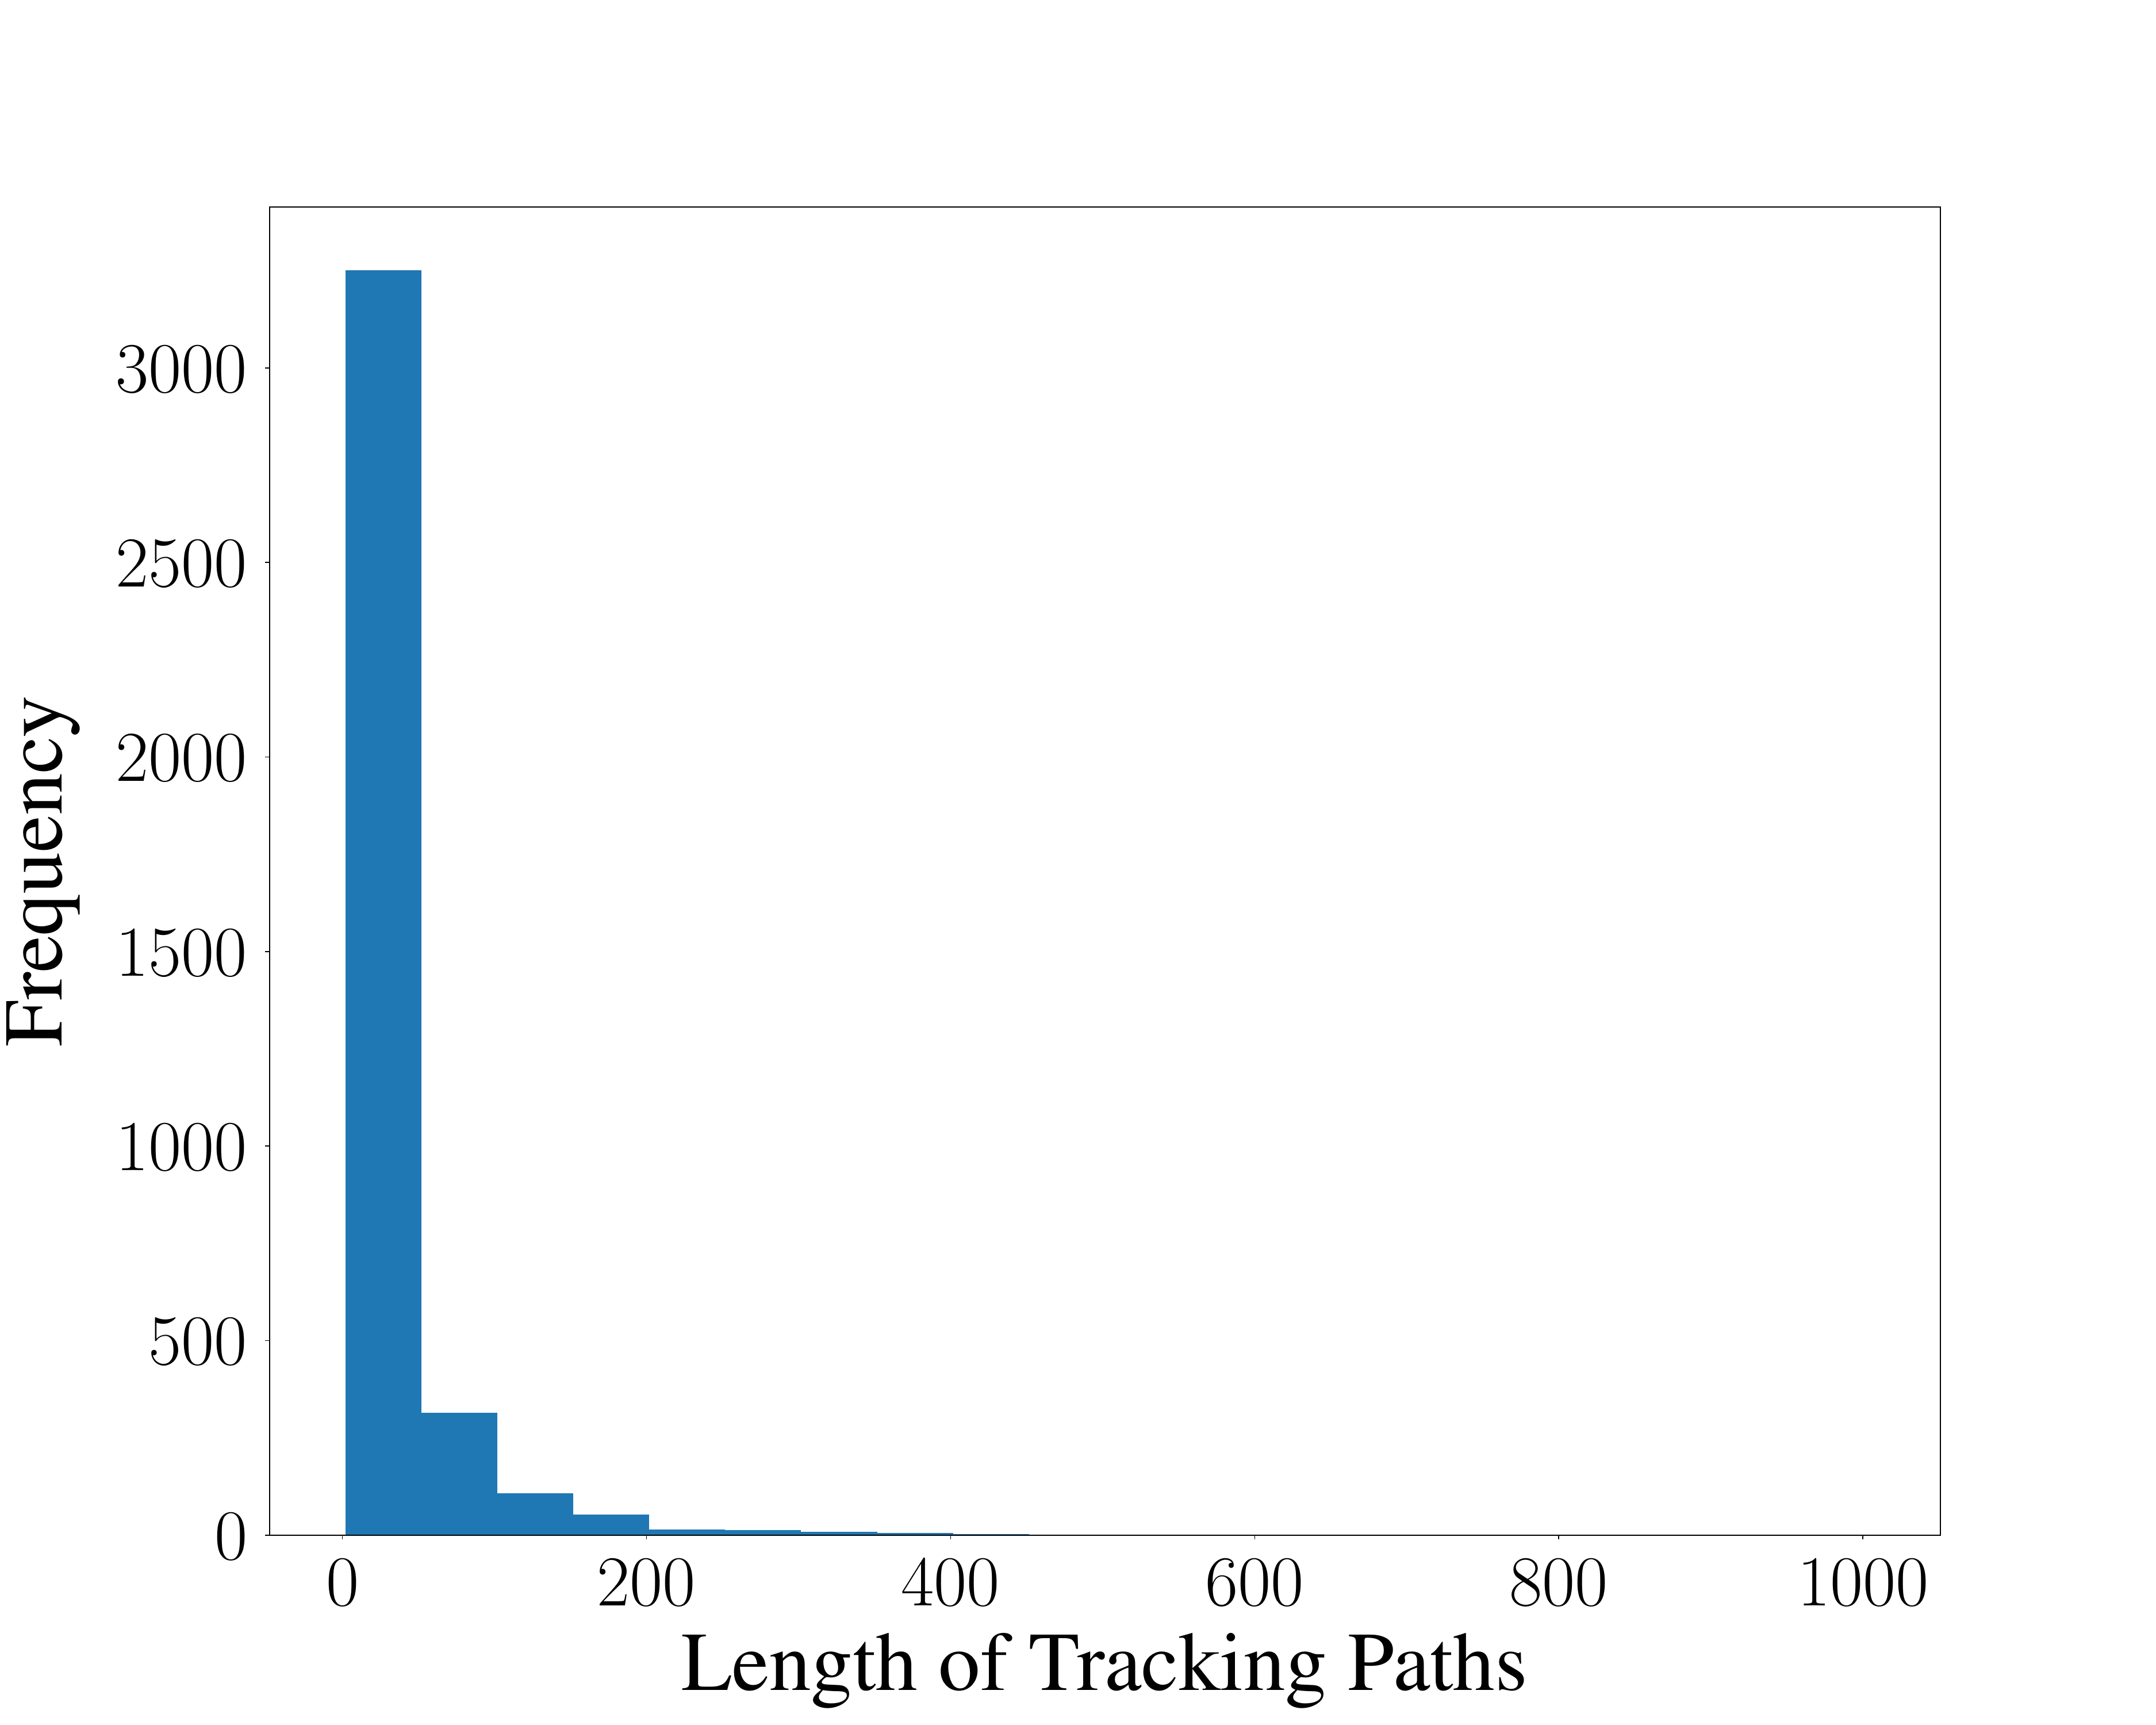}%
\caption{$d_b$.}%
\label{fig-LengthHistogramBoussinesq2DB}%
\end{subfigure}%
\hfill%
\begin{subfigure}[t]{\ltwopicwidth}%
\includegraphics[width=\ltwopicwidth]{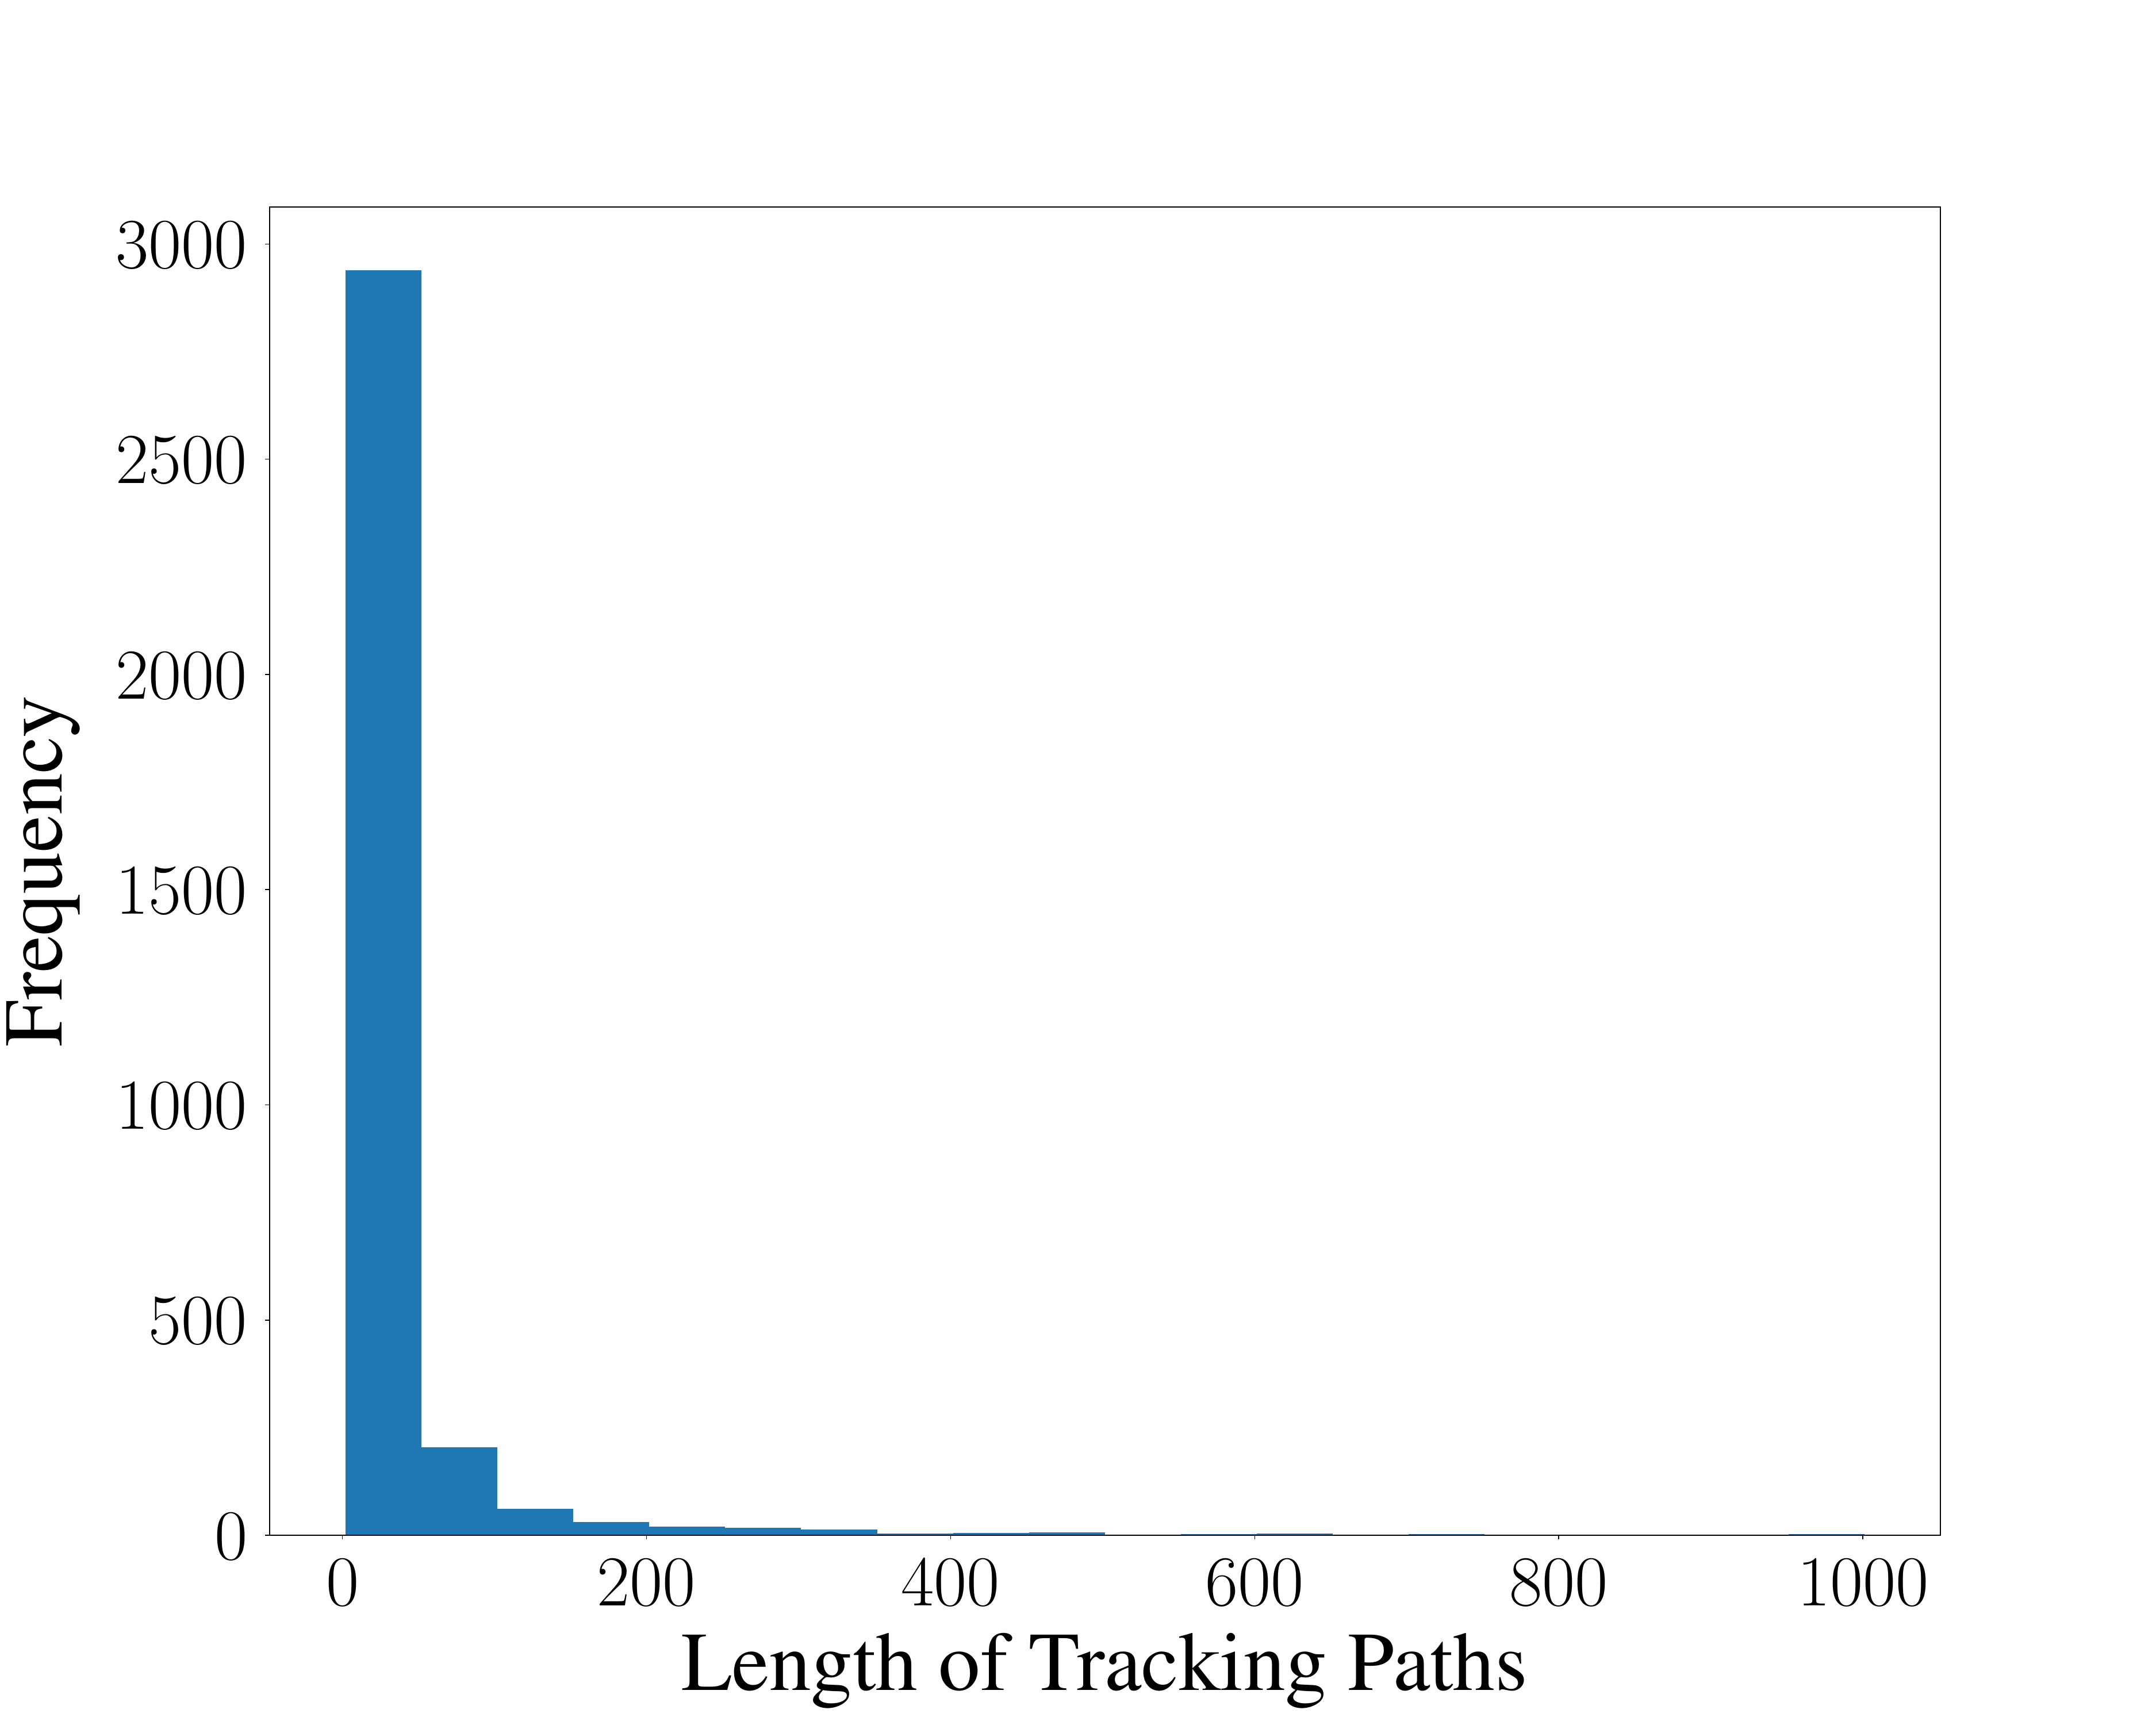}%
\caption{$d_p$.}%
\label{fig-LengthHistogramBoussinesq2DP}%
\end{subfigure}%
\caption{Histograms of the length of the tracking paths 
    using the last $1000$ time steps
    of \dataset{Boussinesq2D}.}%
\label{fig-LengthHisgoramBoussinesq2D}%
\end{figure}

\begin{figure}
\centering
\includegraphics[width=0.8\linewidth]{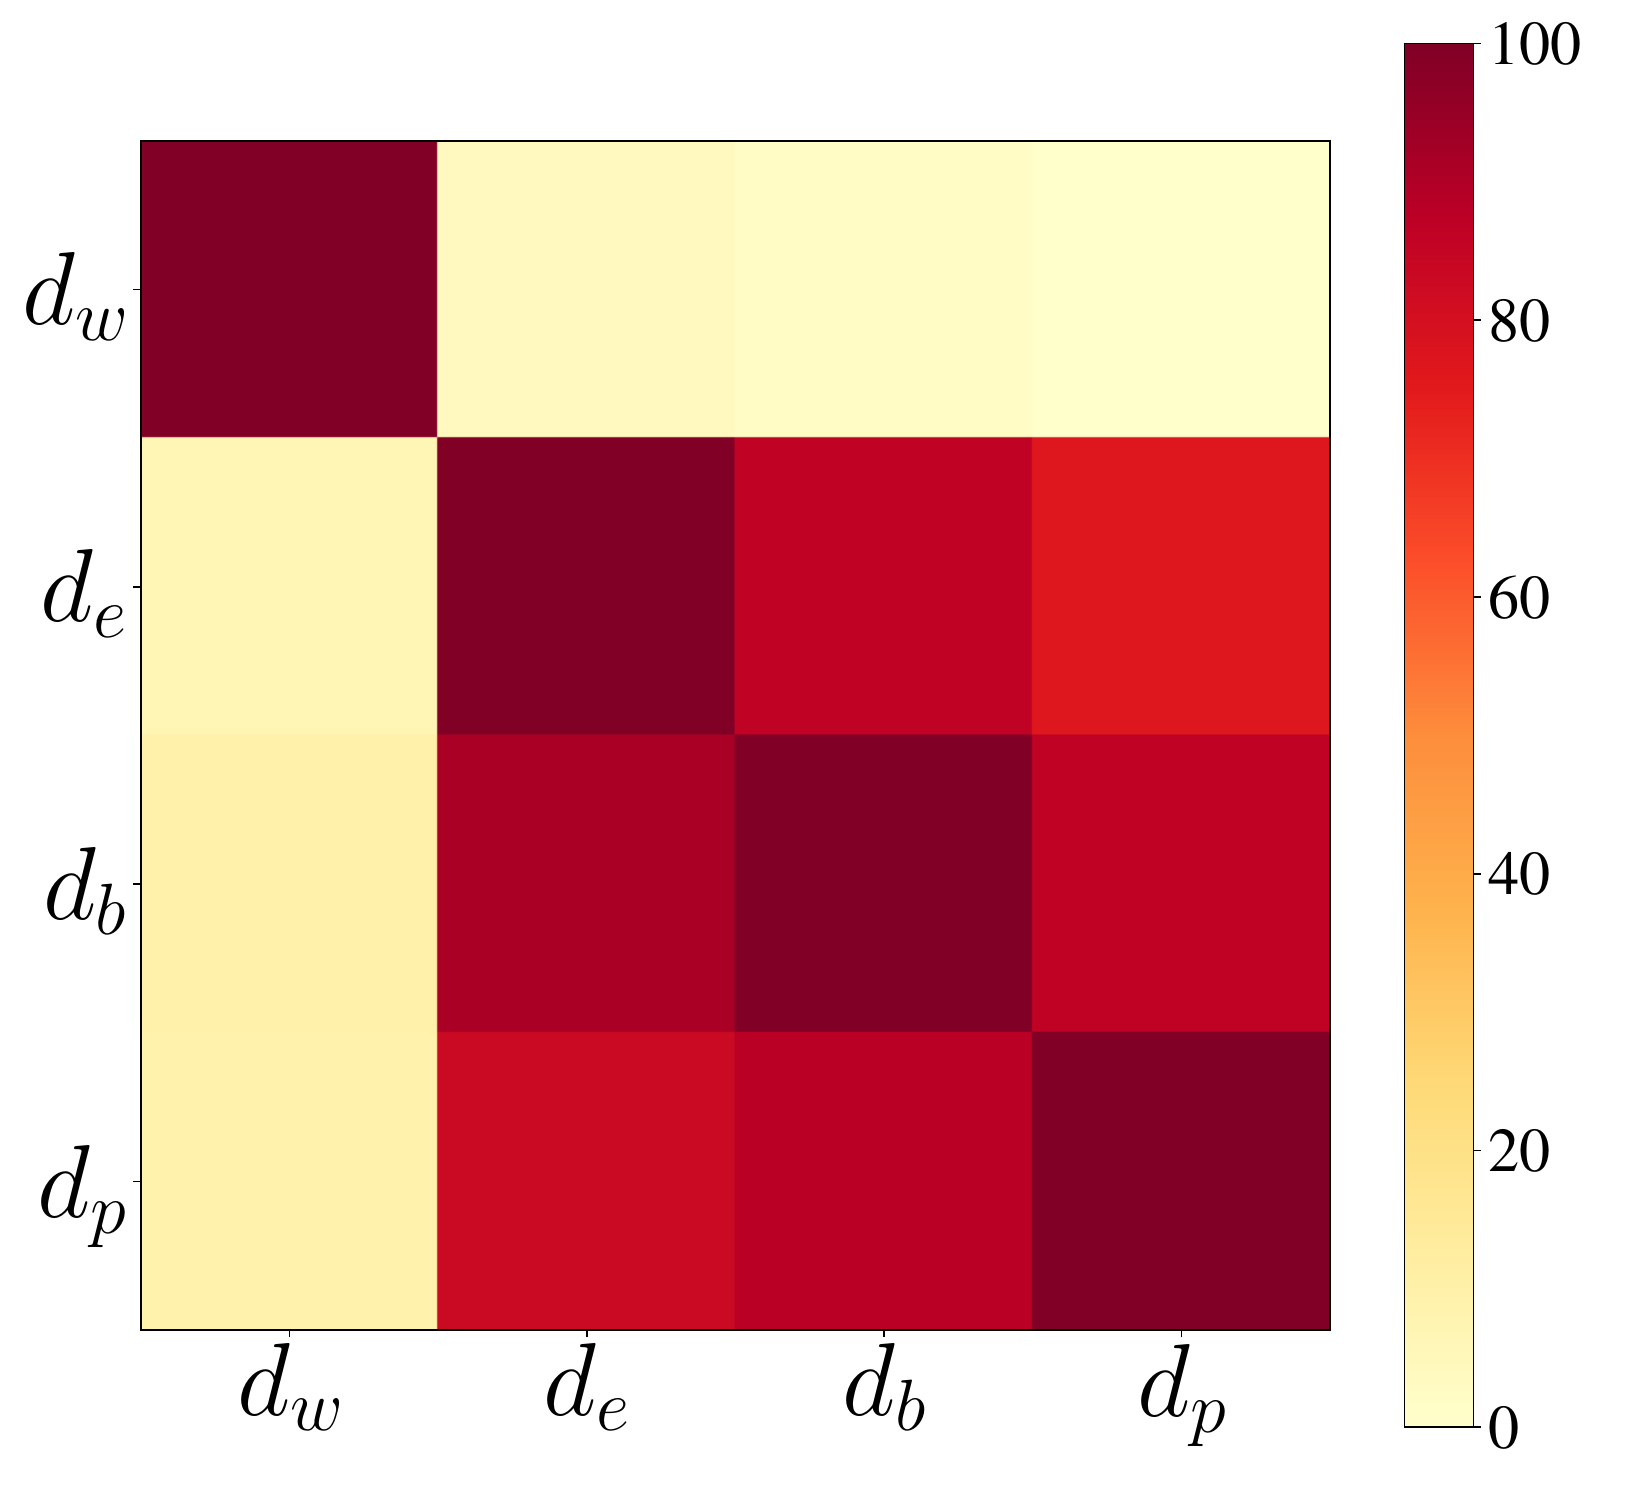}
\caption{
    Pairwise differences between the methods on the columns
    in relation to the methods on the rows
    for \dataset{Boussinesq2D}.
}
\label{fig-Boussinesq2DSimilarities}
\end{figure}

\subsection*{Results using Cylinder3D}
The results of the experiments using \dataset{Cylinder3D}
are shown from \Cref{fig-Cylinder3DAllNodes}
to \Cref{fig-Cylinder3DSimilarities}.

\begin{figure}
\centering
\includegraphics[width=0.8\linewidth]{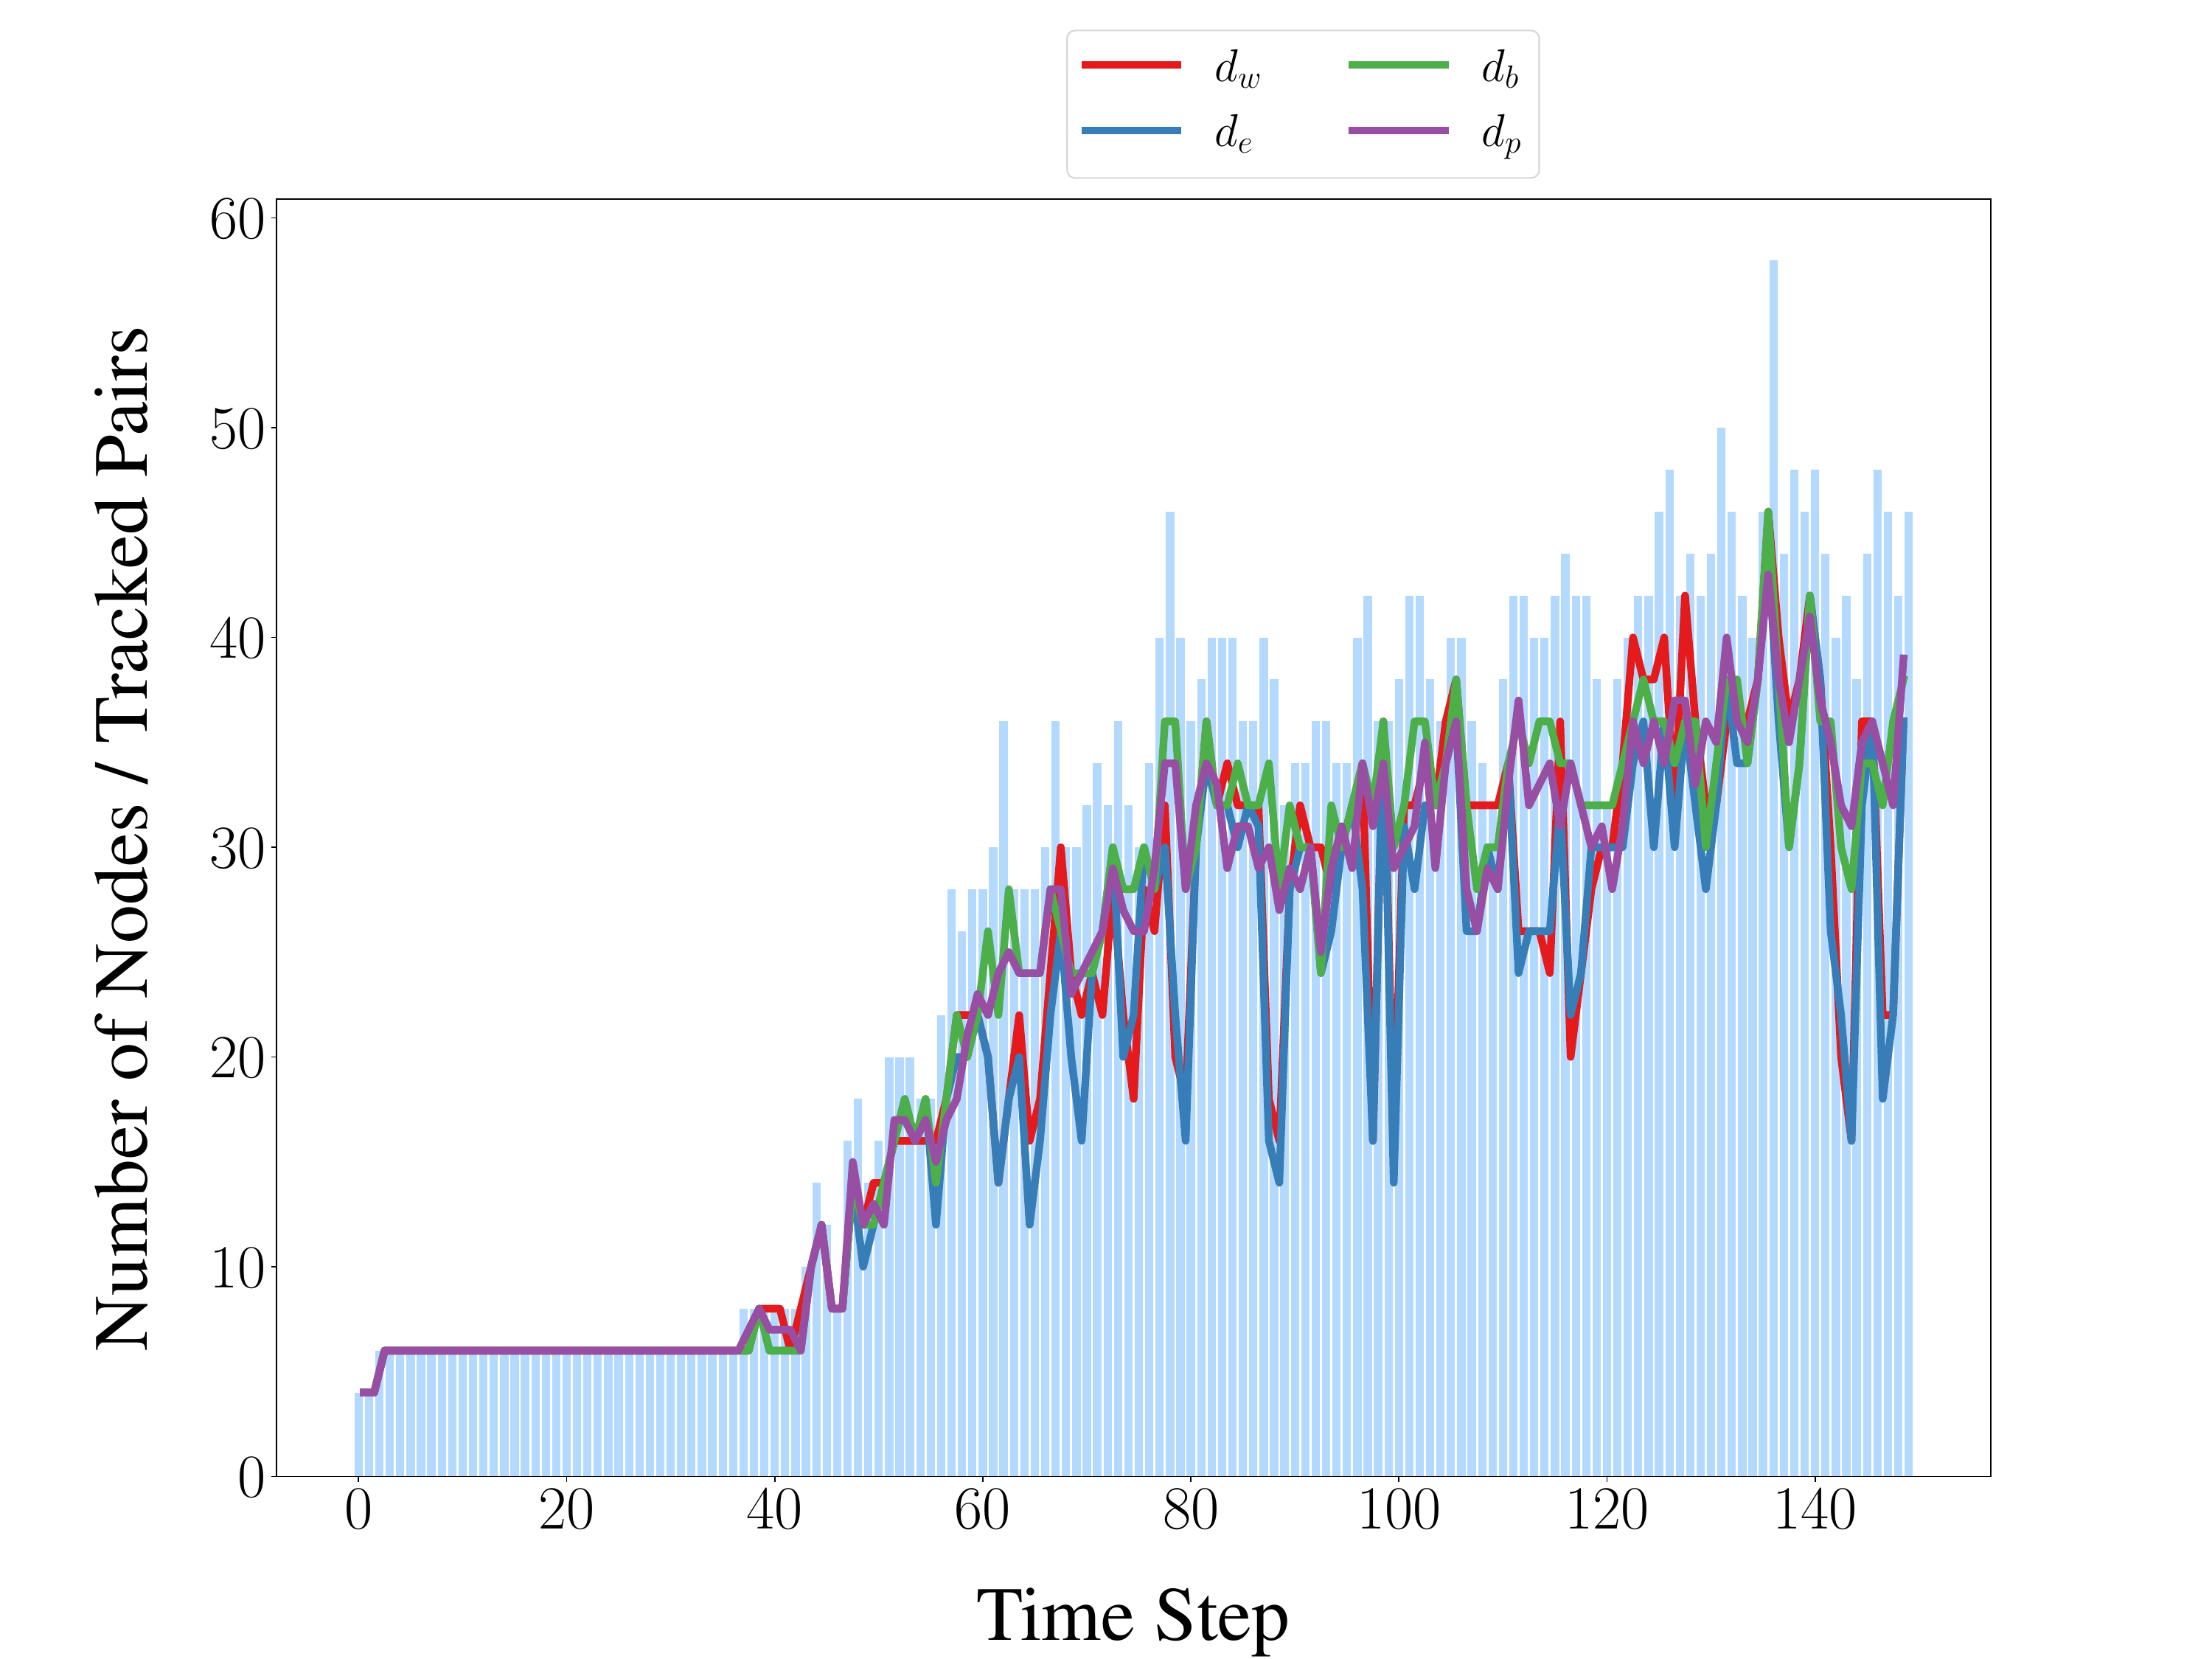}
\caption{
    Number of tracked nodes (colored and labeled) 
    relative to the total nodes of merge trees (light blue bars)
    for \dataset{Cylinder3D}.
}
\label{fig-Cylinder3DAllNodes}
\end{figure}

\begin{figure}
\centering
\includegraphics[width=0.8\linewidth]{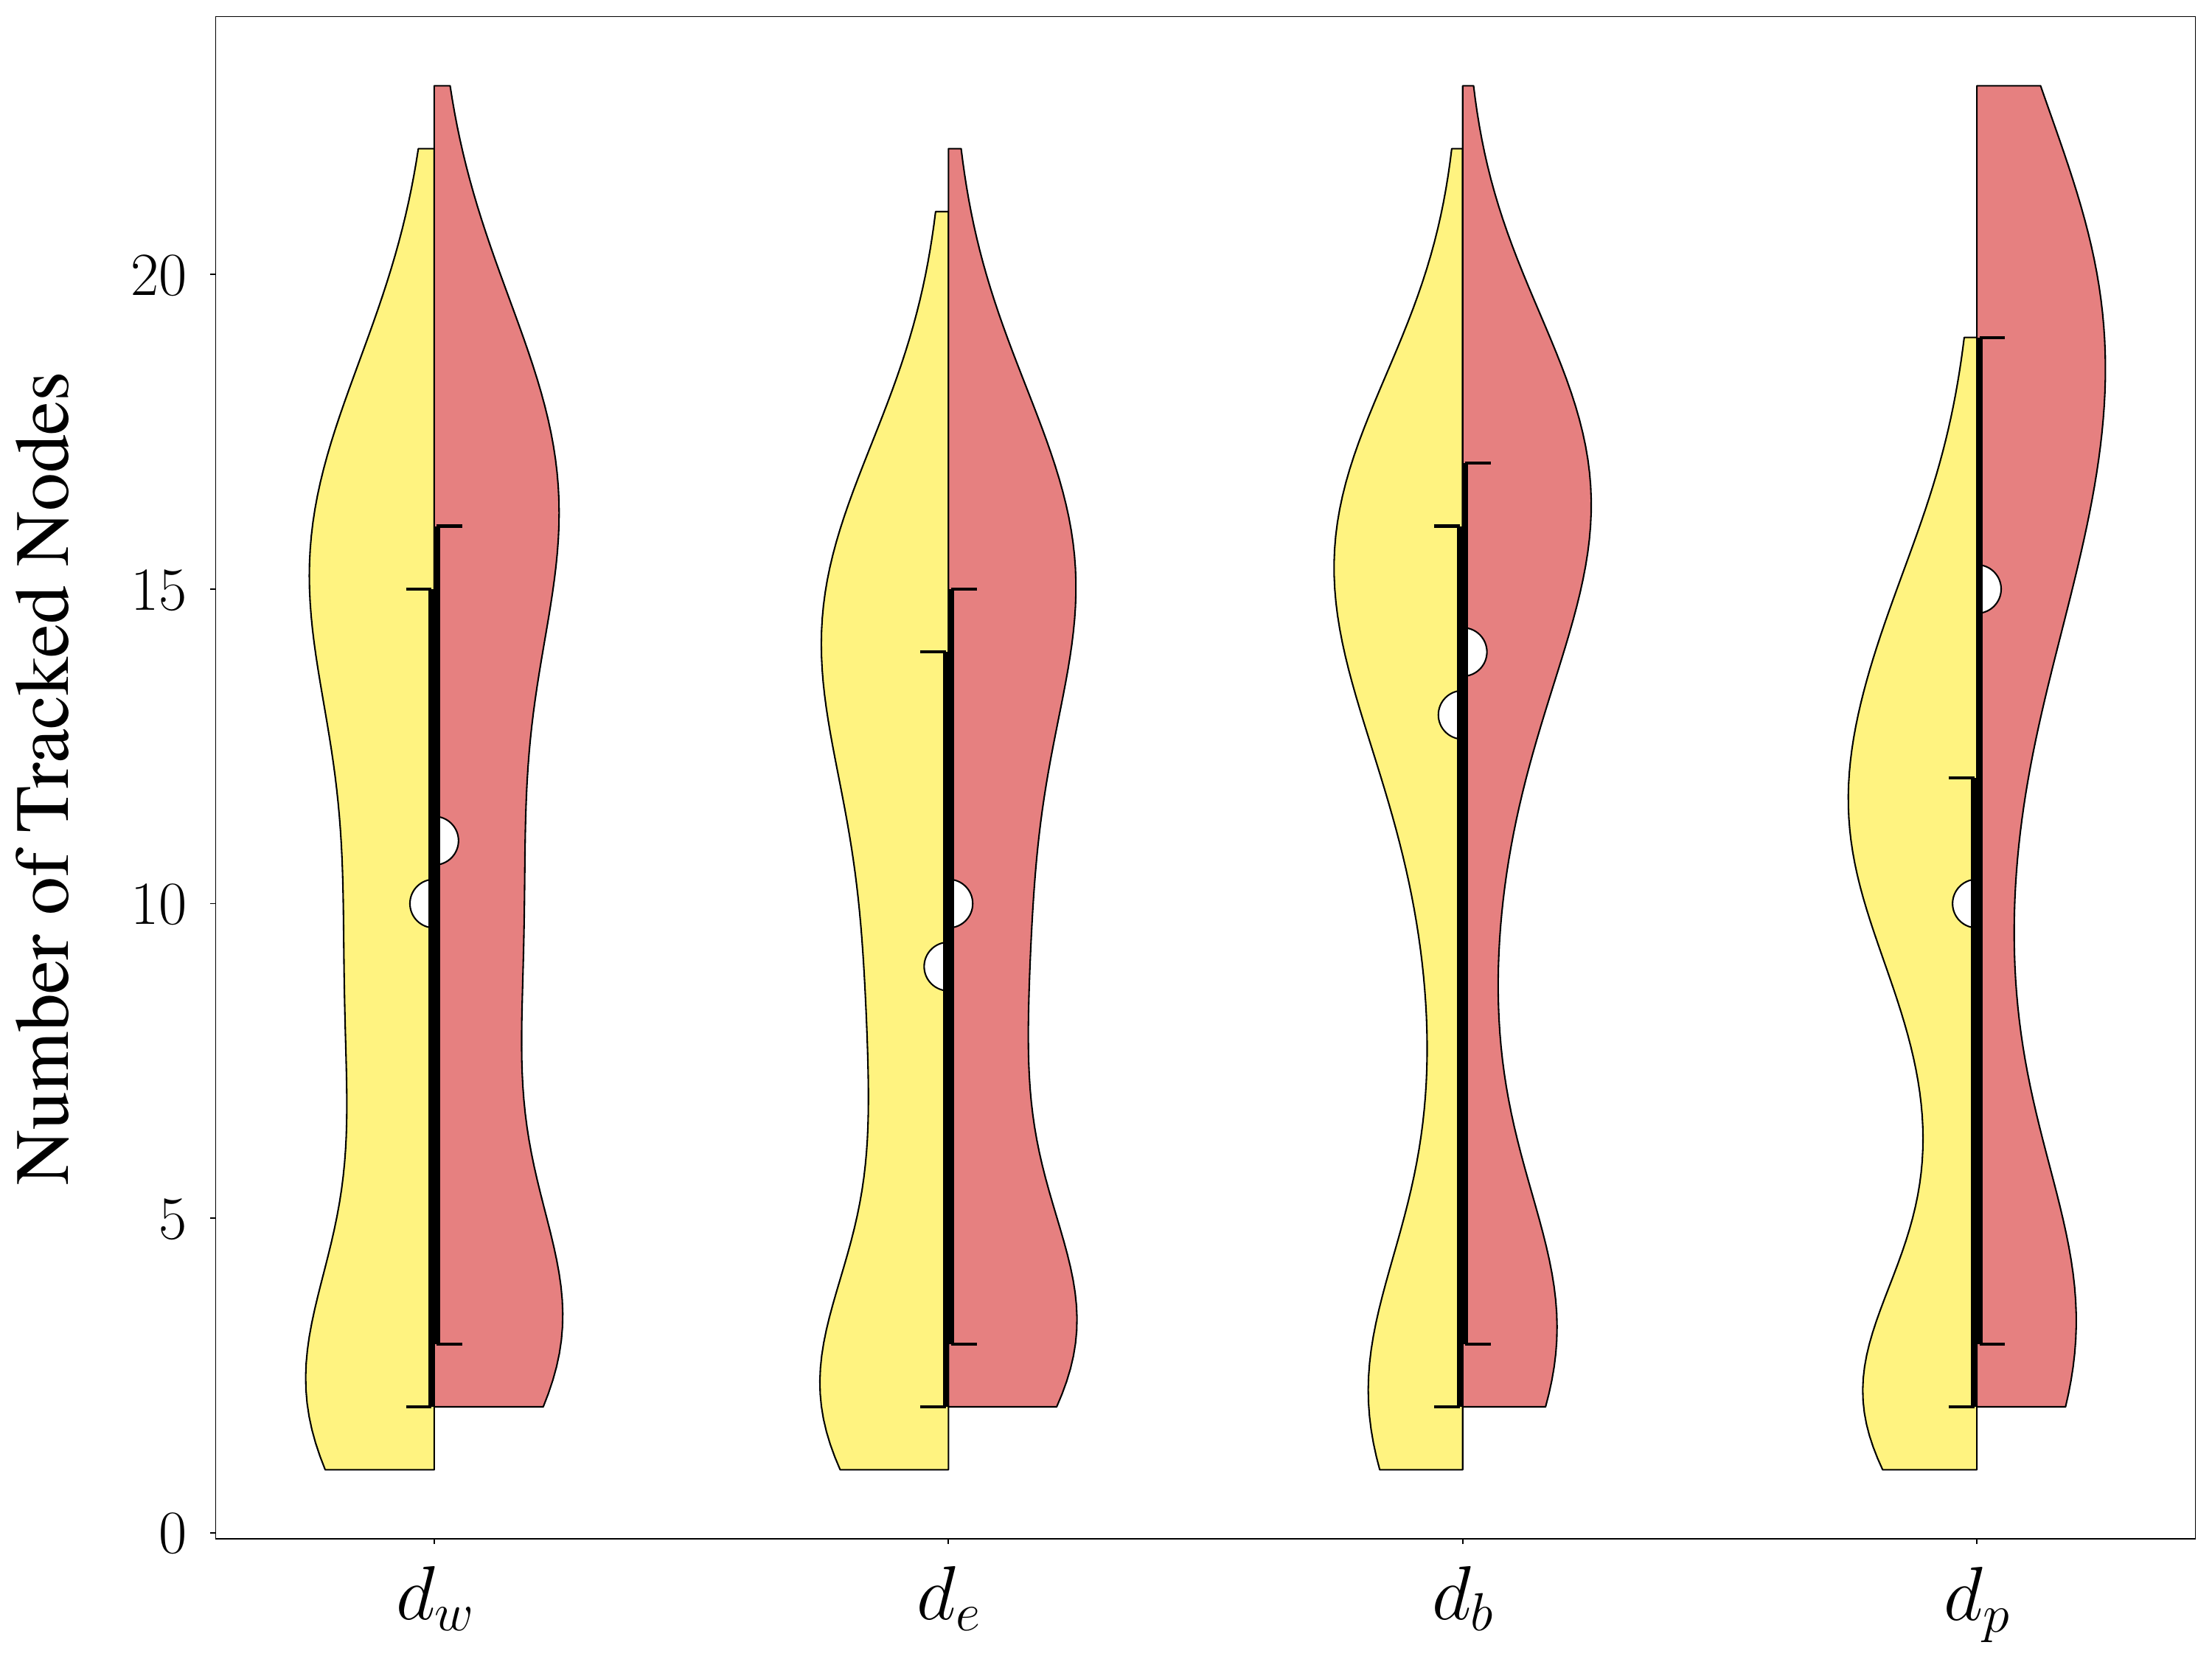}
\caption{
    Distributions of tracked nodes 
    of \dataset{Cylinder3D},  
    divided by types:
    saddle (yellow) and minima (blue).
}
\label{fig-Cylinder3DViolin}
\end{figure}

% Length histogram
\begin{figure}%
\begin{subfigure}[t]{\ltwopicwidth}%
\includegraphics[width=\ltwopicwidth]{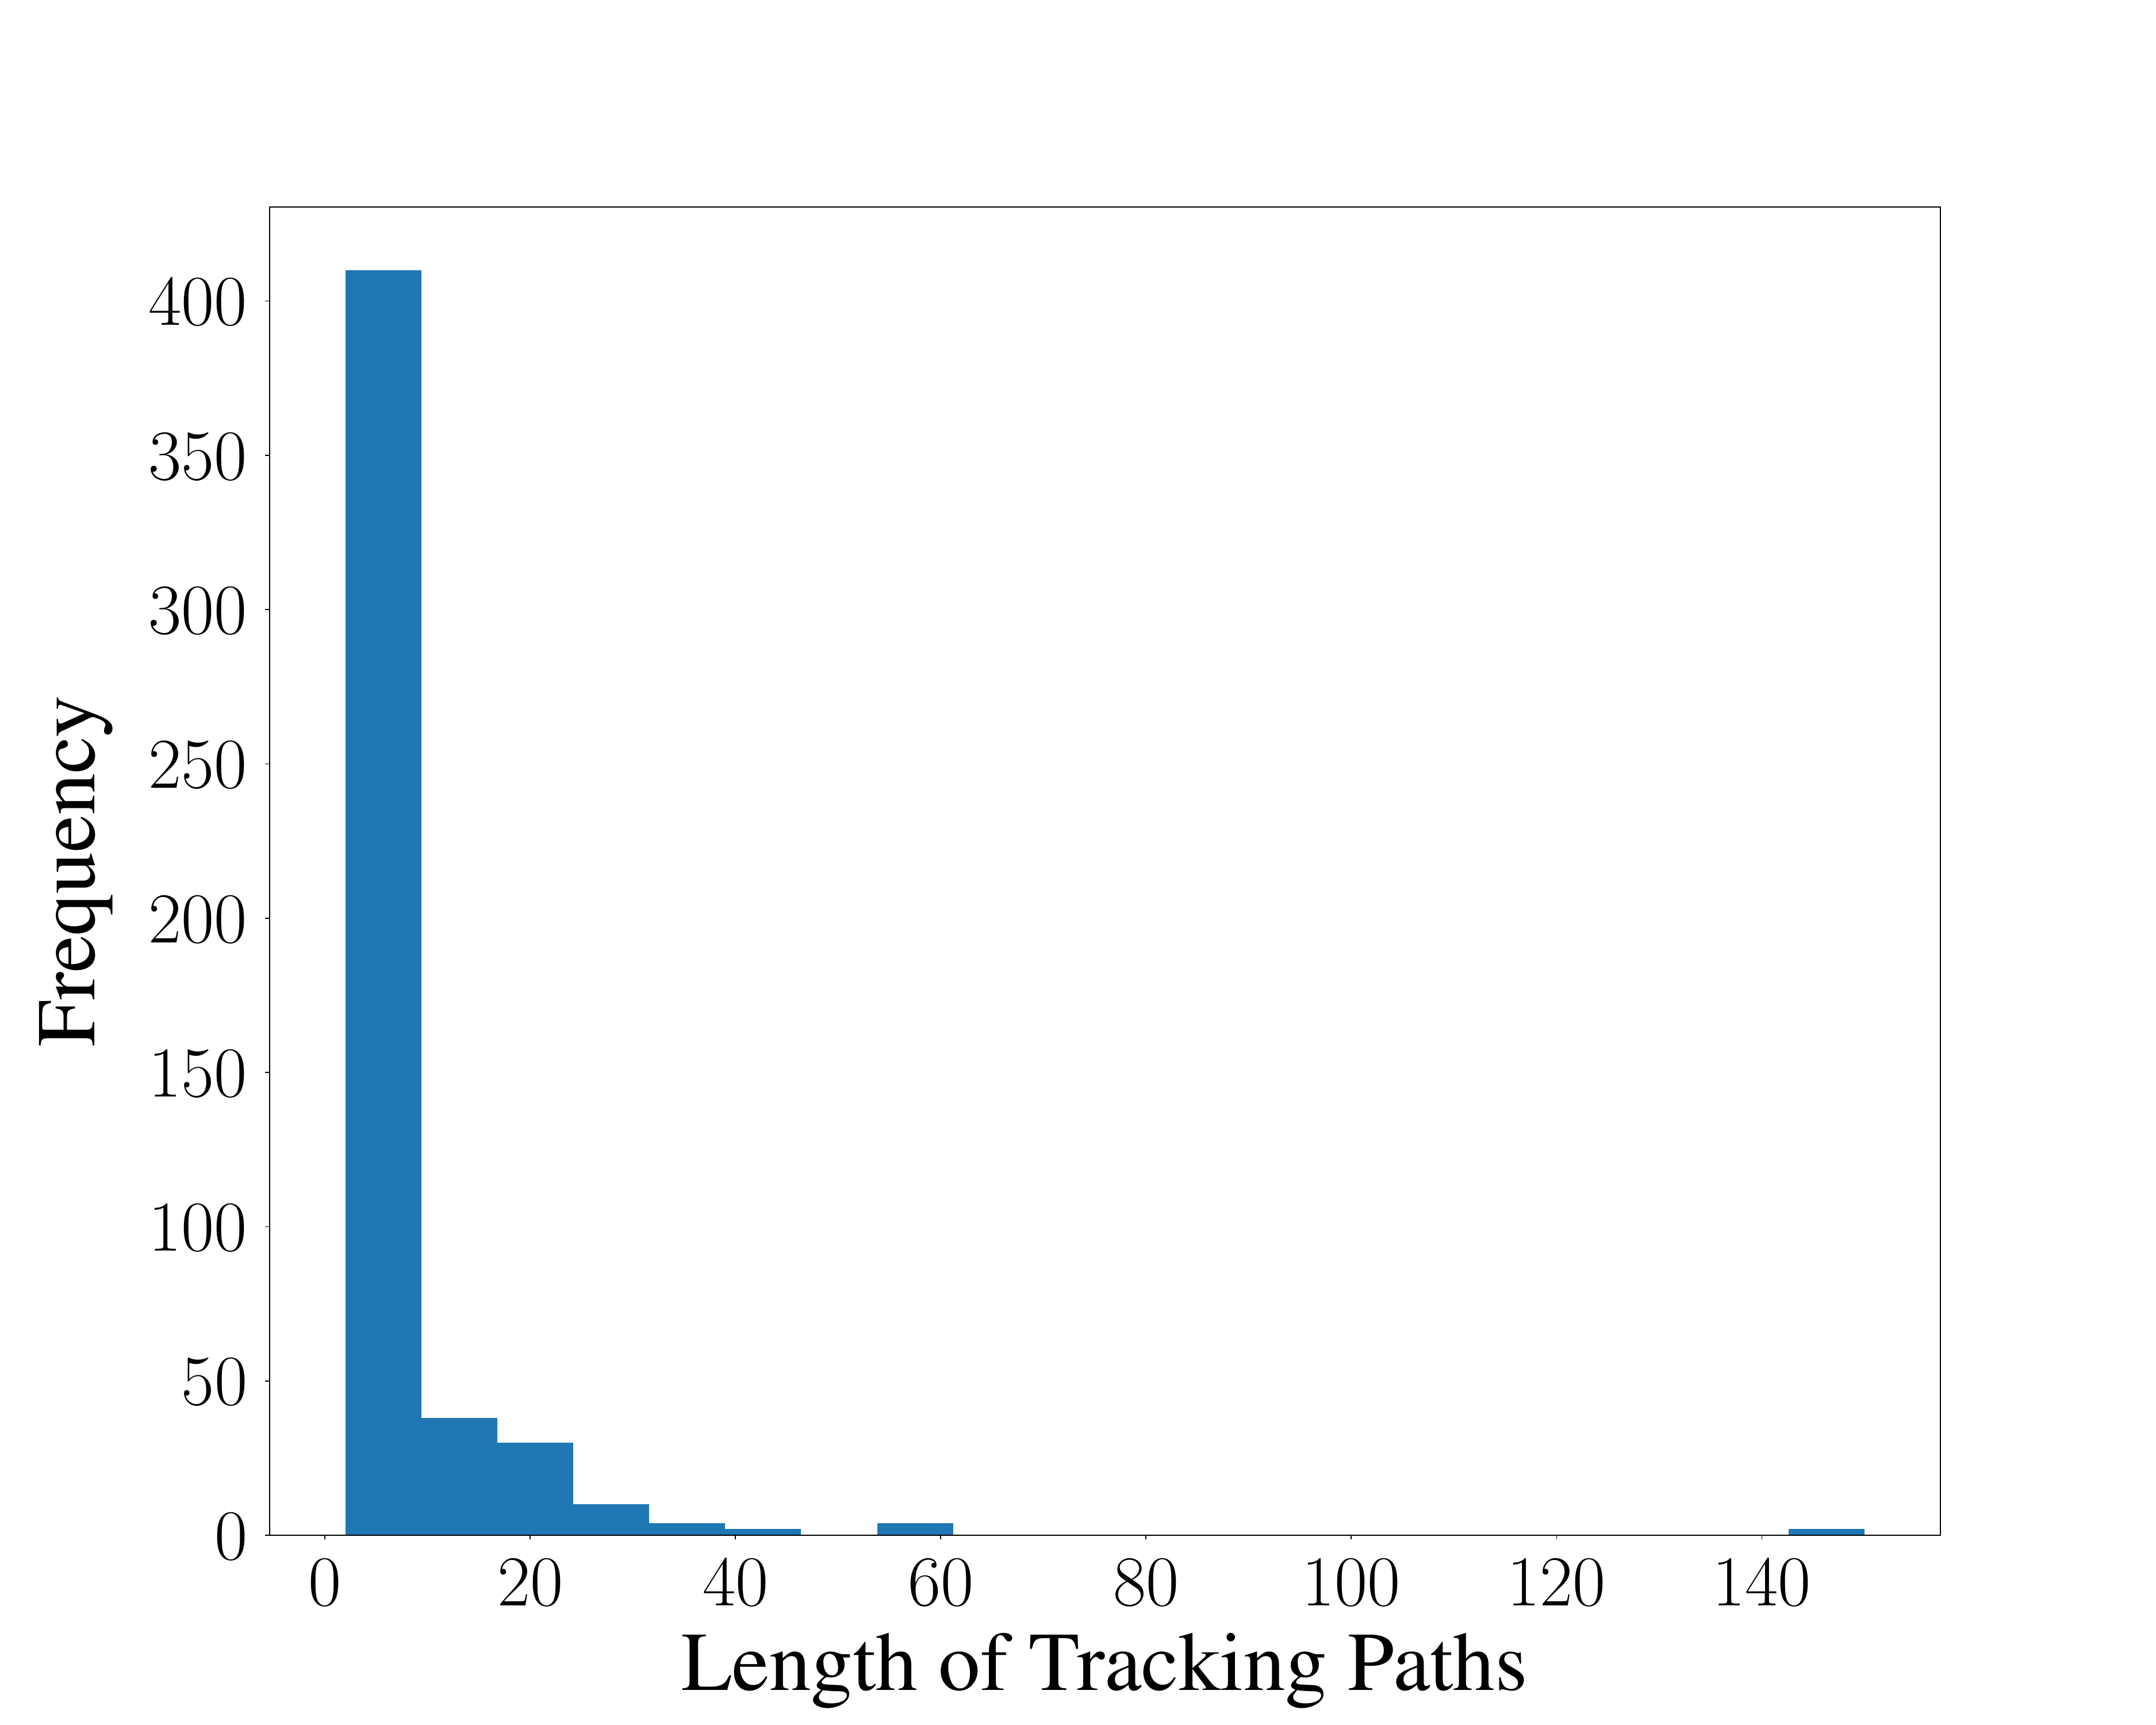}
\caption{$d_w$.}%
\label{fig-LengthHistogramCylinder3DW}%
\end{subfigure}
\hfill%
\begin{subfigure}[t]{\ltwopicwidth}%
\includegraphics[width=\ltwopicwidth]{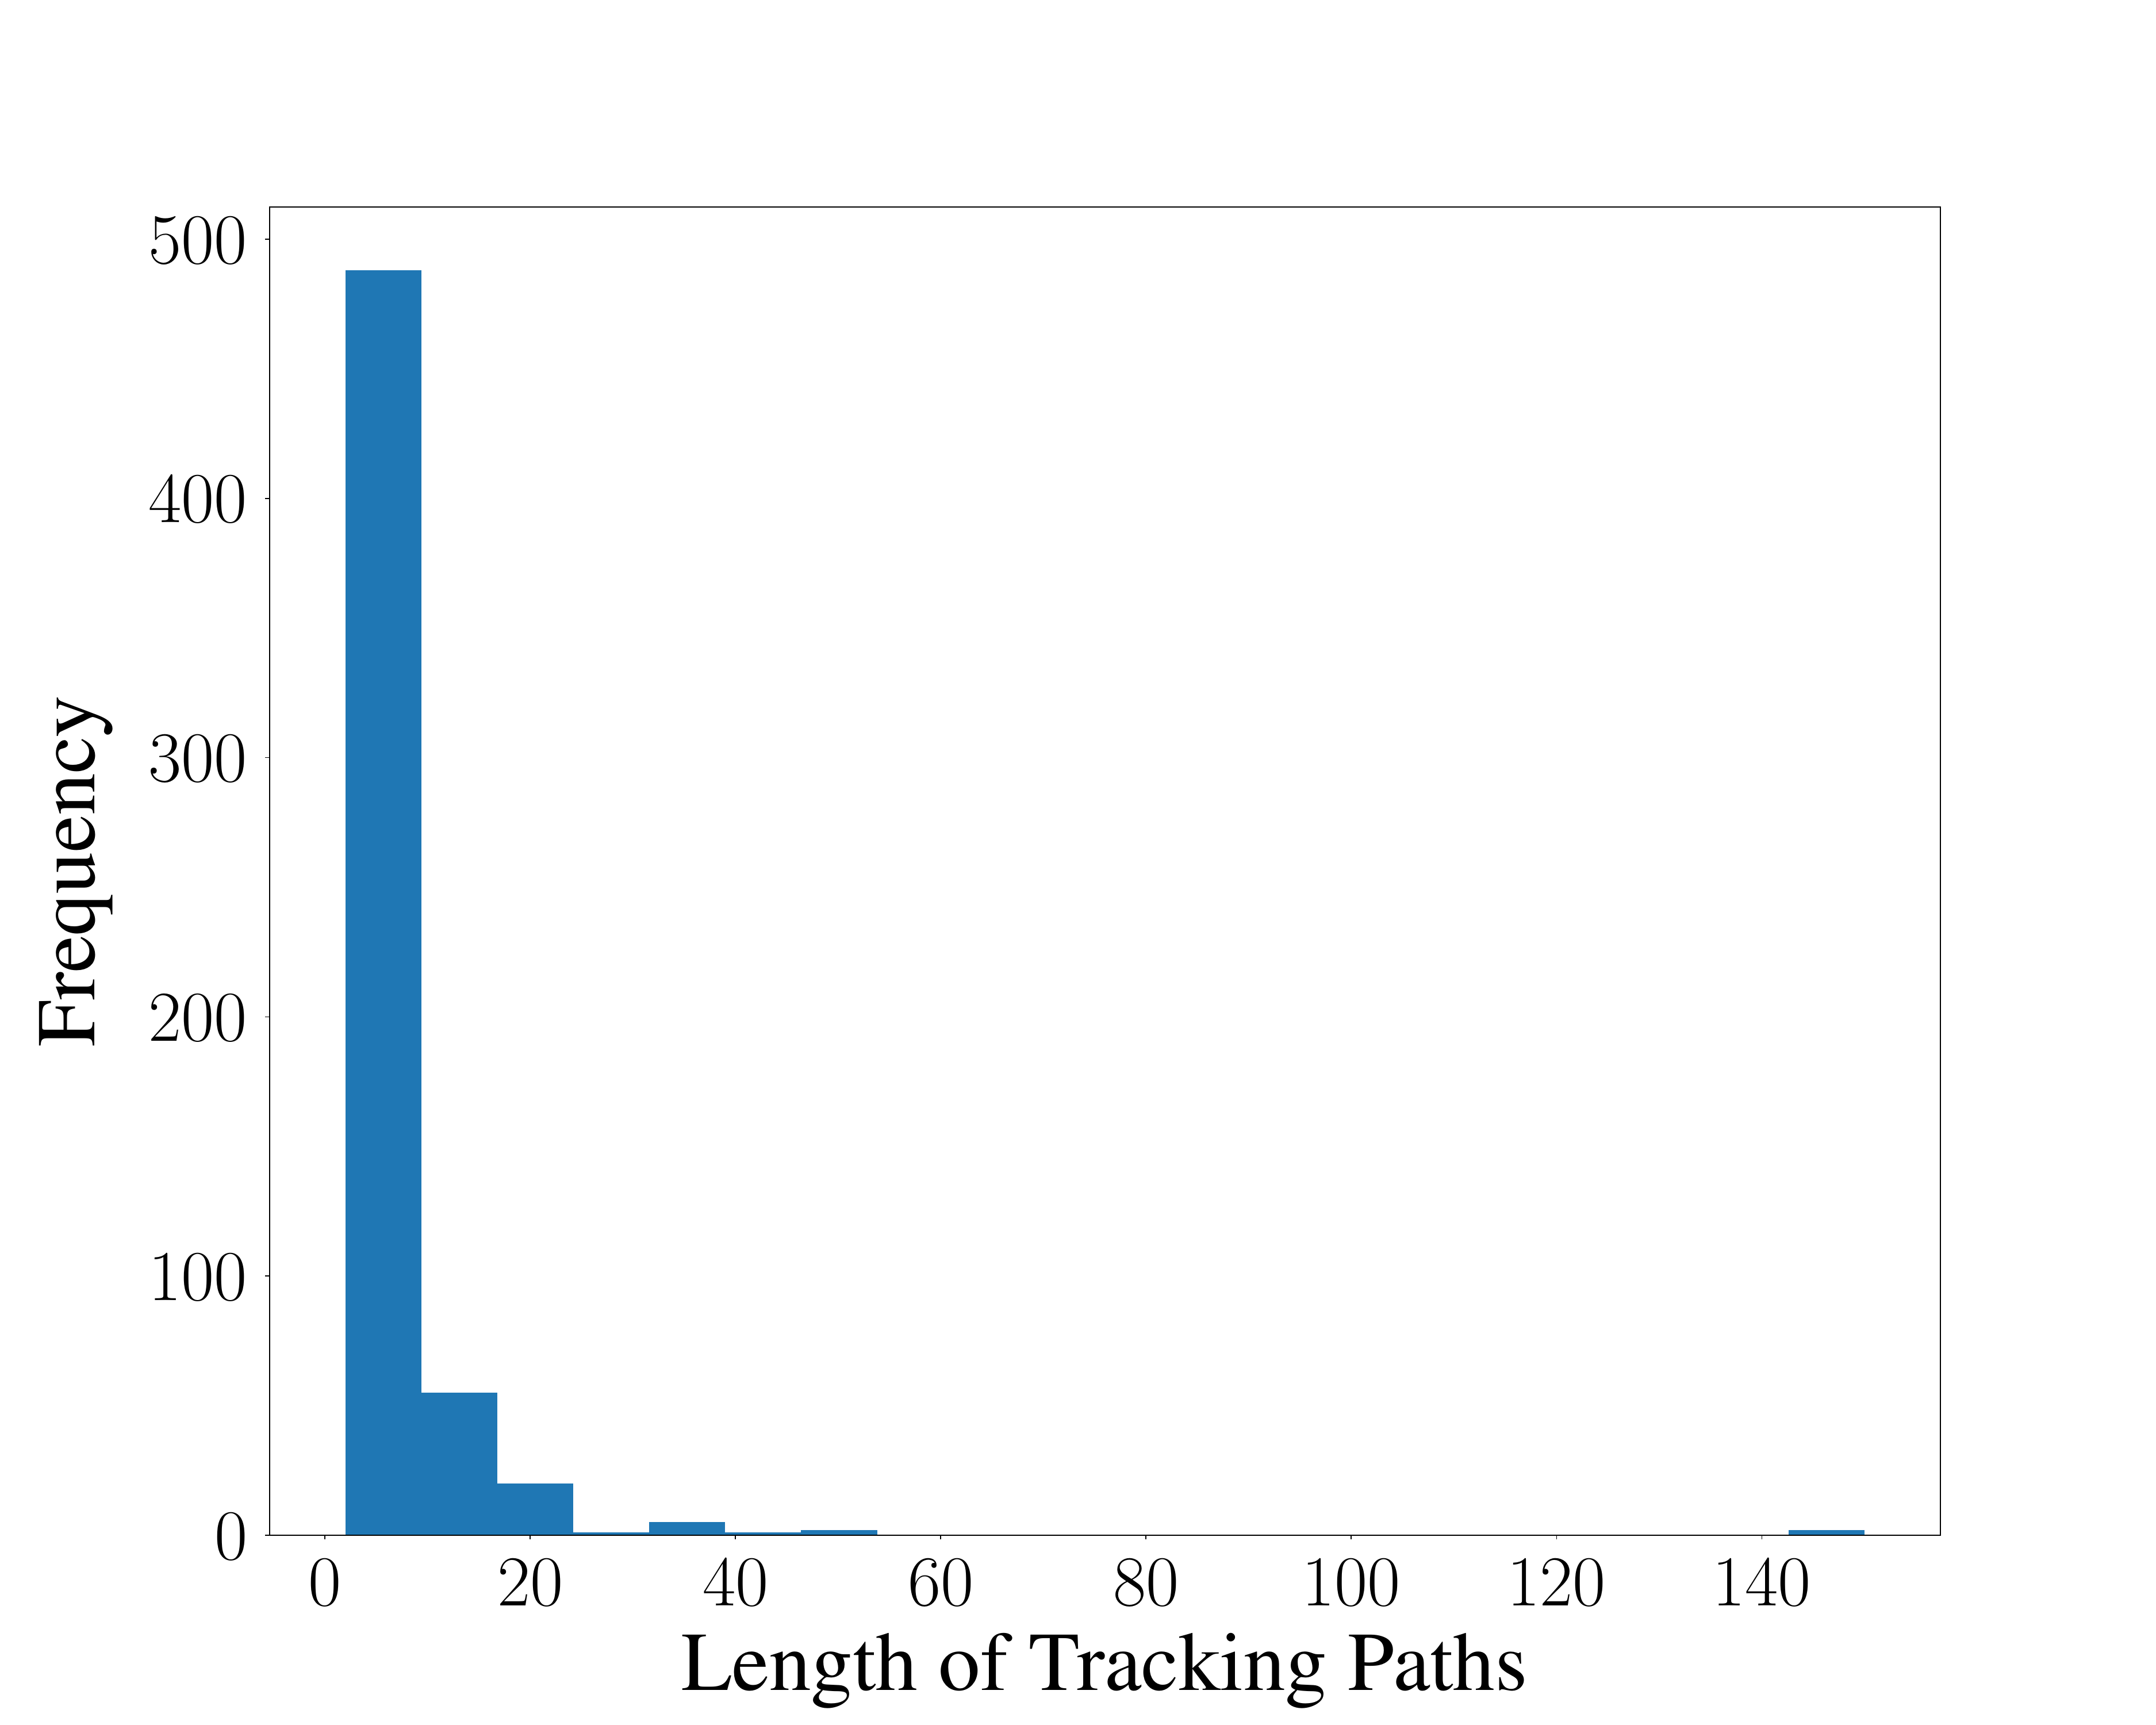}%
\caption{$d_e$.}%
\label{fig-LengthHistogramCylinder3DE}%
\end{subfigure}%
\\%
\begin{subfigure}[t]{\ltwopicwidth}%
\includegraphics[width=\ltwopicwidth]{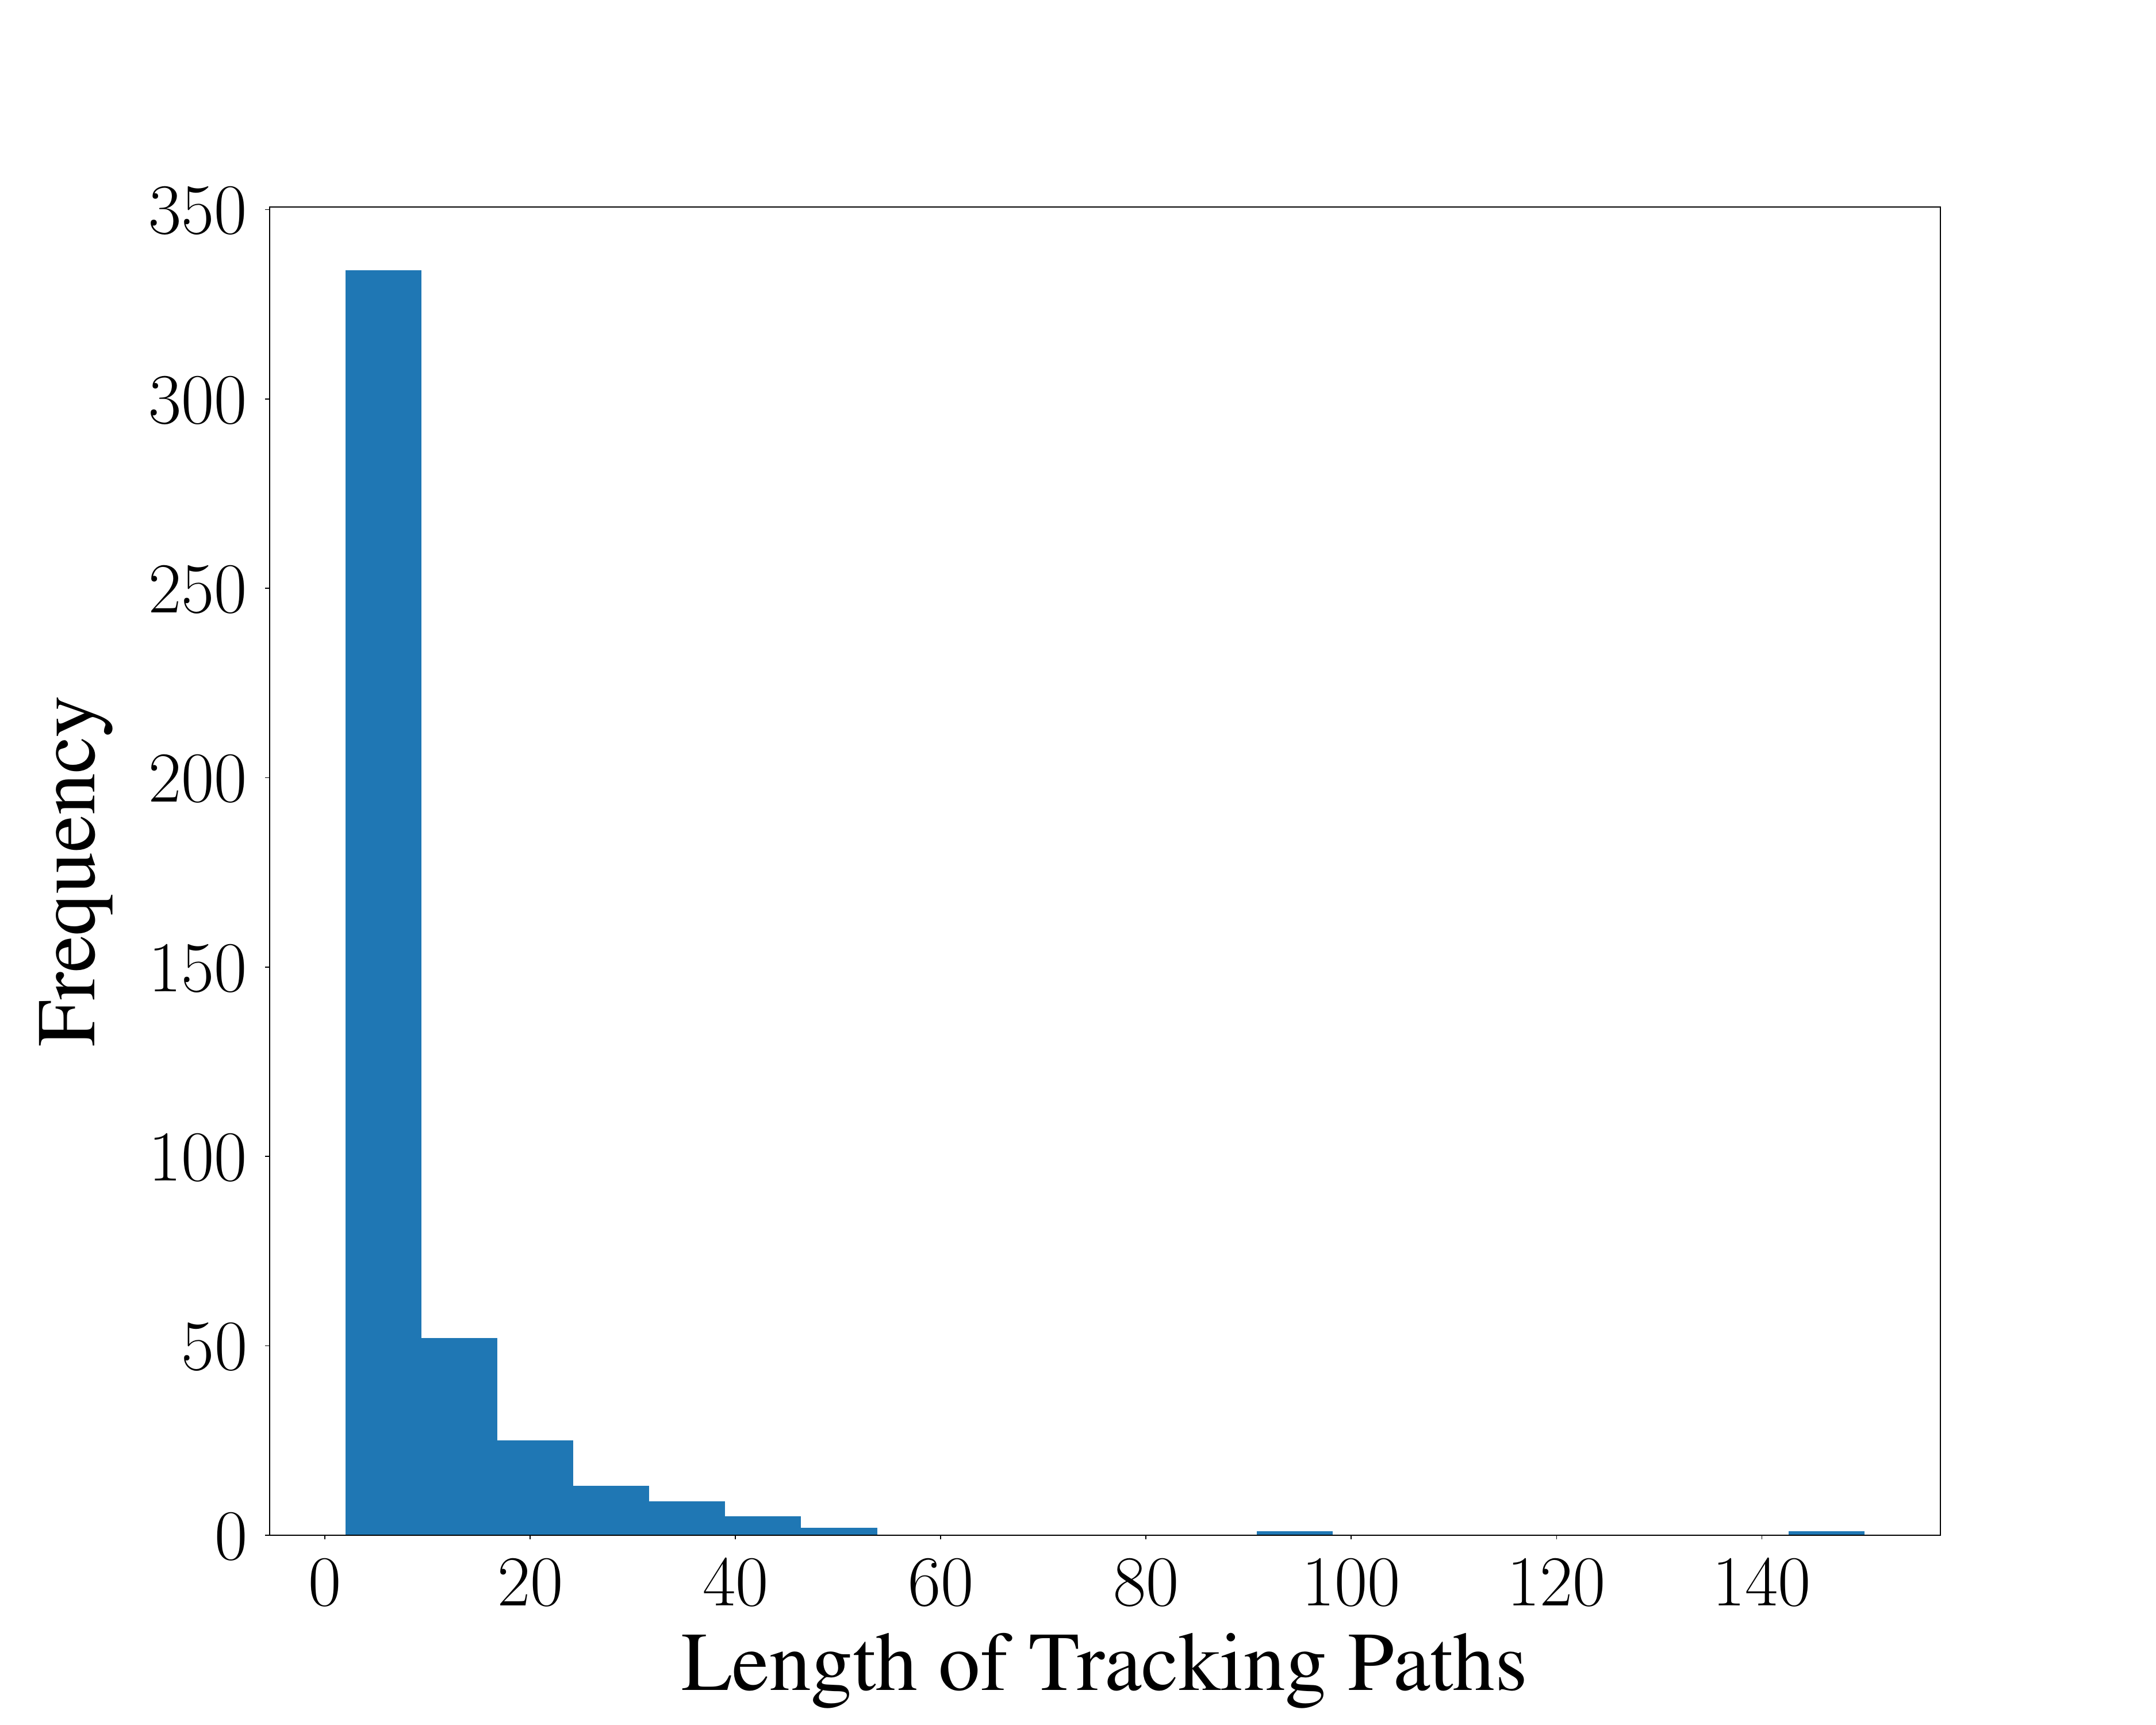}%
\caption{$d_b$.}%
\label{fig-LengthHistogramCylinder3DB}%
\end{subfigure}%
\hfill%
\begin{subfigure}[t]{\ltwopicwidth}%
\includegraphics[width=\ltwopicwidth]{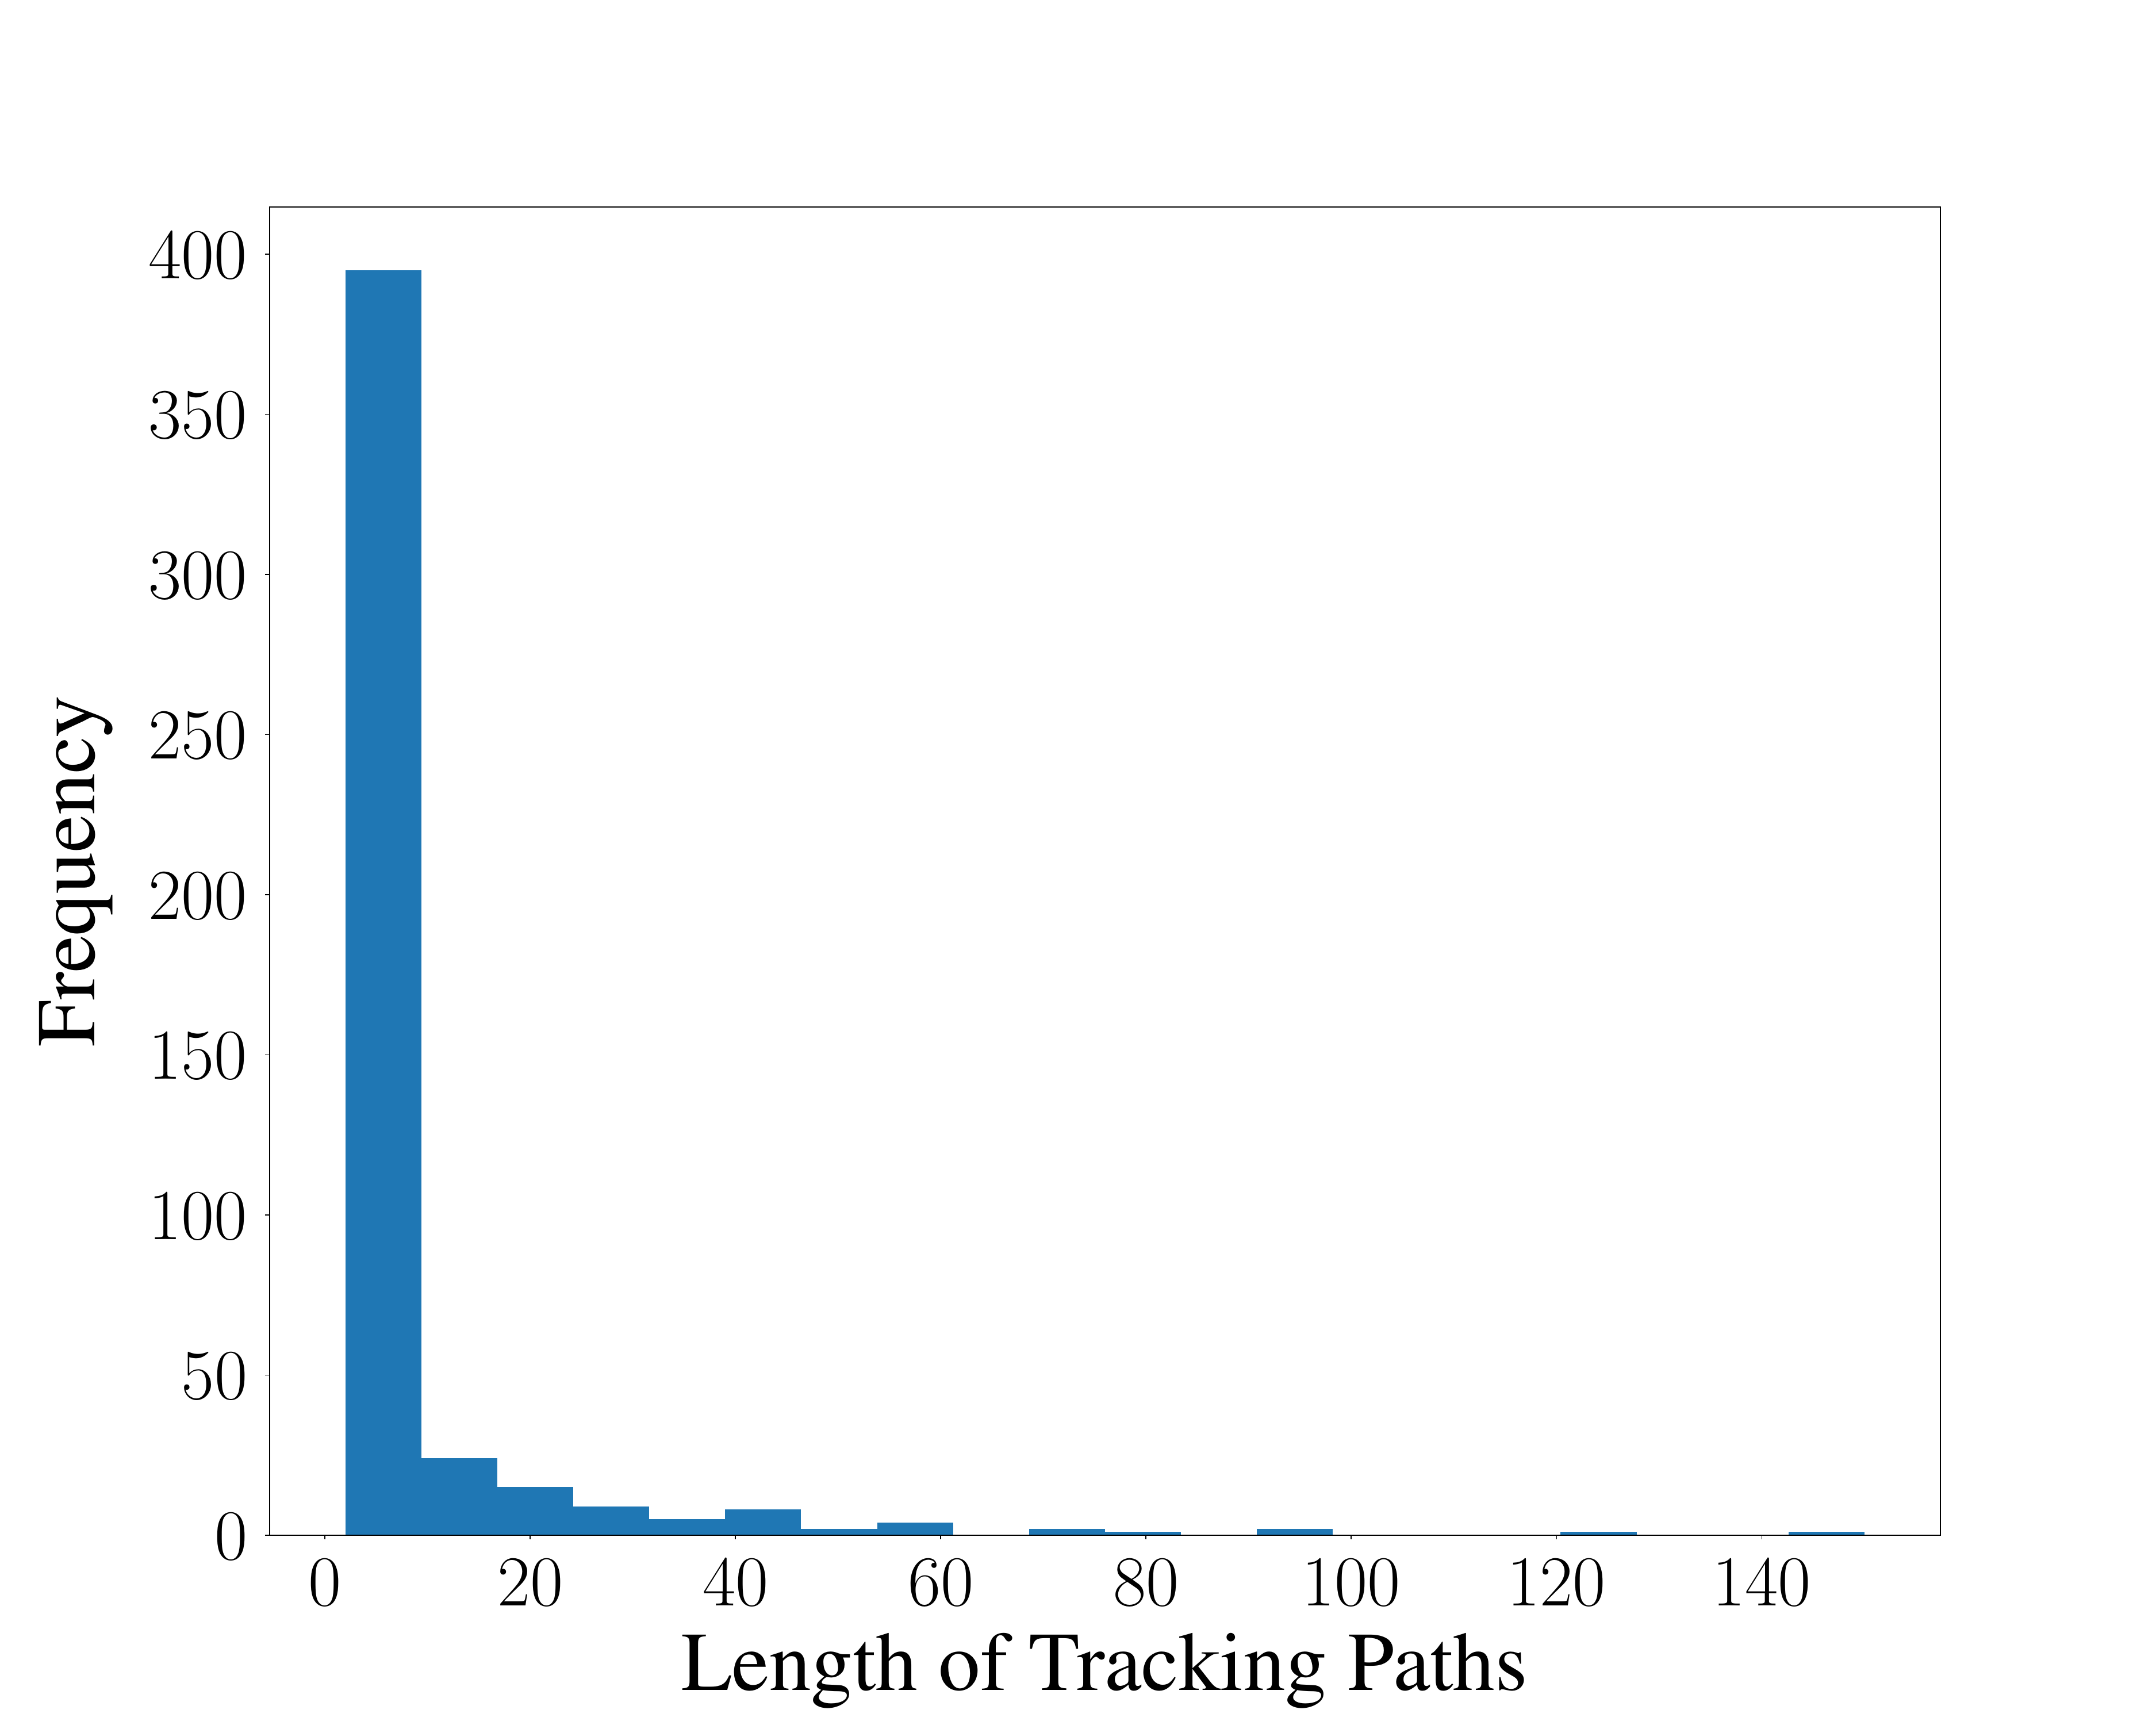}%
\caption{$d_p$.}%
\label{fig-LengthHistogramCylinder3DP}%
\end{subfigure}%
\caption{Histograms of the length of the tracking paths 
    of \dataset{Cylinder3D}.}%
\label{fig-LengthHisgoramCylinder3D}%
\end{figure}

\begin{figure}
\centering
\includegraphics[width=0.8\linewidth]{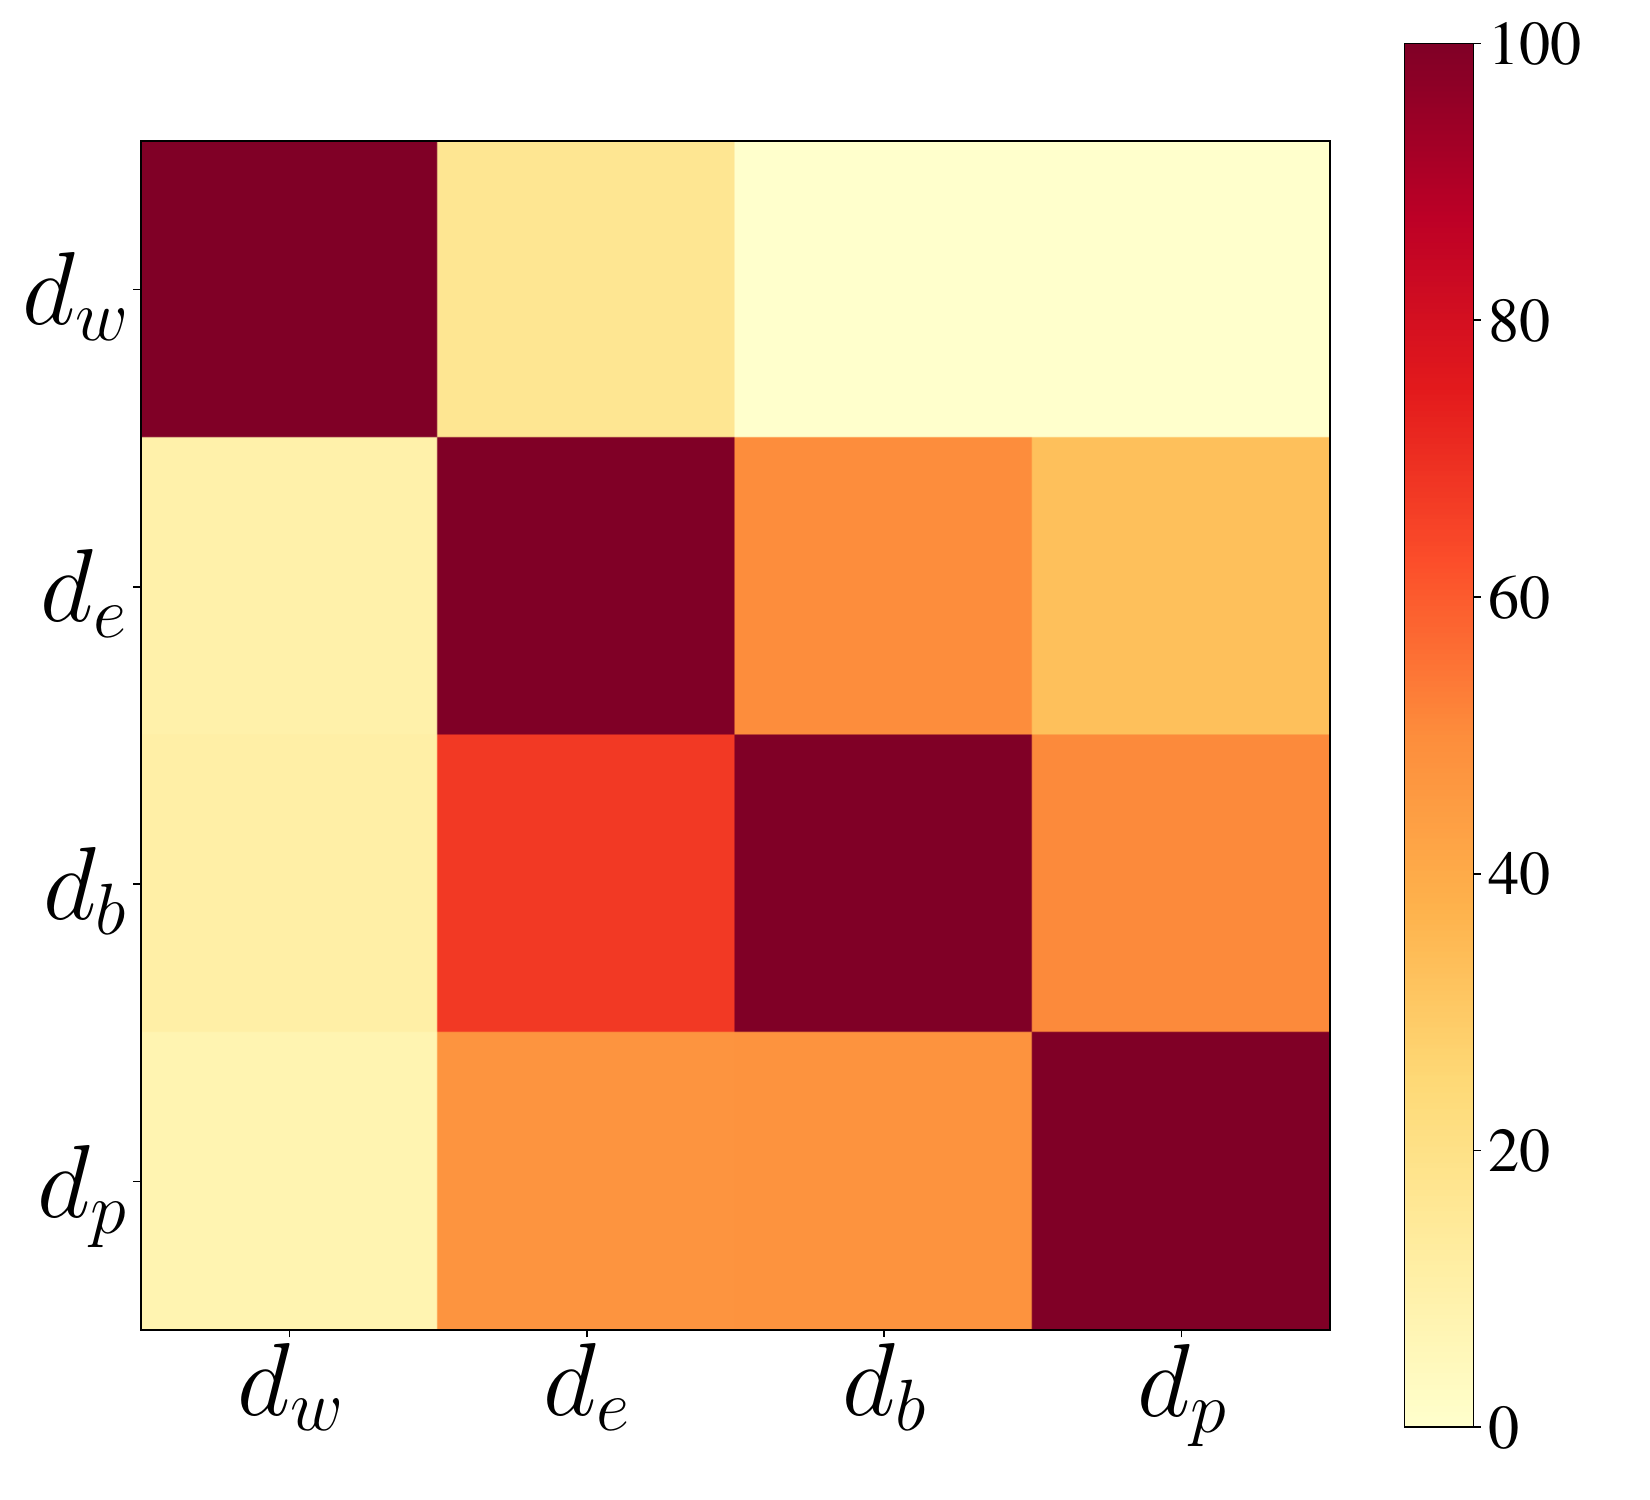}
\caption{
    Pairwise differences between the methods on the columns
    in relation to the methods on the rows
    for \dataset{Cylinder3D}.
}
\label{fig-Cylinder3DSimilarities}
\end{figure}

\subsection*{Results with Tangaroa data set}
The results of the experiments using \dataset{Tangaroa3D}
are shown in \Cref{fig-Tangaroa3DAllNodes}
through \Cref{fig-Tangaroa3DSimilarities}.

\begin{figure}
\centering
\includegraphics[width=0.8\linewidth]{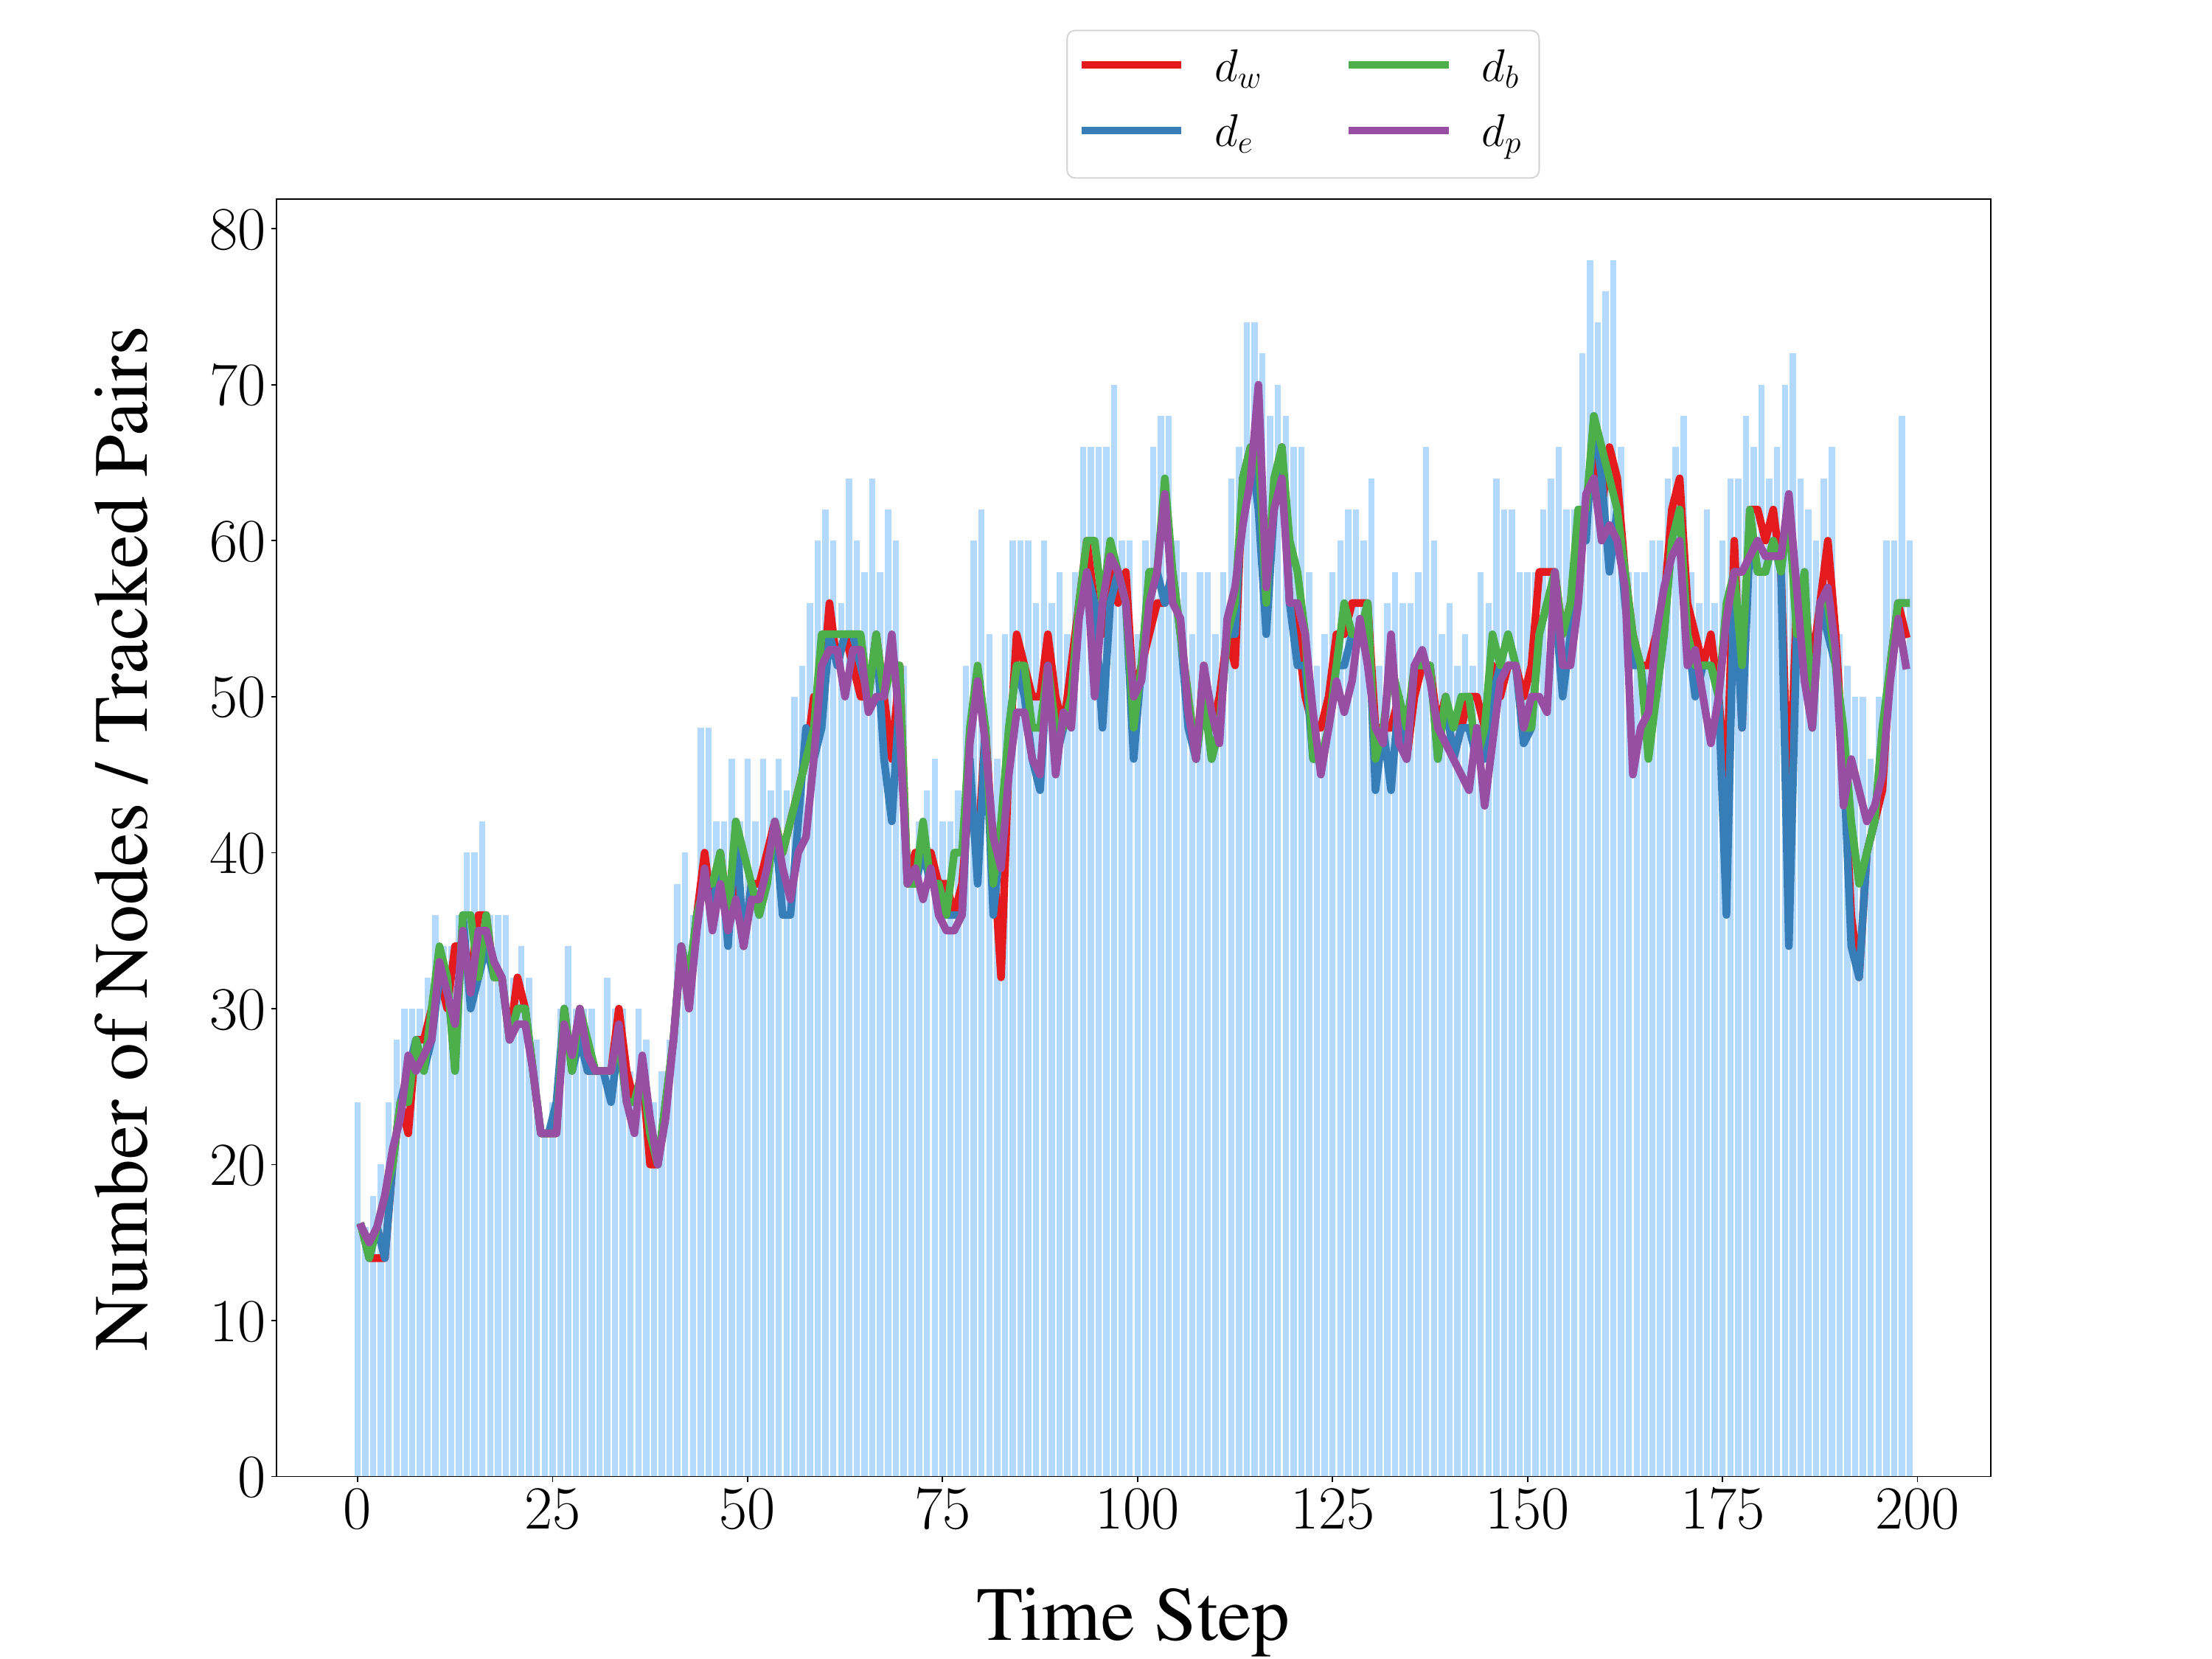}
\caption{
    Number of tracked nodes (colored and labeled) 
    relative to the total nodes of merge trees (light blue bars)
    for \dataset{Tangaroa3D}.
}
\label{fig-Tangaroa3DAllNodes}
\end{figure}

\begin{figure}
\centering
\includegraphics[width=0.8\linewidth]{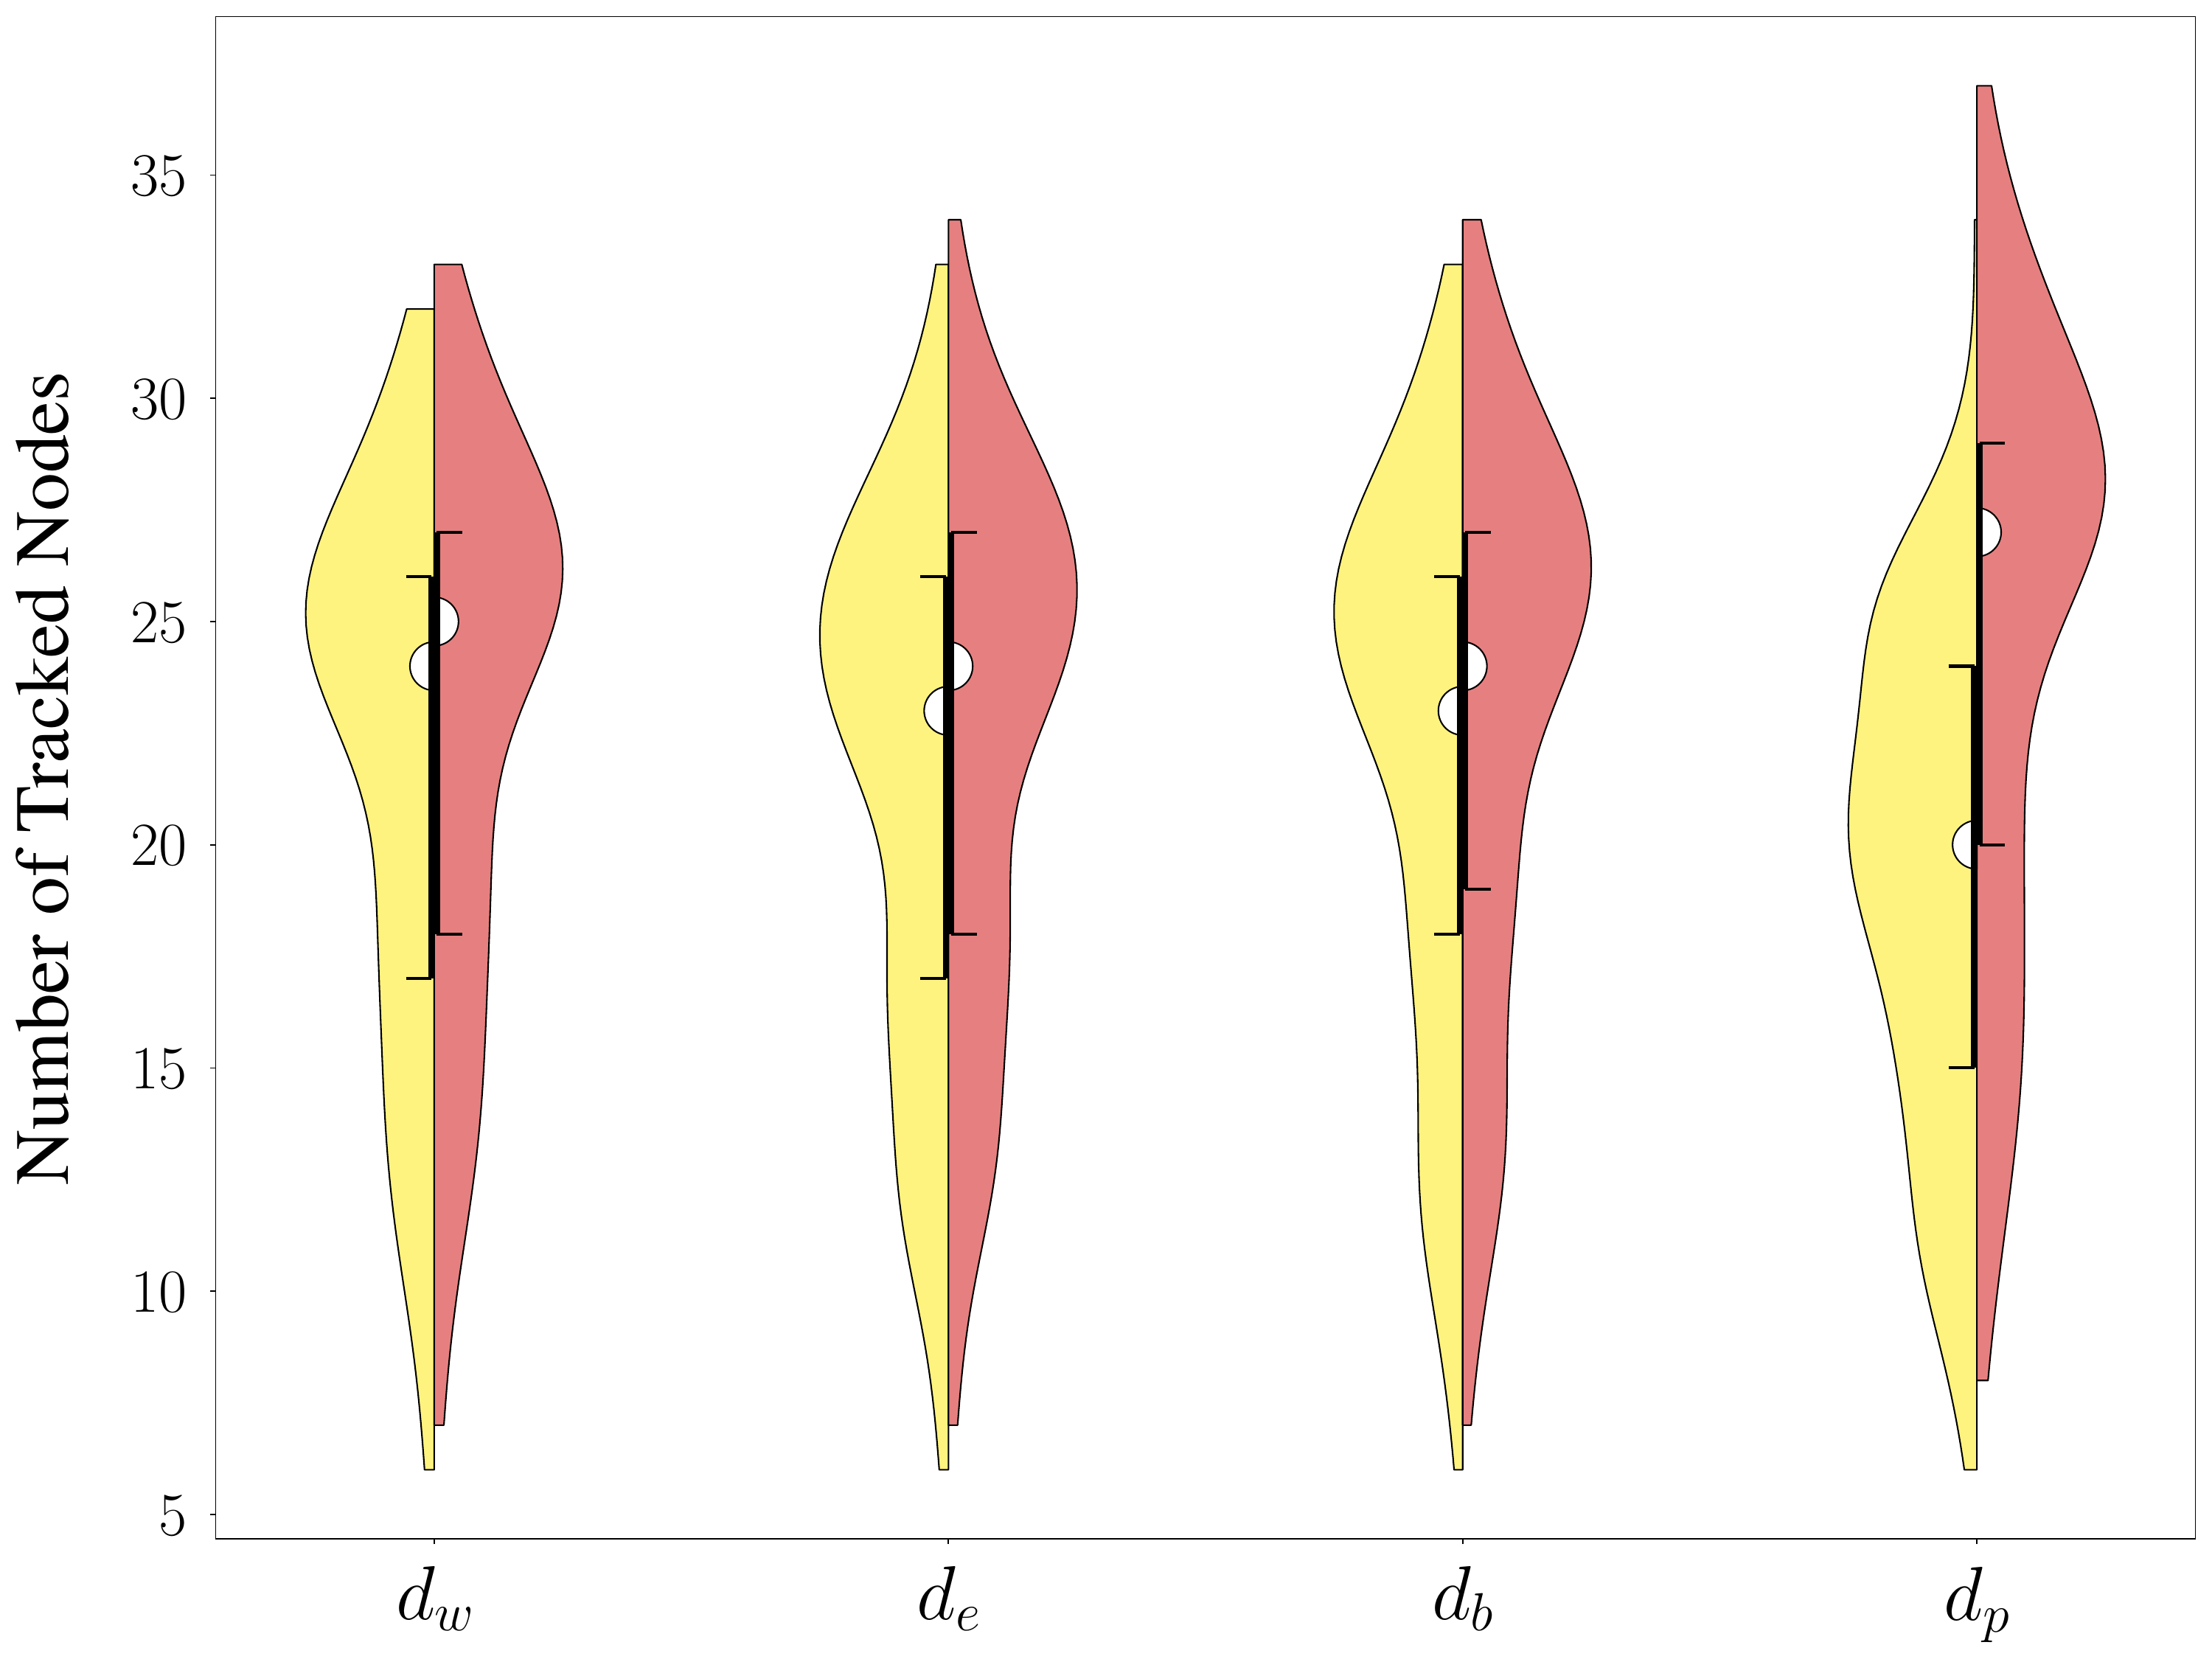}
\caption{
    Distributions of tracked nodes 
    \dataset{Tangaroa3D},  
    divided by types:
    saddle (yellow) and maxima (red).
}
\label{fig-Tangaroa3DViolin}
\end{figure}

% Length histogram
\begin{figure}%
\begin{subfigure}[t]{\ltwopicwidth}%
\includegraphics[width=\ltwopicwidth]{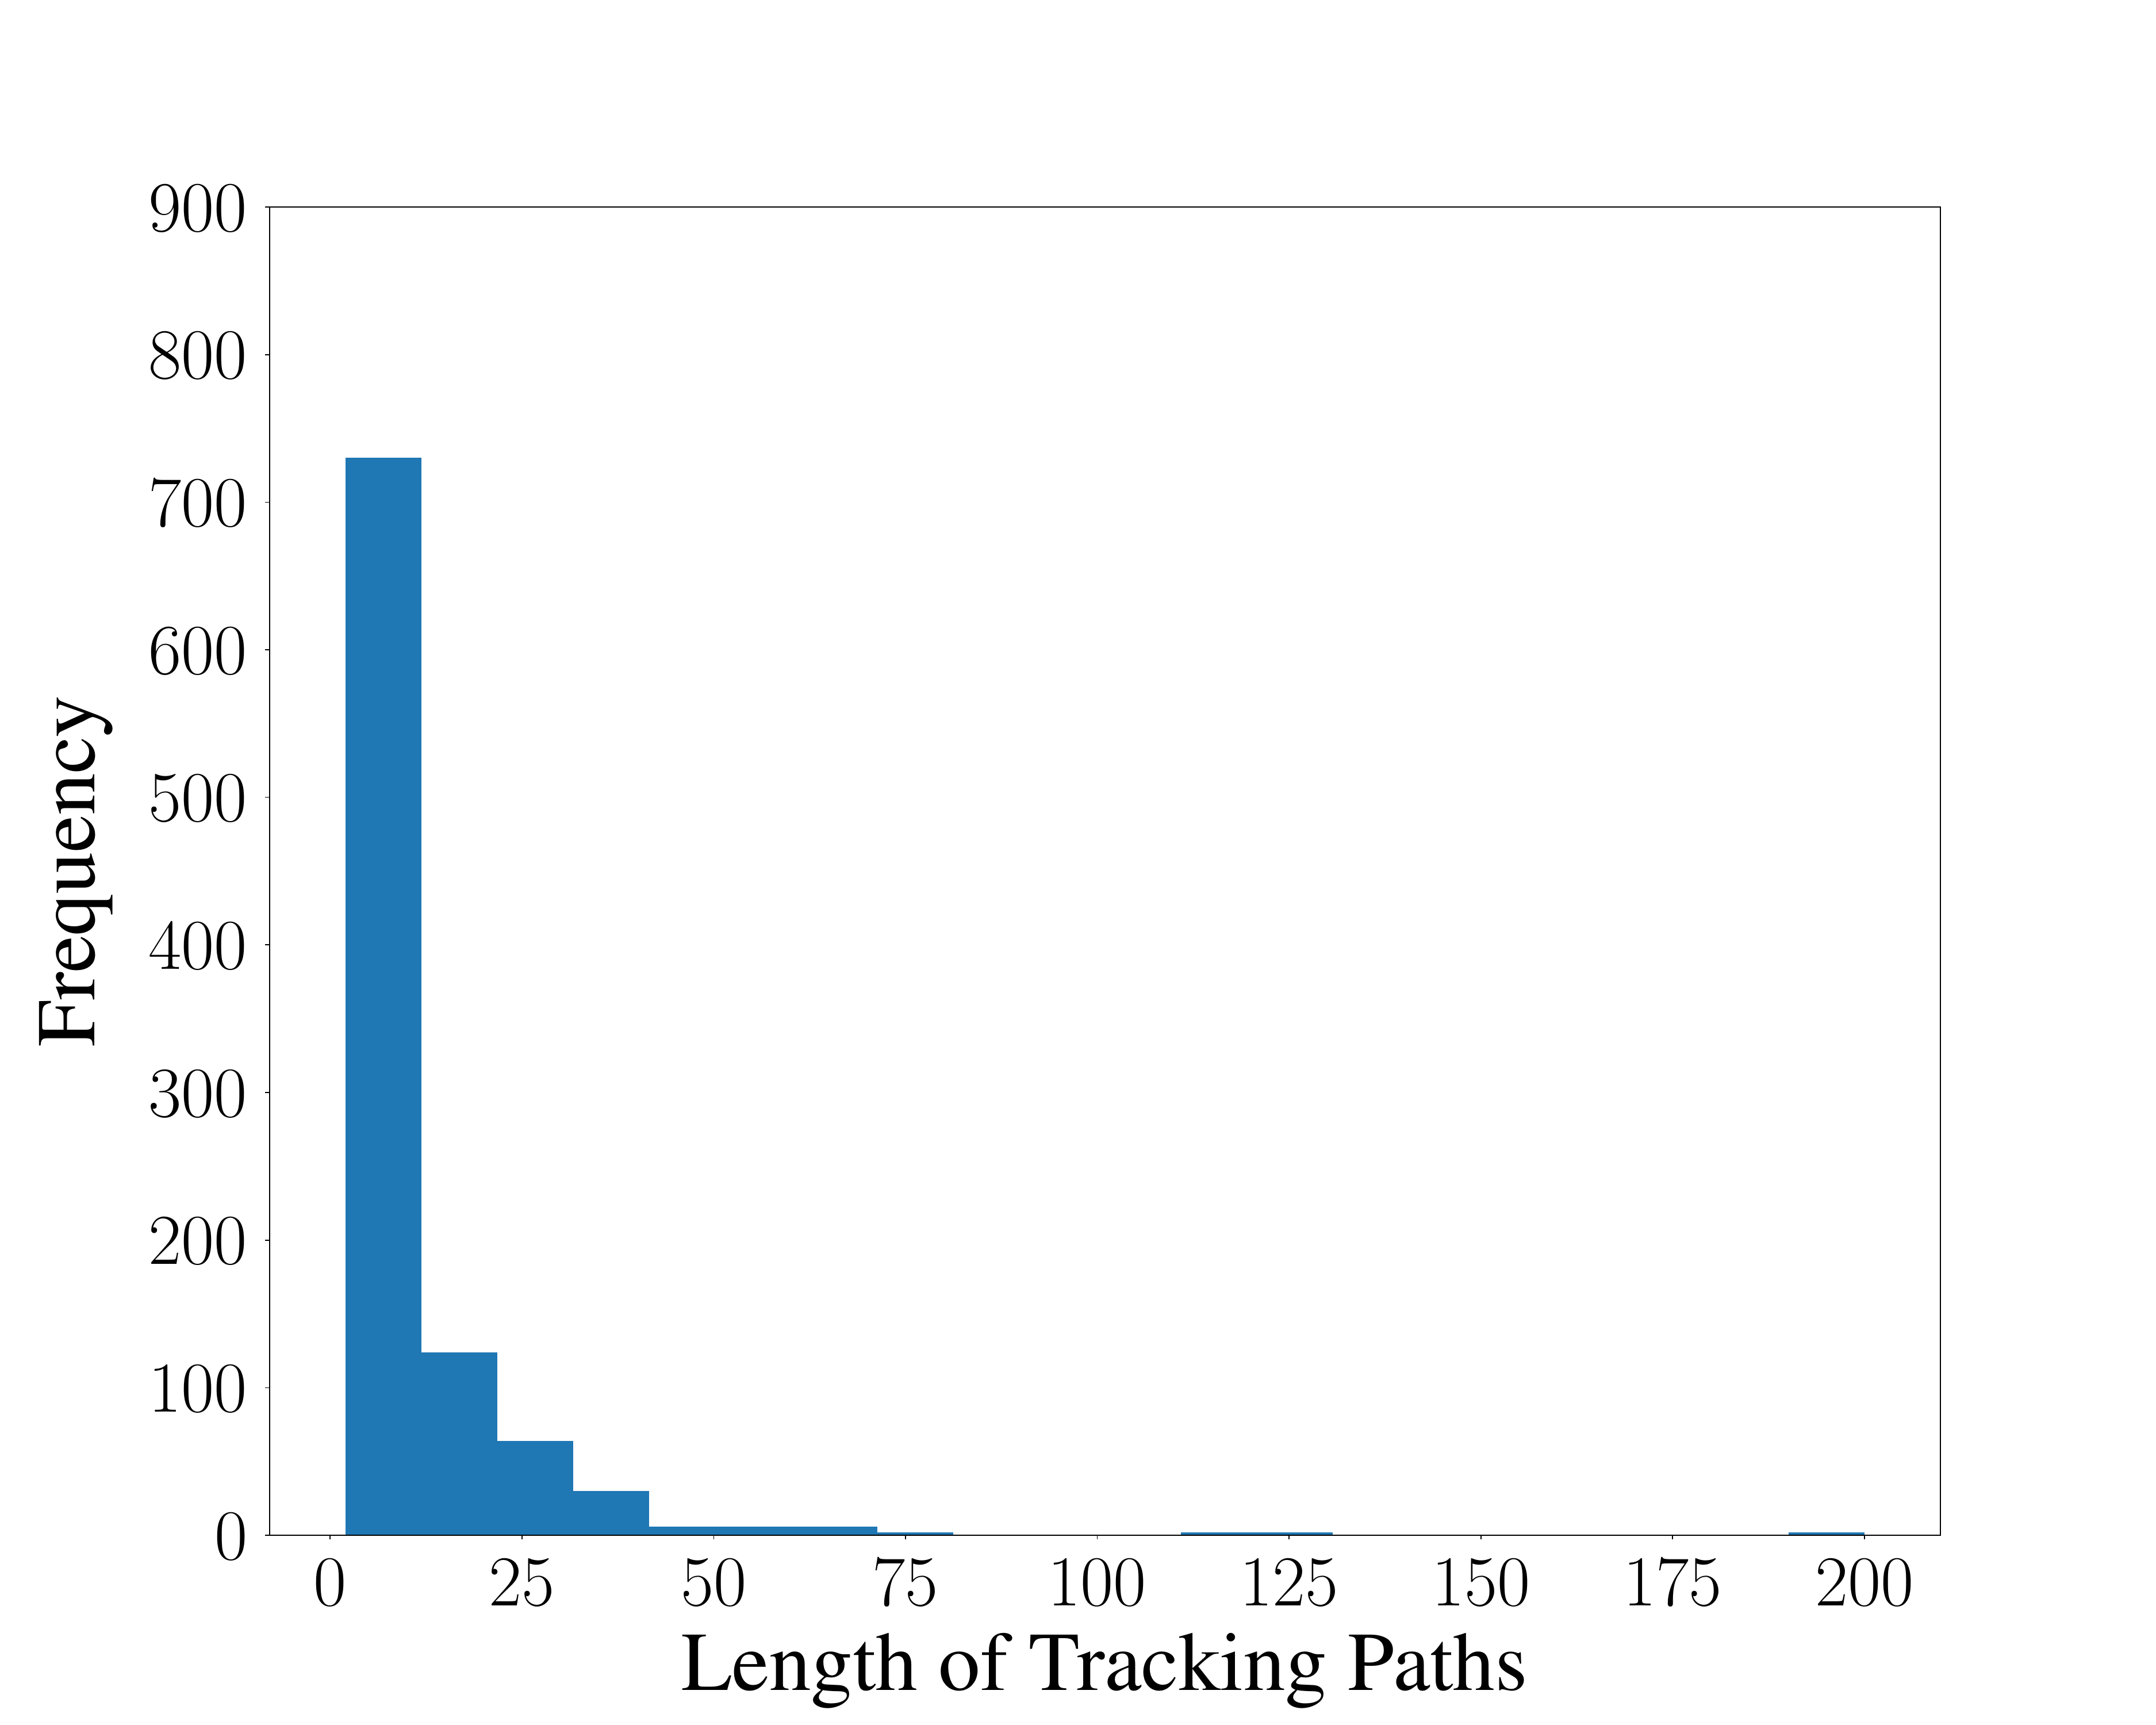}
\caption{$d_w$.}%
\label{fig-LengthHistogramTangaroa3DW}%
\end{subfigure}
\hfill%
\begin{subfigure}[t]{\ltwopicwidth}%
\includegraphics[width=\ltwopicwidth]{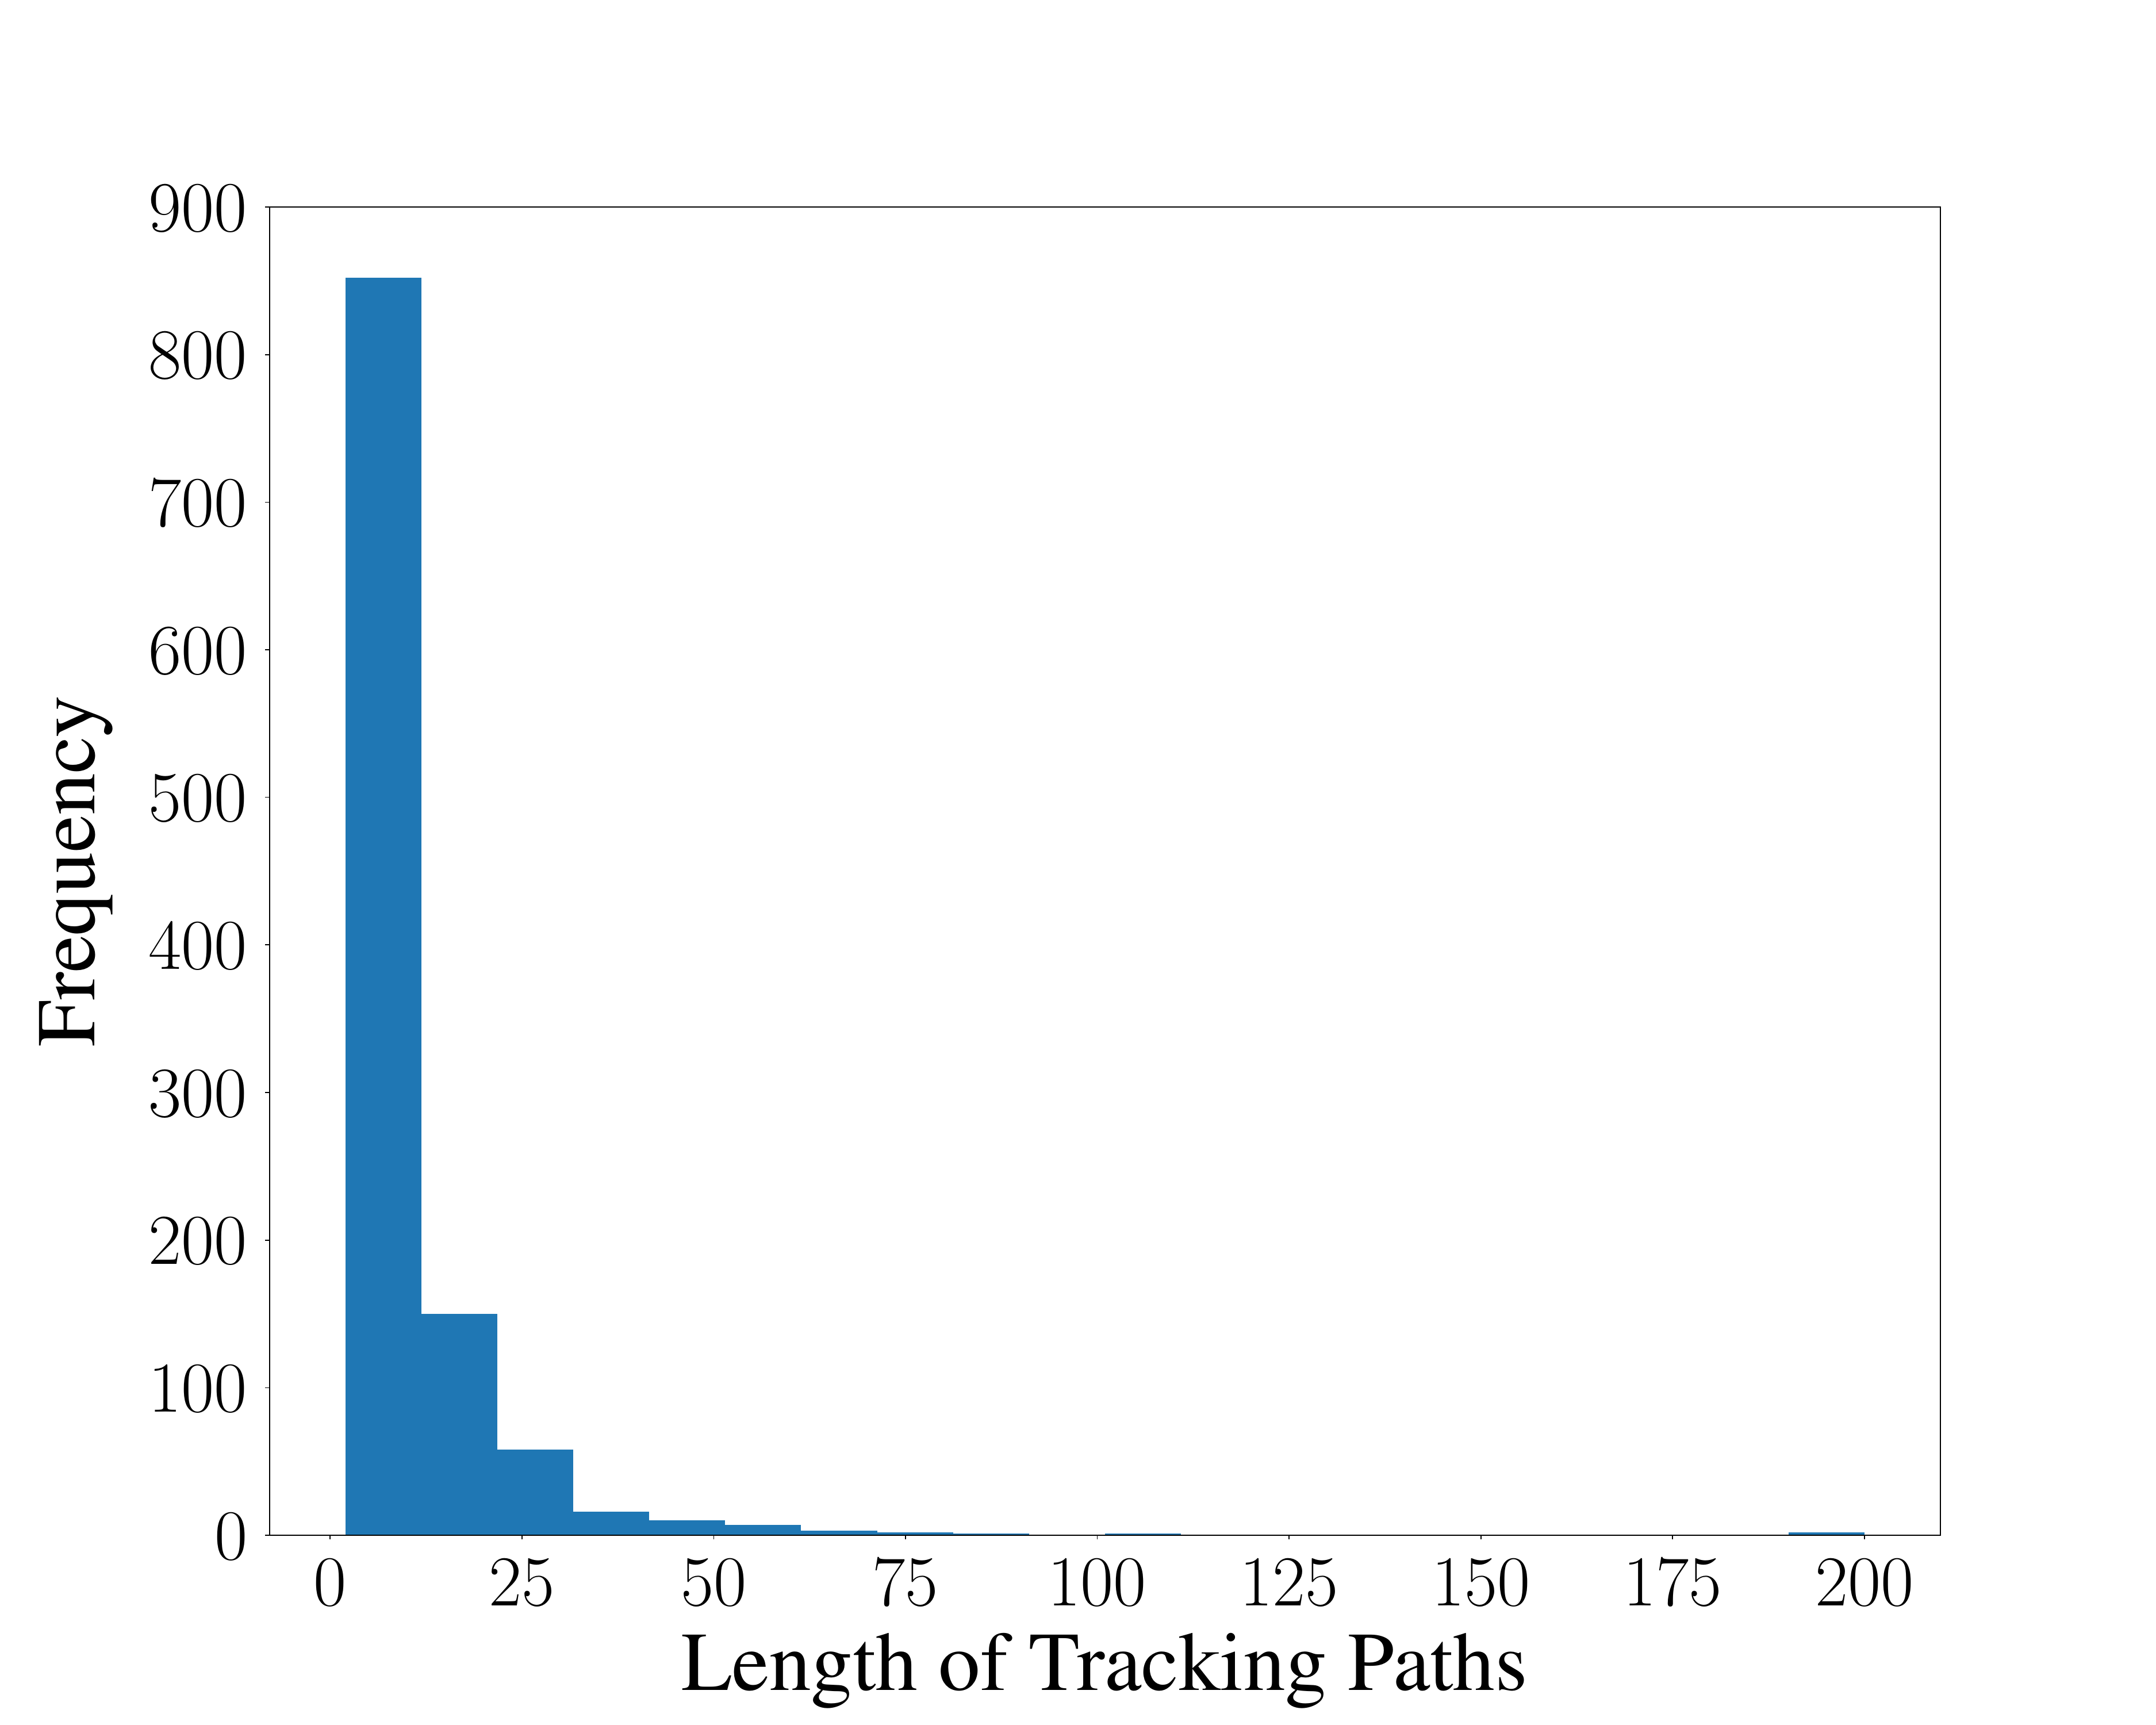}%
\caption{$d_e$.}%
\label{fig-LengthHistogramTangaroa3DE}%
\end{subfigure}%
\\%
\begin{subfigure}[t]{\ltwopicwidth}%
\includegraphics[width=\ltwopicwidth]{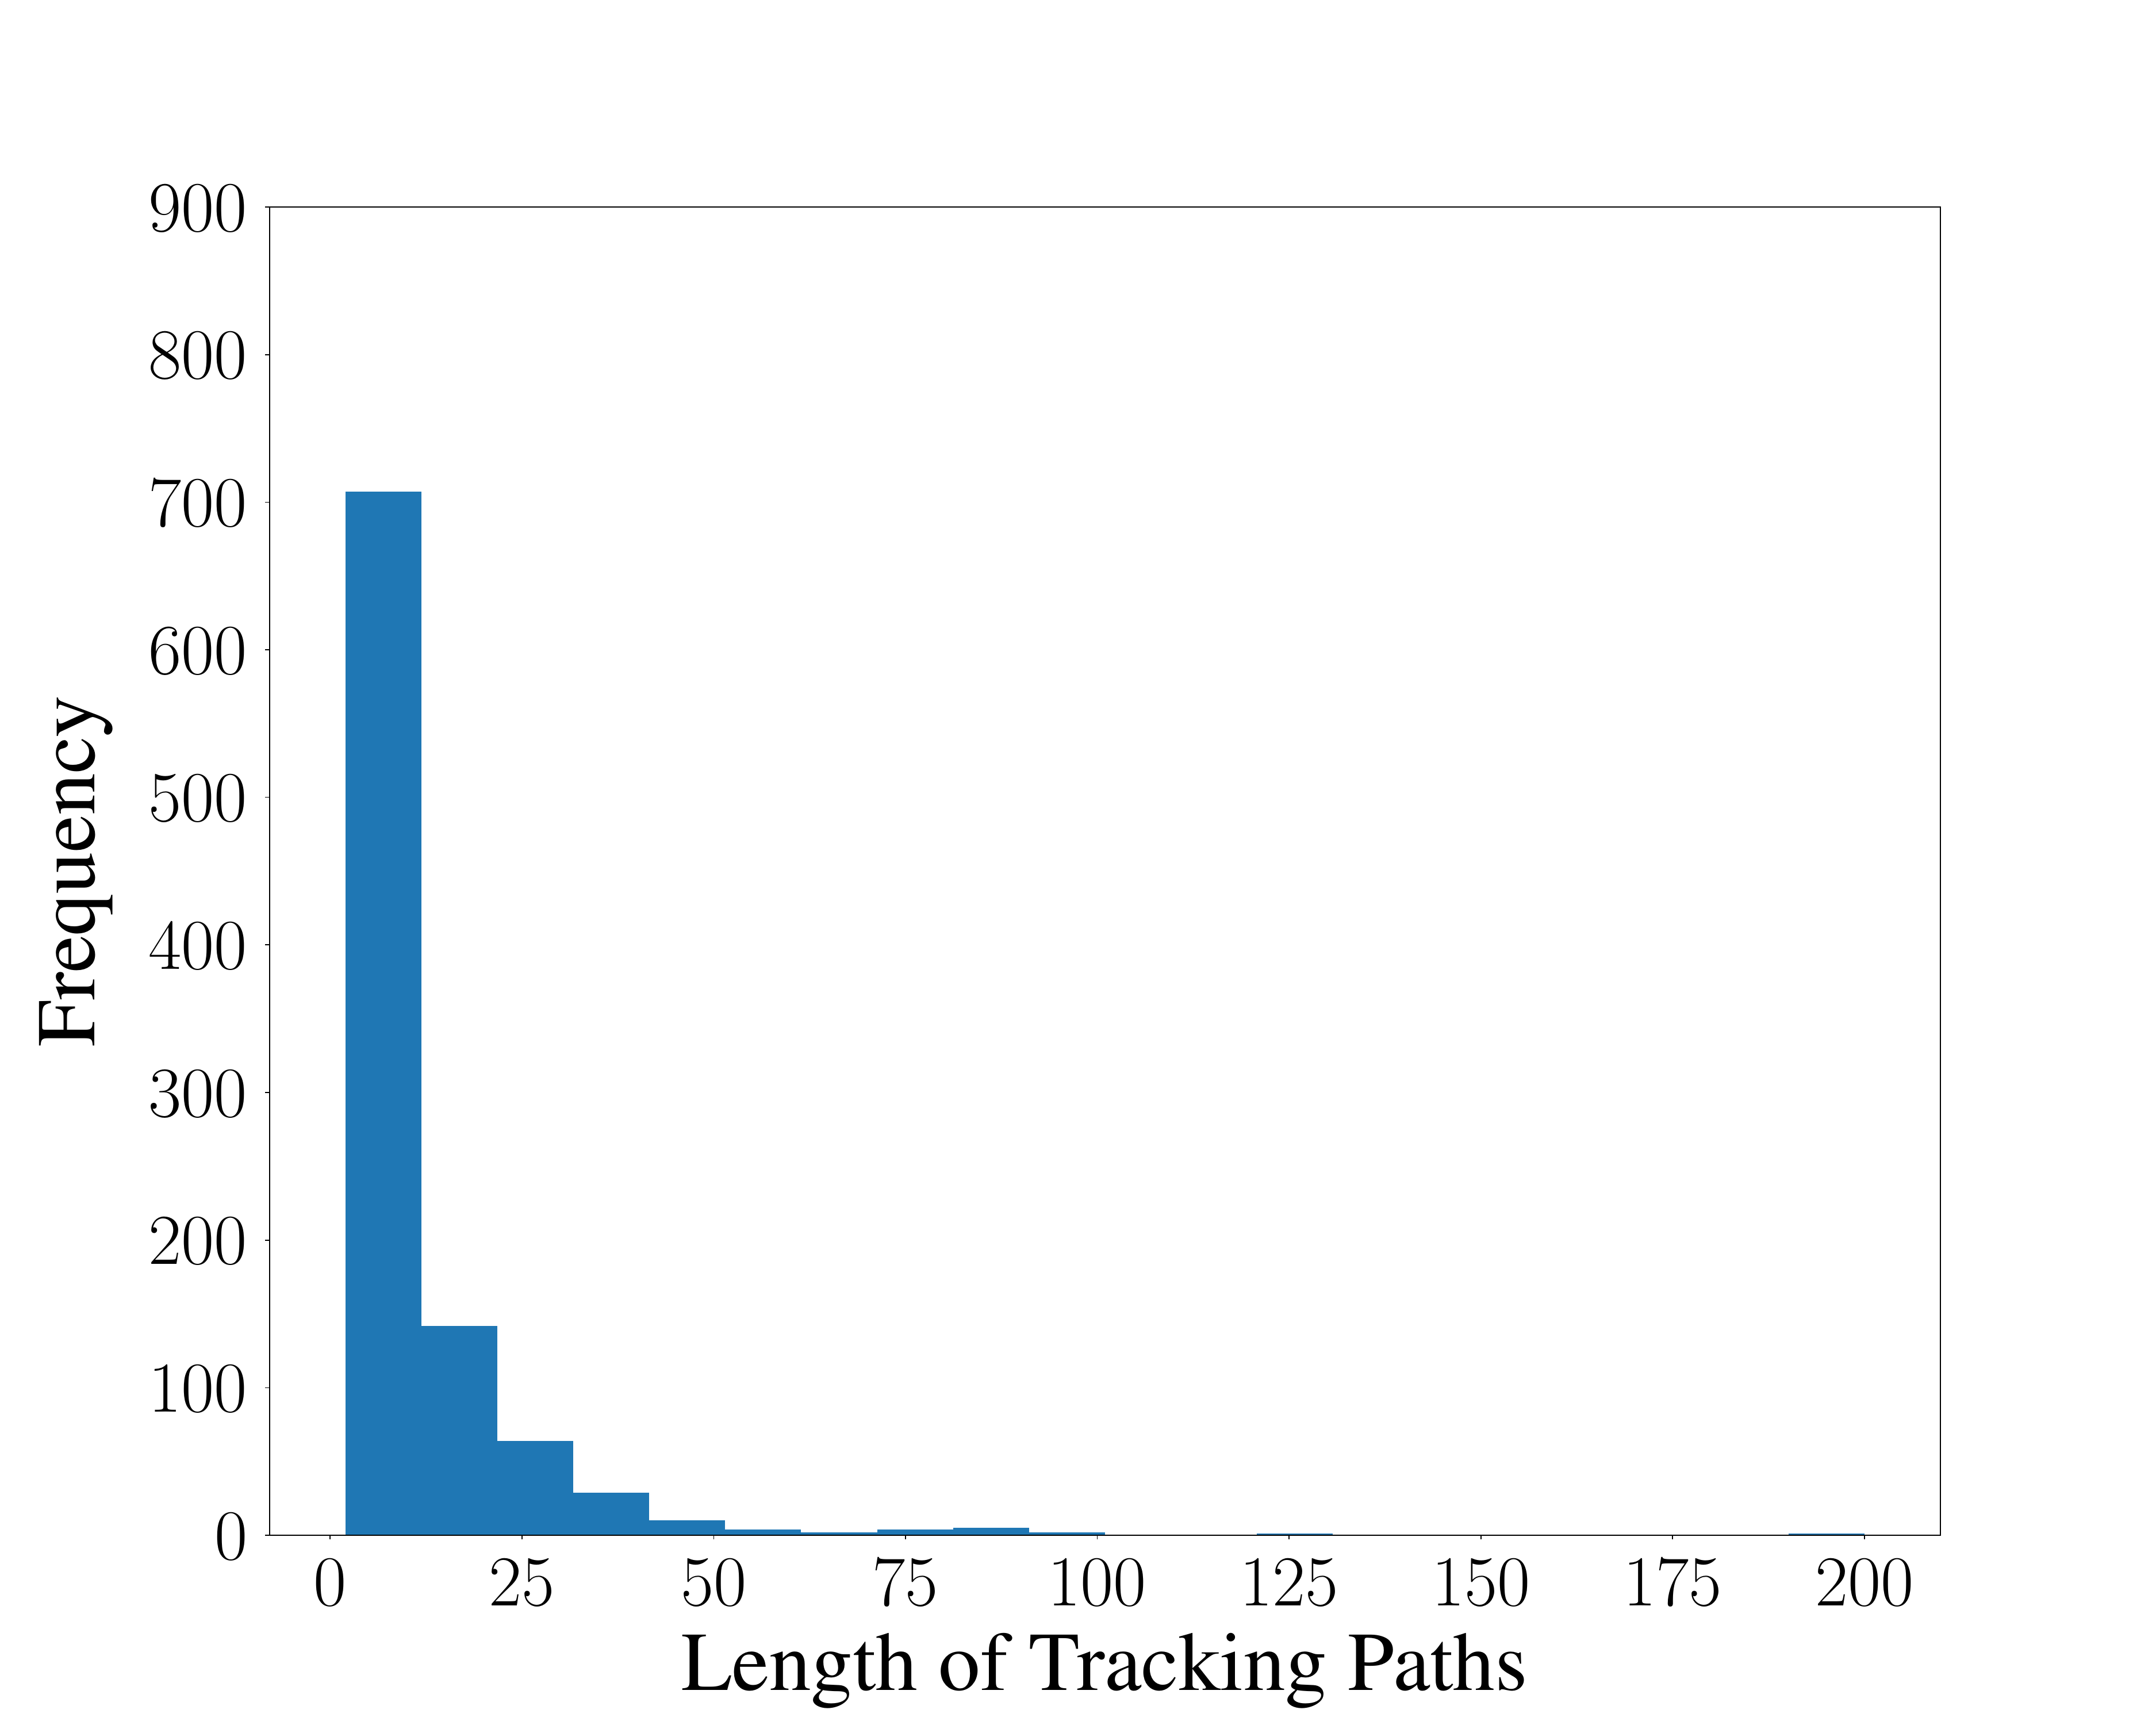}%
\caption{$d_b$.}%
\label{fig-LengthHistogramTangaroa3DB}%
\end{subfigure}%
\hfill%
\begin{subfigure}[t]{\ltwopicwidth}%
\includegraphics[width=\ltwopicwidth]{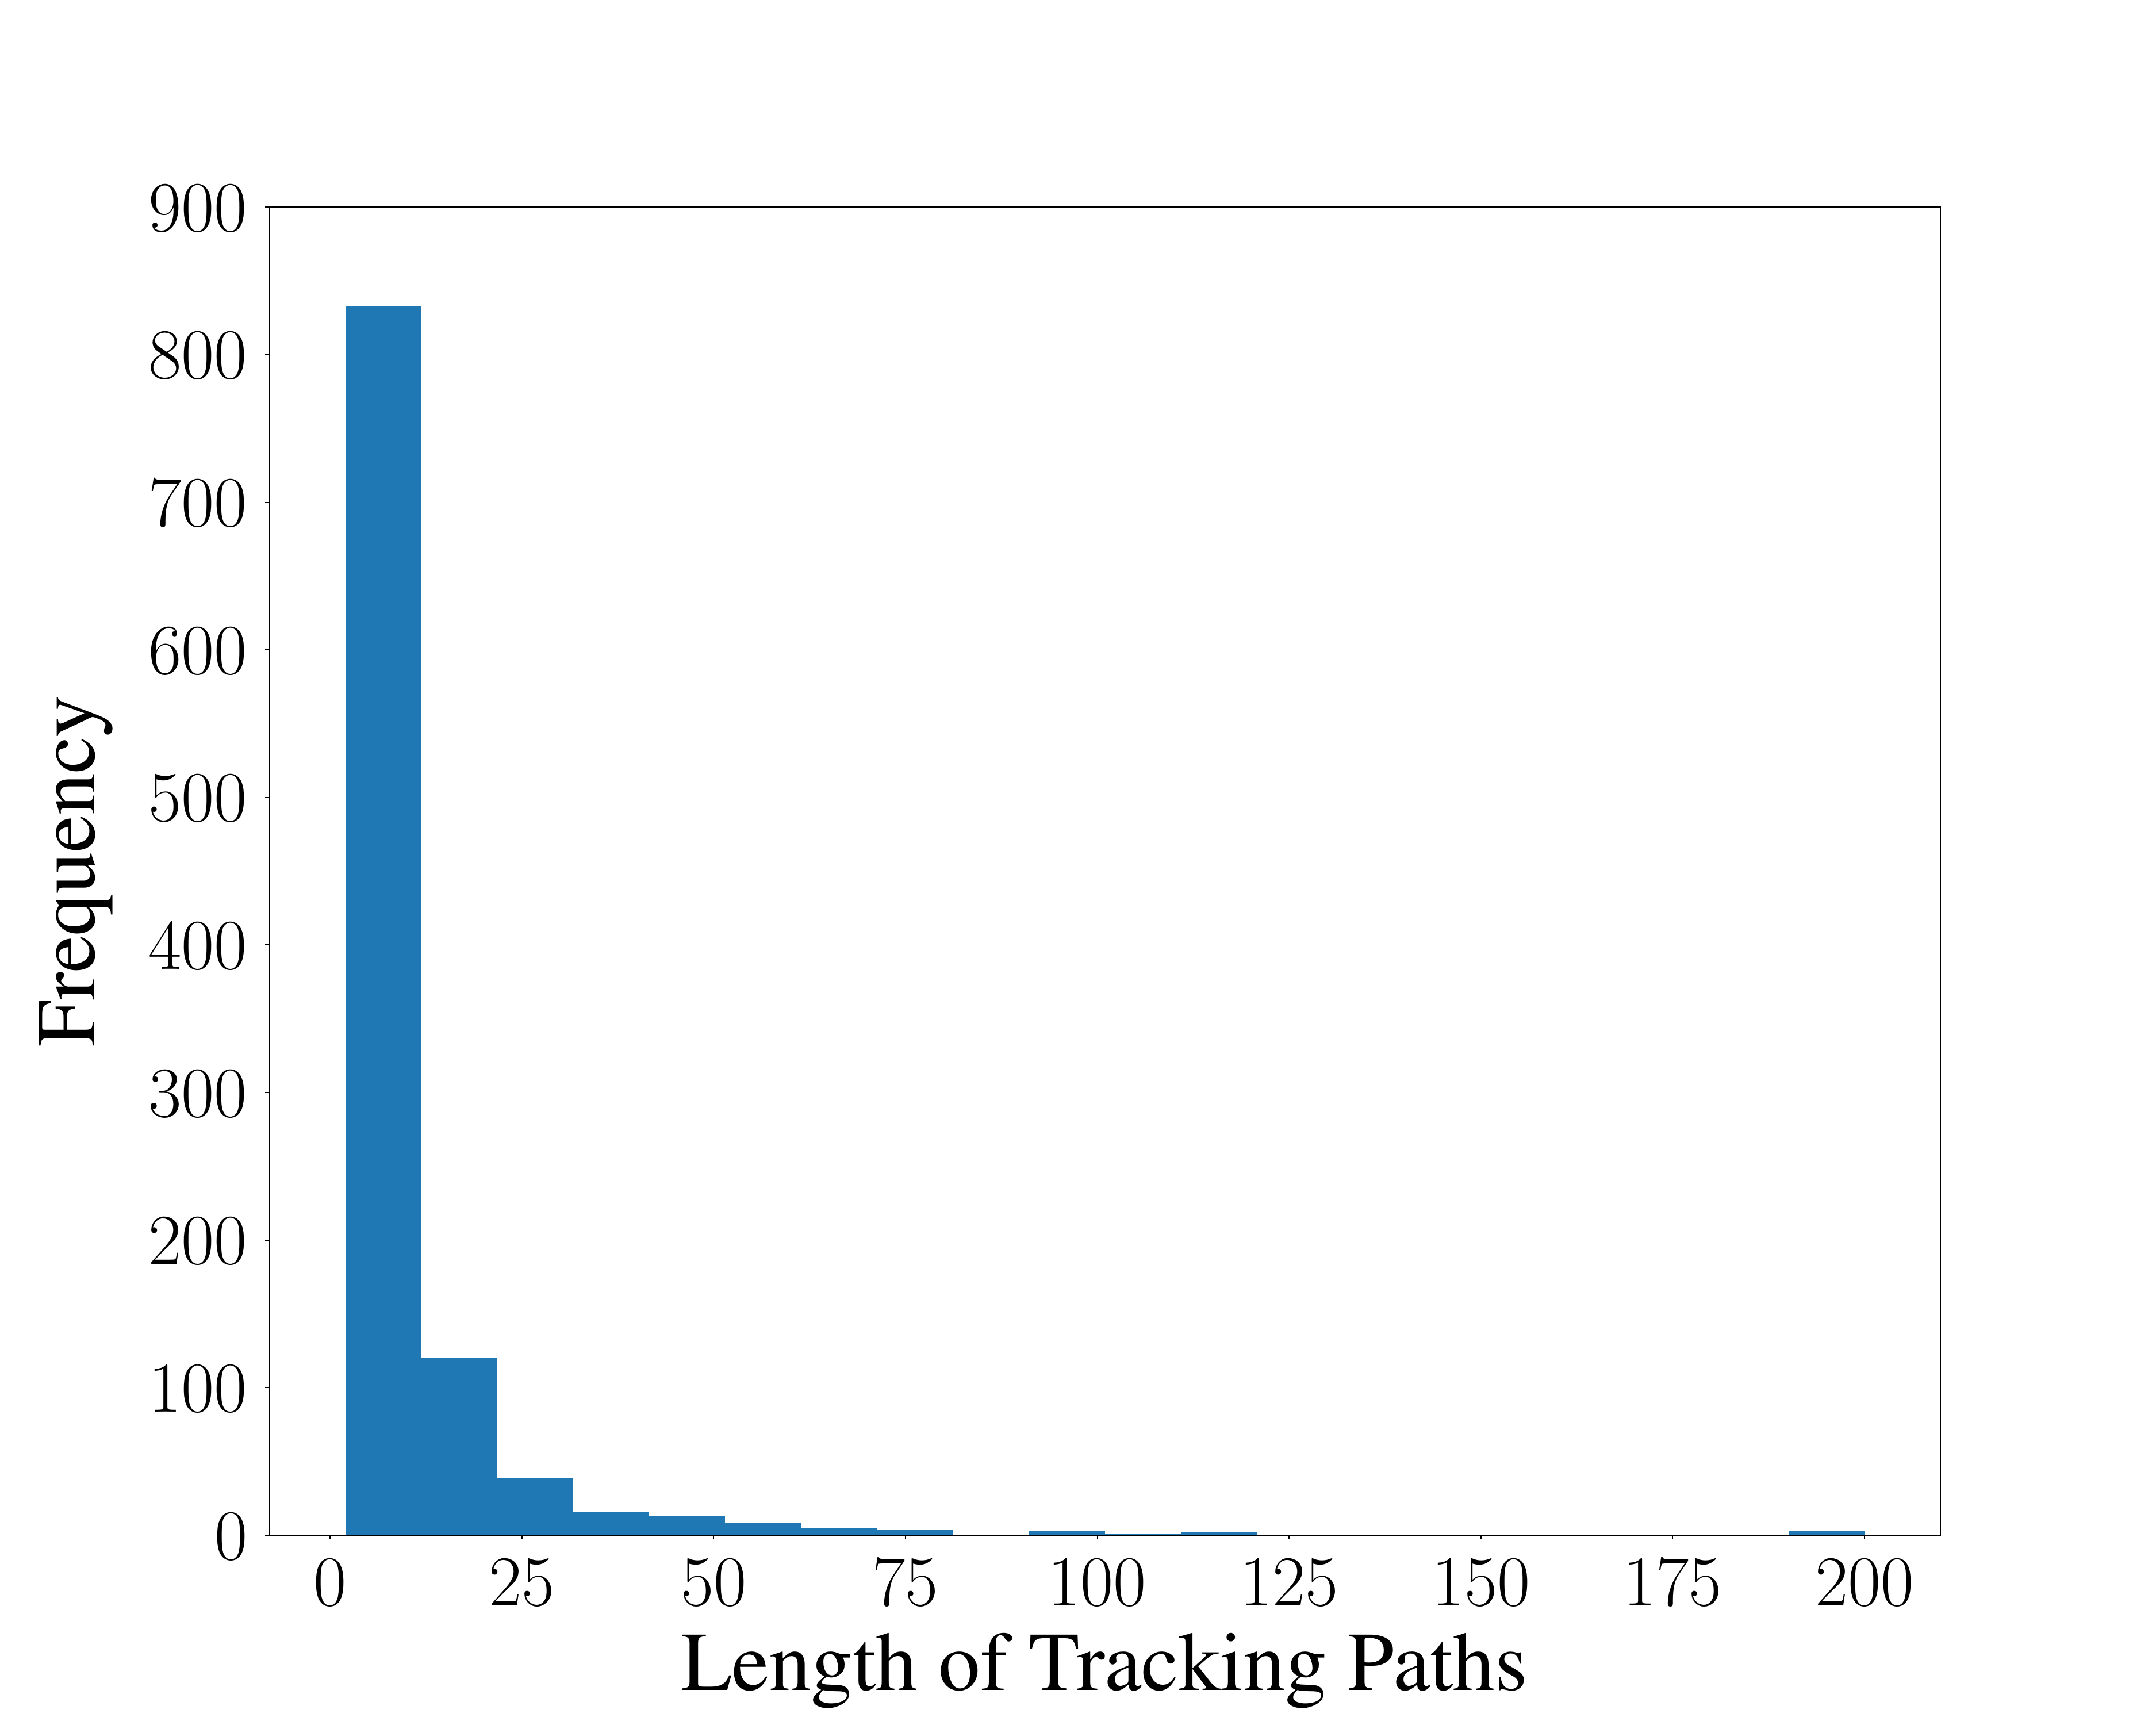}%
\caption{$d_p$.}%
\label{fig-LengthHistogramTangaroa3DP}%
\end{subfigure}%
\caption{Histograms of the length of the tracking paths
    of \dataset{Tangaroa3D}.}%
\label{fig-LengthHisgoramTangaroa3D}%
\end{figure}

\begin{figure}
\centering
\includegraphics[width=0.8\linewidth]{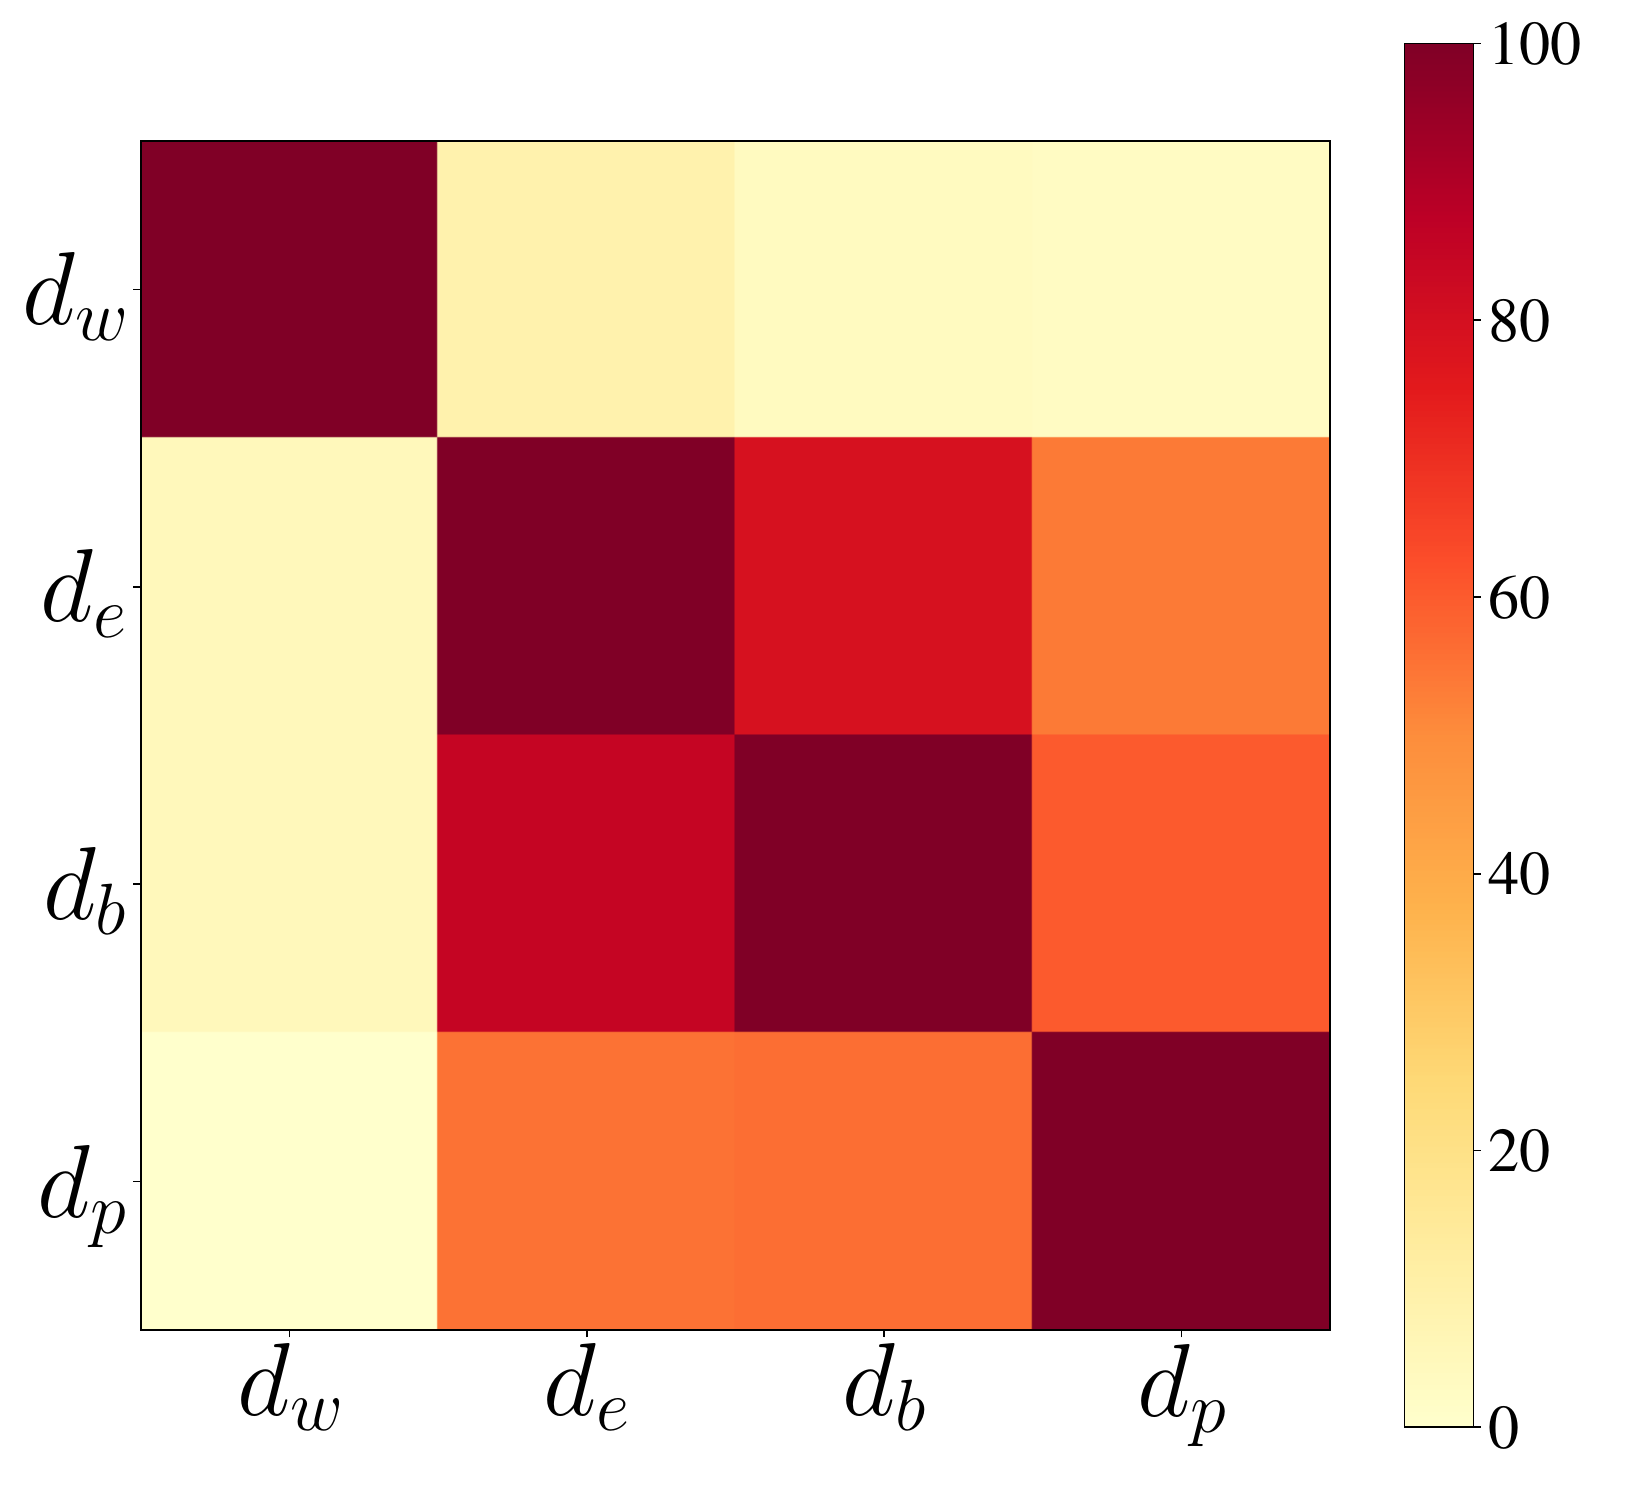}
\caption{
    Pairwise differences between the methods on the columns
    in relation to the methods on the rows
    for \dataset{Tangaroa3D}.
}
\label{fig-Tangaroa3DSimilarities}
\end{figure}

\subsection*{Extra results with Cylinder2D data set}
More results of the experiments using \dataset{Cylinder2D}
are shown in \Cref{fig-Cylinder2DAllNodesLong}
through \Cref{fig-LengthHisgoramCylinder2DLong}.

\begin{figure}
\centering
\includegraphics[width=0.8\linewidth]{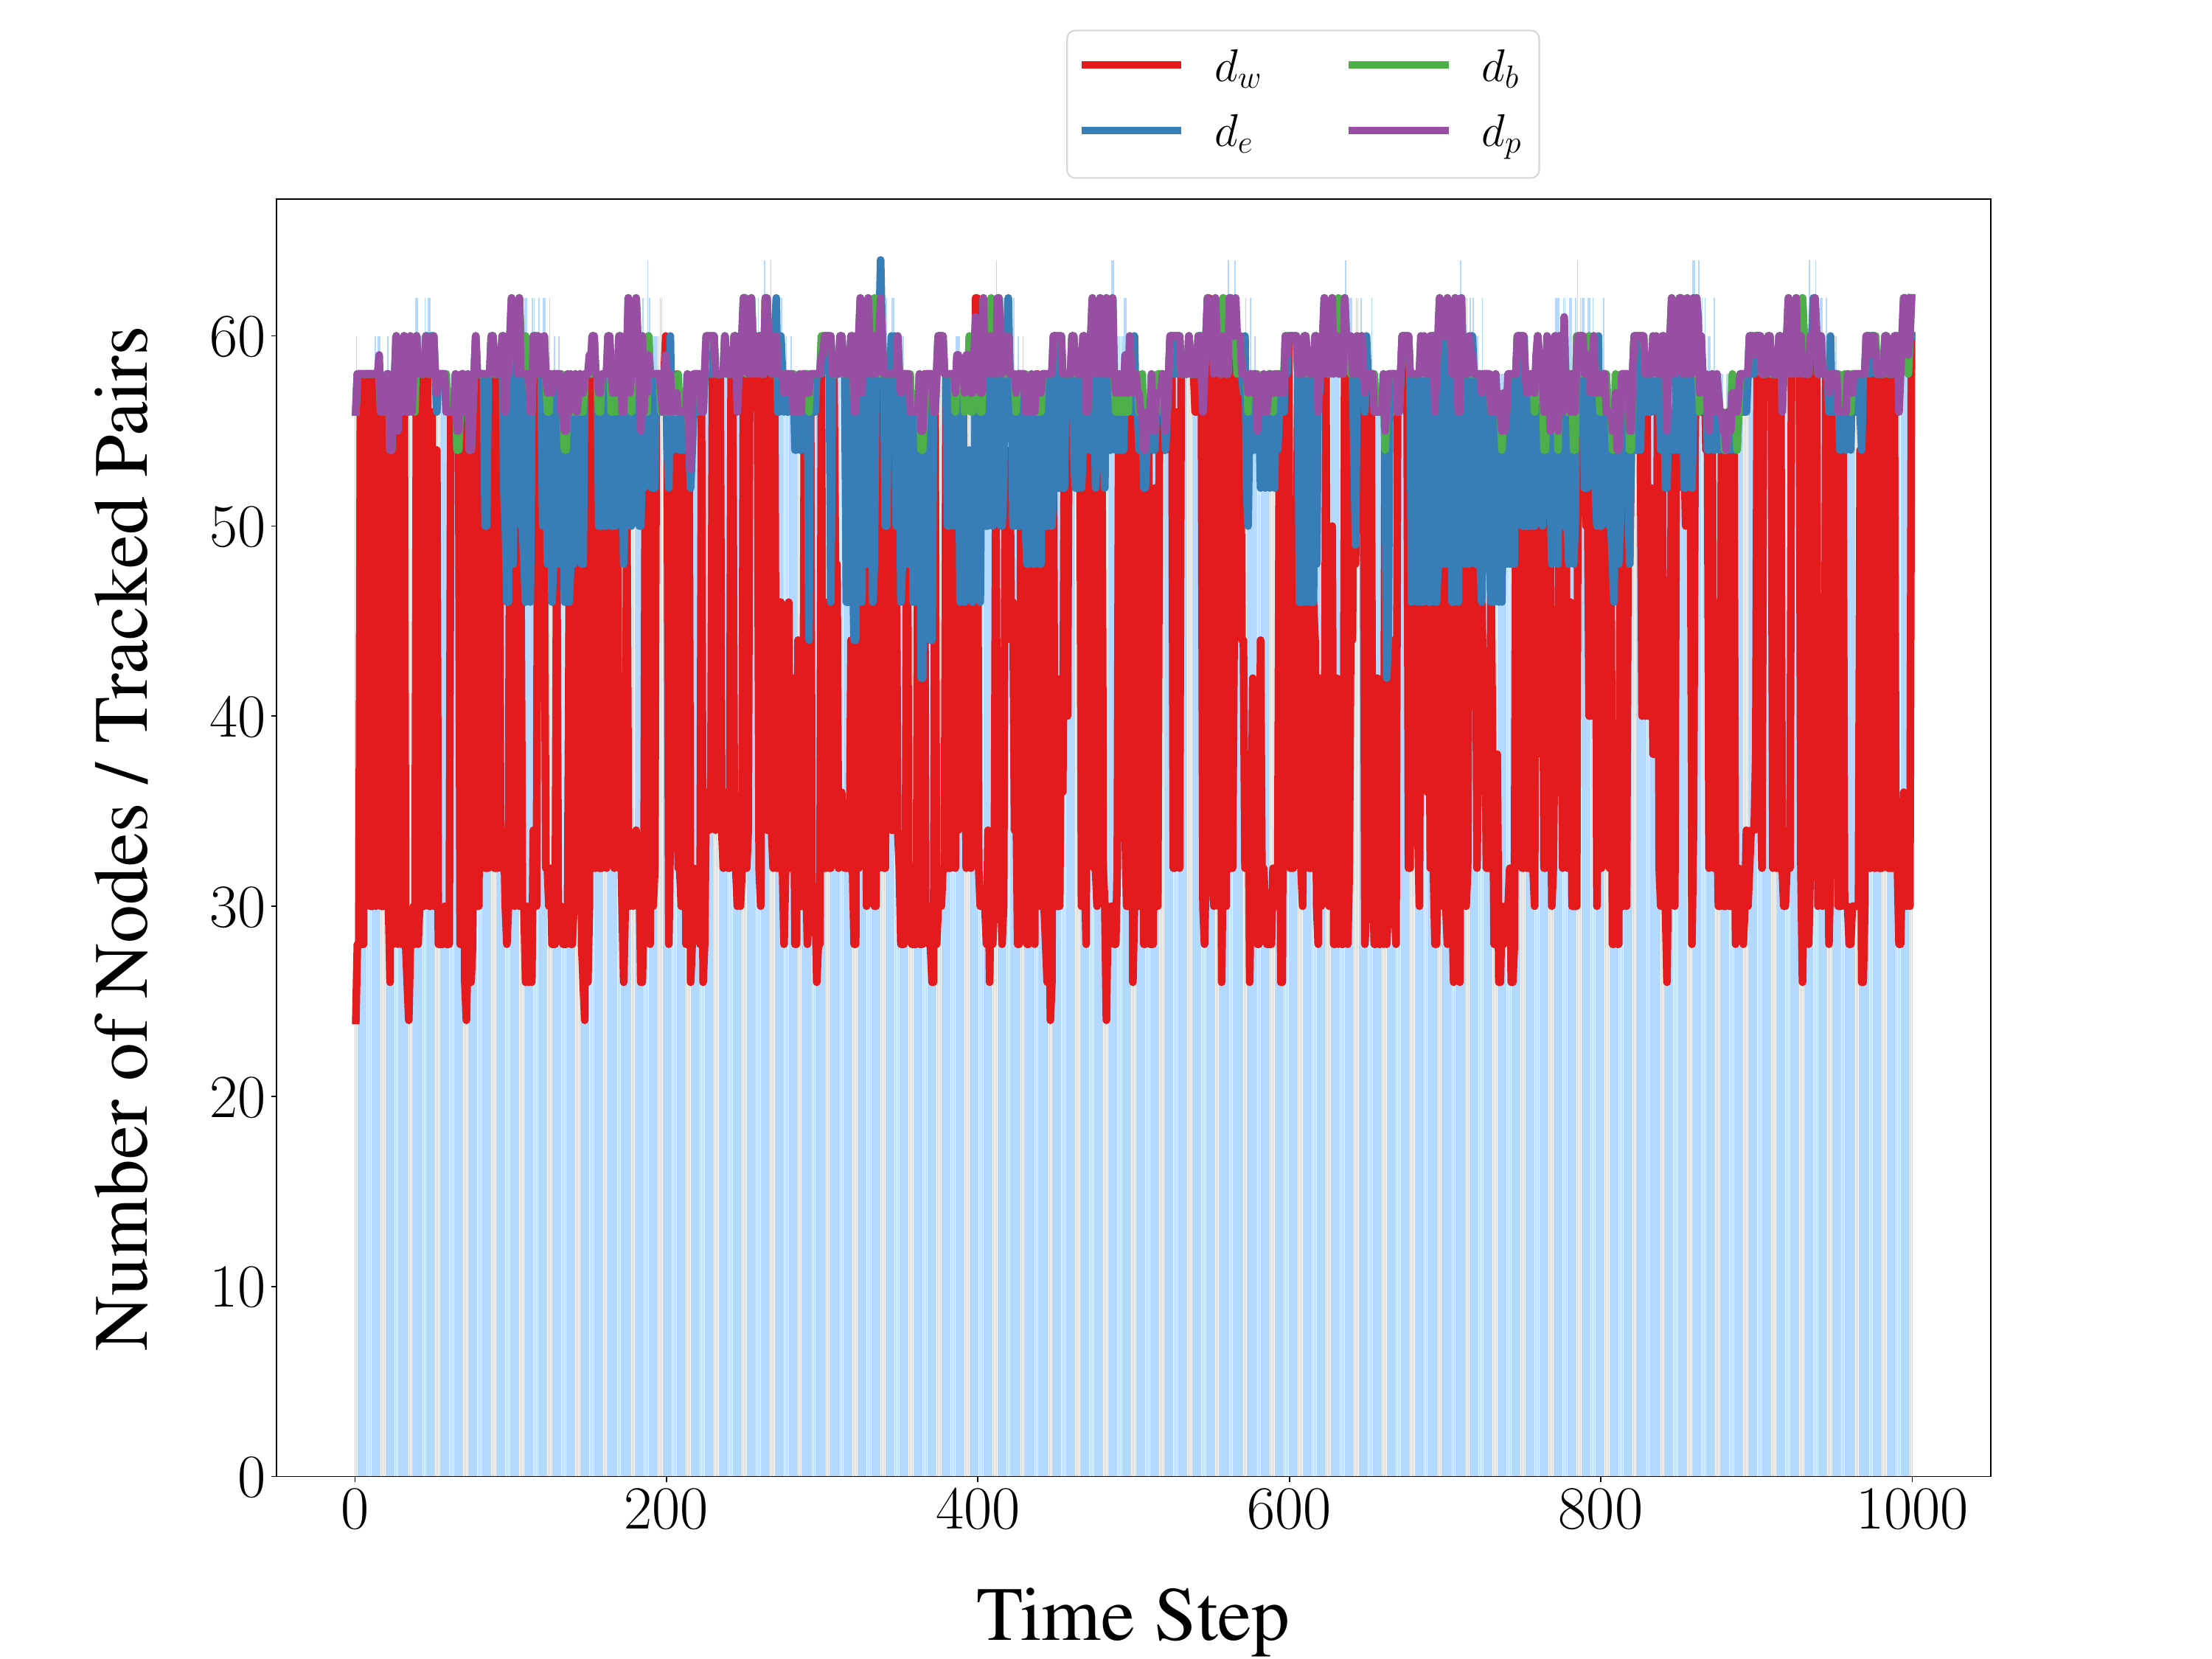}
\caption{
    Number of tracked nodes (colored and labeled) 
    relative to the total nodes of merge trees (light blue bars)
    for \dataset{Cylinder2D}.
}
\label{fig-Cylinder2DAllNodesLong}
\end{figure}

% Length histogram
\begin{figure}%
\begin{subfigure}[t]{\ltwopicwidth}%
\includegraphics[width=\ltwopicwidth]{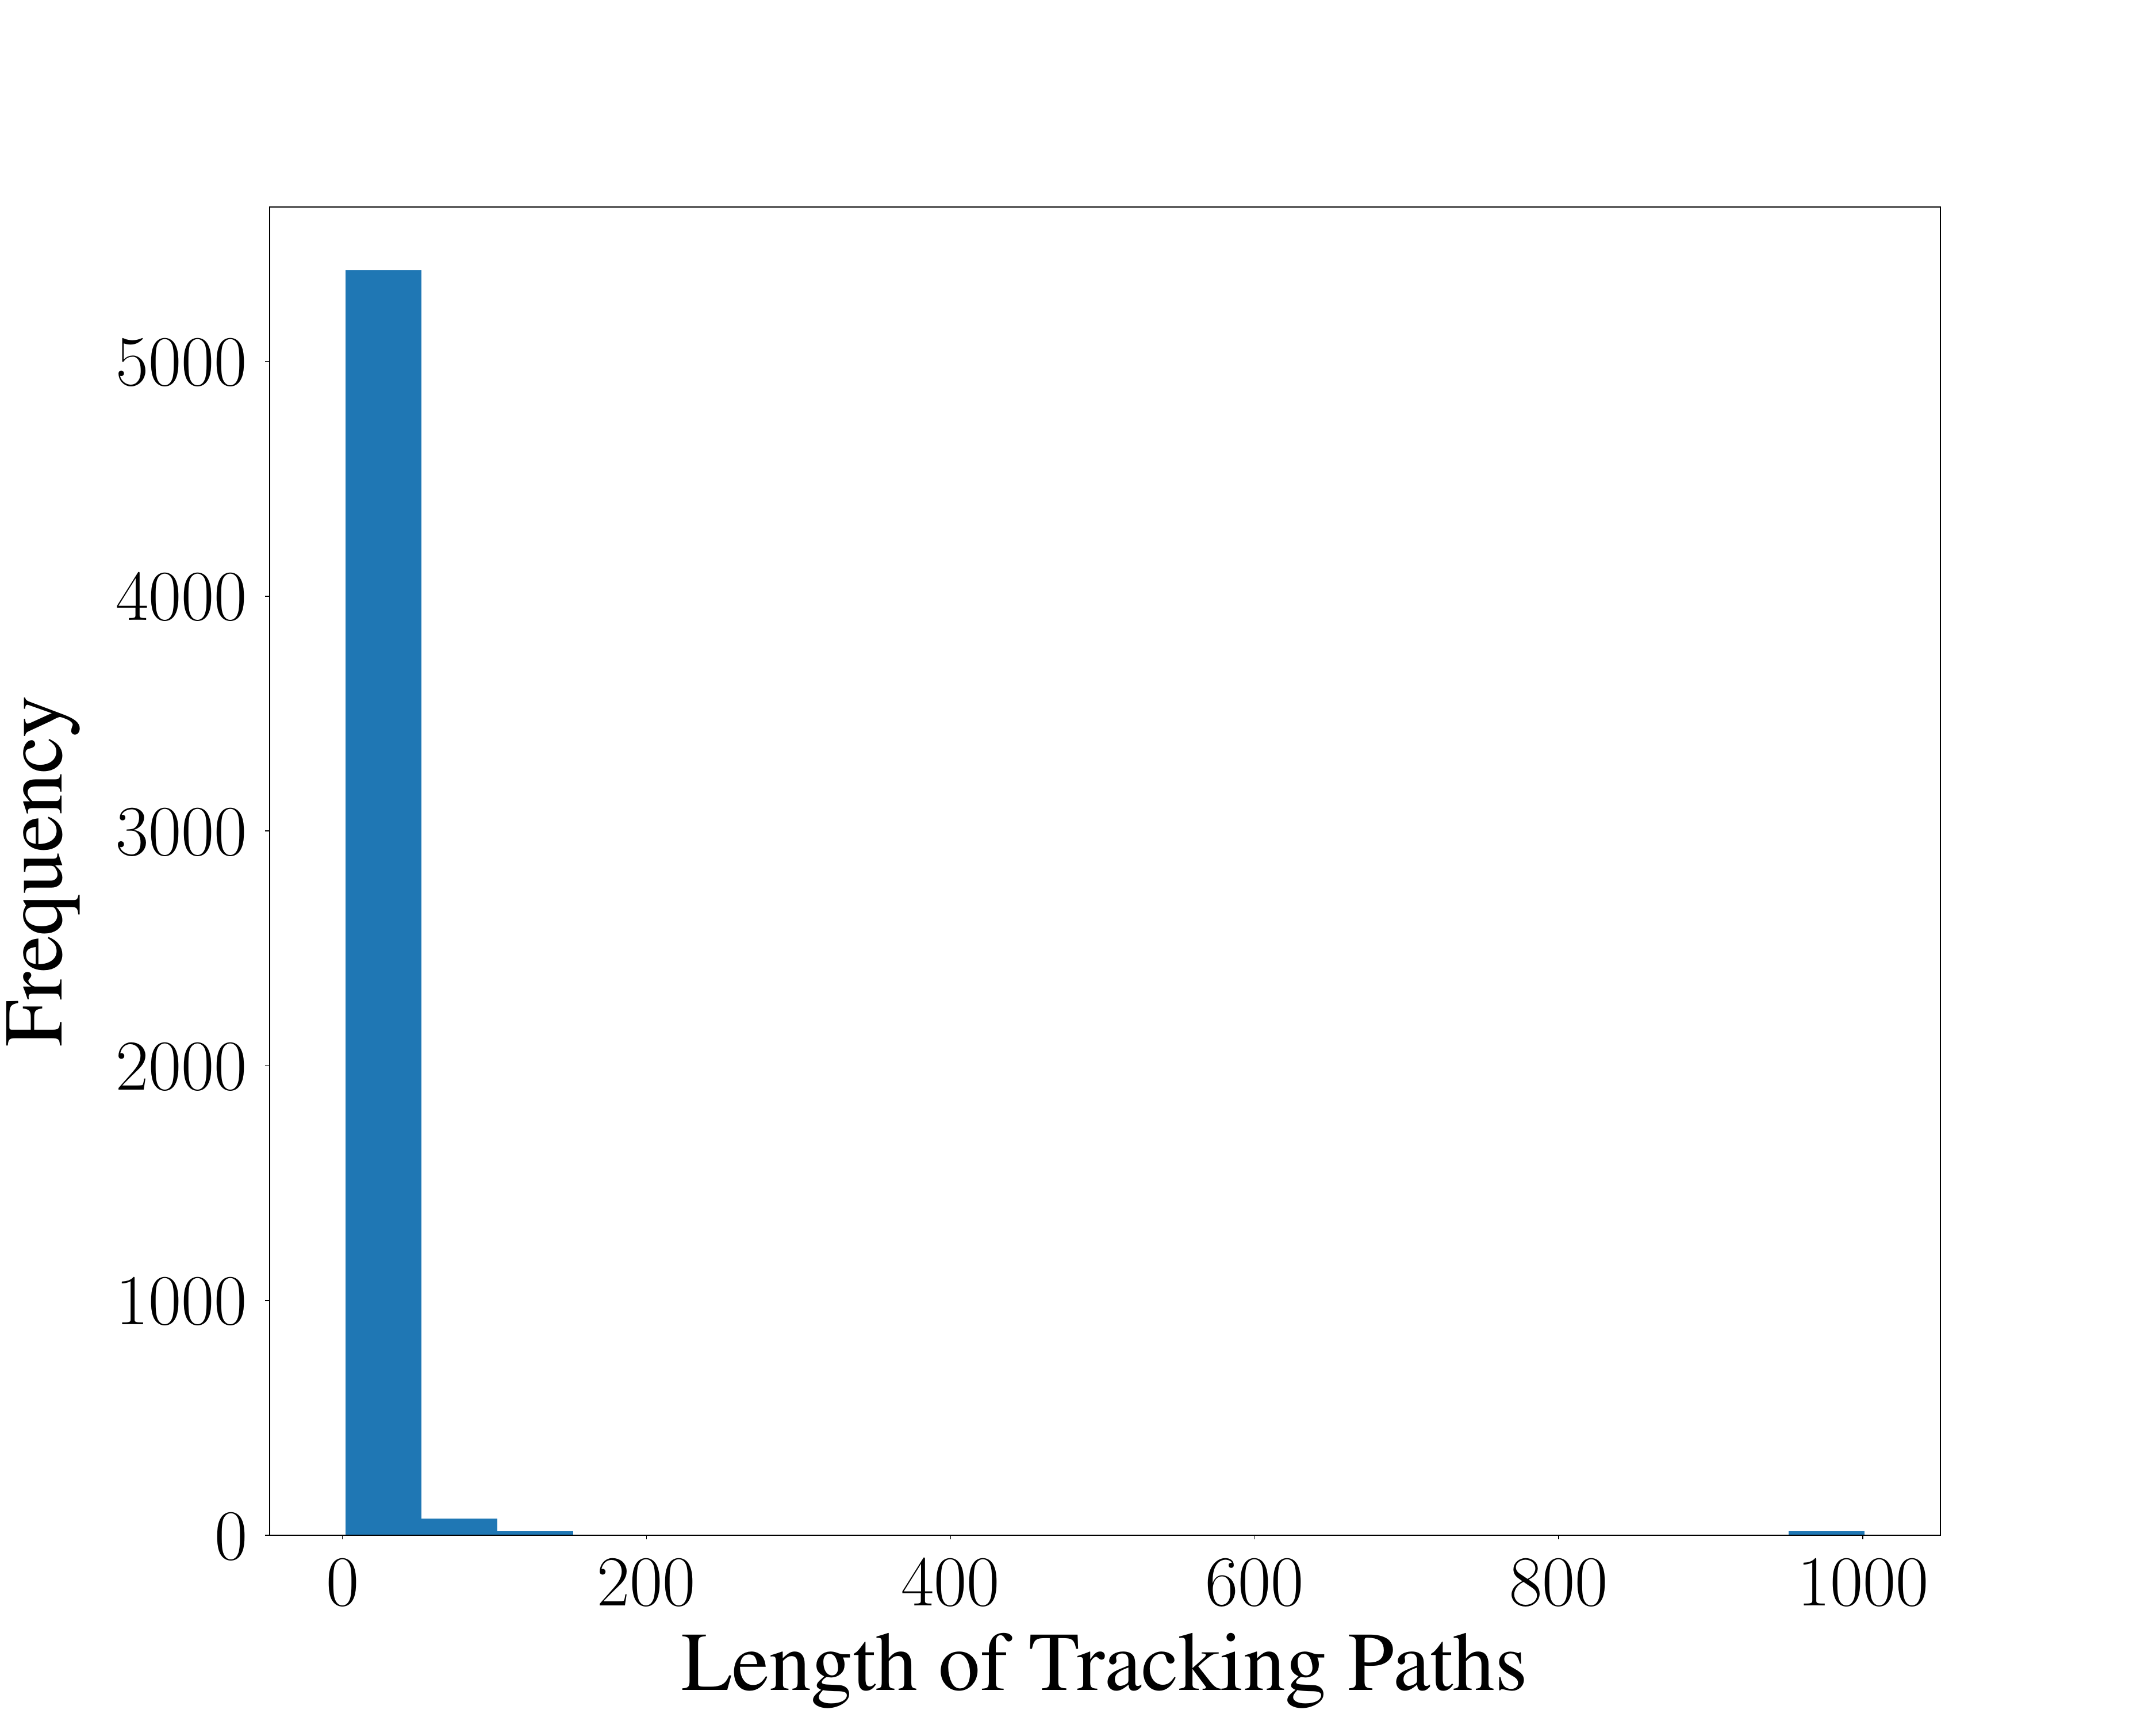}
\caption{$d_w$.}%
\label{fig-LengthHistogramCylinder2DWLong}%
\end{subfigure}
\hfill%
\begin{subfigure}[t]{\ltwopicwidth}%
\includegraphics[width=\ltwopicwidth]{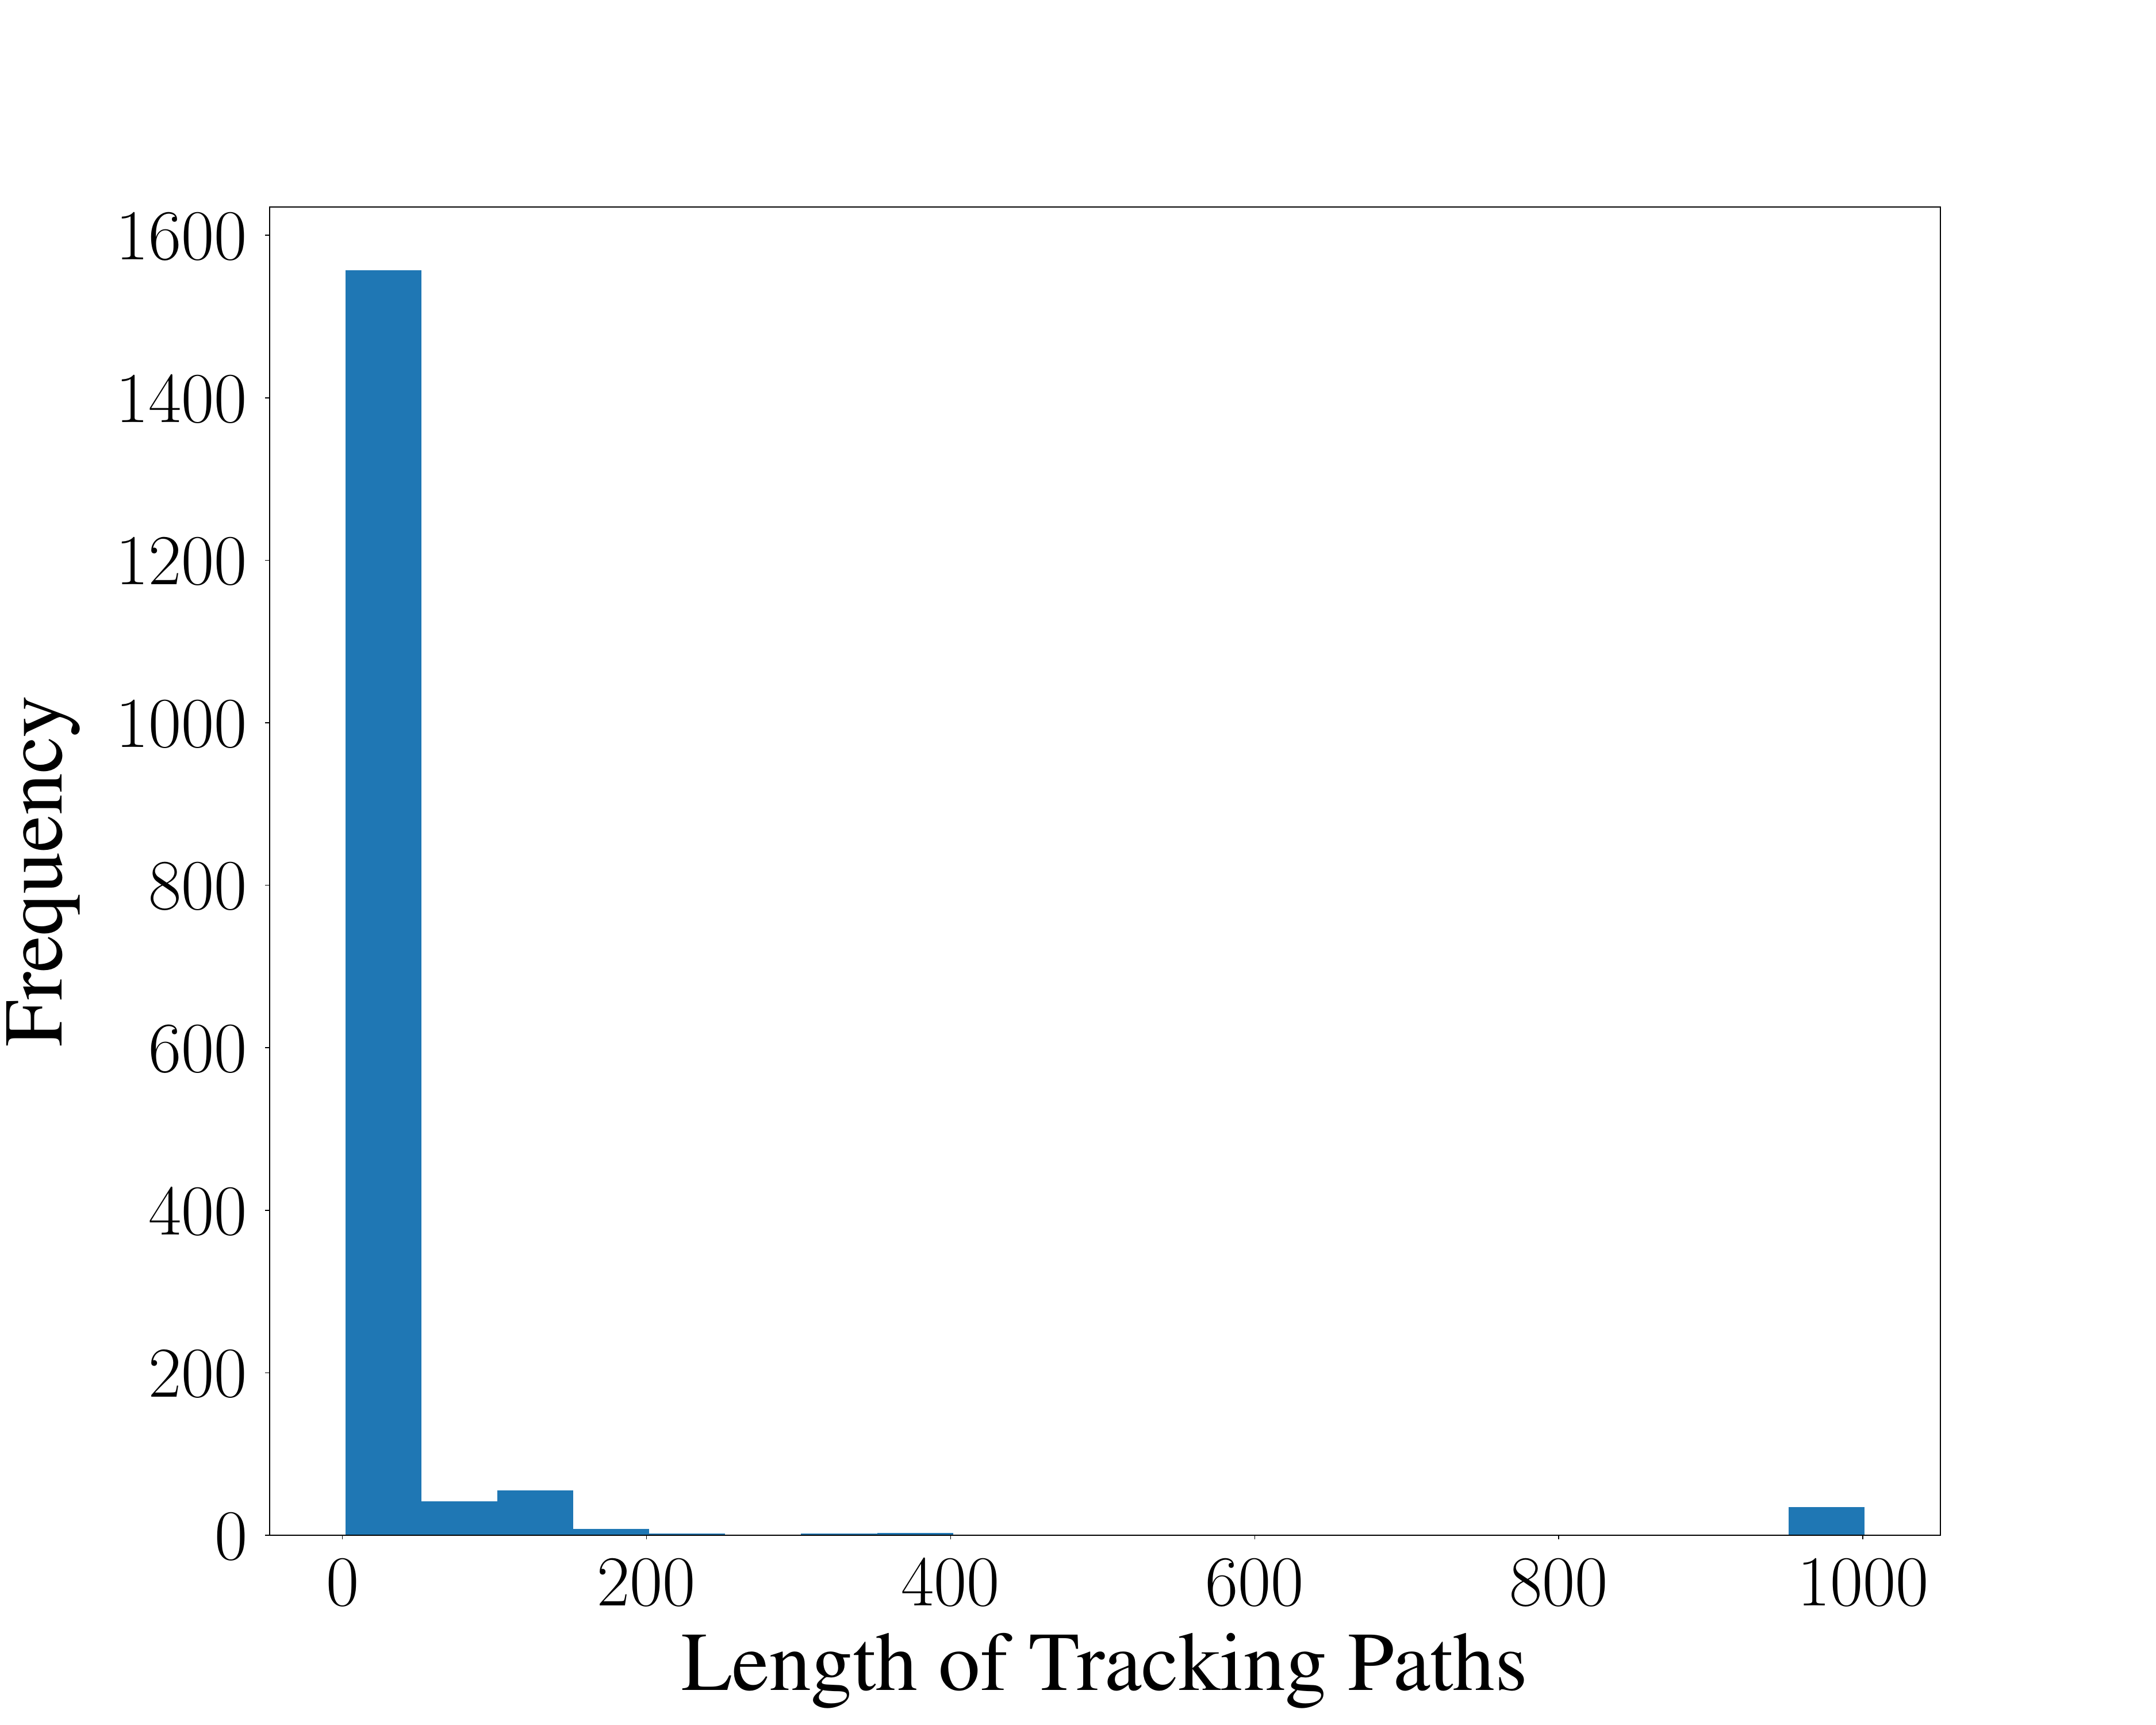}%
\caption{$d_e$.}%`'
\label{fig-LengthHistogramCylinder2DELong}%
\end{subfigure}%
\\%
\begin{subfigure}[t]{\ltwopicwidth}%
\includegraphics[width=\ltwopicwidth]{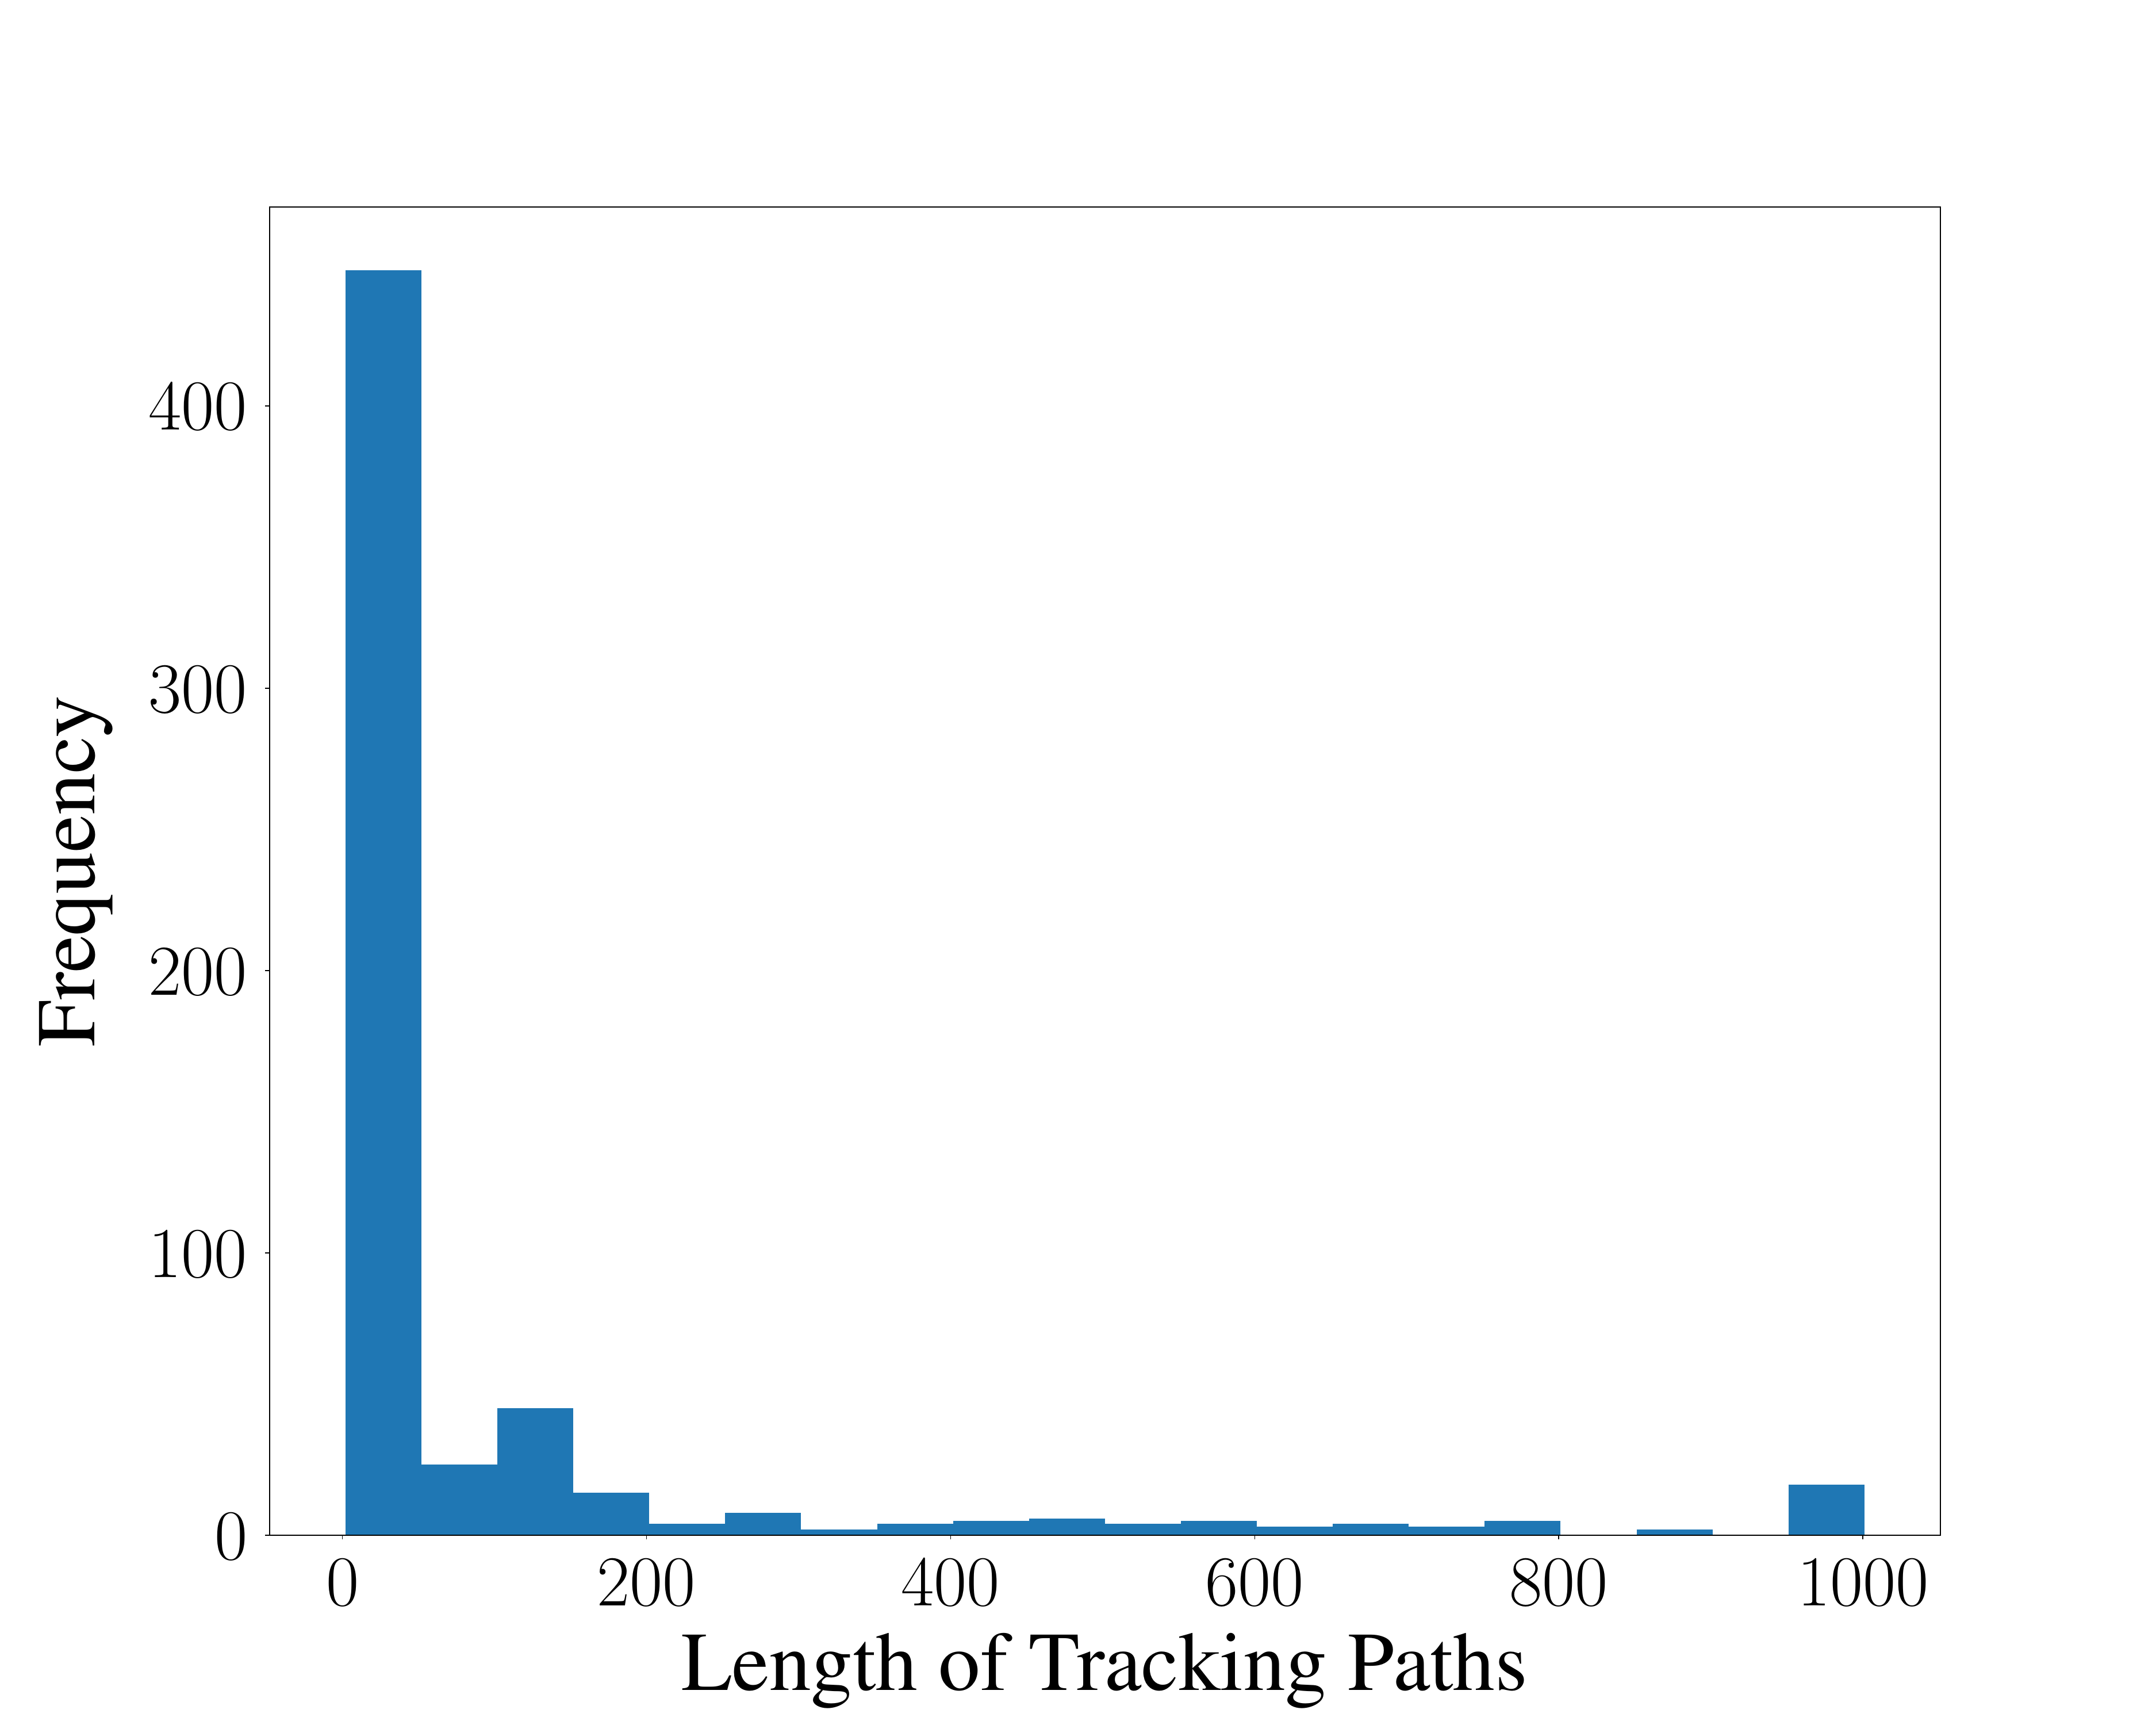}%
\caption{$d_b$.}%
\label{fig-LengthHistogramCylinder2DBLong}%
\end{subfigure}%
\hfill%
\begin{subfigure}[t]{\ltwopicwidth}%
\includegraphics[width=\ltwopicwidth]{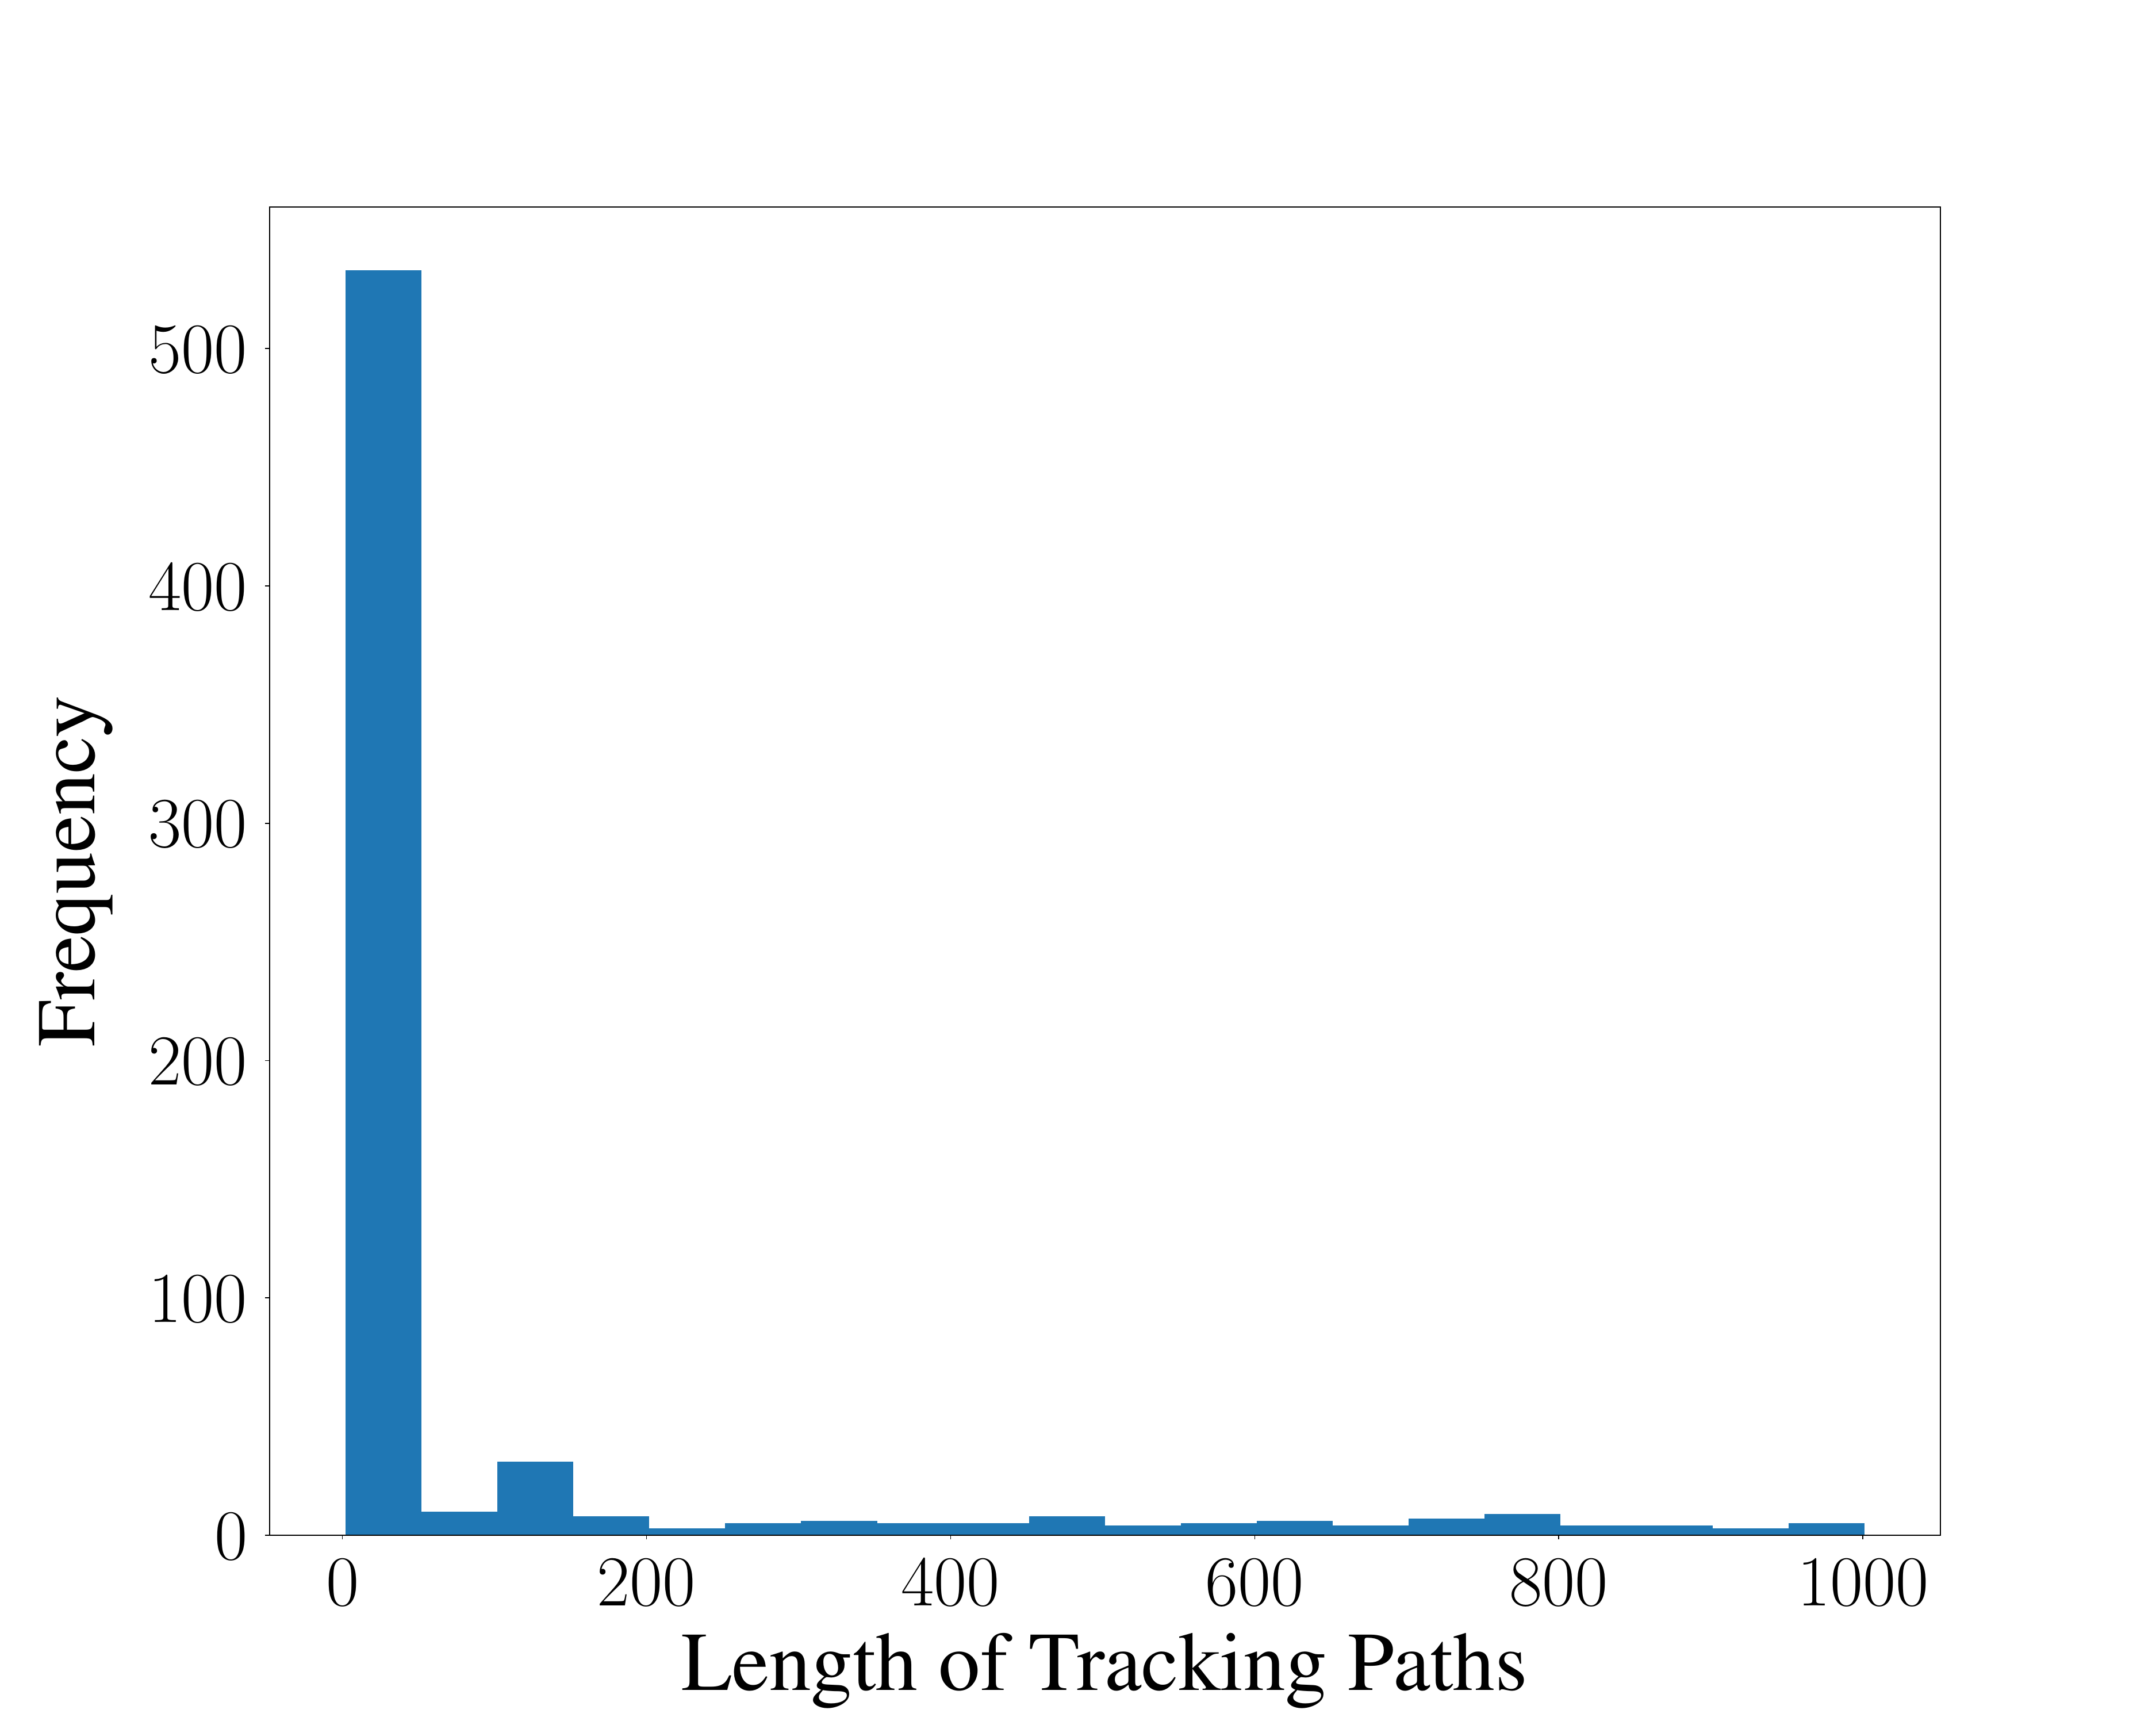}%
\caption{$d_p$.}%
\label{fig-LengthHistogramCylinder2DPLong}%
\end{subfigure}%
\caption{Histograms of the length of the tracking paths
    of \dataset{Cylinder2D}.}%
\label{fig-LengthHisgoramCylinder2DLong}%
\end{figure}
