# Supplementary material for: A Comparative Study of Different Edit Distance-Based Methods for Feature Tracking using Merge Trees on Time-Varying Scalar Fields
Source: arXiv:2509.17974 source file (2025-10-12)
Supplement: Supplementary file 9 [file supp_stableNoise.tex]

\section*{Stability with respect to Noise}
In the section, we show the results of the stability score 
with $\epsilon_\text{max} = 5\%$. 
The results can be seen 
in \Cref{fig-stab10}, \Cref{fig-stab15}, and \Cref{fig-stab20}.

\begin{figure}
    \centering
    \includegraphics[width=0.8\linewidth]{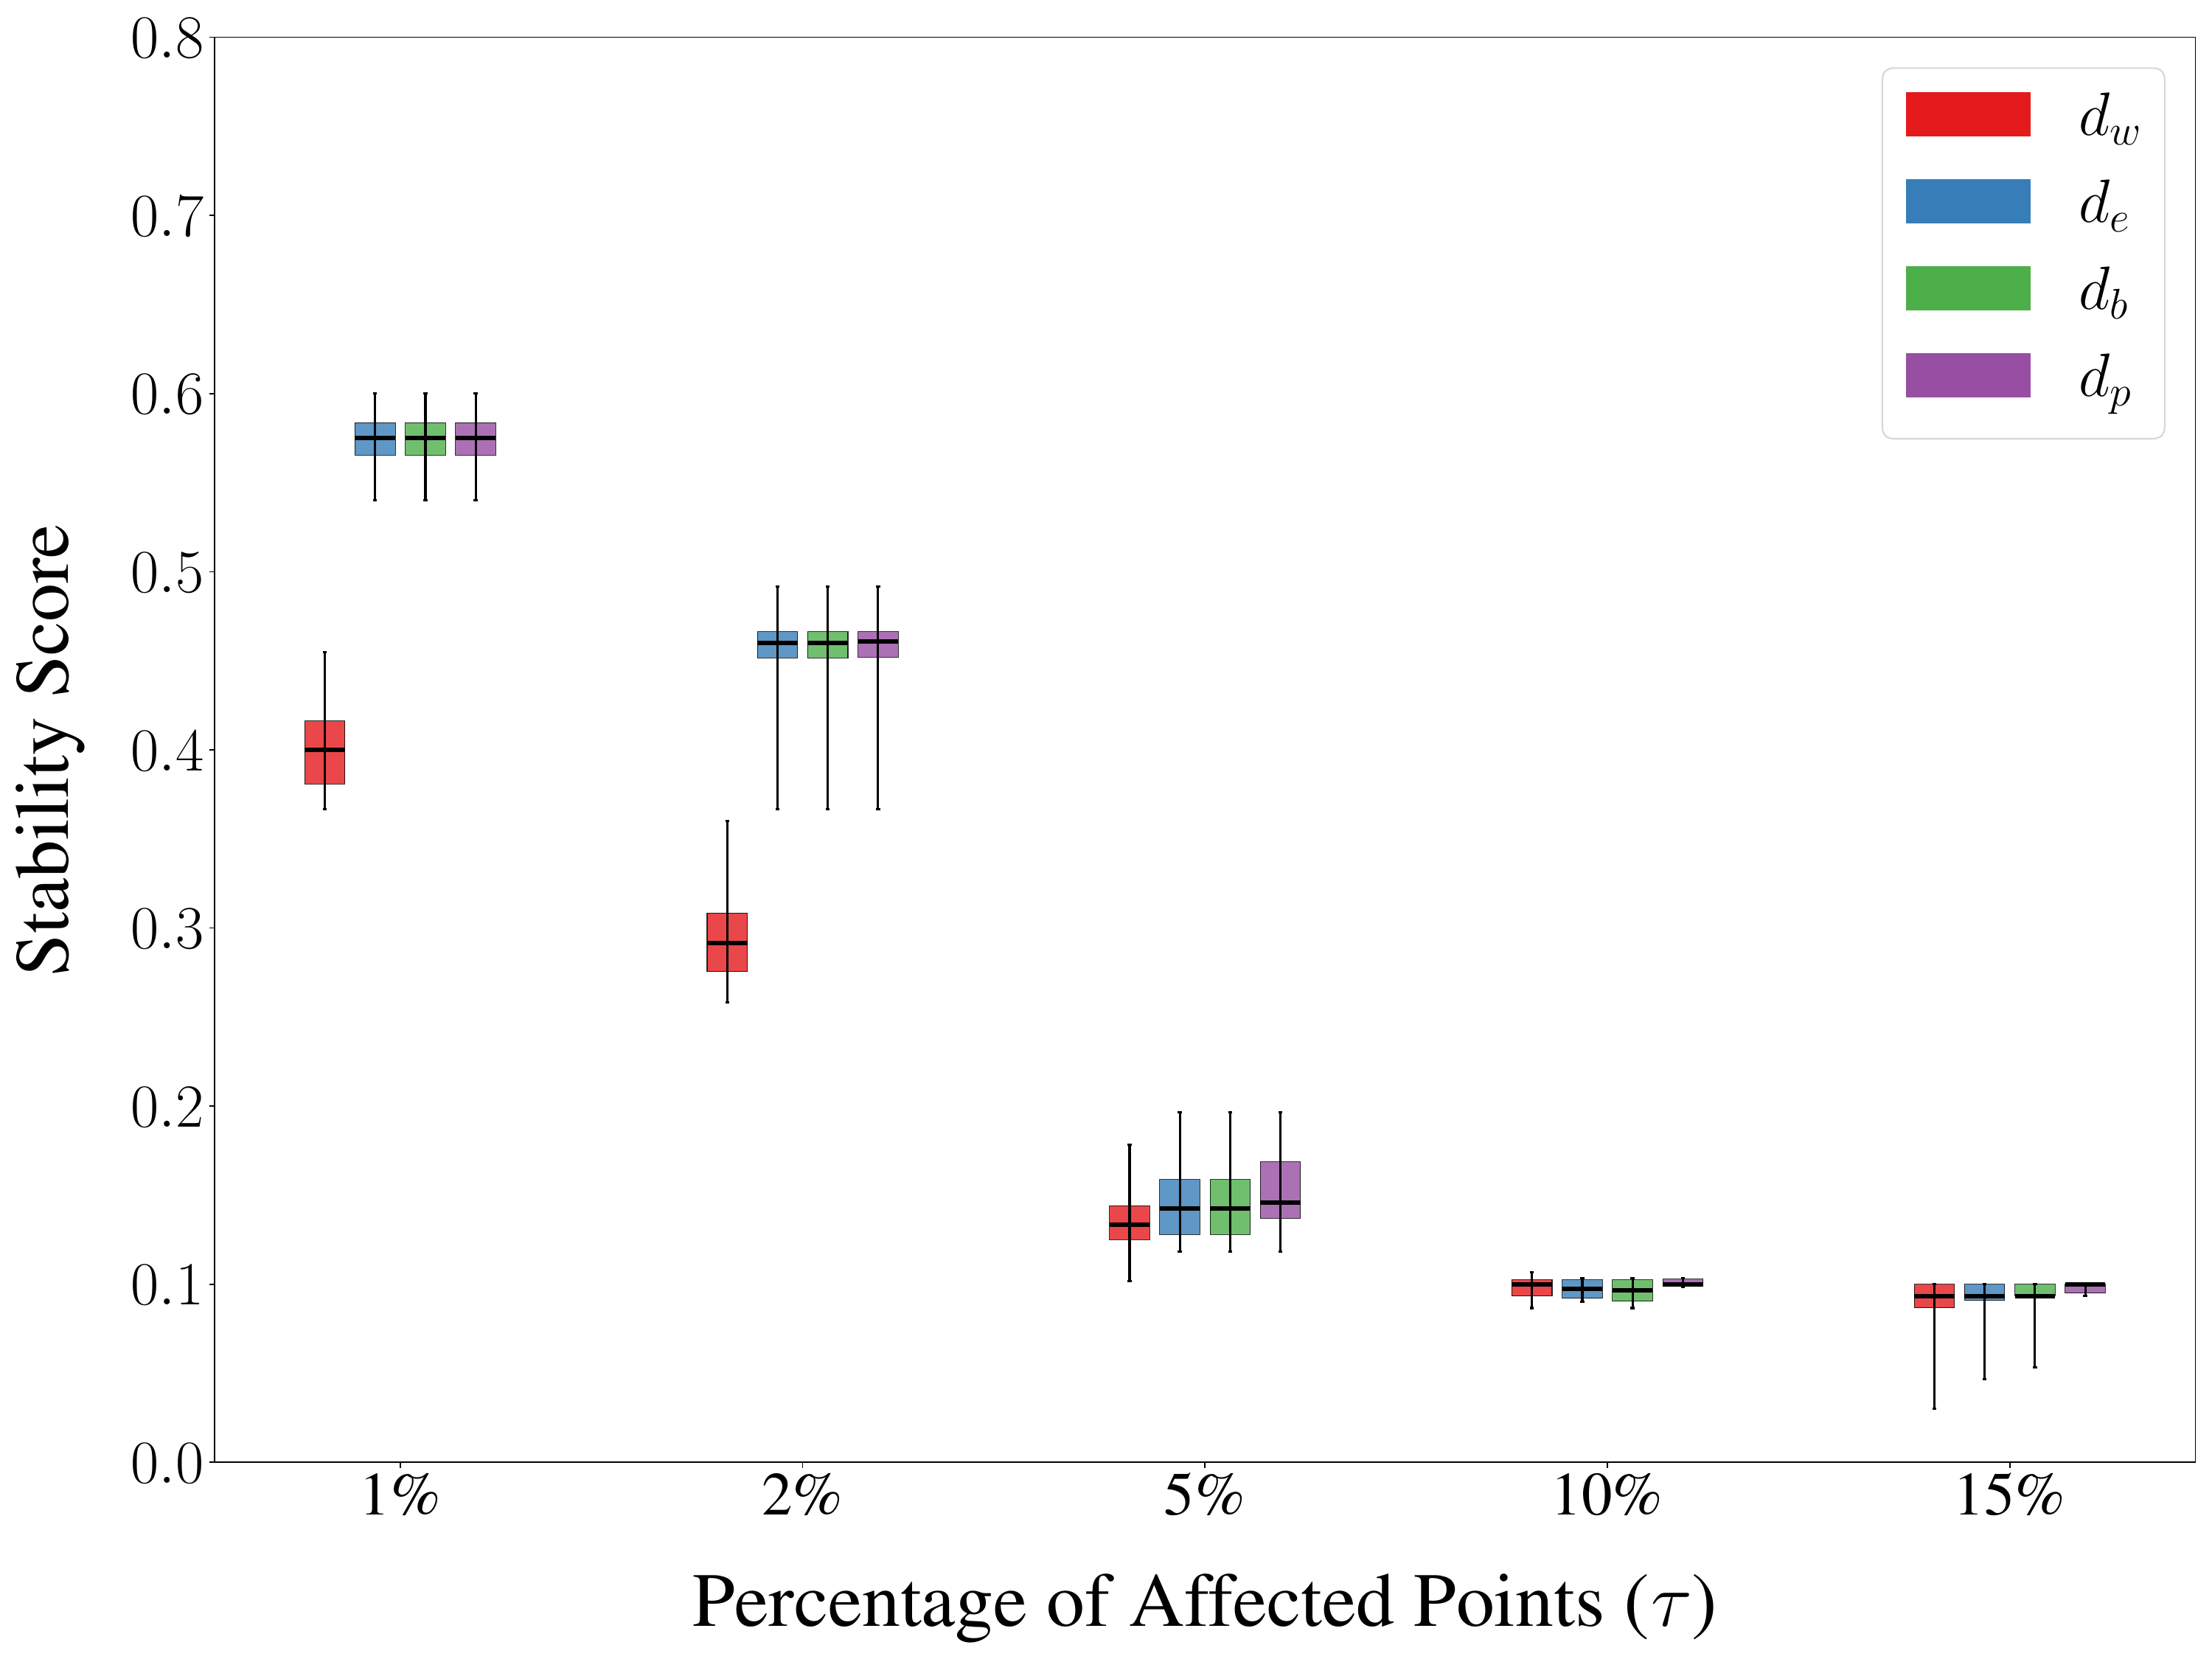}
    \caption{The tracking stability of the extrema of the for methods 
    if we stop at $\epsilon_\text{max}=10\%$. 
    }
    \label{fig-stab10}
\end{figure}

\begin{figure}
    \centering
    \includegraphics[width=0.8\linewidth]{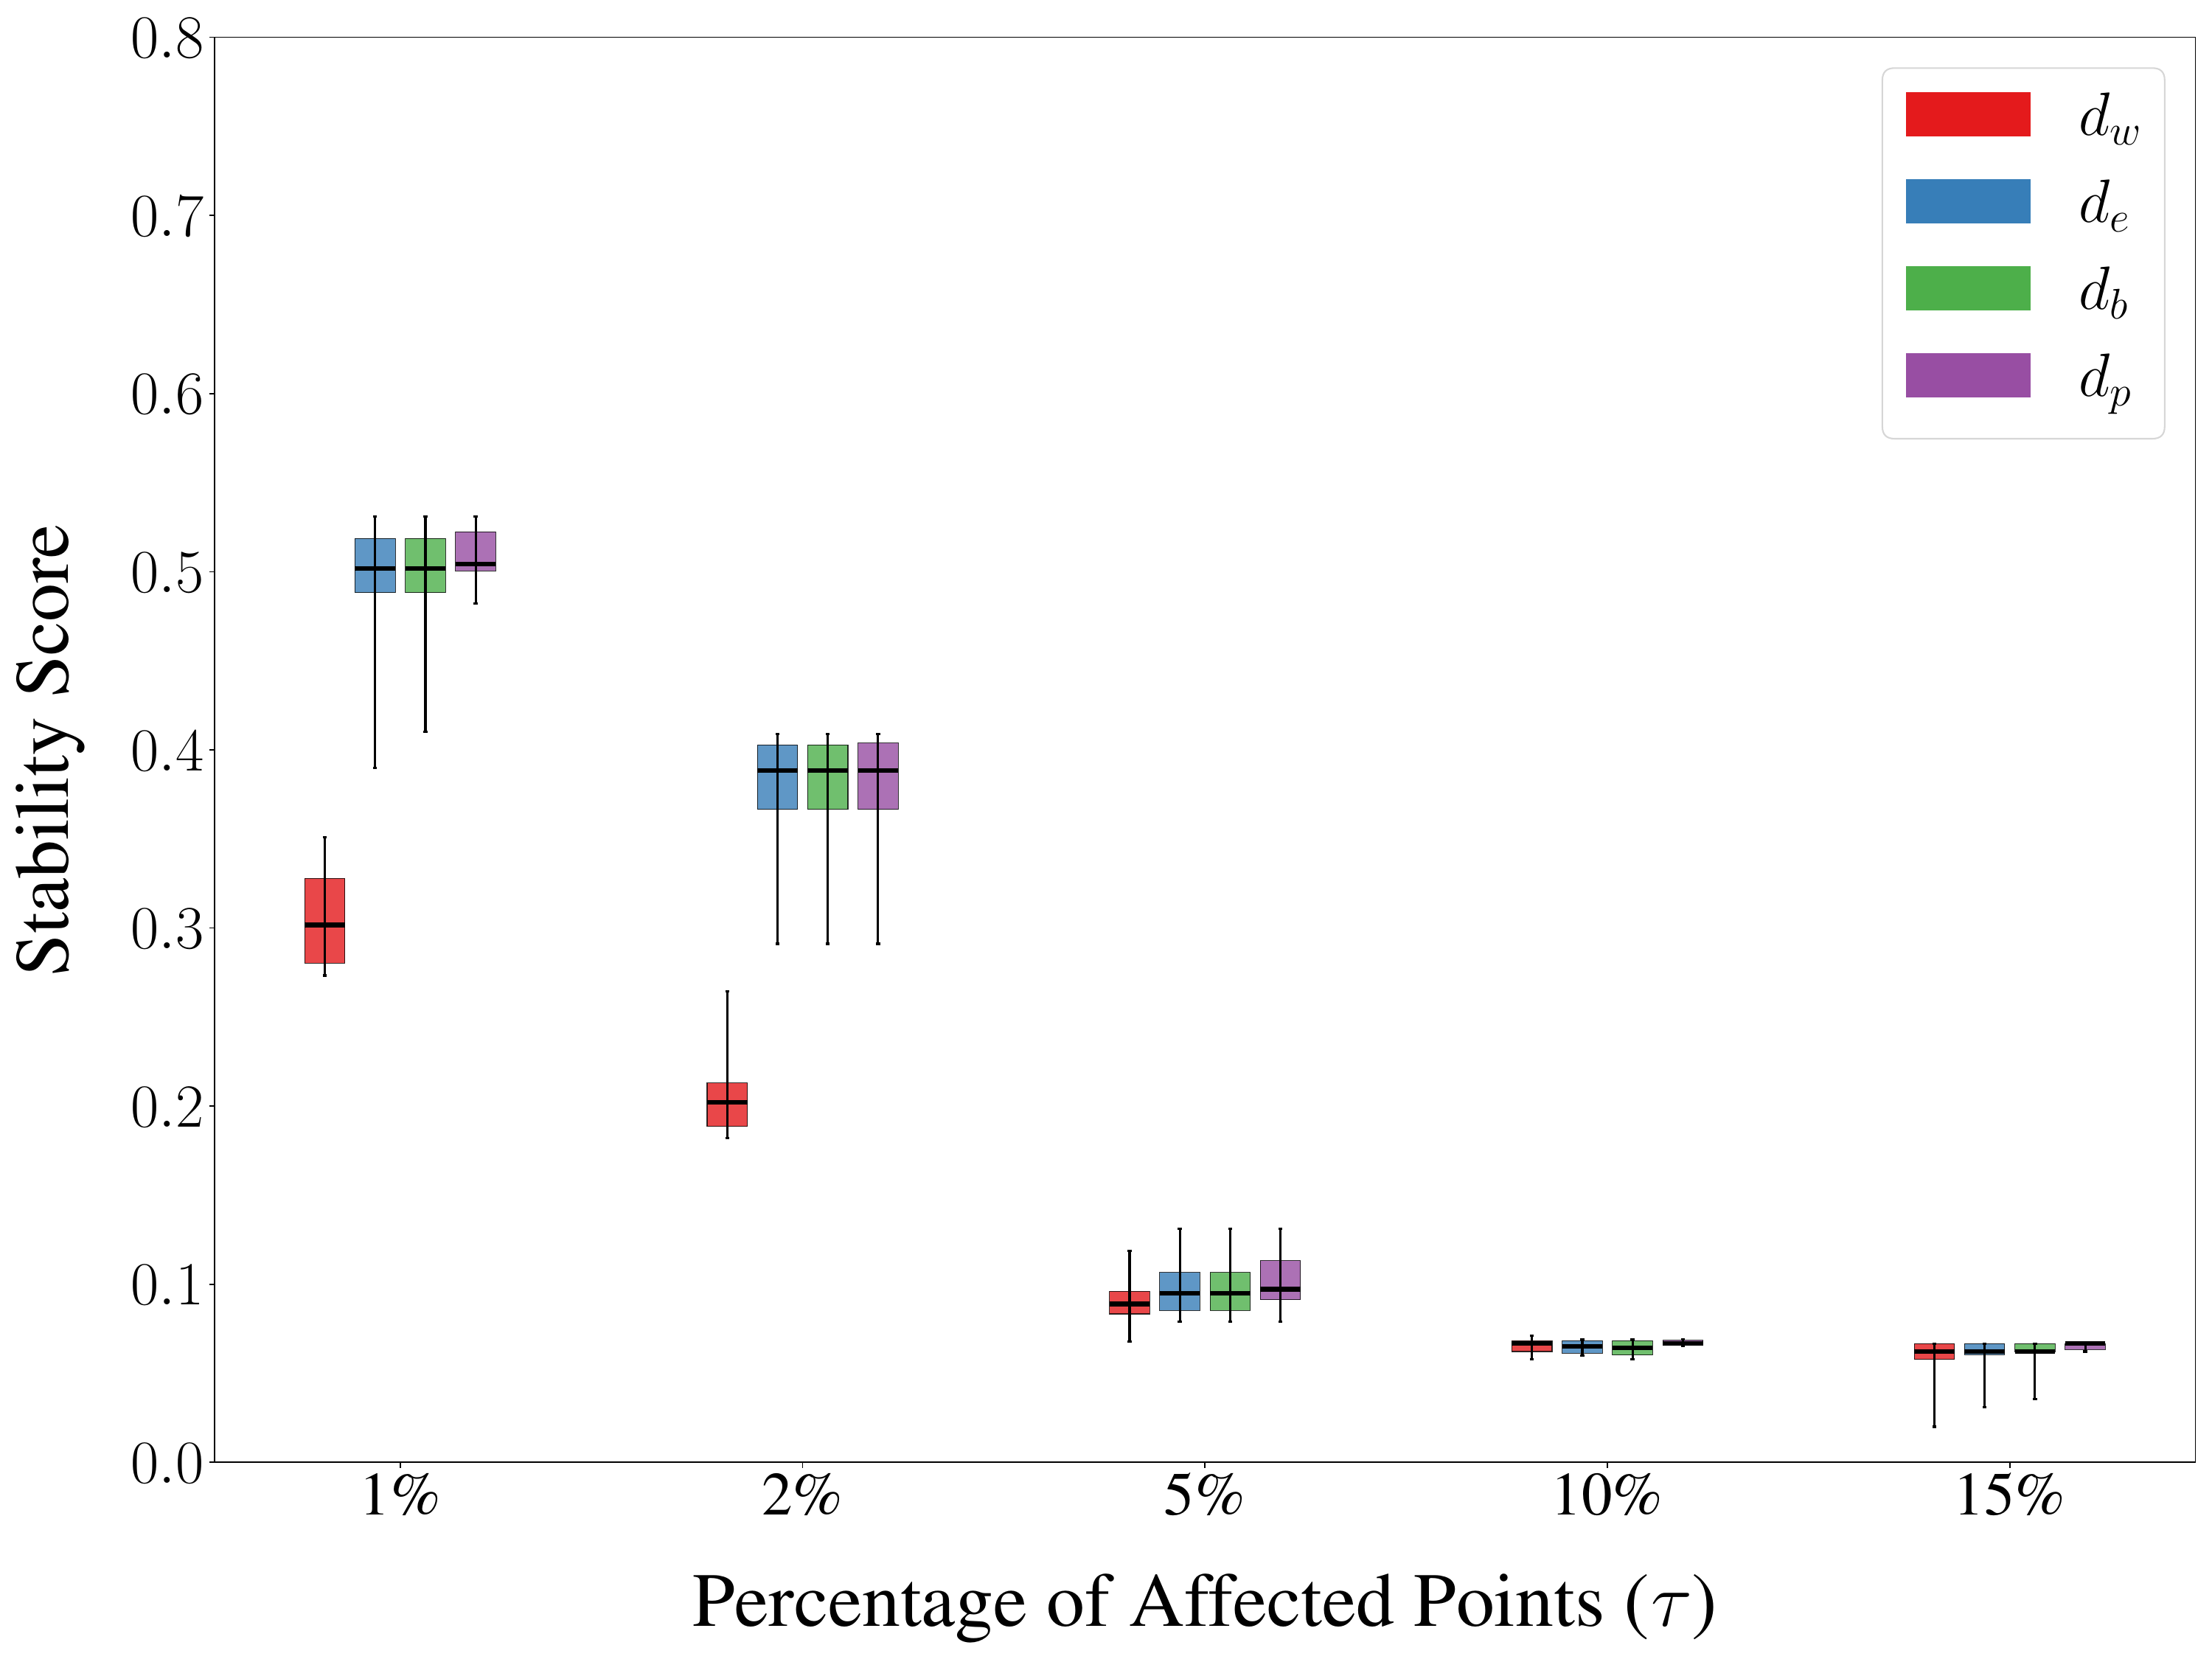}
    \caption{The tracking stability of the extrema of the for methods 
    if we stop at $\epsilon_\text{max}=15\%$.}
    \label{fig-stab15}
\end{figure}

\begin{figure}
    \centering
    \includegraphics[width=0.8\linewidth]{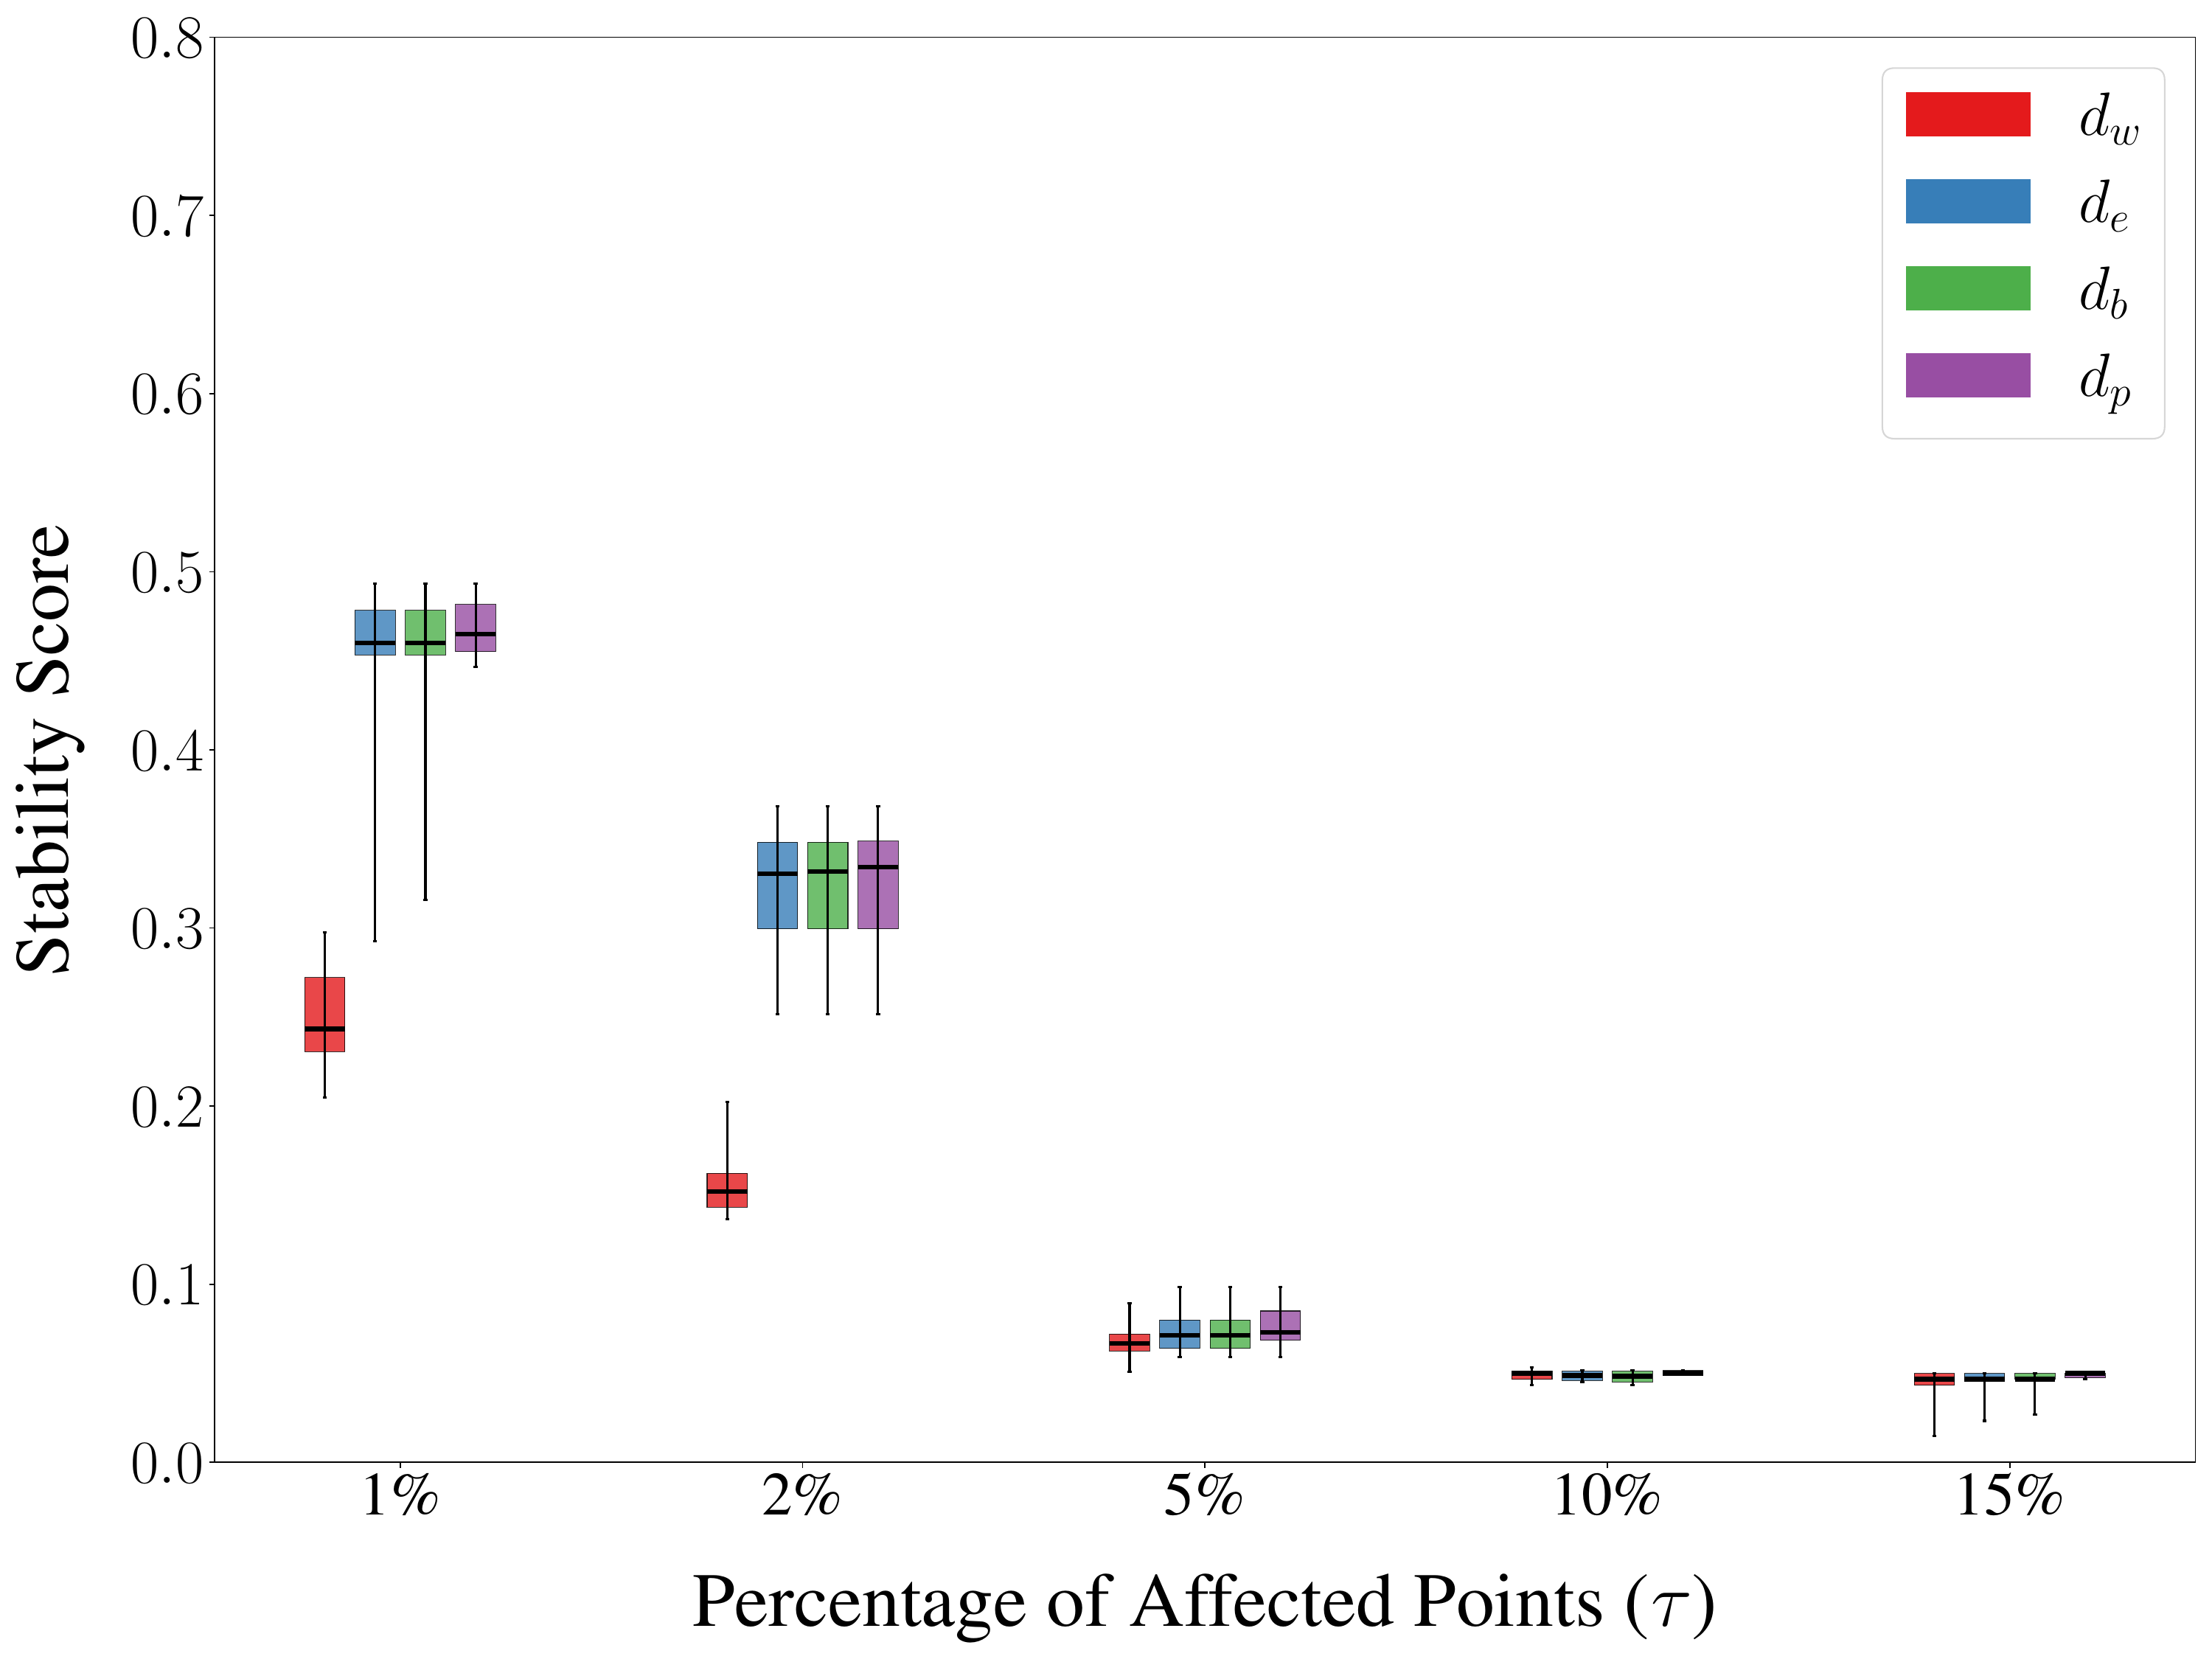}
    \caption{The tracking stability of the extrema of the for methods 
    if we stop at $\epsilon_\text{max}=20\%$.}
    \label{fig-stab20}
\end{figure}
